# Supplementary material for: Importance profiles. Visualization of atomic basis set requirements
Source: arXiv:2309.14844 ancillary file (2023-12-24)
Supplement: Supplementary file 1 [file plots.pdf]

# Supporting Information for “Importance profiles. Visualization of basis set superposition errors”

Susi Lehtola

*Department of Chemistry, University of Helsinki, P.O. Box 55 (A. I. Virtasen aukio 1),*

*FI-00014 University of Helsinki, Finland<sup>a)</sup>*

This document contains the plots of the importance profiles for all the HELFEM calculations<sup>1,2</sup> performed in this work for the diatomic molecules from the database of Weigend and Ahlrichs<sup>3</sup> up to the third row (H–Br). All calculations employed the Perdew–Burke–Ernzerhof functional,<sup>4,5</sup> as implemented in Libxc.<sup>6</sup> The calculations were all started from a superposition of atomic potentials (SAP).<sup>7</sup> The importance profiles were computed from these CBS limit wave functions, determined with the procedure of Lehtola<sup>2</sup>, for Gaussian-type orbital (GTO) and Slater-type orbital probes. In the case of spin-polarized systems, the  $\alpha$ -spin profiles are shown by solid lines, and the  $\beta$ -spin profiles with dashed lines.

## LIST OF FIGURES

|    |                                                                                 |    |
|----|---------------------------------------------------------------------------------|----|
| 1  | GTO importance profile for $\sigma$ orbitals on H atom in CuH. ....             | 13 |
| 2  | GTO importance profile for $\sigma$ orbitals on H atom in H <sub>2</sub> . .... | 13 |
| 3  | GTO importance profile for $\sigma$ orbitals on H atom in HBr. ....             | 13 |
| 4  | GTO importance profile for $\sigma$ orbitals on H atom in HCl. ....             | 13 |
| 5  | GTO importance profile for $\sigma$ orbitals on H atom in HF. ....              | 14 |
| 6  | GTO importance profile for $\sigma$ orbitals on H atom in KH. ....              | 14 |
| 7  | GTO importance profile for $\sigma$ orbitals on H atom in LiH. ....             | 14 |
| 8  | GTO importance profile for $\sigma$ orbitals on H atom in NaH. ....             | 14 |
| 9  | STO importance profile for $\sigma$ orbitals on H atom in CuH. ....             | 15 |
| 10 | STO importance profile for $\sigma$ orbitals on H atom in H <sub>2</sub> . .... | 15 |
| 11 | STO importance profile for $\sigma$ orbitals on H atom in HBr. ....             | 15 |
| 12 | STO importance profile for $\sigma$ orbitals on H atom in HCl. ....             | 15 |
| 13 | STO importance profile for $\sigma$ orbitals on H atom in HF. ....              | 16 |
| 14 | STO importance profile for $\sigma$ orbitals on H atom in KH. ....              | 16 |

|    |                                                                     |    |
|----|---------------------------------------------------------------------|----|
| 15 | STO importance profile for $\sigma$ orbitals on H atom in LiH. .... | 16 |
| 16 | STO importance profile for $\sigma$ orbitals on H atom in NaH. .... | 16 |
| 17 | GTO importance profile for $\pi_-$ orbitals on H atom in CuH. ....  | 17 |
| 18 | GTO importance profile for $\pi_-$ orbitals on H atom in HBr. ....  | 17 |
| 19 | GTO importance profile for $\pi_-$ orbitals on H atom in HCl. ....  | 17 |
| 20 | GTO importance profile for $\pi_-$ orbitals on H atom in HF. ....   | 17 |
| 21 | GTO importance profile for $\pi_-$ orbitals on H atom in KH. ....   | 18 |
| 22 | GTO importance profile for $\pi_-$ orbitals on H atom in NaH. ....  | 18 |
| 23 | STO importance profile for $\pi_-$ orbitals on H atom in CuH. ....  | 18 |
| 24 | STO importance profile for $\pi_-$ orbitals on H atom in HBr. ....  | 18 |
| 25 | STO importance profile for $\pi_-$ orbitals on H atom in HCl. ....  | 19 |
| 26 | STO importance profile for $\pi_-$ orbitals on H atom in HF. ....   | 19 |
| 27 | STO importance profile for $\pi_-$ orbitals on H atom in KH. ....   | 19 |
| 28 | STO importance profile for $\pi_-$ orbitals on H atom in NaH. ....  | 19 |
| 29 | GTO importance profile for $\pi_+$ orbitals on H atom in CuH. ....  | 20 |
| 30 | GTO importance profile for $\pi_+$ orbitals on H atom in HBr. ....  | 20 |
| 31 | GTO importance profile for $\pi_+$ orbitals on H atom in HCl. ....  | 20 |
| 32 | GTO importance profile for $\pi_+$ orbitals on H atom in HF. ....   | 20 |
| 33 | GTO importance profile for $\pi_+$ orbitals on H atom in KH. ....   | 21 |
| 34 | GTO importance profile for $\pi_+$ orbitals on H atom in NaH. ....  | 21 |
| 35 | STO importance profile for $\pi_+$ orbitals on H atom in CuH. ....  | 21 |
| 36 | STO importance profile for $\pi_+$ orbitals on H atom in HBr. ....  | 21 |
| 37 | STO importance profile for $\pi_+$ orbitals on H atom in HCl. ....  | 22 |
| 38 | STO importance profile for $\pi_+$ orbitals on H atom in HF. ....   | 22 |
| 39 | STO importance profile for $\pi_+$ orbitals on H atom in KH. ....   | 22 |

<sup>a)</sup> Electronic mail: susi.lehtola@alumni.helsinki.fi

|    |                                                                                   |    |    |                                                                                 |    |
|----|-----------------------------------------------------------------------------------|----|----|---------------------------------------------------------------------------------|----|
| 40 | STO importance profile for $\pi_+$ orbitals on H atom in NaH. ....                | 22 | 69 | GTO importance profile for $\pi_+$ orbitals on Be atom in BeS. ....             | 30 |
| 41 | GTO importance profile for $\delta_-$ orbitals on H atom in CuH. ....             | 23 | 70 | STO importance profile for $\pi_+$ orbitals on Be atom in BeS. ....             | 30 |
| 42 | GTO importance profile for $\delta_-$ orbitals on H atom in HBr. ....             | 23 | 71 | GTO importance profile for $\sigma$ orbitals on C atom in CO. ....              | 30 |
| 43 | STO importance profile for $\delta_-$ orbitals on H atom in CuH. ....             | 23 | 72 | STO importance profile for $\sigma$ orbitals on C atom in CO. ....              | 30 |
| 44 | STO importance profile for $\delta_-$ orbitals on H atom in HBr. ....             | 23 | 73 | GTO importance profile for $\pi_-$ orbitals on C atom in CO. ....               | 31 |
| 45 | GTO importance profile for $\delta_+$ orbitals on H atom in CuH. ....             | 24 | 74 | STO importance profile for $\pi_-$ orbitals on C atom in CO. ....               | 31 |
| 46 | GTO importance profile for $\delta_+$ orbitals on H atom in HBr. ....             | 24 | 75 | GTO importance profile for $\pi_+$ orbitals on C atom in CO. ....               | 31 |
| 47 | STO importance profile for $\delta_+$ orbitals on H atom in CuH. ....             | 24 | 76 | STO importance profile for $\pi_+$ orbitals on C atom in CO. ....               | 31 |
| 48 | STO importance profile for $\delta_+$ orbitals on H atom in HBr. ....             | 24 | 77 | GTO importance profile for $\sigma$ orbitals on N atom in AlN. ....             | 32 |
| 49 | GTO importance profile for $\sigma$ orbitals on Li atom in Li <sub>2</sub> . .... | 25 | 78 | GTO importance profile for $\sigma$ orbitals on N atom in N <sub>2</sub> . .... | 32 |
| 50 | GTO importance profile for $\sigma$ orbitals on Li atom in LiCl. ....             | 25 | 79 | STO importance profile for $\sigma$ orbitals on N atom in AlN. ....             | 32 |
| 51 | GTO importance profile for $\sigma$ orbitals on Li atom in LiF. ....              | 25 | 80 | STO importance profile for $\sigma$ orbitals on N atom in N <sub>2</sub> . .... | 32 |
| 52 | GTO importance profile for $\sigma$ orbitals on Li atom in LiH. ....              | 25 | 81 | GTO importance profile for $\pi_-$ orbitals on N atom in AlN. ....              | 33 |
| 53 | STO importance profile for $\sigma$ orbitals on Li atom in Li <sub>2</sub> . .... | 26 | 82 | GTO importance profile for $\pi_-$ orbitals on N atom in N <sub>2</sub> . ....  | 33 |
| 54 | STO importance profile for $\sigma$ orbitals on Li atom in LiCl. ....             | 26 | 83 | STO importance profile for $\pi_-$ orbitals on N atom in AlN. ....              | 33 |
| 55 | STO importance profile for $\sigma$ orbitals on Li atom in LiF. ....              | 26 | 84 | STO importance profile for $\pi_-$ orbitals on N atom in N <sub>2</sub> . ....  | 33 |
| 56 | STO importance profile for $\sigma$ orbitals on Li atom in LiH. ....              | 26 | 85 | GTO importance profile for $\pi_+$ orbitals on N atom in AlN. ....              | 34 |
| 57 | GTO importance profile for $\pi_-$ orbitals on Li atom in LiCl. ....              | 27 | 86 | GTO importance profile for $\pi_+$ orbitals on N atom in N <sub>2</sub> . ....  | 34 |
| 58 | GTO importance profile for $\pi_-$ orbitals on Li atom in LiF. ....               | 27 | 87 | STO importance profile for $\pi_+$ orbitals on N atom in AlN. ....              | 34 |
| 59 | STO importance profile for $\pi_-$ orbitals on Li atom in LiCl. ....              | 27 | 88 | STO importance profile for $\pi_+$ orbitals on N atom in N <sub>2</sub> . ....  | 34 |
| 60 | STO importance profile for $\pi_-$ orbitals on Li atom in LiF. ....               | 27 | 89 | GTO importance profile for $\sigma$ orbitals on O atom in CO. ....              | 35 |
| 61 | GTO importance profile for $\pi_+$ orbitals on Li atom in LiCl. ....              | 28 | 90 | GTO importance profile for $\sigma$ orbitals on O atom in FeO. ....             | 35 |
| 62 | GTO importance profile for $\pi_+$ orbitals on Li atom in LiF. ....               | 28 | 91 | GTO importance profile for $\sigma$ orbitals on O atom in GaO. ....             | 35 |
| 63 | STO importance profile for $\pi_+$ orbitals on Li atom in LiCl. ....              | 28 | 92 | GTO importance profile for $\sigma$ orbitals on O atom in GeO. ....             | 35 |
| 64 | STO importance profile for $\pi_+$ orbitals on Li atom in LiF. ....               | 28 | 93 | GTO importance profile for $\sigma$ orbitals on O atom in MnO. ....             | 36 |
| 65 | GTO importance profile for $\sigma$ orbitals on Be atom in BeS. ....              | 29 | 94 | GTO importance profile for $\sigma$ orbitals on O atom in NiO. ....             | 36 |
| 66 | STO importance profile for $\sigma$ orbitals on Be atom in BeS. ....              | 29 | 95 | GTO importance profile for $\sigma$ orbitals on O atom in ScO. ....             | 36 |
| 67 | GTO importance profile for $\pi_-$ orbitals on Be atom in BeS. ....               | 29 | 96 | GTO importance profile for $\sigma$ orbitals on O atom in SeO. ....             | 36 |
| 68 | STO importance profile for $\pi_-$ orbitals on Be atom in BeS. ....               | 29 | 97 | GTO importance profile for $\sigma$ orbitals on O atom in TiO. ....             | 37 |

|     |                                                                    |    |     |                                                                      |    |
|-----|--------------------------------------------------------------------|----|-----|----------------------------------------------------------------------|----|
| 98  | GTO importance profile for $\sigma$ orbitals on O atom in VO.....  | 37 | 127 | STO importance profile for $\pi_-$ orbitals on O atom in TiO.....    | 44 |
| 99  | STO importance profile for $\sigma$ orbitals on O atom in CO.....  | 37 | 128 | STO importance profile for $\pi_-$ orbitals on O atom in VO.....     | 44 |
| 100 | STO importance profile for $\sigma$ orbitals on O atom in FeO..... | 37 | 129 | GTO importance profile for $\pi_+$ orbitals on O atom in CO.....     | 45 |
| 101 | STO importance profile for $\sigma$ orbitals on O atom in GaO..... | 38 | 130 | GTO importance profile for $\pi_+$ orbitals on O atom in FeO.....    | 45 |
| 102 | STO importance profile for $\sigma$ orbitals on O atom in GeO..... | 38 | 131 | GTO importance profile for $\pi_+$ orbitals on O atom in GaO.....    | 45 |
| 103 | STO importance profile for $\sigma$ orbitals on O atom in MnO..... | 38 | 132 | GTO importance profile for $\pi_+$ orbitals on O atom in GeO.....    | 45 |
| 104 | STO importance profile for $\sigma$ orbitals on O atom in NiO..... | 38 | 133 | GTO importance profile for $\pi_+$ orbitals on O atom in MnO.....    | 46 |
| 105 | STO importance profile for $\sigma$ orbitals on O atom in ScO..... | 39 | 134 | GTO importance profile for $\pi_+$ orbitals on O atom in NiO.....    | 46 |
| 106 | STO importance profile for $\sigma$ orbitals on O atom in SeO..... | 39 | 135 | GTO importance profile for $\pi_+$ orbitals on O atom in ScO.....    | 46 |
| 107 | STO importance profile for $\sigma$ orbitals on O atom in TiO..... | 39 | 136 | GTO importance profile for $\pi_+$ orbitals on O atom in SeO.....    | 46 |
| 108 | STO importance profile for $\sigma$ orbitals on O atom in VO.....  | 39 | 137 | GTO importance profile for $\pi_+$ orbitals on O atom in TiO.....    | 47 |
| 109 | GTO importance profile for $\pi_-$ orbitals on O atom in CO.....   | 40 | 138 | GTO importance profile for $\pi_+$ orbitals on O atom in VO.....     | 47 |
| 110 | GTO importance profile for $\pi_-$ orbitals on O atom in FeO.....  | 40 | 139 | STO importance profile for $\pi_+$ orbitals on O atom in CO.....     | 47 |
| 111 | GTO importance profile for $\pi_-$ orbitals on O atom in GaO.....  | 40 | 140 | STO importance profile for $\pi_+$ orbitals on O atom in FeO.....    | 47 |
| 112 | GTO importance profile for $\pi_-$ orbitals on O atom in GeO.....  | 40 | 141 | STO importance profile for $\pi_+$ orbitals on O atom in GaO.....    | 48 |
| 113 | GTO importance profile for $\pi_-$ orbitals on O atom in MnO.....  | 41 | 142 | STO importance profile for $\pi_+$ orbitals on O atom in GeO.....    | 48 |
| 114 | GTO importance profile for $\pi_-$ orbitals on O atom in NiO.....  | 41 | 143 | STO importance profile for $\pi_+$ orbitals on O atom in MnO.....    | 48 |
| 115 | GTO importance profile for $\pi_-$ orbitals on O atom in ScO.....  | 41 | 144 | STO importance profile for $\pi_+$ orbitals on O atom in NiO.....    | 48 |
| 116 | GTO importance profile for $\pi_-$ orbitals on O atom in SeO.....  | 41 | 145 | STO importance profile for $\pi_+$ orbitals on O atom in ScO.....    | 49 |
| 117 | GTO importance profile for $\pi_-$ orbitals on O atom in TiO.....  | 42 | 146 | STO importance profile for $\pi_+$ orbitals on O atom in SeO.....    | 49 |
| 118 | GTO importance profile for $\pi_-$ orbitals on O atom in VO.....   | 42 | 147 | STO importance profile for $\pi_+$ orbitals on O atom in TiO.....    | 49 |
| 119 | STO importance profile for $\pi_-$ orbitals on O atom in CO.....   | 42 | 148 | STO importance profile for $\pi_+$ orbitals on O atom in VO.....     | 49 |
| 120 | STO importance profile for $\pi_-$ orbitals on O atom in FeO.....  | 42 | 149 | GTO importance profile for $\delta_-$ orbitals on O atom in FeO..... | 50 |
| 121 | STO importance profile for $\pi_-$ orbitals on O atom in GaO.....  | 43 | 150 | GTO importance profile for $\delta_-$ orbitals on O atom in GaO..... | 50 |
| 122 | STO importance profile for $\pi_-$ orbitals on O atom in GeO.....  | 43 | 151 | GTO importance profile for $\delta_-$ orbitals on O atom in GeO..... | 50 |
| 123 | STO importance profile for $\pi_-$ orbitals on O atom in MnO.....  | 43 | 152 | GTO importance profile for $\delta_-$ orbitals on O atom in MnO..... | 50 |
| 124 | STO importance profile for $\pi_-$ orbitals on O atom in NiO.....  | 43 | 153 | GTO importance profile for $\delta_-$ orbitals on O atom in NiO..... | 51 |
| 125 | STO importance profile for $\pi_-$ orbitals on O atom in ScO.....  | 44 | 154 | GTO importance profile for $\delta_-$ orbitals on O atom in ScO..... | 51 |
| 126 | STO importance profile for $\pi_-$ orbitals on O atom in SeO.....  | 44 | 155 | GTO importance profile for $\delta_-$ orbitals on O atom in SeO..... | 51 |

|     |                                                                       |    |     |                                                                                 |    |
|-----|-----------------------------------------------------------------------|----|-----|---------------------------------------------------------------------------------|----|
| 156 | GTO importance profile for $\delta_-$ orbitals on O atom in TiO. .... | 51 | 185 | GTO importance profile for $\sigma$ orbitals on F atom in ClF. ....             | 59 |
| 157 | GTO importance profile for $\delta_-$ orbitals on O atom in VO. ....  | 52 | 186 | GTO importance profile for $\sigma$ orbitals on F atom in CuF. ....             | 59 |
| 158 | STO importance profile for $\delta_-$ orbitals on O atom in FeO. .... | 52 | 187 | GTO importance profile for $\sigma$ orbitals on F atom in F <sub>2</sub> . .... | 59 |
| 159 | STO importance profile for $\delta_-$ orbitals on O atom in GaO. .... | 52 | 188 | GTO importance profile for $\sigma$ orbitals on F atom in GaF. ....             | 59 |
| 160 | STO importance profile for $\delta_-$ orbitals on O atom in GeO. .... | 52 | 189 | GTO importance profile for $\sigma$ orbitals on F atom in HF. ....              | 60 |
| 161 | STO importance profile for $\delta_-$ orbitals on O atom in MnO. .... | 53 | 190 | GTO importance profile for $\sigma$ orbitals on F atom in KF. ....              | 60 |
| 162 | STO importance profile for $\delta_-$ orbitals on O atom in NiO. .... | 53 | 191 | GTO importance profile for $\sigma$ orbitals on F atom in LiF. ....             | 60 |
| 163 | STO importance profile for $\delta_-$ orbitals on O atom in ScO. .... | 53 | 192 | GTO importance profile for $\sigma$ orbitals on F atom in MgF. ....             | 60 |
| 164 | STO importance profile for $\delta_-$ orbitals on O atom in SeO. .... | 53 | 193 | GTO importance profile for $\sigma$ orbitals on F atom in NaF. ....             | 61 |
| 165 | STO importance profile for $\delta_-$ orbitals on O atom in TiO. .... | 54 | 194 | STO importance profile for $\sigma$ orbitals on F atom in ClF. ....             | 61 |
| 166 | STO importance profile for $\delta_-$ orbitals on O atom in VO. ....  | 54 | 195 | STO importance profile for $\sigma$ orbitals on F atom in CuF. ....             | 61 |
| 167 | GTO importance profile for $\delta_+$ orbitals on O atom in FeO. .... | 54 | 196 | STO importance profile for $\sigma$ orbitals on F atom in F <sub>2</sub> . .... | 61 |
| 168 | GTO importance profile for $\delta_+$ orbitals on O atom in GaO. .... | 54 | 197 | STO importance profile for $\sigma$ orbitals on F atom in GaF. ....             | 62 |
| 169 | GTO importance profile for $\delta_+$ orbitals on O atom in GeO. .... | 55 | 198 | STO importance profile for $\sigma$ orbitals on F atom in HF. ....              | 62 |
| 170 | GTO importance profile for $\delta_+$ orbitals on O atom in MnO. .... | 55 | 199 | STO importance profile for $\sigma$ orbitals on F atom in KF. ....              | 62 |
| 171 | GTO importance profile for $\delta_+$ orbitals on O atom in NiO. .... | 55 | 200 | STO importance profile for $\sigma$ orbitals on F atom in LiF. ....             | 62 |
| 172 | GTO importance profile for $\delta_+$ orbitals on O atom in ScO. .... | 55 | 201 | STO importance profile for $\sigma$ orbitals on F atom in MgF. ....             | 63 |
| 173 | GTO importance profile for $\delta_+$ orbitals on O atom in SeO. .... | 56 | 202 | STO importance profile for $\sigma$ orbitals on F atom in NaF. ....             | 63 |
| 174 | GTO importance profile for $\delta_+$ orbitals on O atom in TiO. .... | 56 | 203 | GTO importance profile for $\pi_-$ orbitals on F atom in ClF. ....              | 63 |
| 175 | GTO importance profile for $\delta_+$ orbitals on O atom in VO. ....  | 56 | 204 | GTO importance profile for $\pi_-$ orbitals on F atom in CuF. ....              | 63 |
| 176 | STO importance profile for $\delta_+$ orbitals on O atom in FeO. .... | 56 | 205 | GTO importance profile for $\pi_-$ orbitals on F atom in F <sub>2</sub> . ....  | 64 |
| 177 | STO importance profile for $\delta_+$ orbitals on O atom in GaO. .... | 57 | 206 | GTO importance profile for $\pi_-$ orbitals on F atom in GaF. ....              | 64 |
| 178 | STO importance profile for $\delta_+$ orbitals on O atom in GeO. .... | 57 | 207 | GTO importance profile for $\pi_-$ orbitals on F atom in HF. ....               | 64 |
| 179 | STO importance profile for $\delta_+$ orbitals on O atom in MnO. .... | 57 | 208 | GTO importance profile for $\pi_-$ orbitals on F atom in KF. ....               | 64 |
| 180 | STO importance profile for $\delta_+$ orbitals on O atom in NiO. .... | 57 | 209 | GTO importance profile for $\pi_-$ orbitals on F atom in LiF. ....              | 65 |
| 181 | STO importance profile for $\delta_+$ orbitals on O atom in ScO. .... | 58 | 210 | GTO importance profile for $\pi_-$ orbitals on F atom in MgF. ....              | 65 |
| 182 | STO importance profile for $\delta_+$ orbitals on O atom in SeO. .... | 58 | 211 | GTO importance profile for $\pi_-$ orbitals on F atom in NaF. ....              | 65 |
| 183 | STO importance profile for $\delta_+$ orbitals on O atom in TiO. .... | 58 | 212 | STO importance profile for $\pi_-$ orbitals on F atom in ClF. ....              | 65 |
| 184 | STO importance profile for $\delta_+$ orbitals on O atom in VO. ....  | 58 | 213 | STO importance profile for $\pi_-$ orbitals on F atom in CuF. ....              | 66 |

|     |                                                                       |    |     |                                                                       |    |
|-----|-----------------------------------------------------------------------|----|-----|-----------------------------------------------------------------------|----|
| 214 | STO importance profile for $\pi_-$ orbitals on F atom in $F_2$ .....  | 66 | 243 | GTO importance profile for $\delta_+$ orbitals on F atom in CuF. .... | 73 |
| 215 | STO importance profile for $\pi_-$ orbitals on F atom in GaF. ....    | 66 | 244 | GTO importance profile for $\delta_+$ orbitals on F atom in GaF. .... | 73 |
| 216 | STO importance profile for $\pi_-$ orbitals on F atom in HF. ....     | 66 | 245 | STO importance profile for $\delta_+$ orbitals on F atom in CuF. .... | 74 |
| 217 | STO importance profile for $\pi_-$ orbitals on F atom in KF. ....     | 67 | 246 | STO importance profile for $\delta_+$ orbitals on F atom in GaF. .... | 74 |
| 218 | STO importance profile for $\pi_-$ orbitals on F atom in LiF. ....    | 67 | 247 | GTO importance profile for $\sigma$ orbitals on Na atom in NaCl. .... | 74 |
| 219 | STO importance profile for $\pi_-$ orbitals on F atom in MgF. ....    | 67 | 248 | GTO importance profile for $\sigma$ orbitals on Na atom in NaF. ....  | 74 |
| 220 | STO importance profile for $\pi_-$ orbitals on F atom in NaF. ....    | 67 | 249 | GTO importance profile for $\sigma$ orbitals on Na atom in NaH. ....  | 75 |
| 221 | GTO importance profile for $\pi_+$ orbitals on F atom in ClF. ....    | 68 | 250 | STO importance profile for $\sigma$ orbitals on Na atom in NaCl. .... | 75 |
| 222 | GTO importance profile for $\pi_+$ orbitals on F atom in CuF. ....    | 68 | 251 | STO importance profile for $\sigma$ orbitals on Na atom in NaF. ....  | 75 |
| 223 | GTO importance profile for $\pi_+$ orbitals on F atom in $F_2$ . .... | 68 | 252 | STO importance profile for $\sigma$ orbitals on Na atom in NaH. ....  | 75 |
| 224 | GTO importance profile for $\pi_+$ orbitals on F atom in GaF. ....    | 68 | 253 | GTO importance profile for $\pi_-$ orbitals on Na atom in NaCl. ....  | 76 |
| 225 | GTO importance profile for $\pi_+$ orbitals on F atom in HF. ....     | 69 | 254 | GTO importance profile for $\pi_-$ orbitals on Na atom in NaF. ....   | 76 |
| 226 | GTO importance profile for $\pi_+$ orbitals on F atom in KF. ....     | 69 | 255 | GTO importance profile for $\pi_-$ orbitals on Na atom in NaH. ....   | 76 |
| 227 | GTO importance profile for $\pi_+$ orbitals on F atom in LiF. ....    | 69 | 256 | STO importance profile for $\pi_-$ orbitals on Na atom in NaCl. ....  | 76 |
| 228 | GTO importance profile for $\pi_+$ orbitals on F atom in MgF. ....    | 69 | 257 | STO importance profile for $\pi_-$ orbitals on Na atom in NaF. ....   | 77 |
| 229 | GTO importance profile for $\pi_+$ orbitals on F atom in NaF. ....    | 70 | 258 | STO importance profile for $\pi_-$ orbitals on Na atom in NaH. ....   | 77 |
| 230 | STO importance profile for $\pi_+$ orbitals on F atom in ClF. ....    | 70 | 259 | GTO importance profile for $\pi_+$ orbitals on Na atom in NaCl. ....  | 77 |
| 231 | STO importance profile for $\pi_+$ orbitals on F atom in CuF. ....    | 70 | 260 | GTO importance profile for $\pi_+$ orbitals on Na atom in NaF. ....   | 77 |
| 232 | STO importance profile for $\pi_+$ orbitals on F atom in $F_2$ . .... | 70 | 261 | GTO importance profile for $\pi_+$ orbitals on Na atom in NaH. ....   | 78 |
| 233 | STO importance profile for $\pi_+$ orbitals on F atom in GaF. ....    | 71 | 262 | STO importance profile for $\pi_+$ orbitals on Na atom in NaCl. ....  | 78 |
| 234 | STO importance profile for $\pi_+$ orbitals on F atom in HF. ....     | 71 | 263 | STO importance profile for $\pi_+$ orbitals on Na atom in NaF. ....   | 78 |
| 235 | STO importance profile for $\pi_+$ orbitals on F atom in KF. ....     | 71 | 264 | STO importance profile for $\pi_+$ orbitals on Na atom in NaH. ....   | 78 |
| 236 | STO importance profile for $\pi_+$ orbitals on F atom in LiF. ....    | 71 | 265 | GTO importance profile for $\sigma$ orbitals on Mg atom in MgF. ....  | 79 |
| 237 | STO importance profile for $\pi_+$ orbitals on F atom in MgF. ....    | 72 | 266 | STO importance profile for $\sigma$ orbitals on Mg atom in MgF. ....  | 79 |
| 238 | STO importance profile for $\pi_+$ orbitals on F atom in NaF. ....    | 72 | 267 | GTO importance profile for $\pi_-$ orbitals on Mg atom in MgF. ....   | 79 |
| 239 | GTO importance profile for $\delta_-$ orbitals on F atom in CuF. .... | 72 | 268 | STO importance profile for $\pi_-$ orbitals on Mg atom in MgF. ....   | 79 |
| 240 | GTO importance profile for $\delta_-$ orbitals on F atom in GaF. .... | 72 | 269 | GTO importance profile for $\pi_+$ orbitals on Mg atom in MgF. ....   | 80 |
| 241 | STO importance profile for $\delta_-$ orbitals on F atom in CuF. .... | 73 | 270 | STO importance profile for $\pi_+$ orbitals on Mg atom in MgF. ....   | 80 |
| 242 | STO importance profile for $\delta_-$ orbitals on F atom in GaF. .... | 73 | 271 | GTO importance profile for $\sigma$ orbitals on Al atom in AlN. ....  | 80 |

|     |                                                                                |    |     |                                                                                  |    |
|-----|--------------------------------------------------------------------------------|----|-----|----------------------------------------------------------------------------------|----|
| 272 | STO importance profile for $\sigma$ orbitals on Al atom in AlN.....            | 80 | 301 | GTO importance profile for $\pi_+$ orbitals on S atom in NiS.....                | 88 |
| 273 | GTO importance profile for $\pi_-$ orbitals on Al atom in AlN.....             | 81 | 302 | GTO importance profile for $\pi_+$ orbitals on S atom in S <sub>2</sub> .....    | 88 |
| 274 | STO importance profile for $\pi_-$ orbitals on Al atom in AlN.....             | 81 | 303 | STO importance profile for $\pi_+$ orbitals on S atom in BeS.....                | 88 |
| 275 | GTO importance profile for $\pi_+$ orbitals on Al atom in AlN.....             | 81 | 304 | STO importance profile for $\pi_+$ orbitals on S atom in MnS.....                | 88 |
| 276 | STO importance profile for $\pi_+$ orbitals on Al atom in AlN.....             | 81 | 305 | STO importance profile for $\pi_+$ orbitals on S atom in NiS.....                | 89 |
| 277 | GTO importance profile for $\sigma$ orbitals on P atom in P <sub>2</sub> ..... | 82 | 306 | STO importance profile for $\pi_+$ orbitals on S atom in S <sub>2</sub> .....    | 89 |
| 278 | STO importance profile for $\sigma$ orbitals on P atom in P <sub>2</sub> ..... | 82 | 307 | GTO importance profile for $\delta_-$ orbitals on S atom in MnS.....             | 89 |
| 279 | GTO importance profile for $\pi_-$ orbitals on P atom in P <sub>2</sub> .....  | 82 | 308 | GTO importance profile for $\delta_-$ orbitals on S atom in NiS.....             | 89 |
| 280 | STO importance profile for $\pi_-$ orbitals on P atom in P <sub>2</sub> .....  | 82 | 309 | STO importance profile for $\delta_-$ orbitals on S atom in MnS.....             | 90 |
| 281 | GTO importance profile for $\pi_+$ orbitals on P atom in P <sub>2</sub> .....  | 83 | 310 | STO importance profile for $\delta_-$ orbitals on S atom in NiS.....             | 90 |
| 282 | STO importance profile for $\pi_+$ orbitals on P atom in P <sub>2</sub> .....  | 83 | 311 | GTO importance profile for $\delta_+$ orbitals on S atom in MnS.....             | 90 |
| 283 | GTO importance profile for $\sigma$ orbitals on S atom in BeS.....             | 83 | 312 | GTO importance profile for $\delta_+$ orbitals on S atom in NiS.....             | 90 |
| 284 | GTO importance profile for $\sigma$ orbitals on S atom in MnS.....             | 83 | 313 | STO importance profile for $\delta_+$ orbitals on S atom in MnS.....             | 91 |
| 285 | GTO importance profile for $\sigma$ orbitals on S atom in NiS.....             | 84 | 314 | STO importance profile for $\delta_+$ orbitals on S atom in NiS.....             | 91 |
| 286 | GTO importance profile for $\sigma$ orbitals on S atom in S <sub>2</sub> ..... | 84 | 315 | GTO importance profile for $\sigma$ orbitals on Cl atom in BrCl.....             | 91 |
| 287 | STO importance profile for $\sigma$ orbitals on S atom in BeS.....             | 84 | 316 | GTO importance profile for $\sigma$ orbitals on Cl atom in Cl <sub>2</sub> ..... | 91 |
| 288 | STO importance profile for $\sigma$ orbitals on S atom in MnS.....             | 84 | 317 | GTO importance profile for $\sigma$ orbitals on Cl atom in ClF.....              | 92 |
| 289 | STO importance profile for $\sigma$ orbitals on S atom in NiS.....             | 85 | 318 | GTO importance profile for $\sigma$ orbitals on Cl atom in CuCl.....             | 92 |
| 290 | STO importance profile for $\sigma$ orbitals on S atom in S <sub>2</sub> ..... | 85 | 319 | GTO importance profile for $\sigma$ orbitals on Cl atom in GaCl.....             | 92 |
| 291 | GTO importance profile for $\pi_-$ orbitals on S atom in BeS.....              | 85 | 320 | GTO importance profile for $\sigma$ orbitals on Cl atom in HCl.....              | 92 |
| 292 | GTO importance profile for $\pi_-$ orbitals on S atom in MnS.....              | 85 | 321 | GTO importance profile for $\sigma$ orbitals on Cl atom in KCl.....              | 93 |
| 293 | GTO importance profile for $\pi_-$ orbitals on S atom in NiS.....              | 86 | 322 | GTO importance profile for $\sigma$ orbitals on Cl atom in LiCl.....             | 93 |
| 294 | GTO importance profile for $\pi_-$ orbitals on S atom in S <sub>2</sub> .....  | 86 | 323 | GTO importance profile for $\sigma$ orbitals on Cl atom in NaCl.....             | 93 |
| 295 | STO importance profile for $\pi_-$ orbitals on S atom in BeS.....              | 86 | 324 | STO importance profile for $\sigma$ orbitals on Cl atom in BrCl.....             | 93 |
| 296 | STO importance profile for $\pi_-$ orbitals on S atom in MnS.....              | 86 | 325 | STO importance profile for $\sigma$ orbitals on Cl atom in Cl <sub>2</sub> ..... | 94 |
| 297 | STO importance profile for $\pi_-$ orbitals on S atom in NiS.....              | 87 | 326 | STO importance profile for $\sigma$ orbitals on Cl atom in ClF.....              | 94 |
| 298 | STO importance profile for $\pi_-$ orbitals on S atom in S <sub>2</sub> .....  | 87 | 327 | STO importance profile for $\sigma$ orbitals on Cl atom in CuCl.....             | 94 |
| 299 | GTO importance profile for $\pi_+$ orbitals on S atom in BeS.....              | 87 | 328 | STO importance profile for $\sigma$ orbitals on Cl atom in GaCl.....             | 94 |
| 300 | GTO importance profile for $\pi_+$ orbitals on S atom in MnS.....              | 87 | 329 | STO importance profile for $\sigma$ orbitals on Cl atom in HCl.....              | 95 |

|     |                                                                                  |     |     |                                                                                  |     |
|-----|----------------------------------------------------------------------------------|-----|-----|----------------------------------------------------------------------------------|-----|
| 330 | STO importance profile for $\sigma$ orbitals on Cl atom in KCl. ....             | 95  | 359 | GTO importance profile for $\pi_+$ orbitals on Cl atom in NaCl. ....             | 102 |
| 331 | STO importance profile for $\sigma$ orbitals on Cl atom in LiCl. ....            | 95  | 360 | STO importance profile for $\pi_+$ orbitals on Cl atom in BrCl. ....             | 102 |
| 332 | STO importance profile for $\sigma$ orbitals on Cl atom in NaCl. ....            | 95  | 361 | STO importance profile for $\pi_+$ orbitals on Cl atom in Cl <sub>2</sub> . .... | 103 |
| 333 | GTO importance profile for $\pi_-$ orbitals on Cl atom in BrCl. ....             | 96  | 362 | STO importance profile for $\pi_+$ orbitals on Cl atom in ClF. ....              | 103 |
| 334 | GTO importance profile for $\pi_-$ orbitals on Cl atom in Cl <sub>2</sub> . .... | 96  | 363 | STO importance profile for $\pi_+$ orbitals on Cl atom in CuCl. ....             | 103 |
| 335 | GTO importance profile for $\pi_-$ orbitals on Cl atom in ClF. ....              | 96  | 364 | STO importance profile for $\pi_+$ orbitals on Cl atom in GaCl. ....             | 103 |
| 336 | GTO importance profile for $\pi_-$ orbitals on Cl atom in CuCl. ....             | 96  | 365 | STO importance profile for $\pi_+$ orbitals on Cl atom in HCl. ....              | 104 |
| 337 | GTO importance profile for $\pi_-$ orbitals on Cl atom in GaCl. ....             | 97  | 366 | STO importance profile for $\pi_+$ orbitals on Cl atom in KCl. ....              | 104 |
| 338 | GTO importance profile for $\pi_-$ orbitals on Cl atom in HCl. ....              | 97  | 367 | STO importance profile for $\pi_+$ orbitals on Cl atom in LiCl. ....             | 104 |
| 339 | GTO importance profile for $\pi_-$ orbitals on Cl atom in KCl. ....              | 97  | 368 | STO importance profile for $\pi_+$ orbitals on Cl atom in NaCl. ....             | 104 |
| 340 | GTO importance profile for $\pi_-$ orbitals on Cl atom in LiCl. ....             | 97  | 369 | GTO importance profile for $\delta_-$ orbitals on Cl atom in BrCl. ....          | 105 |
| 341 | GTO importance profile for $\pi_-$ orbitals on Cl atom in NaCl. ....             | 98  | 370 | GTO importance profile for $\delta_-$ orbitals on Cl atom in CuCl. ....          | 105 |
| 342 | STO importance profile for $\pi_-$ orbitals on Cl atom in BrCl. ....             | 98  | 371 | GTO importance profile for $\delta_-$ orbitals on Cl atom in GaCl. ....          | 105 |
| 343 | STO importance profile for $\pi_-$ orbitals on Cl atom in Cl <sub>2</sub> . .... | 98  | 372 | STO importance profile for $\delta_-$ orbitals on Cl atom in BrCl. ....          | 105 |
| 344 | STO importance profile for $\pi_-$ orbitals on Cl atom in ClF. ....              | 98  | 373 | STO importance profile for $\delta_-$ orbitals on Cl atom in CuCl. ....          | 106 |
| 345 | STO importance profile for $\pi_-$ orbitals on Cl atom in CuCl. ....             | 99  | 374 | STO importance profile for $\delta_-$ orbitals on Cl atom in GaCl. ....          | 106 |
| 346 | STO importance profile for $\pi_-$ orbitals on Cl atom in GaCl. ....             | 99  | 375 | GTO importance profile for $\delta_+$ orbitals on Cl atom in BrCl. ....          | 106 |
| 347 | STO importance profile for $\pi_-$ orbitals on Cl atom in HCl. ....              | 99  | 376 | GTO importance profile for $\delta_+$ orbitals on Cl atom in CuCl. ....          | 106 |
| 348 | STO importance profile for $\pi_-$ orbitals on Cl atom in KCl. ....              | 99  | 377 | GTO importance profile for $\delta_+$ orbitals on Cl atom in GaCl. ....          | 107 |
| 349 | STO importance profile for $\pi_-$ orbitals on Cl atom in LiCl. ....             | 100 | 378 | STO importance profile for $\delta_+$ orbitals on Cl atom in BrCl. ....          | 107 |
| 350 | STO importance profile for $\pi_-$ orbitals on Cl atom in NaCl. ....             | 100 | 379 | STO importance profile for $\delta_+$ orbitals on Cl atom in CuCl. ....          | 107 |
| 351 | GTO importance profile for $\pi_+$ orbitals on Cl atom in BrCl. ....             | 100 | 380 | STO importance profile for $\delta_+$ orbitals on Cl atom in GaCl. ....          | 107 |
| 352 | GTO importance profile for $\pi_+$ orbitals on Cl atom in Cl <sub>2</sub> . .... | 100 | 381 | GTO importance profile for $\sigma$ orbitals on K atom in KBr. ....              | 108 |
| 353 | GTO importance profile for $\pi_+$ orbitals on Cl atom in ClF. ....              | 101 | 382 | GTO importance profile for $\sigma$ orbitals on K atom in KCl. ....              | 108 |
| 354 | GTO importance profile for $\pi_+$ orbitals on Cl atom in CuCl. ....             | 101 | 383 | GTO importance profile for $\sigma$ orbitals on K atom in KF. ....               | 108 |
| 355 | GTO importance profile for $\pi_+$ orbitals on Cl atom in GaCl. ....             | 101 | 384 | GTO importance profile for $\sigma$ orbitals on K atom in KH. ....               | 108 |
| 356 | GTO importance profile for $\pi_+$ orbitals on Cl atom in HCl. ....              | 101 | 385 | STO importance profile for $\sigma$ orbitals on K atom in KBr. ....              | 109 |
| 357 | GTO importance profile for $\pi_+$ orbitals on Cl atom in KCl. ....              | 102 | 386 | STO importance profile for $\sigma$ orbitals on K atom in KCl. ....              | 109 |
| 358 | GTO importance profile for $\pi_+$ orbitals on Cl atom in LiCl. ....             | 102 | 387 | STO importance profile for $\sigma$ orbitals on K atom in KF. ....               | 109 |

|     |                                                                        |     |     |                                                                        |     |
|-----|------------------------------------------------------------------------|-----|-----|------------------------------------------------------------------------|-----|
| 388 | STO importance profile for $\sigma$ orbitals on K atom in KH. ....     | 109 | 417 | GTO importance profile for $\delta_+$ orbitals on Sc atom in ScO. .... | 117 |
| 389 | GTO importance profile for $\pi_-$ orbitals on K atom in KBr. ....     | 110 | 418 | STO importance profile for $\delta_+$ orbitals on Sc atom in ScO. .... | 117 |
| 390 | GTO importance profile for $\pi_-$ orbitals on K atom in KCl. ....     | 110 | 419 | GTO importance profile for $\sigma$ orbitals on Ti atom in TiO. ....   | 117 |
| 391 | GTO importance profile for $\pi_-$ orbitals on K atom in KF. ....      | 110 | 420 | STO importance profile for $\sigma$ orbitals on Ti atom in TiO. ....   | 117 |
| 392 | GTO importance profile for $\pi_-$ orbitals on K atom in KH. ....      | 110 | 421 | GTO importance profile for $\pi_-$ orbitals on Ti atom in TiO. ....    | 118 |
| 393 | STO importance profile for $\pi_-$ orbitals on K atom in KBr. ....     | 111 | 422 | STO importance profile for $\pi_-$ orbitals on Ti atom in TiO. ....    | 118 |
| 394 | STO importance profile for $\pi_-$ orbitals on K atom in KCl. ....     | 111 | 423 | GTO importance profile for $\pi_+$ orbitals on Ti atom in TiO. ....    | 118 |
| 395 | STO importance profile for $\pi_-$ orbitals on K atom in KF. ....      | 111 | 424 | STO importance profile for $\pi_+$ orbitals on Ti atom in TiO. ....    | 118 |
| 396 | STO importance profile for $\pi_-$ orbitals on K atom in KH. ....      | 111 | 425 | GTO importance profile for $\delta_-$ orbitals on Ti atom in TiO. .... | 119 |
| 397 | GTO importance profile for $\pi_+$ orbitals on K atom in KBr. ....     | 112 | 426 | STO importance profile for $\delta_-$ orbitals on Ti atom in TiO. .... | 119 |
| 398 | GTO importance profile for $\pi_+$ orbitals on K atom in KCl. ....     | 112 | 427 | GTO importance profile for $\delta_+$ orbitals on Ti atom in TiO. .... | 119 |
| 399 | GTO importance profile for $\pi_+$ orbitals on K atom in KF. ....      | 112 | 428 | STO importance profile for $\delta_+$ orbitals on Ti atom in TiO. .... | 119 |
| 400 | GTO importance profile for $\pi_+$ orbitals on K atom in KH. ....      | 112 | 429 | GTO importance profile for $\sigma$ orbitals on V atom in VO. ....     | 120 |
| 401 | STO importance profile for $\pi_+$ orbitals on K atom in KBr. ....     | 113 | 430 | STO importance profile for $\sigma$ orbitals on V atom in VO. ....     | 120 |
| 402 | STO importance profile for $\pi_+$ orbitals on K atom in KCl. ....     | 113 | 431 | GTO importance profile for $\pi_-$ orbitals on V atom in VO. ....      | 120 |
| 403 | STO importance profile for $\pi_+$ orbitals on K atom in KF. ....      | 113 | 432 | STO importance profile for $\pi_-$ orbitals on V atom in VO. ....      | 120 |
| 404 | STO importance profile for $\pi_+$ orbitals on K atom in KH. ....      | 113 | 433 | GTO importance profile for $\pi_+$ orbitals on V atom in VO. ....      | 121 |
| 405 | GTO importance profile for $\delta_-$ orbitals on K atom in KBr. ....  | 114 | 434 | STO importance profile for $\pi_+$ orbitals on V atom in VO. ....      | 121 |
| 406 | STO importance profile for $\delta_-$ orbitals on K atom in KBr. ....  | 114 | 435 | GTO importance profile for $\delta_-$ orbitals on V atom in VO. ....   | 121 |
| 407 | GTO importance profile for $\delta_+$ orbitals on K atom in KBr. ....  | 114 | 436 | STO importance profile for $\delta_-$ orbitals on V atom in VO. ....   | 121 |
| 408 | STO importance profile for $\delta_+$ orbitals on K atom in KBr. ....  | 114 | 437 | GTO importance profile for $\delta_+$ orbitals on V atom in VO. ....   | 122 |
| 409 | GTO importance profile for $\sigma$ orbitals on Sc atom in ScO. ....   | 115 | 438 | STO importance profile for $\delta_+$ orbitals on V atom in VO. ....   | 122 |
| 410 | STO importance profile for $\sigma$ orbitals on Sc atom in ScO. ....   | 115 | 439 | GTO importance profile for $\sigma$ orbitals on Mn atom in MnO. ....   | 122 |
| 411 | GTO importance profile for $\pi_-$ orbitals on Sc atom in ScO. ....    | 115 | 440 | GTO importance profile for $\sigma$ orbitals on Mn atom in MnS. ....   | 122 |
| 412 | STO importance profile for $\pi_-$ orbitals on Sc atom in ScO. ....    | 115 | 441 | STO importance profile for $\sigma$ orbitals on Mn atom in MnO. ....   | 123 |
| 413 | GTO importance profile for $\pi_+$ orbitals on Sc atom in ScO. ....    | 116 | 442 | STO importance profile for $\sigma$ orbitals on Mn atom in MnS. ....   | 123 |
| 414 | STO importance profile for $\pi_+$ orbitals on Sc atom in ScO. ....    | 116 | 443 | GTO importance profile for $\pi_-$ orbitals on Mn atom in MnO. ....    | 123 |
| 415 | GTO importance profile for $\delta_-$ orbitals on Sc atom in ScO. .... | 116 | 444 | GTO importance profile for $\pi_-$ orbitals on Mn atom in MnS. ....    | 123 |
| 416 | STO importance profile for $\delta_-$ orbitals on Sc atom in ScO. .... | 116 | 445 | STO importance profile for $\pi_-$ orbitals on Mn atom in MnO. ....    | 124 |



|     |                                                                        |     |     |                                                                                   |     |
|-----|------------------------------------------------------------------------|-----|-----|-----------------------------------------------------------------------------------|-----|
| 446 | STO importance profile for $\pi_-$ orbitals on Mn atom in MnS. ....    | 124 | 475 | STO importance profile for $\pi_-$ orbitals on Ni atom in NiO. ....               | 131 |
| 447 | GTO importance profile for $\pi_+$ orbitals on Mn atom in MnO. ....    | 124 | 476 | STO importance profile for $\pi_-$ orbitals on Ni atom in NiS. ....               | 131 |
| 448 | GTO importance profile for $\pi_+$ orbitals on Mn atom in MnS. ....    | 124 | 477 | GTO importance profile for $\pi_+$ orbitals on Ni atom in NiO. ....               | 132 |
| 449 | STO importance profile for $\pi_+$ orbitals on Mn atom in MnO. ....    | 125 | 478 | GTO importance profile for $\pi_+$ orbitals on Ni atom in NiS. ....               | 132 |
| 450 | STO importance profile for $\pi_+$ orbitals on Mn atom in MnS. ....    | 125 | 479 | STO importance profile for $\pi_+$ orbitals on Ni atom in NiO. ....               | 132 |
| 451 | GTO importance profile for $\delta_-$ orbitals on Mn atom in MnO. .... | 125 | 480 | STO importance profile for $\pi_+$ orbitals on Ni atom in NiS. ....               | 132 |
| 452 | GTO importance profile for $\delta_-$ orbitals on Mn atom in MnS. .... | 125 | 481 | GTO importance profile for $\delta_-$ orbitals on Ni atom in NiO. ....            | 133 |
| 453 | STO importance profile for $\delta_-$ orbitals on Mn atom in MnO. .... | 126 | 482 | GTO importance profile for $\delta_-$ orbitals on Ni atom in NiS. ....            | 133 |
| 454 | STO importance profile for $\delta_-$ orbitals on Mn atom in MnS. .... | 126 | 483 | STO importance profile for $\delta_-$ orbitals on Ni atom in NiO. ....            | 133 |
| 455 | GTO importance profile for $\delta_+$ orbitals on Mn atom in MnO. .... | 126 | 484 | STO importance profile for $\delta_-$ orbitals on Ni atom in NiS. ....            | 133 |
| 456 | GTO importance profile for $\delta_+$ orbitals on Mn atom in MnS. .... | 126 | 485 | GTO importance profile for $\delta_+$ orbitals on Ni atom in NiO. ....            | 134 |
| 457 | STO importance profile for $\delta_+$ orbitals on Mn atom in MnO. .... | 127 | 486 | GTO importance profile for $\delta_+$ orbitals on Ni atom in NiS. ....            | 134 |
| 458 | STO importance profile for $\delta_+$ orbitals on Mn atom in MnS. .... | 127 | 487 | STO importance profile for $\delta_+$ orbitals on Ni atom in NiO. ....            | 134 |
| 459 | GTO importance profile for $\sigma$ orbitals on Fe atom in FeO. ....   | 127 | 488 | STO importance profile for $\delta_+$ orbitals on Ni atom in NiS. ....            | 134 |
| 460 | STO importance profile for $\sigma$ orbitals on Fe atom in FeO. ....   | 127 | 489 | GTO importance profile for $\sigma$ orbitals on Cu atom in Cu <sub>2</sub> . .... | 135 |
| 461 | GTO importance profile for $\pi_-$ orbitals on Fe atom in FeO. ....    | 128 | 490 | GTO importance profile for $\sigma$ orbitals on Cu atom in CuCl. ....             | 135 |
| 462 | STO importance profile for $\pi_-$ orbitals on Fe atom in FeO. ....    | 128 | 491 | GTO importance profile for $\sigma$ orbitals on Cu atom in CuF. ....              | 135 |
| 463 | GTO importance profile for $\pi_+$ orbitals on Fe atom in FeO. ....    | 128 | 492 | GTO importance profile for $\sigma$ orbitals on Cu atom in CuH. ....              | 135 |
| 464 | STO importance profile for $\pi_+$ orbitals on Fe atom in FeO. ....    | 128 | 493 | STO importance profile for $\sigma$ orbitals on Cu atom in Cu <sub>2</sub> . .... | 136 |
| 465 | GTO importance profile for $\delta_-$ orbitals on Fe atom in FeO. .... | 129 | 494 | STO importance profile for $\sigma$ orbitals on Cu atom in CuCl. ....             | 136 |
| 466 | STO importance profile for $\delta_-$ orbitals on Fe atom in FeO. .... | 129 | 495 | STO importance profile for $\sigma$ orbitals on Cu atom in CuF. ....              | 136 |
| 467 | GTO importance profile for $\delta_+$ orbitals on Fe atom in FeO. .... | 129 | 496 | STO importance profile for $\sigma$ orbitals on Cu atom in CuH. ....              | 136 |
| 468 | STO importance profile for $\delta_+$ orbitals on Fe atom in FeO. .... | 129 | 497 | GTO importance profile for $\pi_-$ orbitals on Cu atom in Cu <sub>2</sub> . ....  | 137 |
| 469 | GTO importance profile for $\sigma$ orbitals on Ni atom in NiO. ....   | 130 | 498 | GTO importance profile for $\pi_-$ orbitals on Cu atom in CuCl. ....              | 137 |
| 470 | GTO importance profile for $\sigma$ orbitals on Ni atom in NiS. ....   | 130 | 499 | GTO importance profile for $\pi_-$ orbitals on Cu atom in CuF. ....               | 137 |
| 471 | STO importance profile for $\sigma$ orbitals on Ni atom in NiO. ....   | 130 | 500 | GTO importance profile for $\pi_-$ orbitals on Cu atom in CuH. ....               | 137 |
| 472 | STO importance profile for $\sigma$ orbitals on Ni atom in NiS. ....   | 130 | 501 | STO importance profile for $\pi_-$ orbitals on Cu atom in Cu <sub>2</sub> . ....  | 138 |
| 473 | GTO importance profile for $\pi_-$ orbitals on Ni atom in NiO. ....    | 131 | 502 | STO importance profile for $\pi_-$ orbitals on Cu atom in CuCl. ....              | 138 |
| 474 | GTO importance profile for $\pi_-$ orbitals on Ni atom in NiS. ....    | 131 | 503 | STO importance profile for $\pi_-$ orbitals on Cu atom in CuF. ....               | 138 |

|     |                                                                                        |     |     |                                                                            |     |
|-----|----------------------------------------------------------------------------------------|-----|-----|----------------------------------------------------------------------------|-----|
| 504 | STO importance profile for $\pi_-$ orbitals on<br>Cu atom in CuH. ....                 | 138 | 533 | STO importance profile for $\sigma$ orbitals on<br>Ga atom in GaF. ....    | 146 |
| 505 | GTO importance profile for $\pi_+$ orbitals on<br>Cu atom in Cu <sub>2</sub> . ....    | 139 | 534 | STO importance profile for $\sigma$ orbitals on<br>Ga atom in GaO. ....    | 146 |
| 506 | GTO importance profile for $\pi_+$ orbitals on<br>Cu atom in CuCl. ....                | 139 | 535 | GTO importance profile for $\pi_-$ orbitals on<br>Ga atom in GaCl. ....    | 146 |
| 507 | GTO importance profile for $\pi_+$ orbitals on<br>Cu atom in CuF. ....                 | 139 | 536 | GTO importance profile for $\pi_-$ orbitals on<br>Ga atom in GaF. ....     | 146 |
| 508 | GTO importance profile for $\pi_+$ orbitals on<br>Cu atom in CuH. ....                 | 139 | 537 | GTO importance profile for $\pi_-$ orbitals on<br>Ga atom in GaO. ....     | 147 |
| 509 | STO importance profile for $\pi_+$ orbitals on<br>Cu atom in Cu <sub>2</sub> . ....    | 140 | 538 | STO importance profile for $\pi_-$ orbitals on<br>Ga atom in GaCl. ....    | 147 |
| 510 | STO importance profile for $\pi_+$ orbitals on<br>Cu atom in CuCl. ....                | 140 | 539 | STO importance profile for $\pi_-$ orbitals on<br>Ga atom in GaF. ....     | 147 |
| 511 | STO importance profile for $\pi_+$ orbitals on<br>Cu atom in CuF. ....                 | 140 | 540 | STO importance profile for $\pi_-$ orbitals on<br>Ga atom in GaO. ....     | 147 |
| 512 | STO importance profile for $\pi_+$ orbitals on<br>Cu atom in CuH. ....                 | 140 | 541 | GTO importance profile for $\pi_+$ orbitals on<br>Ga atom in GaCl. ....    | 148 |
| 513 | GTO importance profile for $\delta_-$ orbitals on<br>Cu atom in Cu <sub>2</sub> . .... | 141 | 542 | GTO importance profile for $\pi_+$ orbitals on<br>Ga atom in GaF. ....     | 148 |
| 514 | GTO importance profile for $\delta_-$ orbitals on<br>Cu atom in CuCl. ....             | 141 | 543 | GTO importance profile for $\pi_+$ orbitals on<br>Ga atom in GaO. ....     | 148 |
| 515 | GTO importance profile for $\delta_-$ orbitals on<br>Cu atom in CuF. ....              | 141 | 544 | STO importance profile for $\pi_+$ orbitals on<br>Ga atom in GaCl. ....    | 148 |
| 516 | GTO importance profile for $\delta_-$ orbitals on<br>Cu atom in CuH. ....              | 141 | 545 | STO importance profile for $\pi_+$ orbitals on<br>Ga atom in GaF. ....     | 149 |
| 517 | STO importance profile for $\delta_-$ orbitals on<br>Cu atom in Cu <sub>2</sub> . .... | 142 | 546 | STO importance profile for $\pi_+$ orbitals on<br>Ga atom in GaO. ....     | 149 |
| 518 | STO importance profile for $\delta_-$ orbitals on<br>Cu atom in CuCl. ....             | 142 | 547 | GTO importance profile for $\delta_-$ orbitals on<br>Ga atom in GaCl. .... | 149 |
| 519 | STO importance profile for $\delta_-$ orbitals on<br>Cu atom in CuF. ....              | 142 | 548 | GTO importance profile for $\delta_-$ orbitals on<br>Ga atom in GaF. ....  | 149 |
| 520 | STO importance profile for $\delta_-$ orbitals on<br>Cu atom in CuH. ....              | 142 | 549 | GTO importance profile for $\delta_-$ orbitals on<br>Ga atom in GaO. ....  | 150 |
| 521 | GTO importance profile for $\delta_+$ orbitals on<br>Cu atom in Cu <sub>2</sub> . .... | 143 | 550 | STO importance profile for $\delta_-$ orbitals on<br>Ga atom in GaCl. .... | 150 |
| 522 | GTO importance profile for $\delta_+$ orbitals on<br>Cu atom in CuCl. ....             | 143 | 551 | STO importance profile for $\delta_-$ orbitals on<br>Ga atom in GaF. ....  | 150 |
| 523 | GTO importance profile for $\delta_+$ orbitals on<br>Cu atom in CuF. ....              | 143 | 552 | STO importance profile for $\delta_-$ orbitals on<br>Ga atom in GaO. ....  | 150 |
| 524 | GTO importance profile for $\delta_+$ orbitals on<br>Cu atom in CuH. ....              | 143 | 553 | GTO importance profile for $\delta_+$ orbitals on<br>Ga atom in GaCl. .... | 151 |
| 525 | STO importance profile for $\delta_+$ orbitals on<br>Cu atom in Cu <sub>2</sub> . .... | 144 | 554 | GTO importance profile for $\delta_+$ orbitals on<br>Ga atom in GaF. ....  | 151 |
| 526 | STO importance profile for $\delta_+$ orbitals on<br>Cu atom in CuCl. ....             | 144 | 555 | GTO importance profile for $\delta_+$ orbitals on<br>Ga atom in GaO. ....  | 151 |
| 527 | STO importance profile for $\delta_+$ orbitals on<br>Cu atom in CuF. ....              | 144 | 556 | STO importance profile for $\delta_+$ orbitals on<br>Ga atom in GaCl. .... | 151 |
| 528 | STO importance profile for $\delta_+$ orbitals on<br>Cu atom in CuH. ....              | 144 | 557 | STO importance profile for $\delta_+$ orbitals on<br>Ga atom in GaF. ....  | 152 |
| 529 | GTO importance profile for $\sigma$ orbitals on<br>Ga atom in GaCl. ....               | 145 | 558 | STO importance profile for $\delta_+$ orbitals on<br>Ga atom in GaO. ....  | 152 |
| 530 | GTO importance profile for $\sigma$ orbitals on<br>Ga atom in GaF. ....                | 145 | 559 | GTO importance profile for $\sigma$ orbitals on<br>Ge atom in GeO. ....    | 152 |
| 531 | GTO importance profile for $\sigma$ orbitals on<br>Ga atom in GaO. ....                | 145 | 560 | STO importance profile for $\sigma$ orbitals on<br>Ge atom in GeO. ....    | 152 |
| 532 | STO importance profile for $\sigma$ orbitals on<br>Ga atom in GaCl. ....               | 145 | 561 | GTO importance profile for $\pi_-$ orbitals on<br>Ge atom in GeO. ....     | 153 |

|     |                                                                                      |     |     |                                                                                        |     |
|-----|--------------------------------------------------------------------------------------|-----|-----|----------------------------------------------------------------------------------------|-----|
| 562 | STO importance profile for $\pi_-$ orbitals on<br>Ge atom in GeO. ....               | 153 | 591 | STO importance profile for $\pi_-$ orbitals on<br>Br atom in Br <sub>2</sub> . ....    | 160 |
| 563 | GTO importance profile for $\pi_+$ orbitals on<br>Ge atom in GeO. ....               | 153 | 592 | STO importance profile for $\pi_-$ orbitals on<br>Br atom in BrCl. ....                | 160 |
| 564 | STO importance profile for $\pi_+$ orbitals on<br>Ge atom in GeO. ....               | 153 | 593 | STO importance profile for $\pi_-$ orbitals on<br>Br atom in HBr. ....                 | 161 |
| 565 | GTO importance profile for $\delta_-$ orbitals on<br>Ge atom in GeO. ....            | 154 | 594 | STO importance profile for $\pi_-$ orbitals on<br>Br atom in KBr. ....                 | 161 |
| 566 | STO importance profile for $\delta_-$ orbitals on<br>Ge atom in GeO. ....            | 154 | 595 | GTO importance profile for $\pi_+$ orbitals on<br>Br atom in Br <sub>2</sub> . ....    | 161 |
| 567 | GTO importance profile for $\delta_+$ orbitals on<br>Ge atom in GeO. ....            | 154 | 596 | GTO importance profile for $\pi_+$ orbitals on<br>Br atom in BrCl. ....                | 161 |
| 568 | STO importance profile for $\delta_+$ orbitals on<br>Ge atom in GeO. ....            | 154 | 597 | GTO importance profile for $\pi_+$ orbitals on<br>Br atom in HBr. ....                 | 162 |
| 569 | GTO importance profile for $\sigma$ orbitals on<br>Se atom in SeO. ....              | 155 | 598 | GTO importance profile for $\pi_+$ orbitals on<br>Br atom in KBr. ....                 | 162 |
| 570 | STO importance profile for $\sigma$ orbitals on<br>Se atom in SeO. ....              | 155 | 599 | STO importance profile for $\pi_+$ orbitals on<br>Br atom in Br <sub>2</sub> . ....    | 162 |
| 571 | GTO importance profile for $\pi_-$ orbitals on<br>Se atom in SeO. ....               | 155 | 600 | STO importance profile for $\pi_+$ orbitals on<br>Br atom in BrCl. ....                | 162 |
| 572 | STO importance profile for $\pi_-$ orbitals on<br>Se atom in SeO. ....               | 155 | 601 | STO importance profile for $\pi_+$ orbitals on<br>Br atom in HBr. ....                 | 163 |
| 573 | GTO importance profile for $\pi_+$ orbitals on<br>Se atom in SeO. ....               | 156 | 602 | STO importance profile for $\pi_+$ orbitals on<br>Br atom in KBr. ....                 | 163 |
| 574 | STO importance profile for $\pi_+$ orbitals on<br>Se atom in SeO. ....               | 156 | 603 | GTO importance profile for $\delta_-$ orbitals on<br>Br atom in Br <sub>2</sub> . .... | 163 |
| 575 | GTO importance profile for $\delta_-$ orbitals on<br>Se atom in SeO. ....            | 156 | 604 | GTO importance profile for $\delta_-$ orbitals on<br>Br atom in BrCl. ....             | 163 |
| 576 | STO importance profile for $\delta_-$ orbitals on<br>Se atom in SeO. ....            | 156 | 605 | GTO importance profile for $\delta_-$ orbitals on<br>Br atom in HBr. ....              | 164 |
| 577 | GTO importance profile for $\delta_+$ orbitals on<br>Se atom in SeO. ....            | 157 | 606 | GTO importance profile for $\delta_-$ orbitals on<br>Br atom in KBr. ....              | 164 |
| 578 | STO importance profile for $\delta_+$ orbitals on<br>Se atom in SeO. ....            | 157 | 607 | STO importance profile for $\delta_-$ orbitals on<br>Br atom in Br <sub>2</sub> . .... | 164 |
| 579 | GTO importance profile for $\sigma$ orbitals on<br>Br atom in Br <sub>2</sub> . .... | 157 | 608 | STO importance profile for $\delta_-$ orbitals on<br>Br atom in BrCl. ....             | 164 |
| 580 | GTO importance profile for $\sigma$ orbitals on<br>Br atom in BrCl. ....             | 157 | 609 | STO importance profile for $\delta_-$ orbitals on<br>Br atom in HBr. ....              | 165 |
| 581 | GTO importance profile for $\sigma$ orbitals on<br>Br atom in HBr. ....              | 158 | 610 | STO importance profile for $\delta_-$ orbitals on<br>Br atom in KBr. ....              | 165 |
| 582 | GTO importance profile for $\sigma$ orbitals on<br>Br atom in KBr. ....              | 158 | 611 | GTO importance profile for $\delta_+$ orbitals on<br>Br atom in Br <sub>2</sub> . .... | 165 |
| 583 | STO importance profile for $\sigma$ orbitals on<br>Br atom in Br <sub>2</sub> . .... | 158 | 612 | GTO importance profile for $\delta_+$ orbitals on<br>Br atom in BrCl. ....             | 165 |
| 584 | STO importance profile for $\sigma$ orbitals on<br>Br atom in BrCl. ....             | 158 | 613 | GTO importance profile for $\delta_+$ orbitals on<br>Br atom in HBr. ....              | 166 |
| 585 | STO importance profile for $\sigma$ orbitals on<br>Br atom in HBr. ....              | 159 | 614 | GTO importance profile for $\delta_+$ orbitals on<br>Br atom in KBr. ....              | 166 |
| 586 | STO importance profile for $\sigma$ orbitals on<br>Br atom in KBr. ....              | 159 | 615 | STO importance profile for $\delta_+$ orbitals on<br>Br atom in Br <sub>2</sub> . .... | 166 |
| 587 | GTO importance profile for $\pi_-$ orbitals on<br>Br atom in Br <sub>2</sub> . ....  | 159 | 616 | STO importance profile for $\delta_+$ orbitals on<br>Br atom in BrCl. ....             | 166 |
| 588 | GTO importance profile for $\pi_-$ orbitals on<br>Br atom in BrCl. ....              | 159 | 617 | STO importance profile for $\delta_+$ orbitals on<br>Br atom in HBr. ....              | 167 |
| 589 | GTO importance profile for $\pi_-$ orbitals on<br>Br atom in HBr. ....               | 160 | 618 | STO importance profile for $\delta_+$ orbitals on<br>Br atom in KBr. ....              | 167 |
| 590 | GTO importance profile for $\pi_-$ orbitals on<br>Br atom in KBr. ....               | 160 |     |                                                                                        |     |

## REFERENCES

- <sup>1</sup>S. Lehtola, “HelfEM – Finite element methods for electronic structure calculations on small systems,” (2023), accessed 26 March 2023.
- <sup>2</sup>S. Lehtola, “Fully numerical Hartree–Fock and density functional calculations. II. Diatomic molecules,” *Int. J. Quantum Chem.* **119**, e25944 (2019), arXiv:1810.11653.
- <sup>3</sup>F. Weigend and R. Ahlrichs, “Balanced basis sets of split valence, triple zeta valence and quadruple zeta valence quality for H to Rn: Design and assessment of accuracy,” *Phys. Chem. Chem. Phys.* **7**, 3297–305 (2005).
- <sup>4</sup>J. P. Perdew, K. Burke, and M. Ernzerhof, “Generalized gradient approximation made simple,” *Phys. Rev. Lett.* **77**, 3865–3868 (1996).
- <sup>5</sup>J. P. Perdew, K. Burke, and M. Ernzerhof, “Generalized gradient approximation made simple [Phys. Rev. Lett. 77, 3865 (1996)],” *Phys. Rev. Lett.* **78**, 1396–1396 (1997).
- <sup>6</sup>S. Lehtola, C. Steigemann, M. J. T. Oliveira, and M. A. L. Marques, “Recent developments in LIBXC—a comprehensive library of functionals for density functional theory,” *SoftwareX* **7**, 1–5 (2018).
- <sup>7</sup>S. Lehtola, “Assessment of initial guesses for self-consistent field calculations. superposition of atomic potentials: Simple yet efficient,” *J. Chem. Theory Comput.* **15**, 1593–1604 (2019), arXiv:1810.11659.

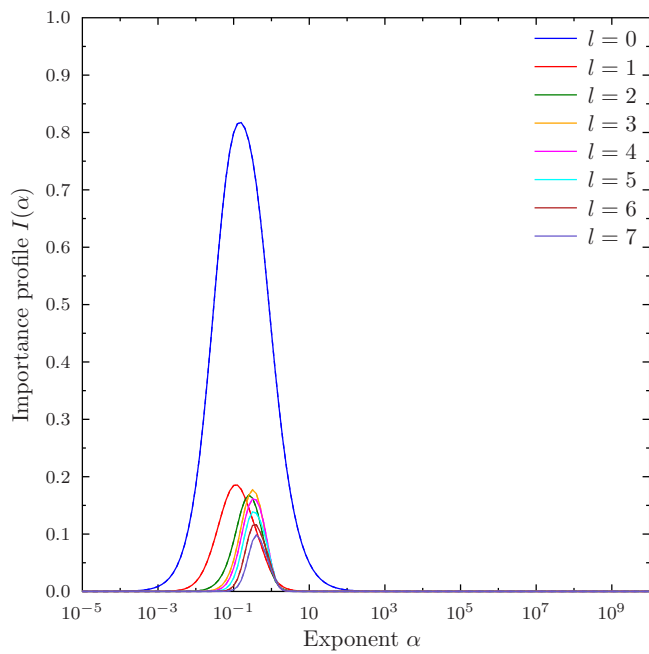

Figure 1. GTO importance profile for  $\sigma$  orbitals on H atom in CuH.

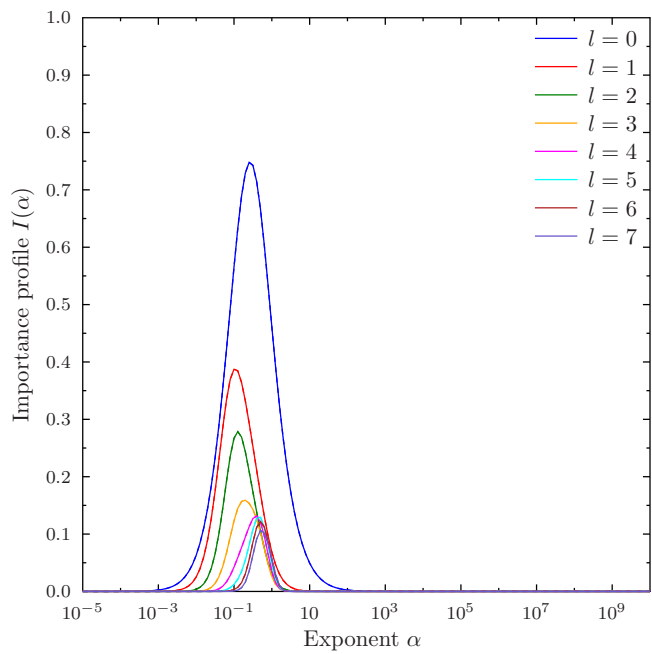

Figure 3. GTO importance profile for  $\sigma$  orbitals on H atom in HBr.

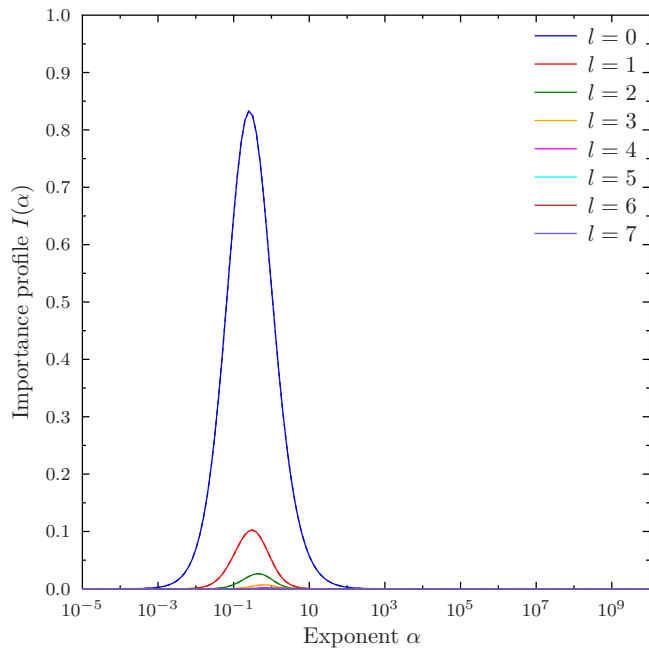

Figure 2. GTO importance profile for  $\sigma$  orbitals on H atom in  $H_2$ .

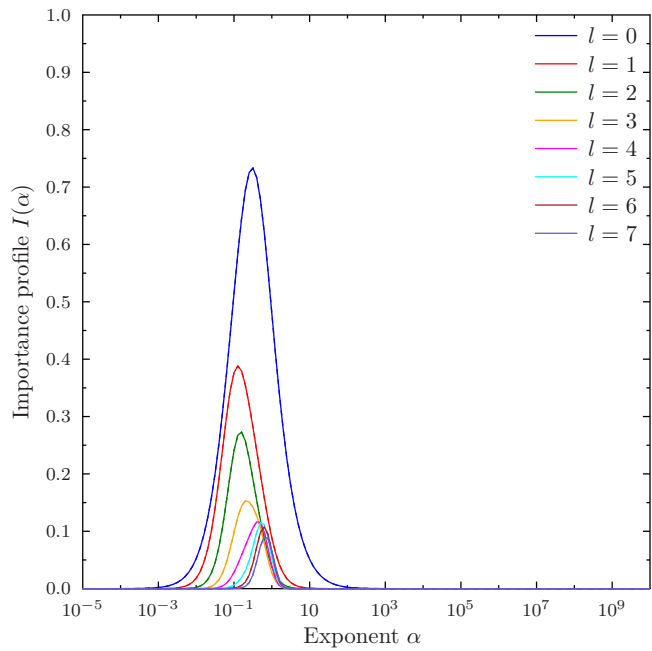

Figure 4. GTO importance profile for  $\sigma$  orbitals on H atom in HCl.

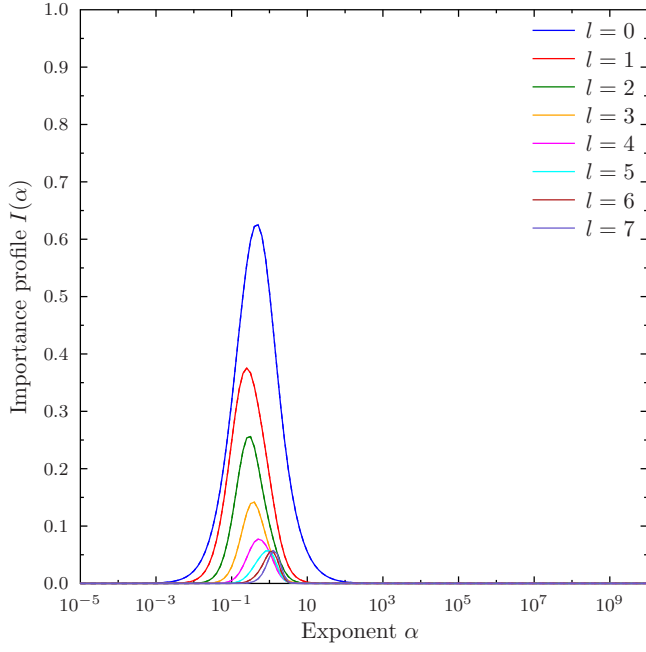

Figure 5. GTO importance profile for  $\sigma$  orbitals on H atom in HF.

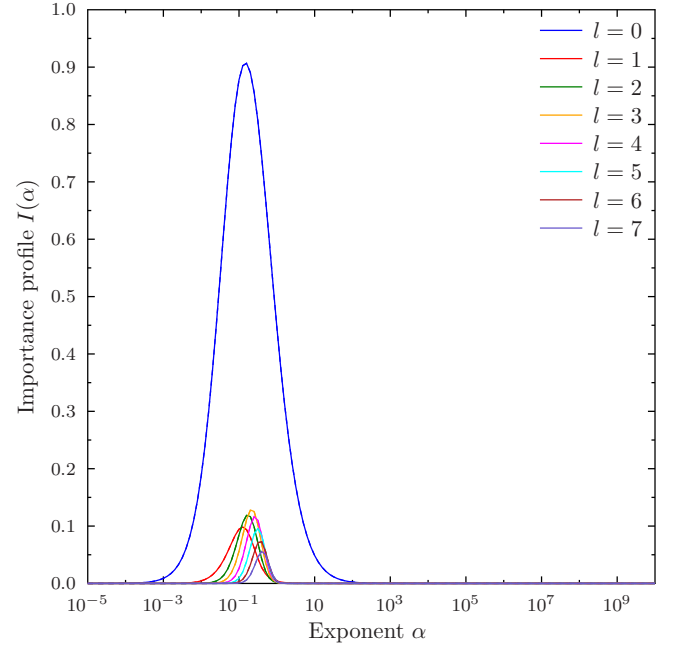

Figure 7. GTO importance profile for  $\sigma$  orbitals on H atom in LiH.

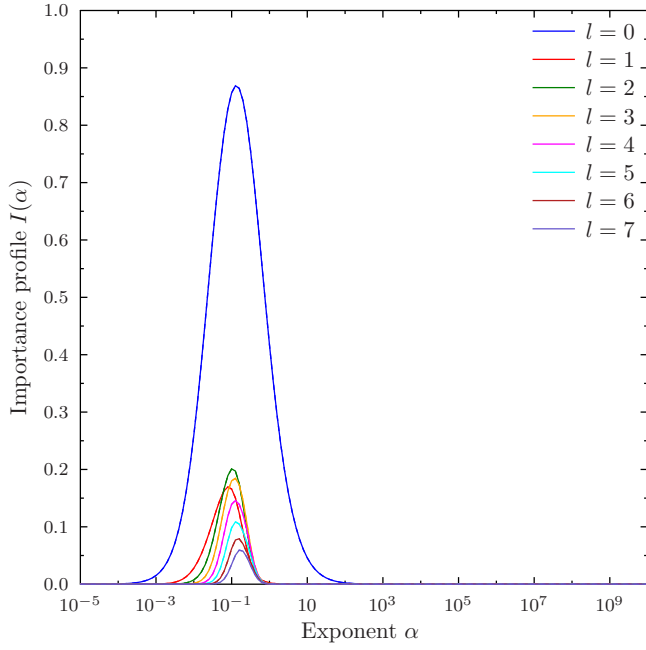

Figure 6. GTO importance profile for  $\sigma$  orbitals on H atom in KH.

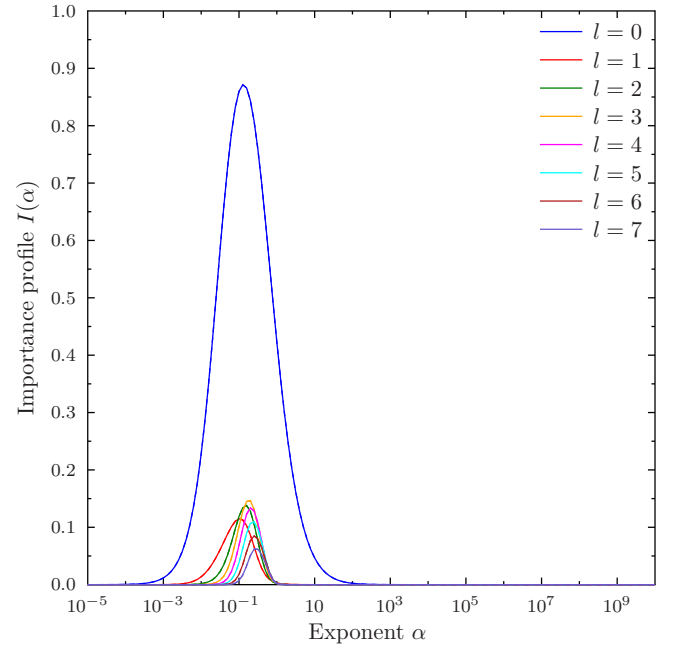

Figure 8. GTO importance profile for  $\sigma$  orbitals on H atom in NaH.

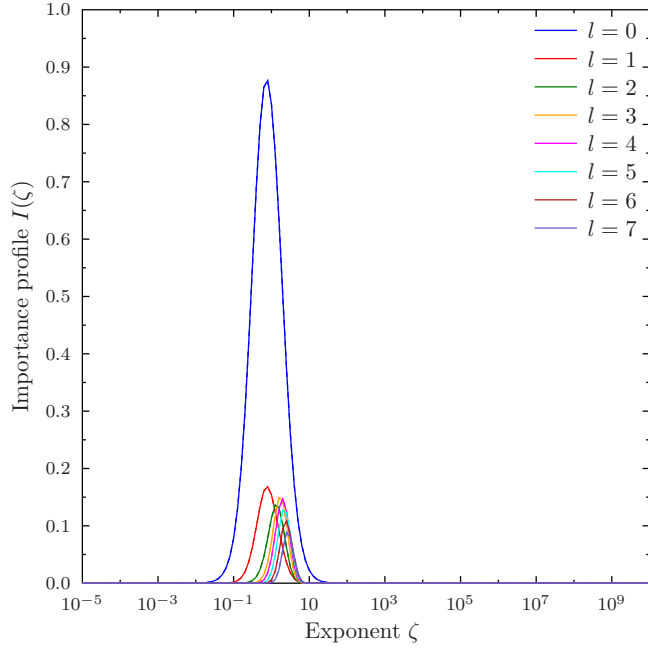

Figure 9. STO importance profile for  $\sigma$  orbitals on H atom in CuH.

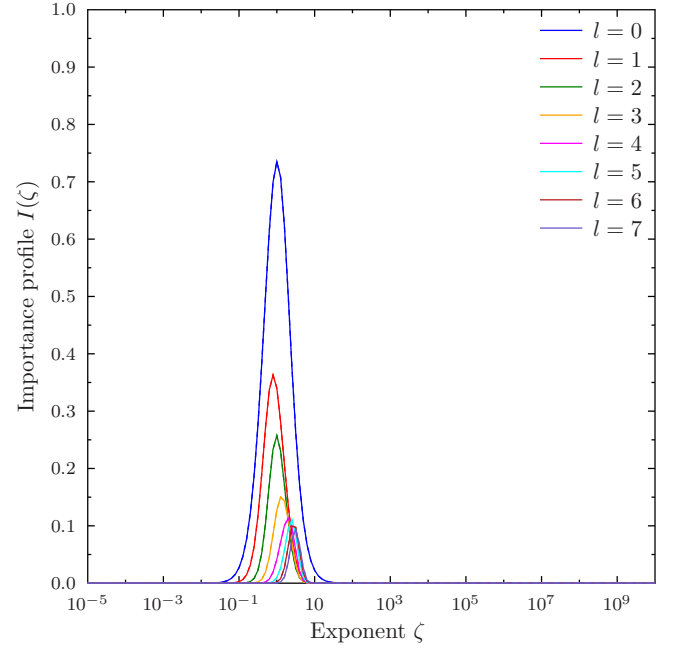

Figure 11. STO importance profile for  $\sigma$  orbitals on H atom in HBr.

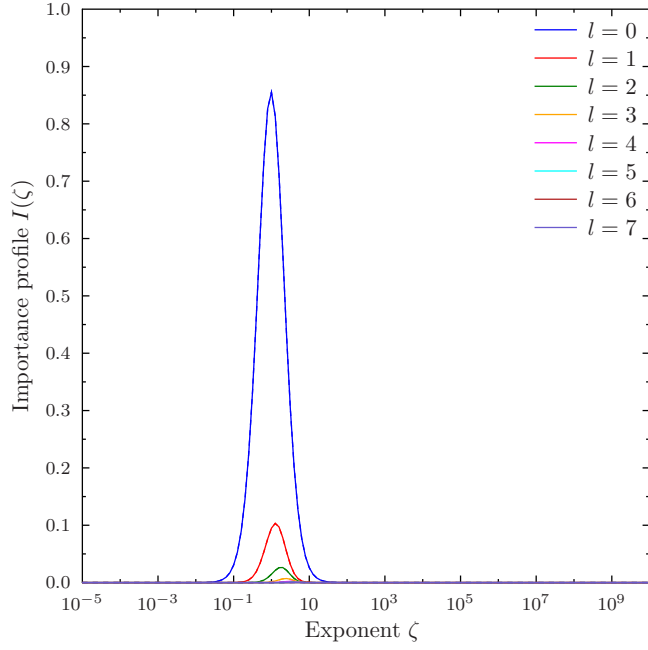

Figure 10. STO importance profile for  $\sigma$  orbitals on H atom in  $H_2$ .

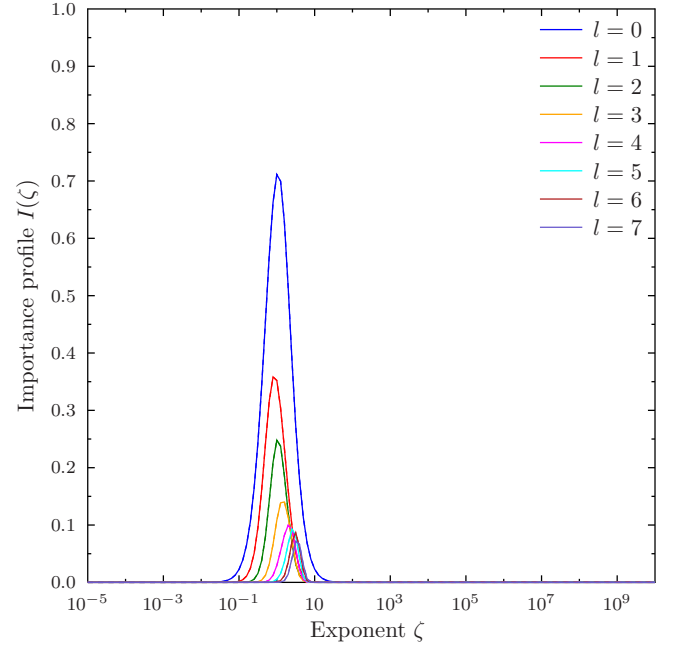

Figure 12. STO importance profile for  $\sigma$  orbitals on H atom in HCl.

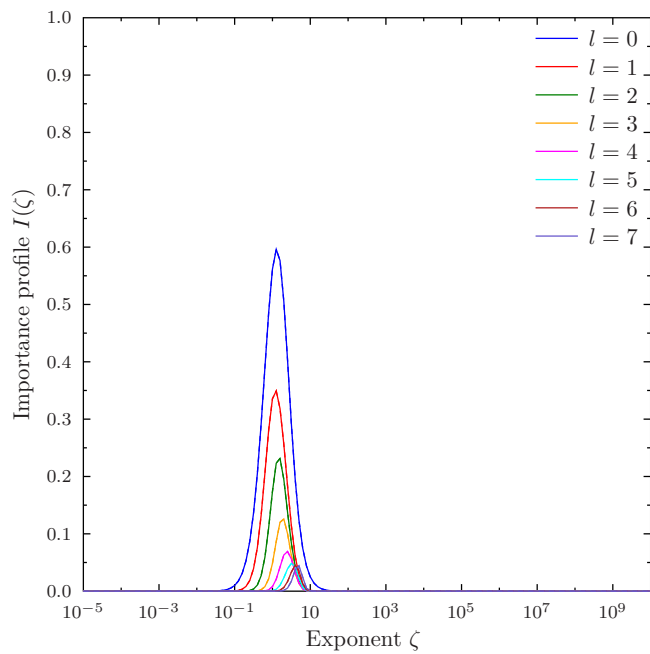

Figure 13. STO importance profile for  $\sigma$  orbitals on H atom in HF.

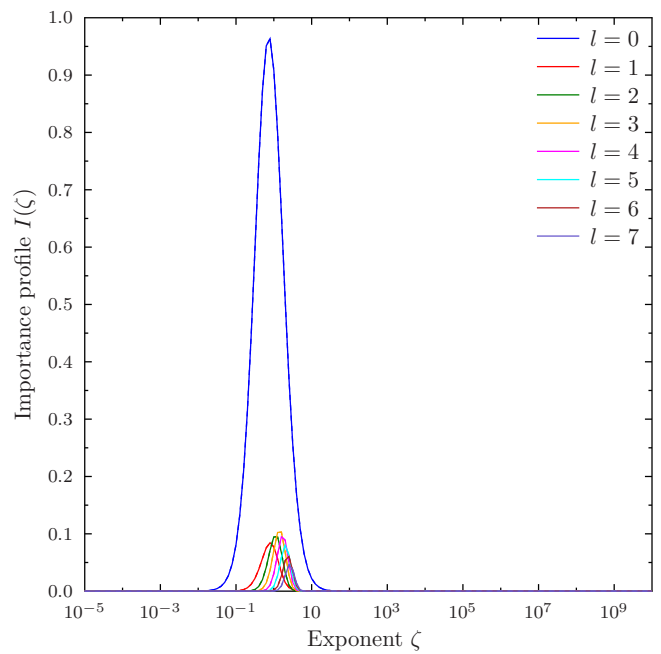

Figure 15. STO importance profile for  $\sigma$  orbitals on H atom in LiH.

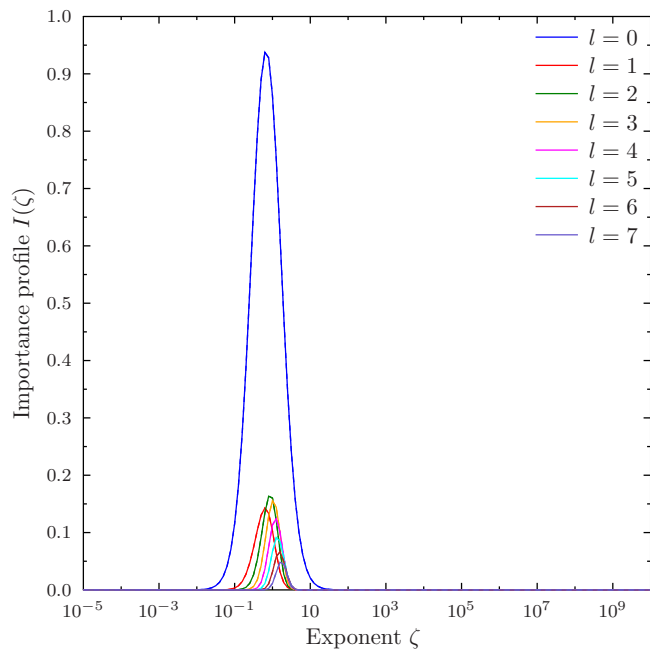

Figure 14. STO importance profile for  $\sigma$  orbitals on H atom in KH.

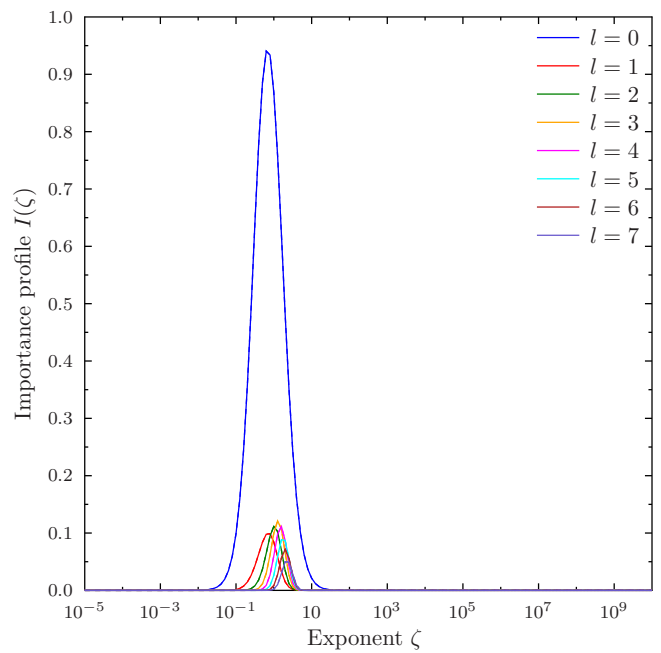

Figure 16. STO importance profile for  $\sigma$  orbitals on H atom in NaH.



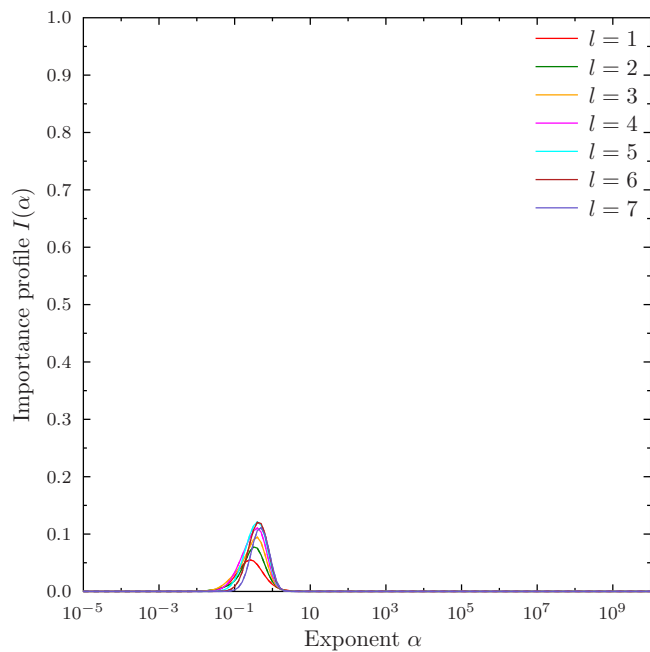

Figure 17. GTO importance profile for  $\pi_-$  orbitals on H atom in CuH.

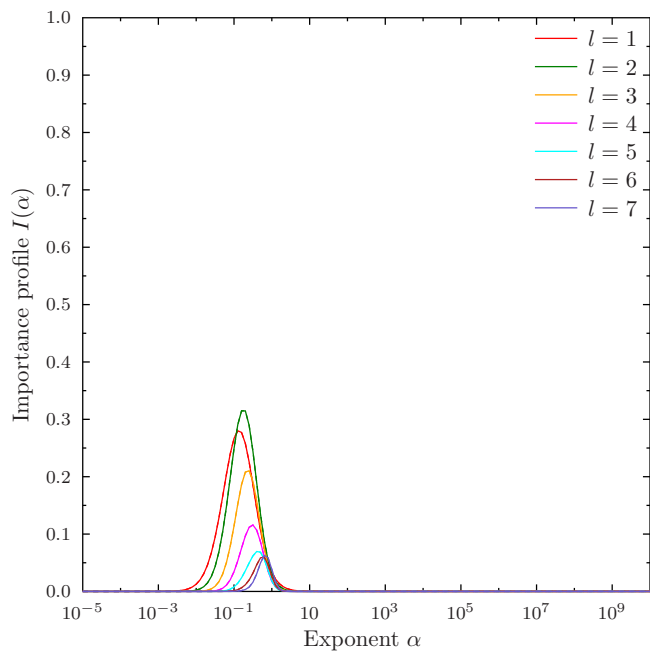

Figure 19. GTO importance profile for  $\pi_-$  orbitals on H atom in HCl.

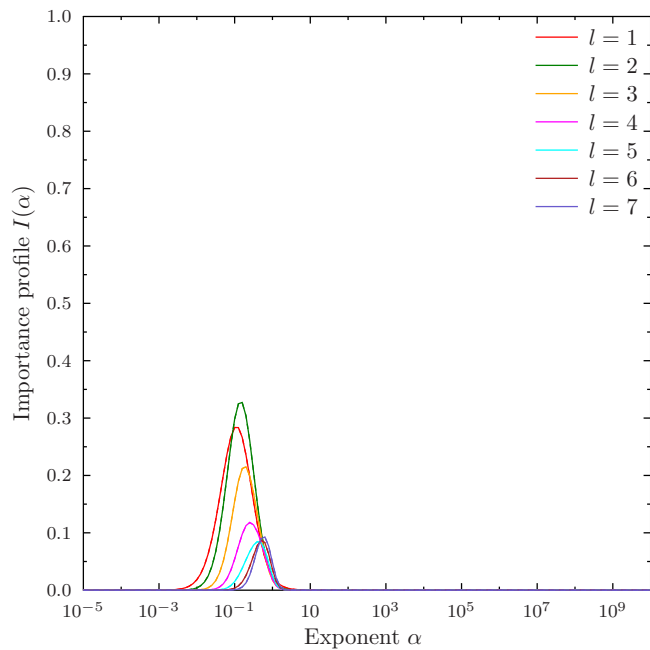

Figure 18. GTO importance profile for  $\pi_-$  orbitals on H atom in HBr.

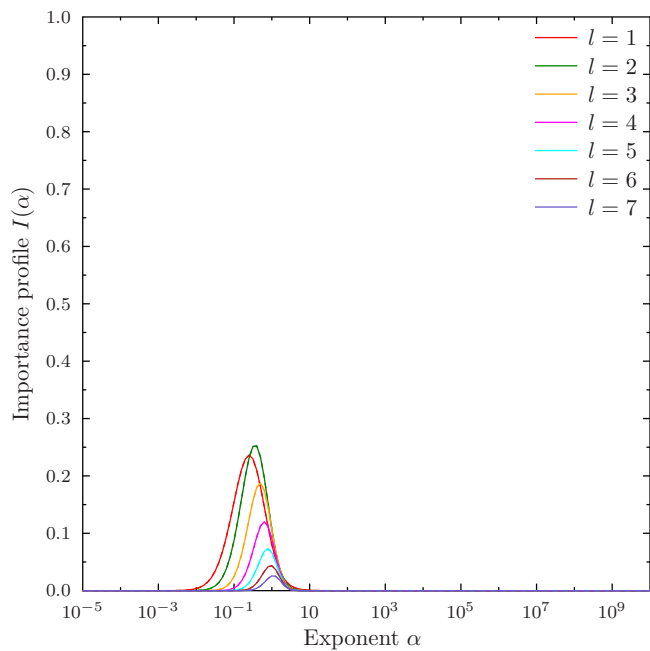

Figure 20. GTO importance profile for  $\pi_-$  orbitals on H atom in HF.

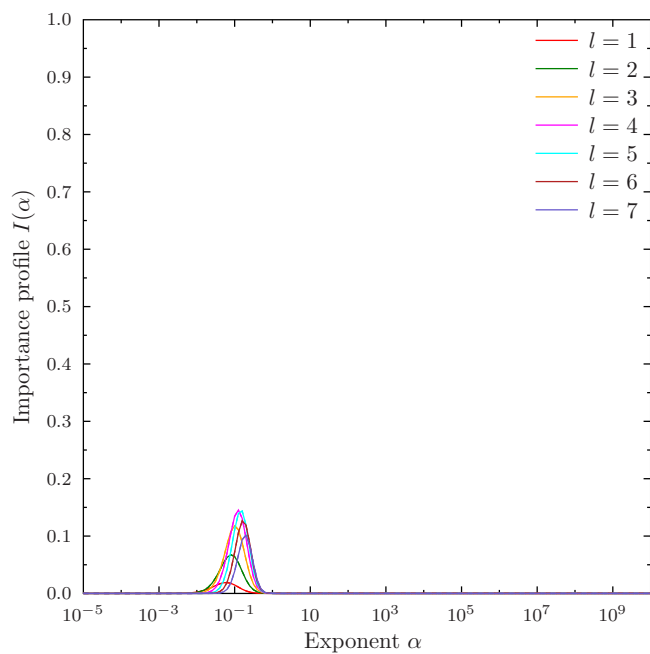

Figure 21. GTO importance profile for  $\pi_-$  orbitals on H atom in KH.

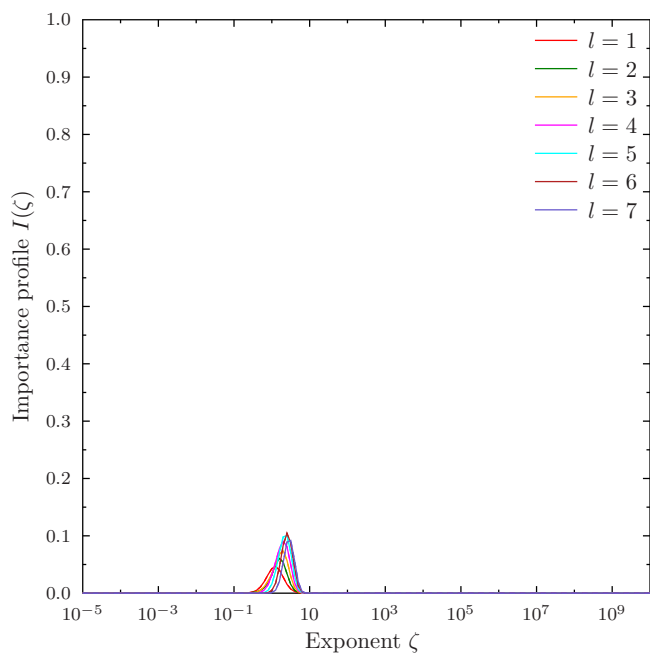

Figure 23. STO importance profile for  $\pi_-$  orbitals on H atom in CuH.

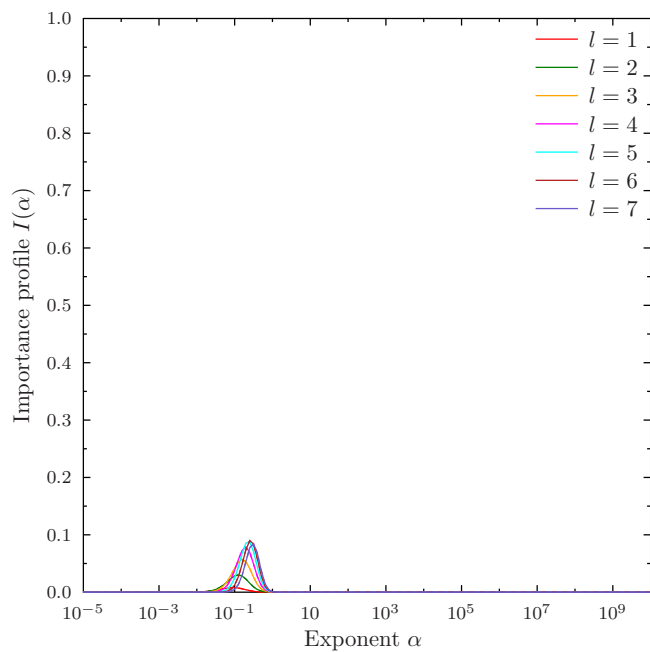

Figure 22. GTO importance profile for  $\pi_-$  orbitals on H atom in NaH.

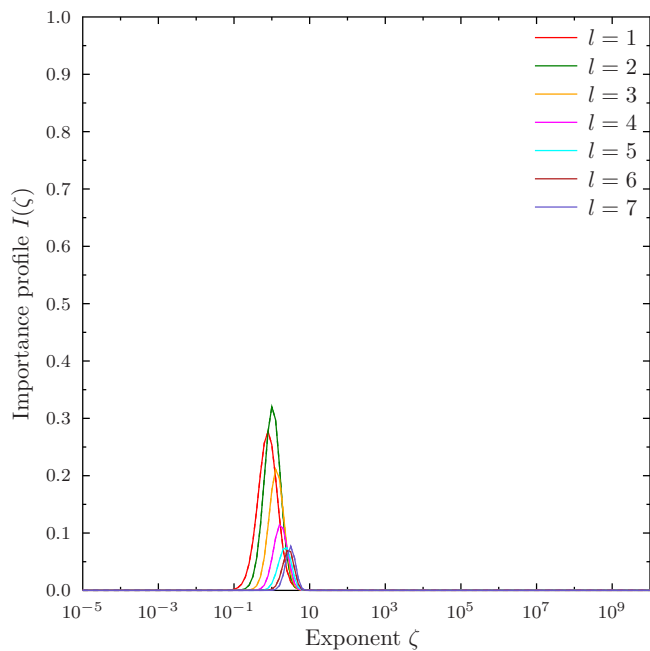

Figure 24. STO importance profile for  $\pi_-$  orbitals on H atom in HBr.

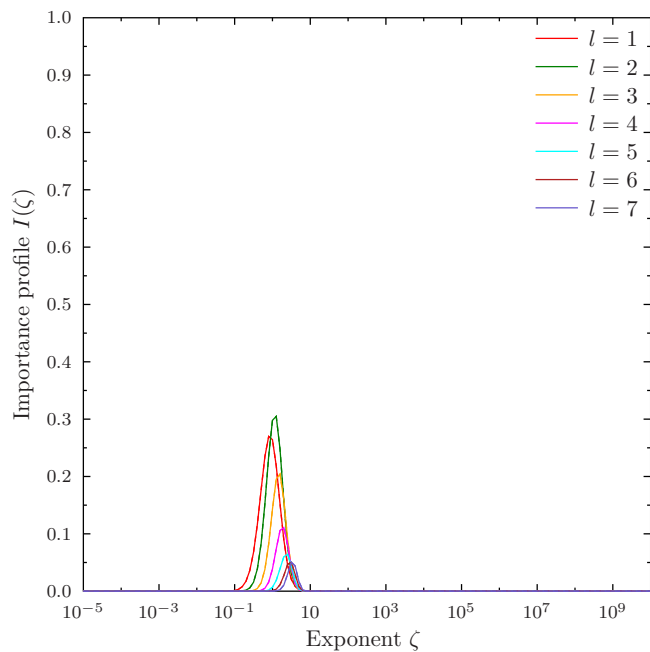

Figure 25. STO importance profile for  $\pi_-$  orbitals on H atom in HCl.

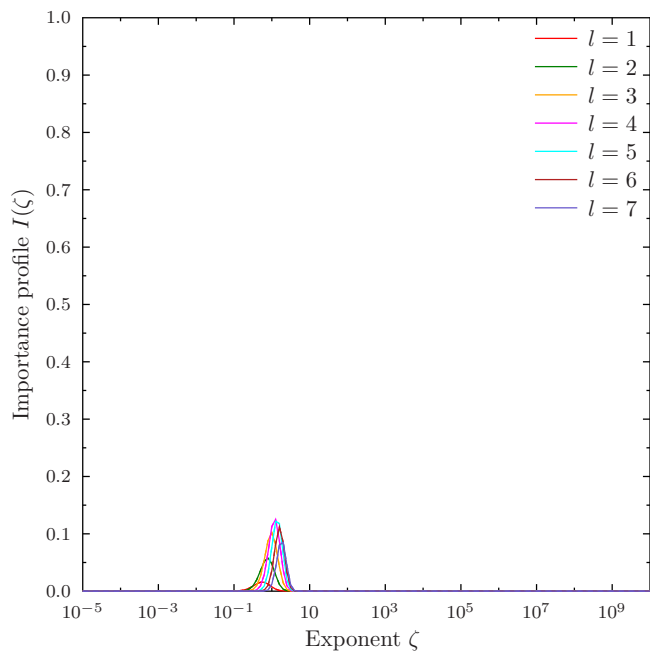

Figure 27. STO importance profile for  $\pi_-$  orbitals on H atom in KH.

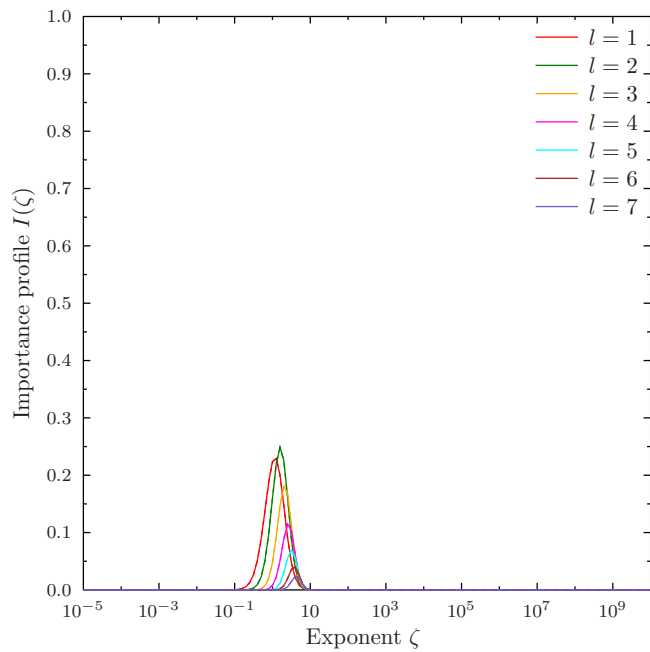

Figure 26. STO importance profile for  $\pi_-$  orbitals on H atom in HF.

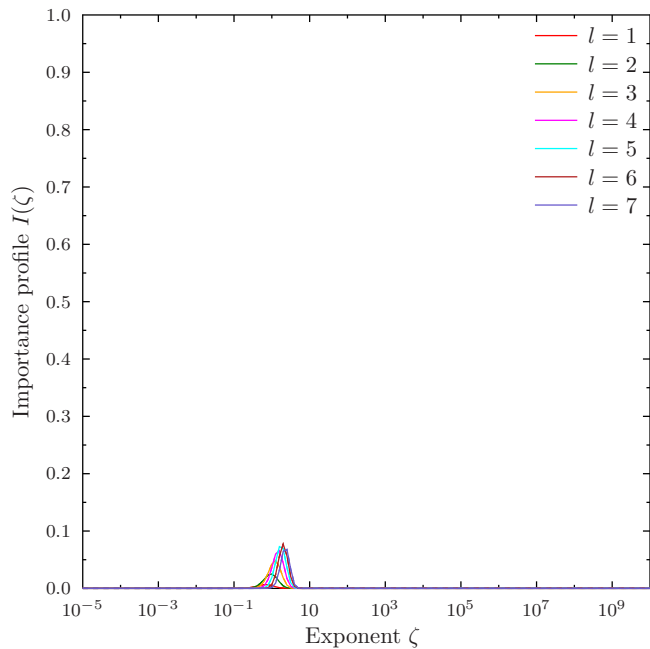

Figure 28. STO importance profile for  $\pi_-$  orbitals on H atom in NaH.

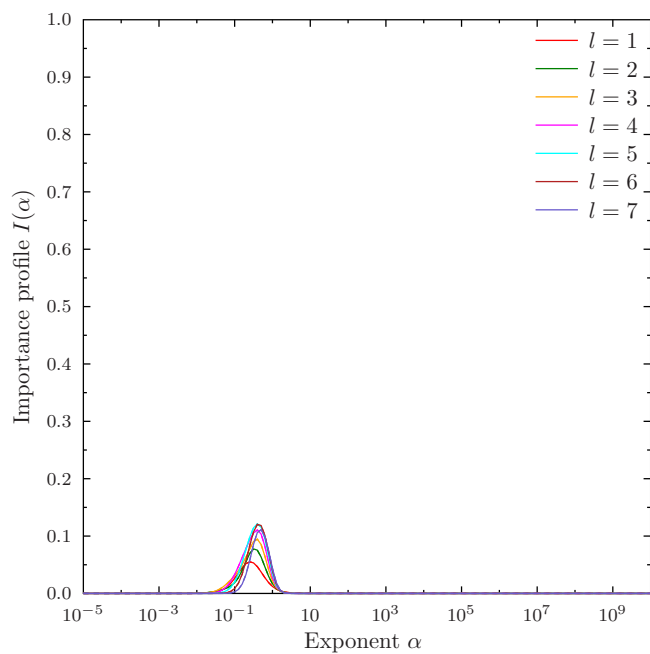

Figure 29. GTO importance profile for  $\pi_+$  orbitals on H atom in CuH.

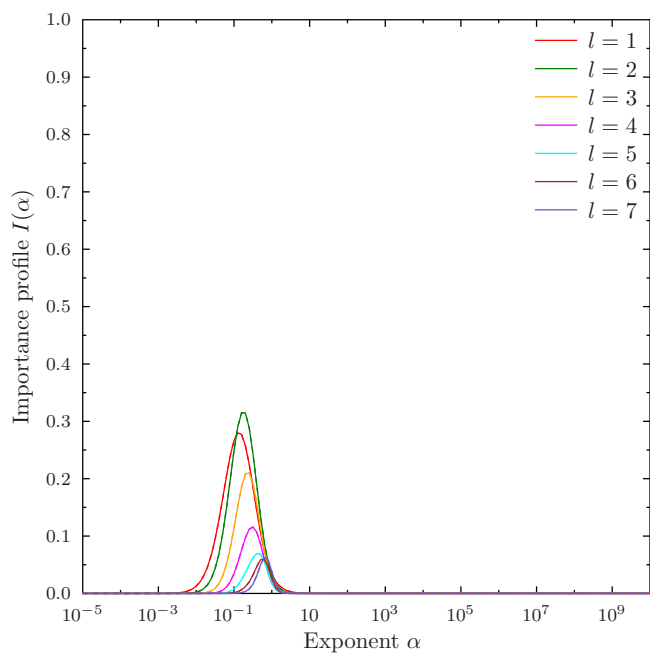

Figure 31. GTO importance profile for  $\pi_+$  orbitals on H atom in HCl.

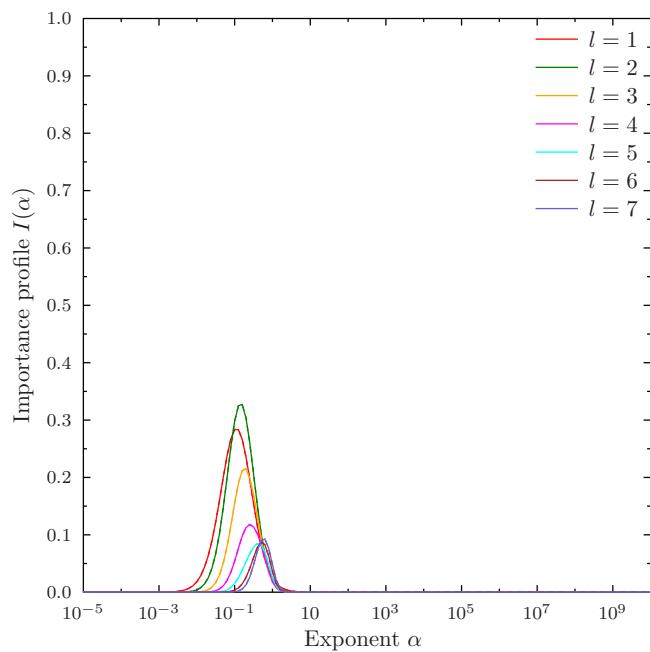

Figure 30. GTO importance profile for  $\pi_+$  orbitals on H atom in HBr.

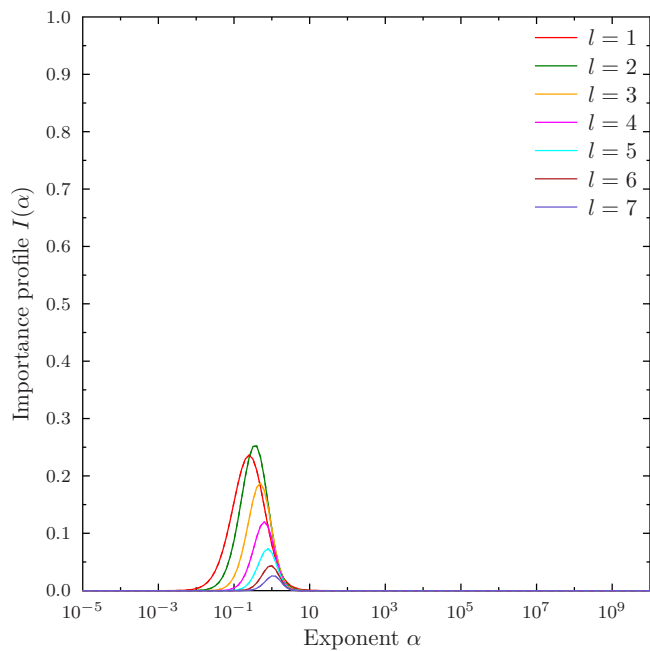

Figure 32. GTO importance profile for  $\pi_+$  orbitals on H atom in HF.

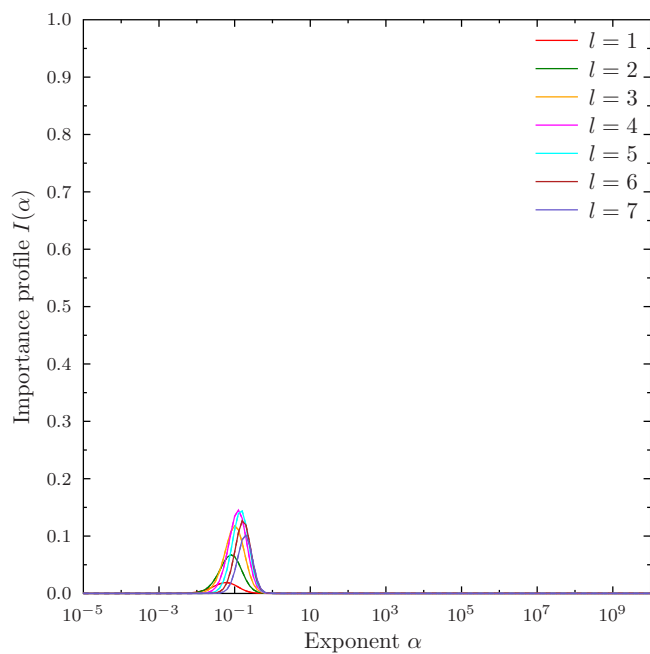

Figure 33. GTO importance profile for  $\pi_+$  orbitals on H atom in KH.

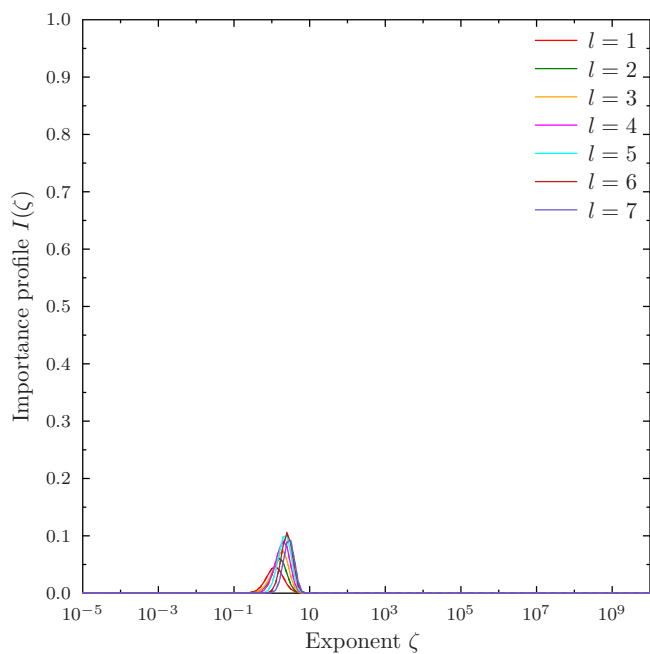

Figure 35. STO importance profile for  $\pi_+$  orbitals on H atom in CuH.

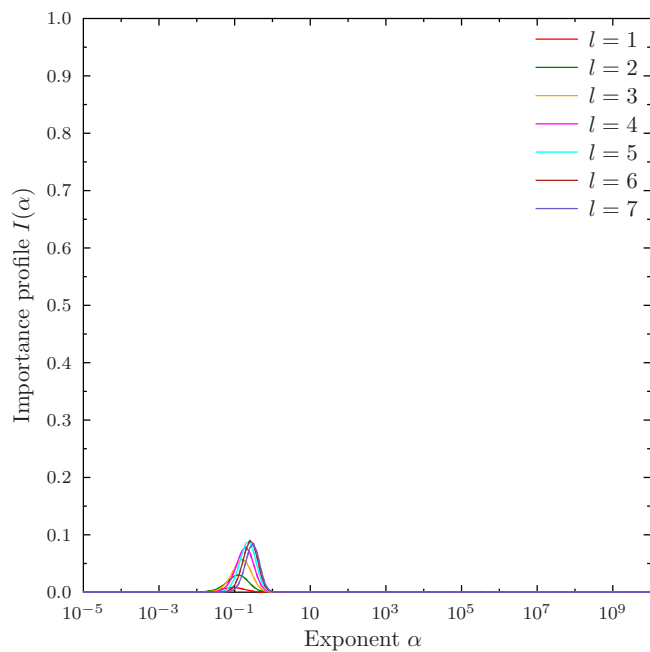

Figure 34. GTO importance profile for  $\pi_+$  orbitals on H atom in NaH.

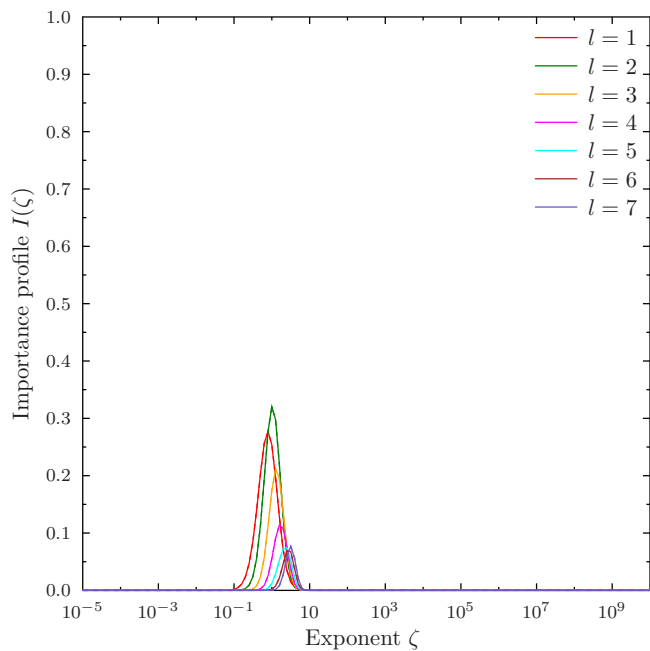

Figure 36. STO importance profile for  $\pi_+$  orbitals on H atom in HBr.

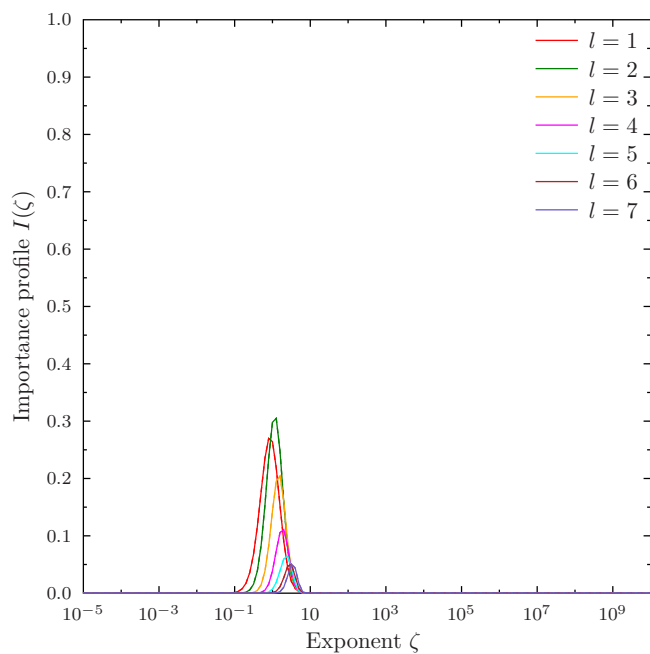

Figure 37. STO importance profile for  $\pi_+$  orbitals on H atom in HCl.

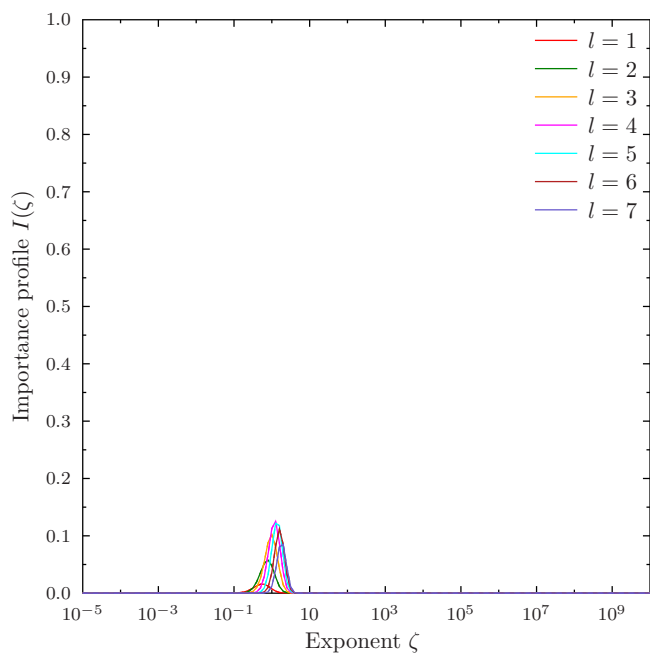

Figure 39. STO importance profile for  $\pi_+$  orbitals on H atom in KH.

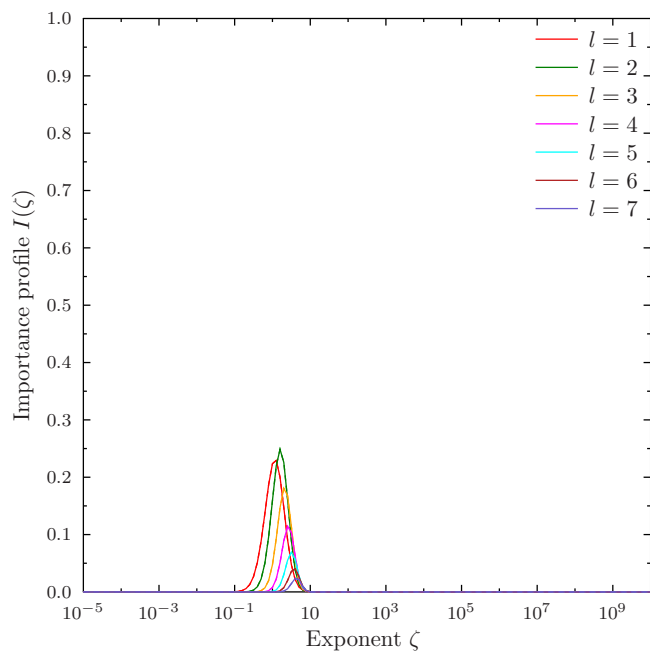

Figure 38. STO importance profile for  $\pi_+$  orbitals on H atom in HF.

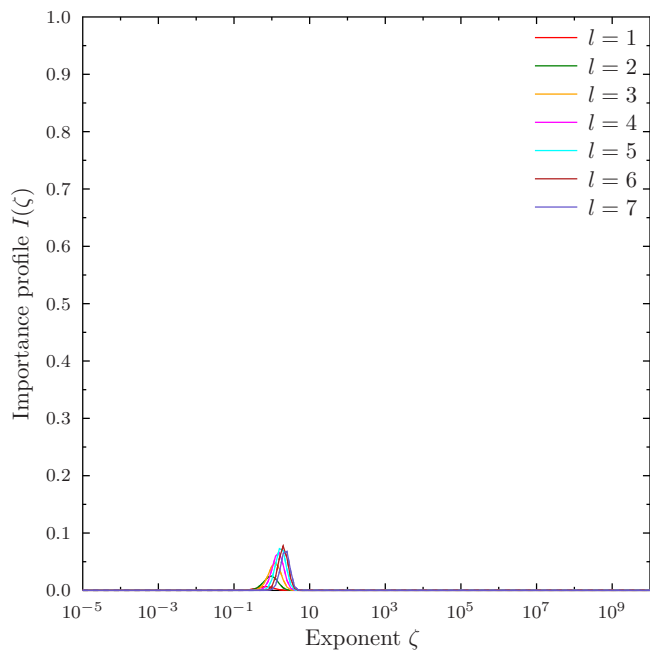

Figure 40. STO importance profile for  $\pi_+$  orbitals on H atom in NaH.

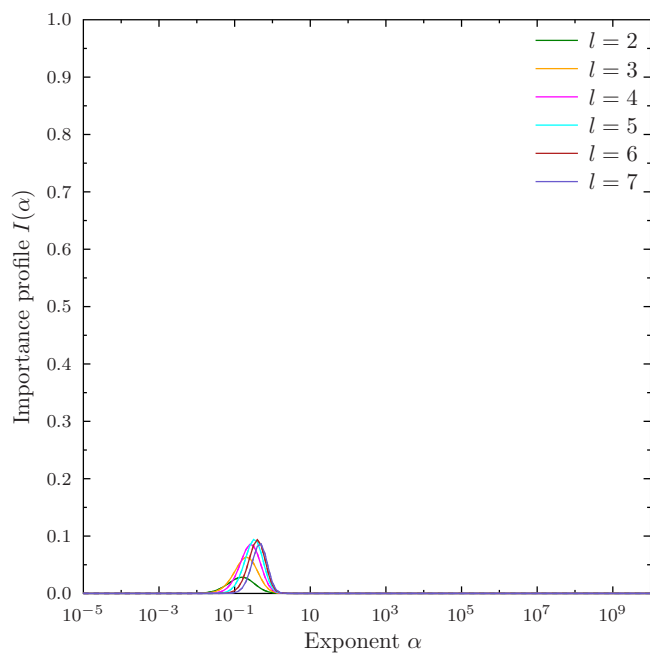

Figure 41. GTO importance profile for  $\delta_-$  orbitals on H atom in CuH.

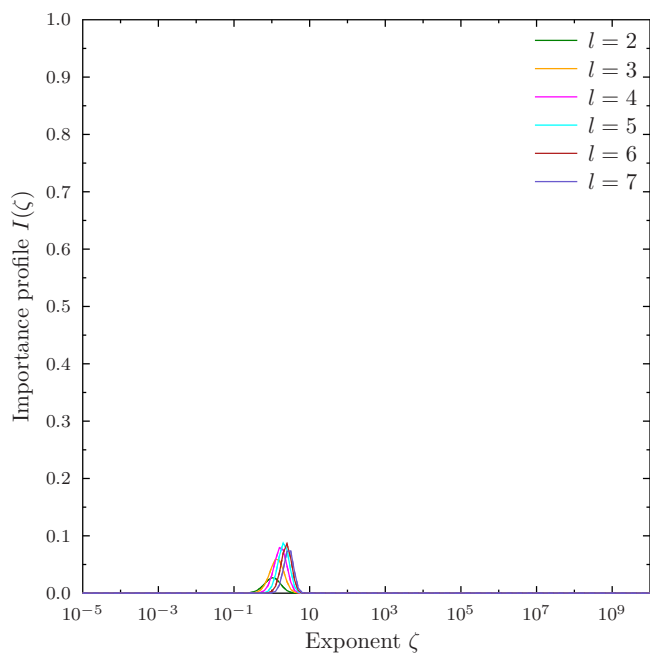

Figure 43. STO importance profile for  $\delta_-$  orbitals on H atom in CuH.

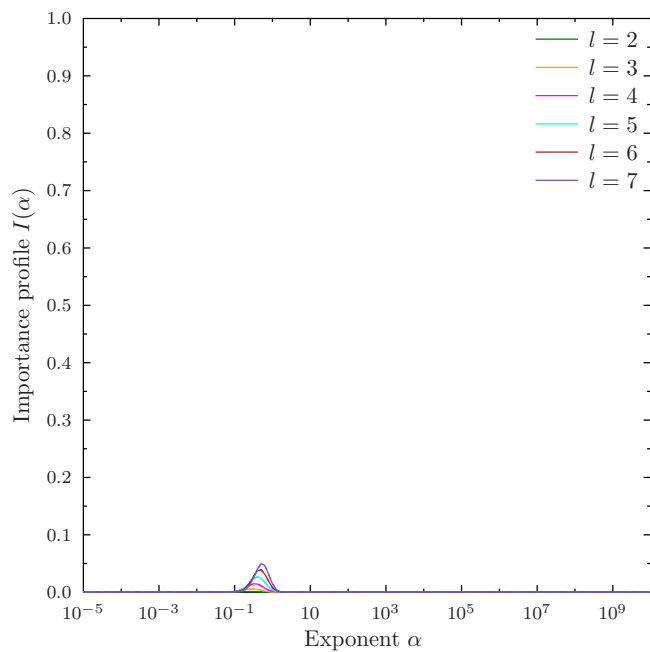

Figure 42. GTO importance profile for  $\delta_-$  orbitals on H atom in HBr.

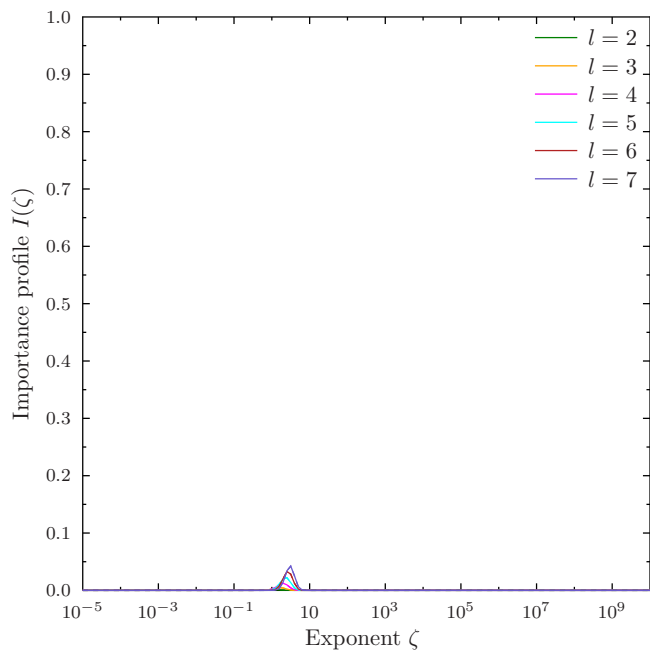

Figure 44. STO importance profile for  $\delta_-$  orbitals on H atom in HBr.

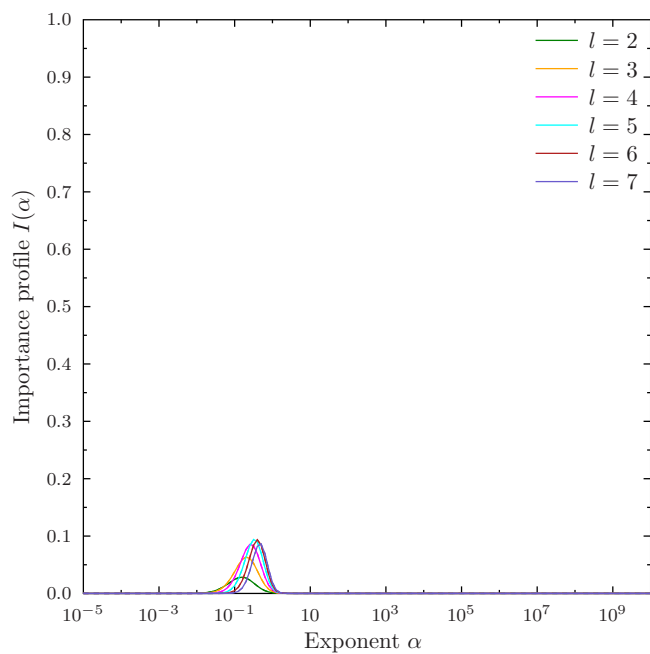

Figure 45. GTO importance profile for  $\delta_+$  orbitals on H atom in CuH.

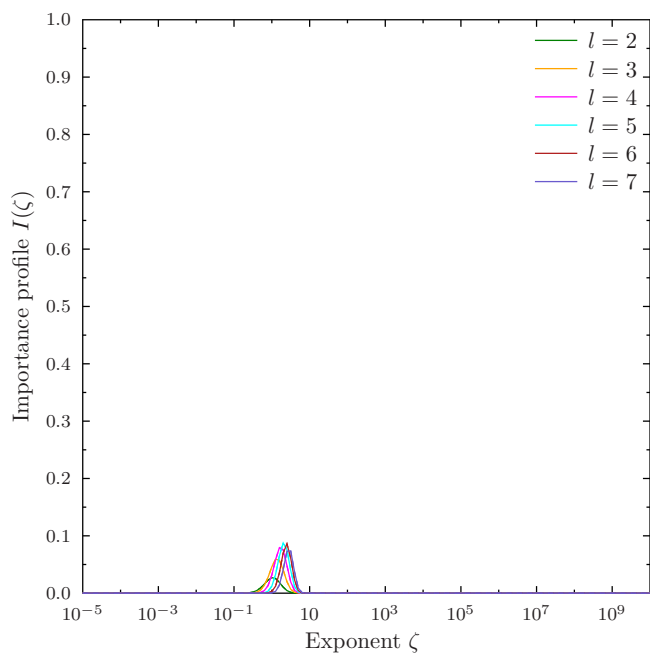

Figure 47. STO importance profile for  $\delta_+$  orbitals on H atom in CuH.

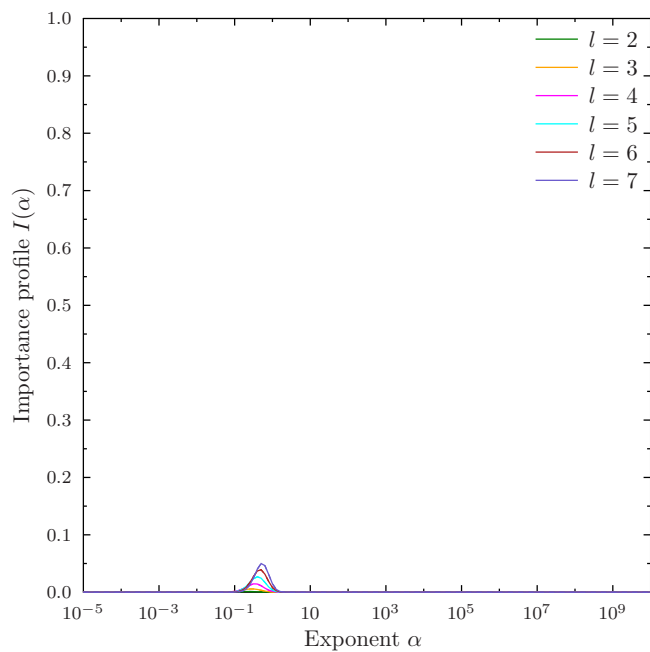

Figure 46. GTO importance profile for  $\delta_+$  orbitals on H atom in HBr.

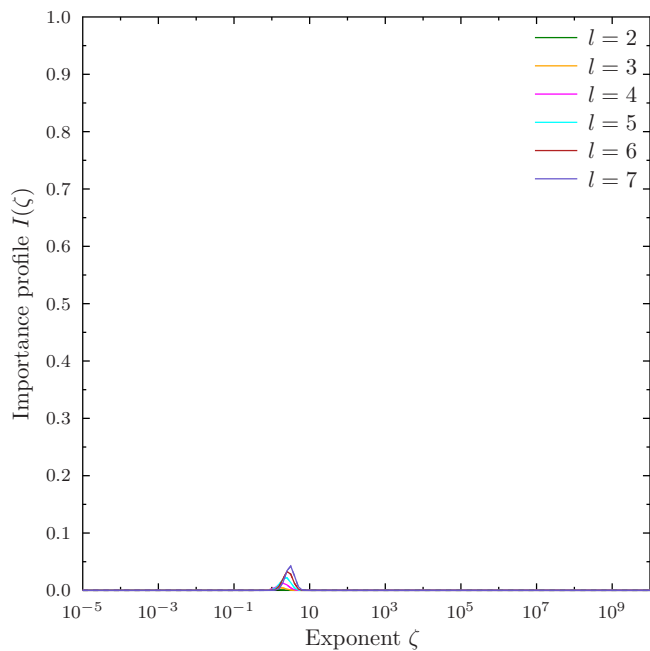

Figure 48. STO importance profile for  $\delta_+$  orbitals on H atom in HBr.



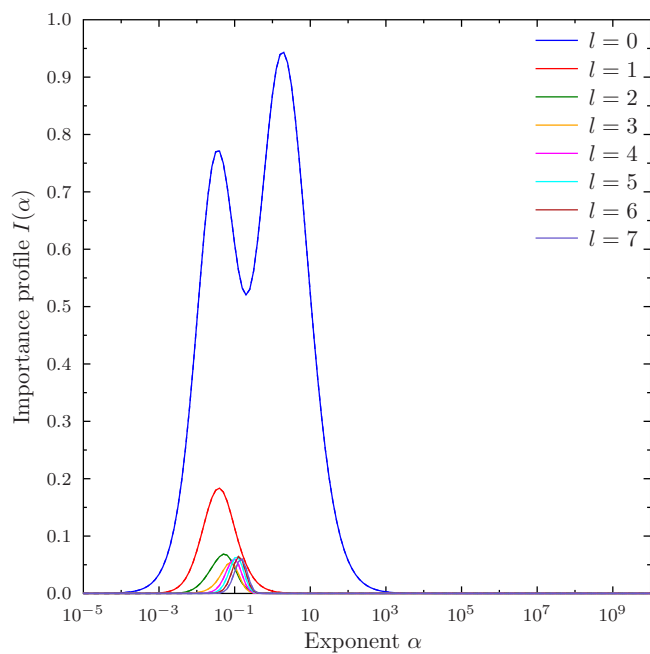

Figure 49. GTO importance profile for  $\sigma$  orbitals on Li atom in  $\text{Li}_2$ .

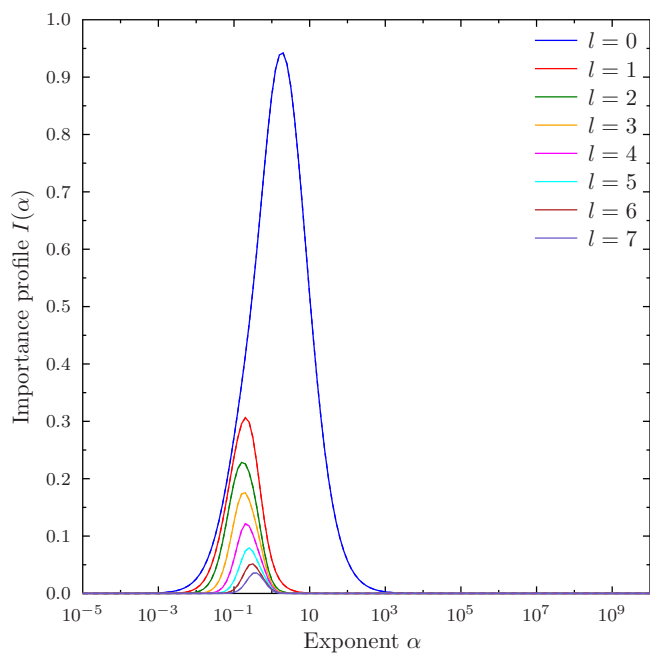

Figure 51. GTO importance profile for  $\sigma$  orbitals on Li atom in  $\text{LiF}$ .

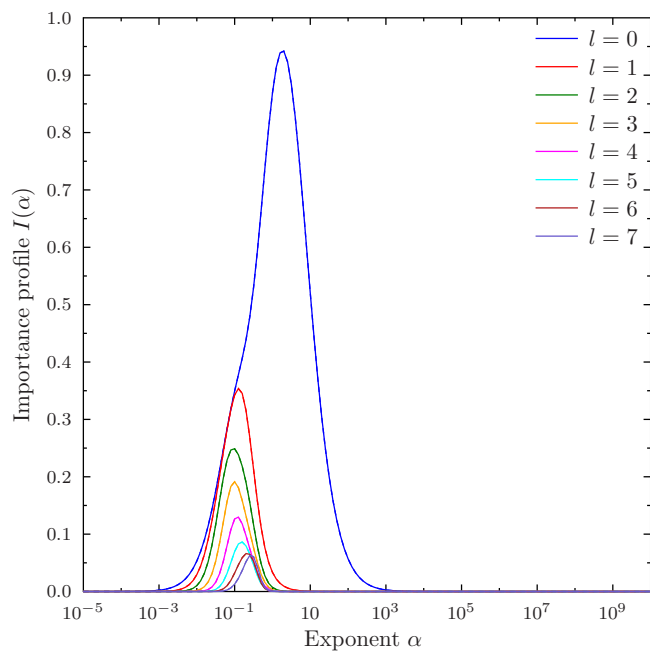

Figure 50. GTO importance profile for  $\sigma$  orbitals on Li atom in  $\text{LiCl}$ .

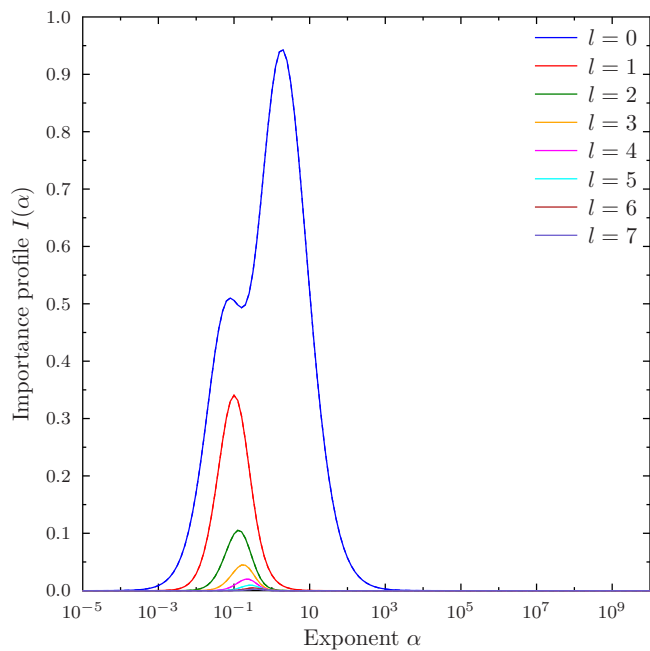

Figure 52. GTO importance profile for  $\sigma$  orbitals on Li atom in  $\text{LiH}$ .

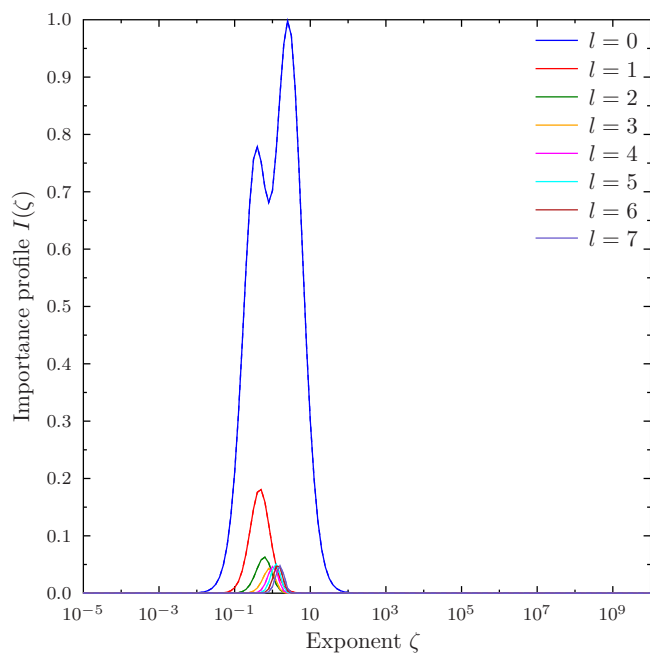

Figure 53. STO importance profile for  $\sigma$  orbitals on Li atom in  $\text{Li}_2$ .

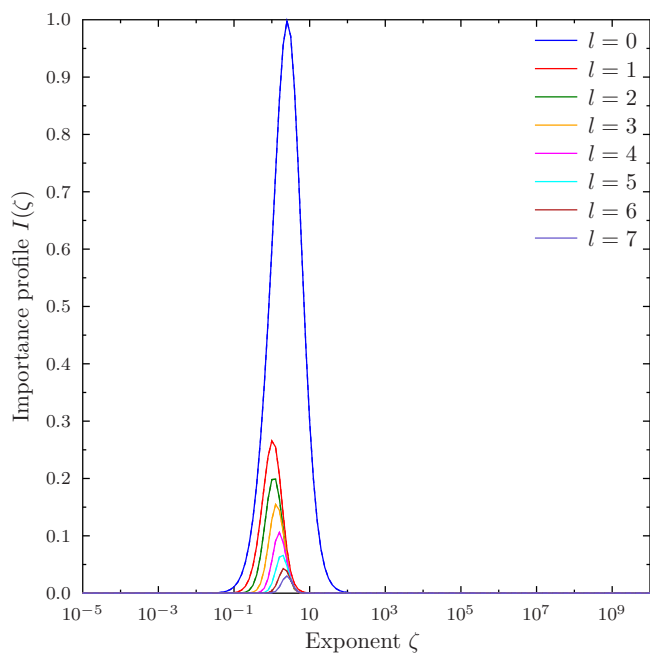

Figure 55. STO importance profile for  $\sigma$  orbitals on Li atom in  $\text{LiF}$ .

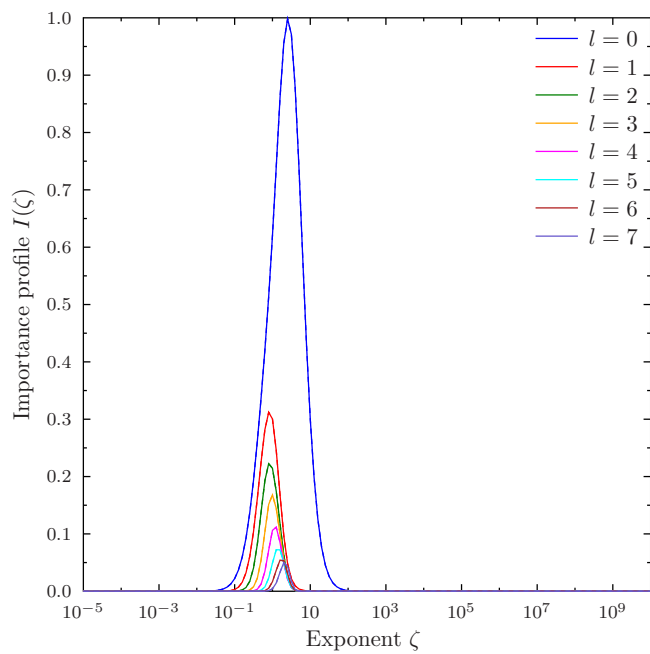

Figure 54. STO importance profile for  $\sigma$  orbitals on Li atom in  $\text{LiCl}$ .

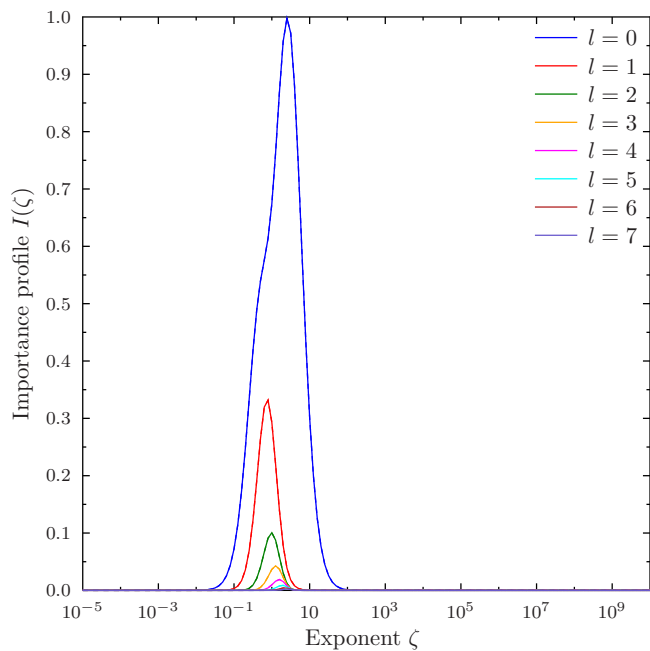

Figure 56. STO importance profile for  $\sigma$  orbitals on Li atom in  $\text{LiH}$ .

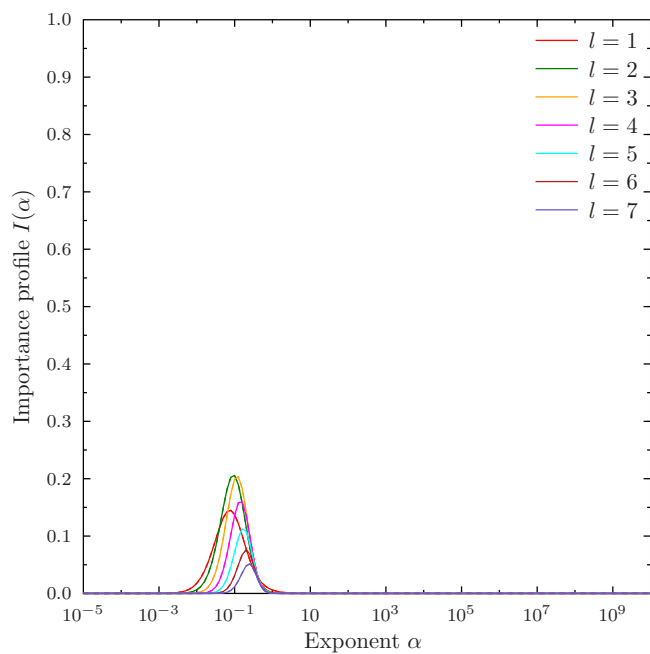

Figure 57. GTO importance profile for  $\pi_-$  orbitals on Li atom in LiCl.

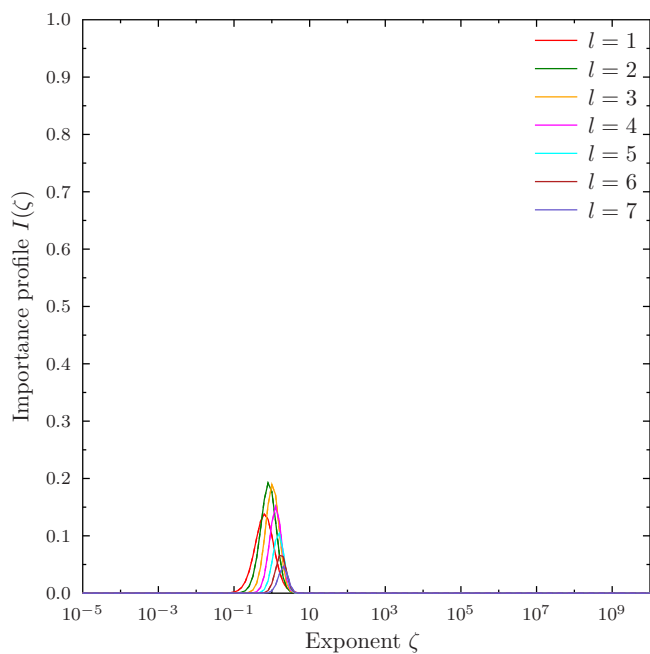

Figure 59. STO importance profile for  $\pi_-$  orbitals on Li atom in LiCl.

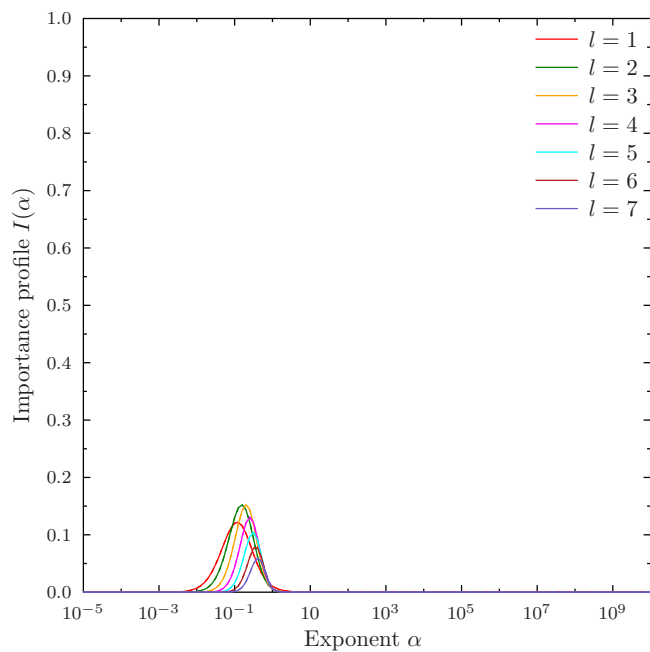

Figure 58. GTO importance profile for  $\pi_-$  orbitals on Li atom in LiF.

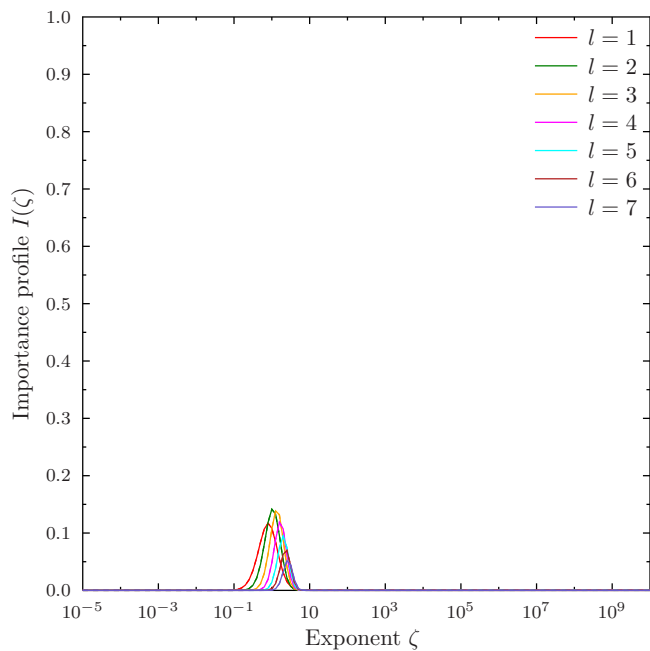

Figure 60. STO importance profile for  $\pi_-$  orbitals on Li atom in LiF.

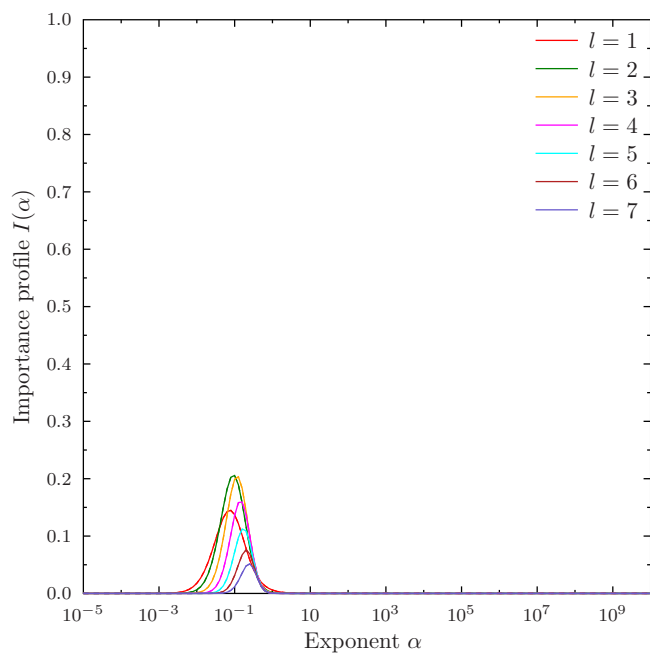

Figure 61. GTO importance profile for  $\pi_+$  orbitals on Li atom in LiCl.

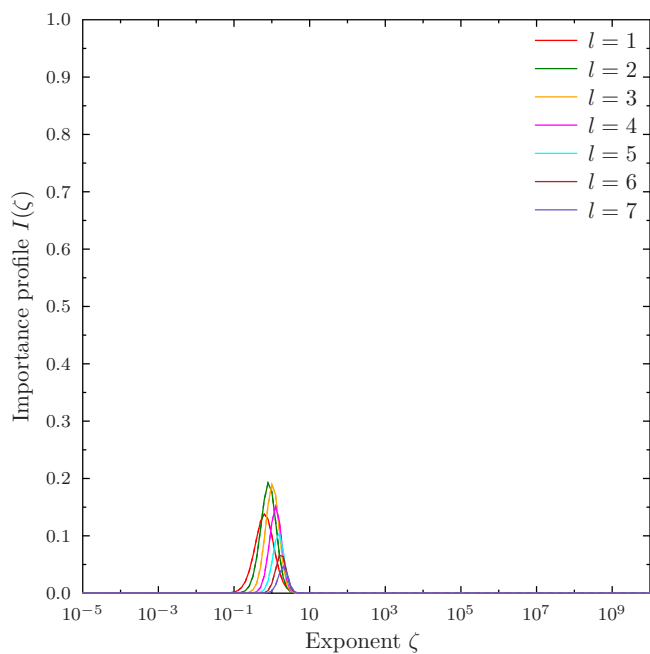

Figure 63. STO importance profile for  $\pi_+$  orbitals on Li atom in LiCl.

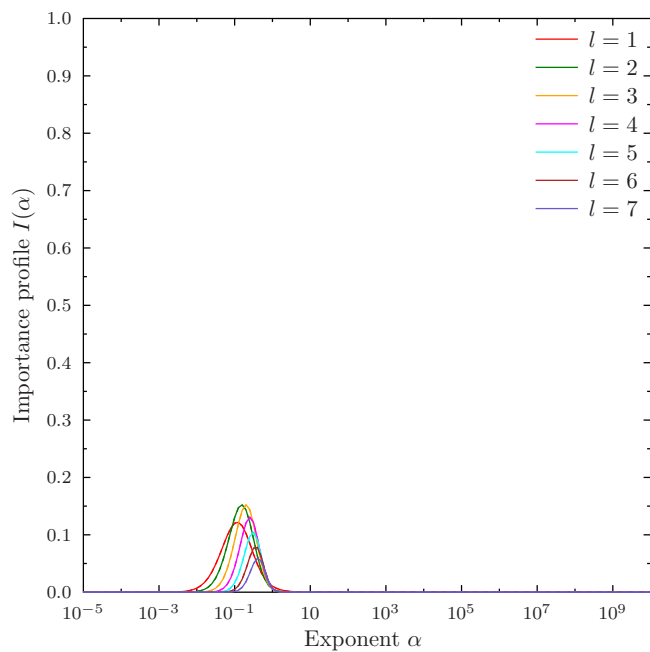

Figure 62. GTO importance profile for  $\pi_+$  orbitals on Li atom in LiF.

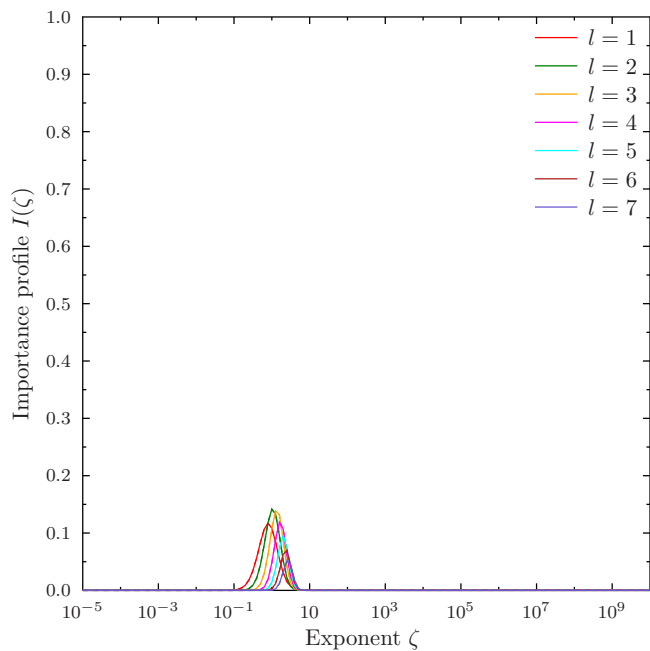

Figure 64. STO importance profile for  $\pi_+$  orbitals on Li atom in LiF.

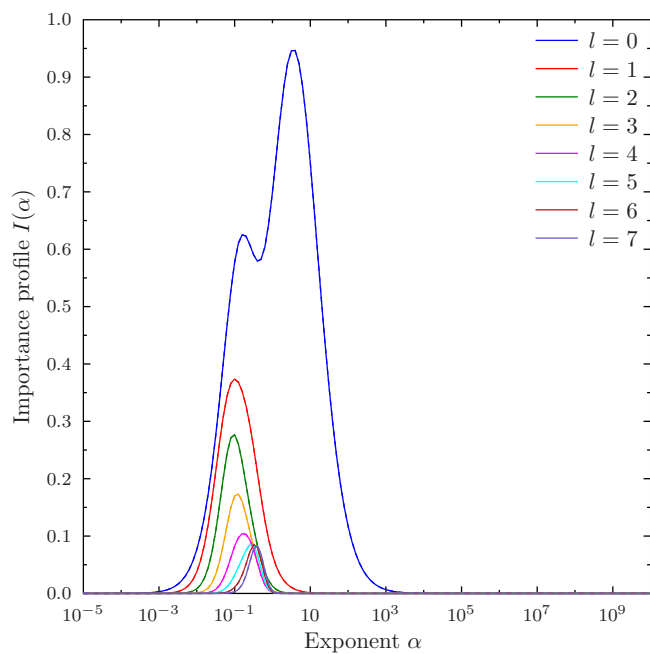

Figure 65. GTO importance profile for  $\sigma$  orbitals on Be atom in BeS.

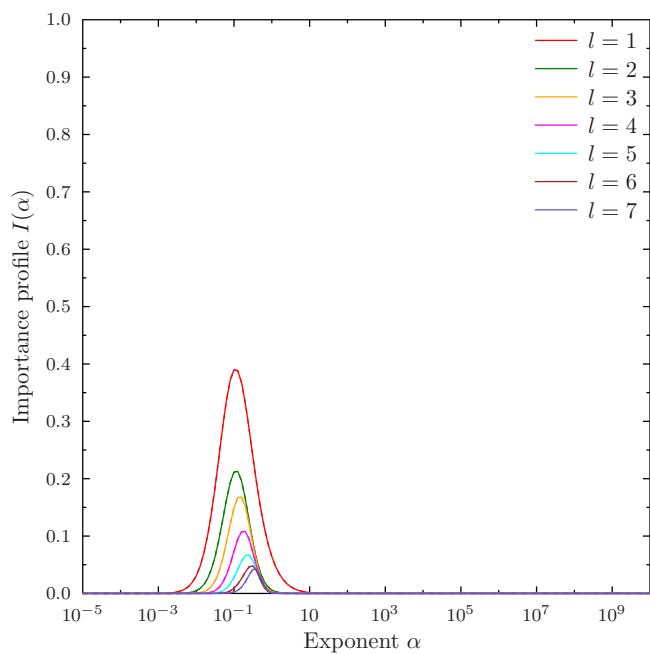

Figure 67. GTO importance profile for  $\pi_-$  orbitals on Be atom in BeS.

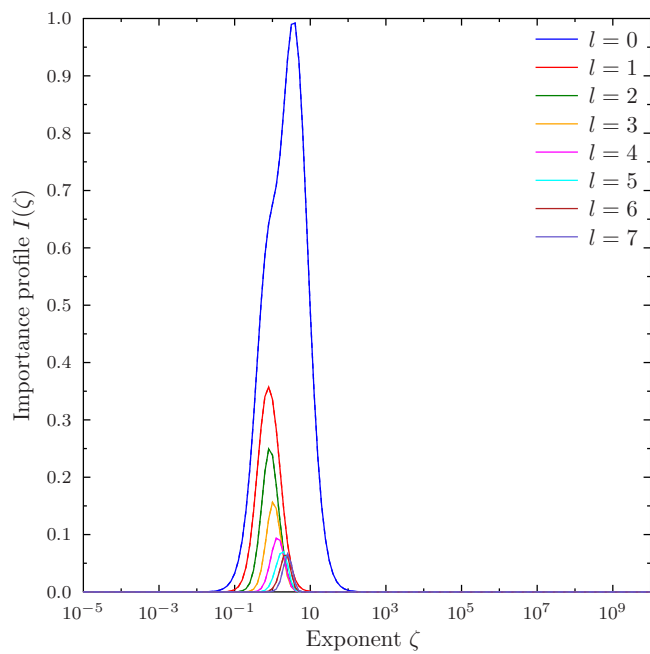

Figure 66. STO importance profile for  $\sigma$  orbitals on Be atom in BeS.

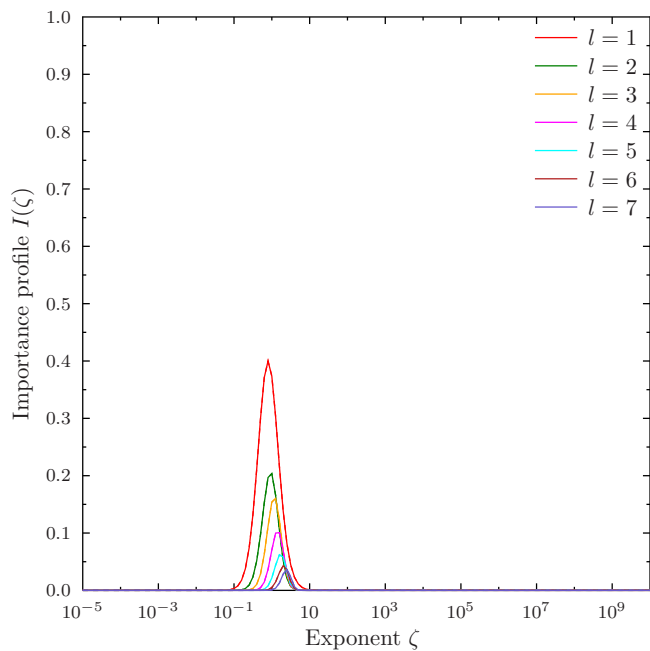

Figure 68. STO importance profile for  $\pi_-$  orbitals on Be atom in BeS.

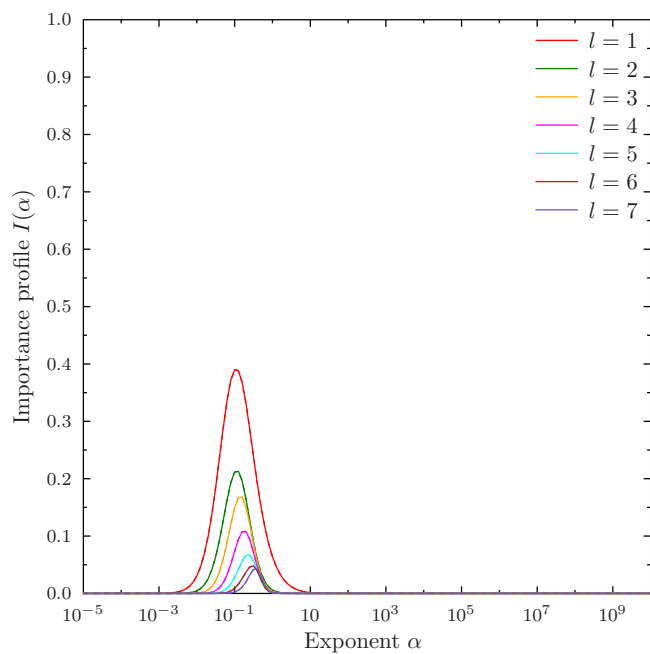

Figure 69. GTO importance profile for  $\pi_+$  orbitals on Be atom in BeS.

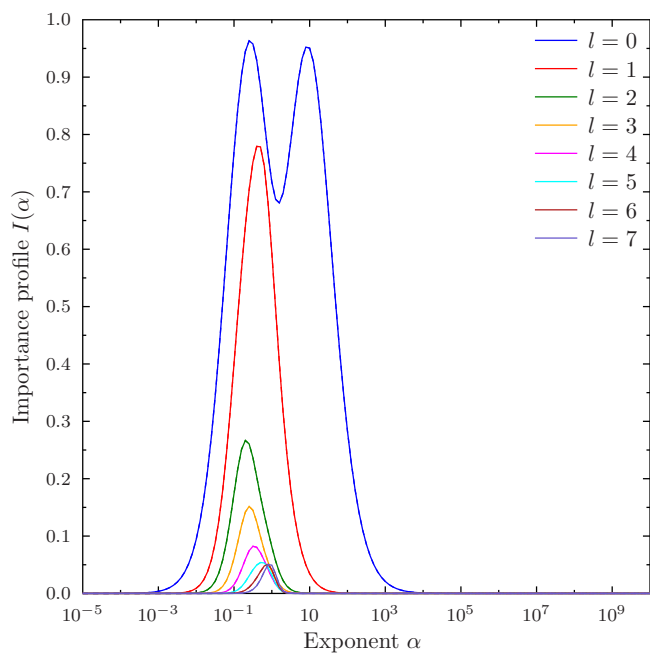

Figure 71. GTO importance profile for  $\sigma$  orbitals on C atom in CO.

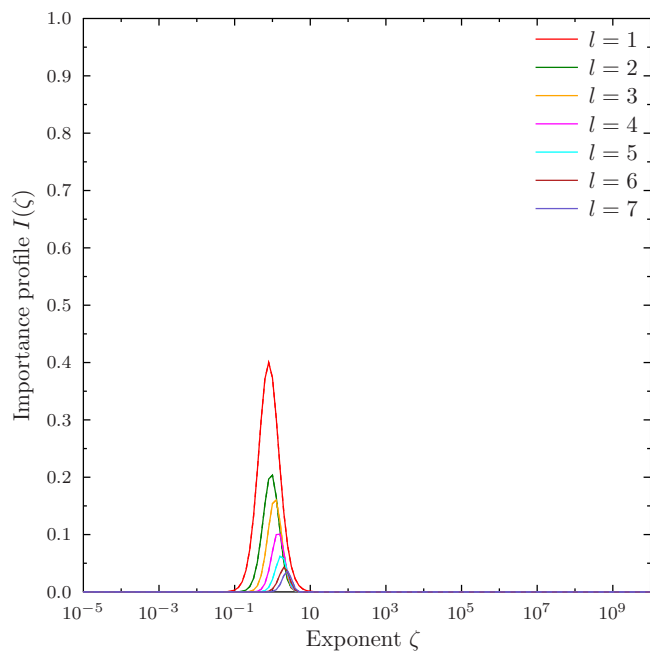

Figure 70. STO importance profile for  $\pi_+$  orbitals on Be atom in BeS.

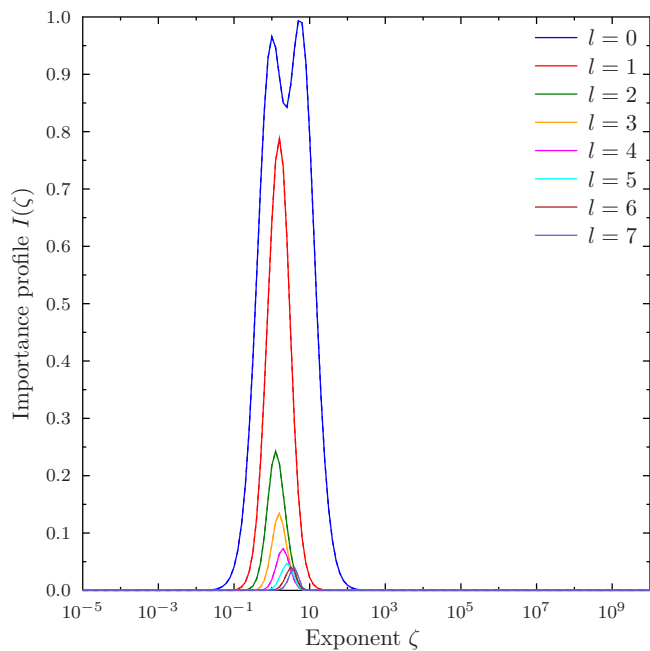

Figure 72. STO importance profile for  $\sigma$  orbitals on C atom in CO.

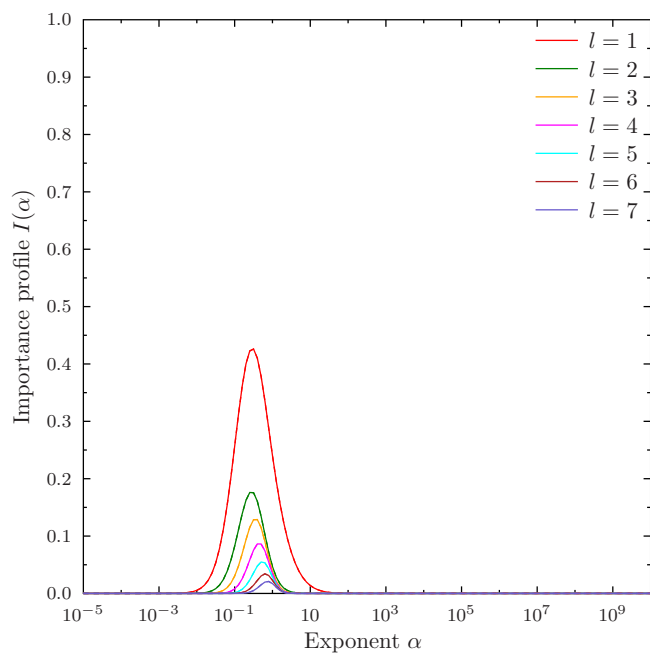

Figure 73. GTO importance profile for  $\pi_-$  orbitals on C atom in CO.

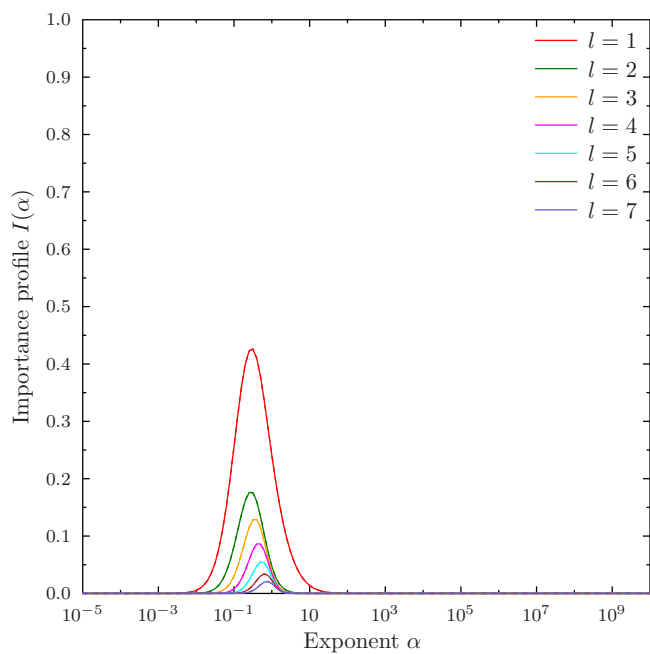

Figure 75. GTO importance profile for  $\pi_+$  orbitals on C atom in CO.

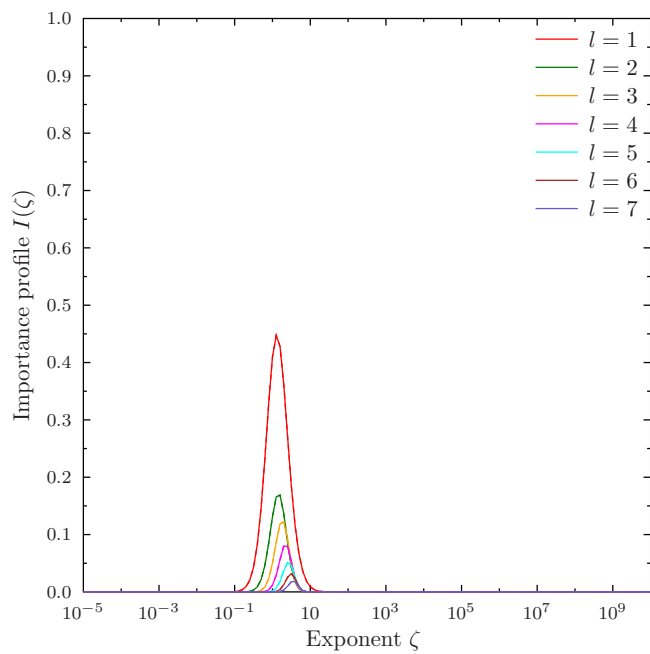

Figure 74. STO importance profile for  $\pi_-$  orbitals on C atom in CO.

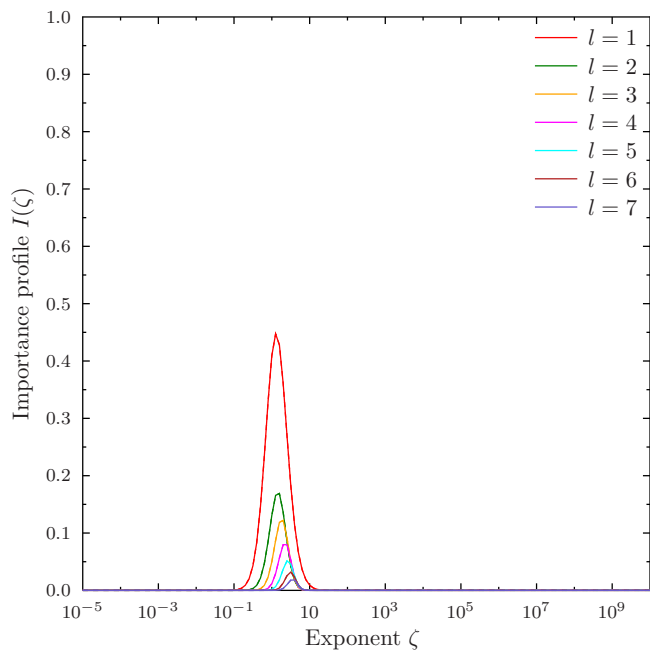

Figure 76. STO importance profile for  $\pi_+$  orbitals on C atom in CO.

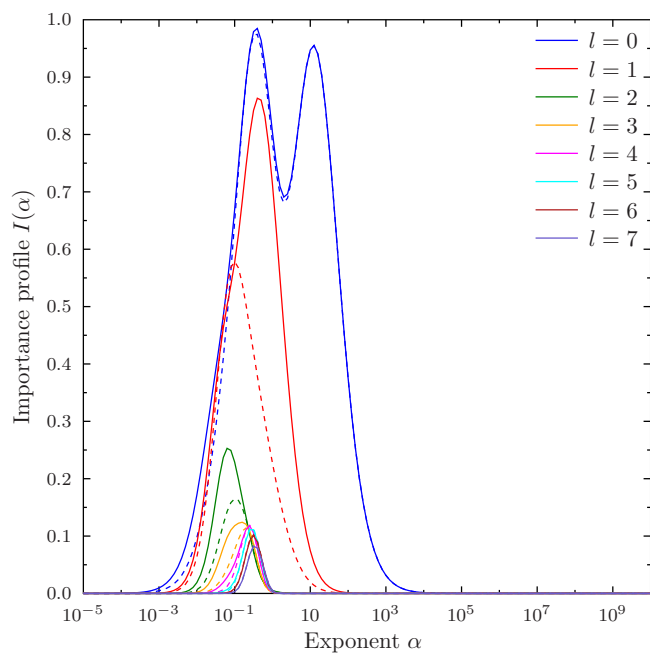

Figure 77. GTO importance profile for  $\sigma$  orbitals on N atom in AlN.

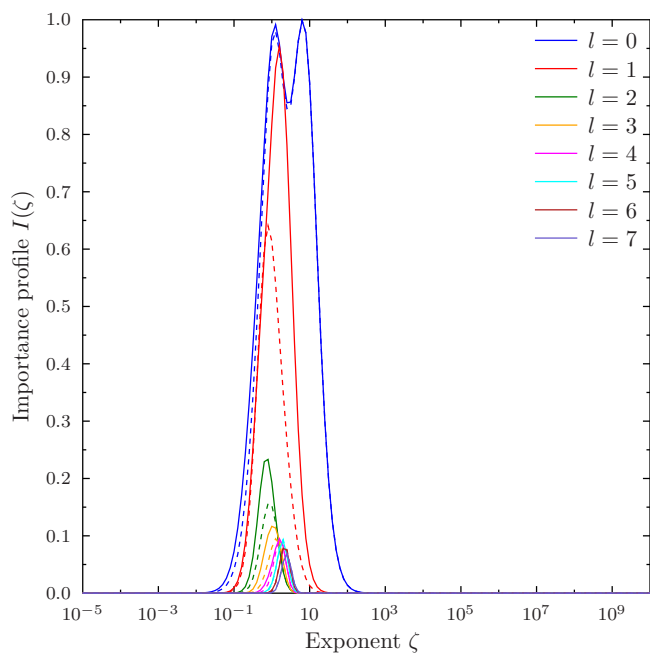

Figure 79. STO importance profile for  $\sigma$  orbitals on N atom in AlN.

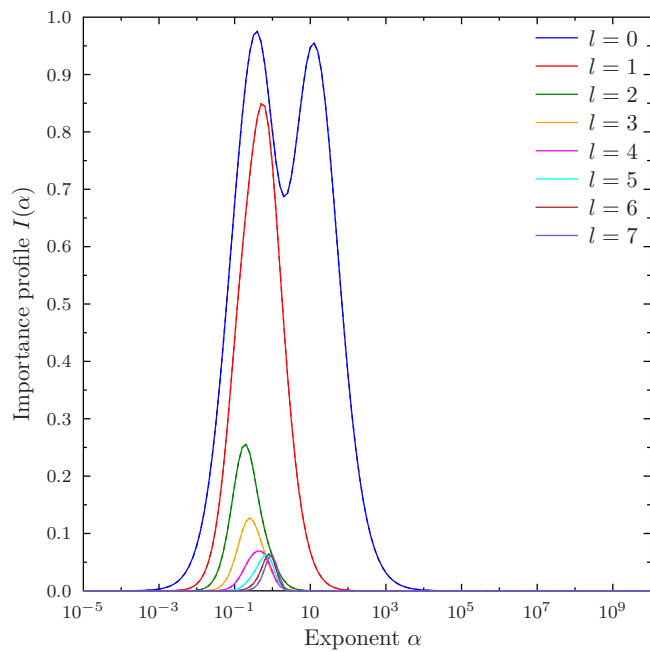

Figure 78. GTO importance profile for  $\sigma$  orbitals on N atom in  $N_2$ .

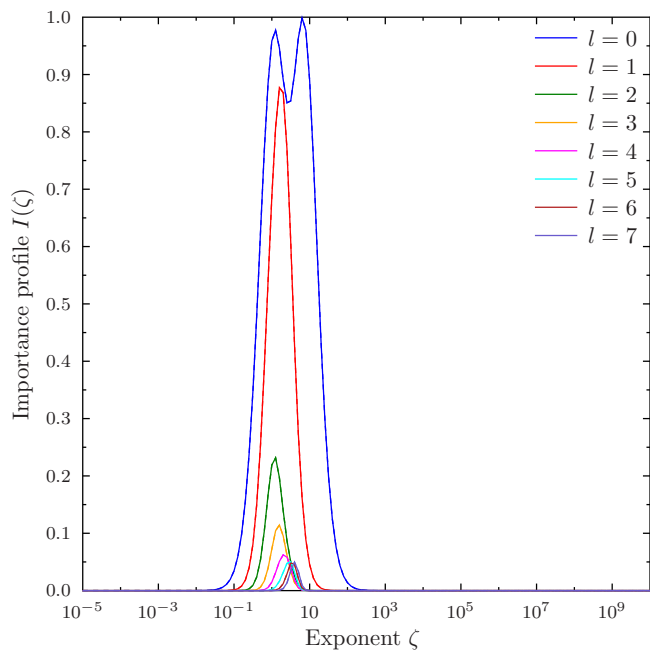

Figure 80. STO importance profile for  $\sigma$  orbitals on N atom in  $N_2$ .



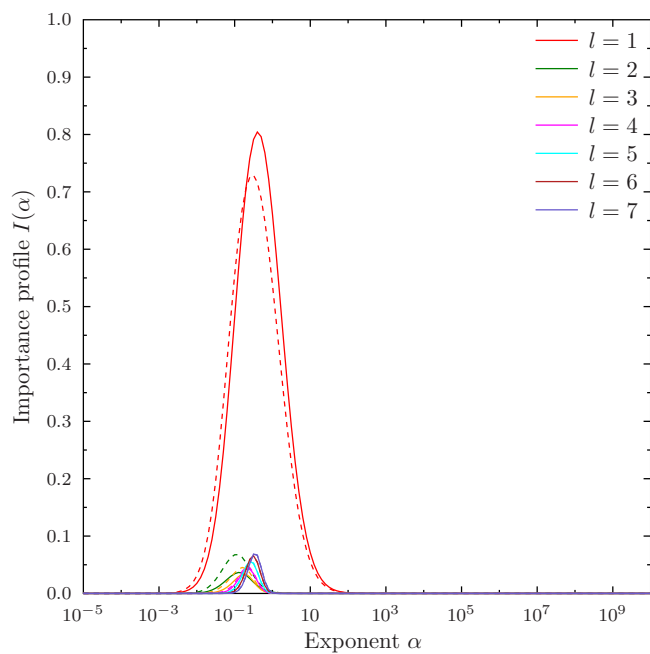

Figure 81. GTO importance profile for  $\pi_-$  orbitals on N atom in AlN.

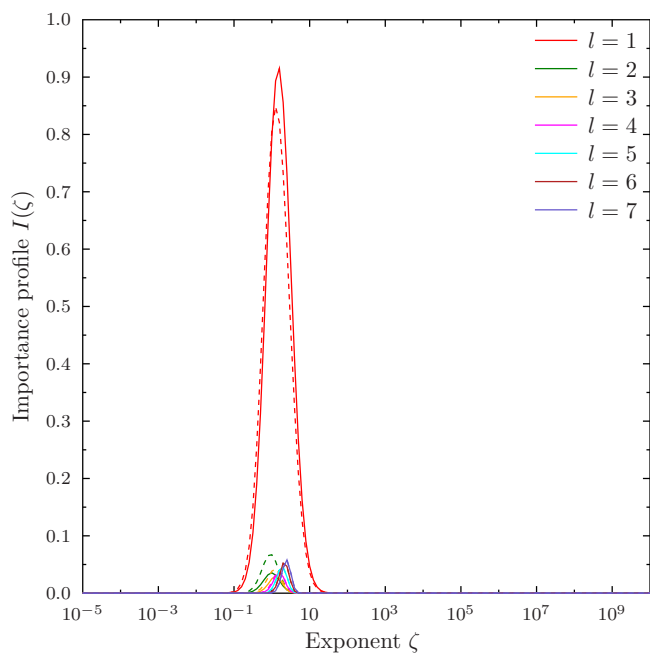

Figure 83. STO importance profile for  $\pi_-$  orbitals on N atom in AlN.

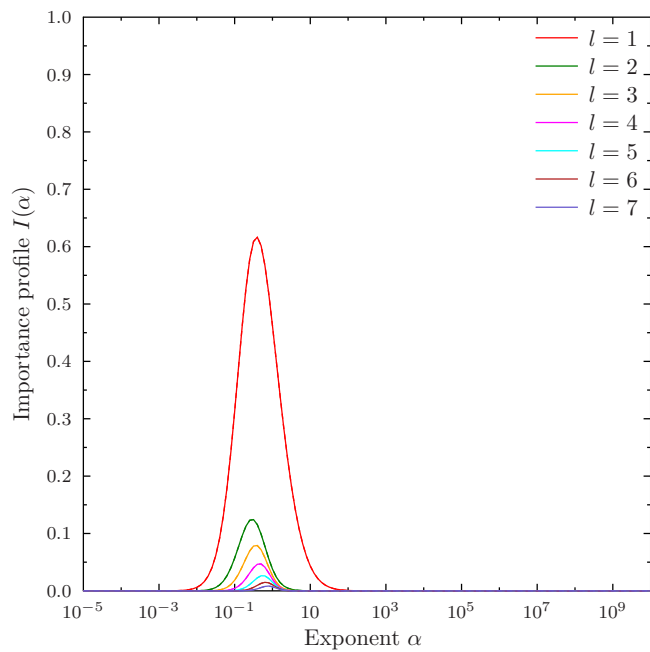

Figure 82. GTO importance profile for  $\pi_-$  orbitals on N atom in  $N_2$ .

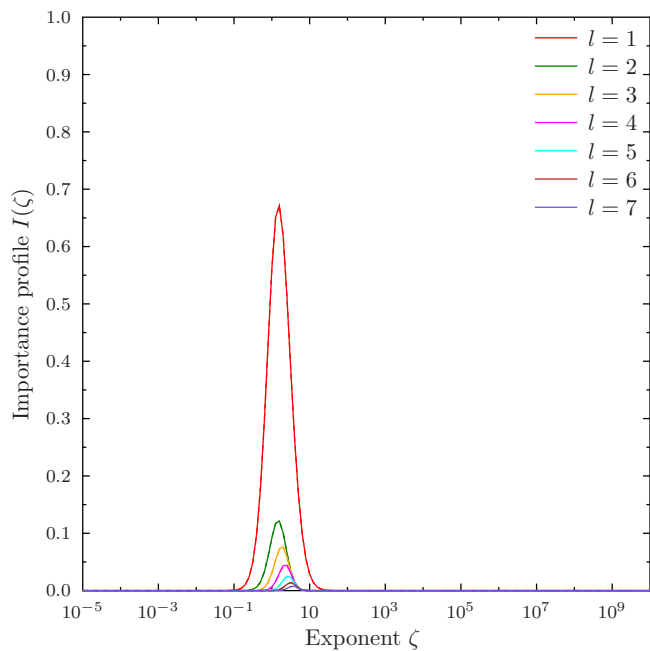

Figure 84. STO importance profile for  $\pi_-$  orbitals on N atom in  $N_2$ .

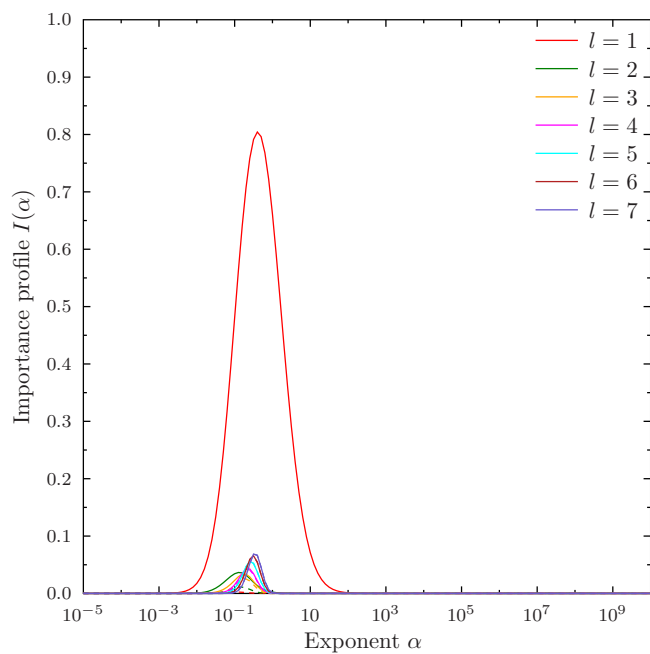

Figure 85. GTO importance profile for  $\pi_+$  orbitals on N atom in AlN.

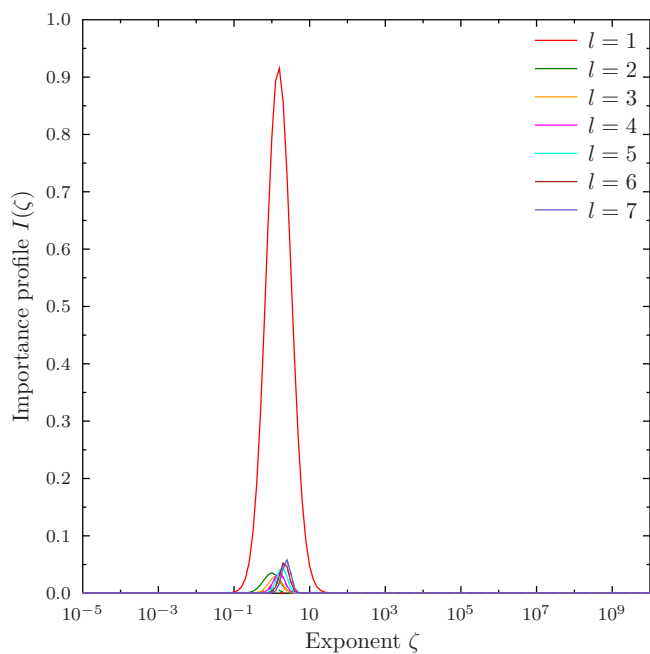

Figure 87. STO importance profile for  $\pi_+$  orbitals on N atom in AlN.

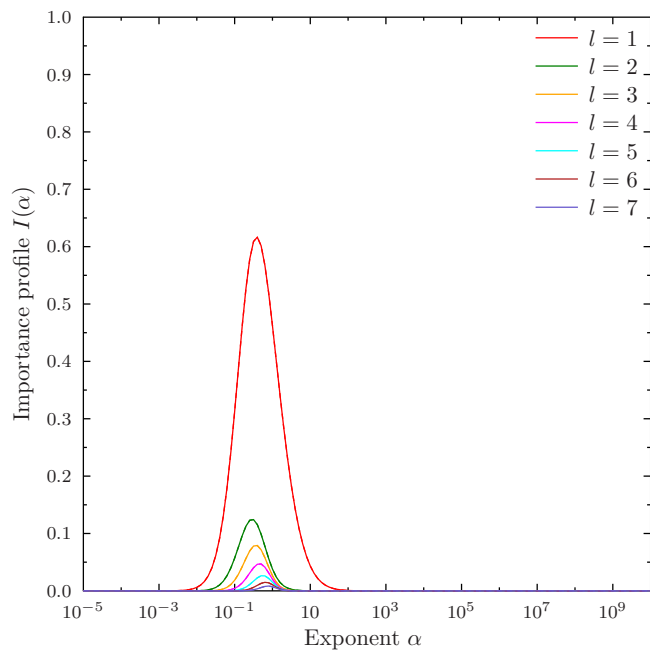

Figure 86. GTO importance profile for  $\pi_+$  orbitals on N atom in  $N_2$ .

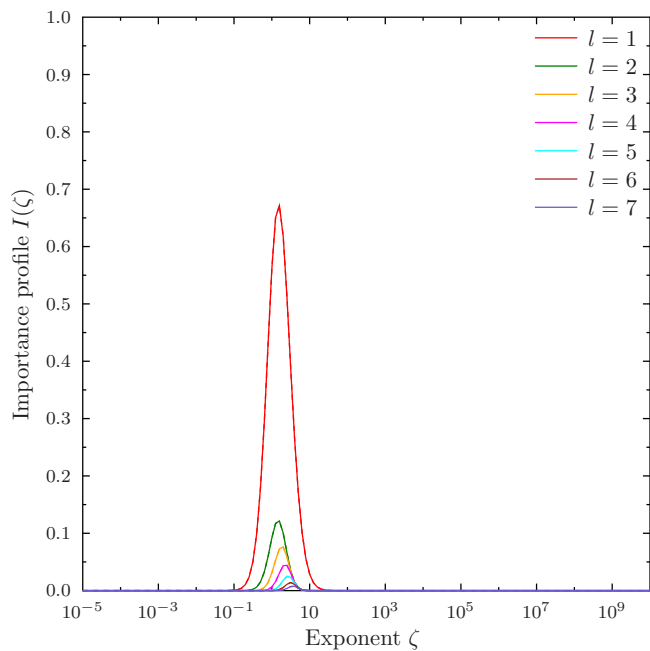

Figure 88. STO importance profile for  $\pi_+$  orbitals on N atom in  $N_2$ .

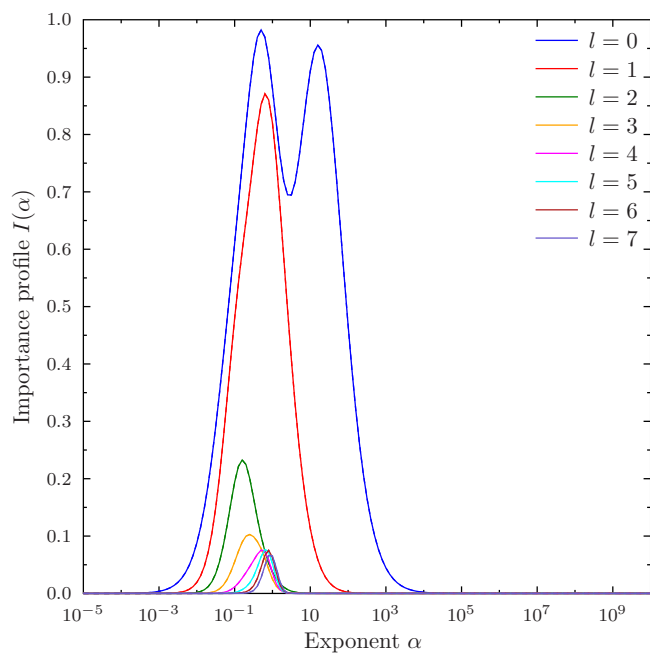

Figure 89. GTO importance profile for  $\sigma$  orbitals on O atom in CO.

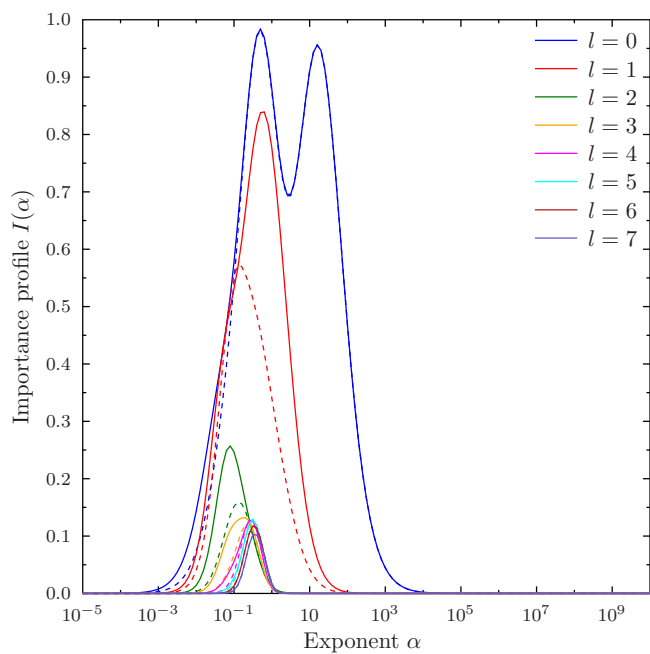

Figure 91. GTO importance profile for  $\sigma$  orbitals on O atom in GaO.

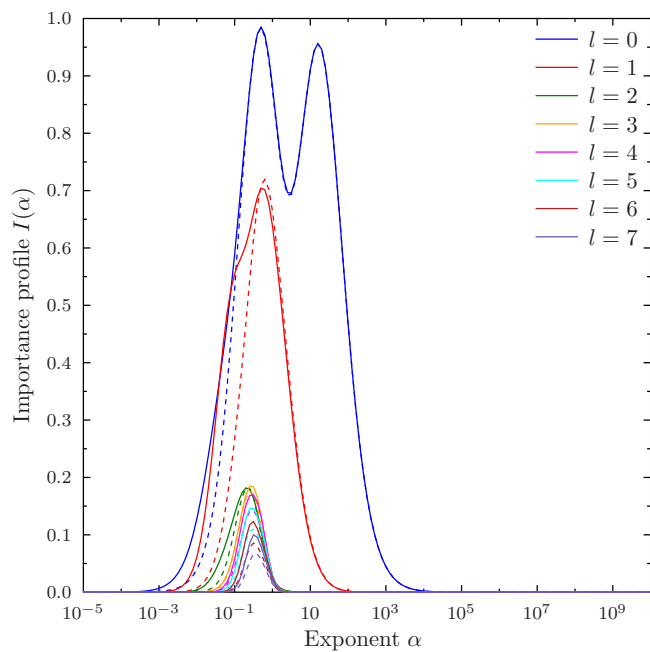

Figure 90. GTO importance profile for  $\sigma$  orbitals on O atom in FeO.

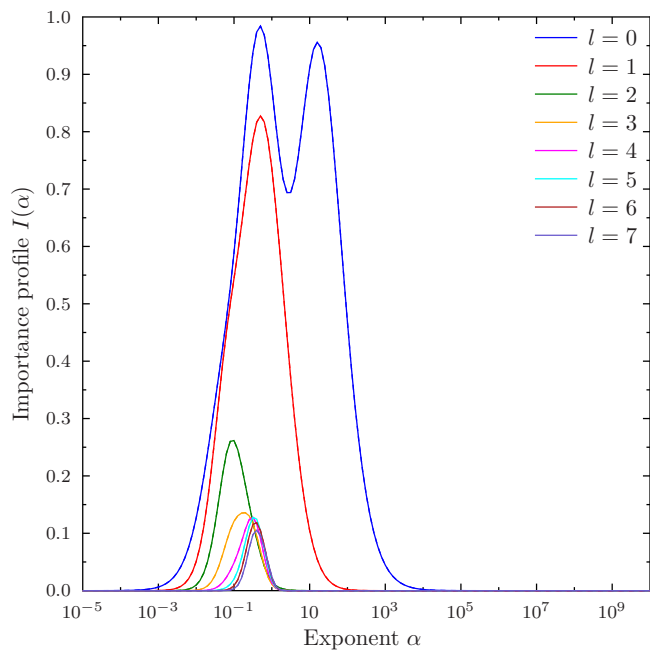

Figure 92. GTO importance profile for  $\sigma$  orbitals on O atom in GeO.

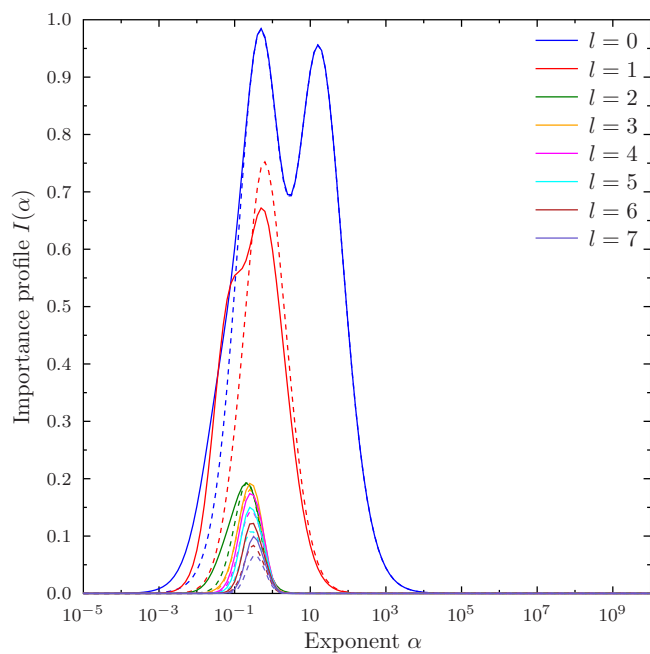

Figure 93. GTO importance profile for  $\sigma$  orbitals on O atom in MnO.

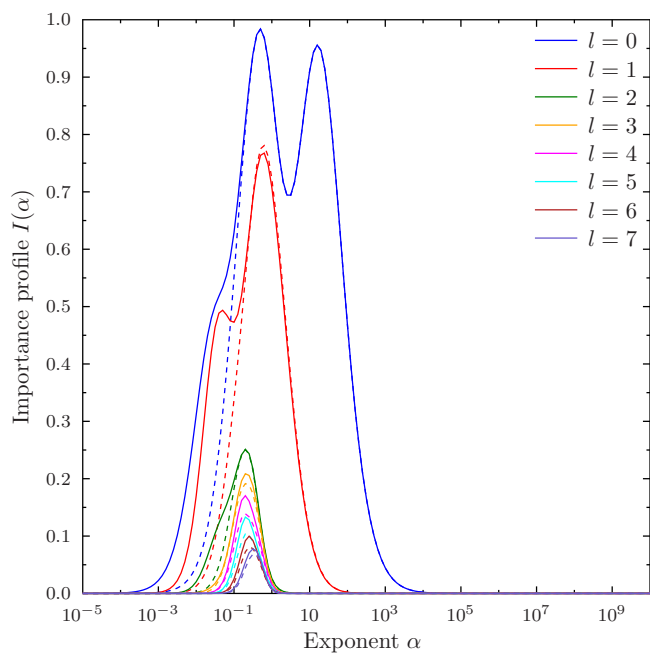

Figure 95. GTO importance profile for  $\sigma$  orbitals on O atom in ScO.

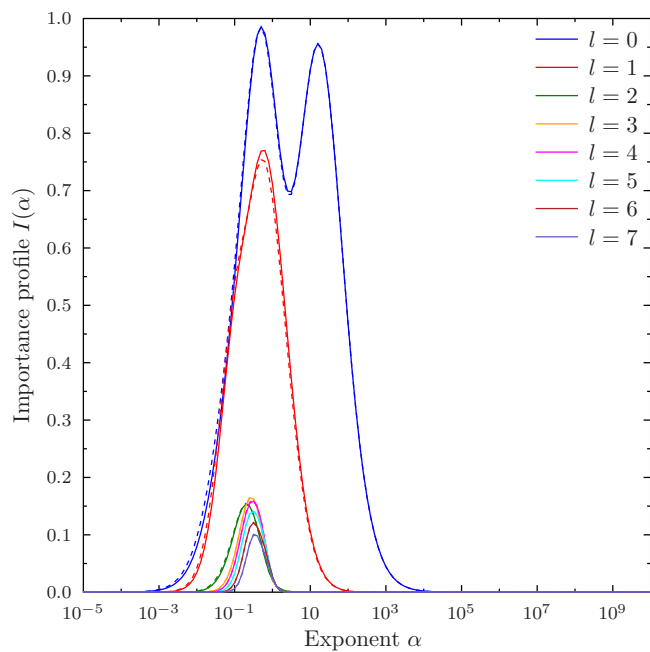

Figure 94. GTO importance profile for  $\sigma$  orbitals on O atom in NiO.

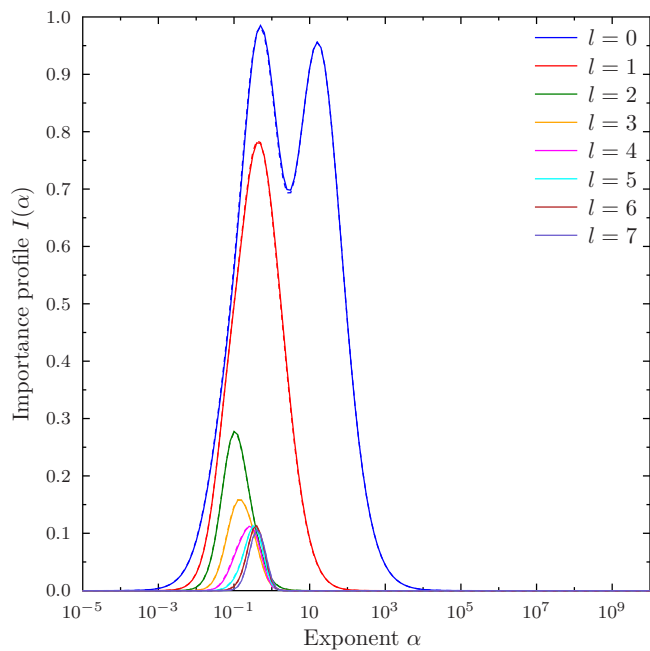

Figure 96. GTO importance profile for  $\sigma$  orbitals on O atom in SeO.

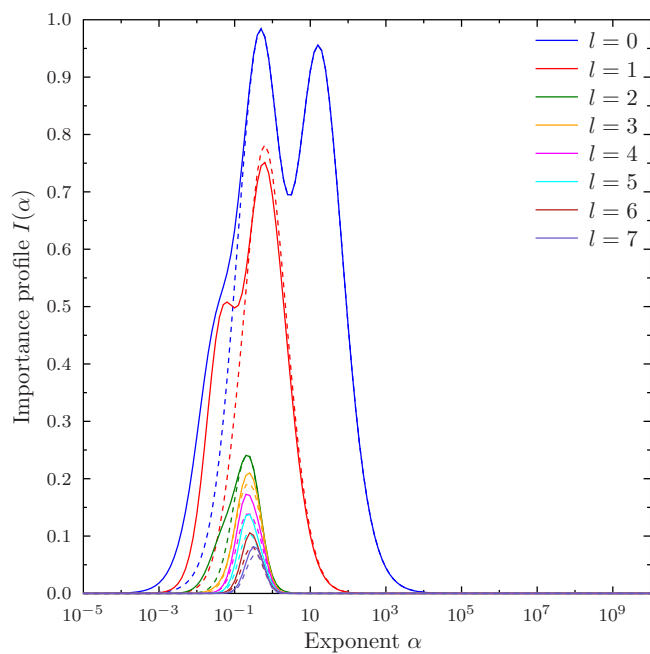

Figure 97. GTO importance profile for  $\sigma$  orbitals on O atom in TiO.

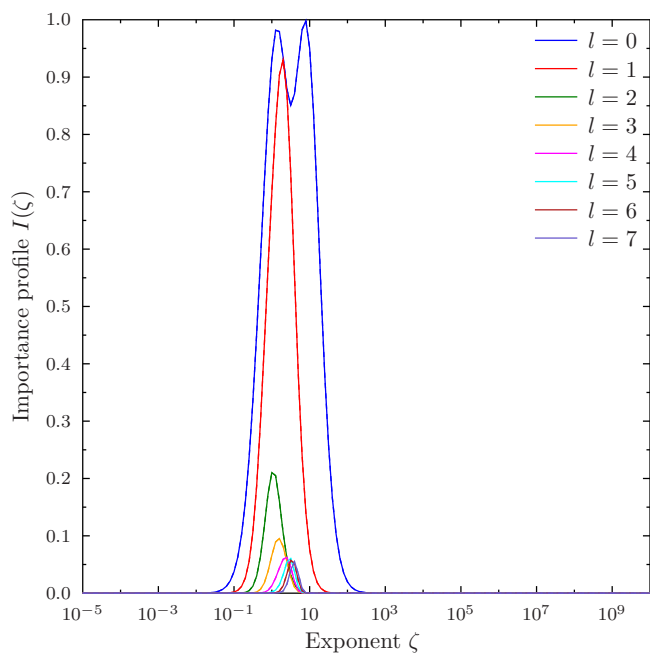

Figure 99. STO importance profile for  $\sigma$  orbitals on O atom in CO.

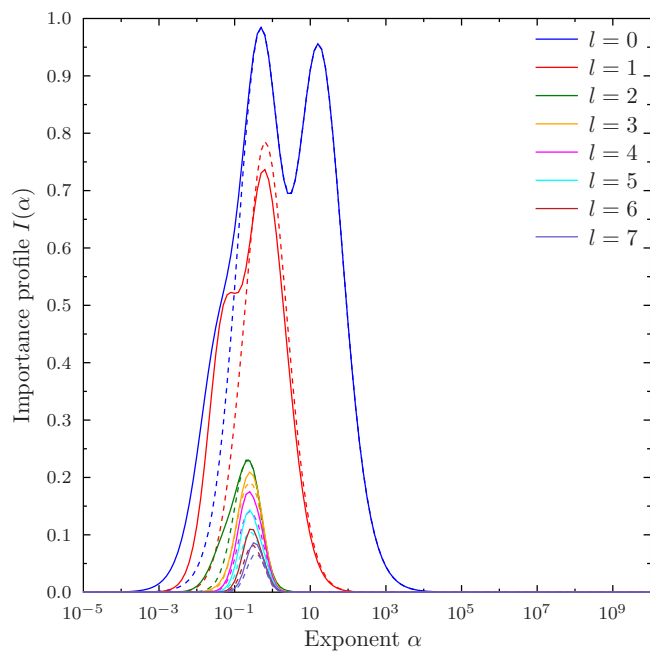

Figure 98. GTO importance profile for  $\sigma$  orbitals on O atom in VO.

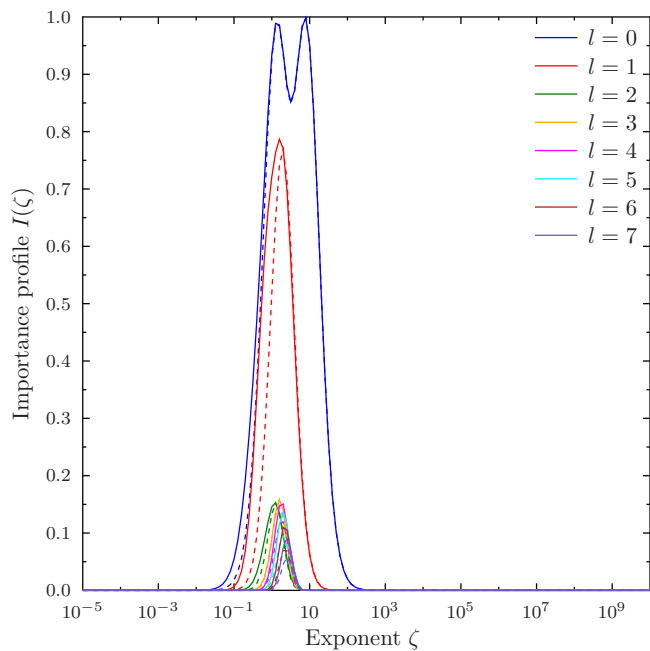

Figure 100. STO importance profile for  $\sigma$  orbitals on O atom in FeO.

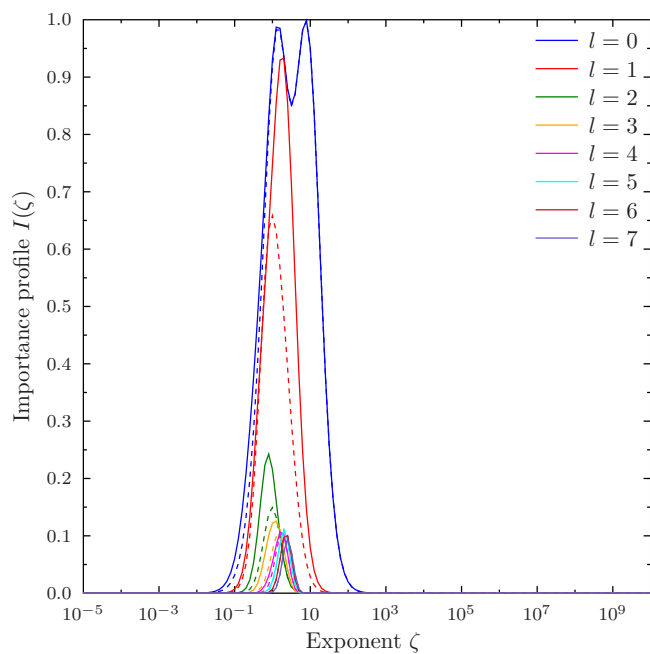

Figure 101. STO importance profile for  $\sigma$  orbitals on O atom in GaO.

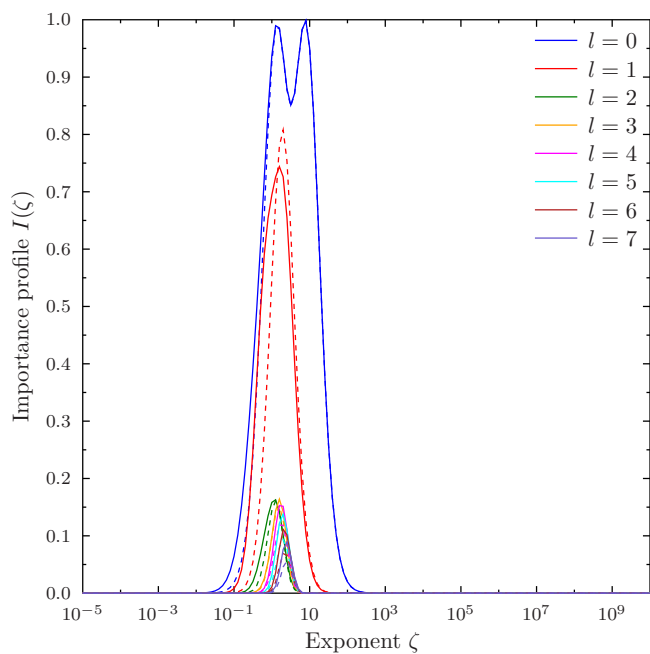

Figure 103. STO importance profile for  $\sigma$  orbitals on O atom in MnO.

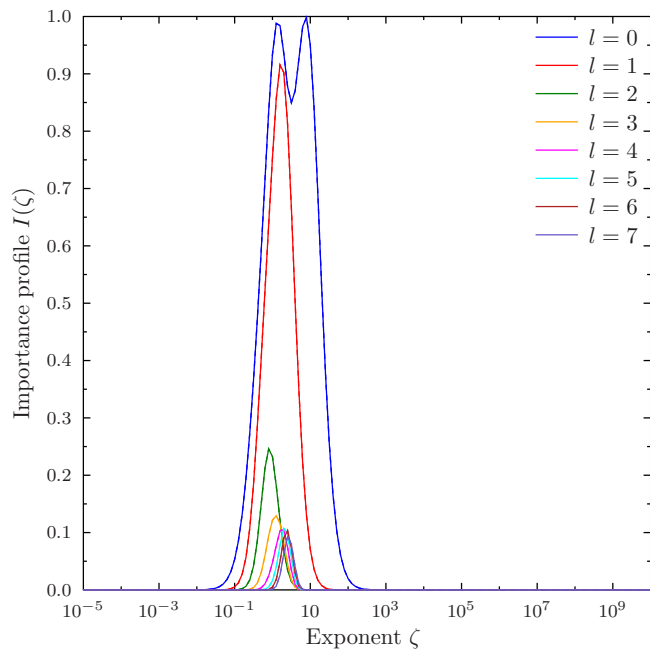

Figure 102. STO importance profile for  $\sigma$  orbitals on O atom in GeO.

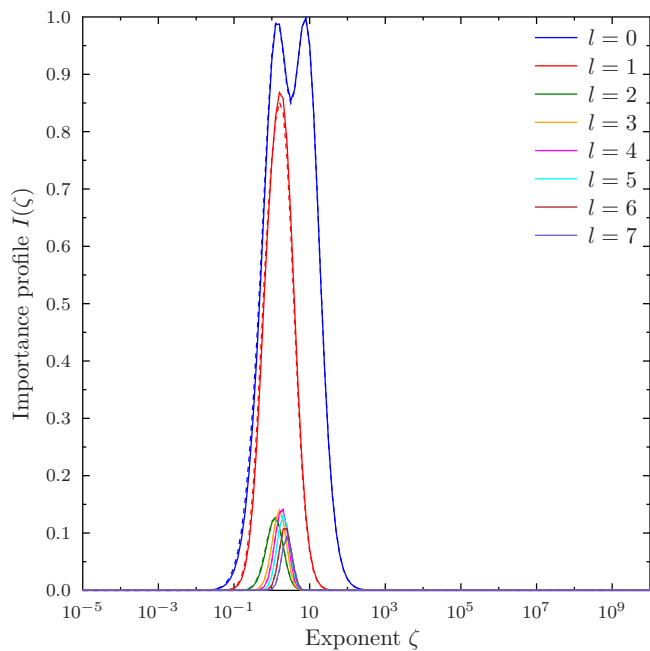

Figure 104. STO importance profile for  $\sigma$  orbitals on O atom in NiO.

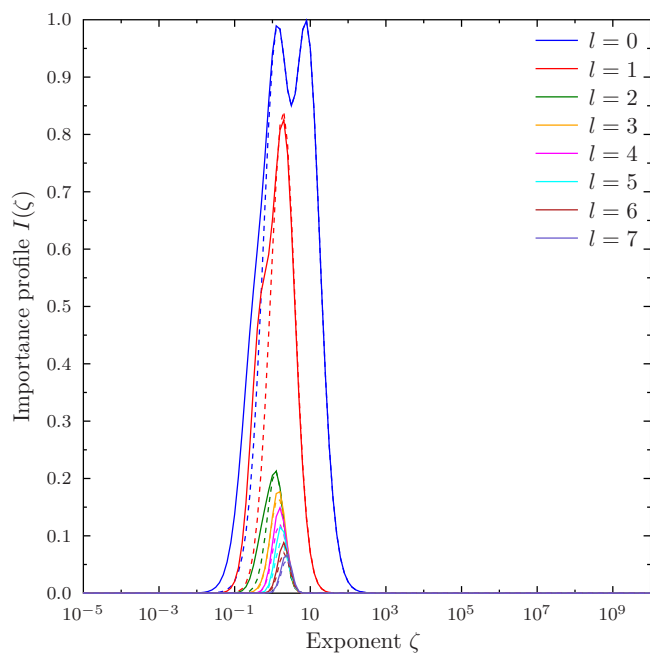

Figure 105. STO importance profile for  $\sigma$  orbitals on O atom in ScO.

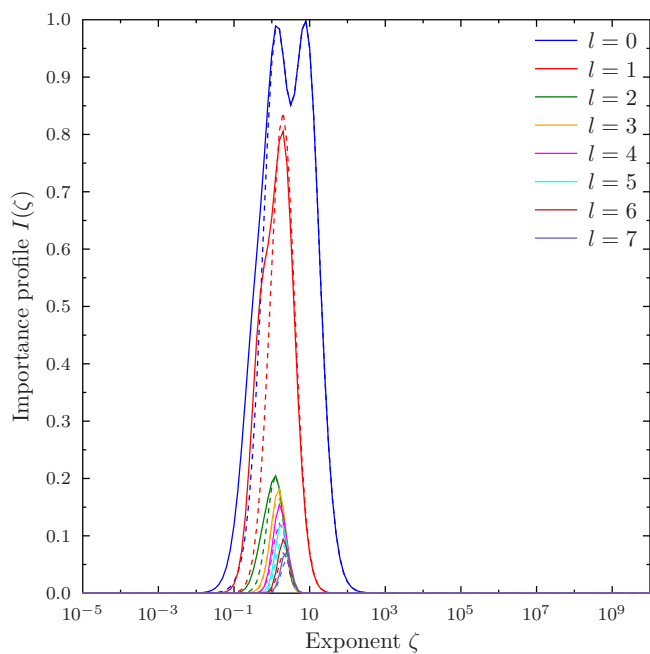

Figure 107. STO importance profile for  $\sigma$  orbitals on O atom in TiO.

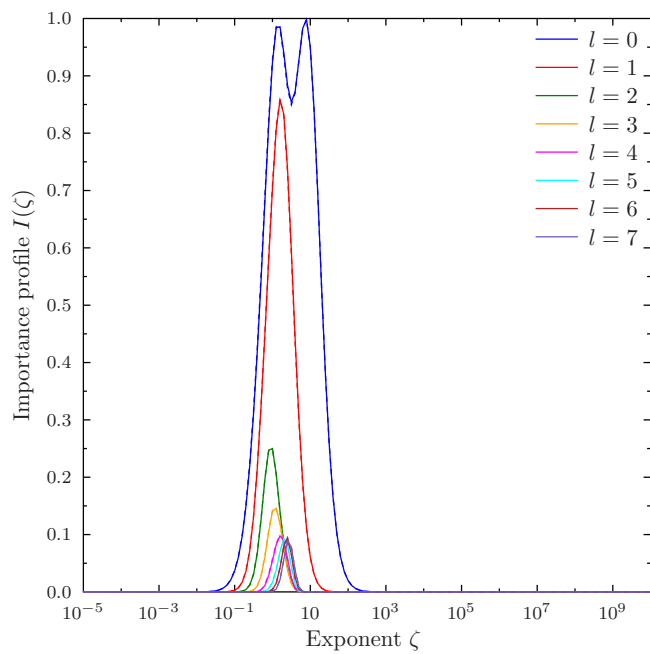

Figure 106. STO importance profile for  $\sigma$  orbitals on O atom in SeO.

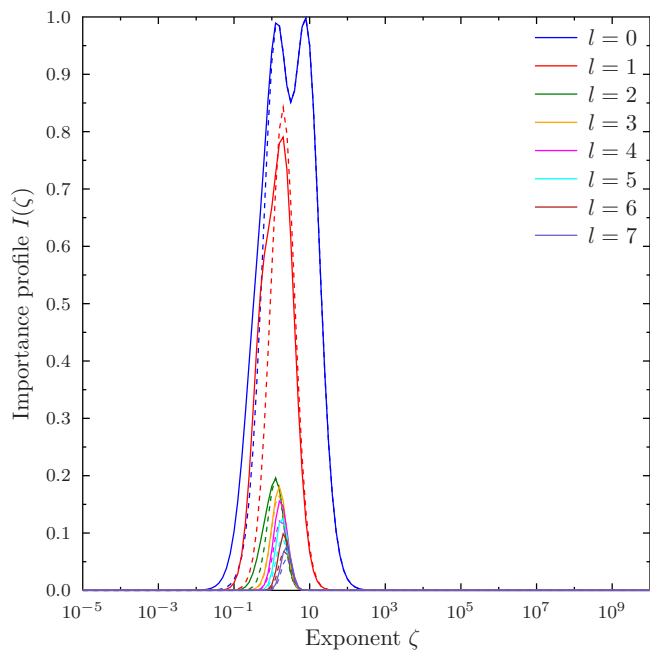

Figure 108. STO importance profile for  $\sigma$  orbitals on O atom in VO.

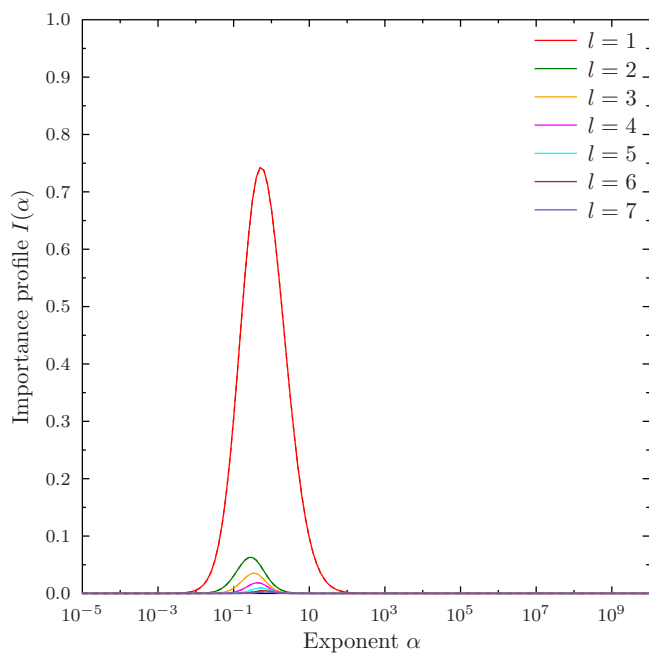

Figure 109. GTO importance profile for  $\pi_-$  orbitals on O atom in CO.

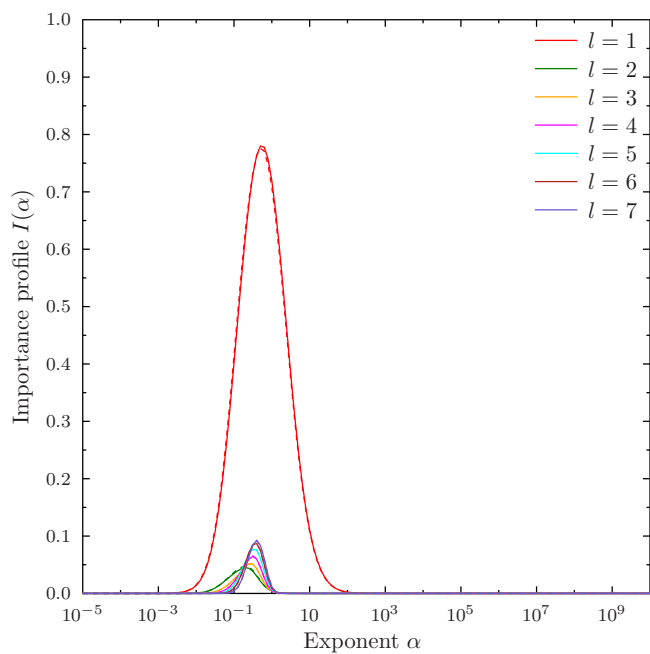

Figure 111. GTO importance profile for  $\pi_-$  orbitals on O atom in GaO.

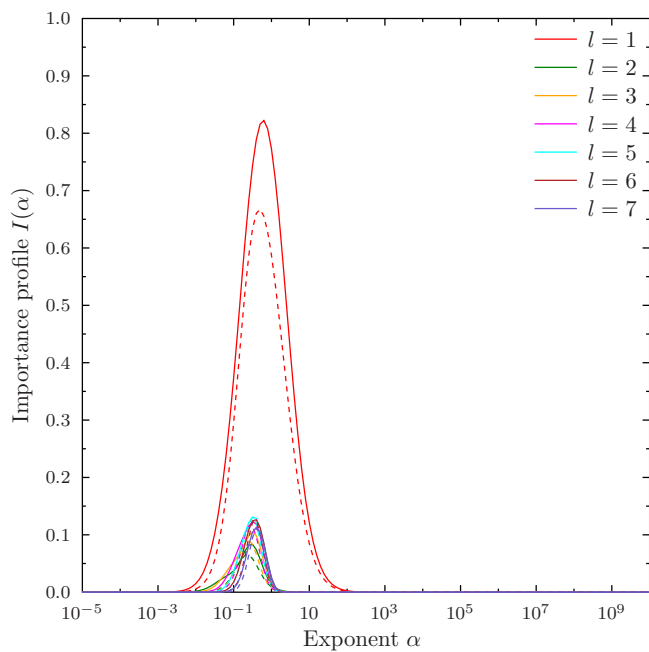

Figure 110. GTO importance profile for  $\pi_-$  orbitals on O atom in FeO.

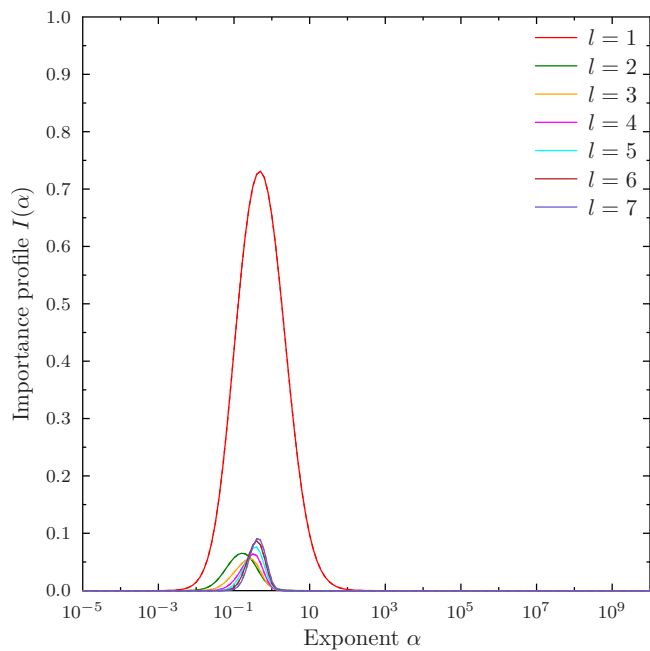

Figure 112. GTO importance profile for  $\pi_-$  orbitals on O atom in GeO.



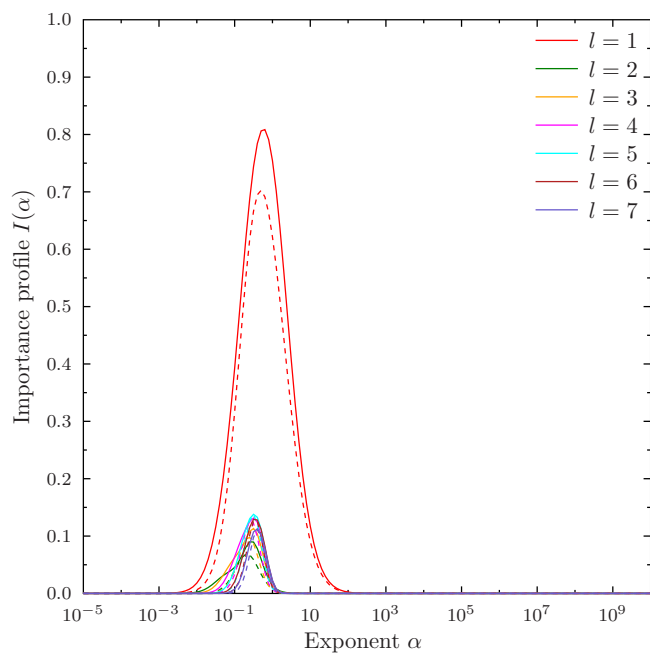

Figure 113. GTO importance profile for  $\pi_-$  orbitals on O atom in MnO.

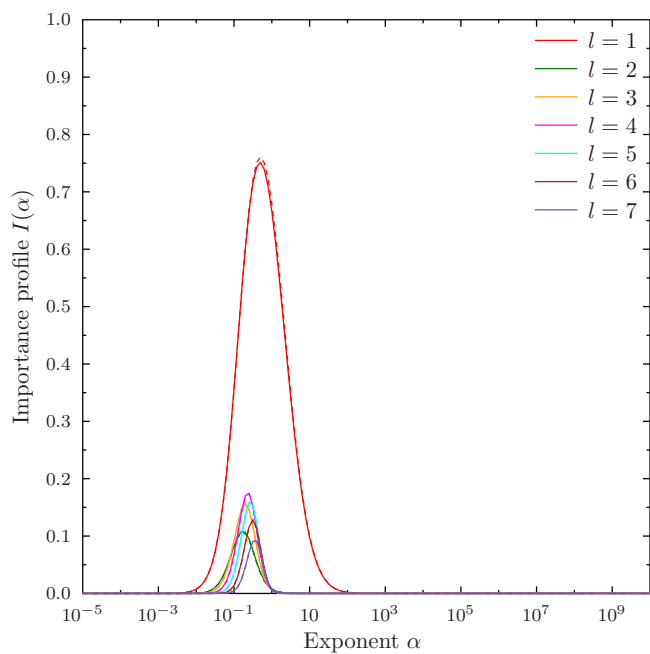

Figure 115. GTO importance profile for  $\pi_-$  orbitals on O atom in ScO.

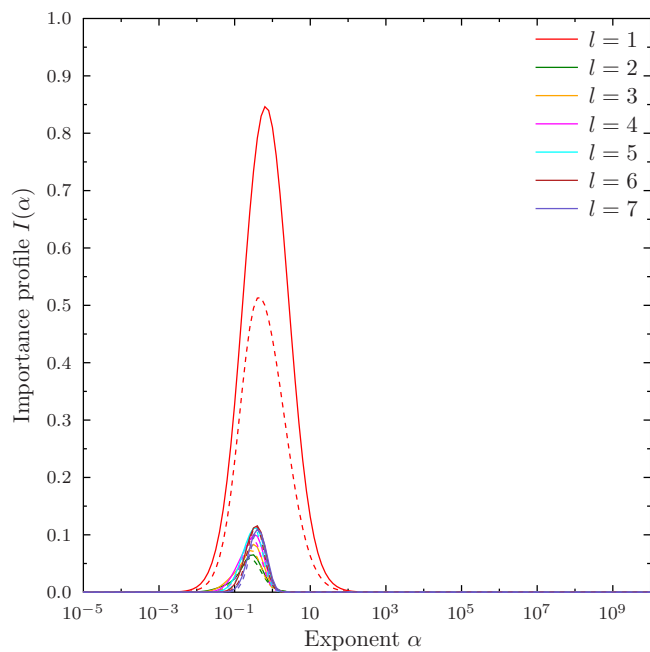

Figure 114. GTO importance profile for  $\pi_-$  orbitals on O atom in NiO.

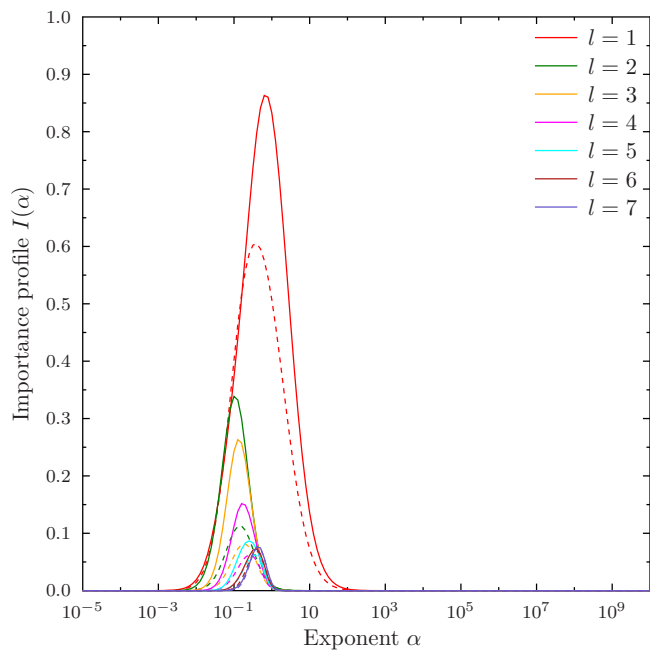

Figure 116. GTO importance profile for  $\pi_-$  orbitals on O atom in SeO.

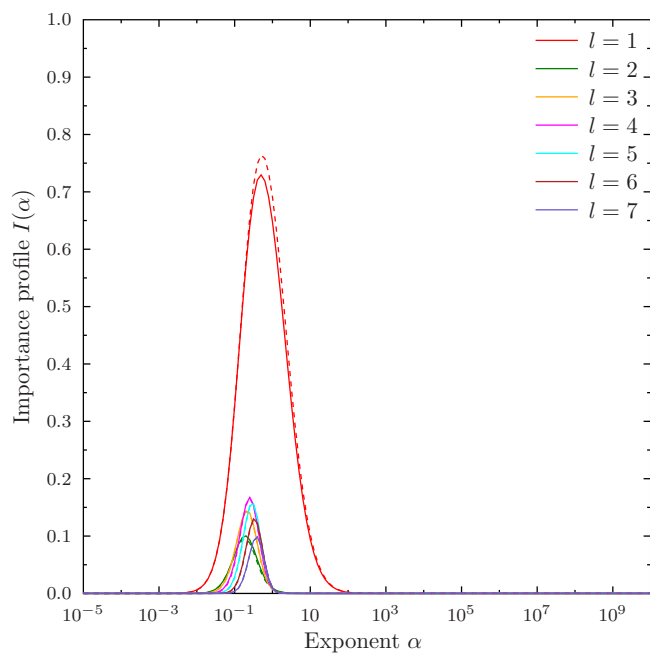

Figure 117. GTO importance profile for  $\pi_-$  orbitals on O atom in TiO.

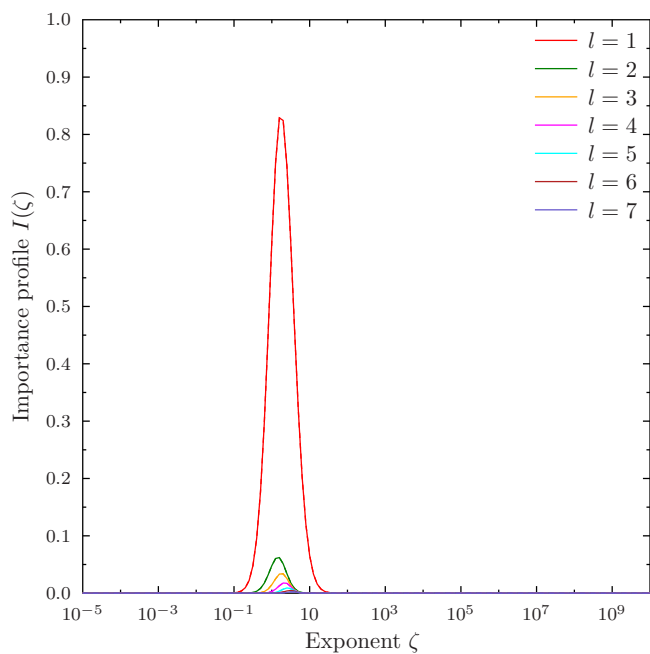

Figure 119. STO importance profile for  $\pi_-$  orbitals on O atom in CO.

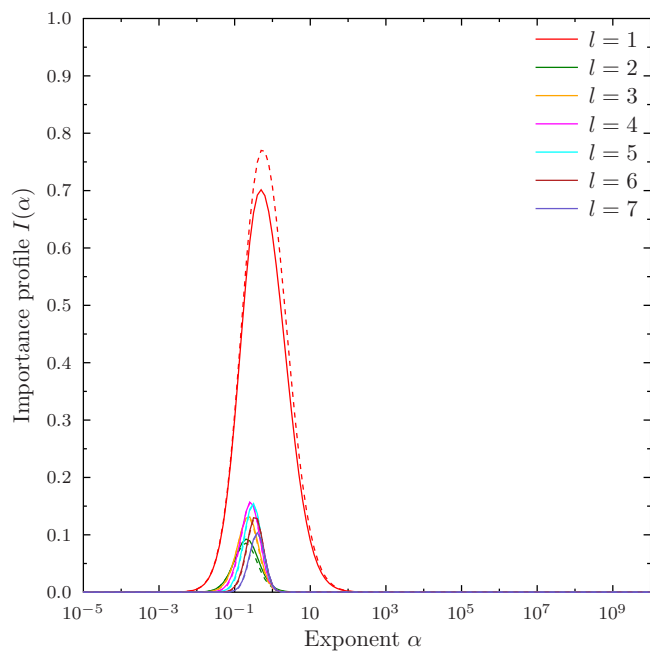

Figure 118. GTO importance profile for  $\pi_-$  orbitals on O atom in VO.

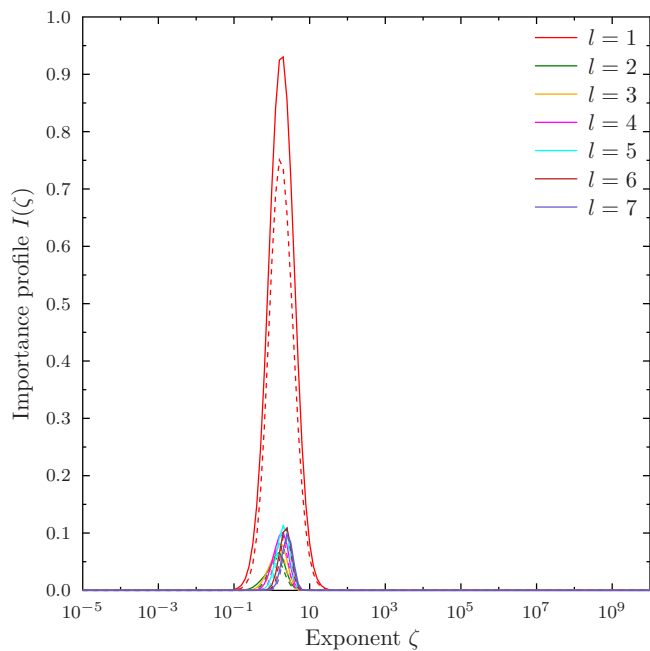

Figure 120. STO importance profile for  $\pi_-$  orbitals on O atom in FeO.

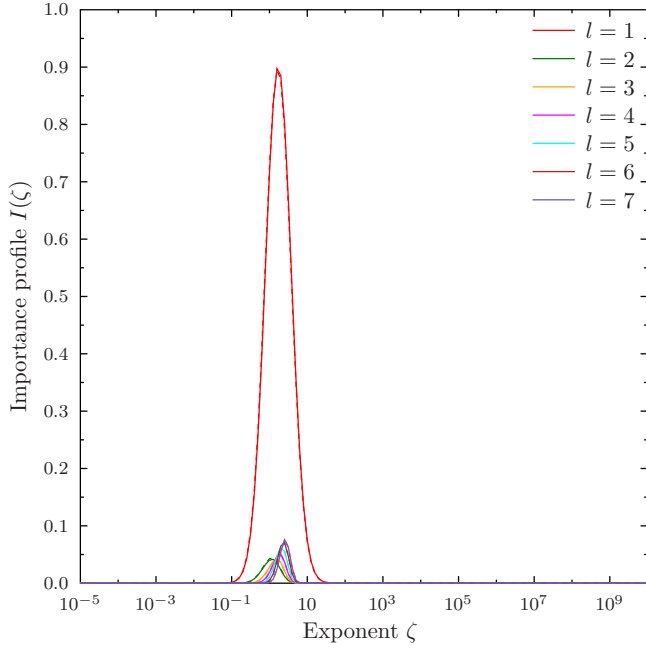

Figure 121. STO importance profile for  $\pi_-$  orbitals on O atom in GaO.

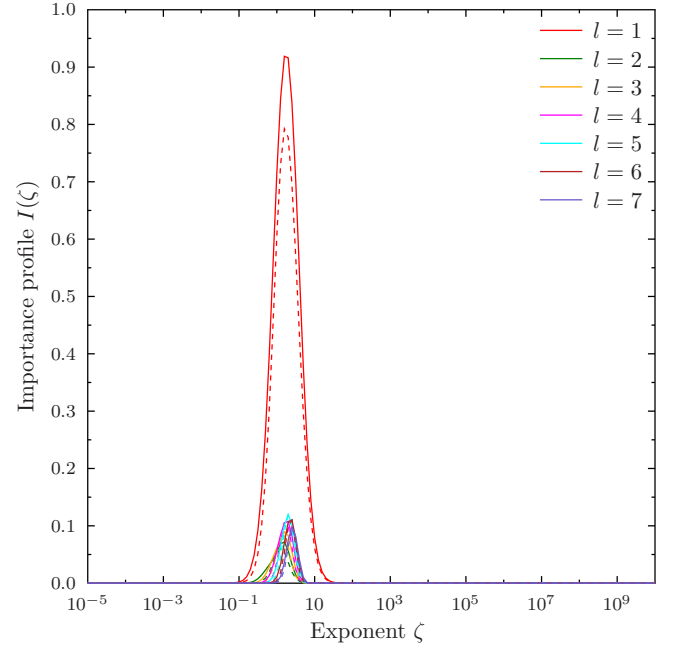

Figure 123. STO importance profile for  $\pi_-$  orbitals on O atom in MnO.

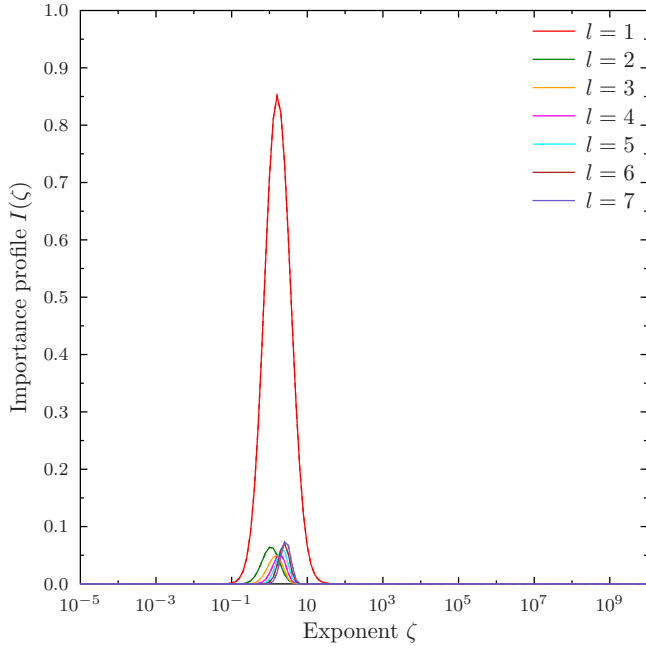

Figure 122. STO importance profile for  $\pi_-$  orbitals on O atom in GeO.

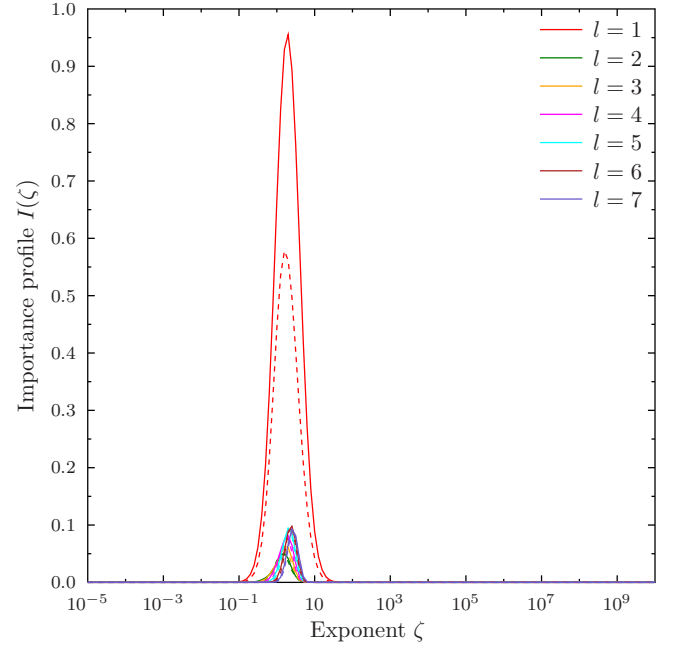

Figure 124. STO importance profile for  $\pi_-$  orbitals on O atom in NiO.

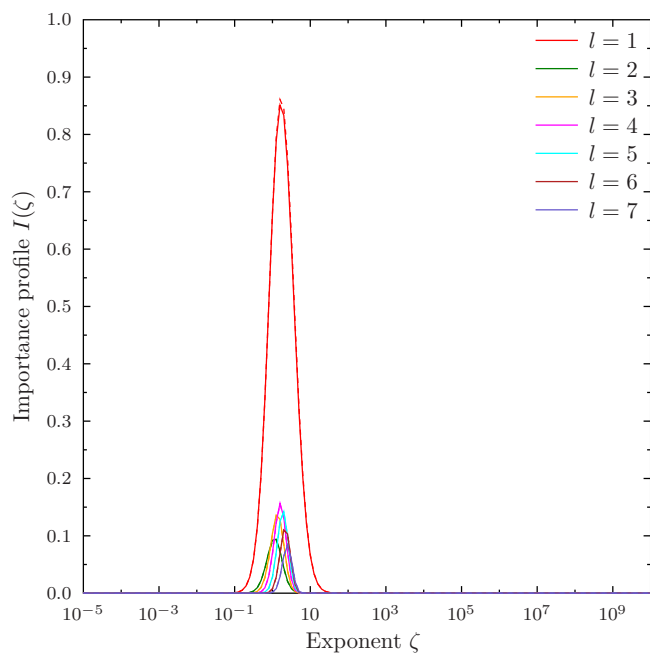

Figure 125. STO importance profile for  $\pi_-$  orbitals on O atom in ScO.

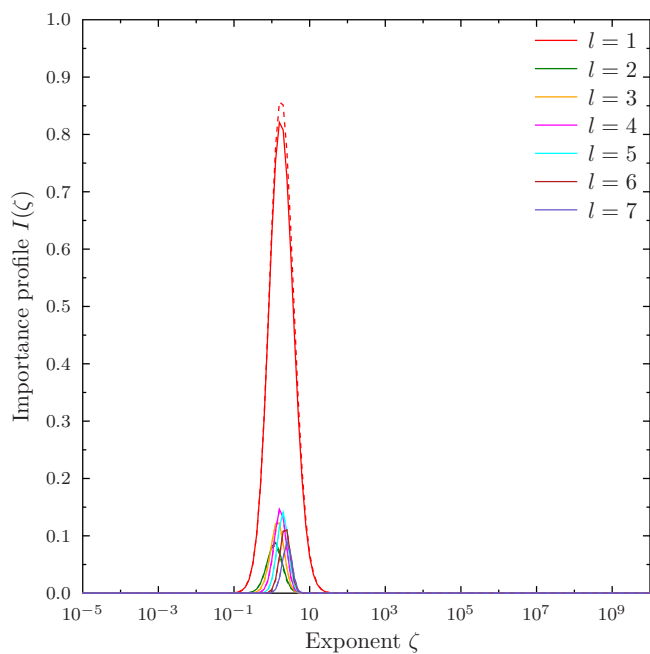

Figure 127. STO importance profile for  $\pi_-$  orbitals on O atom in TiO.

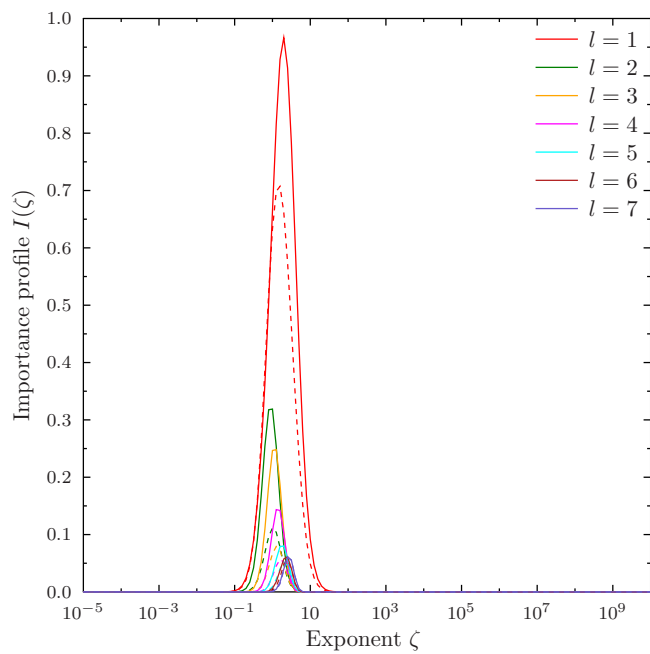

Figure 126. STO importance profile for  $\pi_-$  orbitals on O atom in SeO.

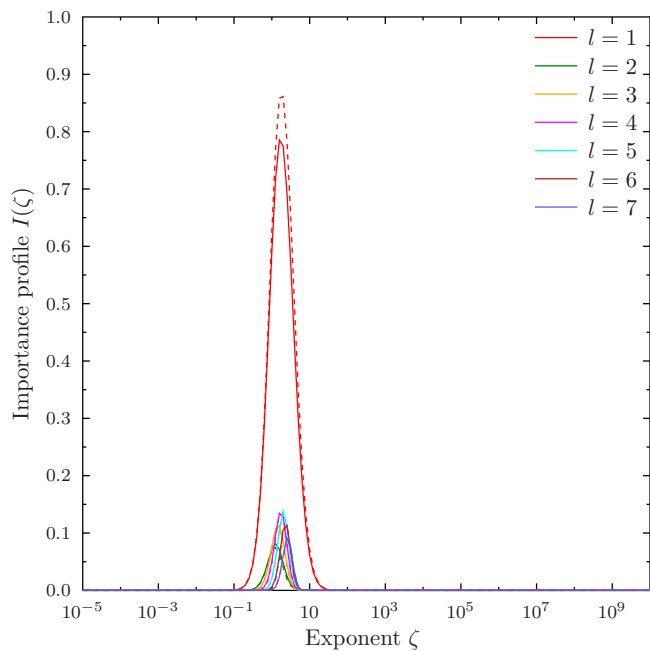

Figure 128. STO importance profile for  $\pi_-$  orbitals on O atom in VO.

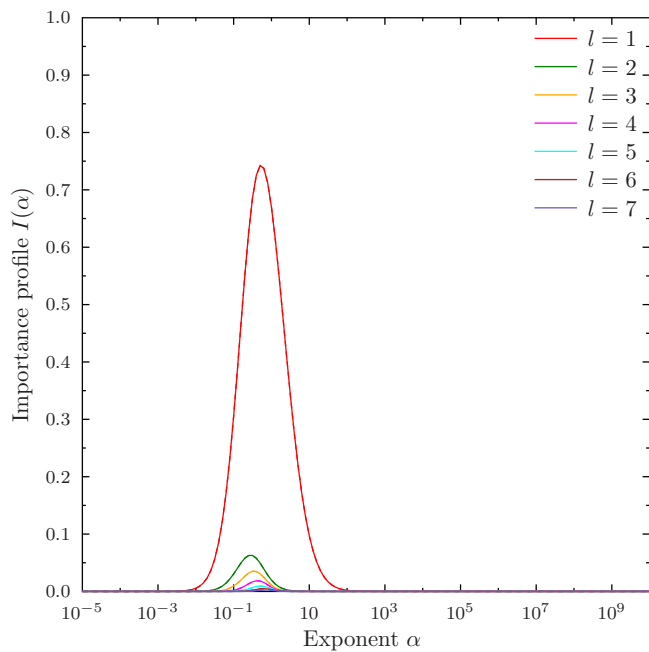

Figure 129. GTO importance profile for  $\pi_+$  orbitals on O atom in CO.

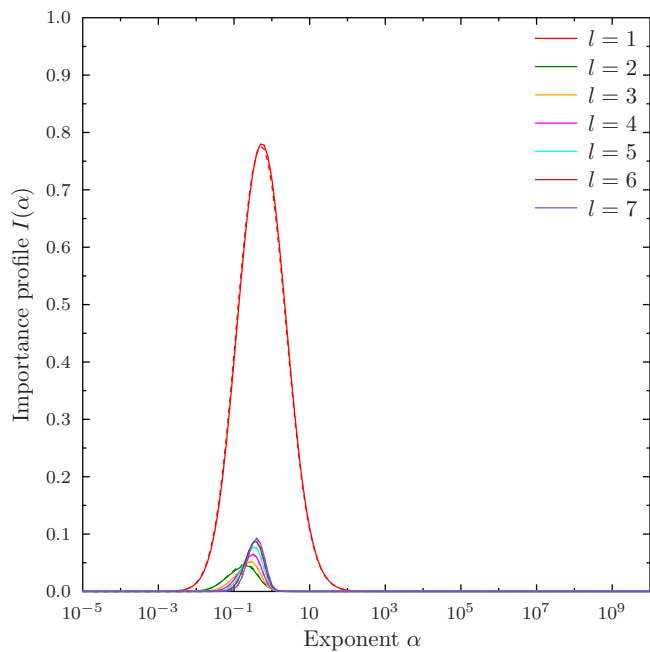

Figure 131. GTO importance profile for  $\pi_+$  orbitals on O atom in GaO.

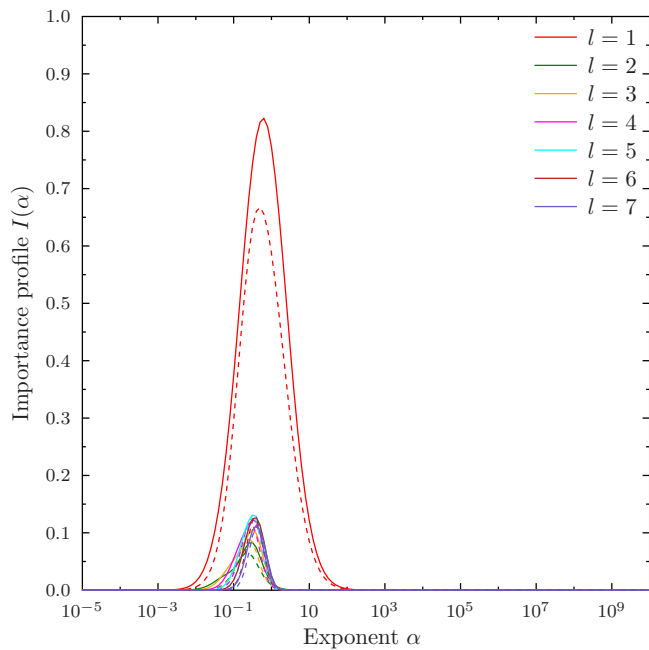

Figure 130. GTO importance profile for  $\pi_+$  orbitals on O atom in FeO.

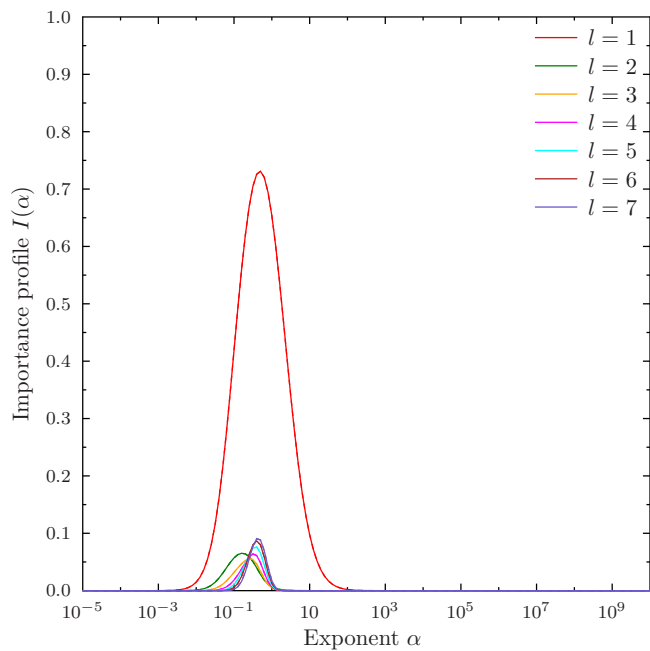

Figure 132. GTO importance profile for  $\pi_+$  orbitals on O atom in GeO.

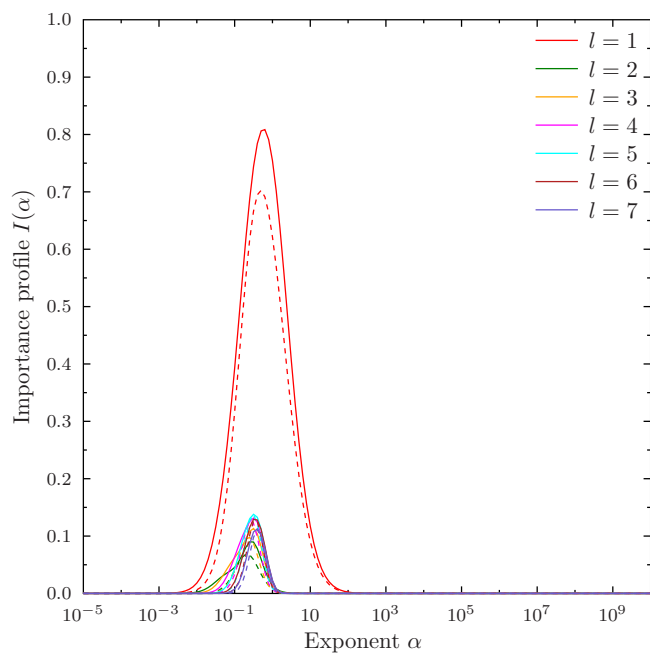

Figure 133. GTO importance profile for  $\pi_+$  orbitals on O atom in MnO.

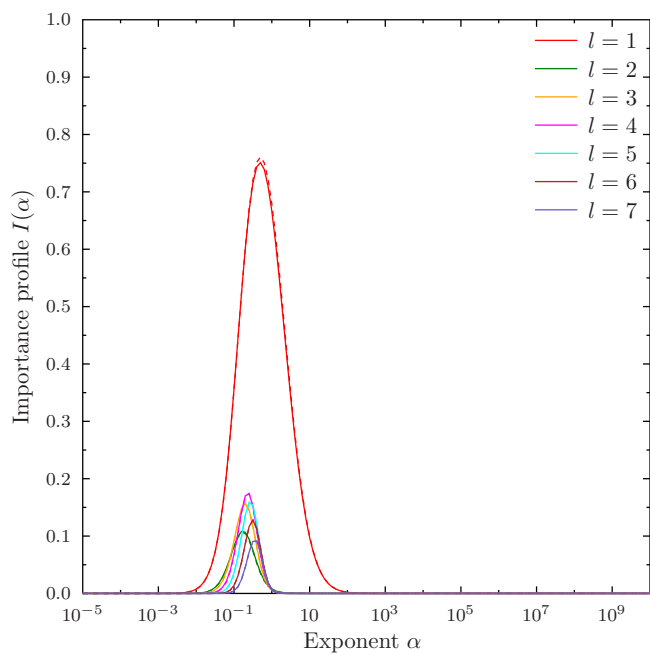

Figure 135. GTO importance profile for  $\pi_+$  orbitals on O atom in ScO.

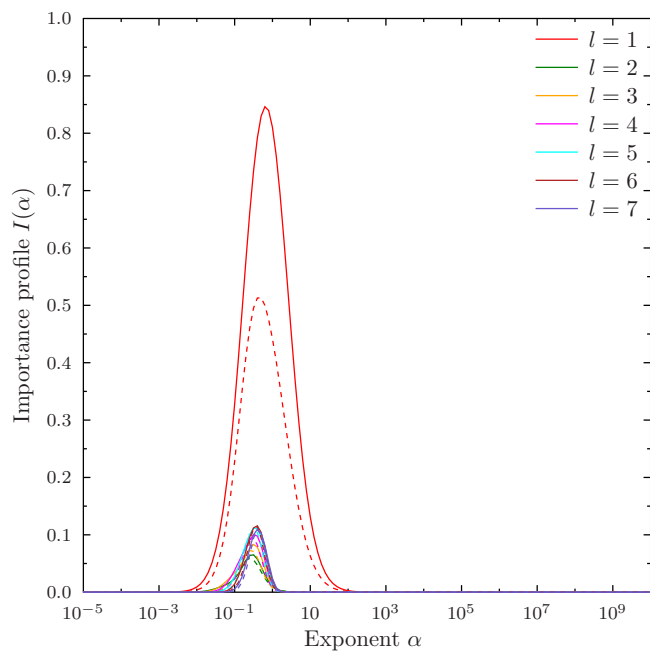

Figure 134. GTO importance profile for  $\pi_+$  orbitals on O atom in NiO.

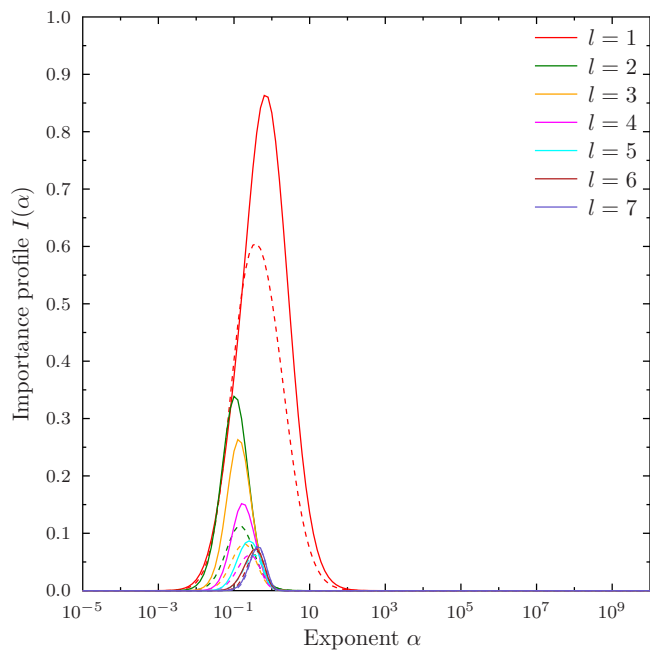

Figure 136. GTO importance profile for  $\pi_+$  orbitals on O atom in SeO.

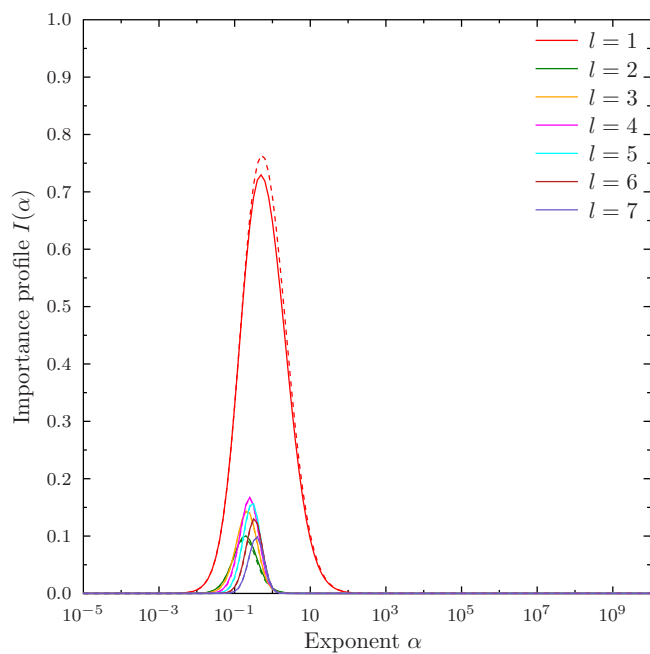

Figure 137. GTO importance profile for  $\pi_+$  orbitals on O atom in TiO.

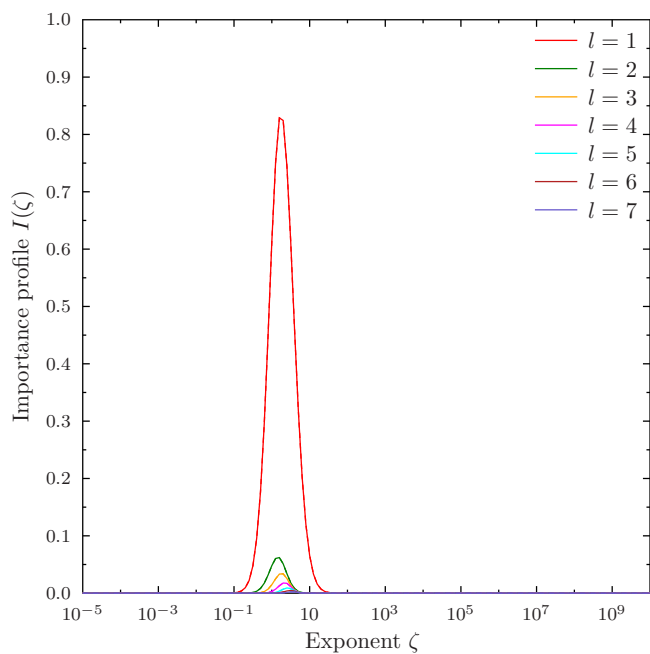

Figure 139. STO importance profile for  $\pi_+$  orbitals on O atom in CO.

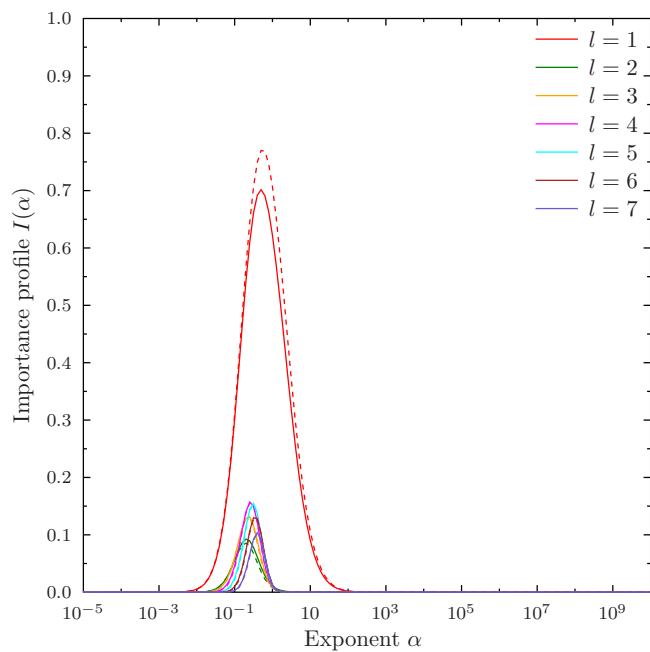

Figure 138. GTO importance profile for  $\pi_+$  orbitals on O atom in VO.

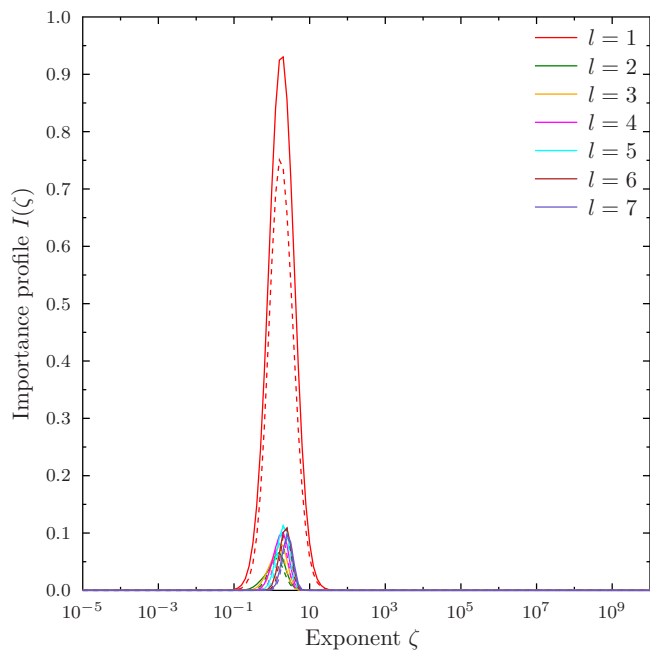

Figure 140. STO importance profile for  $\pi_+$  orbitals on O atom in FeO.

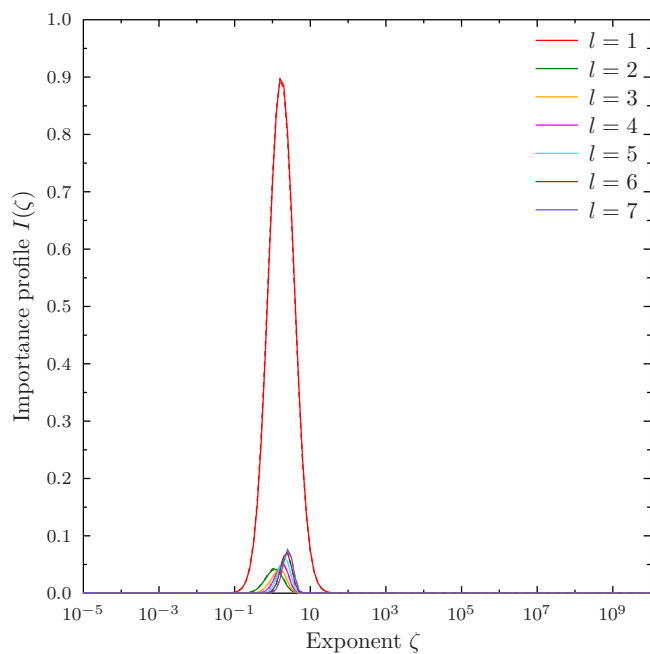

Figure 141. STO importance profile for  $\pi_+$  orbitals on O atom in GaO.

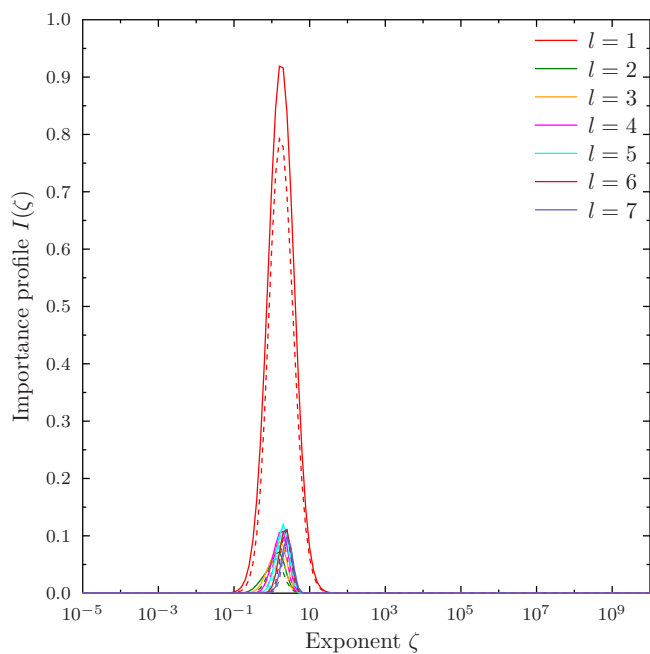

Figure 143. STO importance profile for  $\pi_+$  orbitals on O atom in MnO.

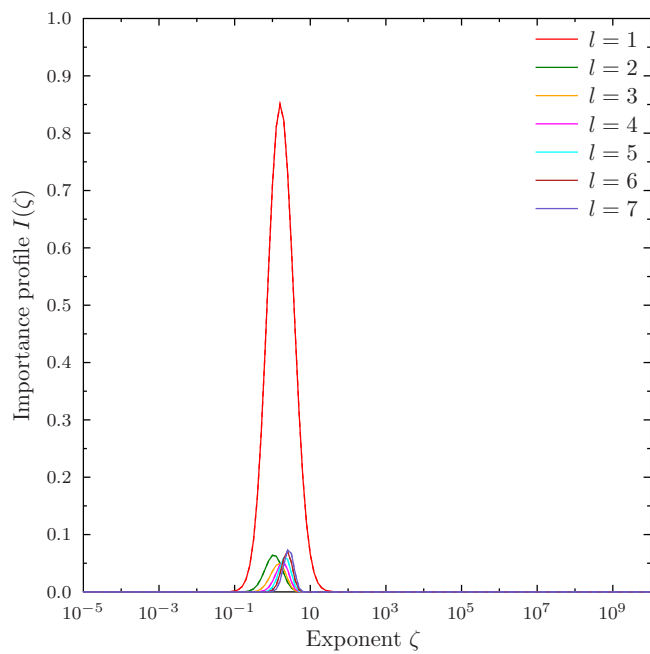

Figure 142. STO importance profile for  $\pi_+$  orbitals on O atom in GeO.

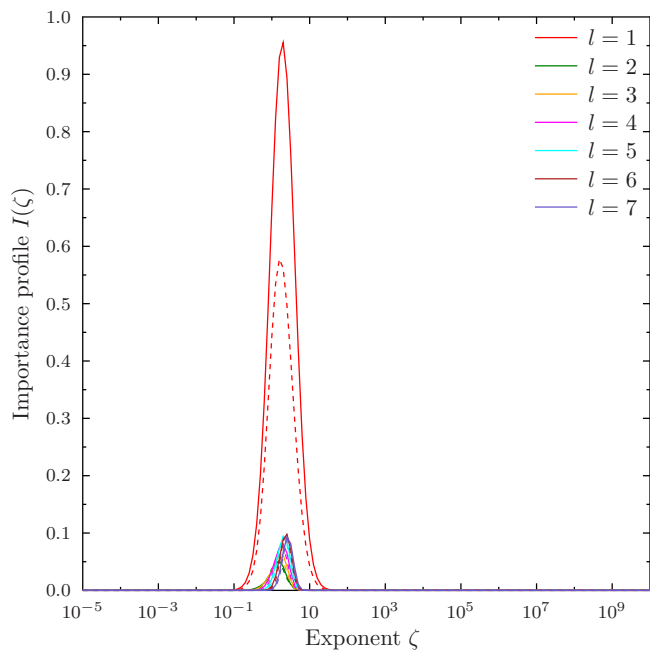

Figure 144. STO importance profile for  $\pi_+$  orbitals on O atom in NiO.



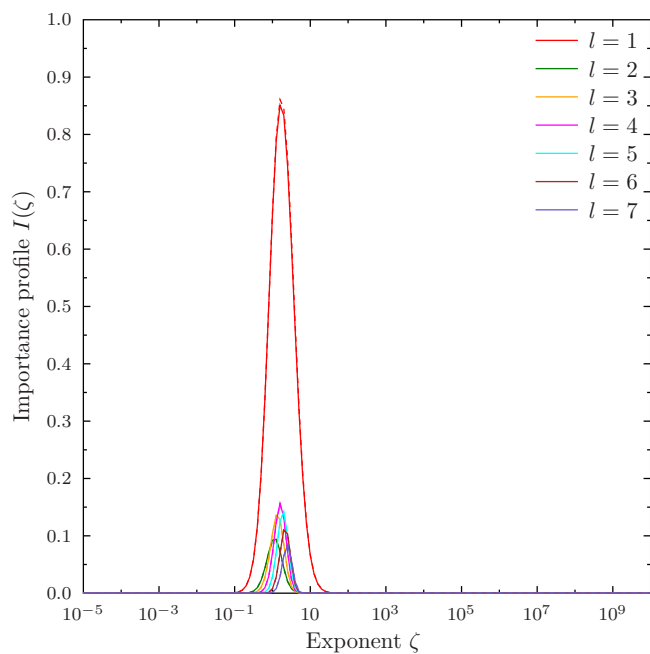

Figure 145. STO importance profile for  $\pi_+$  orbitals on O atom in ScO.

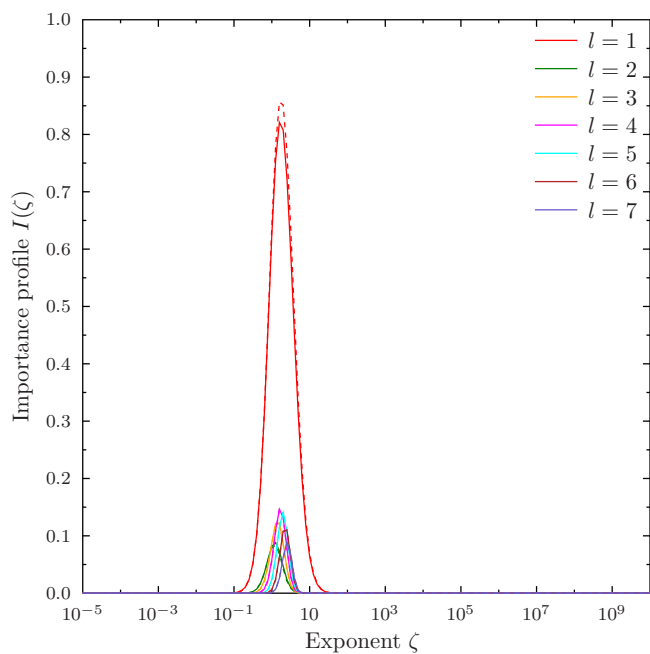

Figure 147. STO importance profile for  $\pi_+$  orbitals on O atom in TiO.

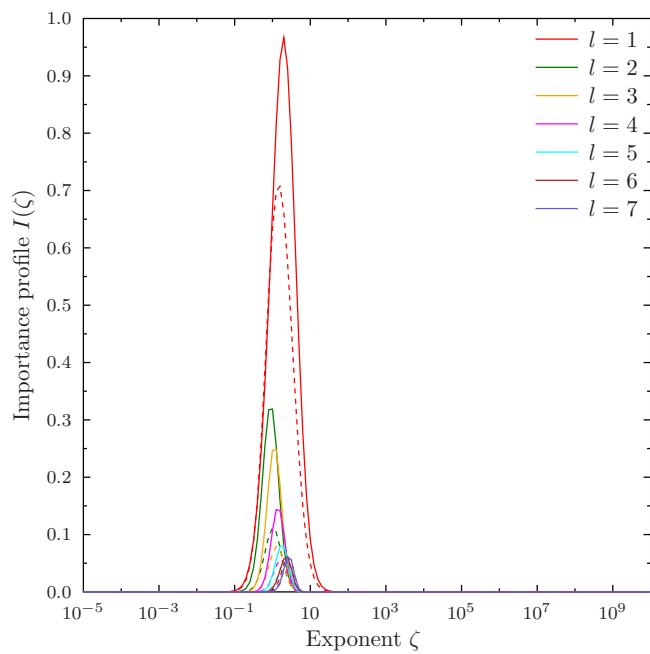

Figure 146. STO importance profile for  $\pi_+$  orbitals on O atom in SeO.

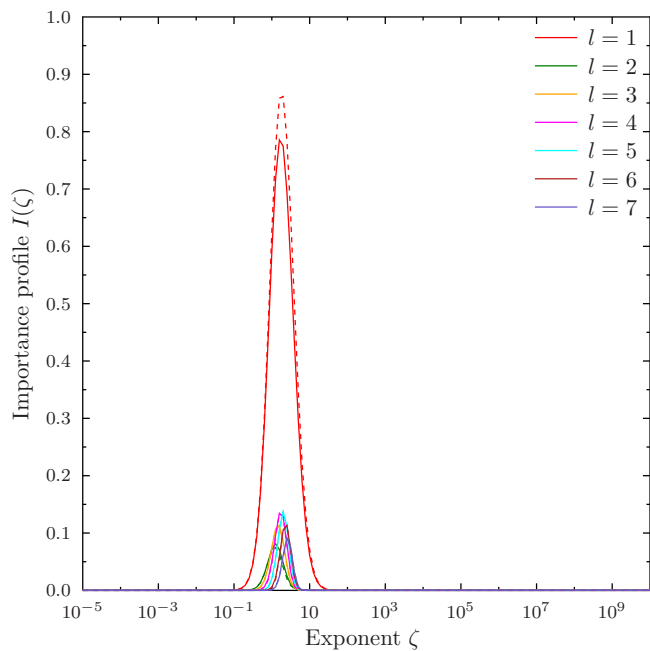

Figure 148. STO importance profile for  $\pi_+$  orbitals on O atom in VO.

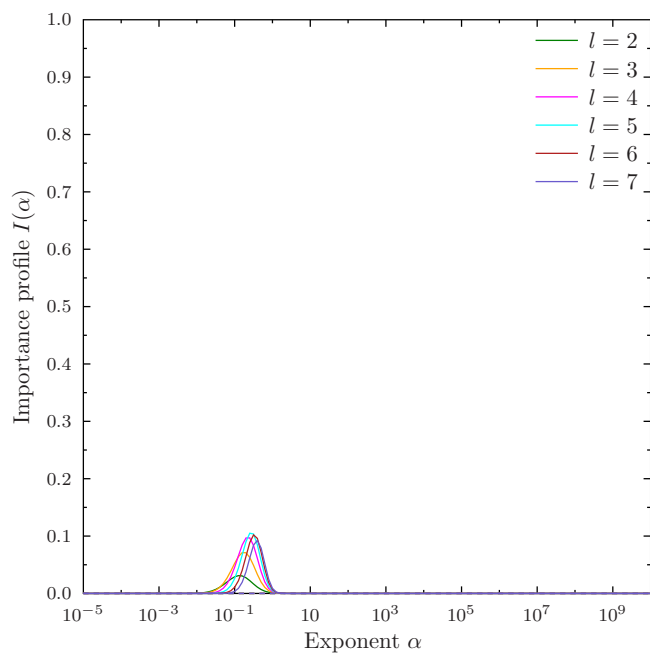

Figure 149. GTO importance profile for  $\delta_-$  orbitals on O atom in FeO.

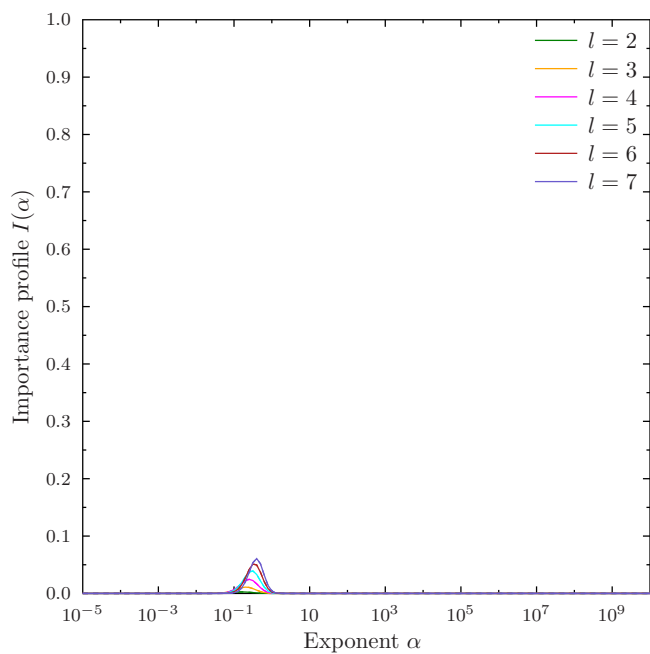

Figure 151. GTO importance profile for  $\delta_-$  orbitals on O atom in GeO.

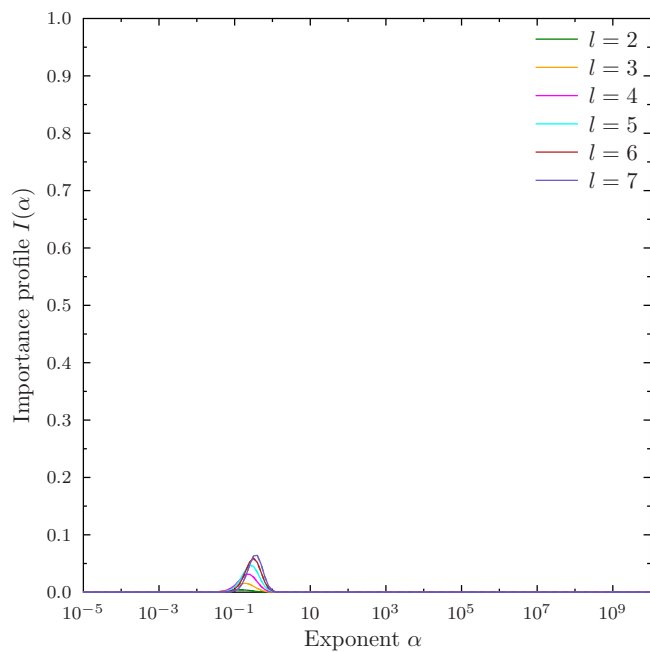

Figure 150. GTO importance profile for  $\delta_-$  orbitals on O atom in GaO.

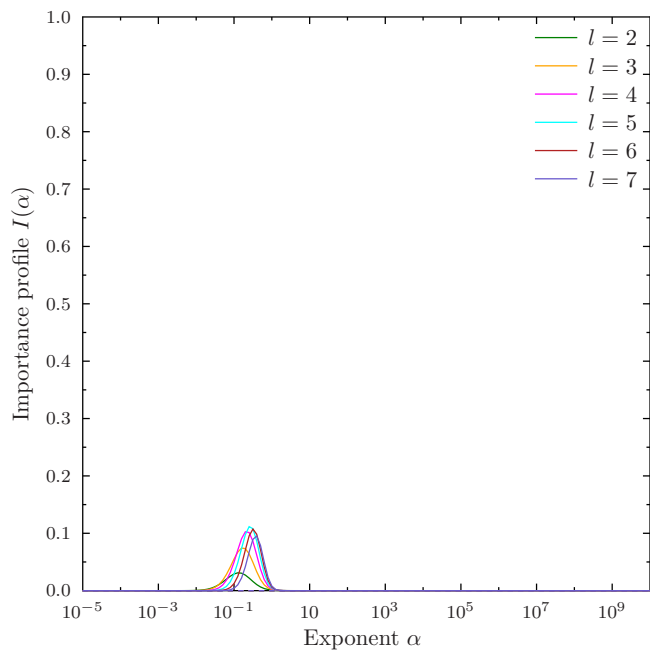

Figure 152. GTO importance profile for  $\delta_-$  orbitals on O atom in MnO.

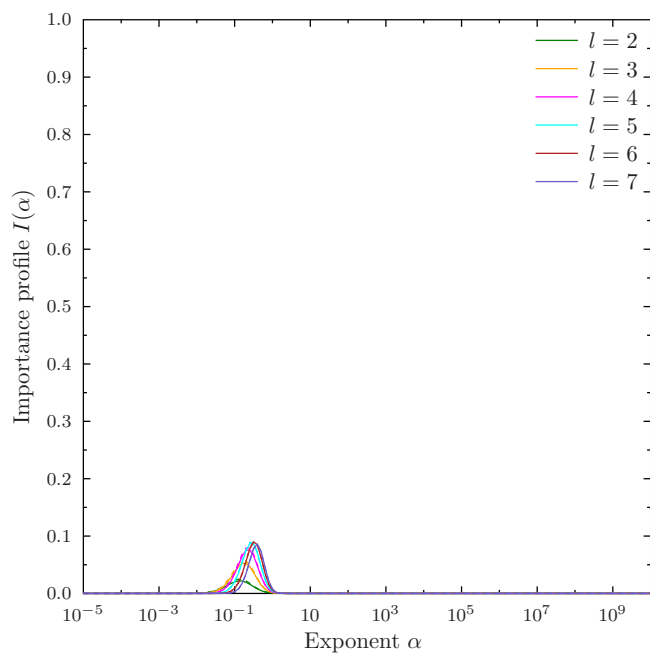

Figure 153. GTO importance profile for  $\delta_-$  orbitals on O atom in NiO.

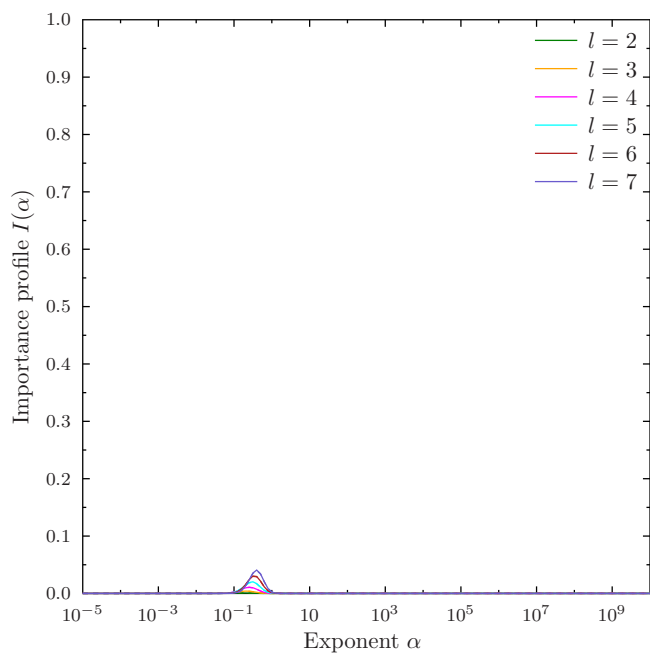

Figure 155. GTO importance profile for  $\delta_-$  orbitals on O atom in SeO.

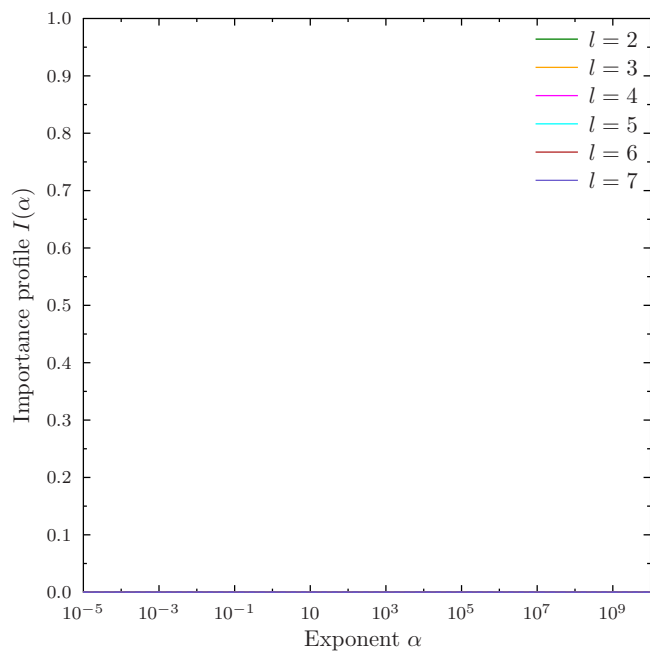

Figure 154. GTO importance profile for  $\delta_-$  orbitals on O atom in ScO.

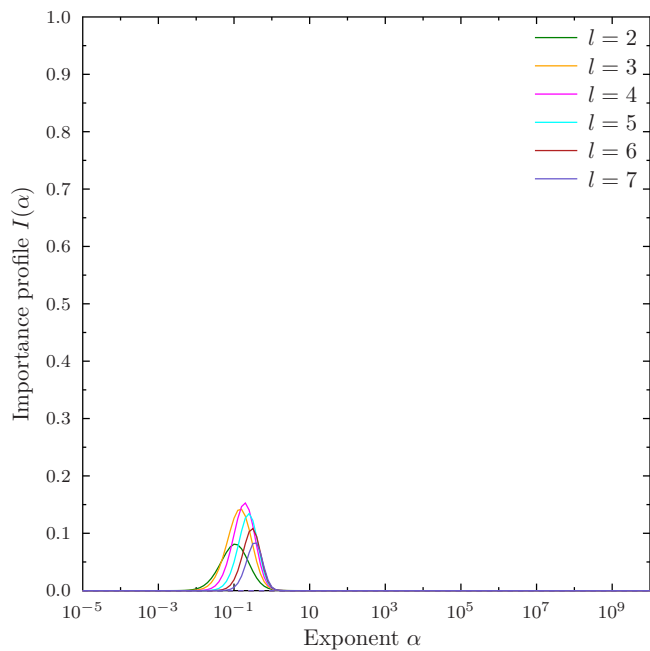

Figure 156. GTO importance profile for  $\delta_-$  orbitals on O atom in TiO.

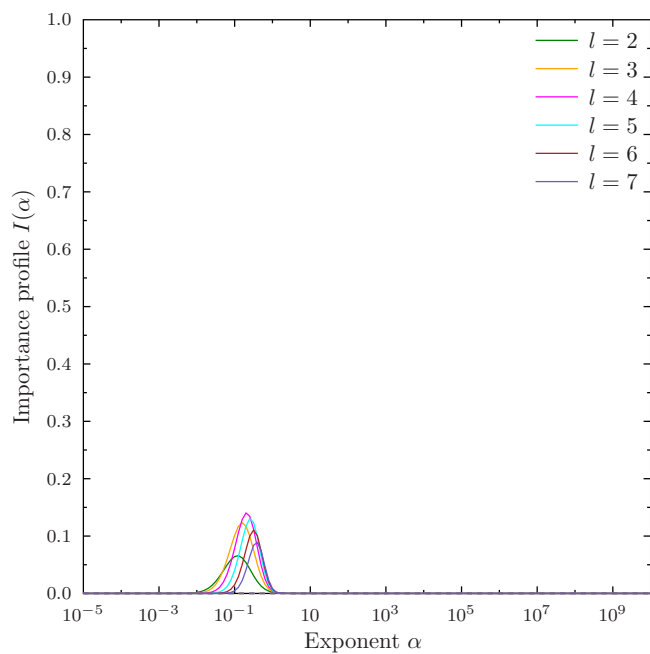

Figure 157. GTO importance profile for  $\delta_-$  orbitals on O atom in VO.

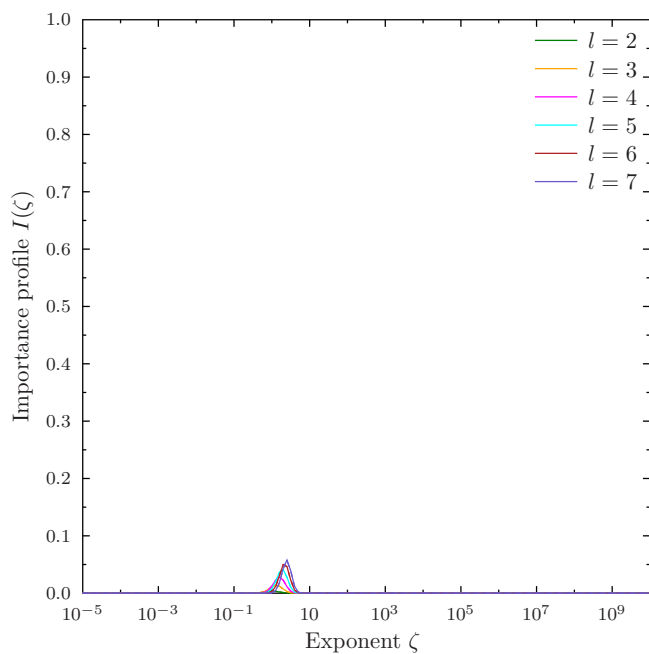

Figure 159. STO importance profile for  $\delta_-$  orbitals on O atom in GaO.

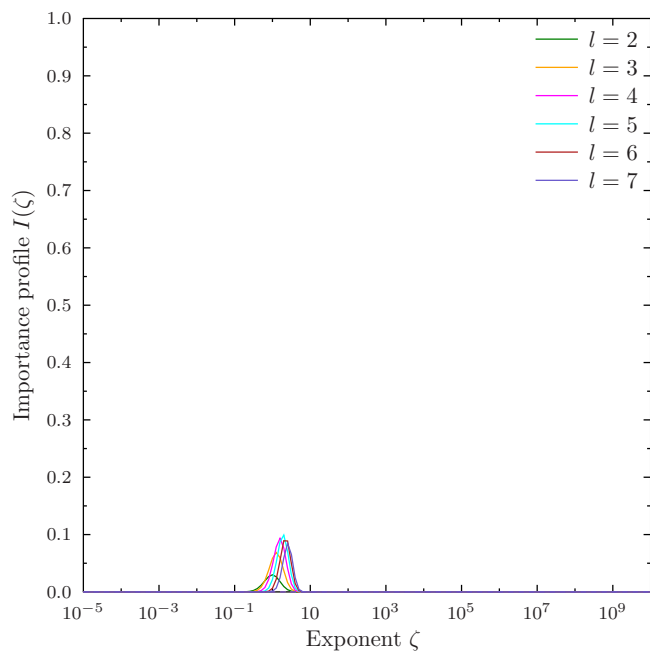

Figure 158. STO importance profile for  $\delta_-$  orbitals on O atom in FeO.

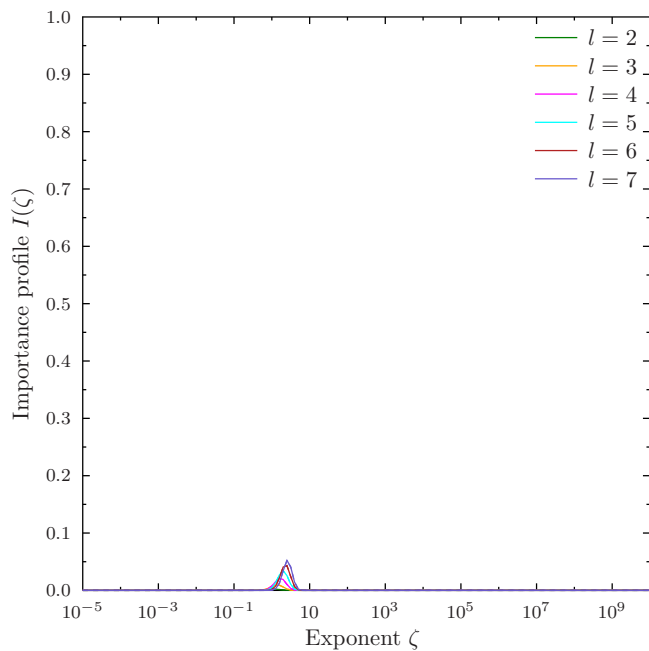

Figure 160. STO importance profile for  $\delta_-$  orbitals on O atom in GeO.

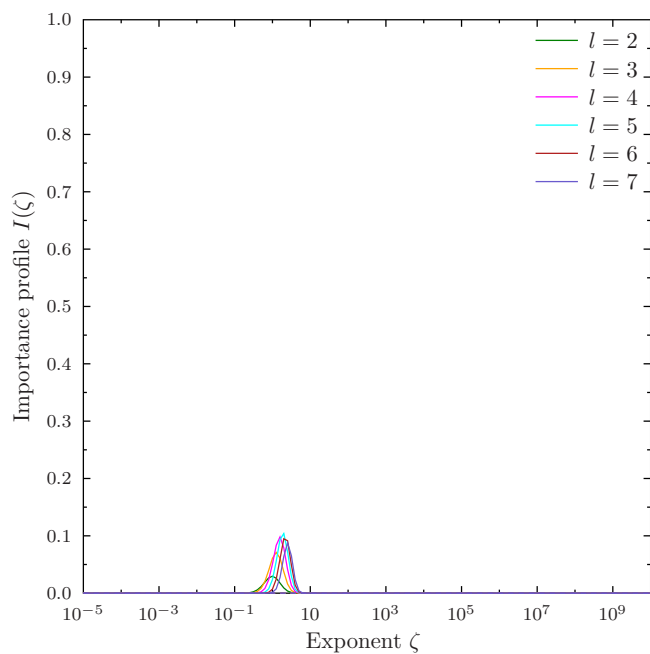

Figure 161. STO importance profile for  $\delta_-$  orbitals on O atom in MnO.

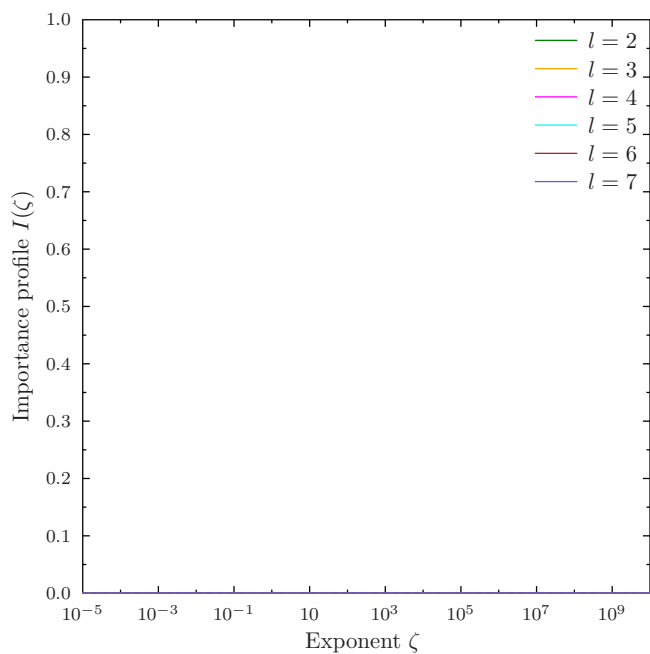

Figure 163. STO importance profile for  $\delta_-$  orbitals on O atom in ScO.

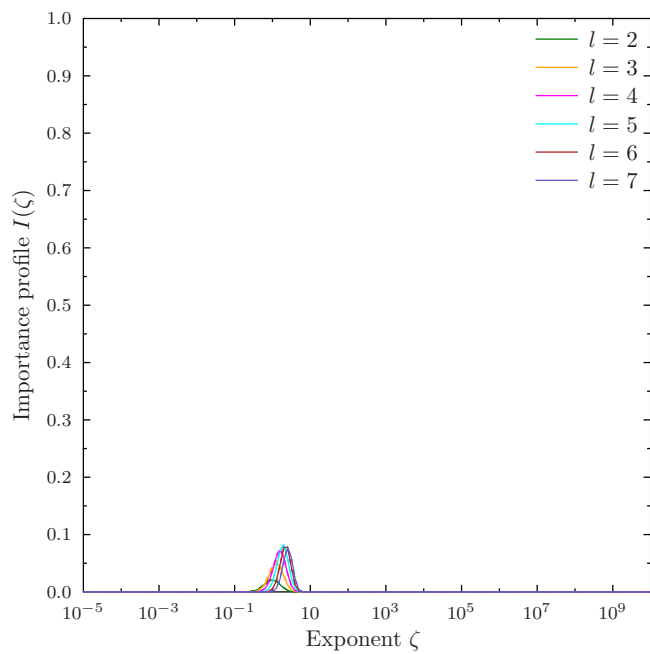

Figure 162. STO importance profile for  $\delta_-$  orbitals on O atom in NiO.

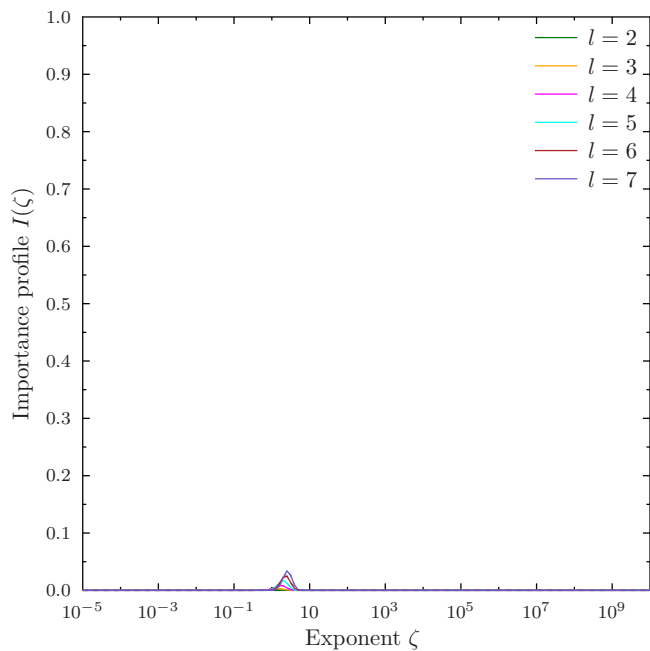

Figure 164. STO importance profile for  $\delta_-$  orbitals on O atom in SeO.

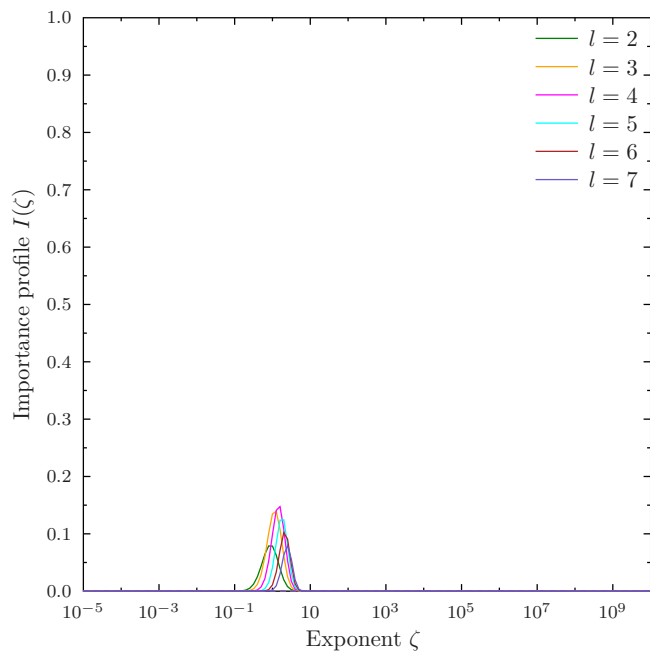

Figure 165. STO importance profile for  $\delta_-$  orbitals on O atom in TiO.

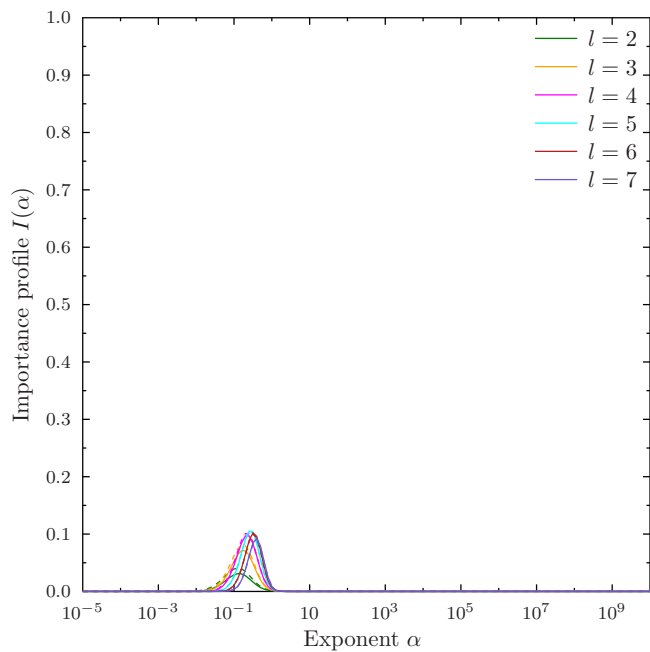

Figure 167. GTO importance profile for  $\delta_+$  orbitals on O atom in FeO.

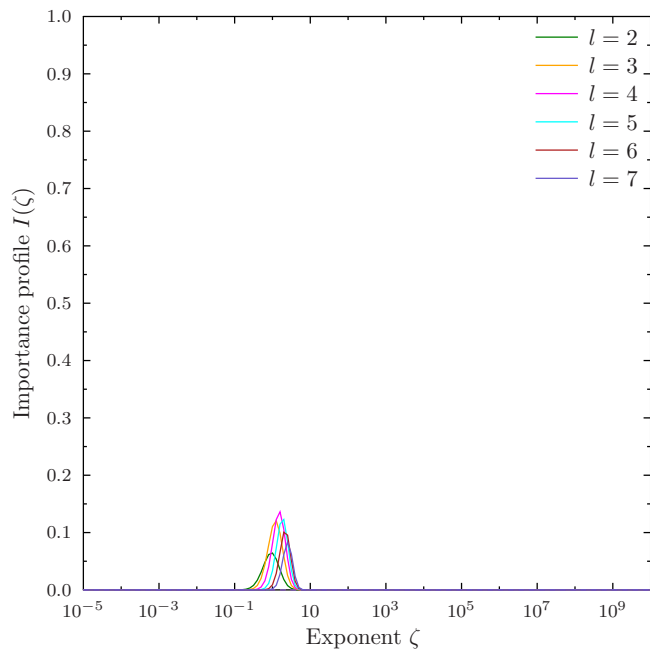

Figure 166. STO importance profile for  $\delta_-$  orbitals on O atom in VO.

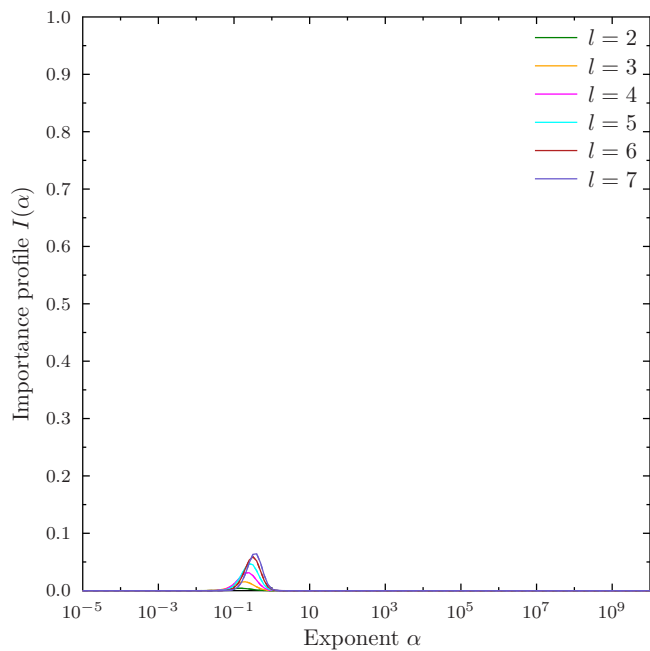

Figure 168. GTO importance profile for  $\delta_+$  orbitals on O atom in GaO.

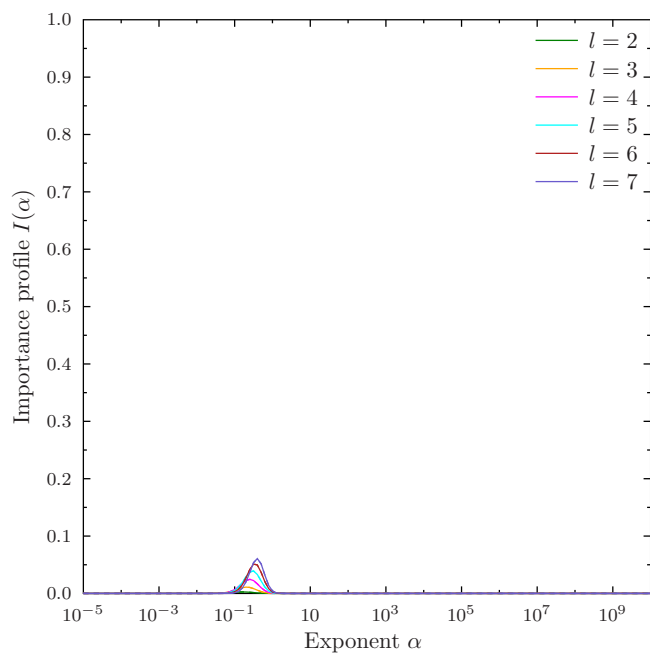

Figure 169. GTO importance profile for  $\delta_+$  orbitals on O atom in GeO.

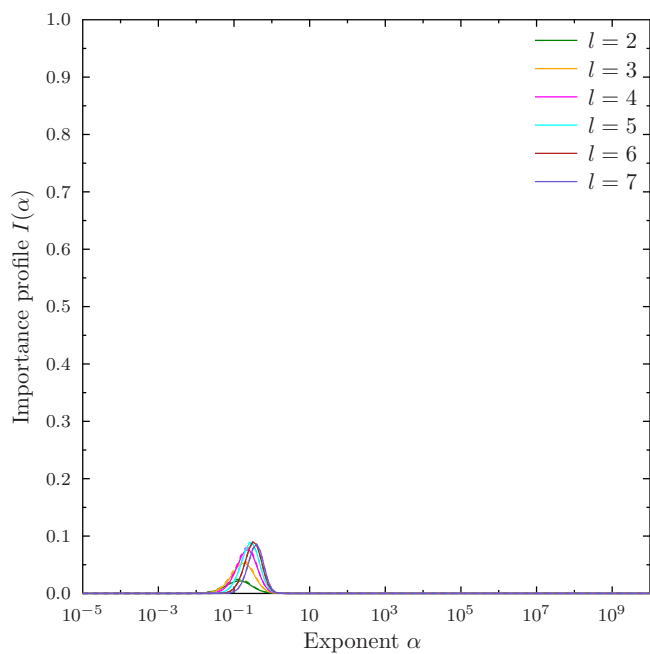

Figure 171. GTO importance profile for  $\delta_+$  orbitals on O atom in NiO.

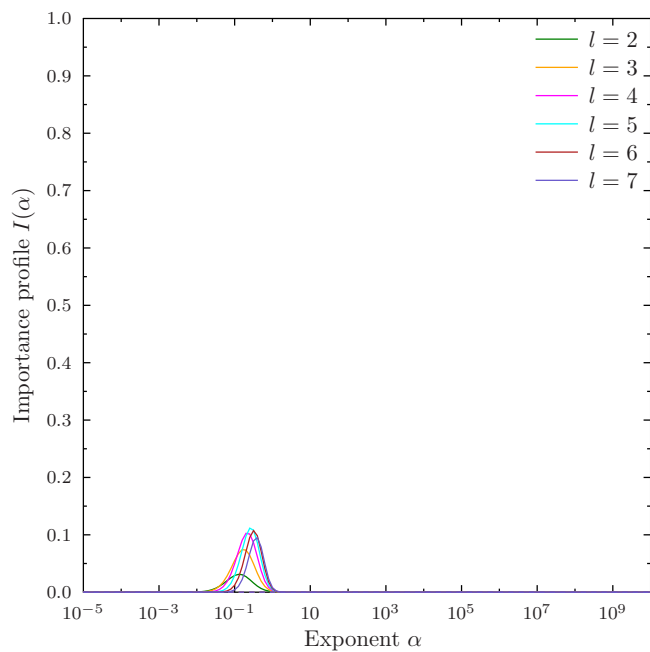

Figure 170. GTO importance profile for  $\delta_+$  orbitals on O atom in MnO.

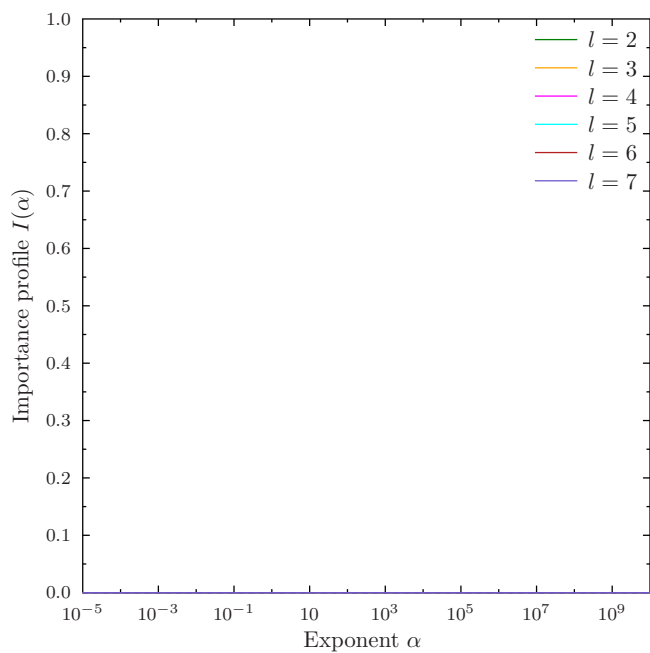

Figure 172. GTO importance profile for  $\delta_+$  orbitals on O atom in ScO.

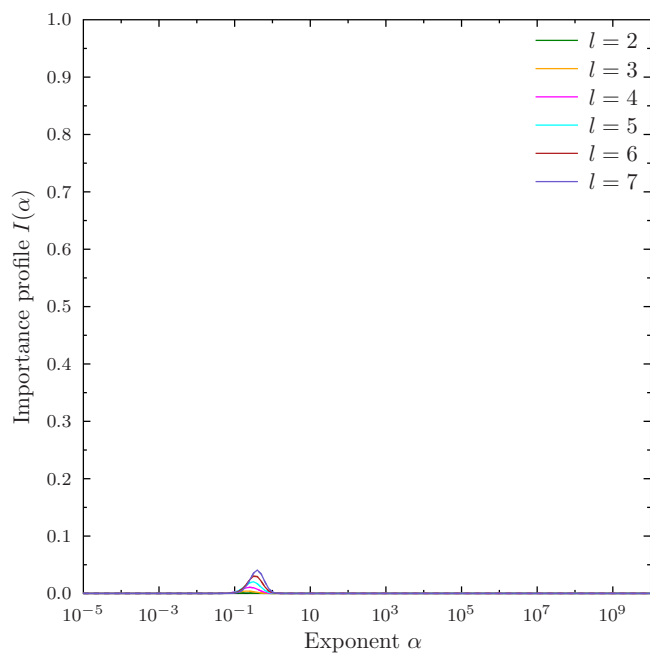

Figure 173. GTO importance profile for  $\delta_+$  orbitals on O atom in SeO.

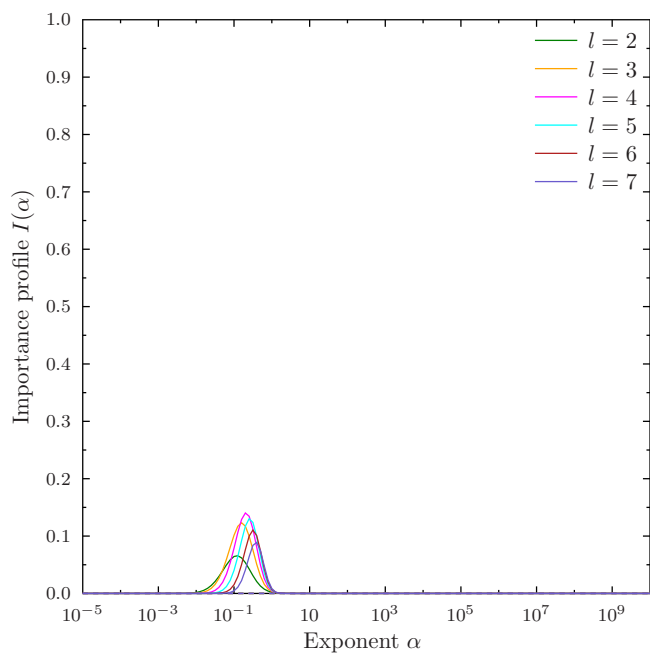

Figure 175. GTO importance profile for  $\delta_+$  orbitals on O atom in VO.

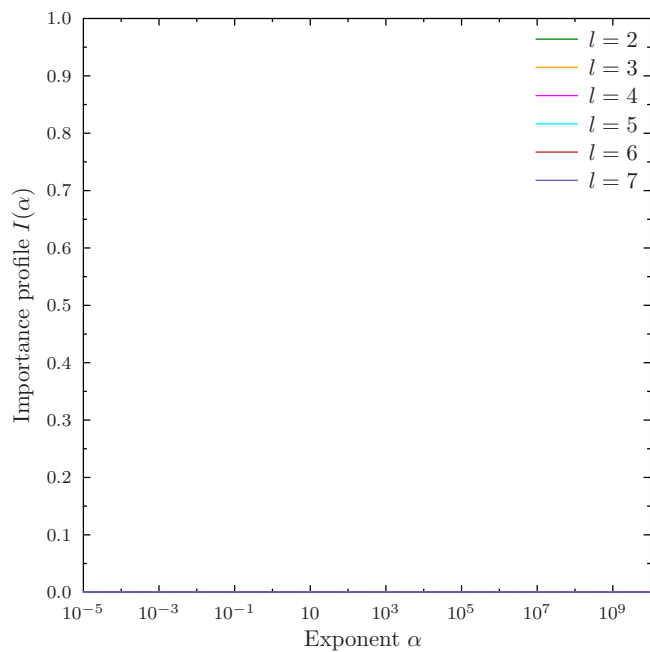

Figure 174. GTO importance profile for  $\delta_+$  orbitals on O atom in TiO.

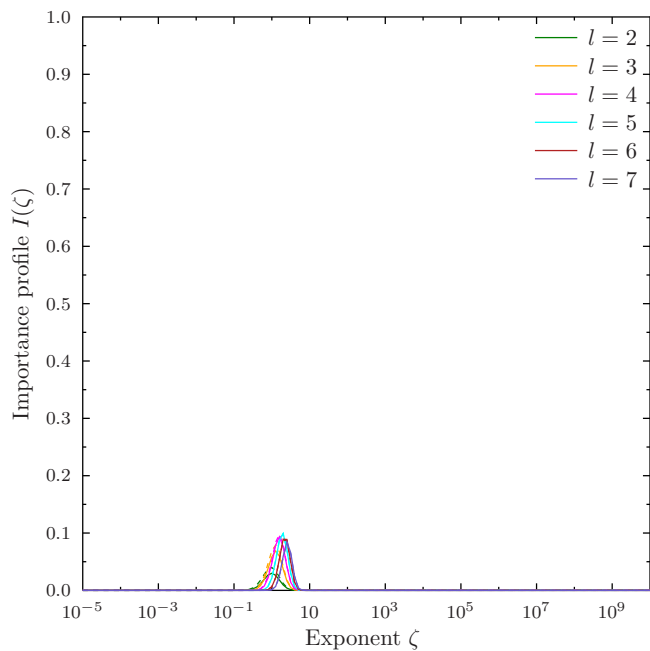

Figure 176. STO importance profile for  $\delta_+$  orbitals on O atom in FeO.



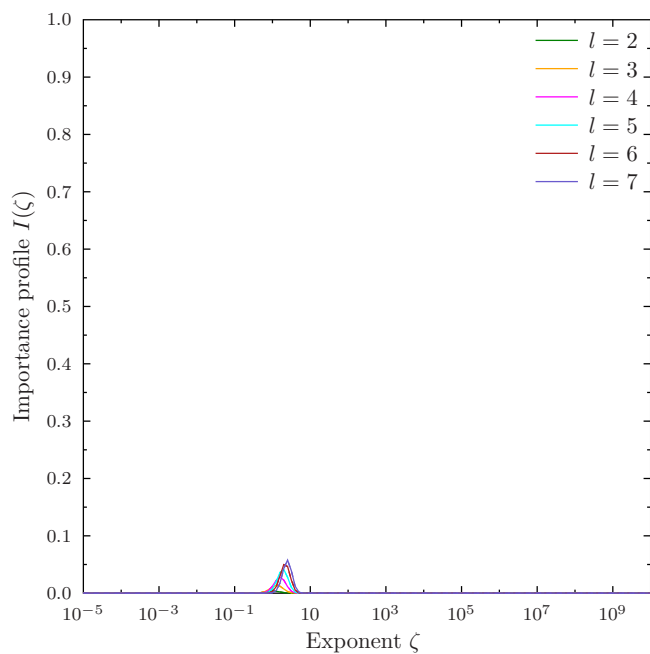

Figure 177. STO importance profile for  $\delta_+$  orbitals on O atom in GaO.

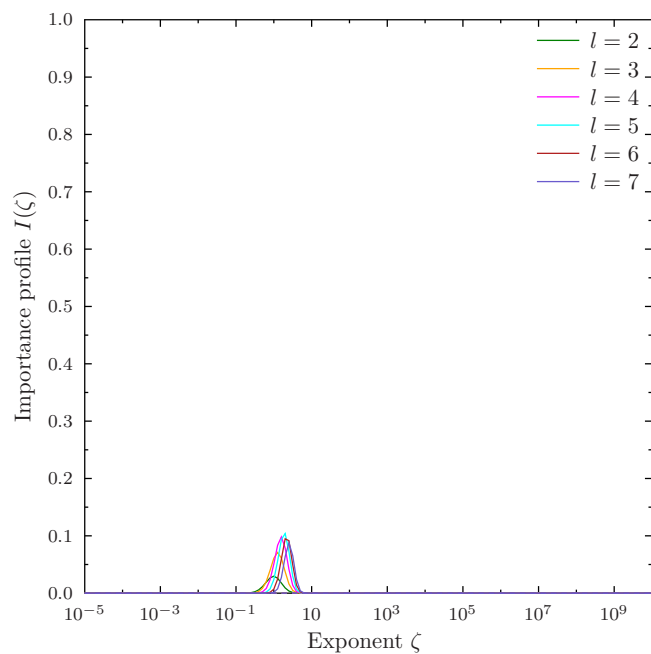

Figure 179. STO importance profile for  $\delta_+$  orbitals on O atom in MnO.

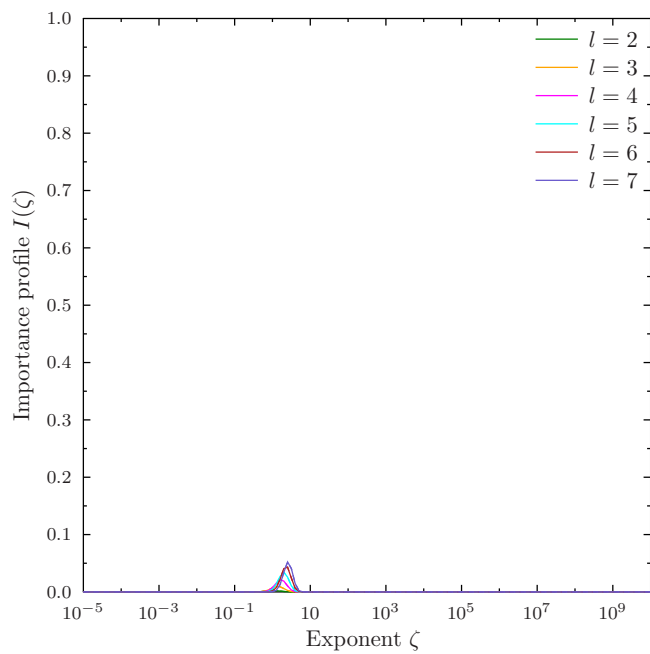

Figure 178. STO importance profile for  $\delta_+$  orbitals on O atom in GeO.

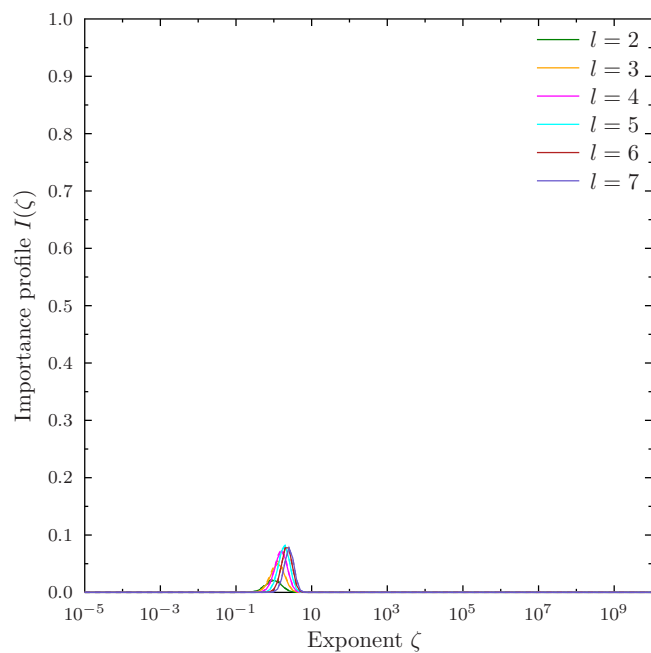

Figure 180. STO importance profile for  $\delta_+$  orbitals on O atom in NiO.

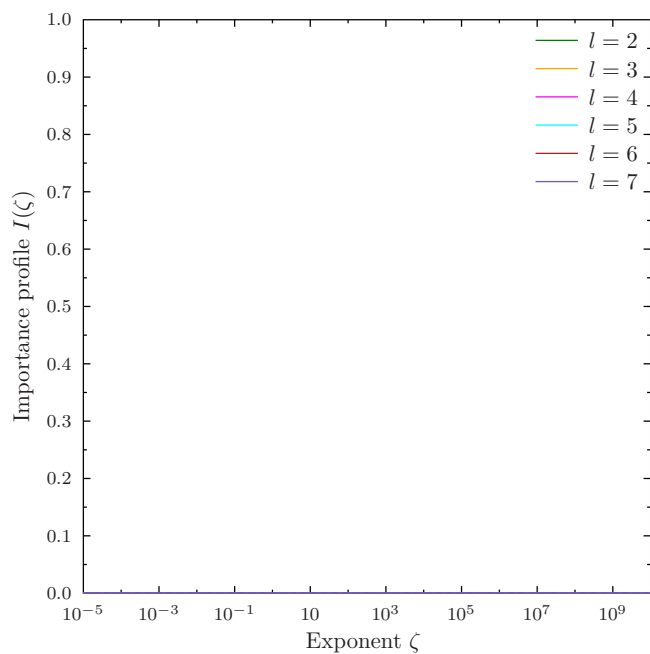

Figure 181. STO importance profile for  $\delta_+$  orbitals on O atom in ScO.

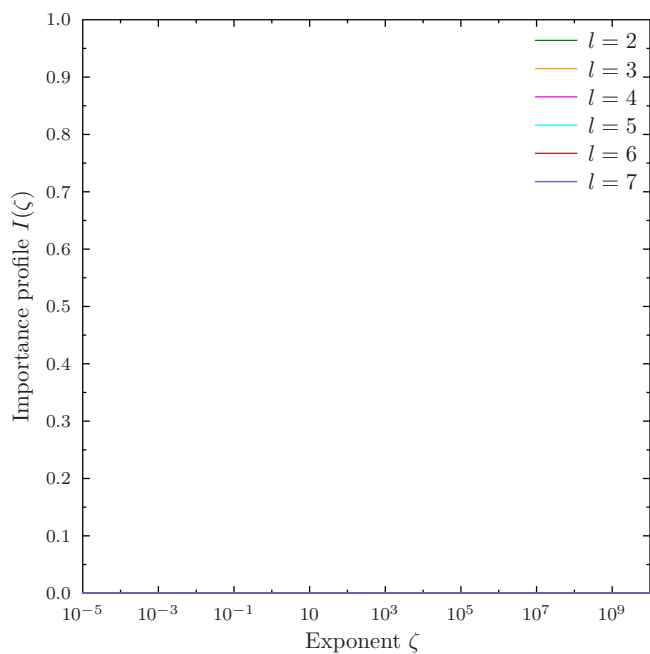

Figure 183. STO importance profile for  $\delta_+$  orbitals on O atom in TiO.

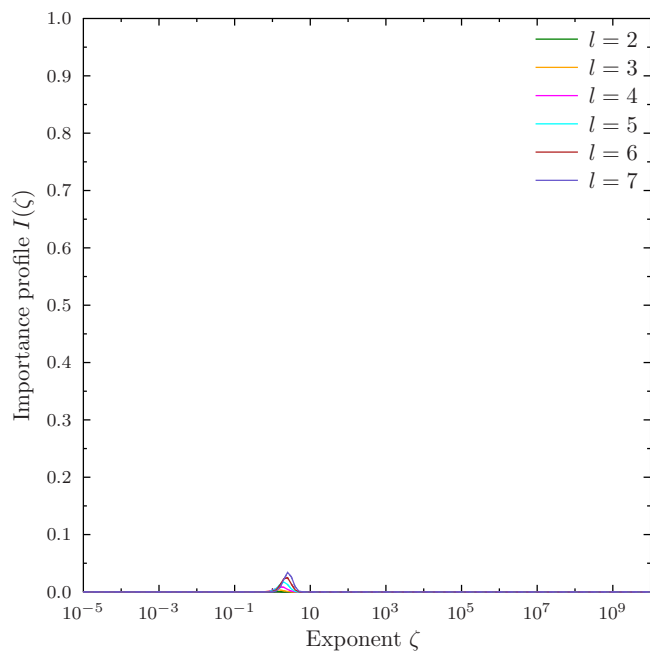

Figure 182. STO importance profile for  $\delta_+$  orbitals on O atom in SeO.

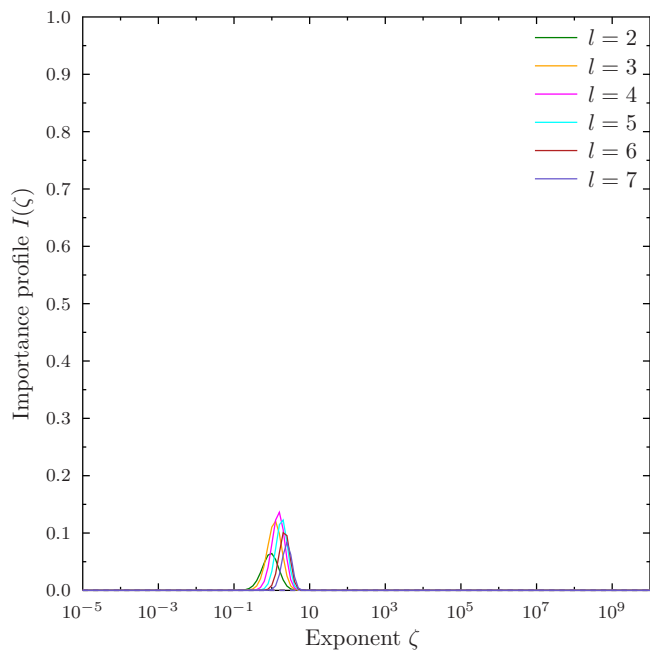

Figure 184. STO importance profile for  $\delta_+$  orbitals on O atom in VO.

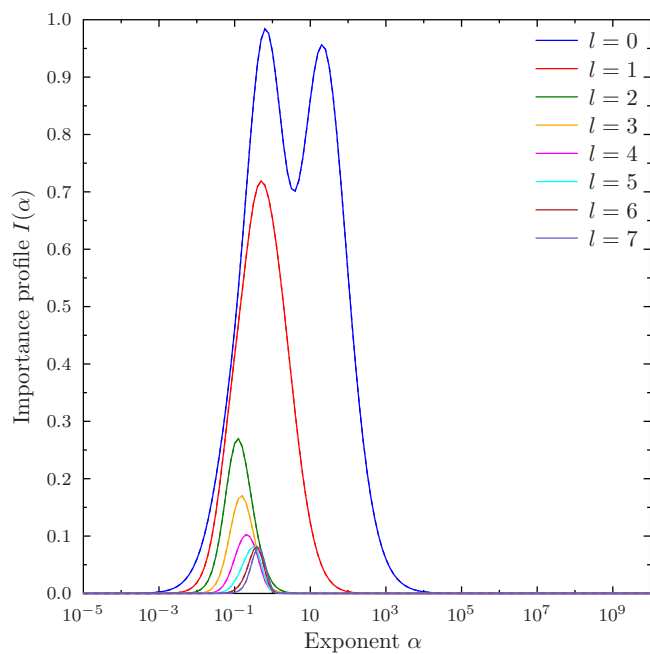

Figure 185. GTO importance profile for  $\sigma$  orbitals on F atom in ClF.

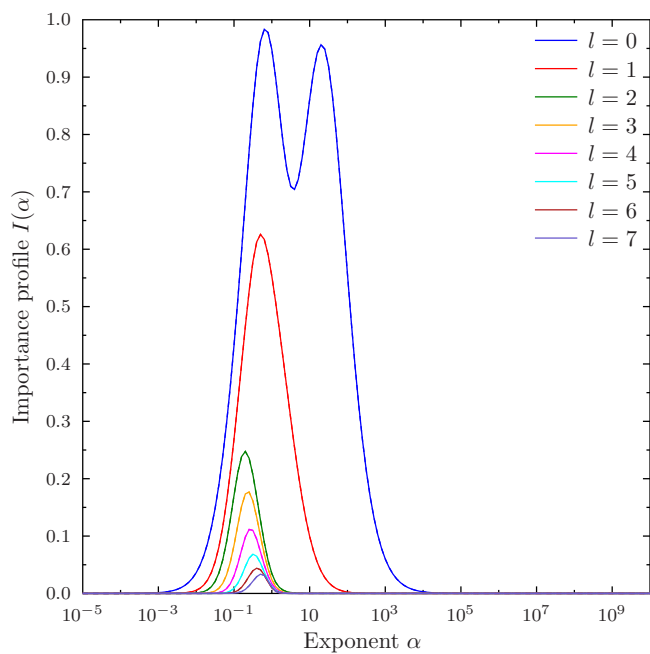

Figure 187. GTO importance profile for  $\sigma$  orbitals on F atom in  $F_2$ .

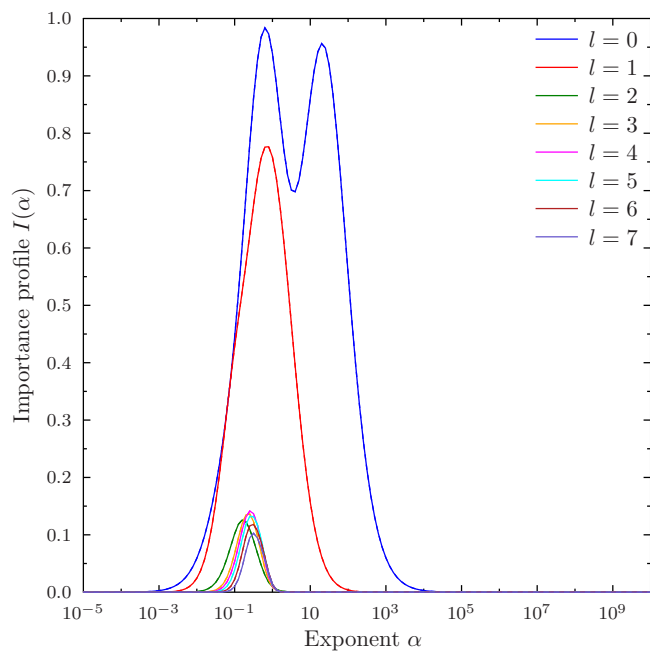

Figure 186. GTO importance profile for  $\sigma$  orbitals on F atom in CuF.

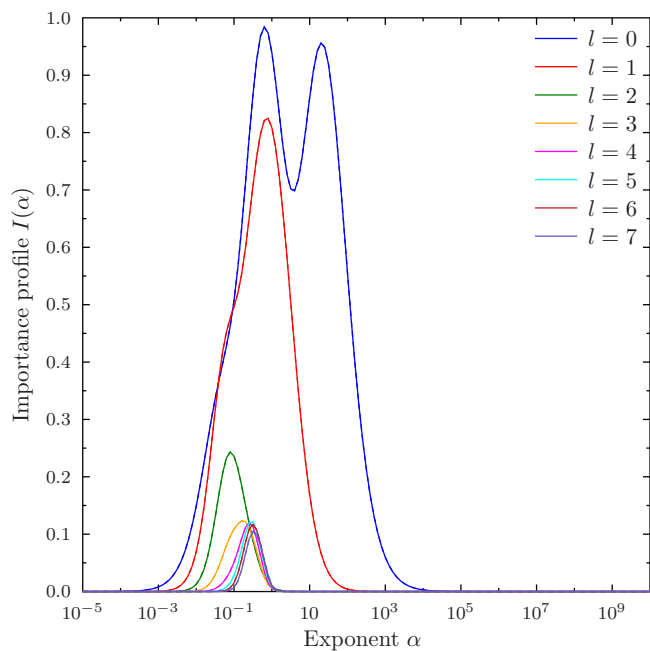

Figure 188. GTO importance profile for  $\sigma$  orbitals on F atom in GaF.

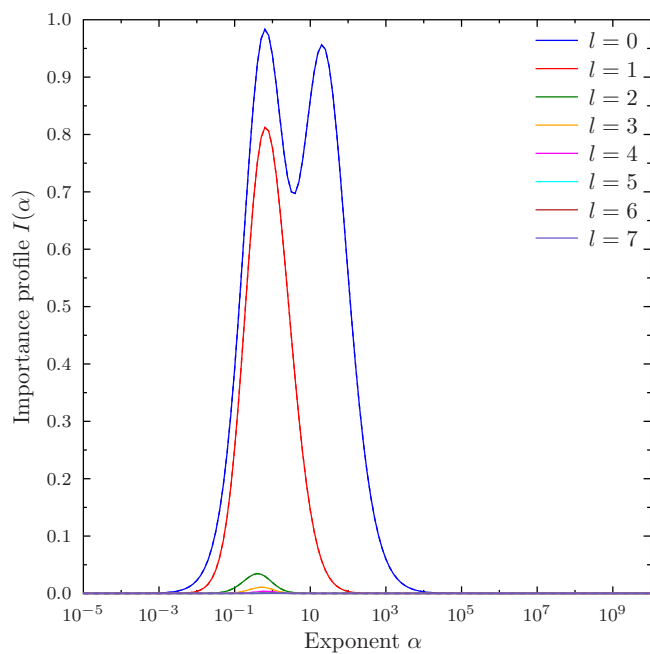

Figure 189. GTO importance profile for  $\sigma$  orbitals on F atom in HF.

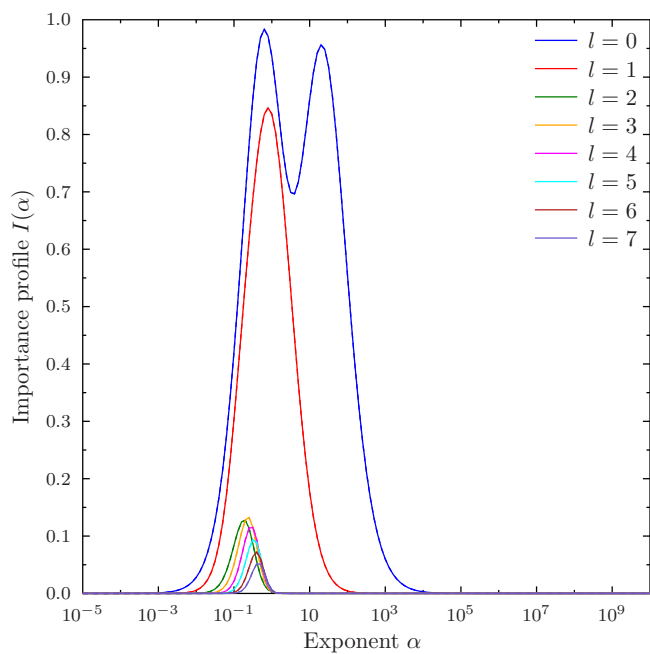

Figure 191. GTO importance profile for  $\sigma$  orbitals on F atom in LiF.

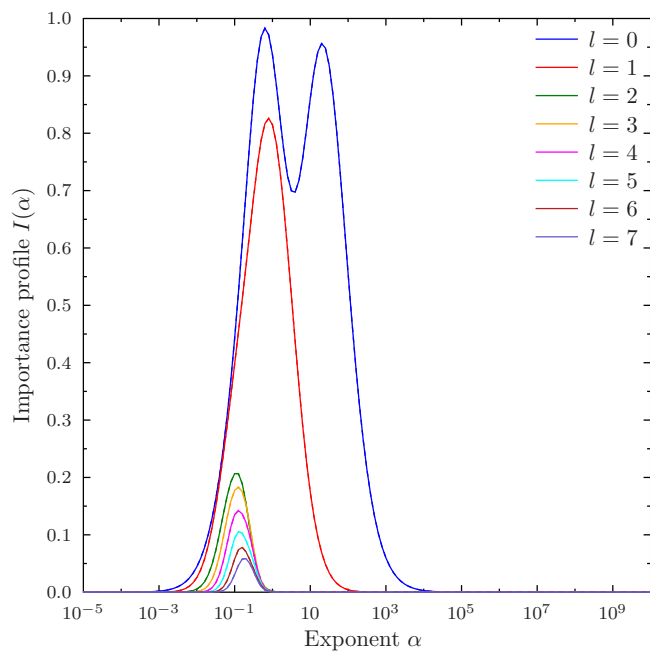

Figure 190. GTO importance profile for  $\sigma$  orbitals on F atom in KF.

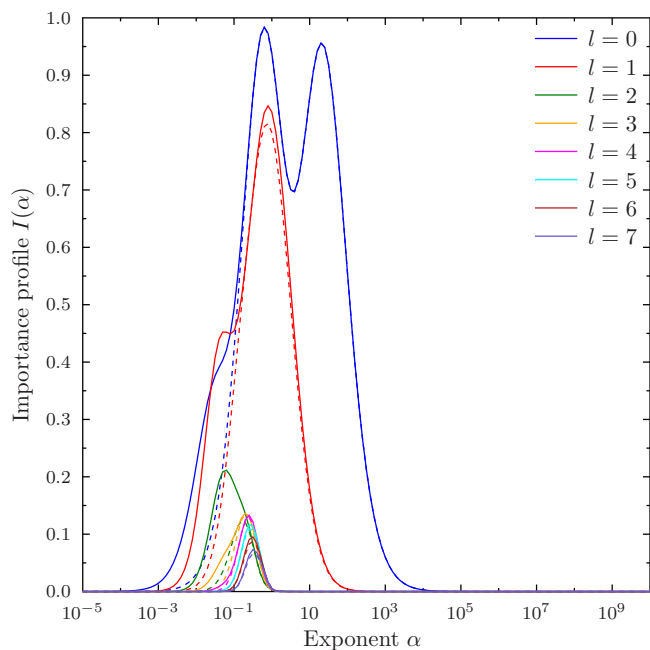

Figure 192. GTO importance profile for  $\sigma$  orbitals on F atom in MgF.

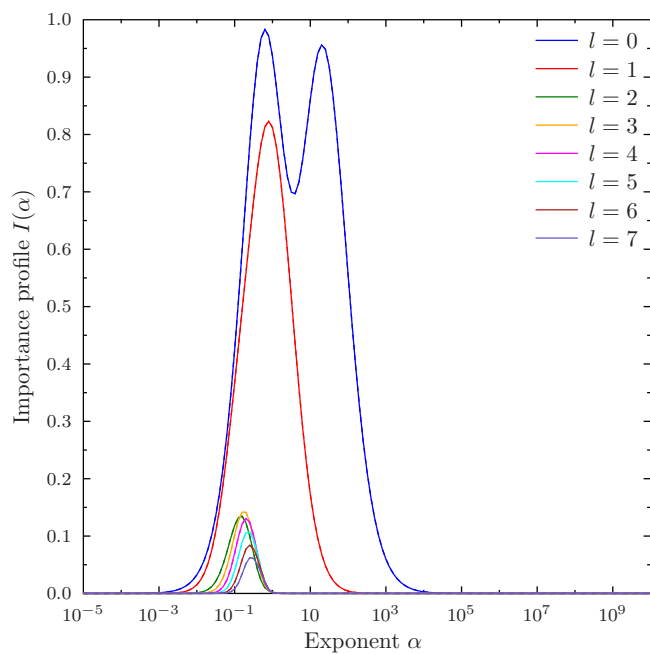

Figure 193. GTO importance profile for  $\sigma$  orbitals on F atom in NaF.

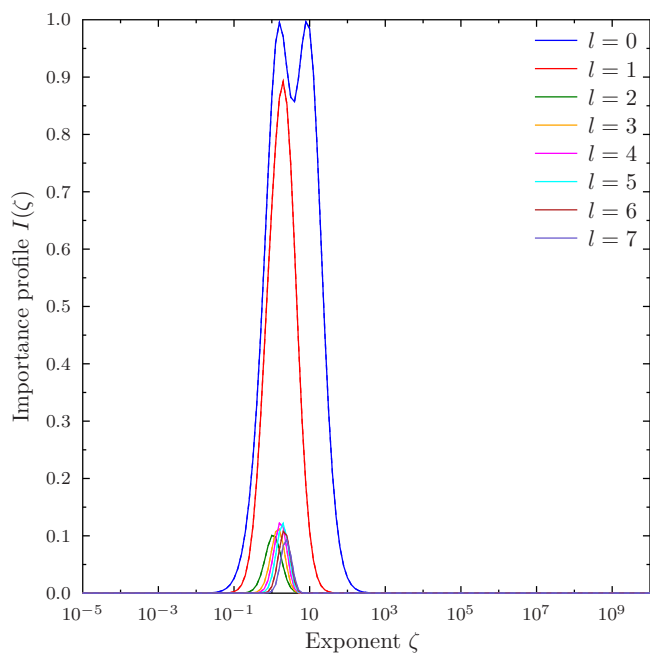

Figure 195. STO importance profile for  $\sigma$  orbitals on F atom in CuF.

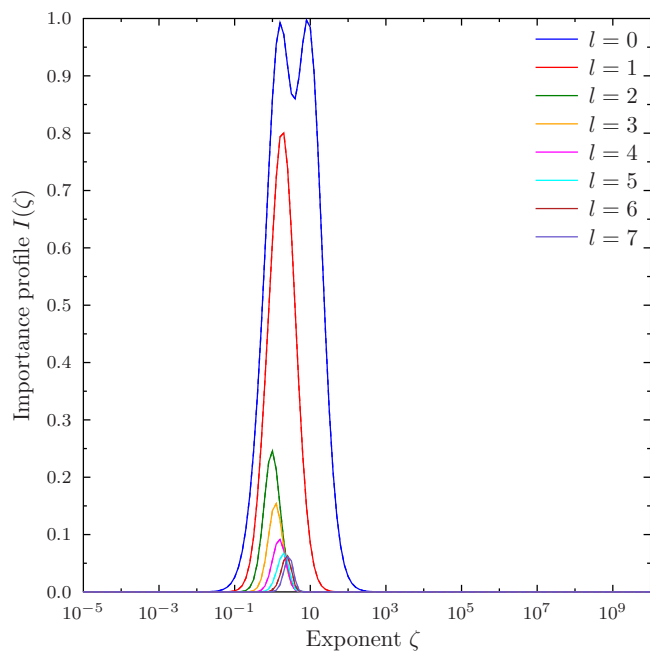

Figure 194. STO importance profile for  $\sigma$  orbitals on F atom in ClF.

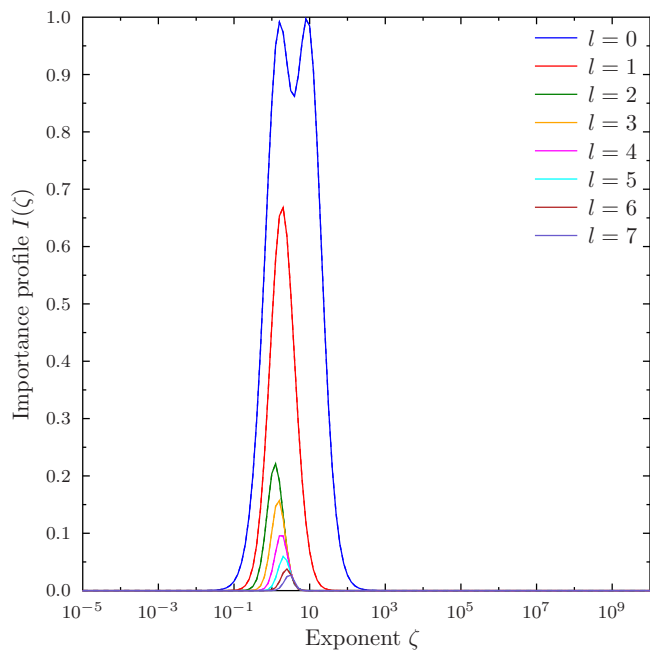

Figure 196. STO importance profile for  $\sigma$  orbitals on F atom in  $F_2$ .

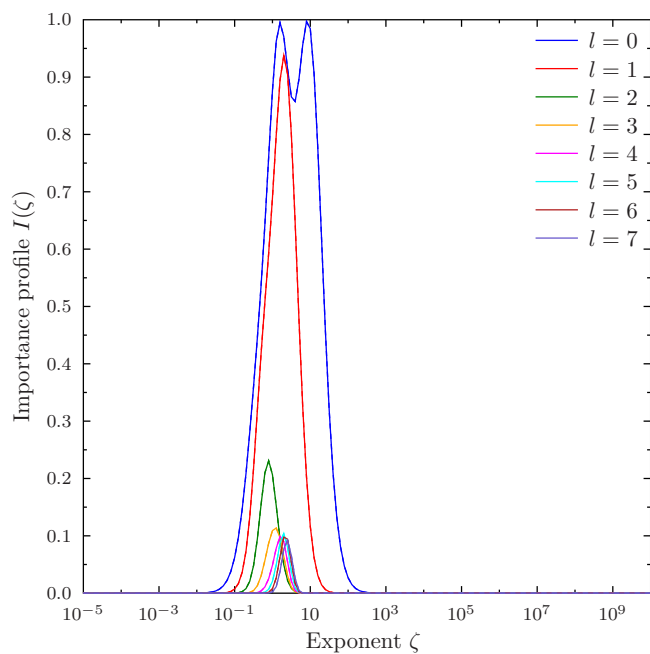

Figure 197. STO importance profile for  $\sigma$  orbitals on F atom in GaF.

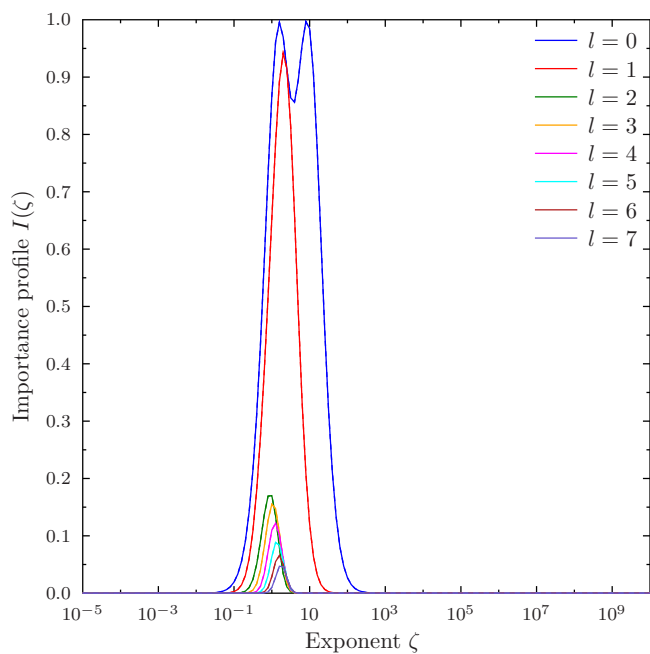

Figure 199. STO importance profile for  $\sigma$  orbitals on F atom in KF.

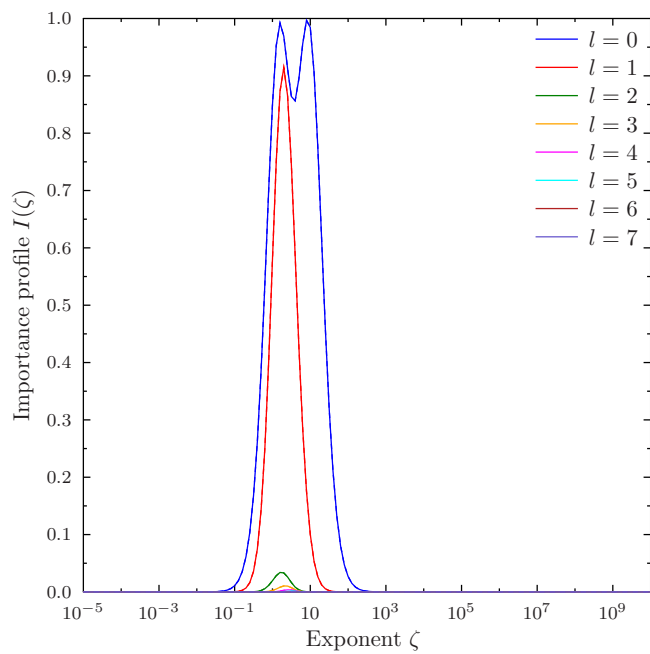

Figure 198. STO importance profile for  $\sigma$  orbitals on F atom in HF.

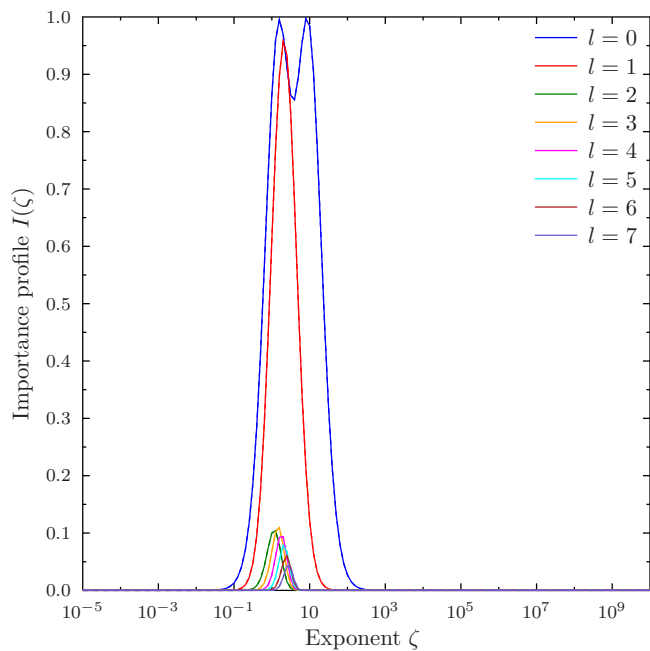

Figure 200. STO importance profile for  $\sigma$  orbitals on F atom in LiF.

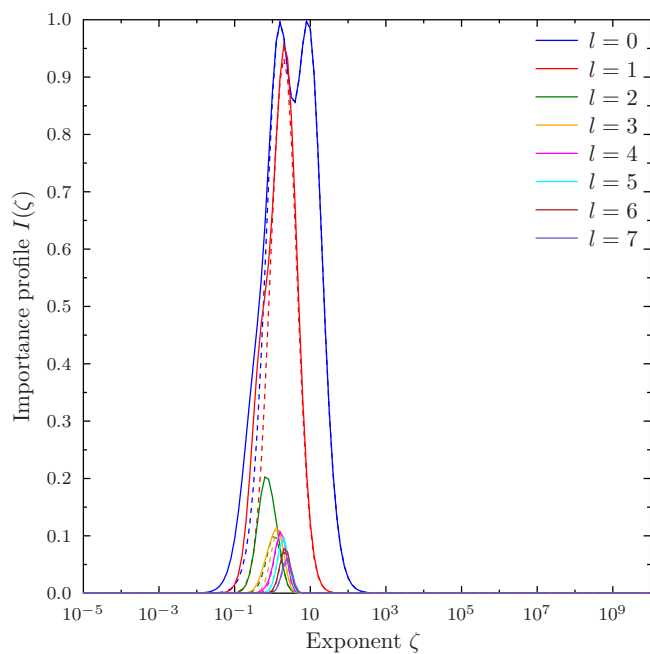

Figure 201. STO importance profile for  $\sigma$  orbitals on F atom in MgF.

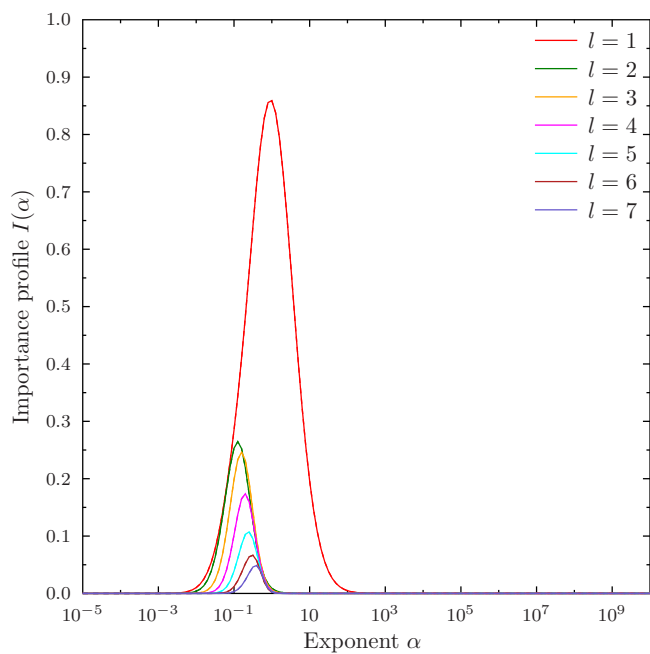

Figure 203. GTO importance profile for  $\pi_-$  orbitals on F atom in ClF.

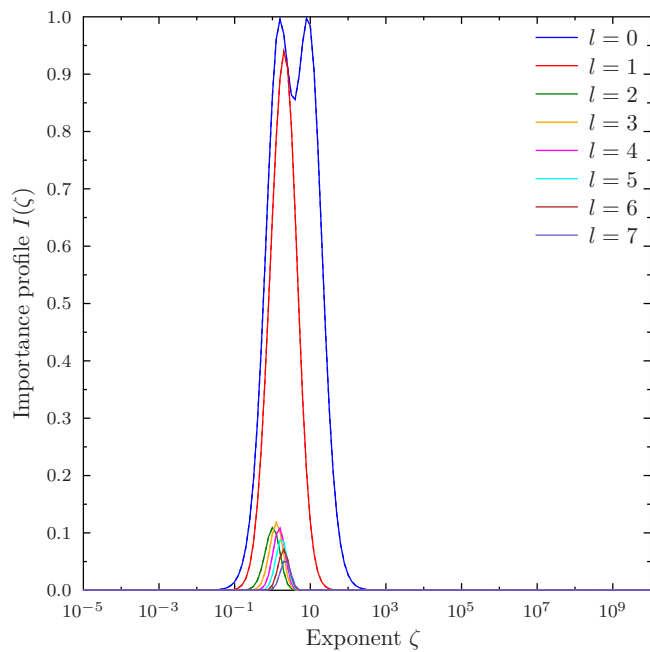

Figure 202. STO importance profile for  $\sigma$  orbitals on F atom in NaF.

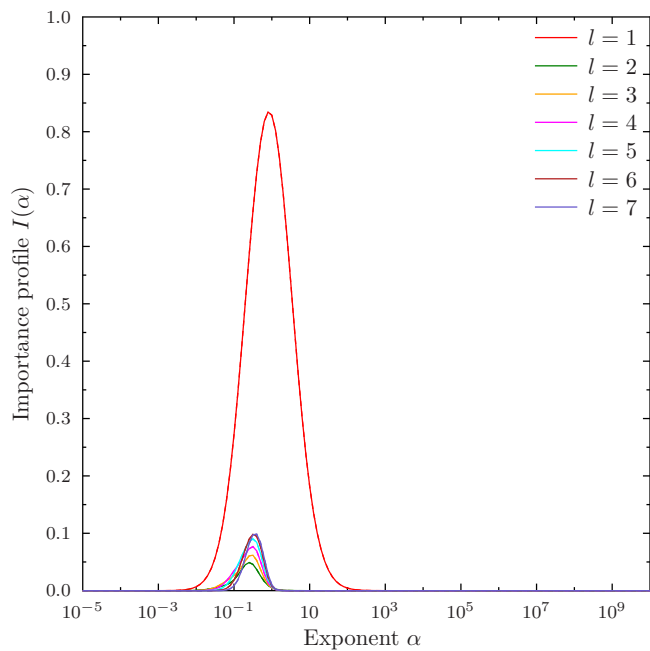

Figure 204. GTO importance profile for  $\pi_-$  orbitals on F atom in CuF.

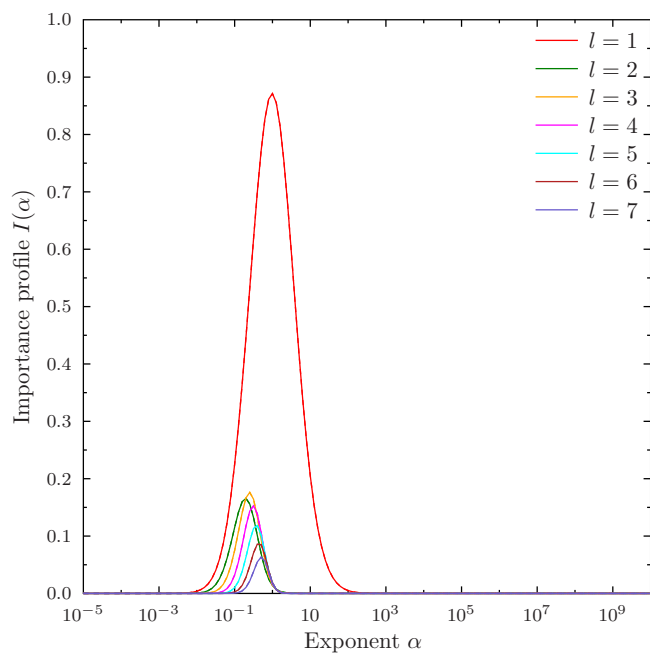

Figure 205. GTO importance profile for  $\pi_-$  orbitals on F atom in  $F_2$ .

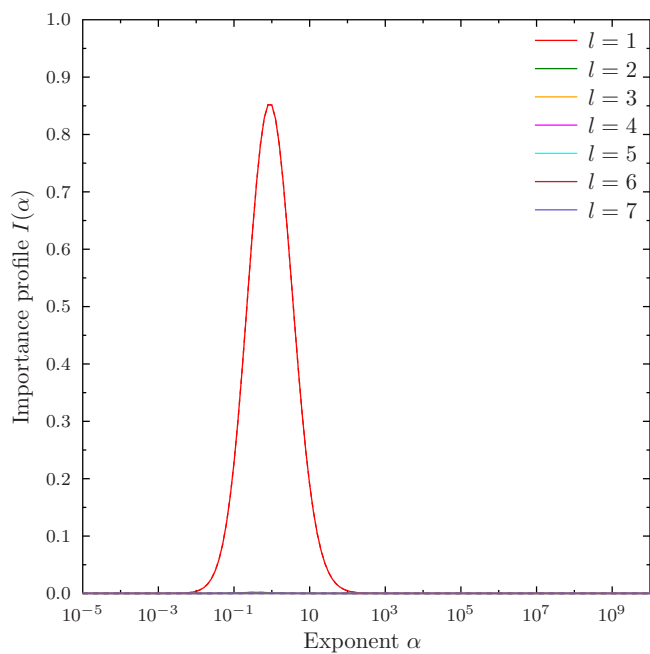

Figure 207. GTO importance profile for  $\pi_-$  orbitals on F atom in HF.

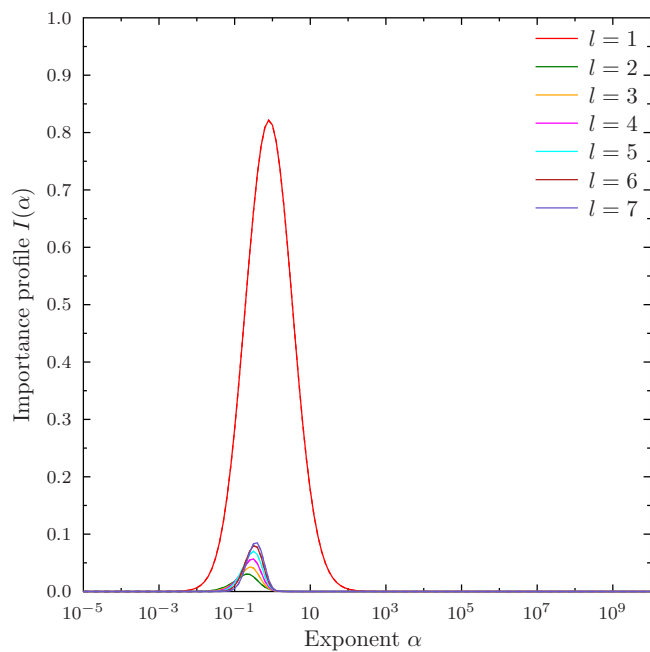

Figure 206. GTO importance profile for  $\pi_-$  orbitals on F atom in GaF.

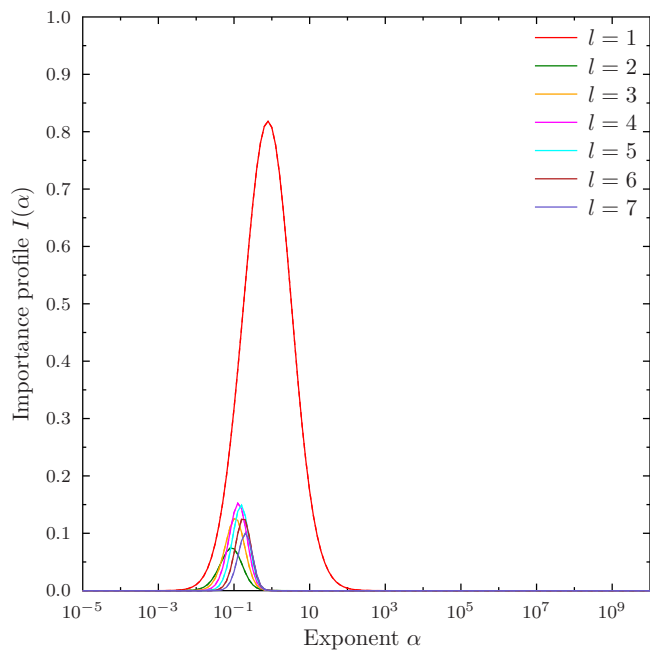

Figure 208. GTO importance profile for  $\pi_-$  orbitals on F atom in KF.



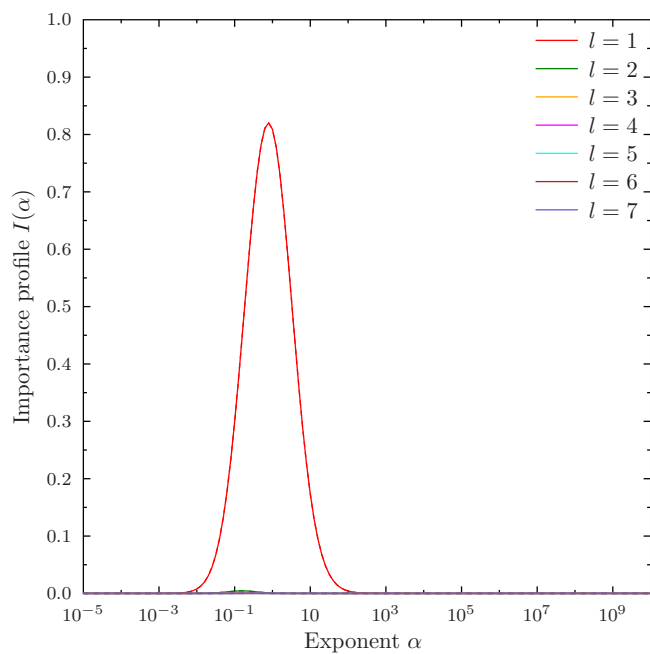

Figure 209. GTO importance profile for  $\pi_-$  orbitals on F atom in LiF.

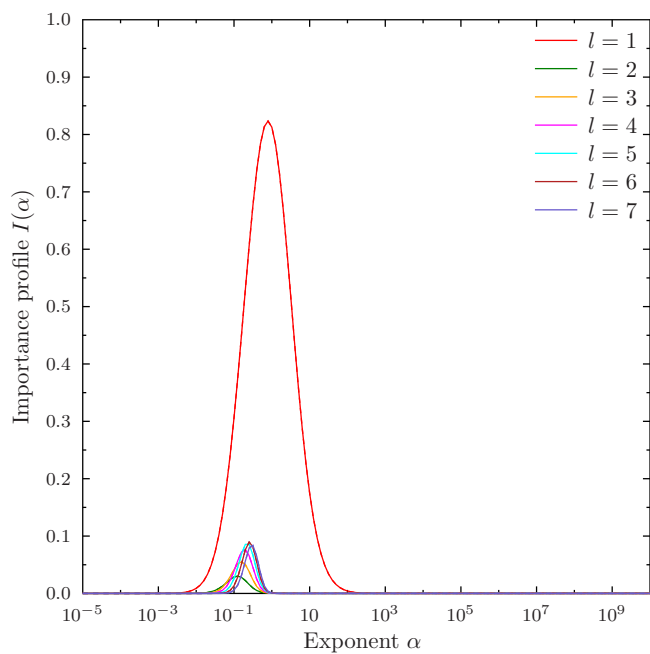

Figure 211. GTO importance profile for  $\pi_-$  orbitals on F atom in NaF.

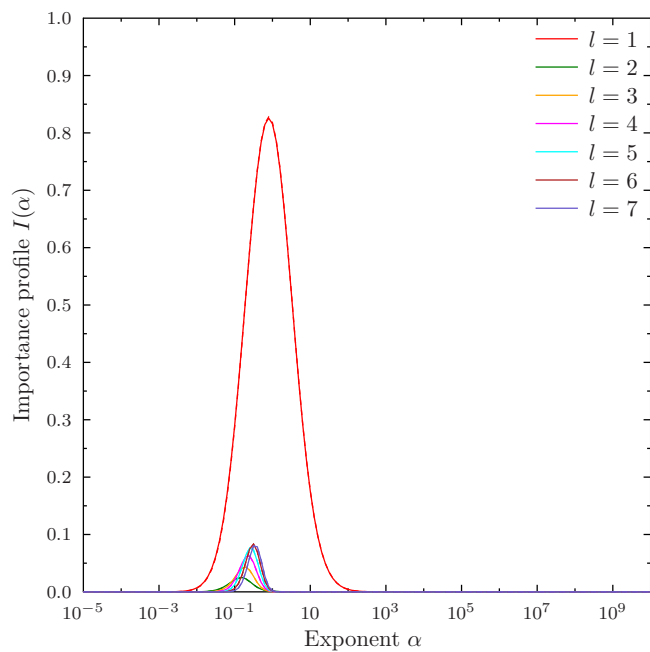

Figure 210. GTO importance profile for  $\pi_-$  orbitals on F atom in MgF.

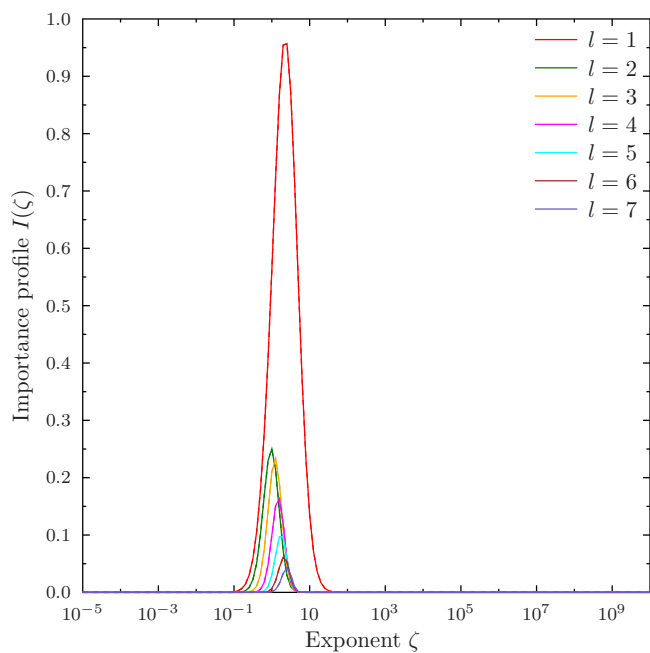

Figure 212. STO importance profile for  $\pi_-$  orbitals on F atom in ClF.

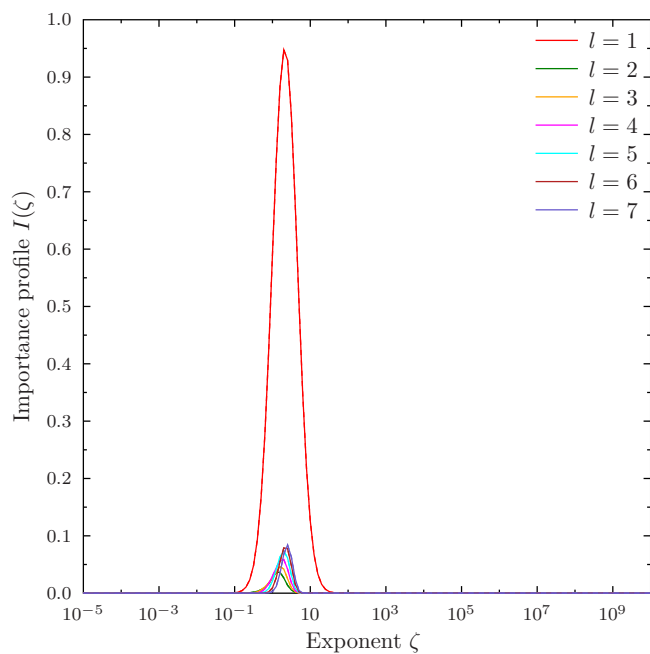

Figure 213. STO importance profile for  $\pi_-$  orbitals on F atom in CuF.

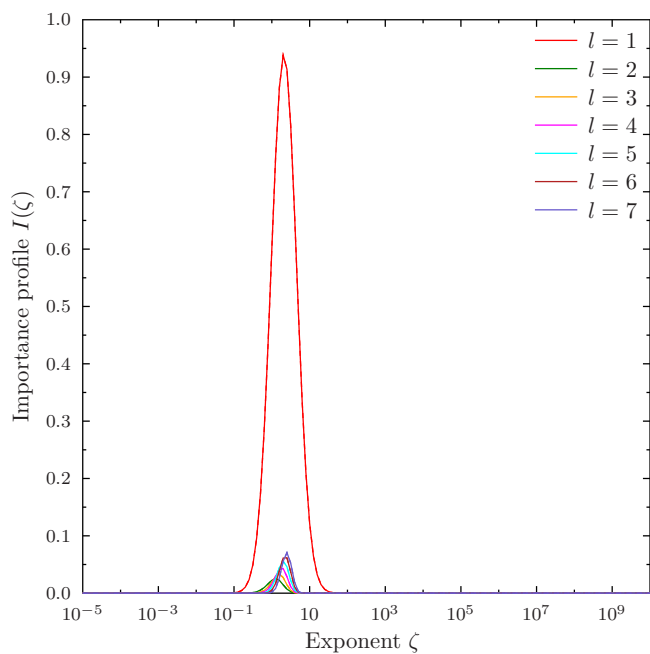

Figure 215. STO importance profile for  $\pi_-$  orbitals on F atom in GaF.

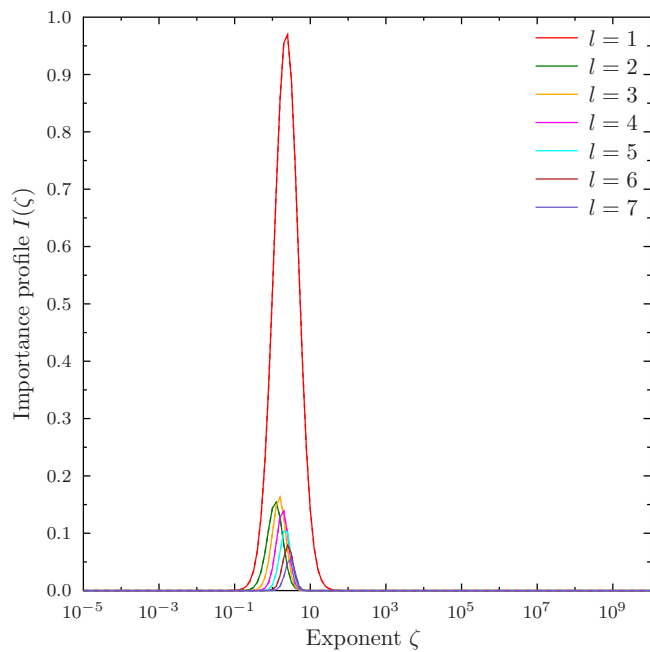

Figure 214. STO importance profile for  $\pi_-$  orbitals on F atom in  $F_2$ .

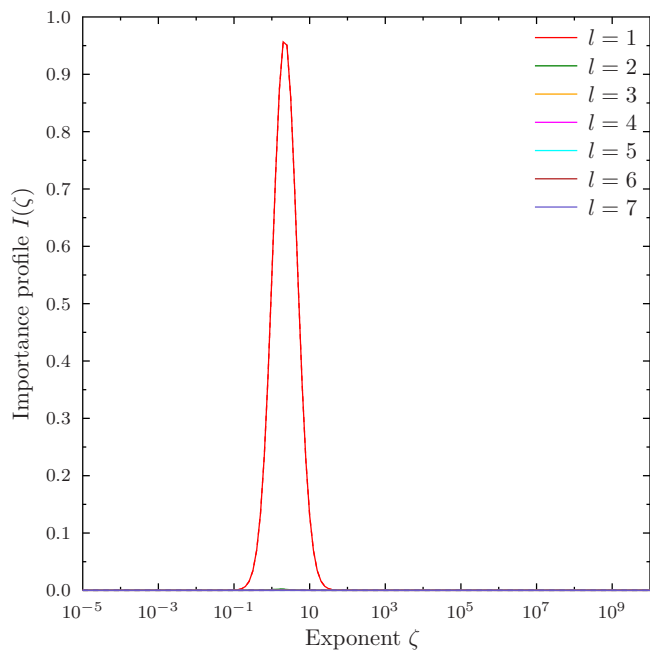

Figure 216. STO importance profile for  $\pi_-$  orbitals on F atom in HF.

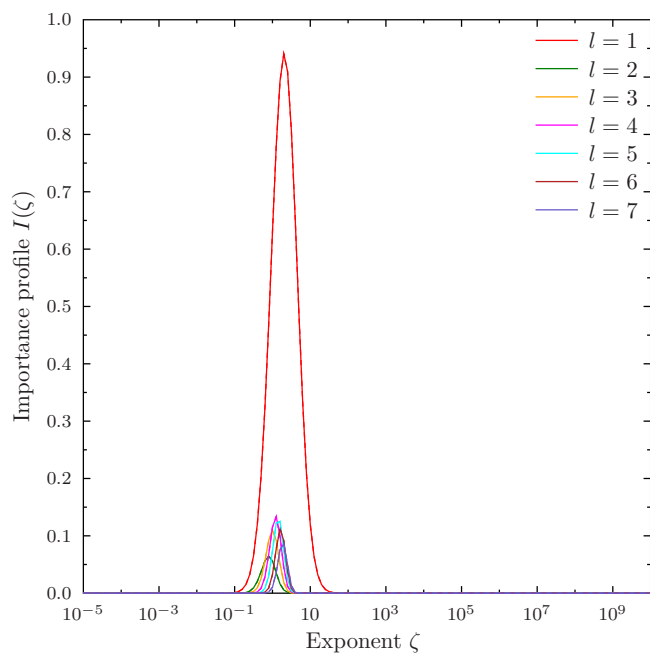

Figure 217. STO importance profile for  $\pi_-$  orbitals on F atom in KF.

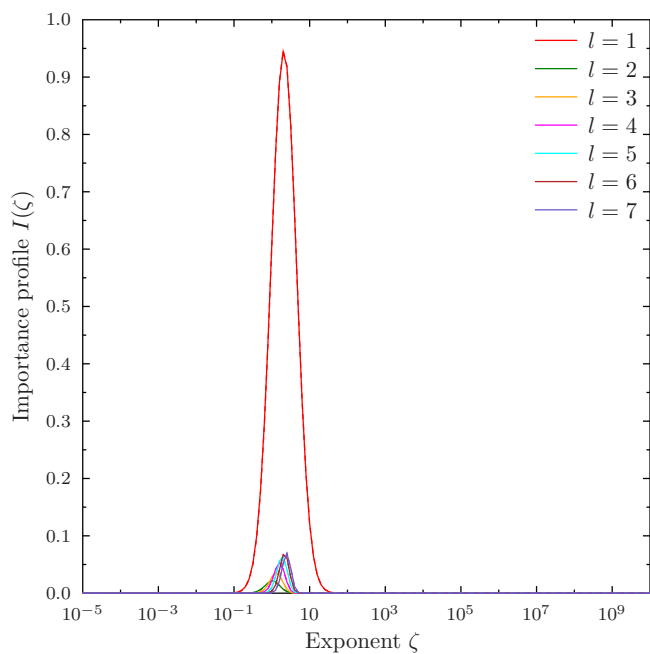

Figure 219. STO importance profile for  $\pi_-$  orbitals on F atom in MgF.

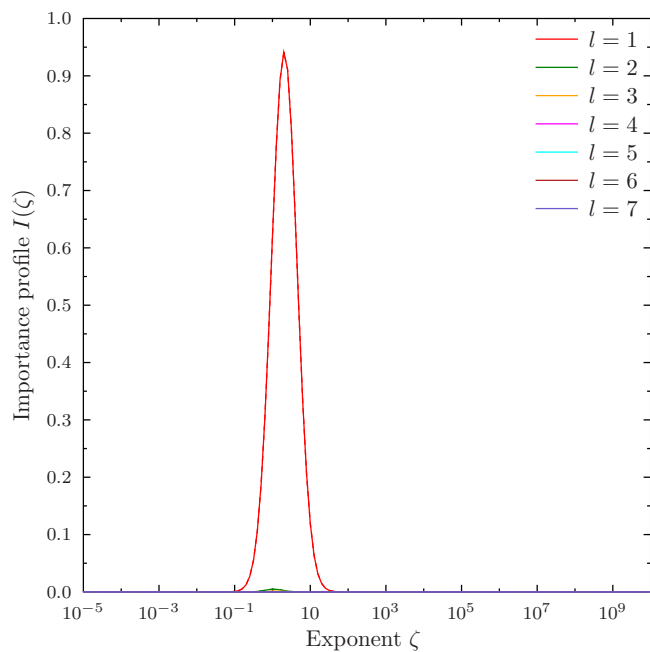

Figure 218. STO importance profile for  $\pi_-$  orbitals on F atom in LiF.

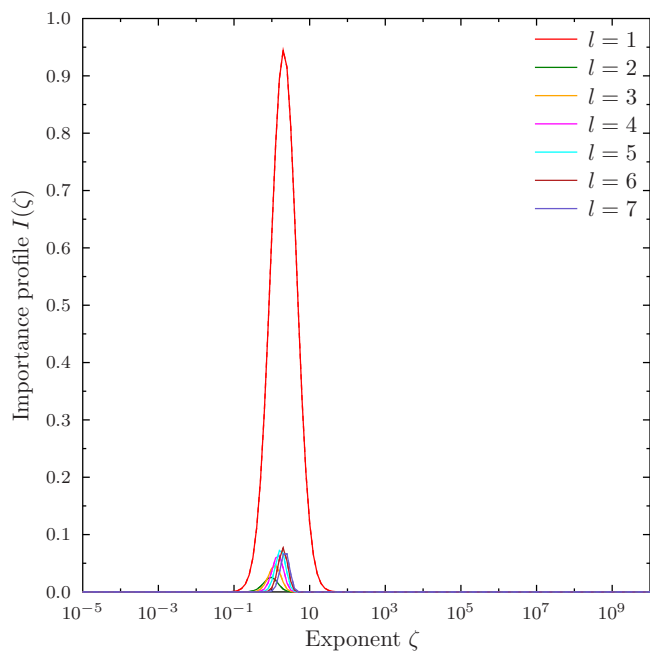

Figure 220. STO importance profile for  $\pi_-$  orbitals on F atom in NaF.

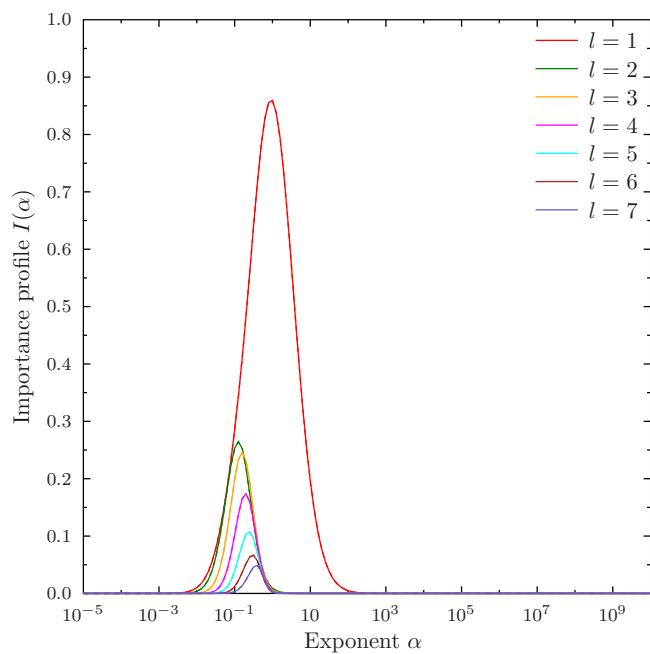

Figure 221. GTO importance profile for  $\pi_+$  orbitals on F atom in ClF.

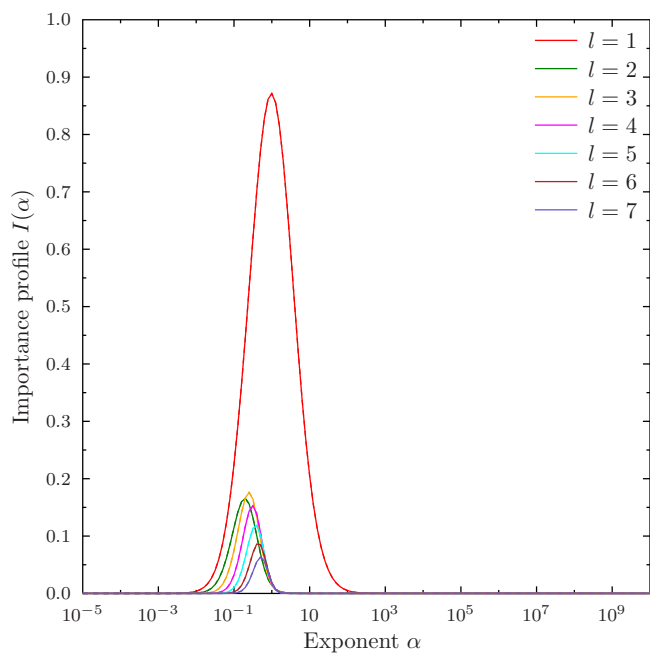

Figure 223. GTO importance profile for  $\pi_+$  orbitals on F atom in  $F_2$ .

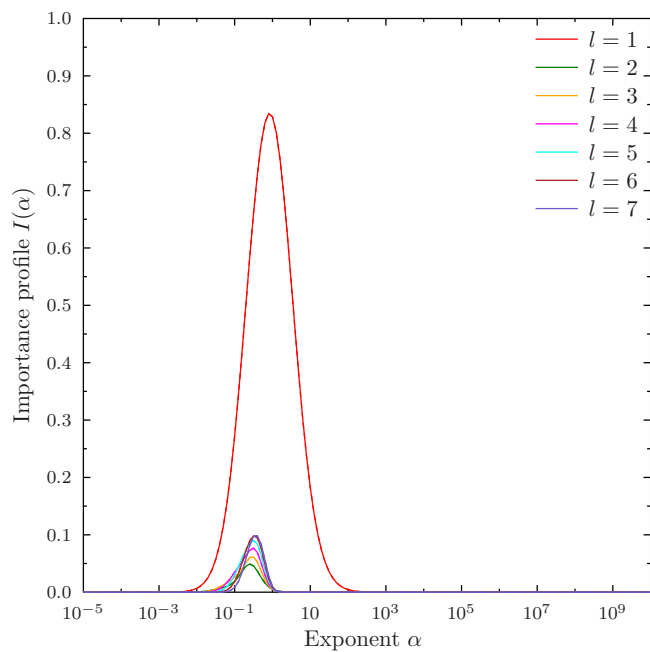

Figure 222. GTO importance profile for  $\pi_+$  orbitals on F atom in CuF.

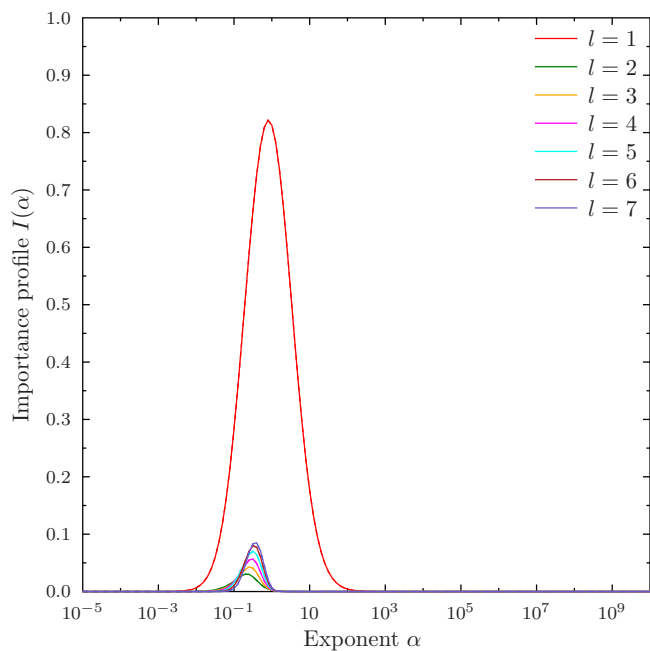

Figure 224. GTO importance profile for  $\pi_+$  orbitals on F atom in GaF.

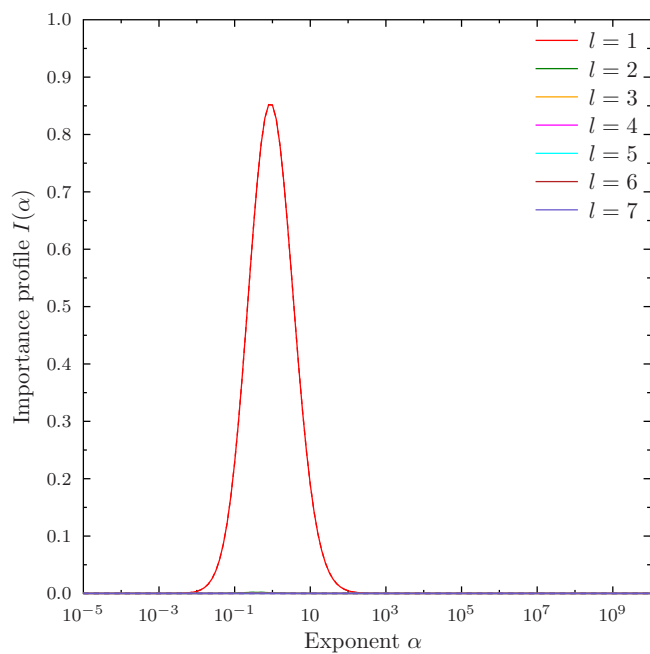

Figure 225. GTO importance profile for  $\pi_+$  orbitals on F atom in HF.

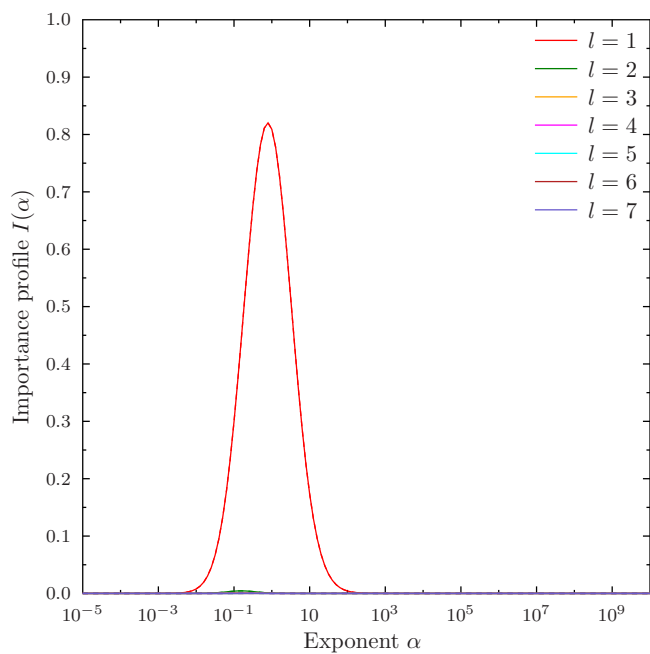

Figure 227. GTO importance profile for  $\pi_+$  orbitals on F atom in LiF.

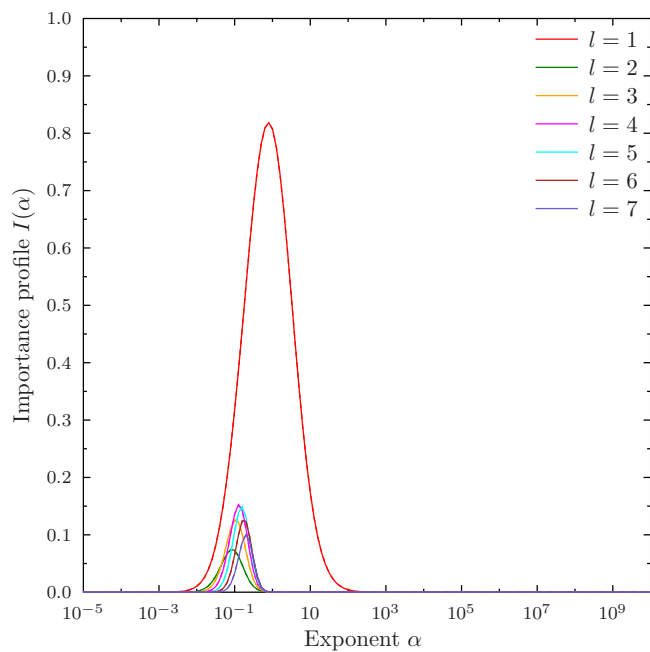

Figure 226. GTO importance profile for  $\pi_+$  orbitals on F atom in KF.

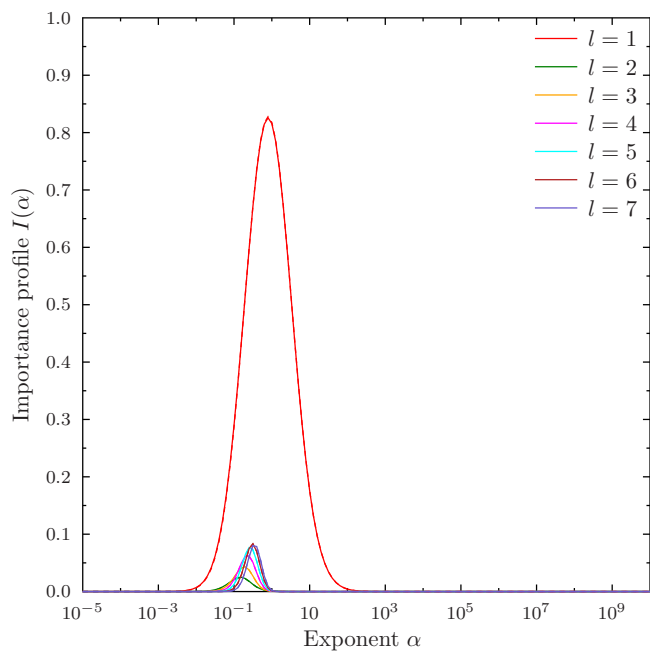

Figure 228. GTO importance profile for  $\pi_+$  orbitals on F atom in MgF.

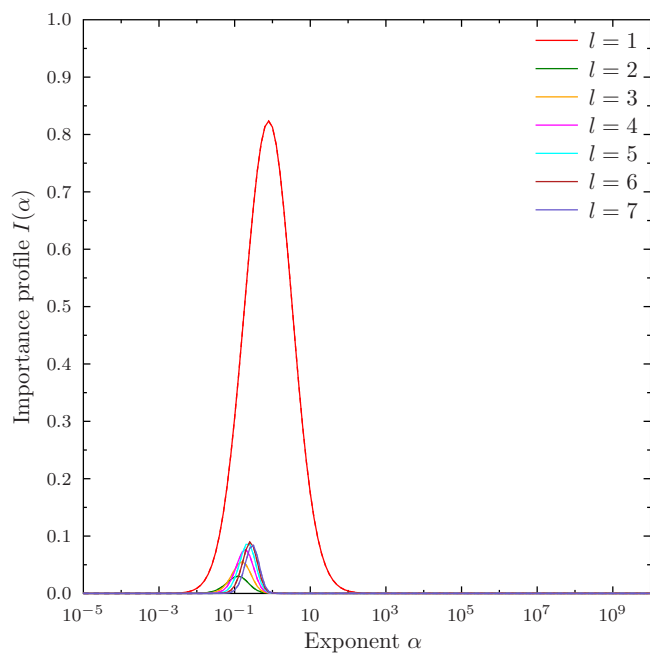

Figure 229. GTO importance profile for  $\pi_+$  orbitals on F atom in NaF.

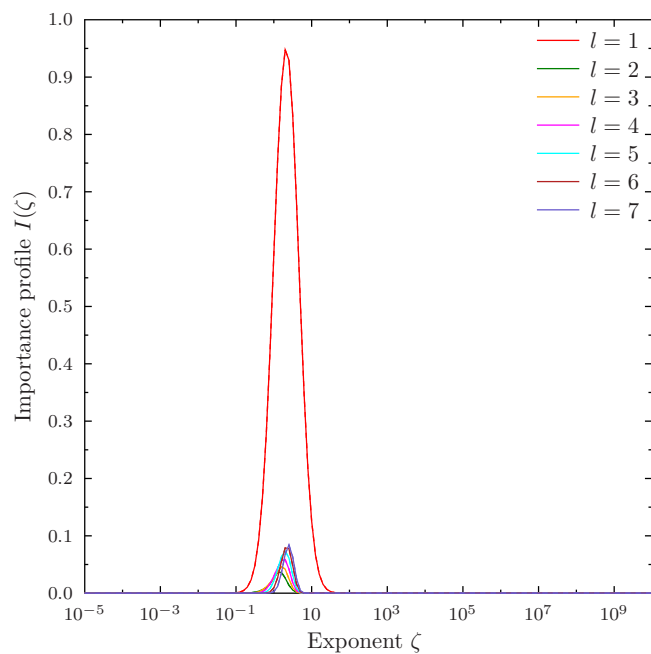

Figure 231. STO importance profile for  $\pi_+$  orbitals on F atom in CuF.

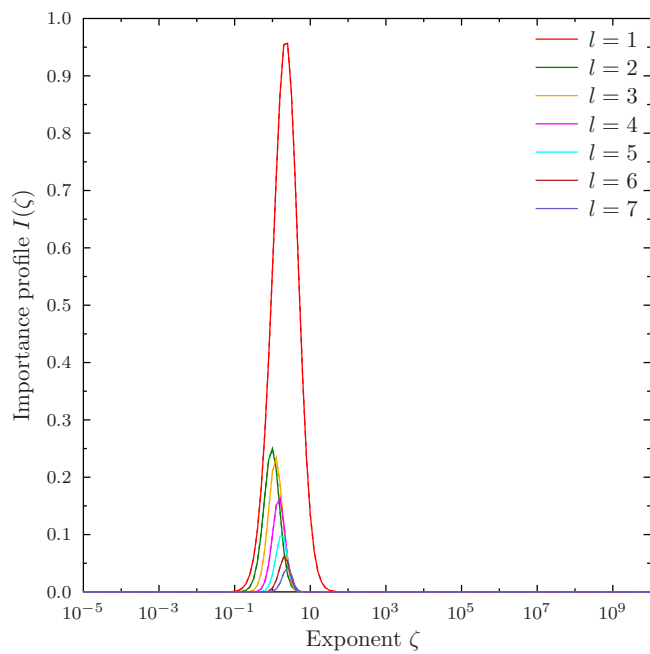

Figure 230. STO importance profile for  $\pi_+$  orbitals on F atom in ClF.

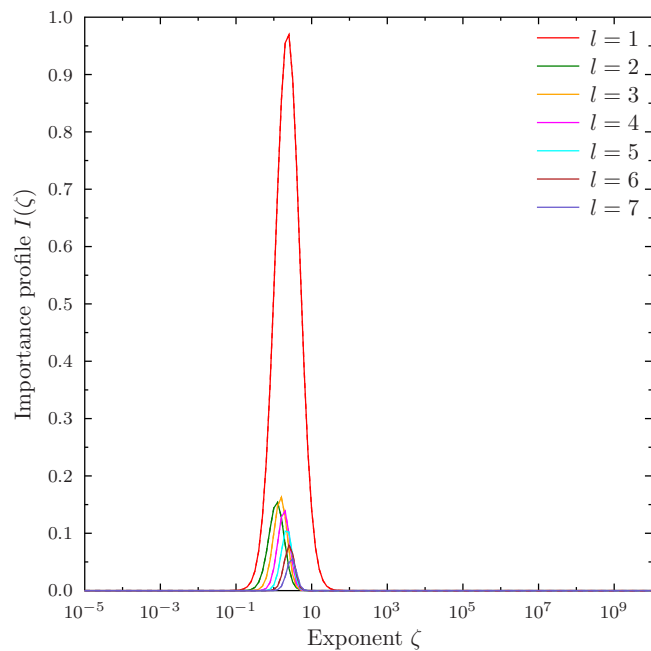

Figure 232. STO importance profile for  $\pi_+$  orbitals on F atom in  $F_2$ .

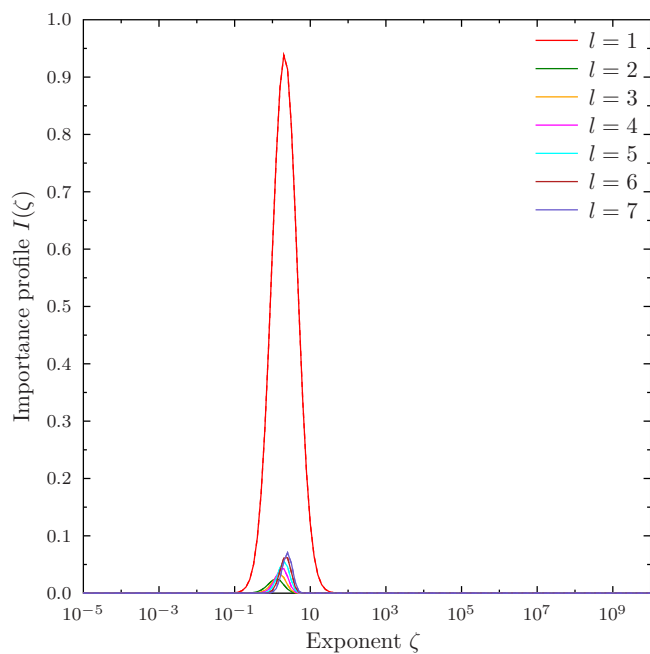

Figure 233. STO importance profile for  $\pi_+$  orbitals on F atom in GaF.

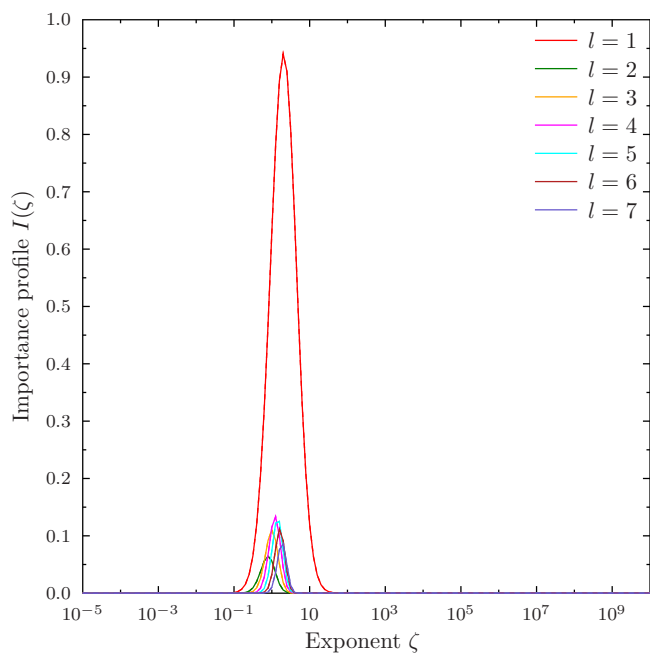

Figure 235. STO importance profile for  $\pi_+$  orbitals on F atom in KF.

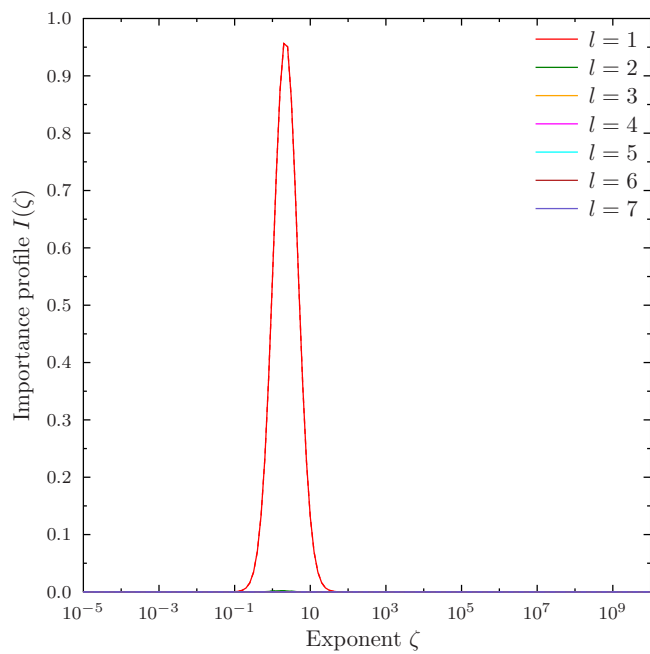

Figure 234. STO importance profile for  $\pi_+$  orbitals on F atom in HF.

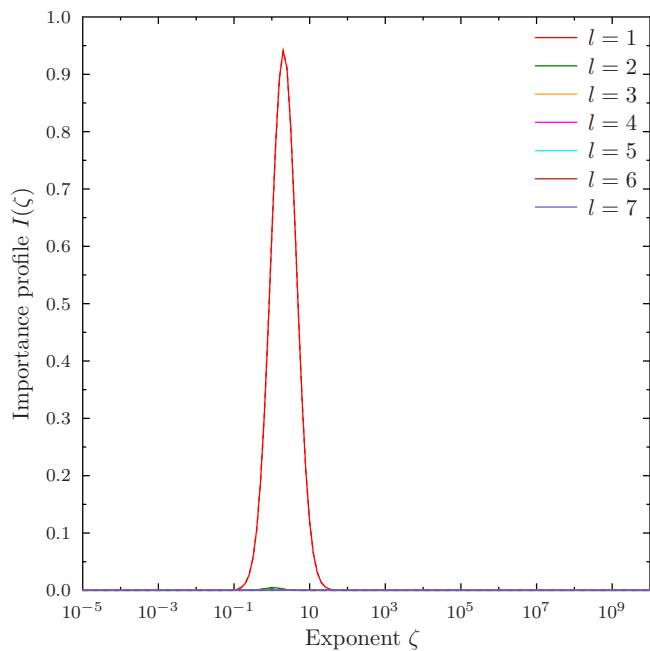

Figure 236. STO importance profile for  $\pi_+$  orbitals on F atom in LiF.

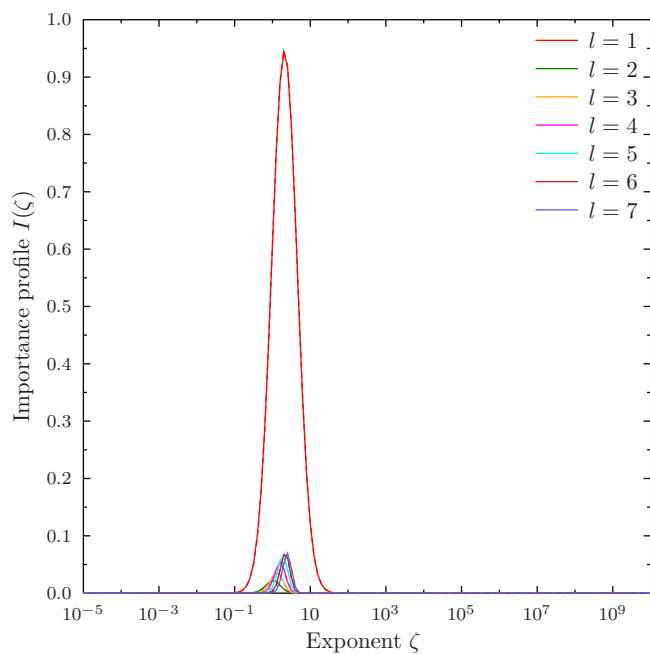

Figure 237. STO importance profile for  $\pi_+$  orbitals on F atom in MgF.

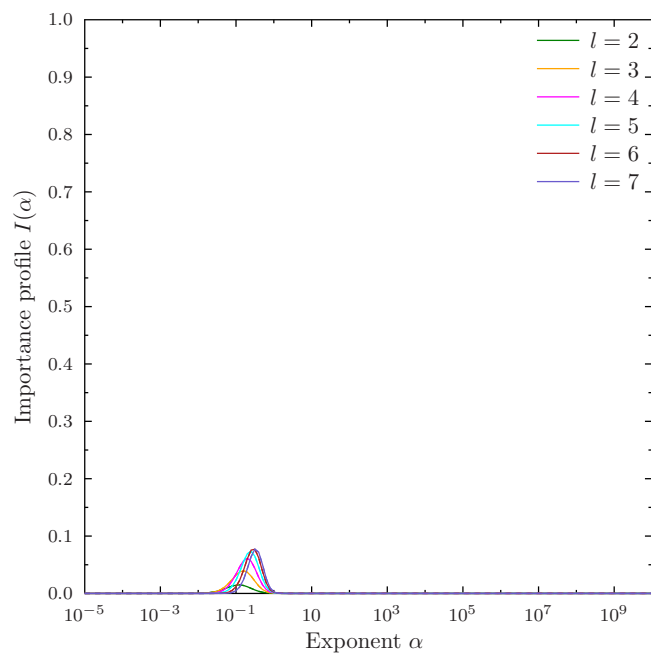

Figure 239. GTO importance profile for  $\delta_-$  orbitals on F atom in CuF.

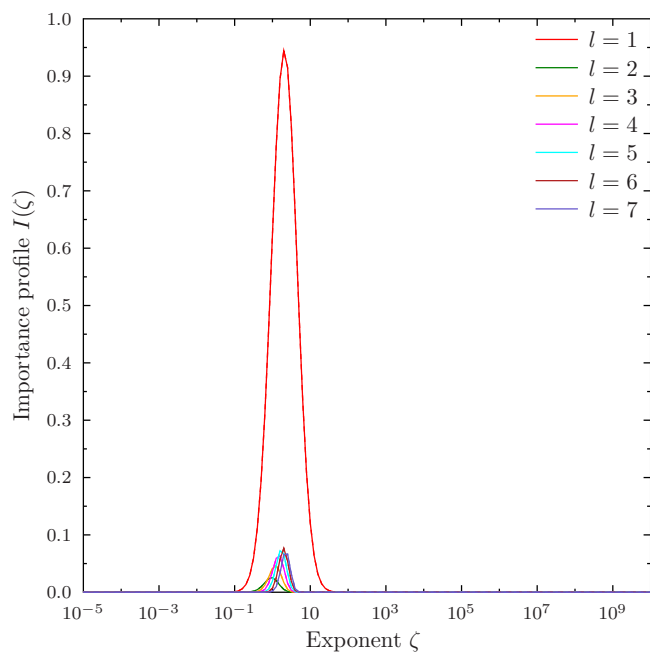

Figure 238. STO importance profile for  $\pi_+$  orbitals on F atom in NaF.

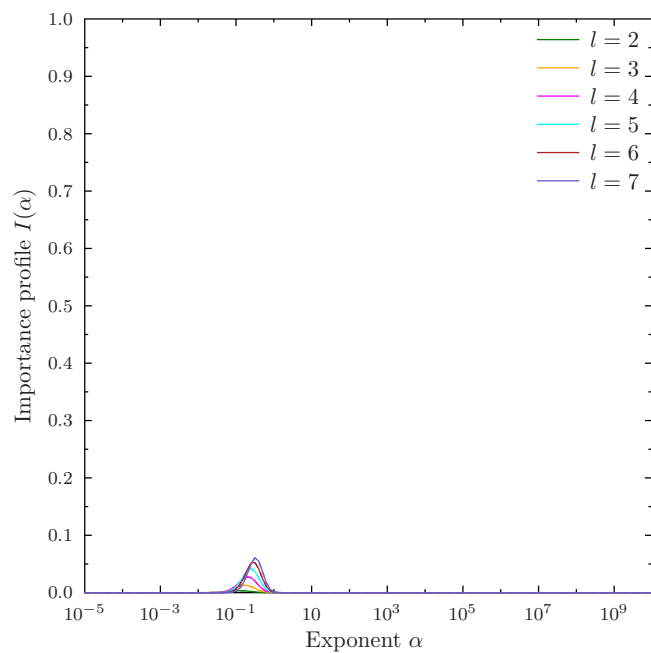

Figure 240. GTO importance profile for  $\delta_-$  orbitals on F atom in GaF.



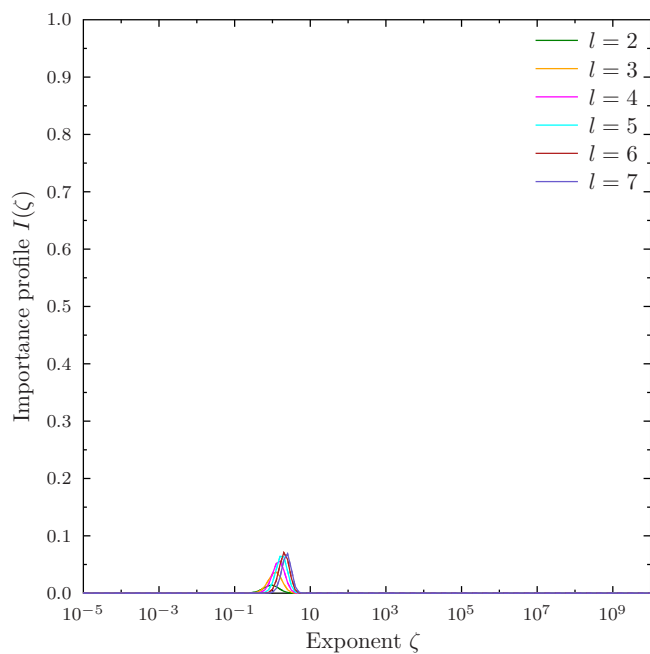

Figure 241. STO importance profile for  $\delta_-$  orbitals on F atom in CuF.

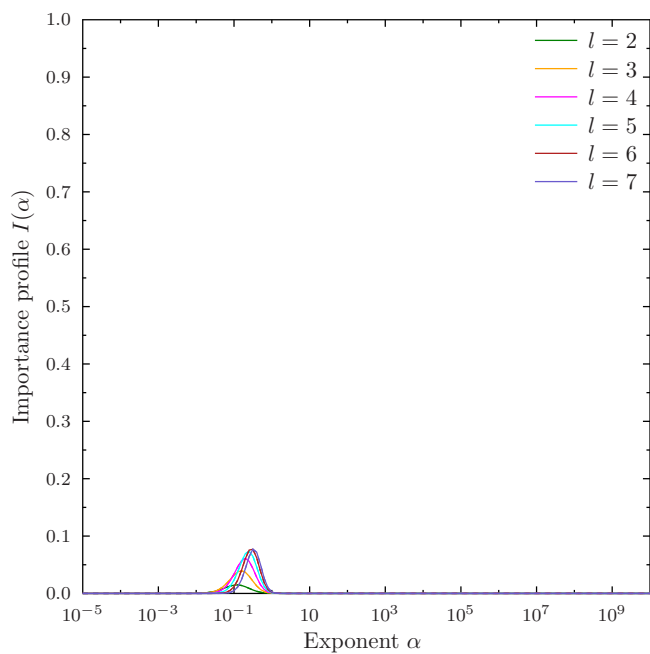

Figure 243. GTO importance profile for  $\delta_+$  orbitals on F atom in CuF.

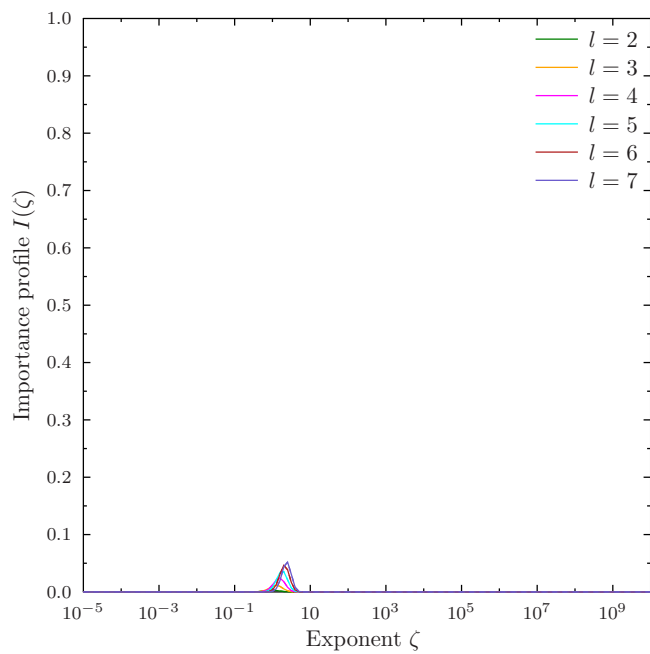

Figure 242. STO importance profile for  $\delta_-$  orbitals on F atom in GaF.

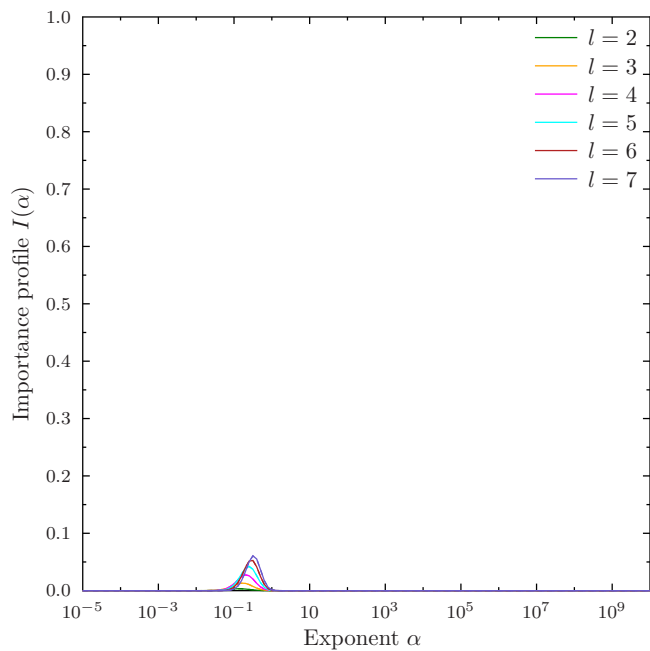

Figure 244. GTO importance profile for  $\delta_+$  orbitals on F atom in GaF.

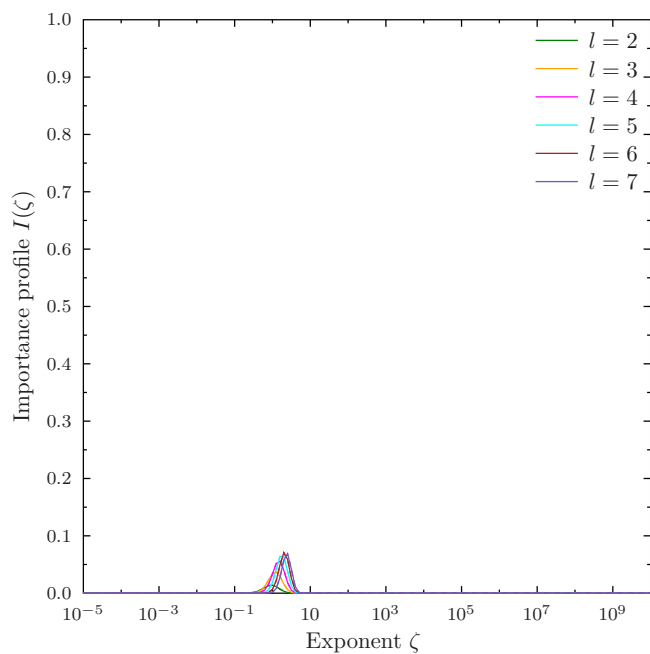

Figure 245. STO importance profile for  $\delta_+$  orbitals on F atom in CuF.

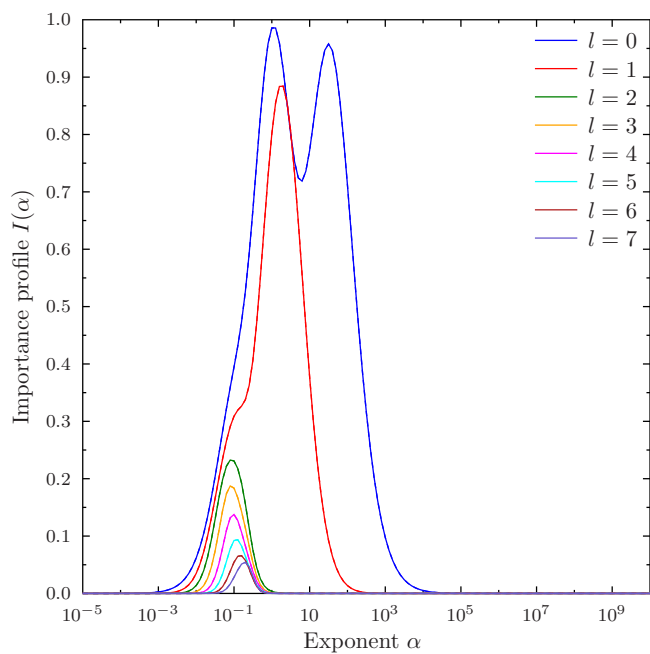

Figure 247. GTO importance profile for  $\sigma$  orbitals on Na atom in NaCl.

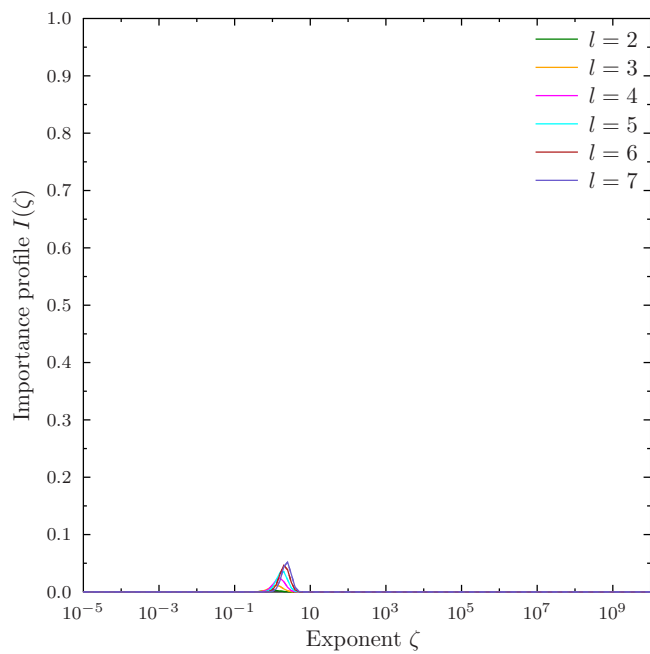

Figure 246. STO importance profile for  $\delta_+$  orbitals on F atom in GaF.

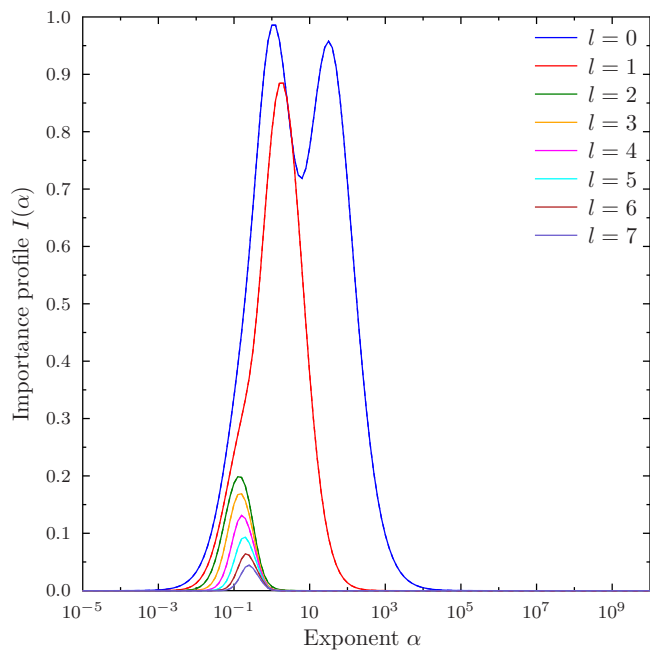

Figure 248. GTO importance profile for  $\sigma$  orbitals on Na atom in NaF.

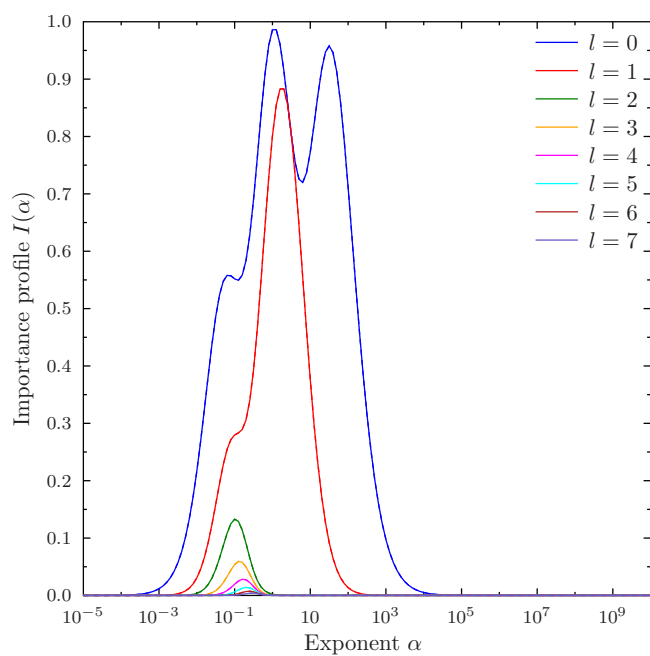

Figure 249. GTO importance profile for  $\sigma$  orbitals on Na atom in NaH.

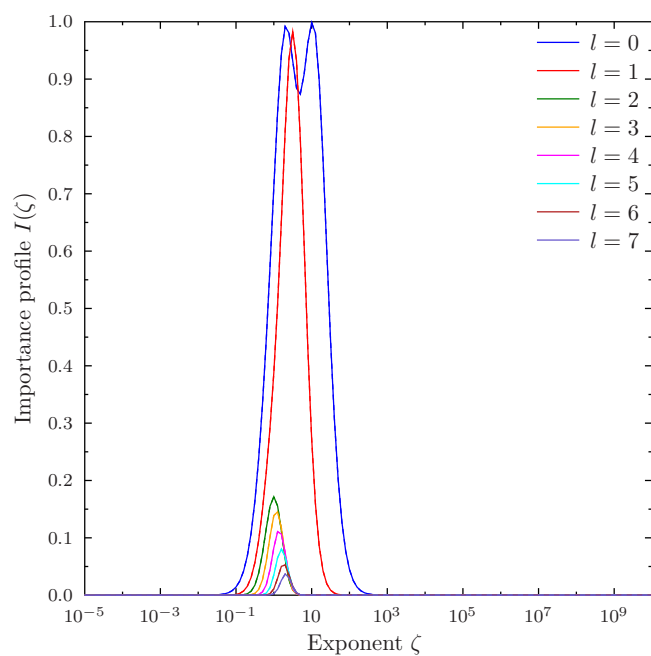

Figure 251. STO importance profile for  $\sigma$  orbitals on Na atom in NaF.

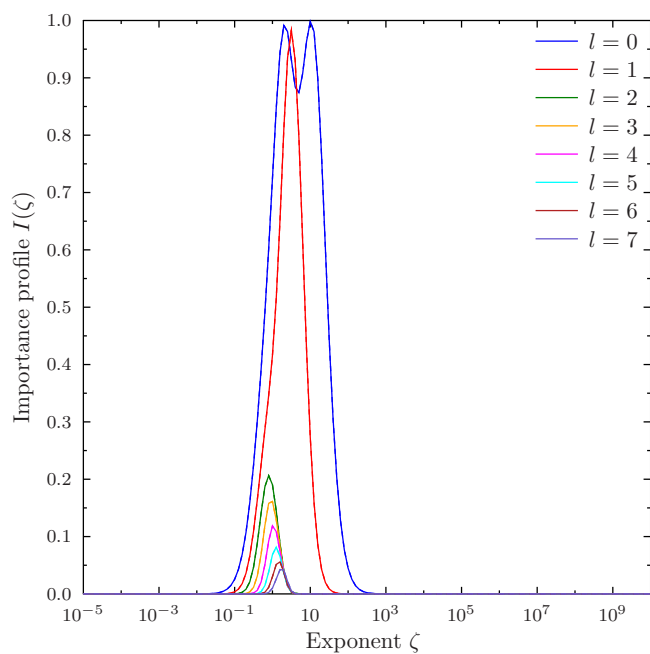

Figure 250. STO importance profile for  $\sigma$  orbitals on Na atom in NaCl.

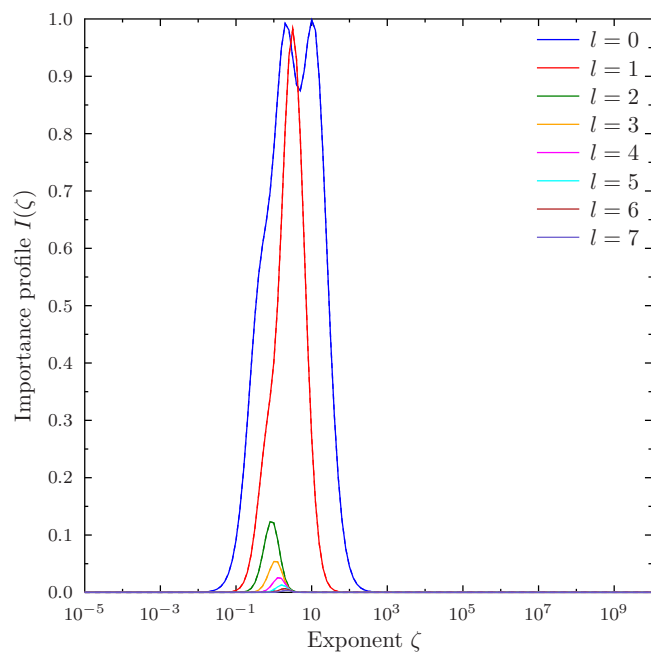

Figure 252. STO importance profile for  $\sigma$  orbitals on Na atom in NaH.

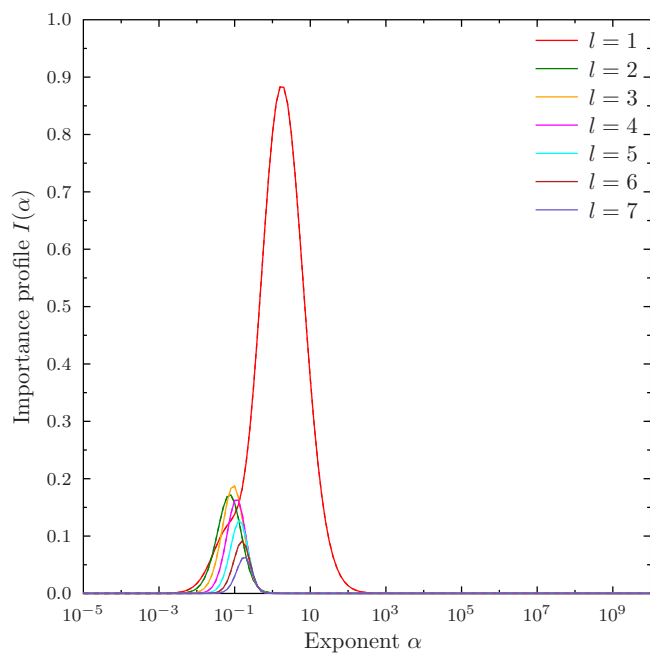

Figure 253. GTO importance profile for  $\pi_-$  orbitals on Na atom in NaCl.

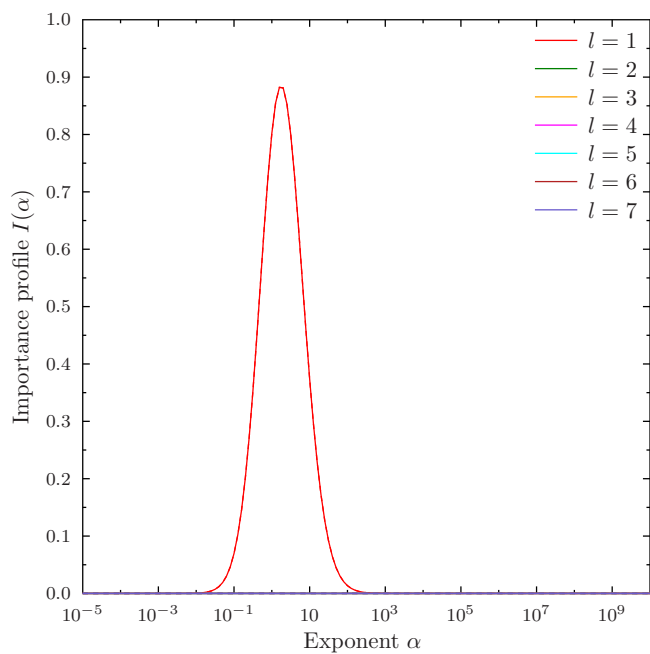

Figure 255. GTO importance profile for  $\pi_-$  orbitals on Na atom in NaH.

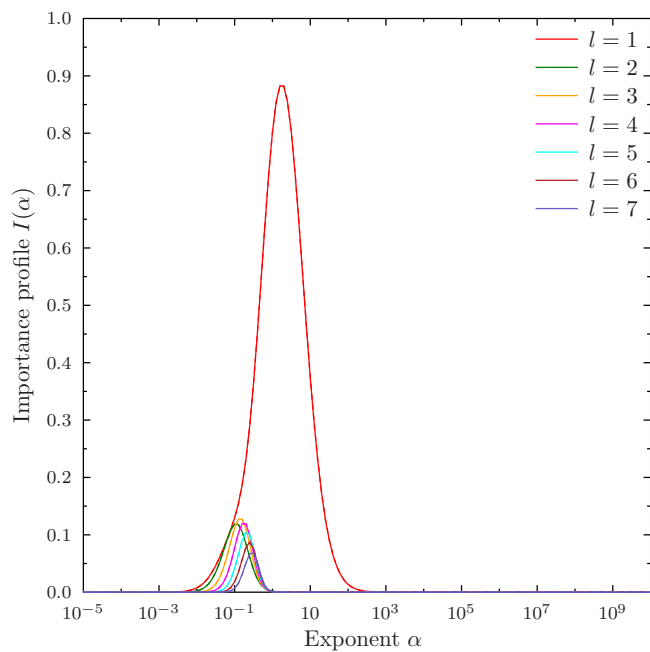

Figure 254. GTO importance profile for  $\pi_-$  orbitals on Na atom in NaF.

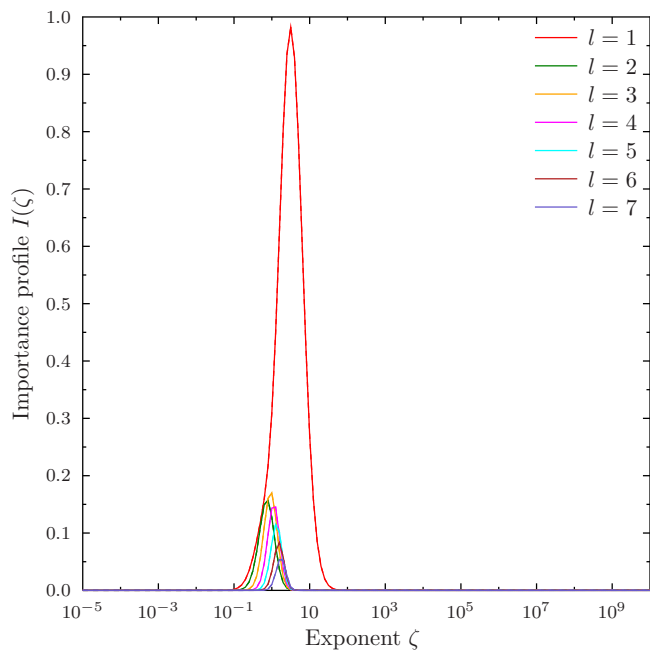

Figure 256. STO importance profile for  $\pi_-$  orbitals on Na atom in NaCl.

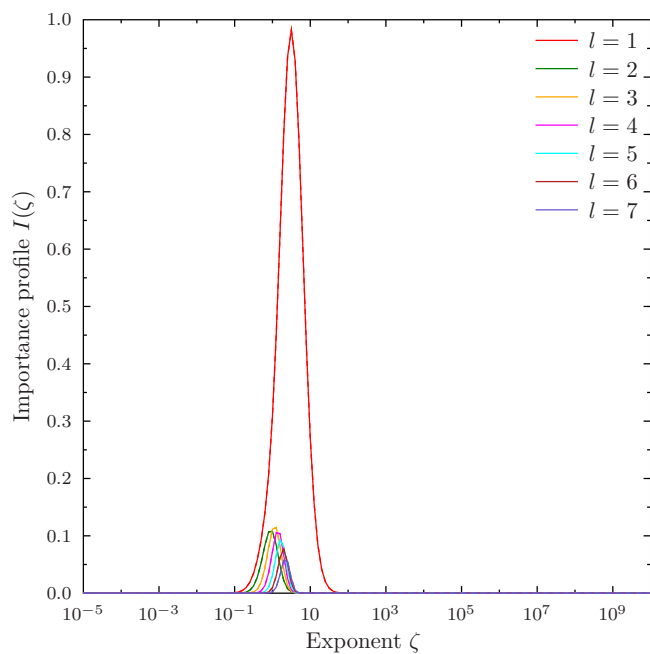

Figure 257. STO importance profile for  $\pi_-$  orbitals on Na atom in NaF.

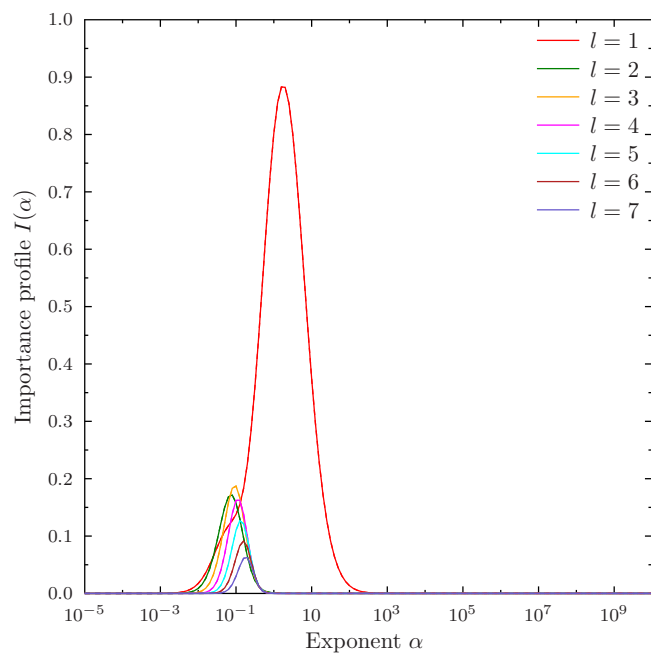

Figure 259. GTO importance profile for  $\pi_+$  orbitals on Na atom in NaCl.

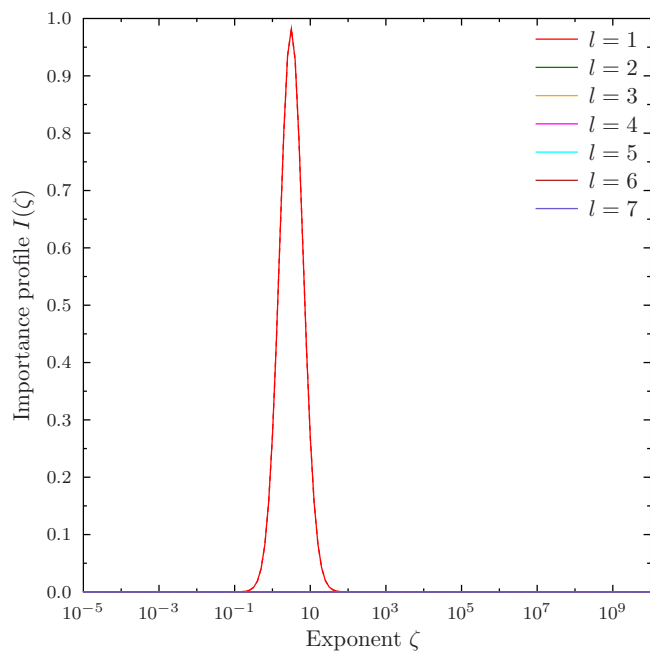

Figure 258. STO importance profile for  $\pi_-$  orbitals on Na atom in NaH.

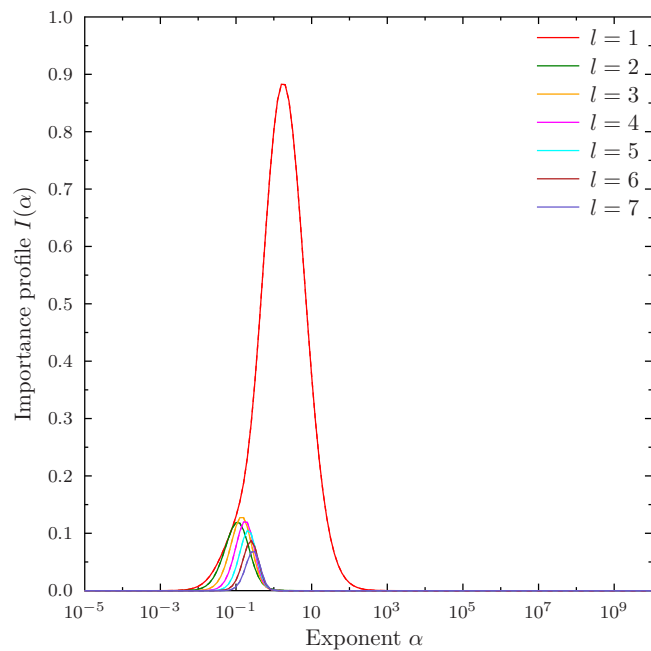

Figure 260. GTO importance profile for  $\pi_+$  orbitals on Na atom in NaF.

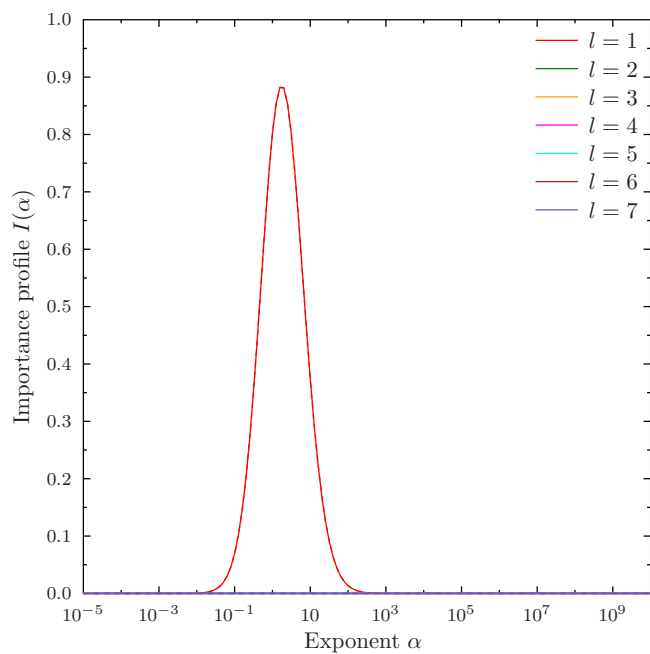

Figure 261. GTO importance profile for  $\pi_+$  orbitals on Na atom in NaH.

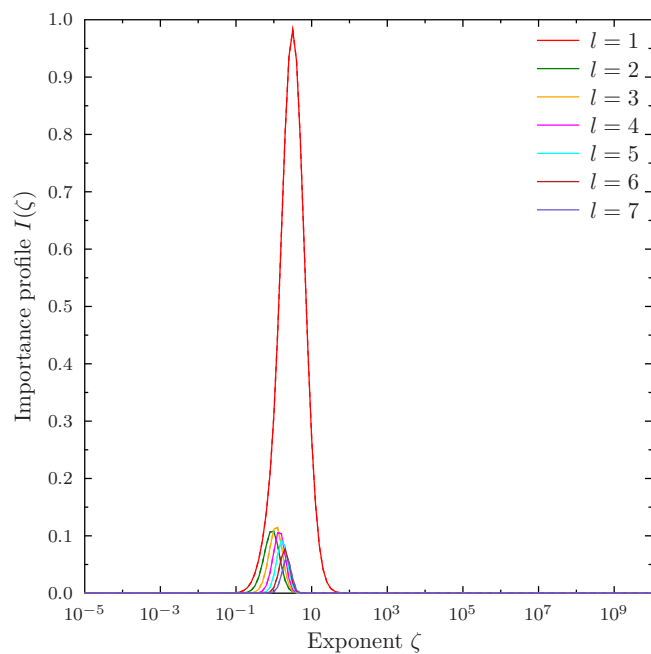

Figure 263. STO importance profile for  $\pi_+$  orbitals on Na atom in NaF.

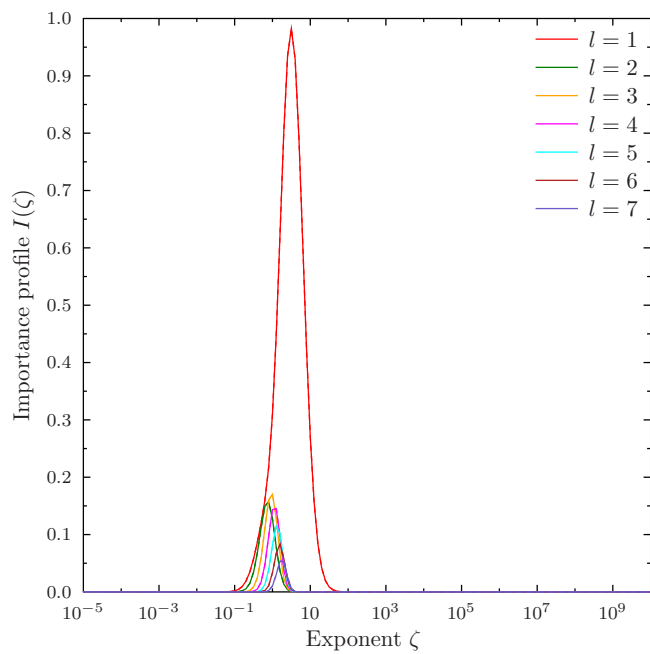

Figure 262. STO importance profile for  $\pi_+$  orbitals on Na atom in NaCl.

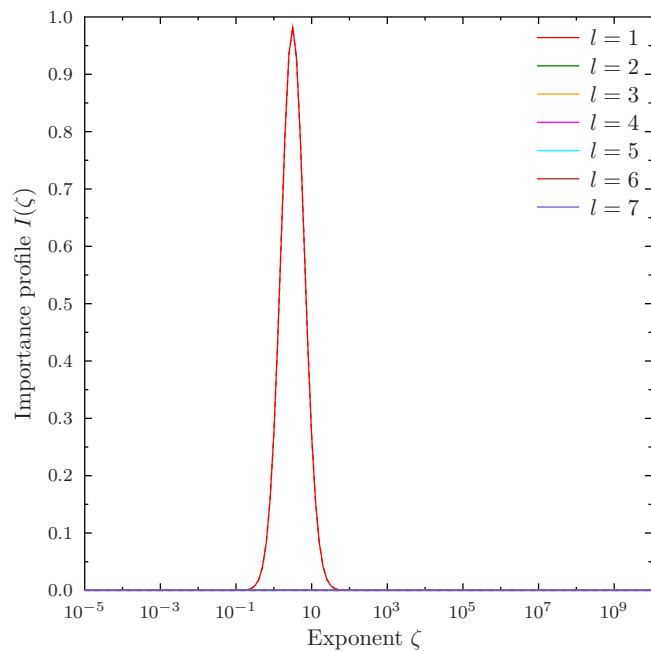

Figure 264. STO importance profile for  $\pi_+$  orbitals on Na atom in NaH.

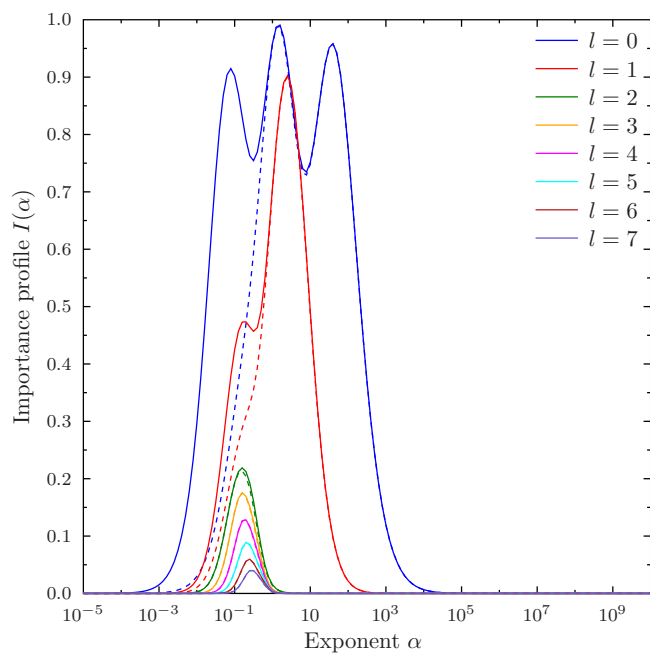

Figure 265. GTO importance profile for  $\sigma$  orbitals on Mg atom in MgF.

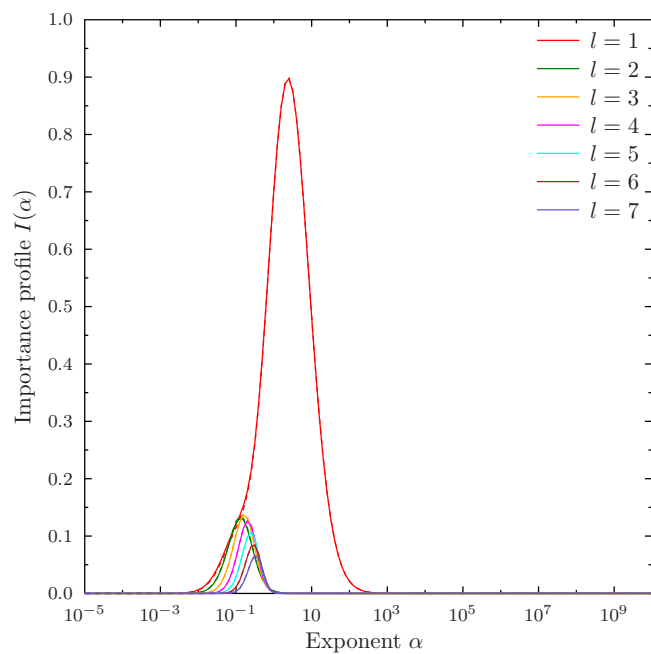

Figure 267. GTO importance profile for  $\pi_-$  orbitals on Mg atom in MgF.

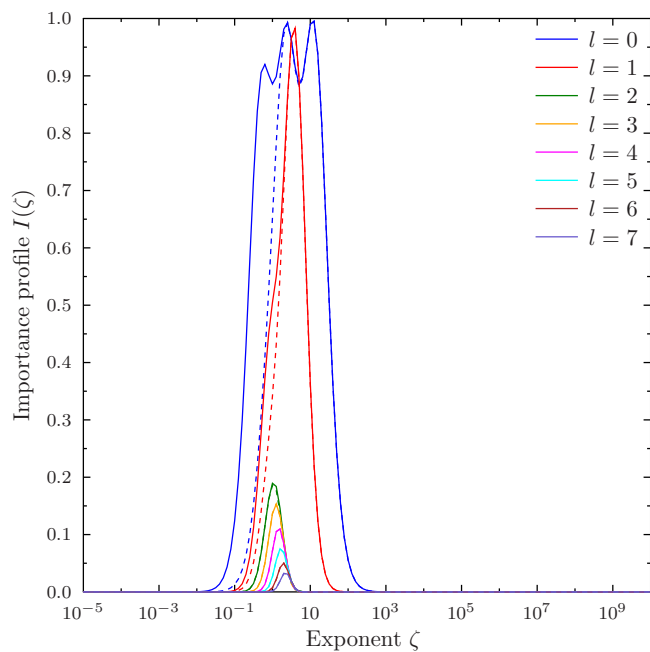

Figure 266. STO importance profile for  $\sigma$  orbitals on Mg atom in MgF.

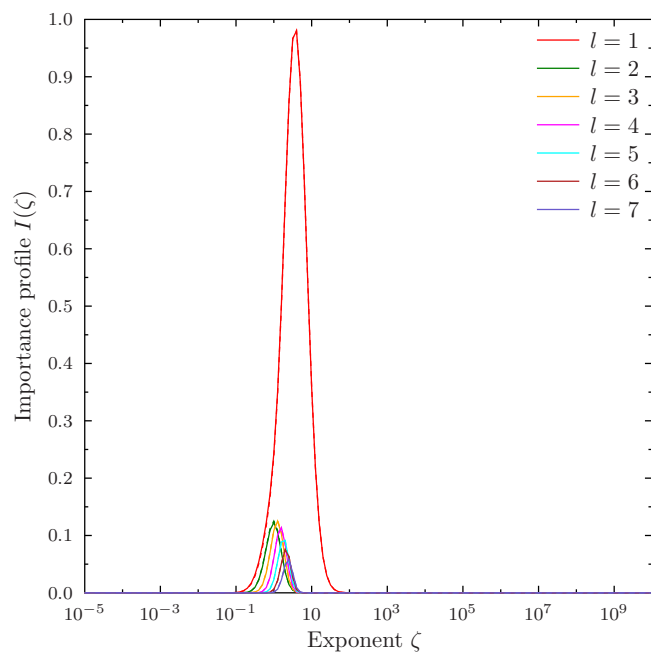

Figure 268. STO importance profile for  $\pi_-$  orbitals on Mg atom in MgF.

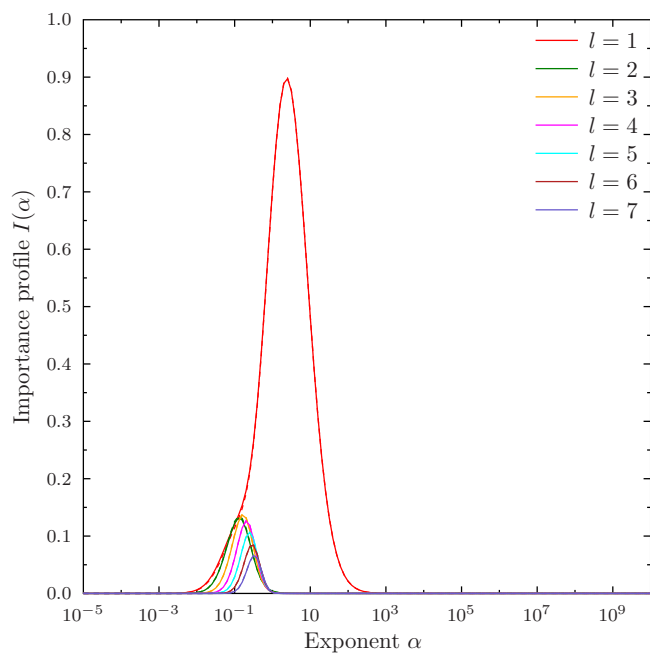

Figure 269. GTO importance profile for  $\pi_+$  orbitals on Mg atom in MgF.

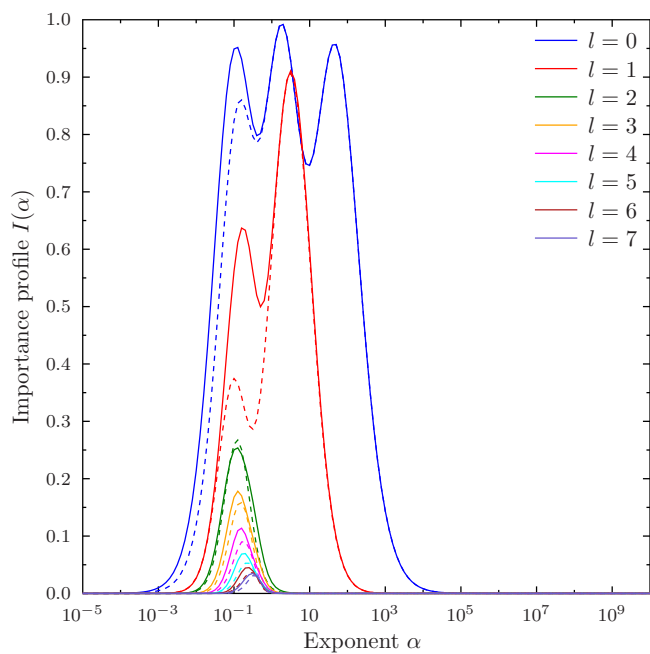

Figure 271. GTO importance profile for  $\sigma$  orbitals on Al atom in AlN.

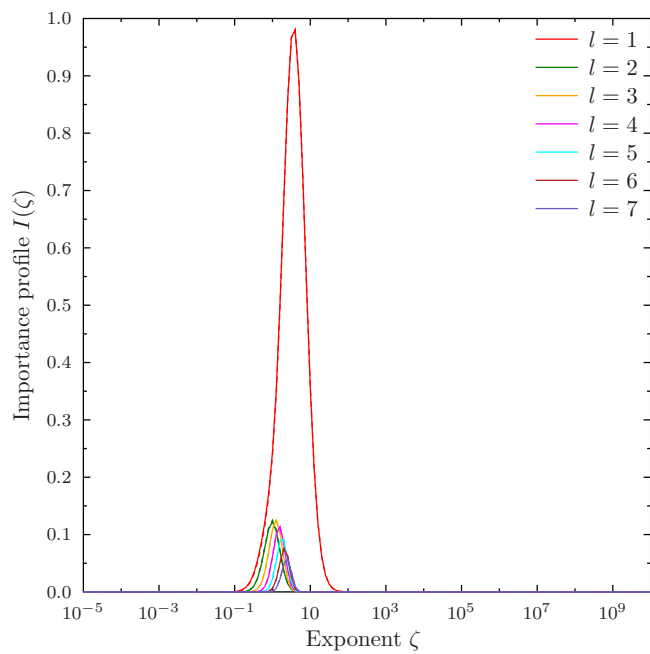

Figure 270. STO importance profile for  $\pi_+$  orbitals on Mg atom in MgF.

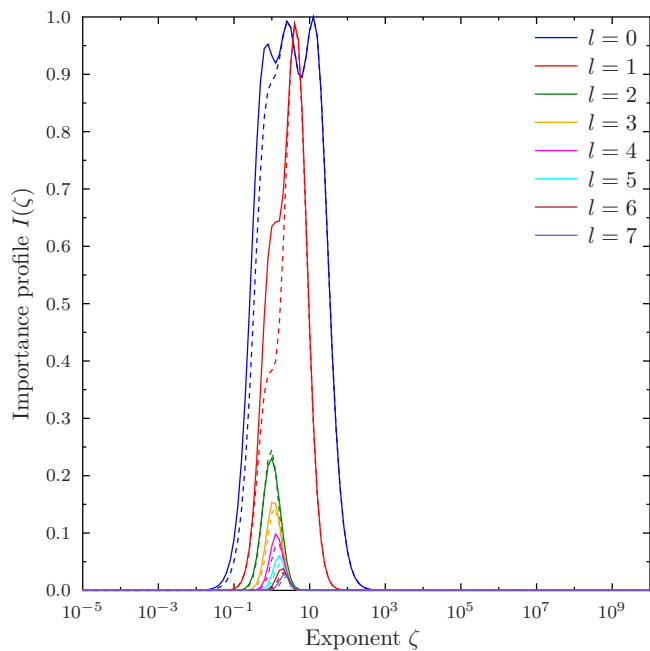

Figure 272. STO importance profile for  $\sigma$  orbitals on Al atom in AlN.



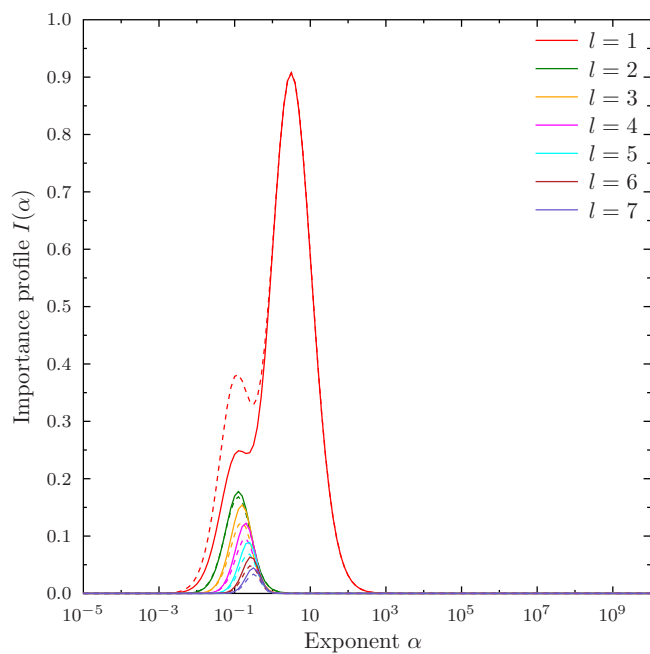

Figure 273. GTO importance profile for  $\pi_-$  orbitals on Al atom in AlN.

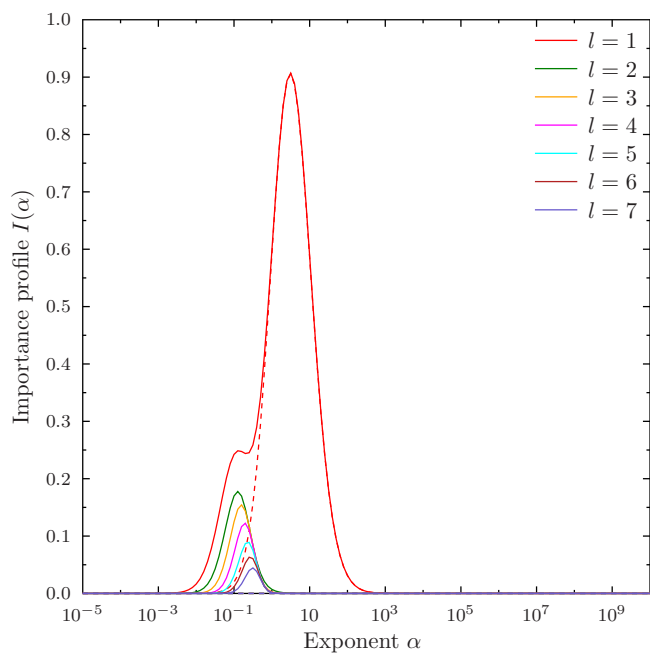

Figure 275. GTO importance profile for  $\pi_+$  orbitals on Al atom in AlN.

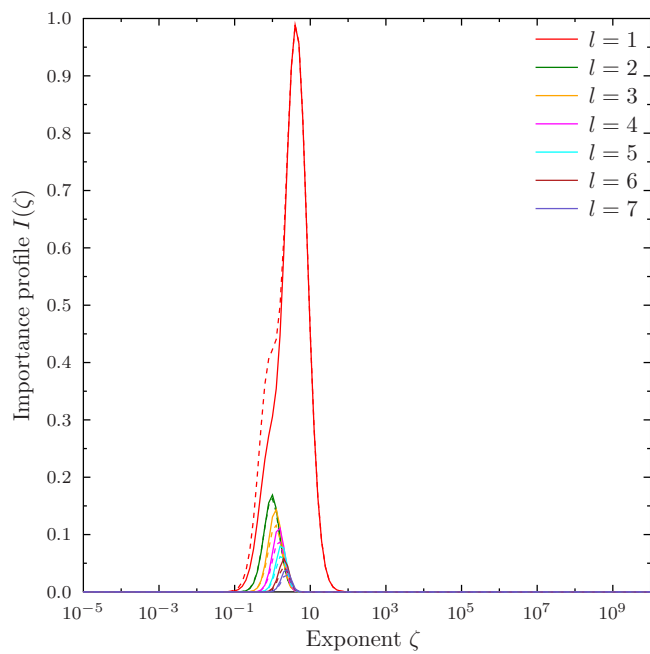

Figure 274. STO importance profile for  $\pi_-$  orbitals on Al atom in AlN.

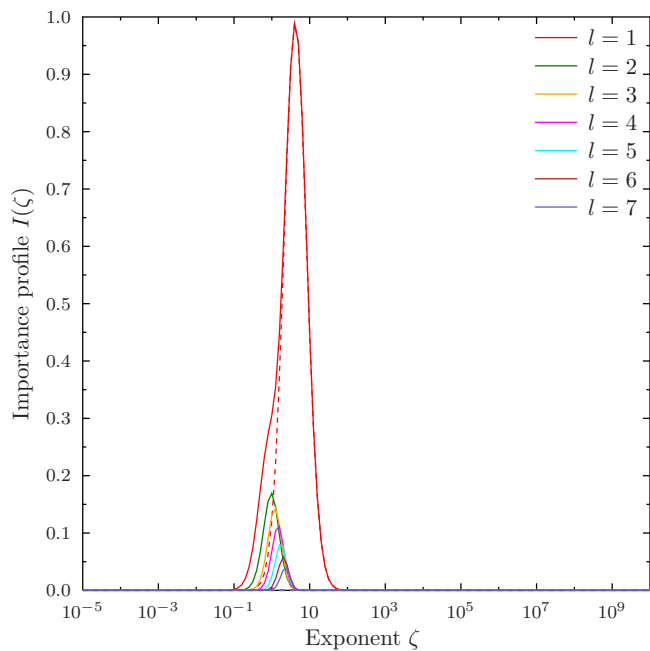

Figure 276. STO importance profile for  $\pi_+$  orbitals on Al atom in AlN.

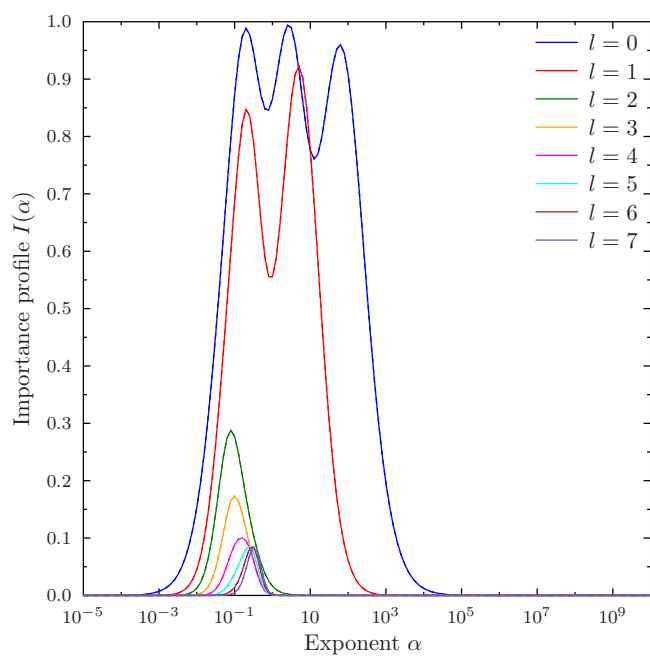

Figure 277. GTO importance profile for  $\sigma$  orbitals on P atom in  $P_2$ .

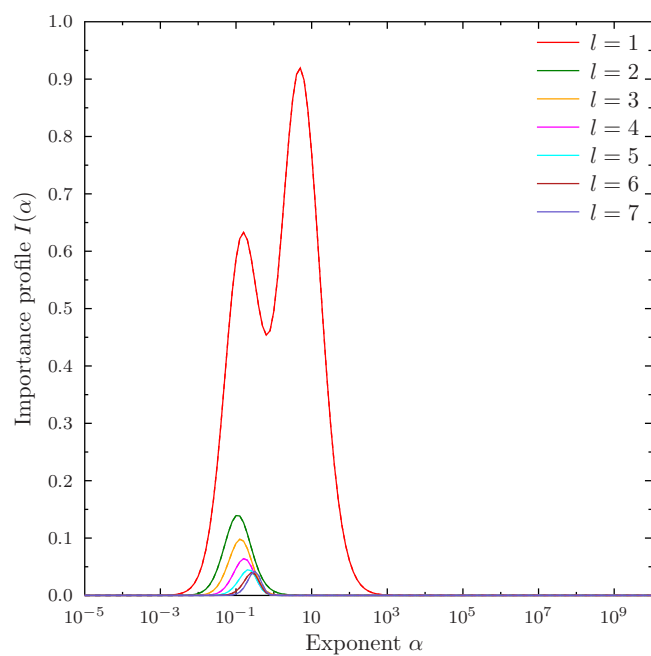

Figure 279. GTO importance profile for  $\pi_-$  orbitals on P atom in  $P_2$ .

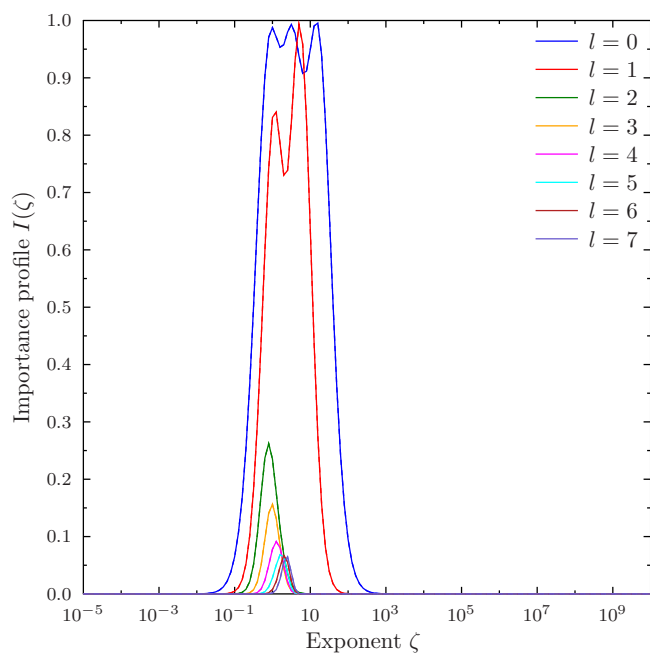

Figure 278. STO importance profile for  $\sigma$  orbitals on P atom in  $P_2$ .

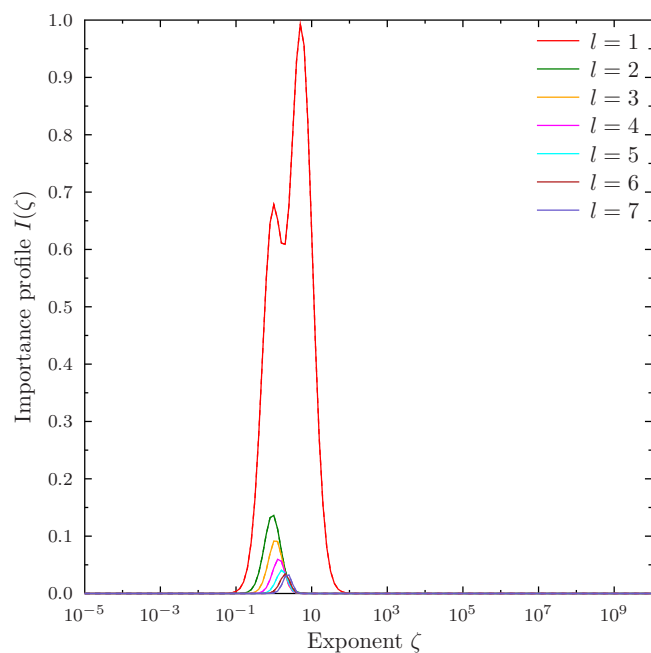

Figure 280. STO importance profile for  $\pi_-$  orbitals on P atom in  $P_2$ .

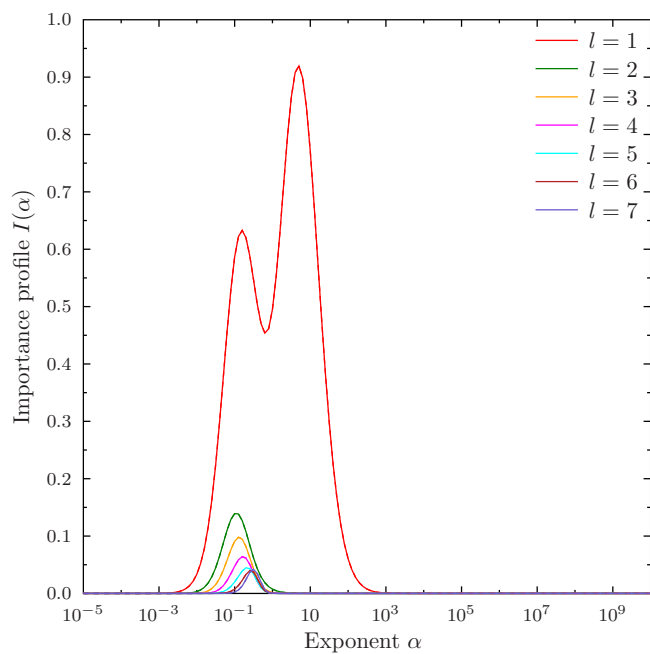

Figure 281. GTO importance profile for  $\pi_+$  orbitals on P atom in  $P_2$ .

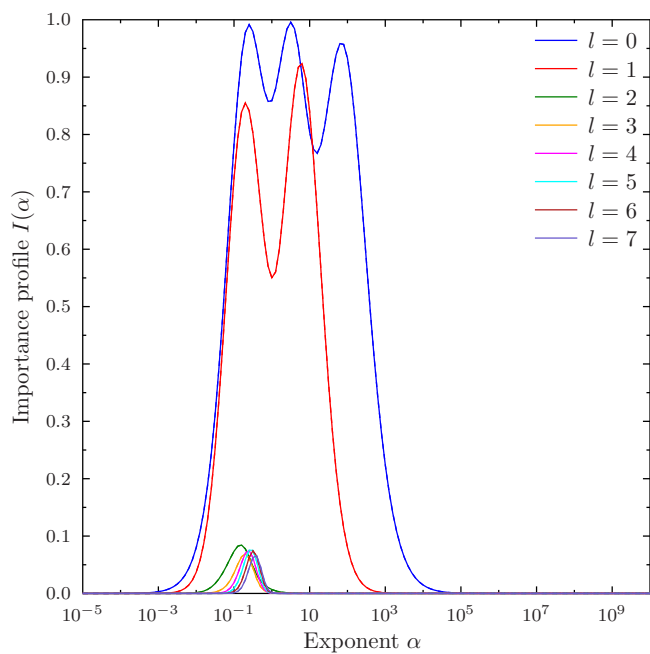

Figure 283. GTO importance profile for  $\sigma$  orbitals on S atom in BeS.

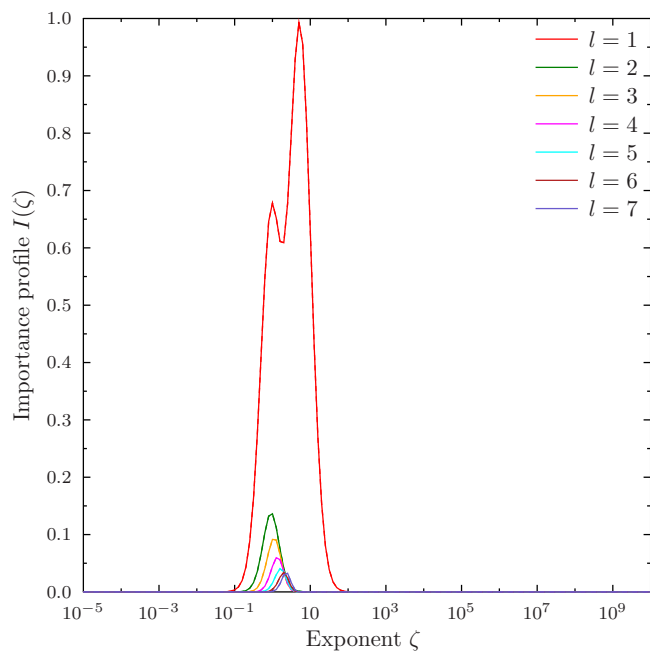

Figure 282. STO importance profile for  $\pi_+$  orbitals on P atom in  $P_2$ .

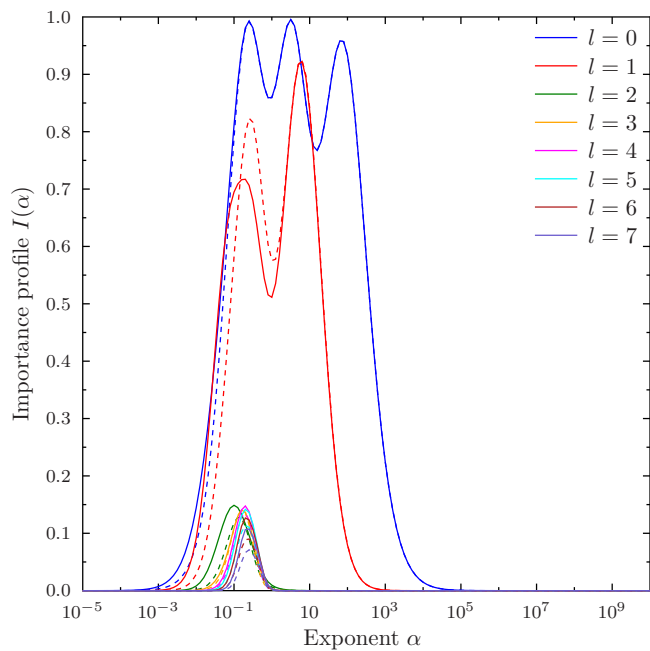

Figure 284. GTO importance profile for  $\sigma$  orbitals on S atom in MnS.

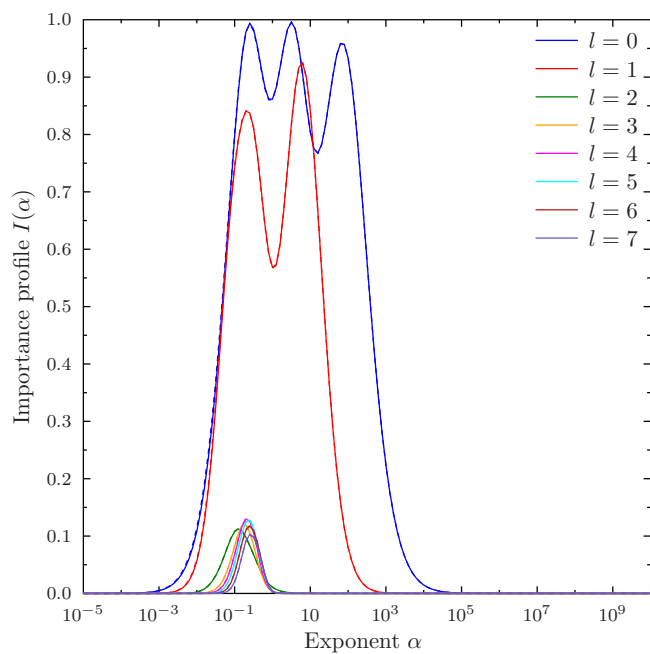

Figure 285. GTO importance profile for  $\sigma$  orbitals on S atom in NiS.

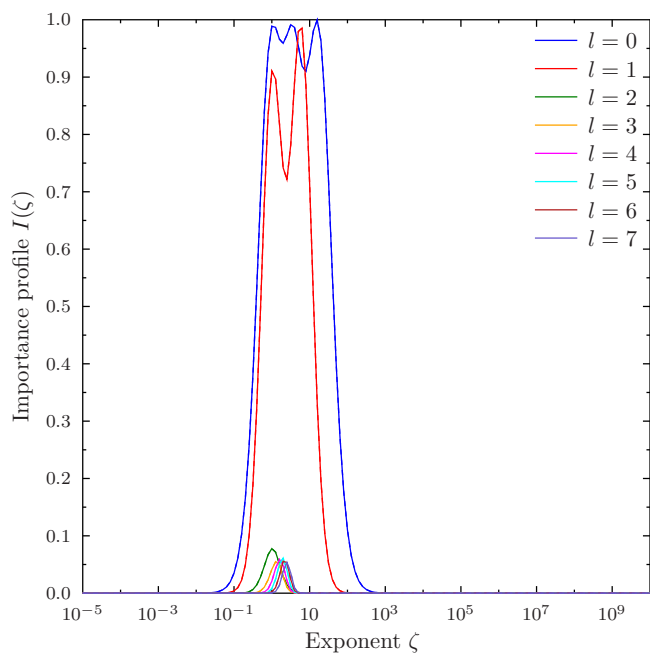

Figure 287. STO importance profile for  $\sigma$  orbitals on S atom in BeS.

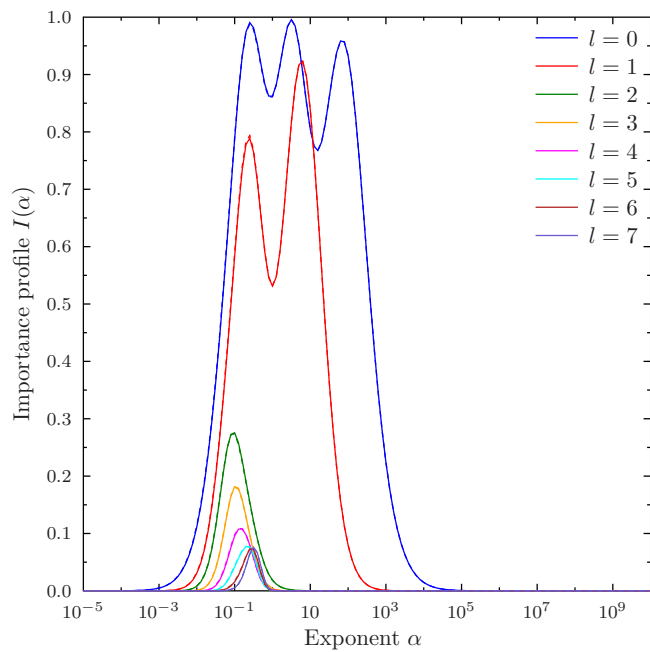

Figure 286. GTO importance profile for  $\sigma$  orbitals on S atom in  $S_2$ .

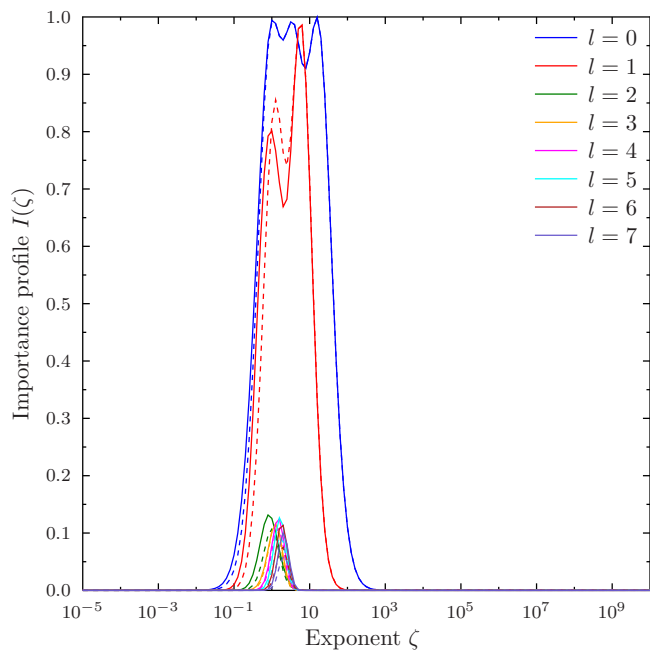

Figure 288. STO importance profile for  $\sigma$  orbitals on S atom in MnS.

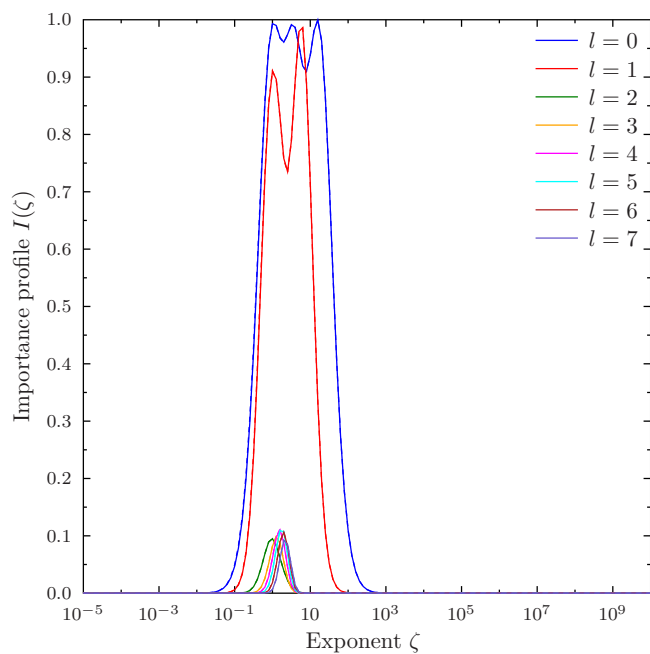

Figure 289. STO importance profile for  $\sigma$  orbitals on S atom in NiS.

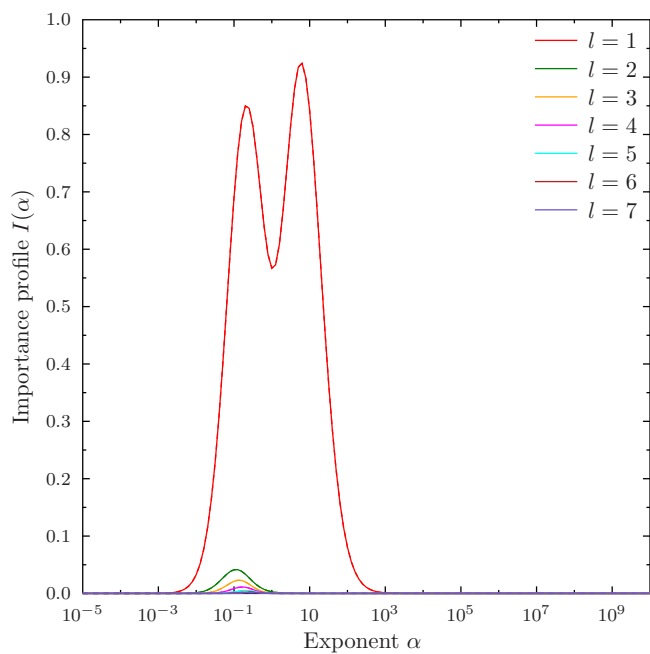

Figure 291. GTO importance profile for  $\pi_-$  orbitals on S atom in BeS.

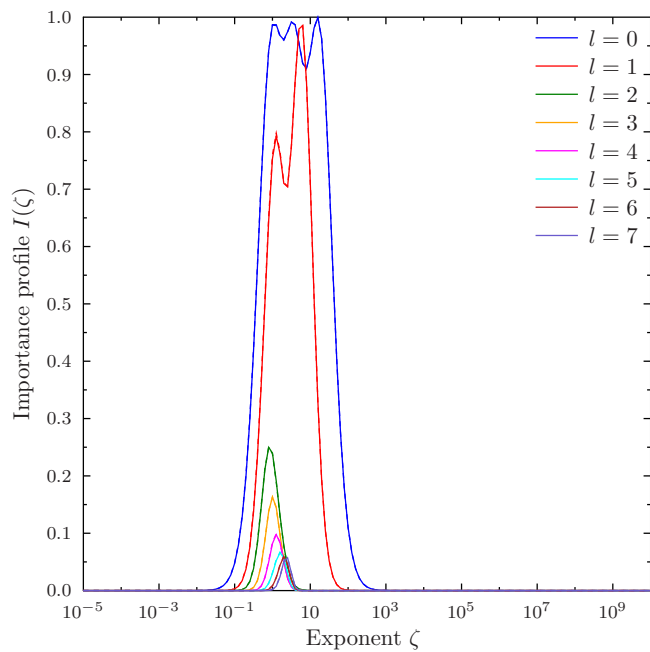

Figure 290. STO importance profile for  $\sigma$  orbitals on S atom in  $S_2$ .

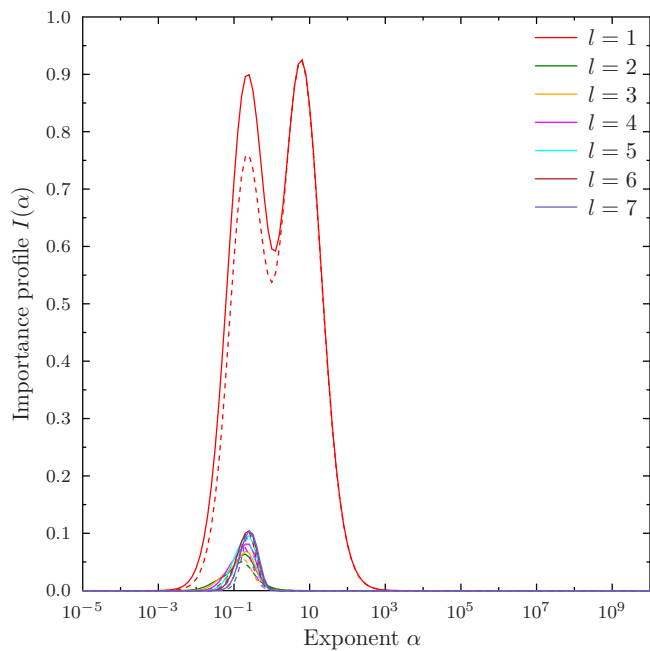

Figure 292. GTO importance profile for  $\pi_-$  orbitals on S atom in MnS.

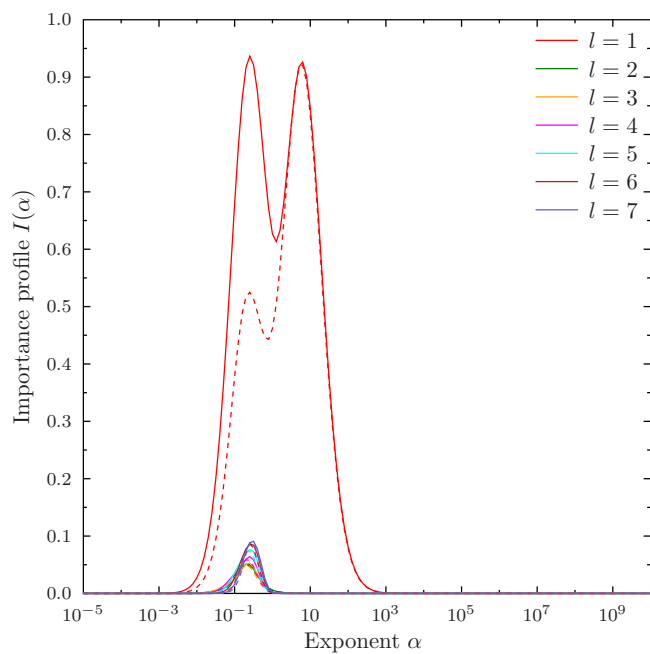

Figure 293. GTO importance profile for  $\pi_-$  orbitals on S atom in NiS.

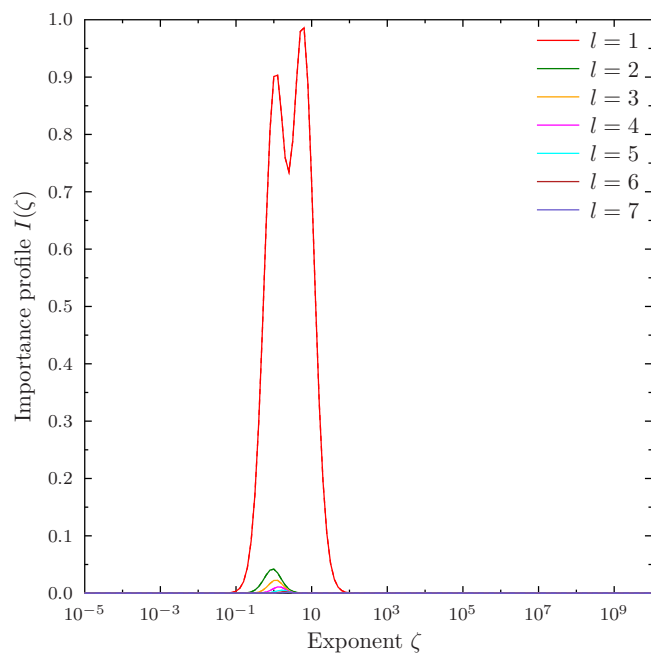

Figure 295. STO importance profile for  $\pi_-$  orbitals on S atom in BeS.

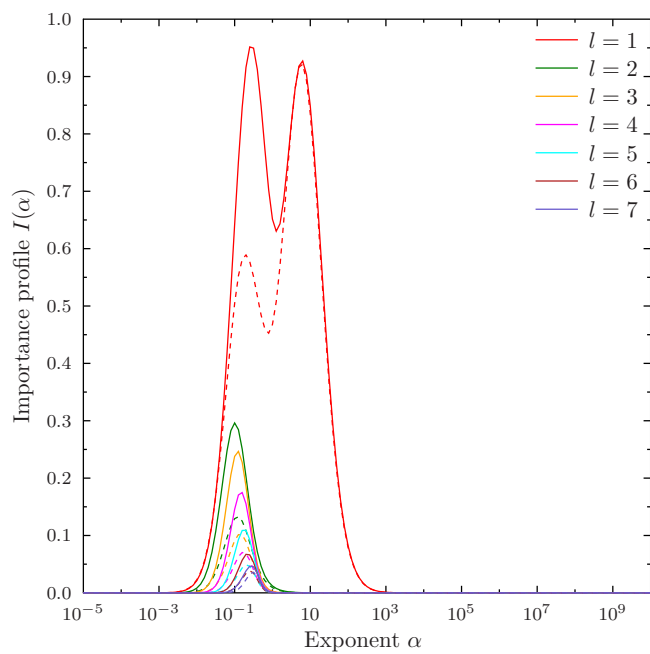

Figure 294. GTO importance profile for  $\pi_-$  orbitals on S atom in  $S_2$ .

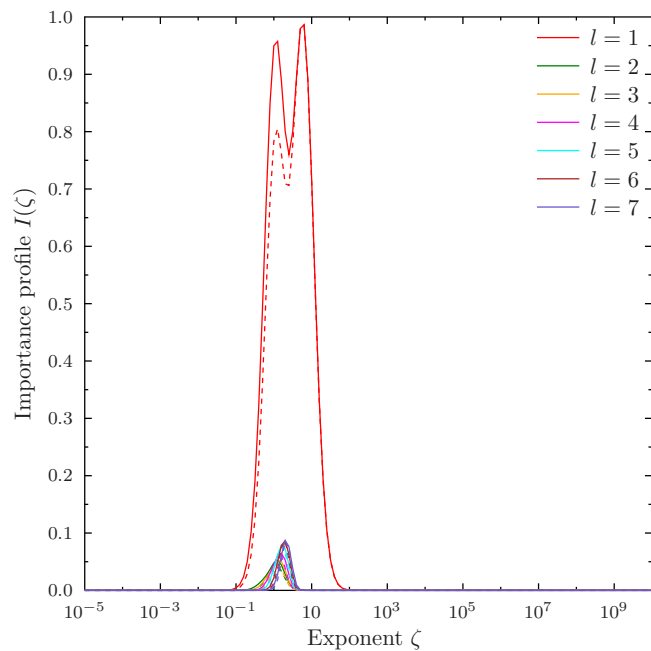

Figure 296. STO importance profile for  $\pi_-$  orbitals on S atom in MnS.

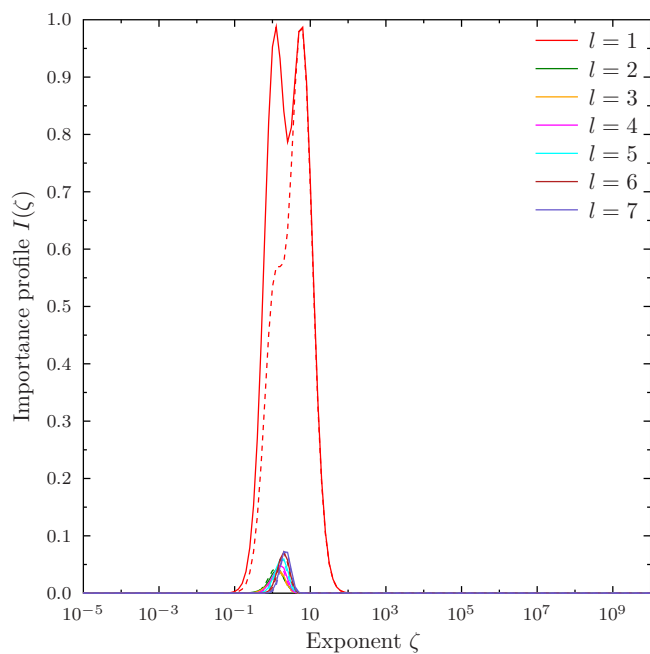

Figure 297. STO importance profile for  $\pi_-$  orbitals on S atom in NiS.

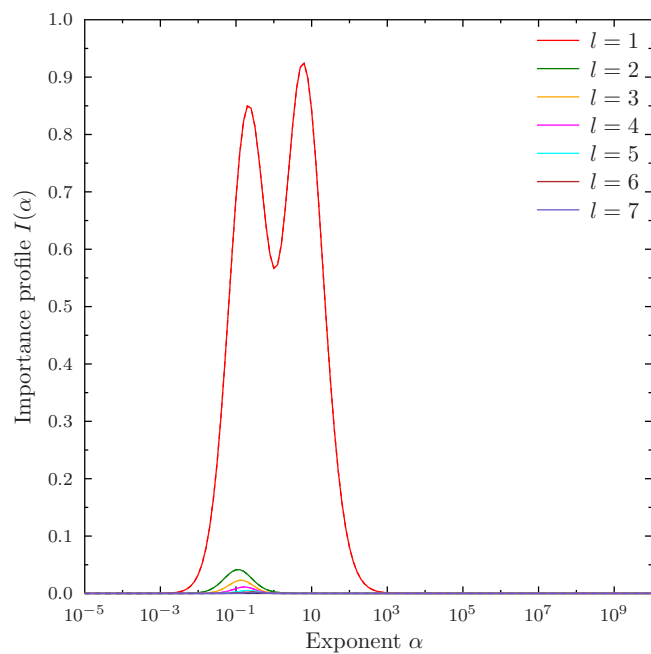

Figure 299. GTO importance profile for  $\pi_+$  orbitals on S atom in BeS.

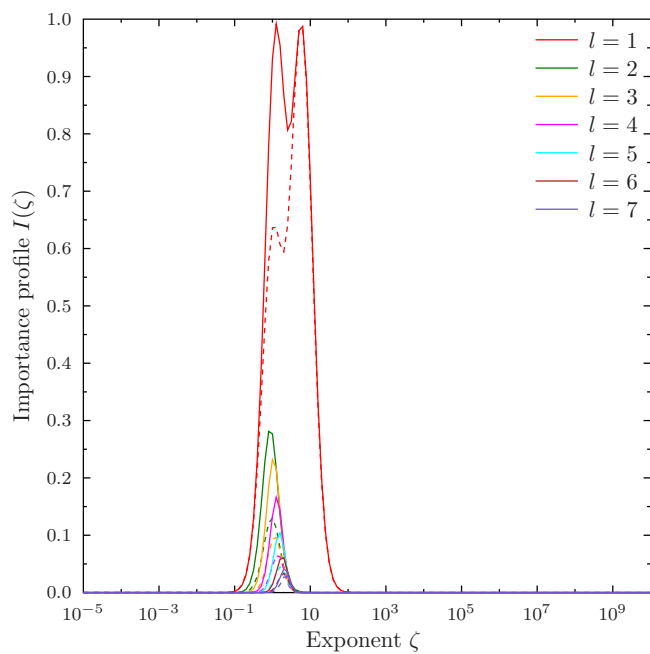

Figure 298. STO importance profile for  $\pi_-$  orbitals on S atom in  $S_2$ .

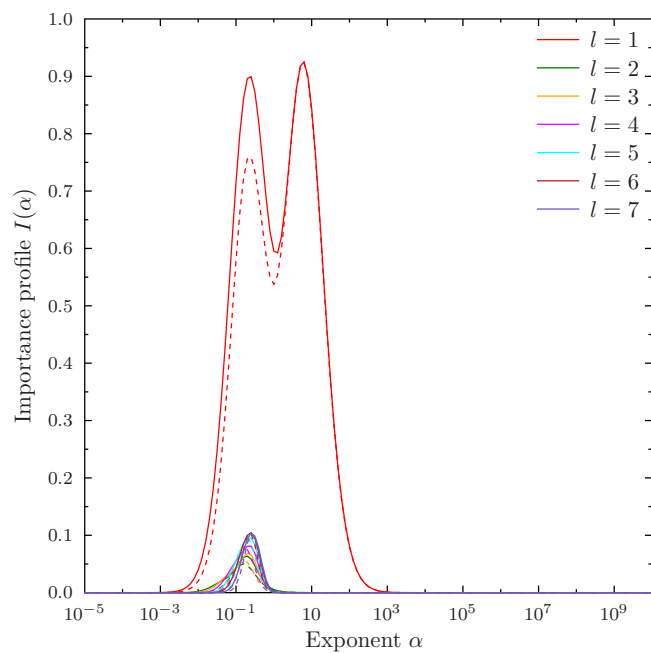

Figure 300. GTO importance profile for  $\pi_+$  orbitals on S atom in MnS.

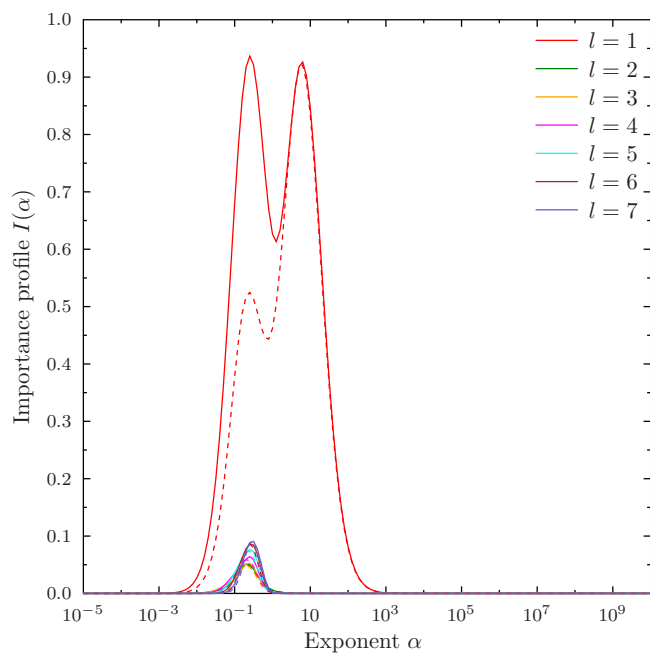

Figure 301. GTO importance profile for  $\pi_+$  orbitals on S atom in NiS.

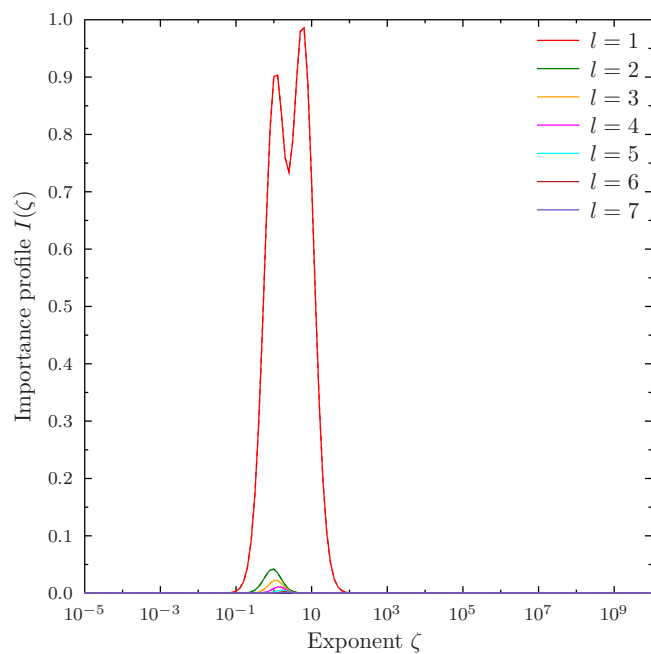

Figure 303. STO importance profile for  $\pi_+$  orbitals on S atom in BeS.

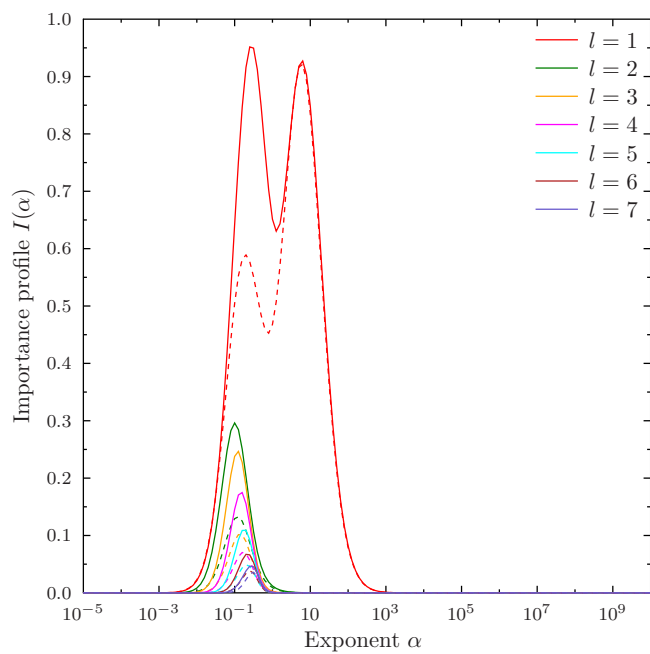

Figure 302. GTO importance profile for  $\pi_+$  orbitals on S atom in  $S_2$ .

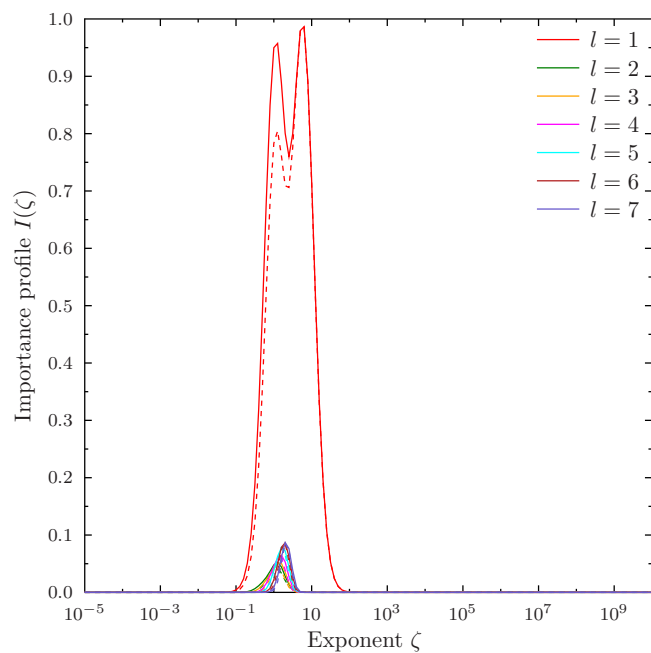

Figure 304. STO importance profile for  $\pi_+$  orbitals on S atom in MnS.



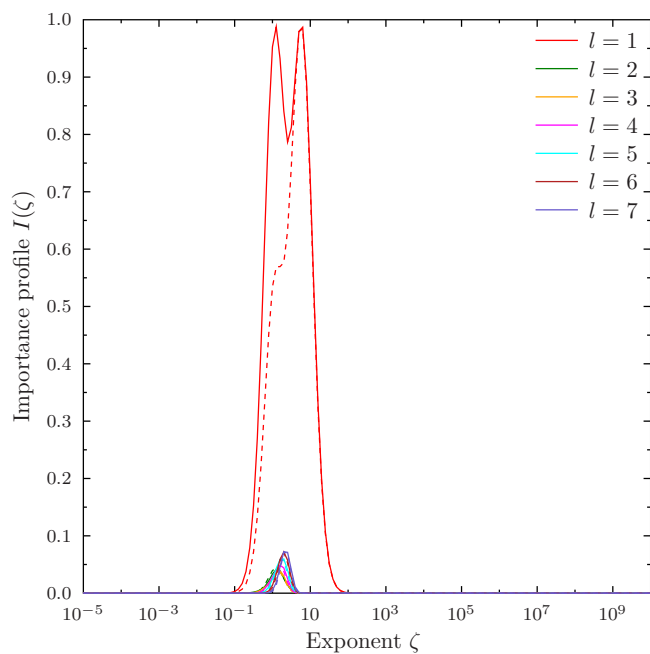

Figure 305. STO importance profile for  $\pi_+$  orbitals on S atom in NiS.

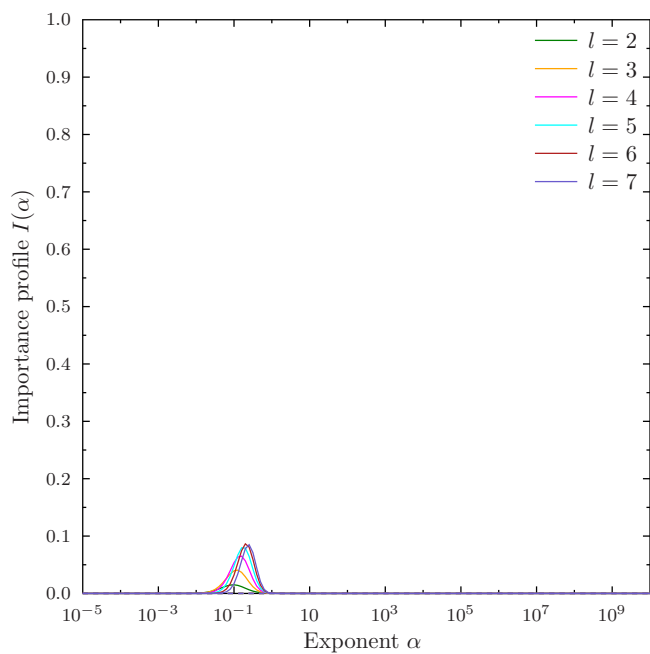

Figure 307. GTO importance profile for  $\delta_-$  orbitals on S atom in MnS.

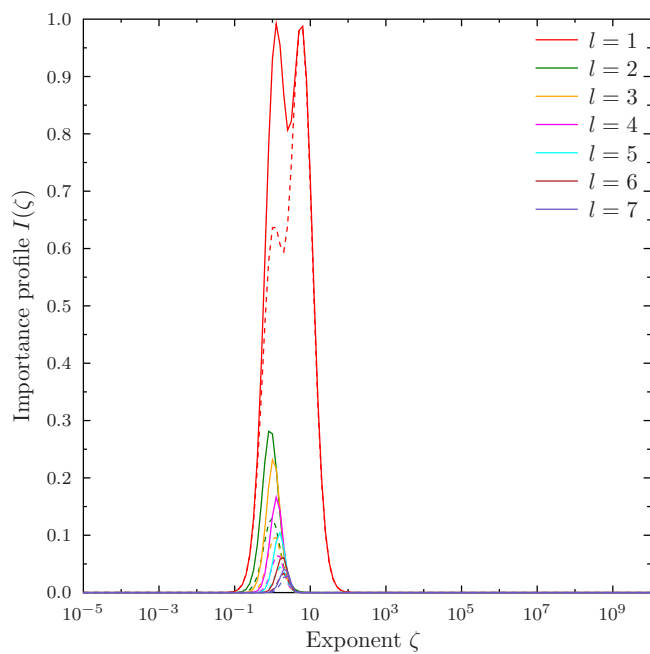

Figure 306. STO importance profile for  $\pi_+$  orbitals on S atom in  $S_2$ .

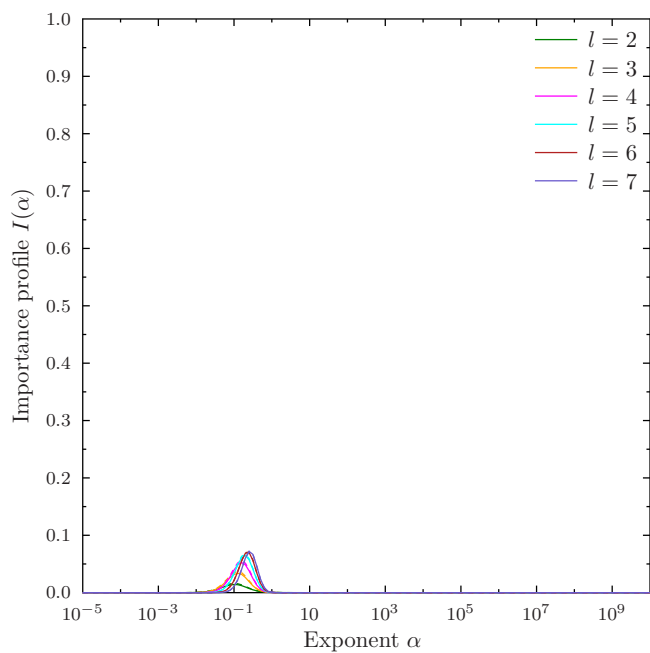

Figure 308. GTO importance profile for  $\delta_-$  orbitals on S atom in NiS.

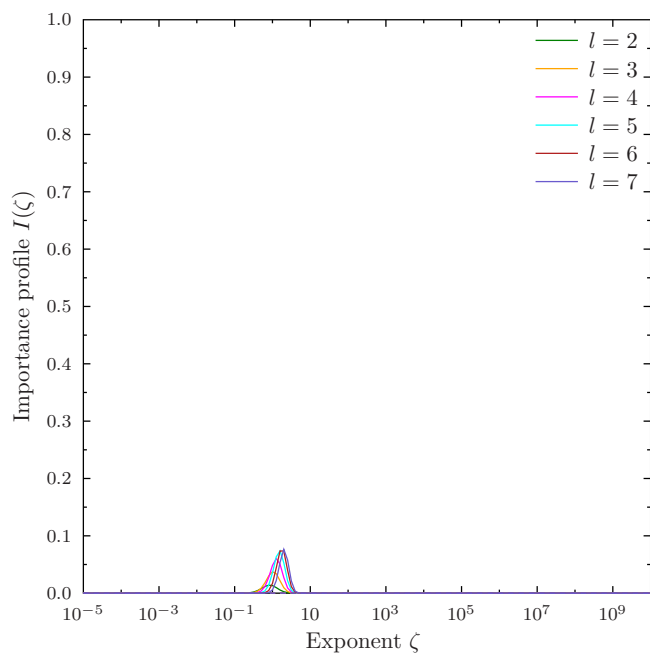

Figure 309. STO importance profile for  $\delta_-$  orbitals on S atom in MnS.

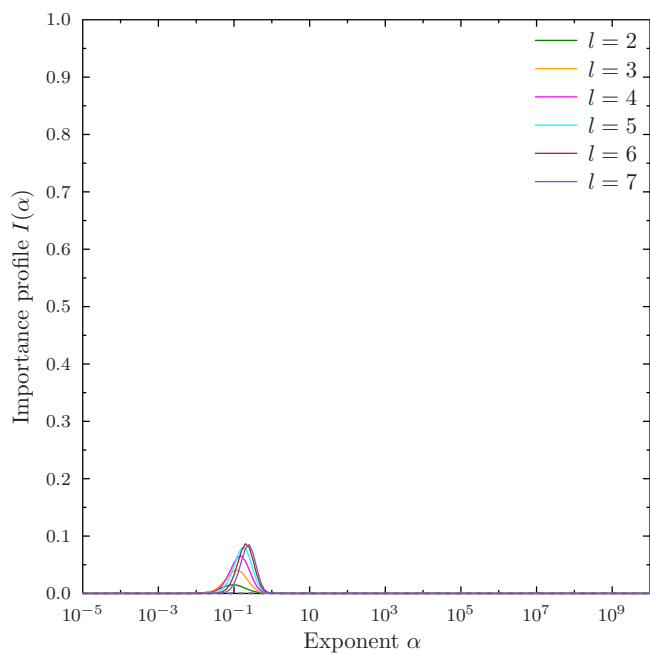

Figure 311. GTO importance profile for  $\delta_+$  orbitals on S atom in MnS.

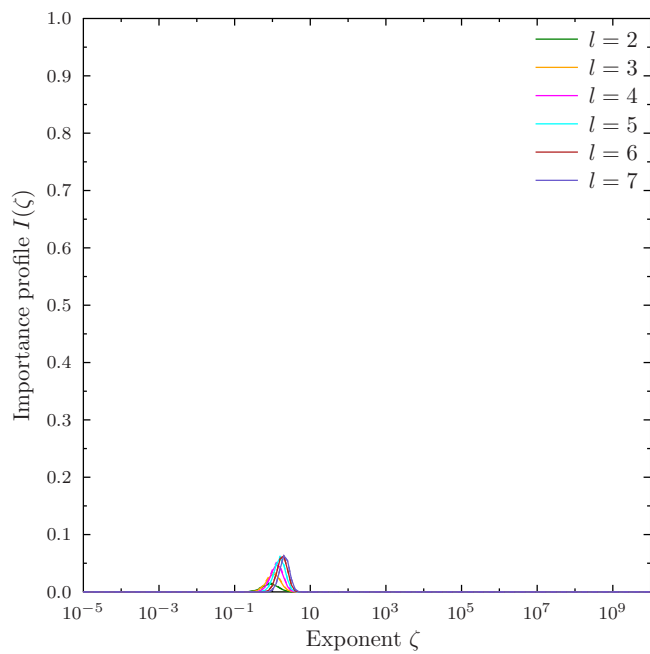

Figure 310. STO importance profile for  $\delta_-$  orbitals on S atom in NiS.

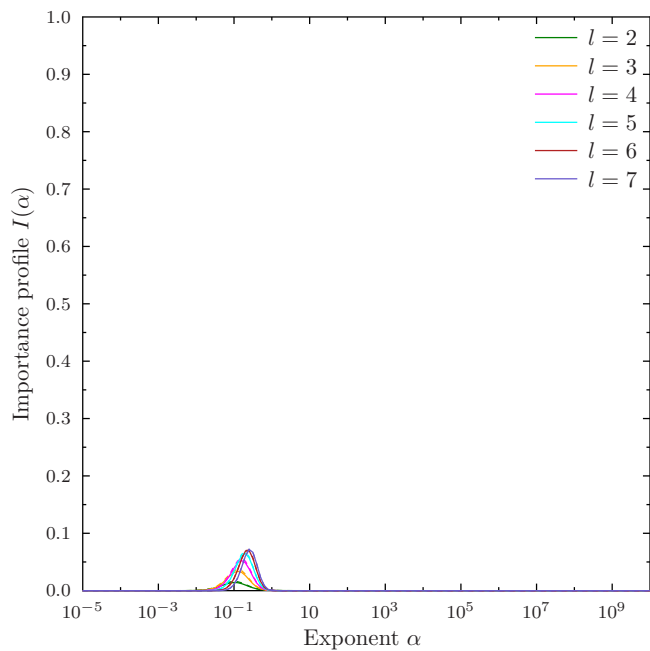

Figure 312. GTO importance profile for  $\delta_+$  orbitals on S atom in NiS.

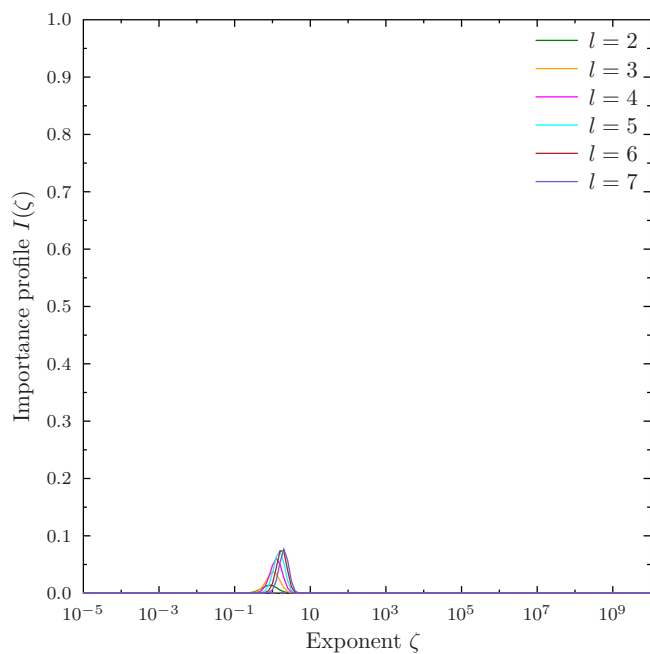

Figure 313. STO importance profile for  $\delta_+$  orbitals on S atom in MnS.

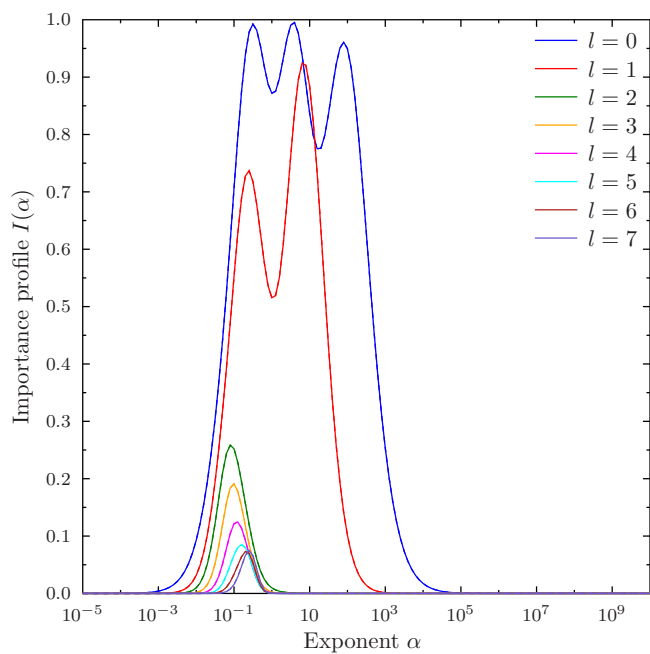

Figure 315. GTO importance profile for  $\sigma$  orbitals on Cl atom in BrCl.

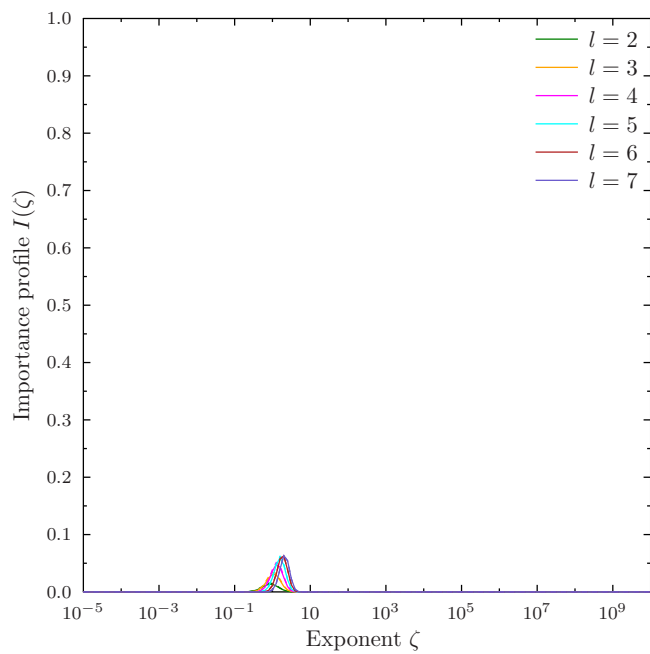

Figure 314. STO importance profile for  $\delta_+$  orbitals on S atom in NiS.

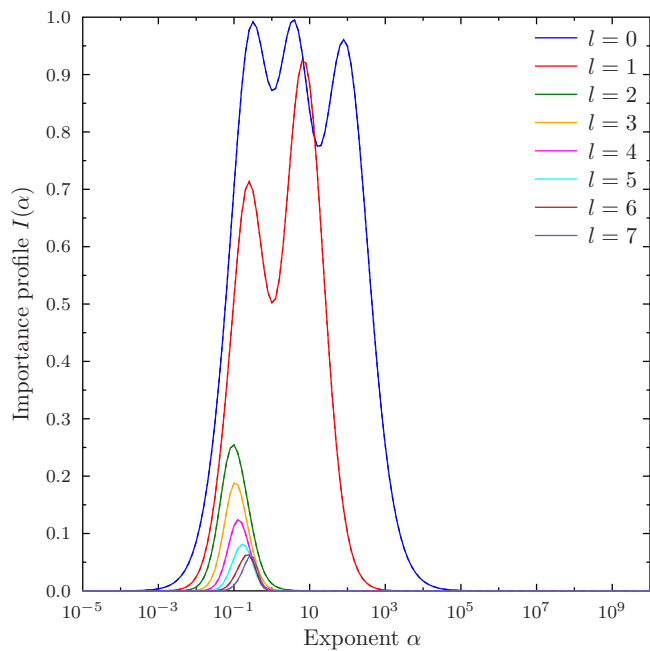

Figure 316. GTO importance profile for  $\sigma$  orbitals on Cl atom in  $\text{Cl}_2$ .

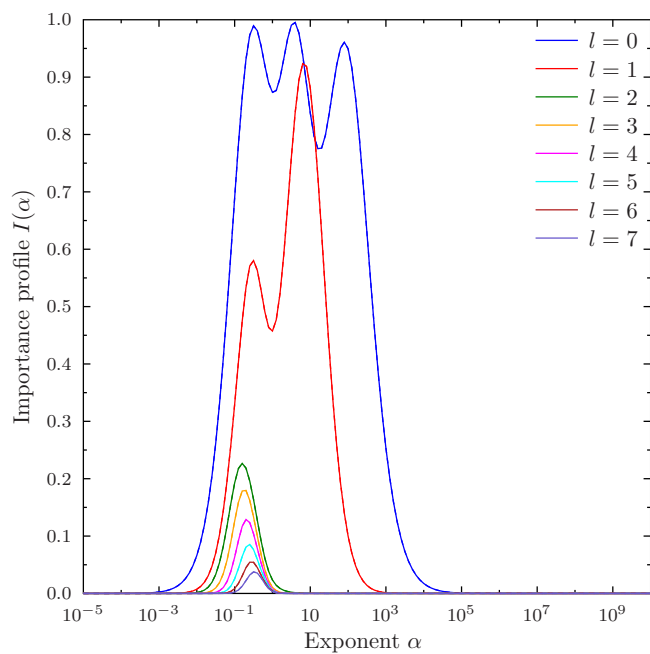

Figure 317. GTO importance profile for  $\sigma$  orbitals on Cl atom in ClF.

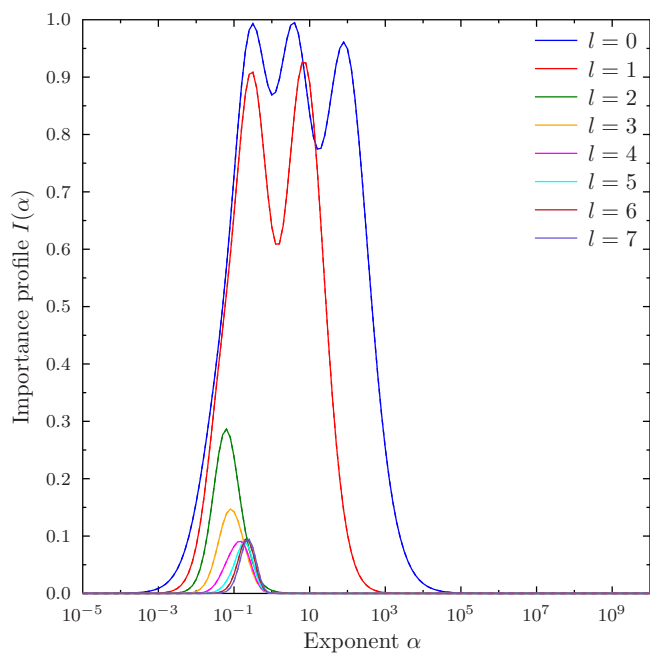

Figure 319. GTO importance profile for  $\sigma$  orbitals on Cl atom in GaCl.

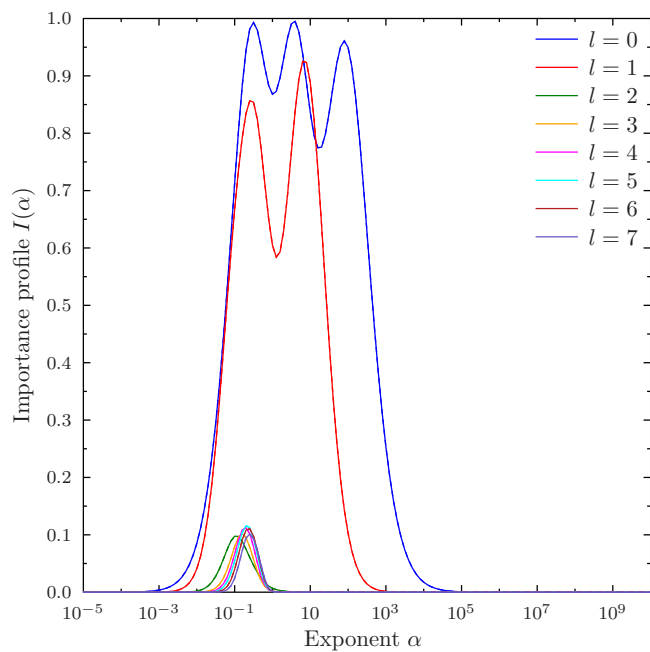

Figure 318. GTO importance profile for  $\sigma$  orbitals on Cl atom in CuCl.

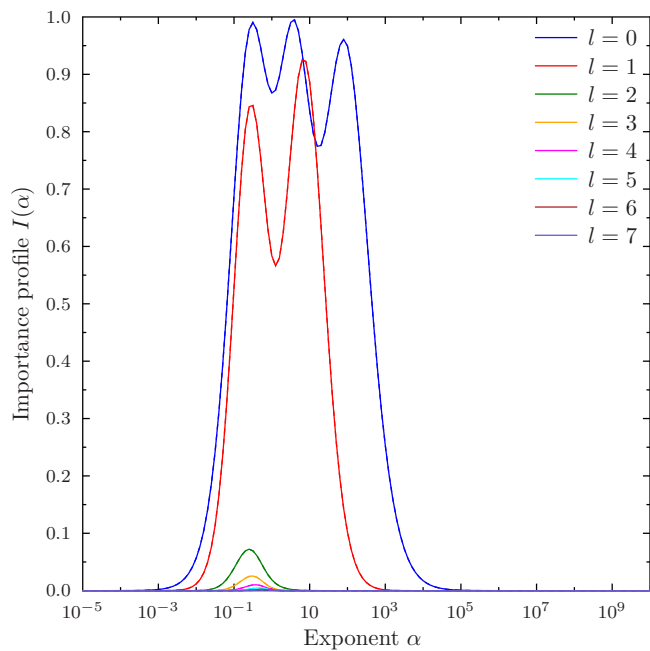

Figure 320. GTO importance profile for  $\sigma$  orbitals on Cl atom in HCl.

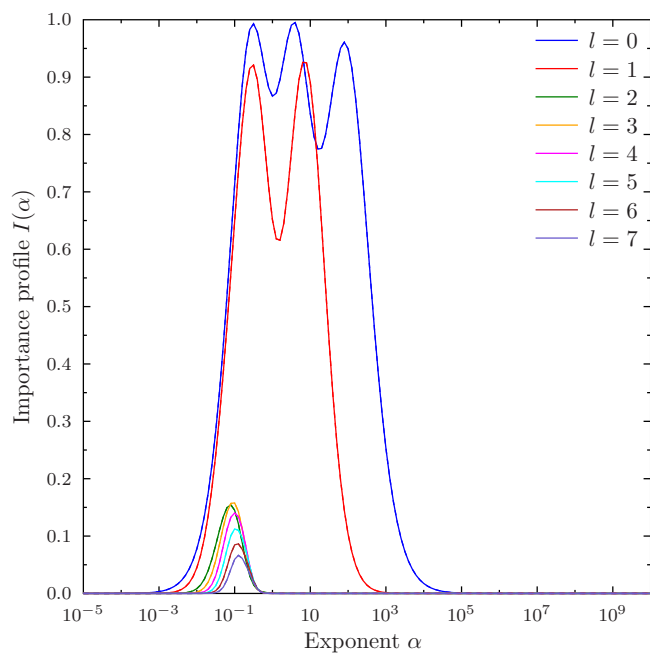

Figure 321. GTO importance profile for  $\sigma$  orbitals on Cl atom in KCl.

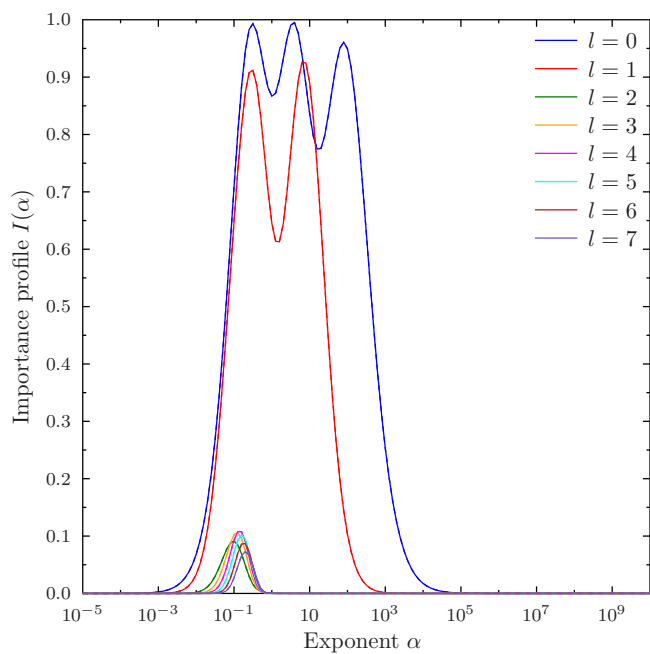

Figure 323. GTO importance profile for  $\sigma$  orbitals on Cl atom in NaCl.

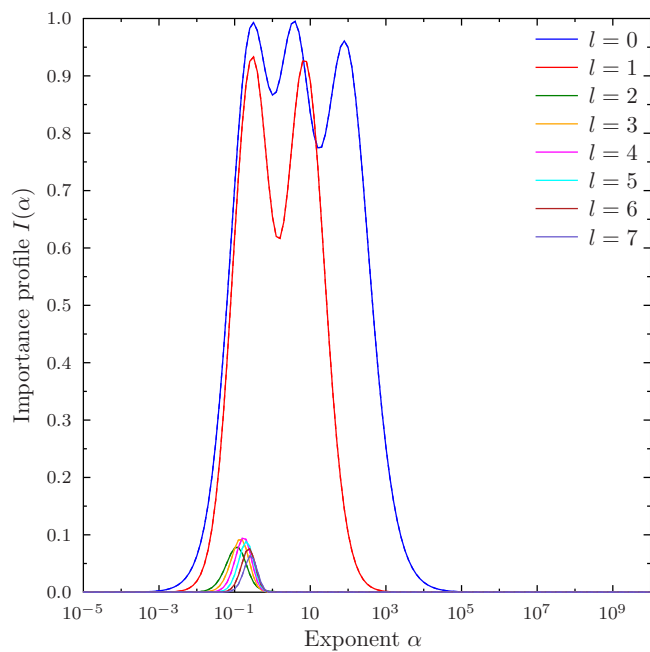

Figure 322. GTO importance profile for  $\sigma$  orbitals on Cl atom in LiCl.

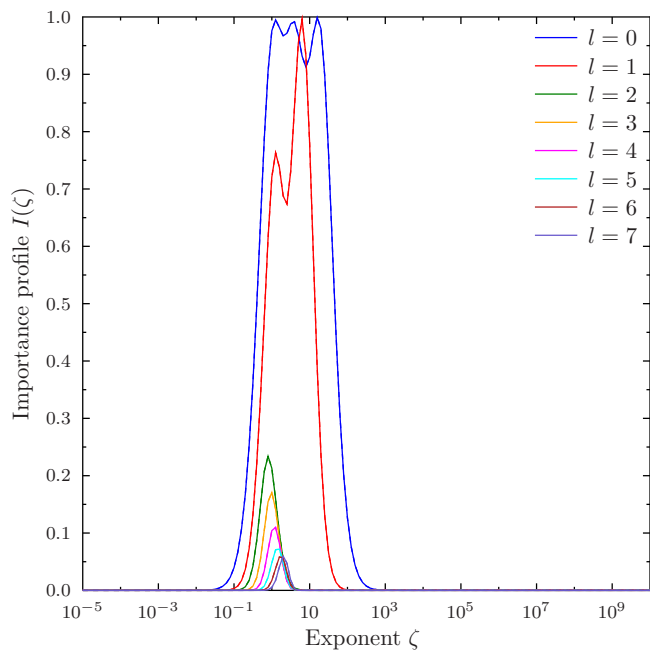

Figure 324. STO importance profile for  $\sigma$  orbitals on Cl atom in BrCl.

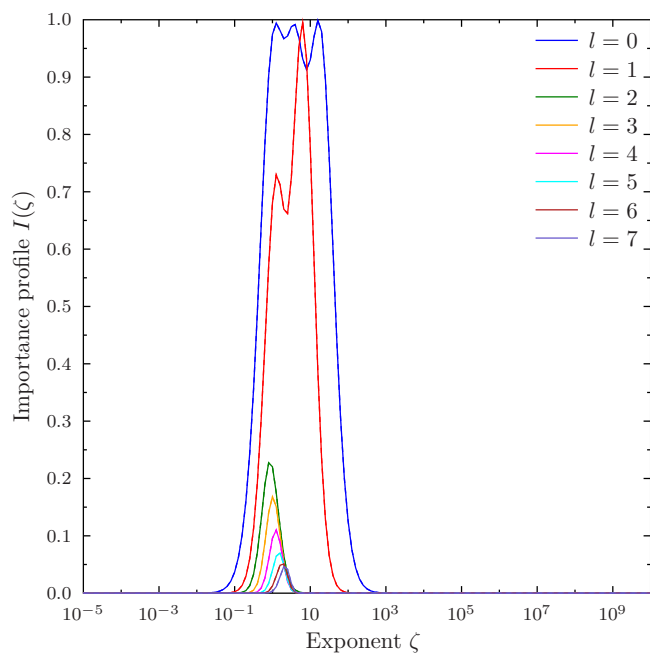

Figure 325. STO importance profile for  $\sigma$  orbitals on Cl atom in  $\text{Cl}_2$ .

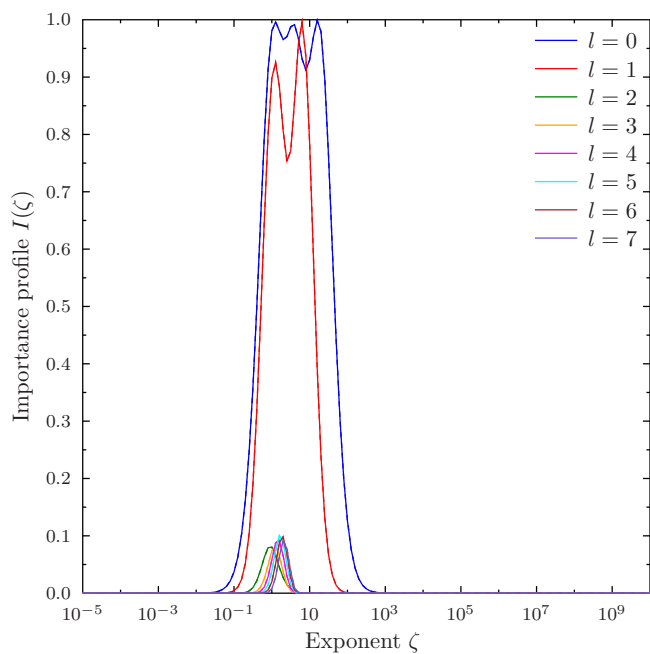

Figure 327. STO importance profile for  $\sigma$  orbitals on Cl atom in  $\text{CuCl}$ .

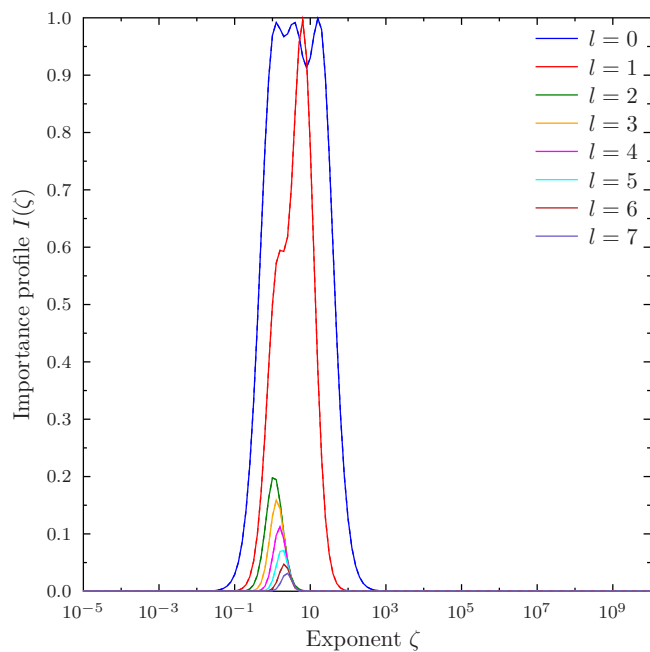

Figure 326. STO importance profile for  $\sigma$  orbitals on Cl atom in  $\text{ClF}$ .

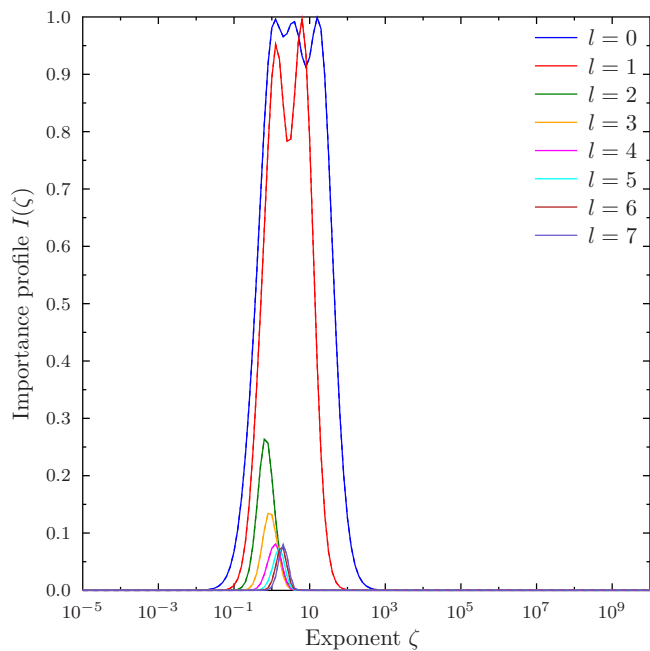

Figure 328. STO importance profile for  $\sigma$  orbitals on Cl atom in  $\text{GaCl}$ .

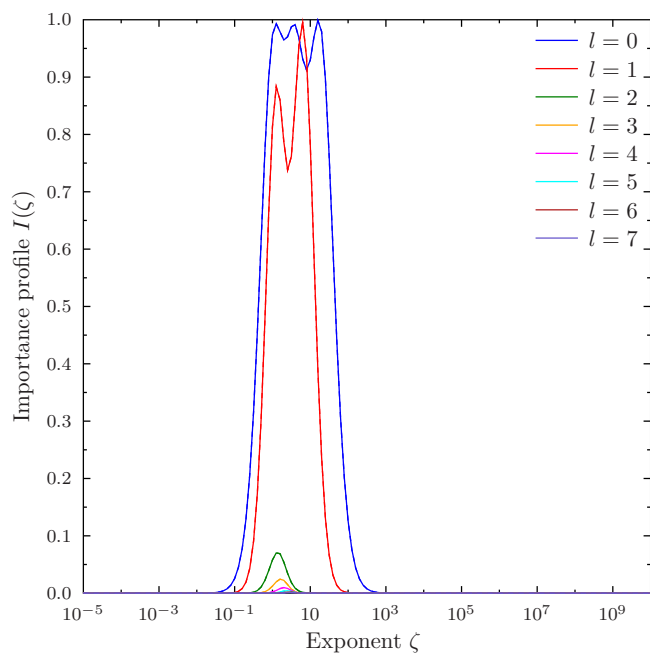

Figure 329. STO importance profile for  $\sigma$  orbitals on Cl atom in HCl.

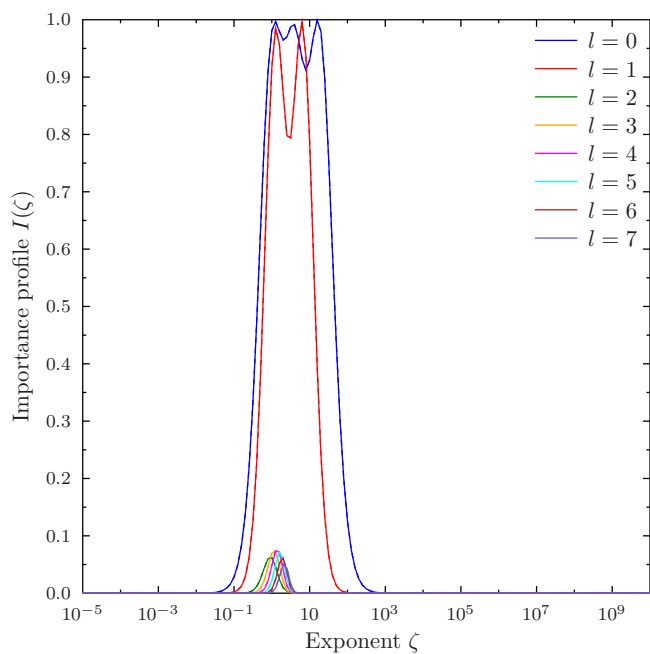

Figure 331. STO importance profile for  $\sigma$  orbitals on Cl atom in LiCl.

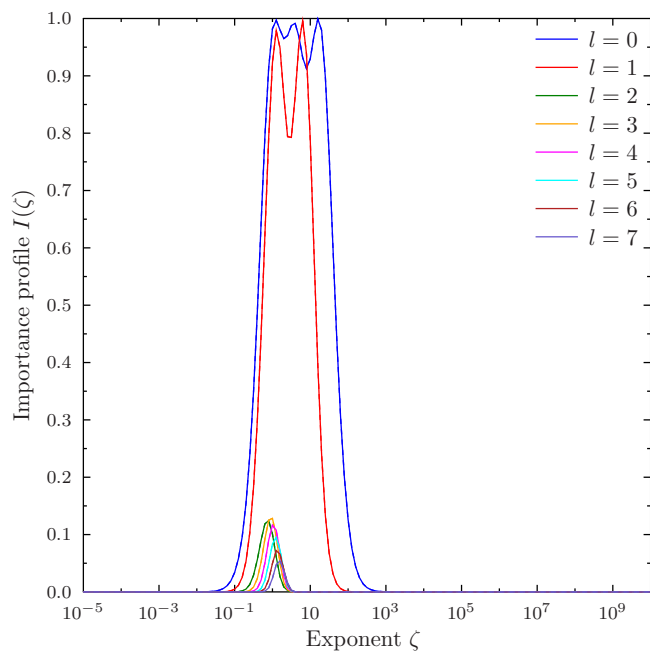

Figure 330. STO importance profile for  $\sigma$  orbitals on Cl atom in KCl.

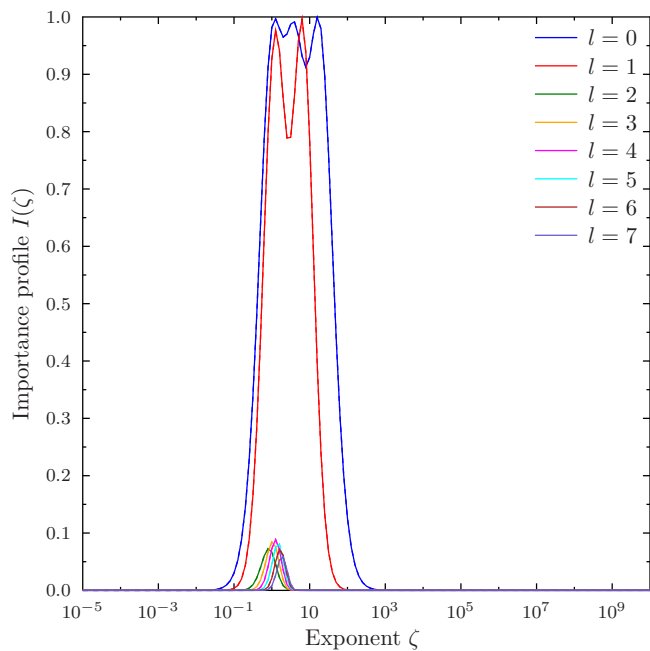

Figure 332. STO importance profile for  $\sigma$  orbitals on Cl atom in NaCl.

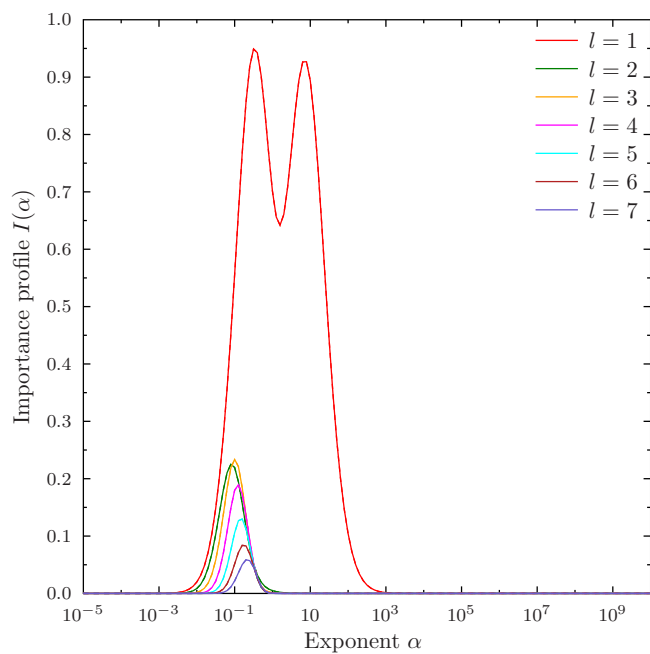

Figure 333. GTO importance profile for  $\pi_-$  orbitals on Cl atom in BrCl.

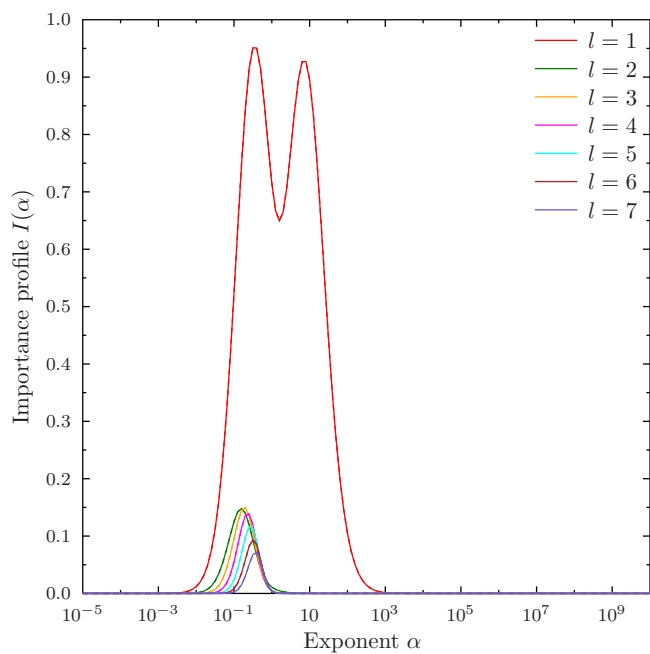

Figure 335. GTO importance profile for  $\pi_-$  orbitals on Cl atom in ClF.

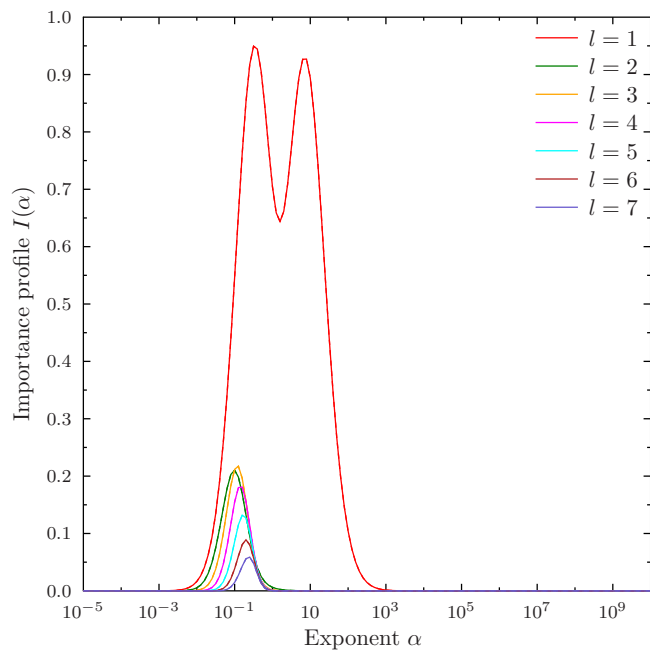

Figure 334. GTO importance profile for  $\pi_-$  orbitals on Cl atom in  $\text{Cl}_2$ .

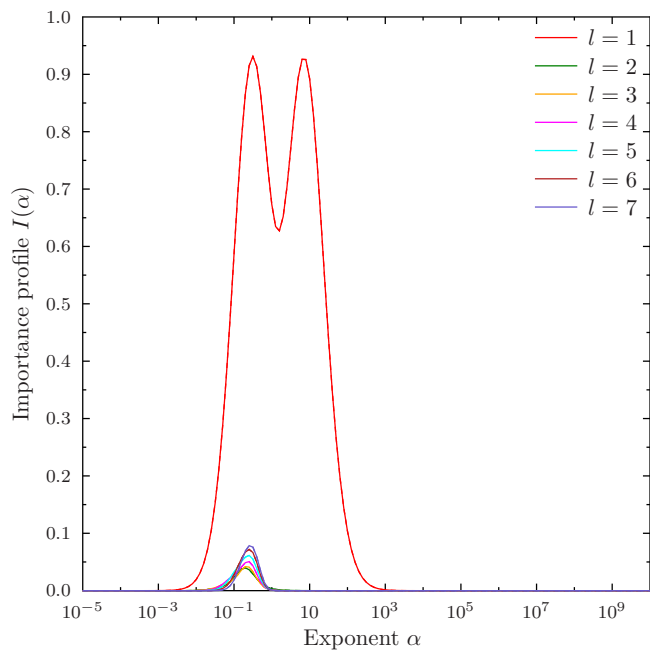

Figure 336. GTO importance profile for  $\pi_-$  orbitals on Cl atom in CuCl.



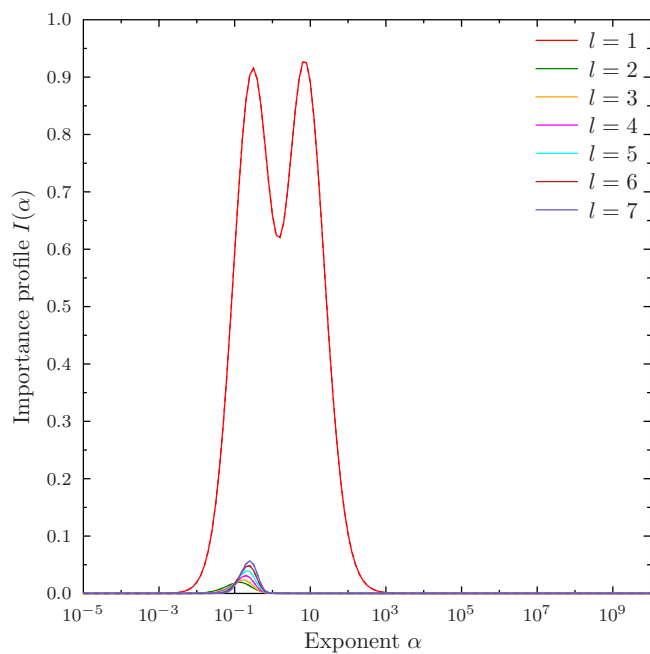

Figure 337. GTO importance profile for  $\pi_-$  orbitals on Cl atom in GaCl.

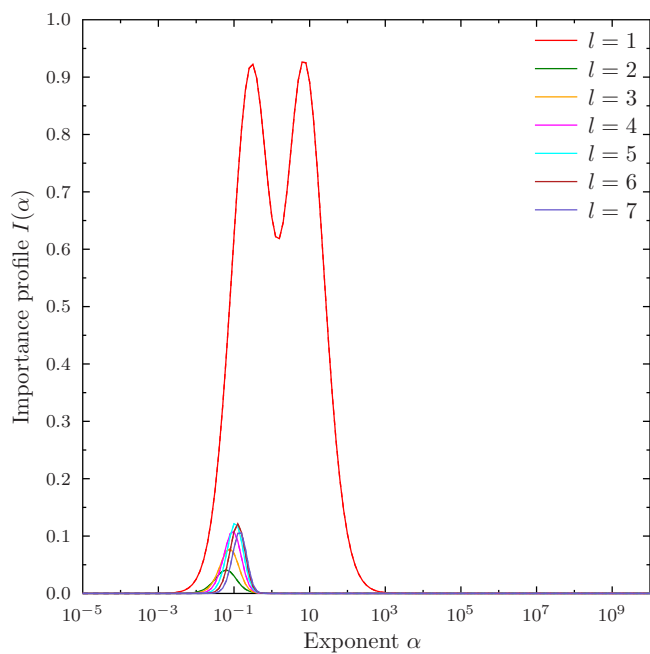

Figure 339. GTO importance profile for  $\pi_-$  orbitals on Cl atom in KCl.

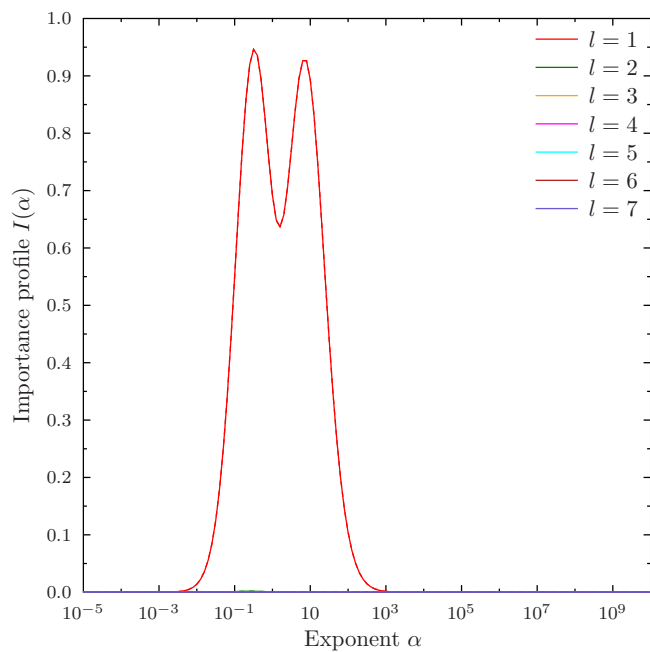

Figure 338. GTO importance profile for  $\pi_-$  orbitals on Cl atom in HCl.

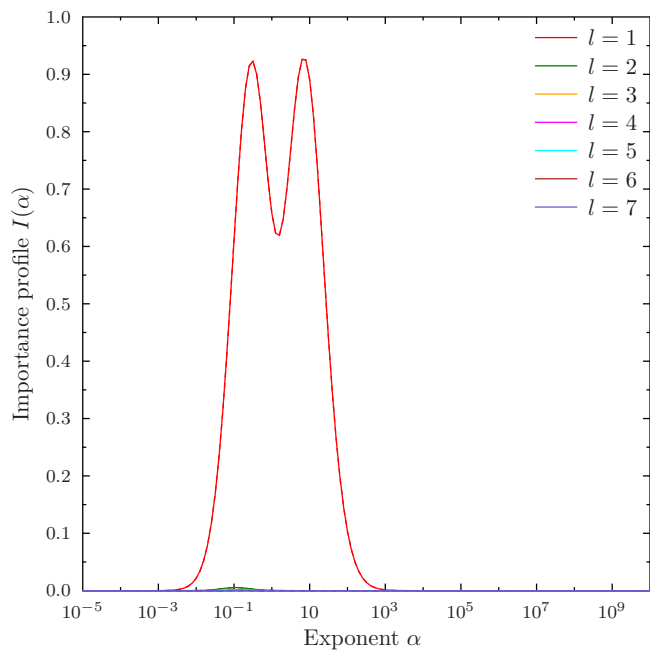

Figure 340. GTO importance profile for  $\pi_-$  orbitals on Cl atom in LiCl.

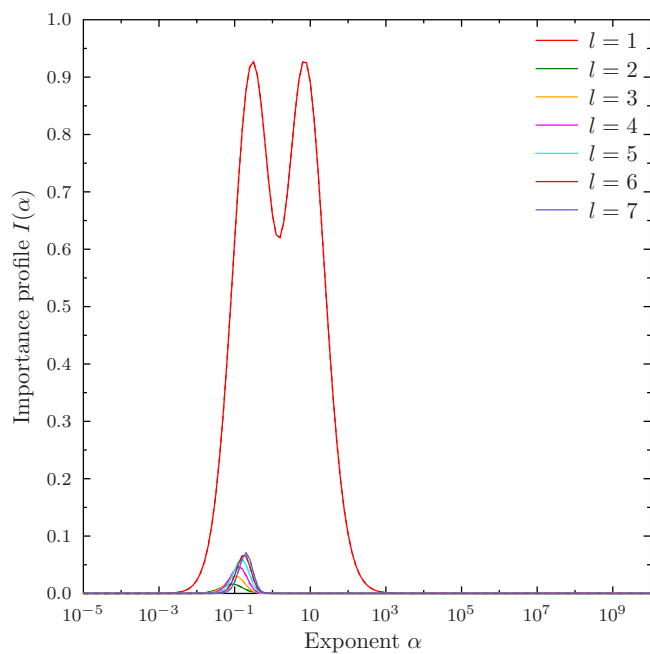

Figure 341. GTO importance profile for  $\pi_-$  orbitals on Cl atom in NaCl.

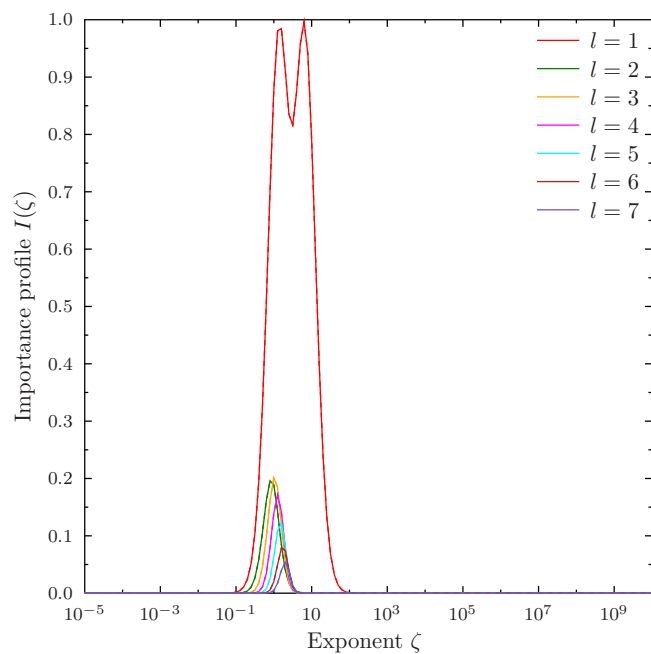

Figure 343. STO importance profile for  $\pi_-$  orbitals on Cl atom in  $\text{Cl}_2$ .

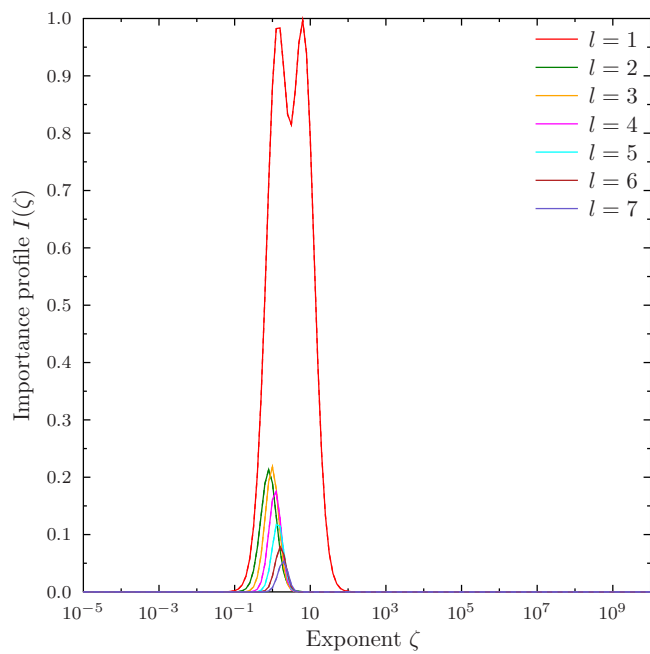

Figure 342. STO importance profile for  $\pi_-$  orbitals on Cl atom in BrCl.

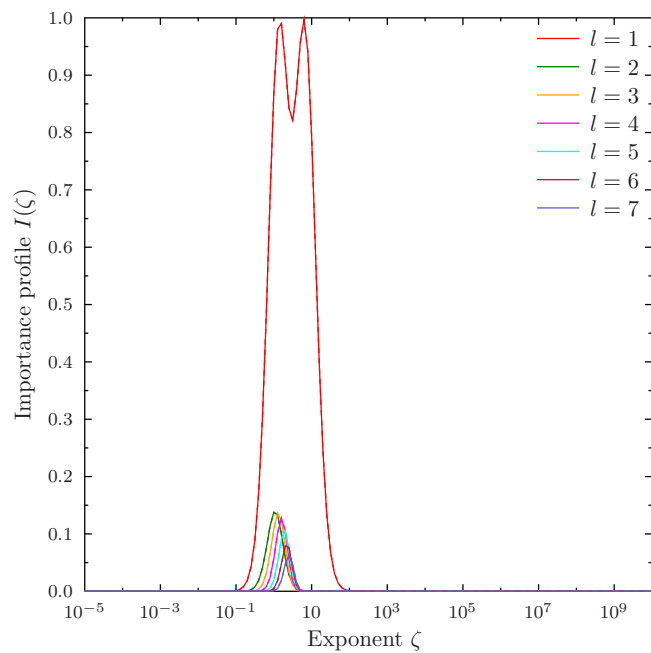

Figure 344. STO importance profile for  $\pi_-$  orbitals on Cl atom in ClF.

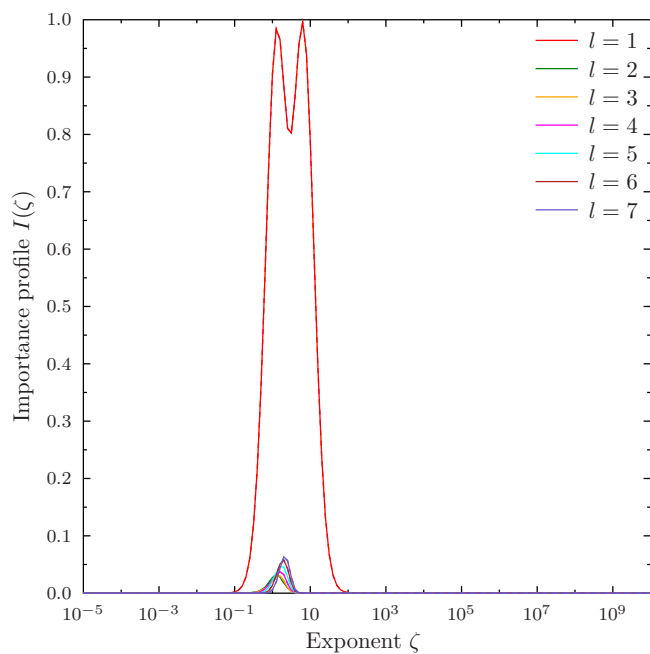

Figure 345. STO importance profile for  $\pi_-$  orbitals on Cl atom in CuCl.

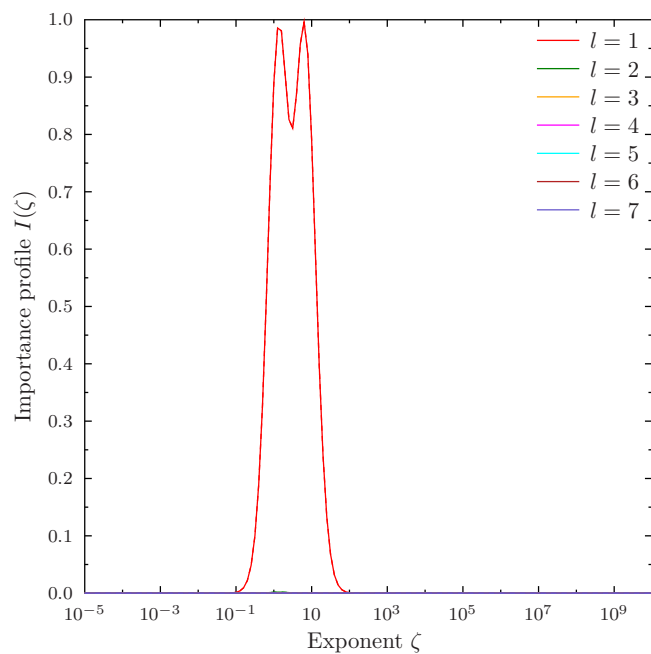

Figure 347. STO importance profile for  $\pi_-$  orbitals on Cl atom in HCl.

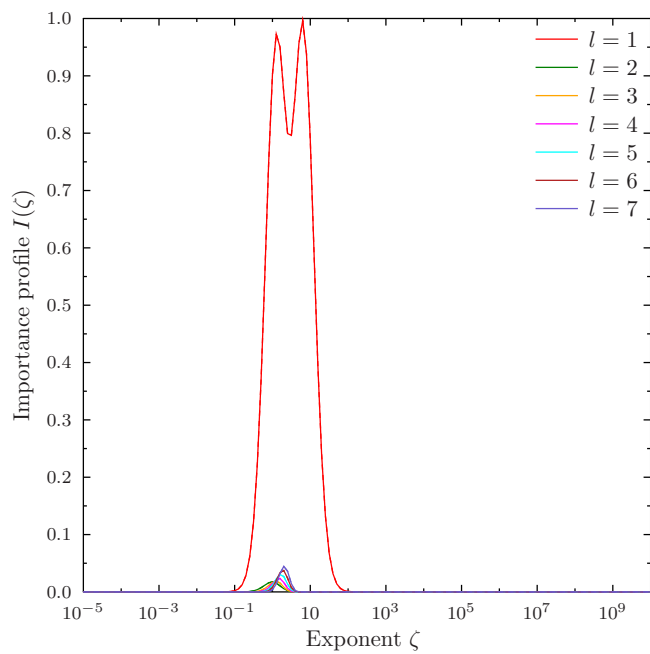

Figure 346. STO importance profile for  $\pi_-$  orbitals on Cl atom in GaCl.

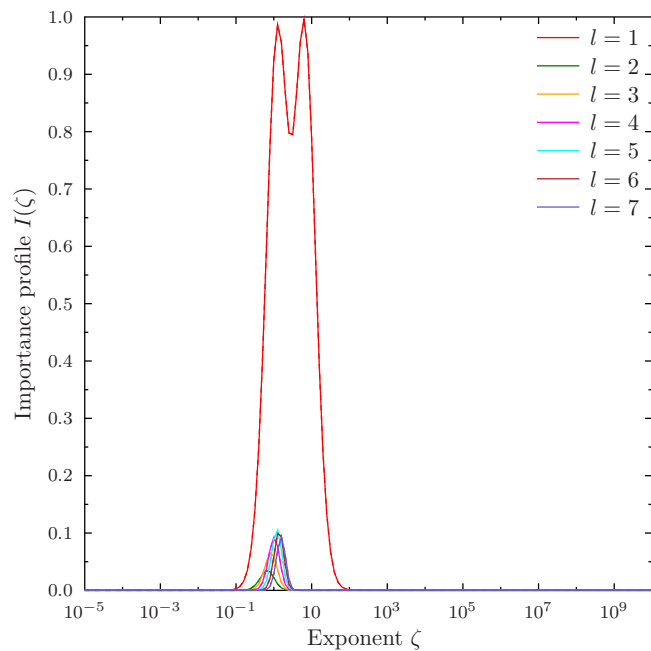

Figure 348. STO importance profile for  $\pi_-$  orbitals on Cl atom in KCl.

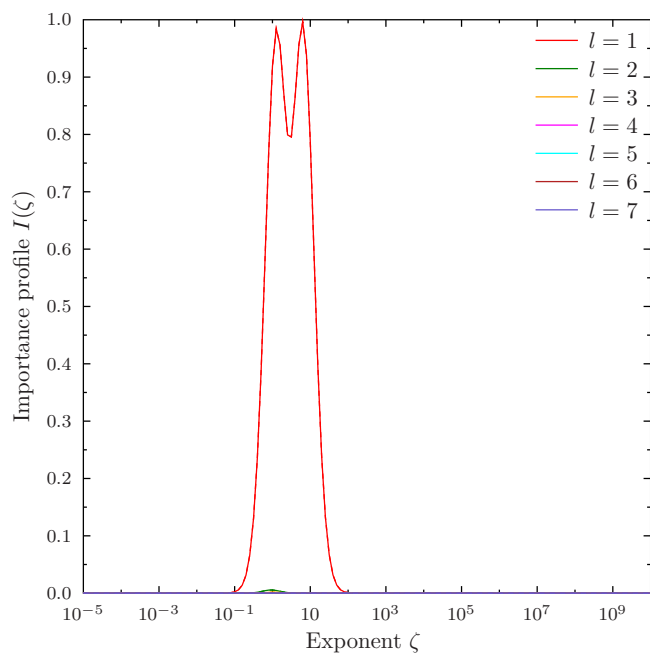

Figure 349. STO importance profile for  $\pi_-$  orbitals on Cl atom in LiCl.

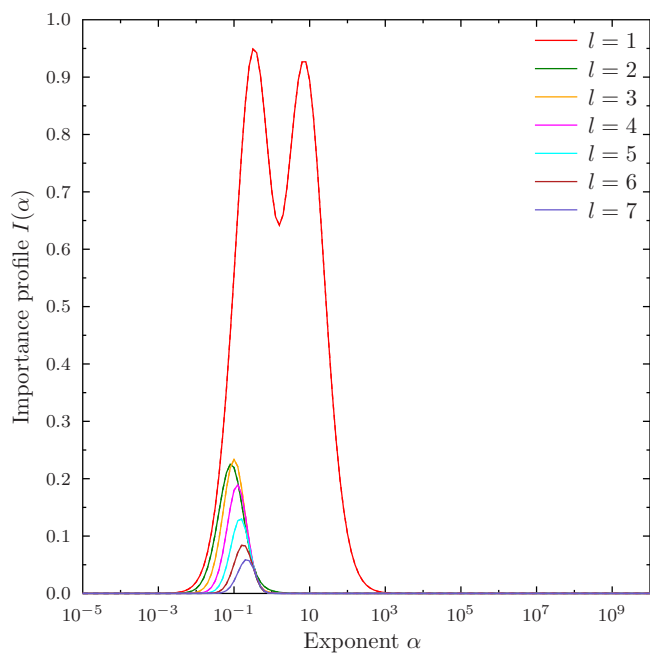

Figure 351. GTO importance profile for  $\pi_+$  orbitals on Cl atom in BrCl.

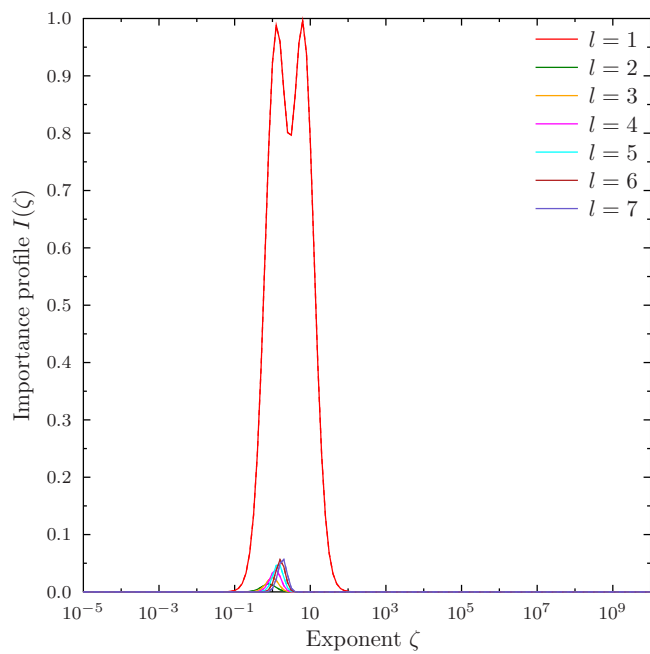

Figure 350. STO importance profile for  $\pi_-$  orbitals on Cl atom in NaCl.

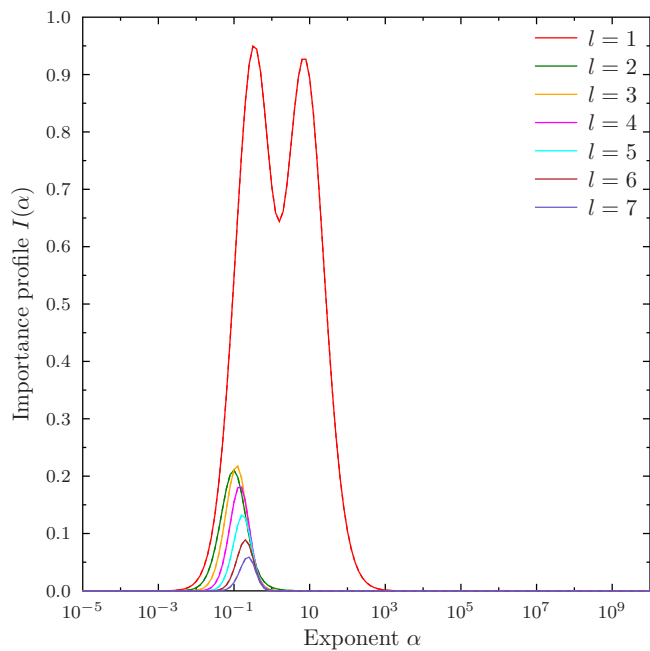

Figure 352. GTO importance profile for  $\pi_+$  orbitals on Cl atom in  $\text{Cl}_2$ .

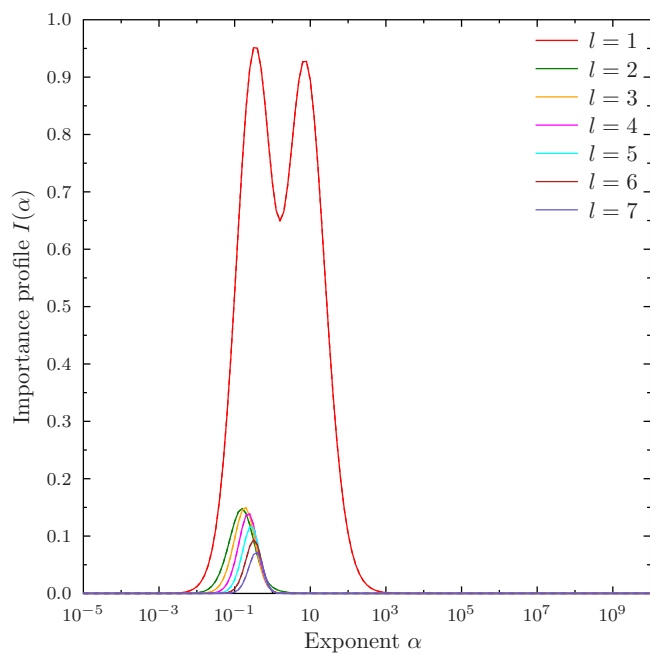

Figure 353. GTO importance profile for  $\pi_+$  orbitals on Cl atom in ClF.

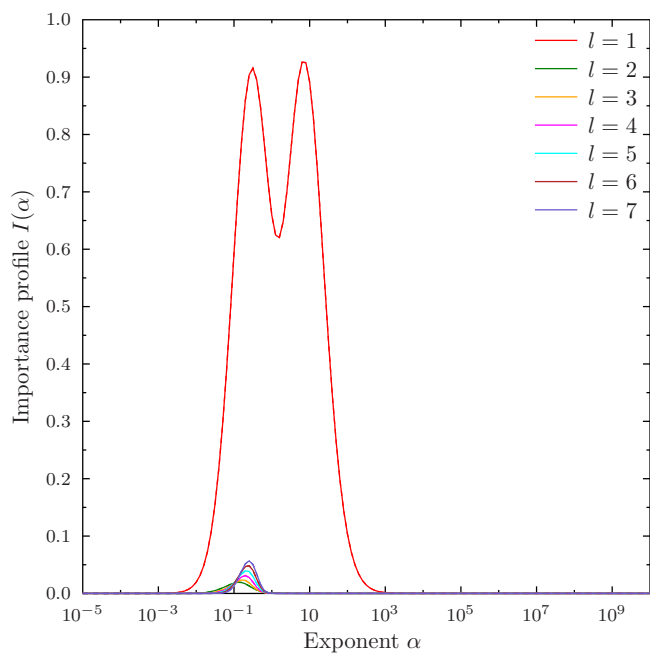

Figure 355. GTO importance profile for  $\pi_+$  orbitals on Cl atom in GaCl.

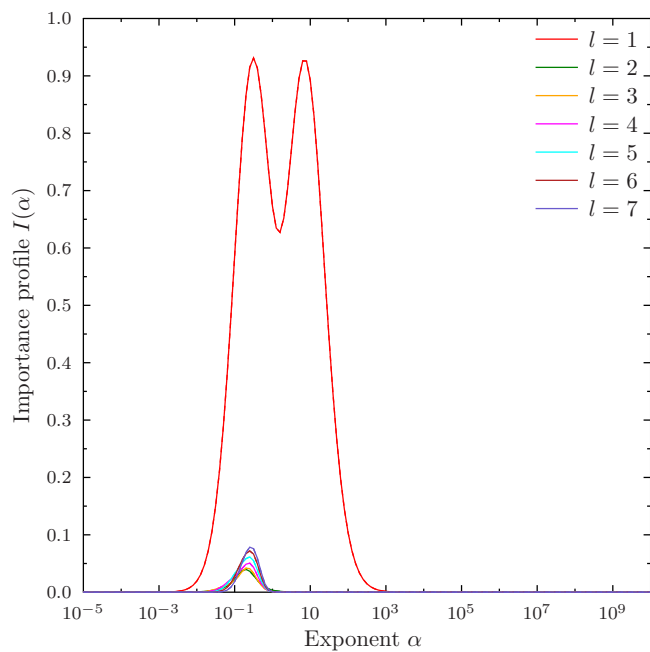

Figure 354. GTO importance profile for  $\pi_+$  orbitals on Cl atom in CuCl.

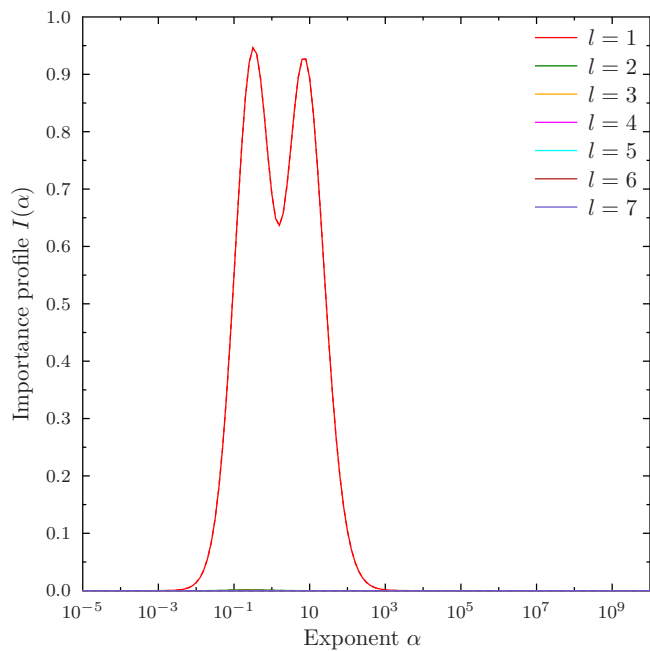

Figure 356. GTO importance profile for  $\pi_+$  orbitals on Cl atom in HCl.

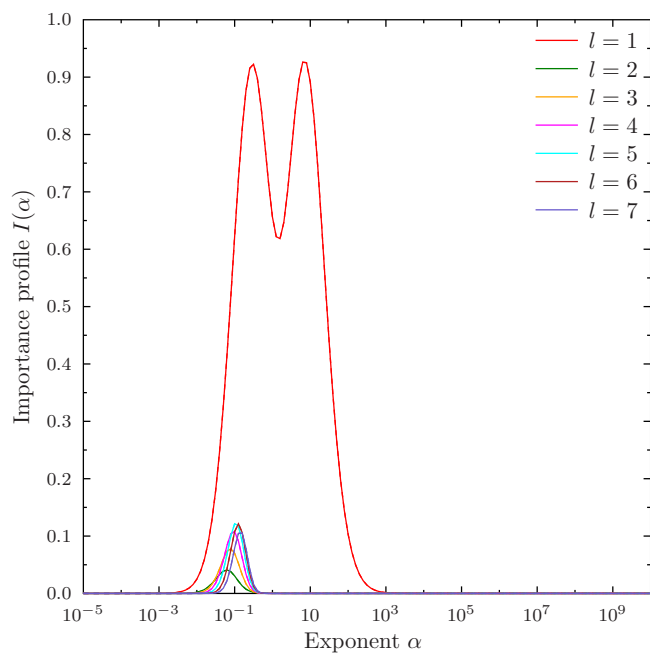

Figure 357. GTO importance profile for  $\pi_+$  orbitals on Cl atom in KCl.

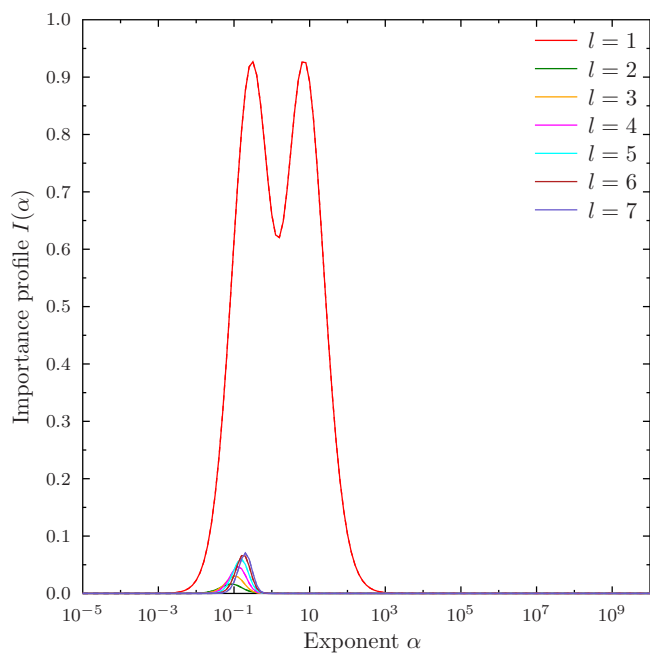

Figure 359. GTO importance profile for  $\pi_+$  orbitals on Cl atom in NaCl.

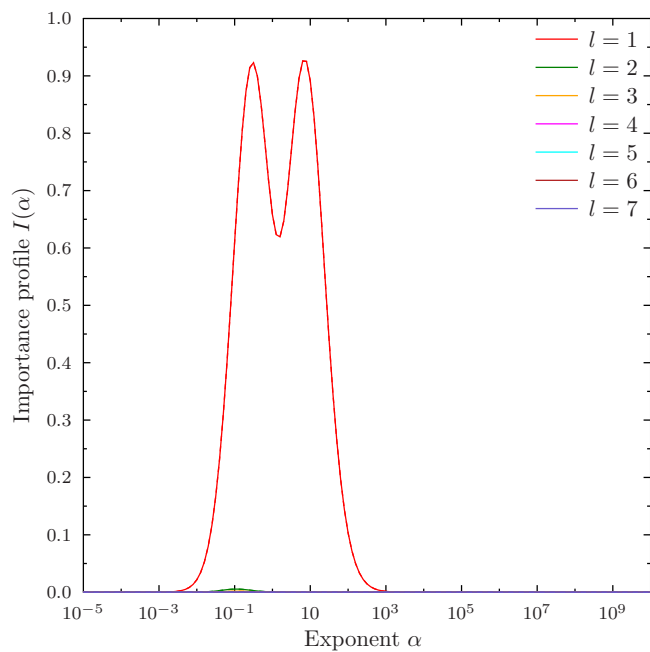

Figure 358. GTO importance profile for  $\pi_+$  orbitals on Cl atom in LiCl.

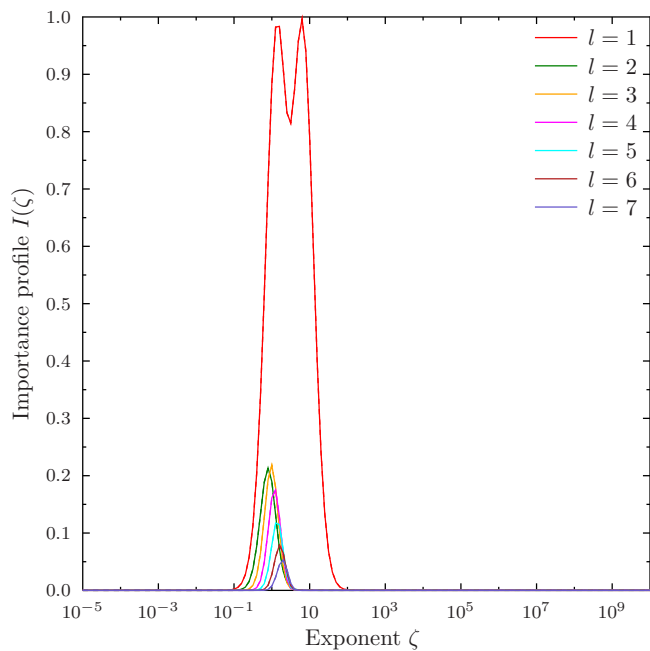

Figure 360. STO importance profile for  $\pi_+$  orbitals on Cl atom in BrCl.

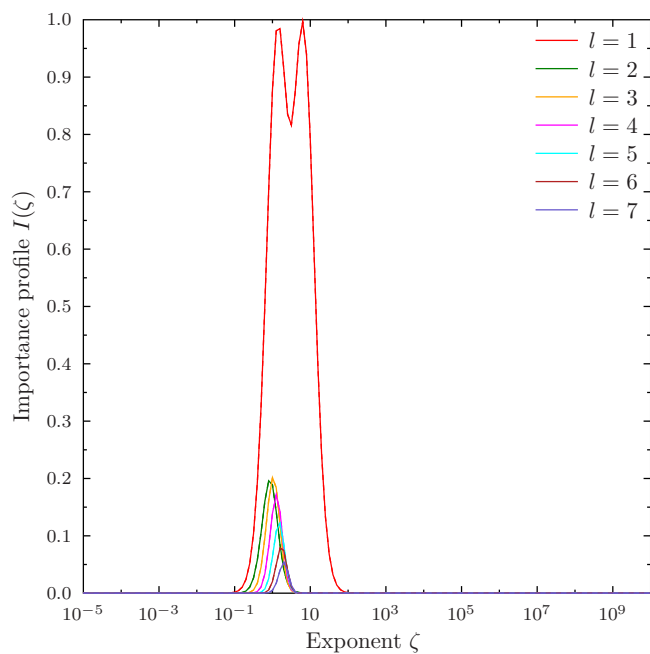

Figure 361. STO importance profile for  $\pi_+$  orbitals on Cl atom in  $\text{Cl}_2$ .

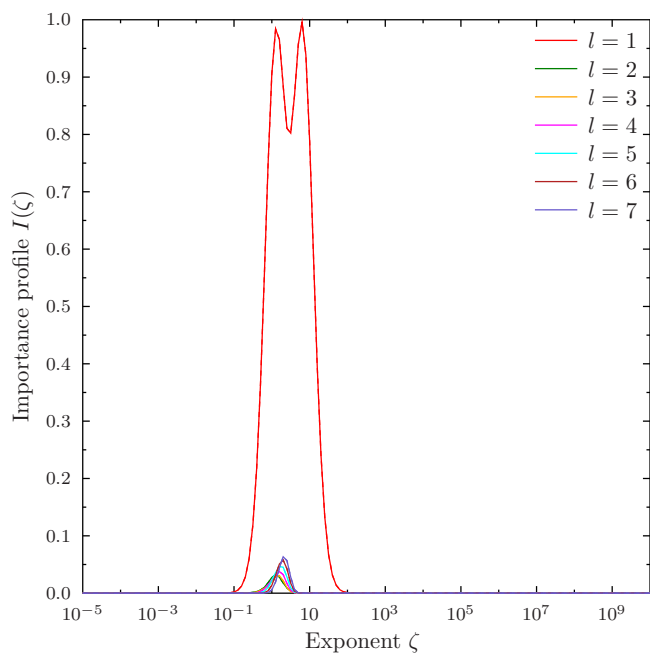

Figure 363. STO importance profile for  $\pi_+$  orbitals on Cl atom in  $\text{CuCl}$ .

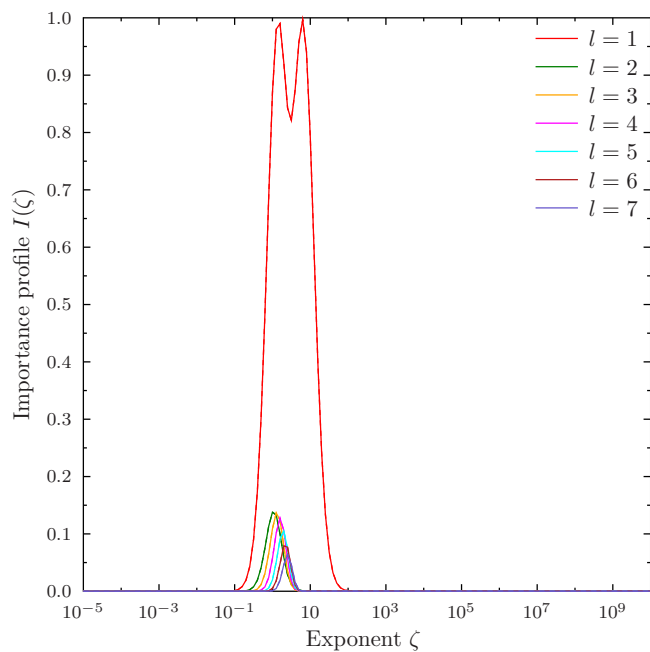

Figure 362. STO importance profile for  $\pi_+$  orbitals on Cl atom in  $\text{ClF}$ .

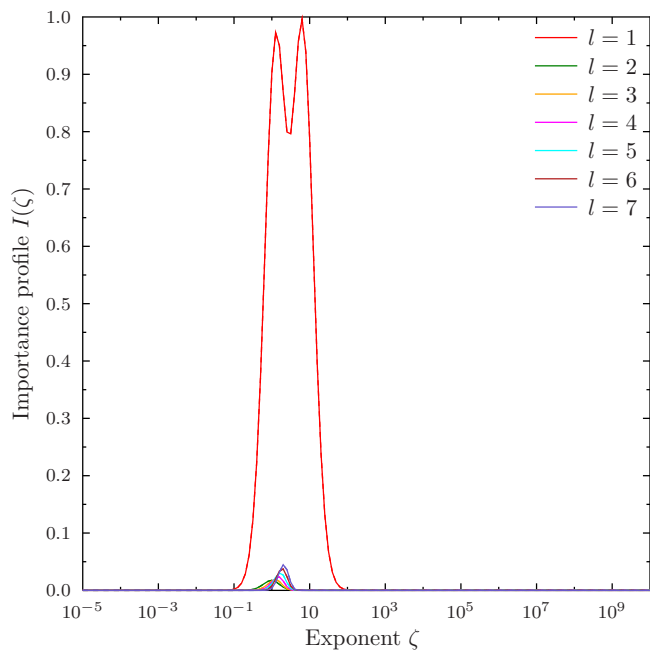

Figure 364. STO importance profile for  $\pi_+$  orbitals on Cl atom in  $\text{GaCl}$ .

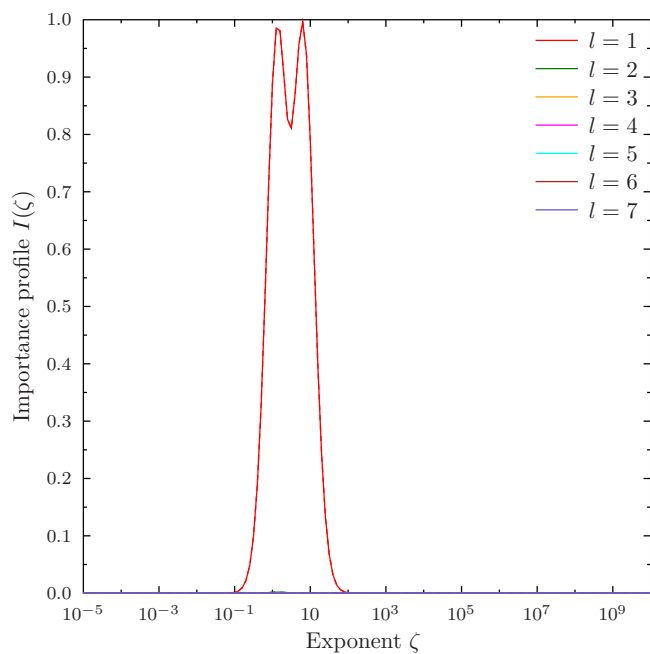

Figure 365. STO importance profile for  $\pi_+$  orbitals on Cl atom in HCl.

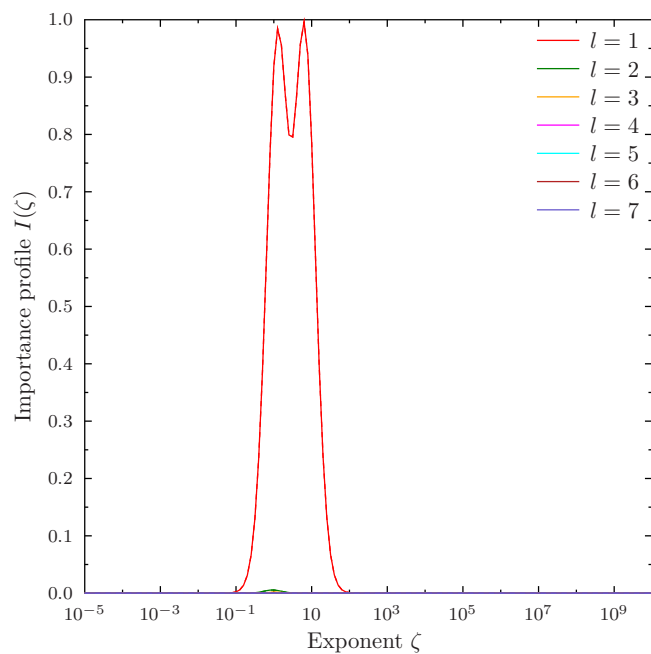

Figure 367. STO importance profile for  $\pi_+$  orbitals on Cl atom in LiCl.

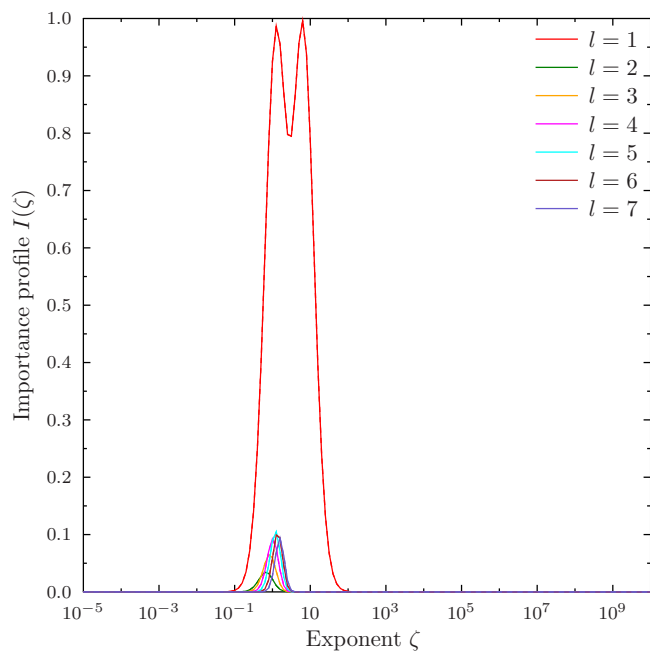

Figure 366. STO importance profile for  $\pi_+$  orbitals on Cl atom in KCl.

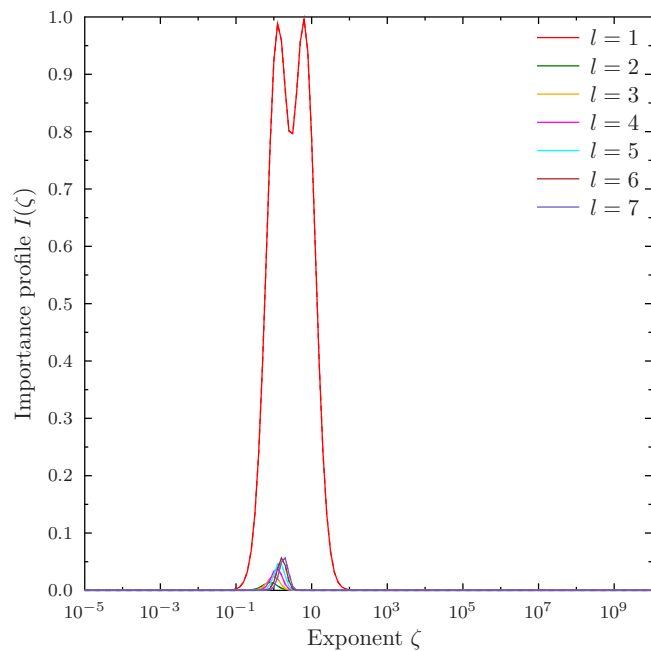

Figure 368. STO importance profile for  $\pi_+$  orbitals on Cl atom in NaCl.



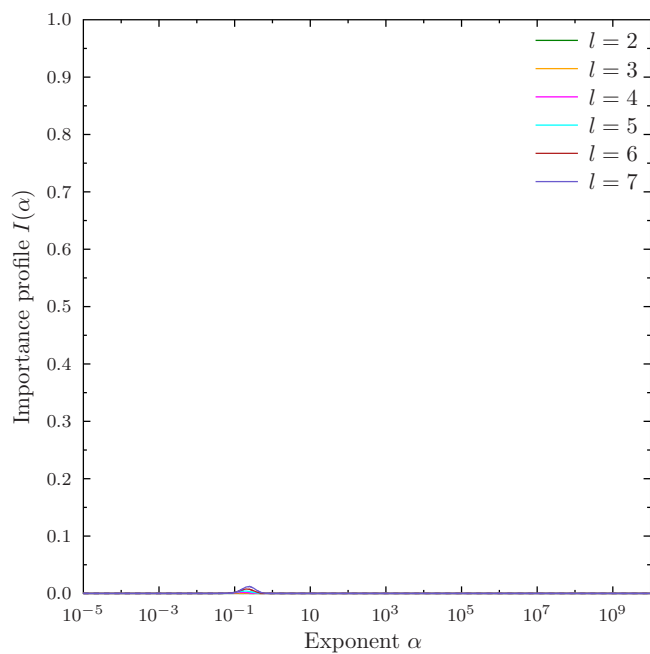

Figure 369. GTO importance profile for  $\delta_-$  orbitals on Cl atom in BrCl.

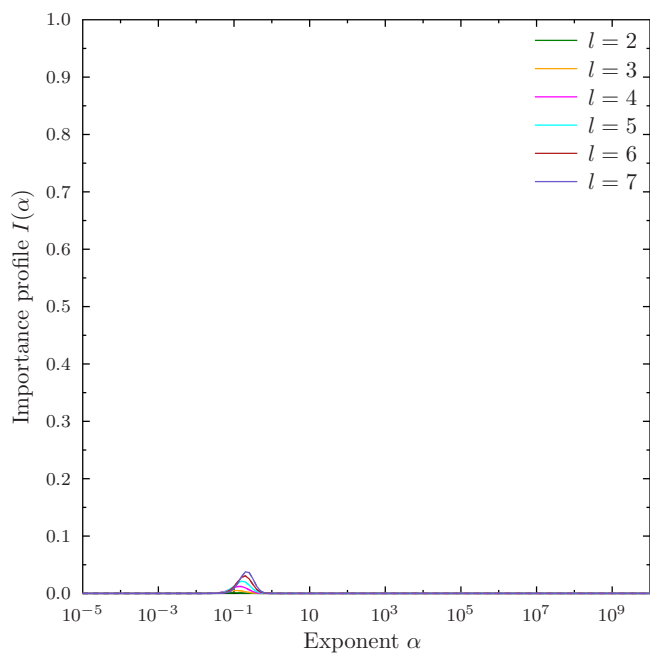

Figure 371. GTO importance profile for  $\delta_-$  orbitals on Cl atom in GaCl.

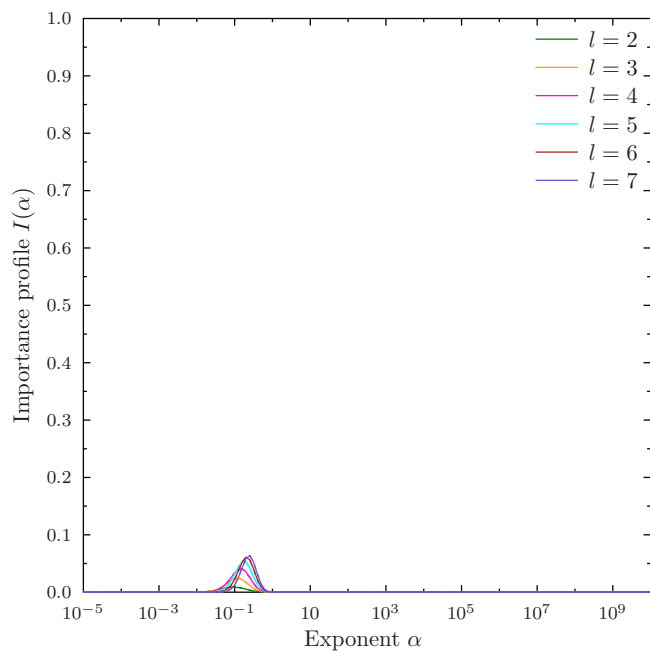

Figure 370. GTO importance profile for  $\delta_-$  orbitals on Cl atom in CuCl.

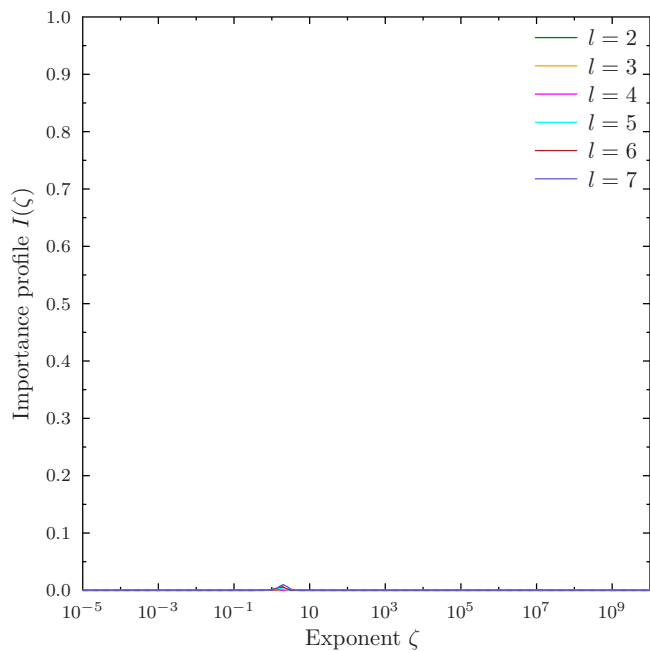

Figure 372. STO importance profile for  $\delta_-$  orbitals on Cl atom in BrCl.

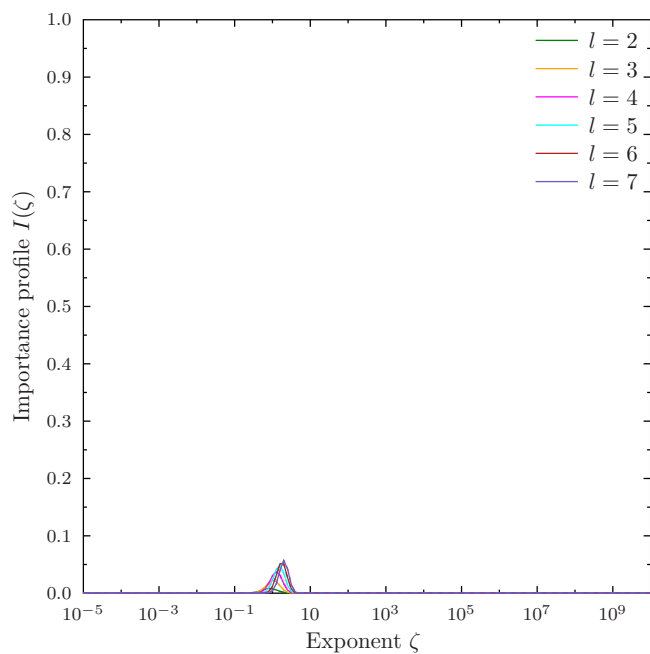

Figure 373. STO importance profile for  $\delta_-$  orbitals on Cl atom in CuCl.

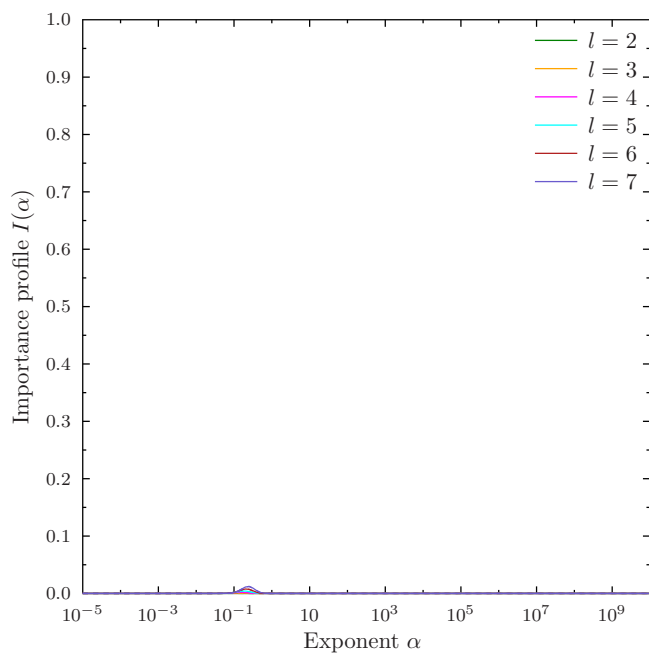

Figure 375. GTO importance profile for  $\delta_+$  orbitals on Cl atom in BrCl.

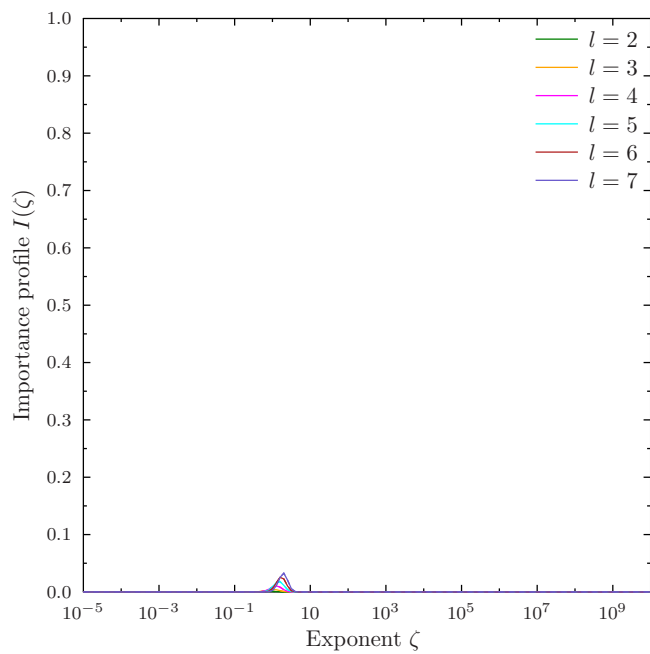

Figure 374. STO importance profile for  $\delta_-$  orbitals on Cl atom in GaCl.

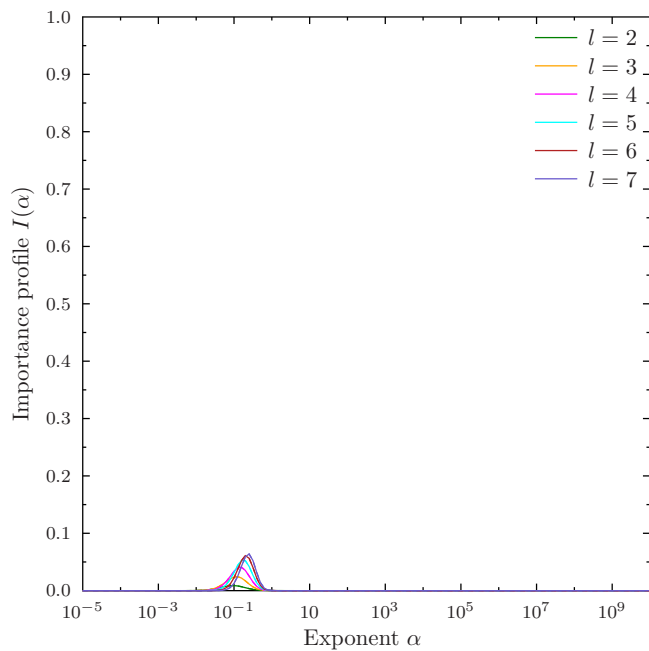

Figure 376. GTO importance profile for  $\delta_+$  orbitals on Cl atom in CuCl.

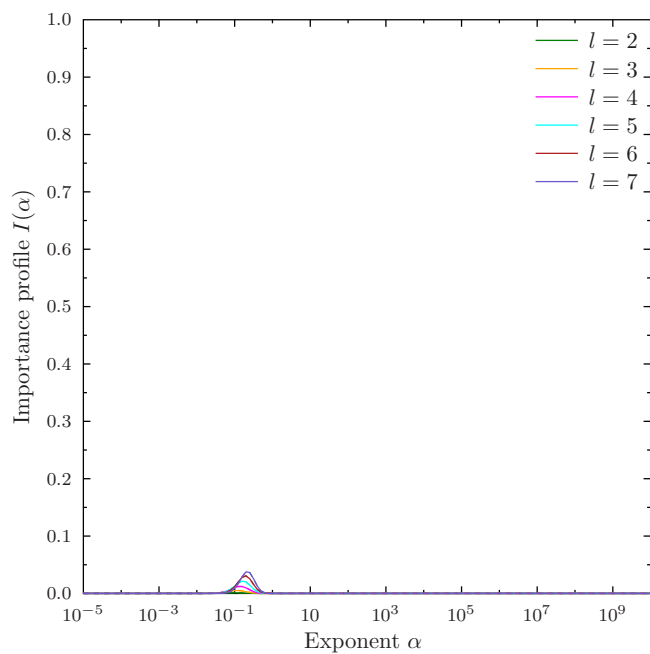

Figure 377. GTO importance profile for  $\delta_+$  orbitals on Cl atom in GaCl.

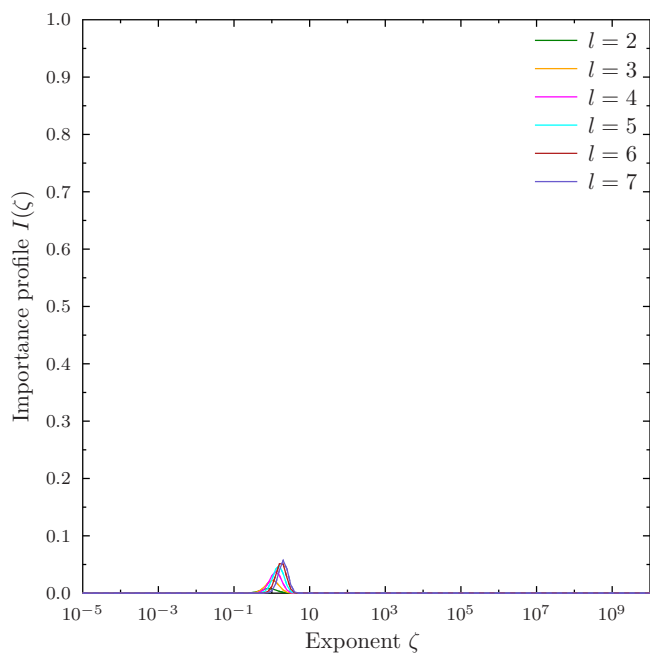

Figure 379. STO importance profile for  $\delta_+$  orbitals on Cl atom in CuCl.

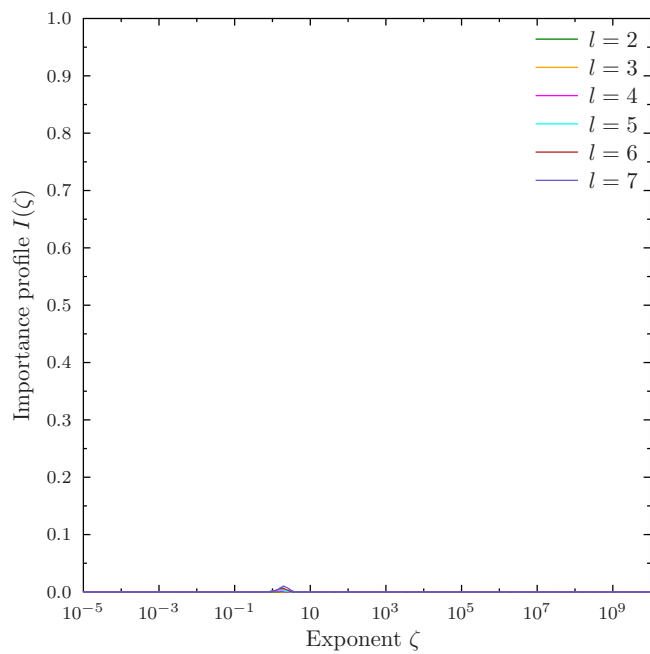

Figure 378. STO importance profile for  $\delta_+$  orbitals on Cl atom in BrCl.

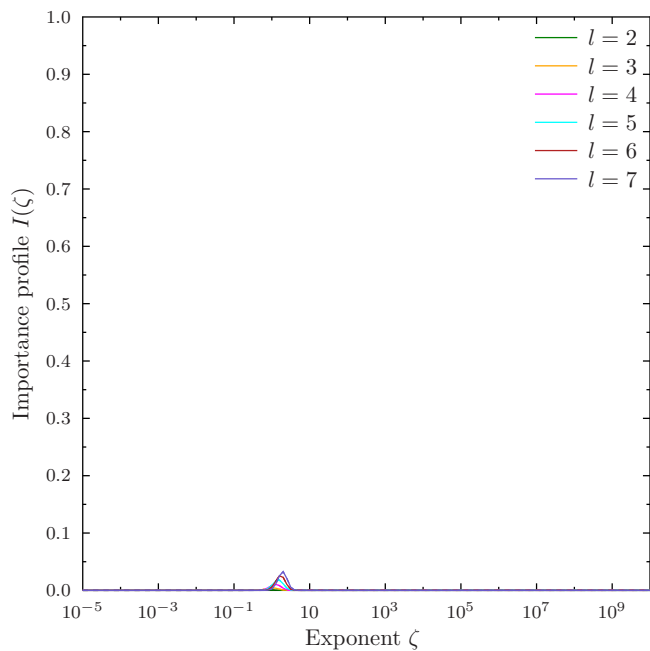

Figure 380. STO importance profile for  $\delta_+$  orbitals on Cl atom in GaCl.

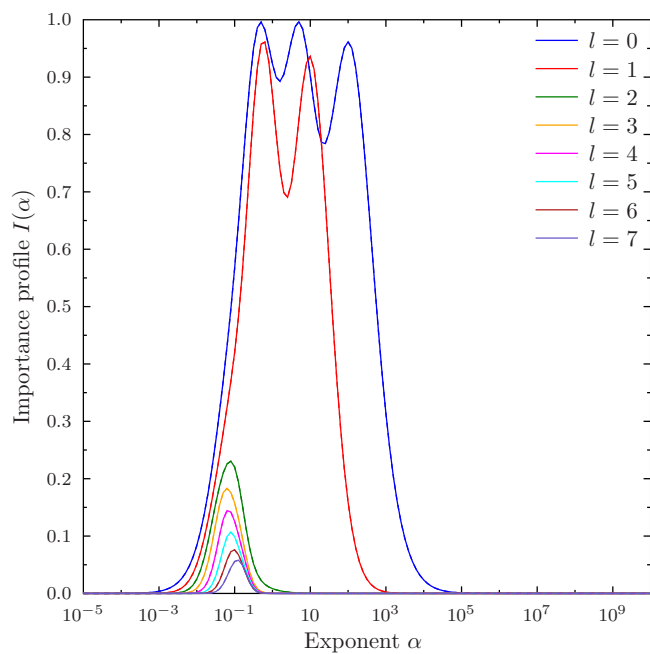

Figure 381. GTO importance profile for  $\sigma$  orbitals on K atom in KBr.

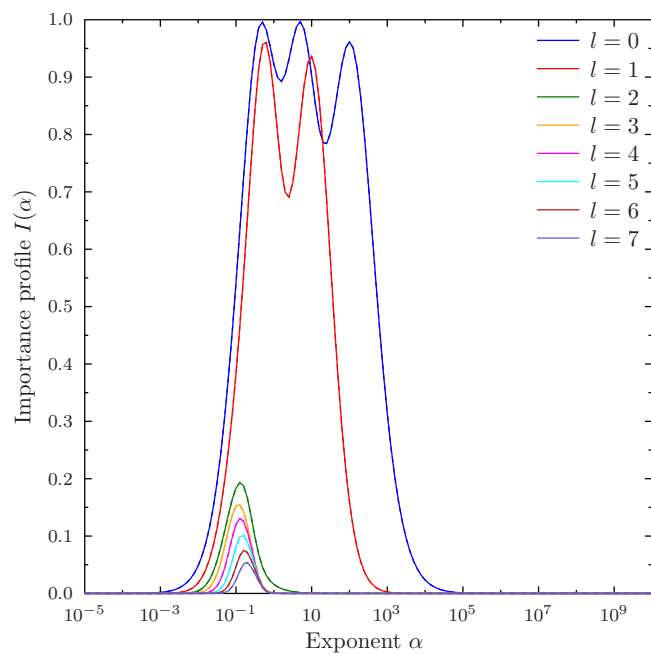

Figure 383. GTO importance profile for  $\sigma$  orbitals on K atom in KF.

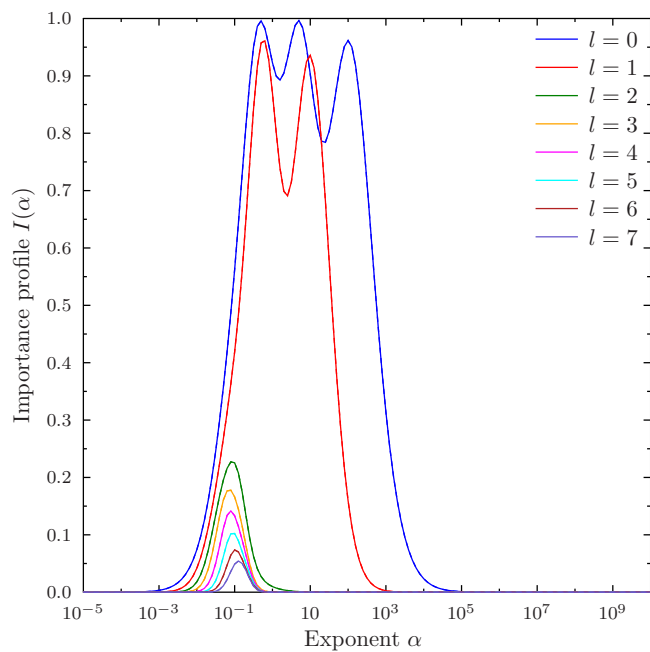

Figure 382. GTO importance profile for  $\sigma$  orbitals on K atom in KCl.

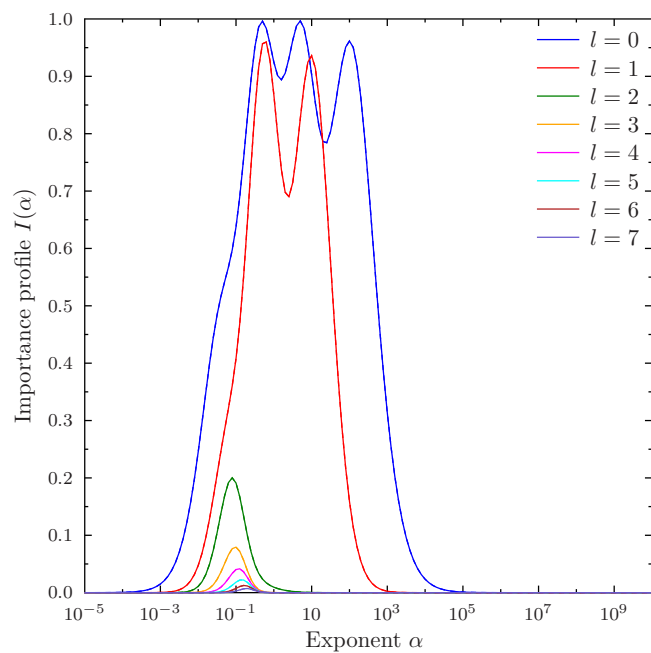

Figure 384. GTO importance profile for  $\sigma$  orbitals on K atom in KH.

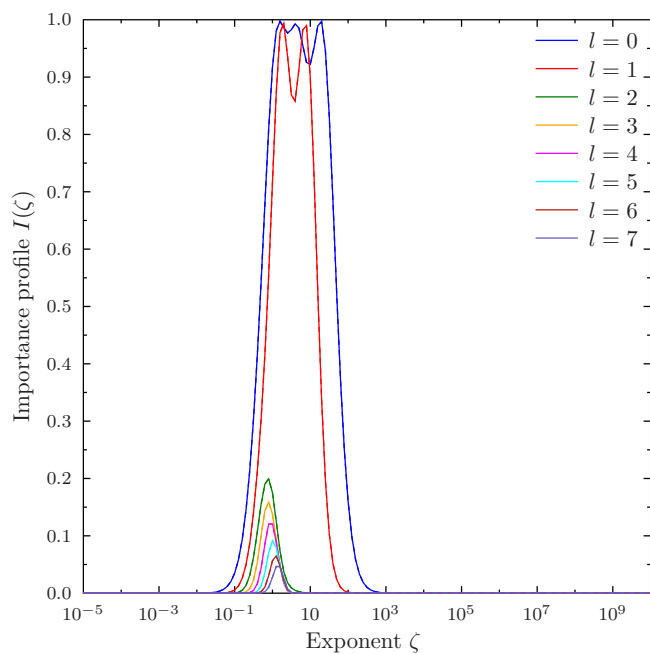

Figure 385. STO importance profile for  $\sigma$  orbitals on K atom in KBr.

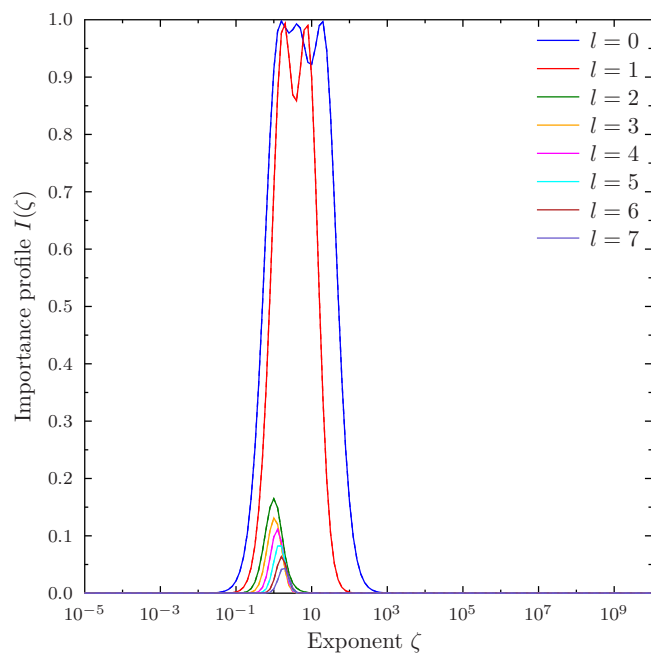

Figure 387. STO importance profile for  $\sigma$  orbitals on K atom in KF.

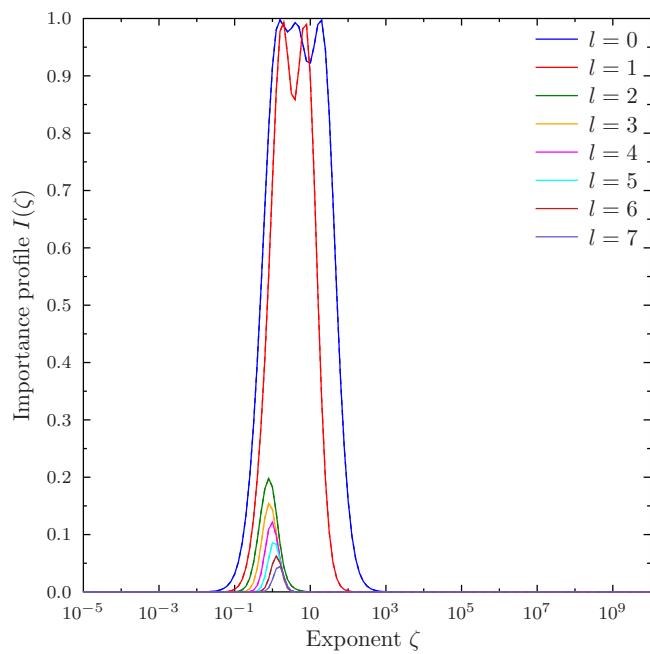

Figure 386. STO importance profile for  $\sigma$  orbitals on K atom in KCl.

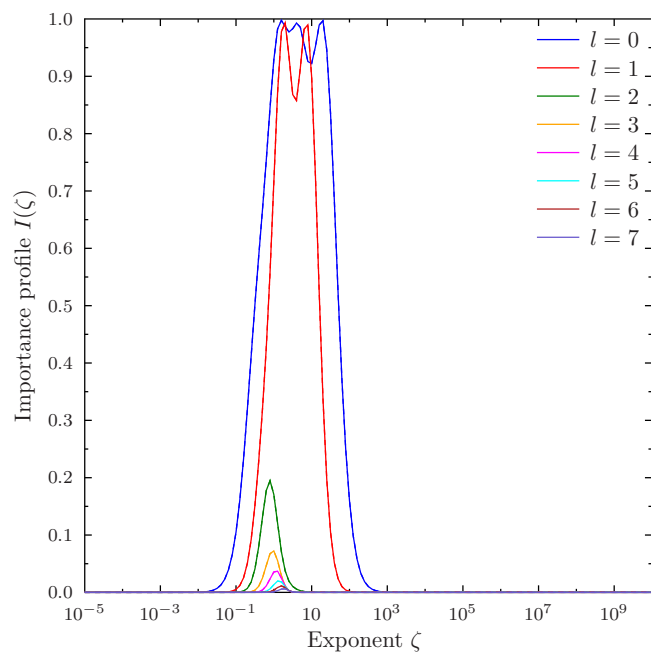

Figure 388. STO importance profile for  $\sigma$  orbitals on K atom in KH.

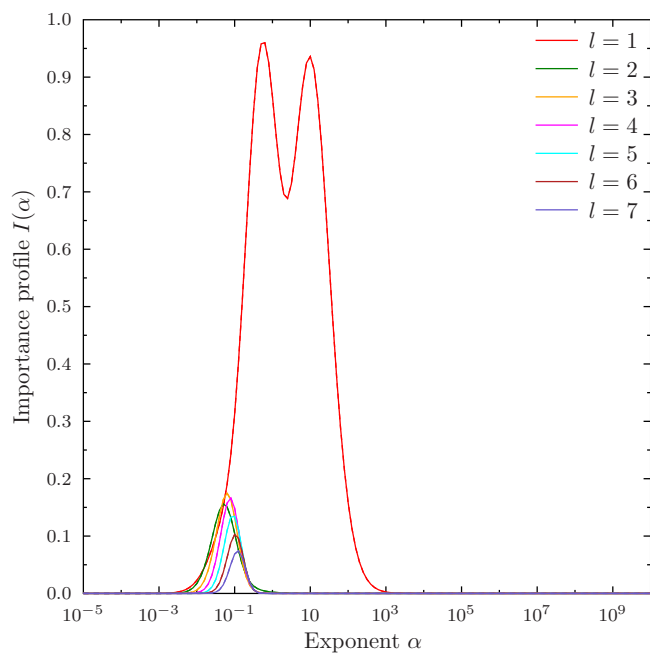

Figure 389. GTO importance profile for  $\pi_-$  orbitals on K atom in KBr.

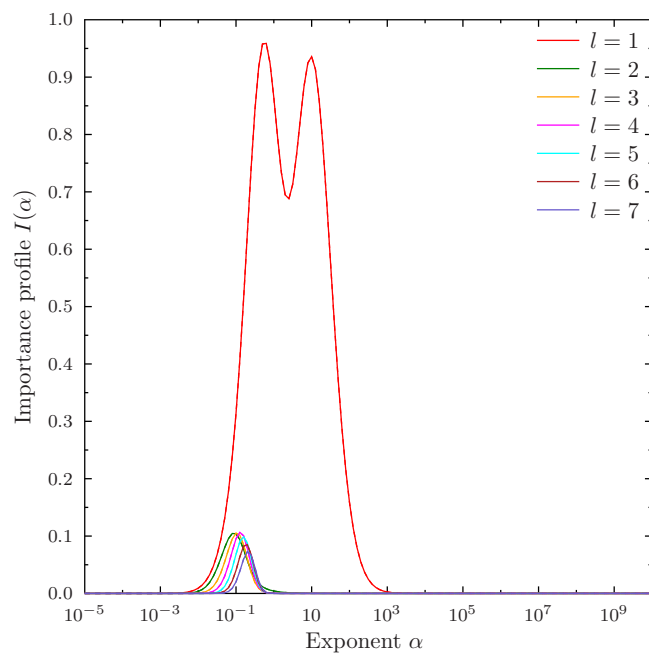

Figure 391. GTO importance profile for  $\pi_-$  orbitals on K atom in KF.

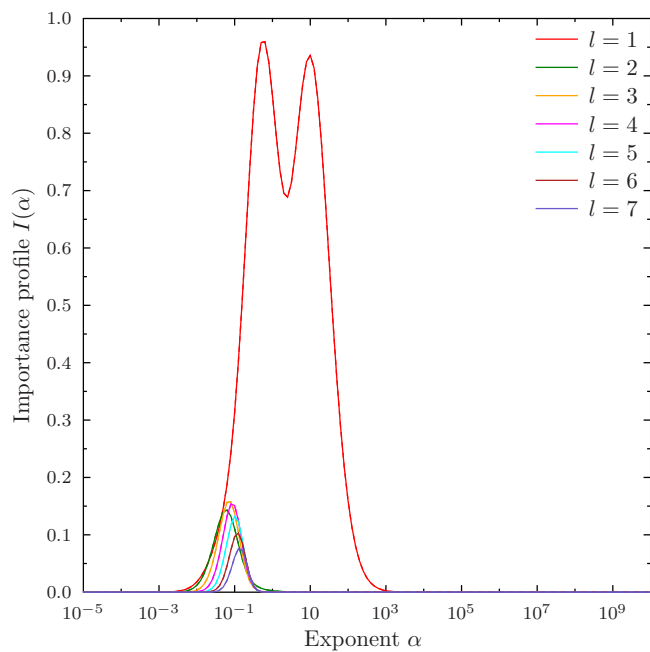

Figure 390. GTO importance profile for  $\pi_-$  orbitals on K atom in KCl.

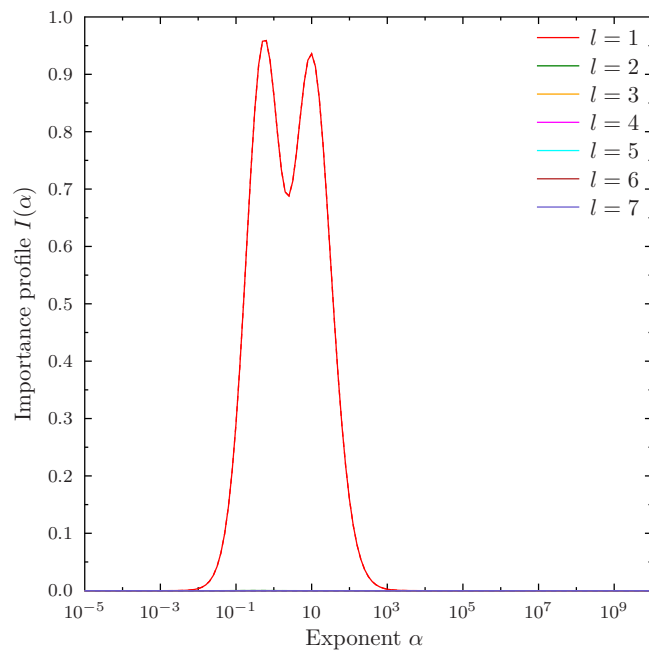

Figure 392. GTO importance profile for  $\pi_-$  orbitals on K atom in KH.

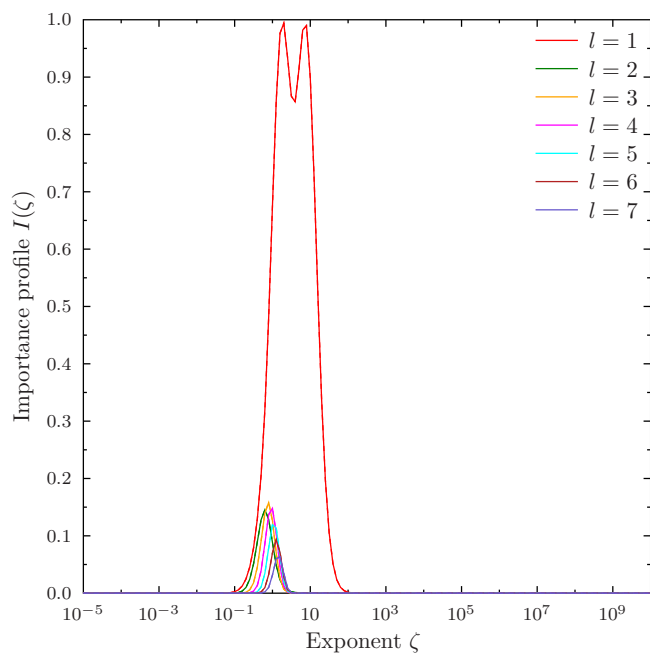

Figure 393. STO importance profile for  $\pi_-$  orbitals on K atom in KBr.

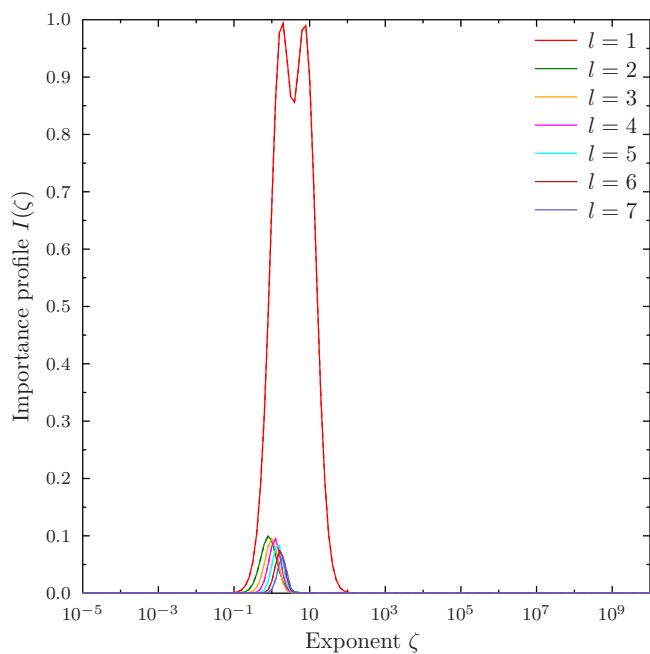

Figure 395. STO importance profile for  $\pi_-$  orbitals on K atom in KF.

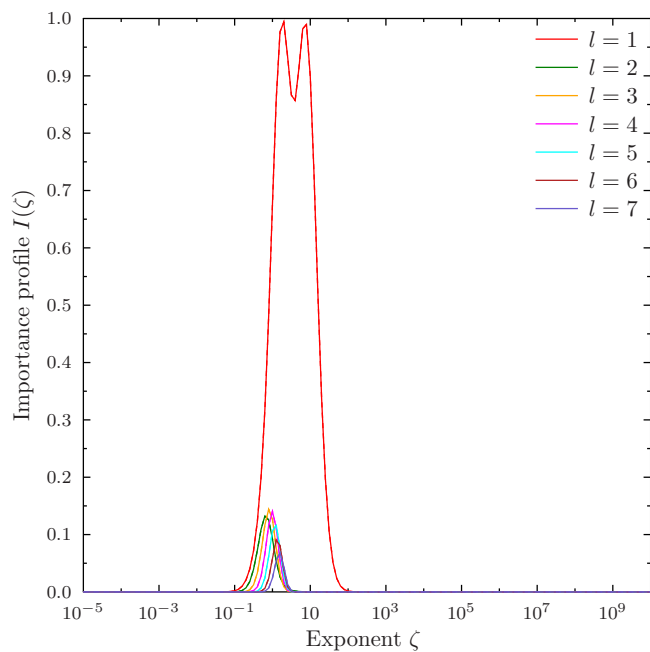

Figure 394. STO importance profile for  $\pi_-$  orbitals on K atom in KCl.

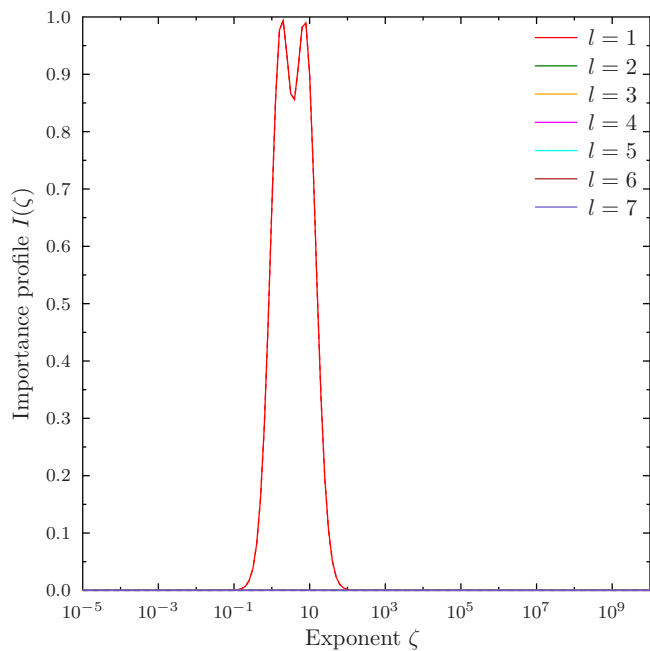

Figure 396. STO importance profile for  $\pi_-$  orbitals on K atom in KH.

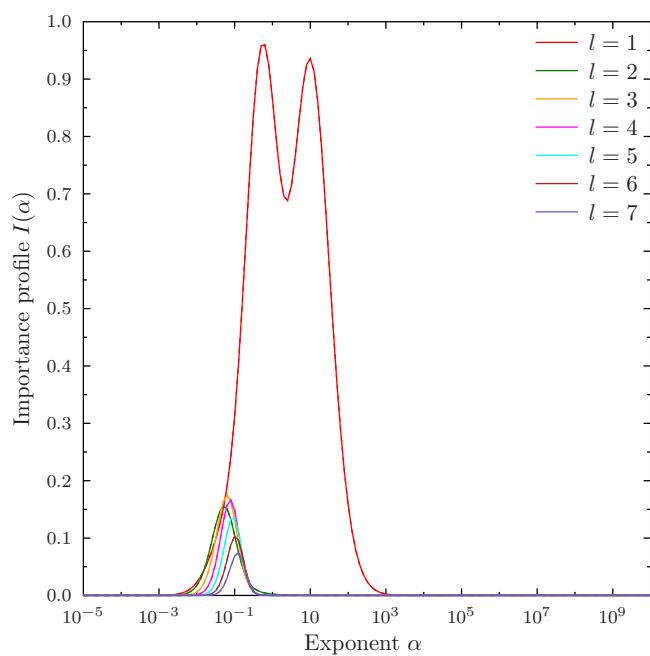

Figure 397. GTO importance profile for  $\pi_+$  orbitals on K atom in KBr.

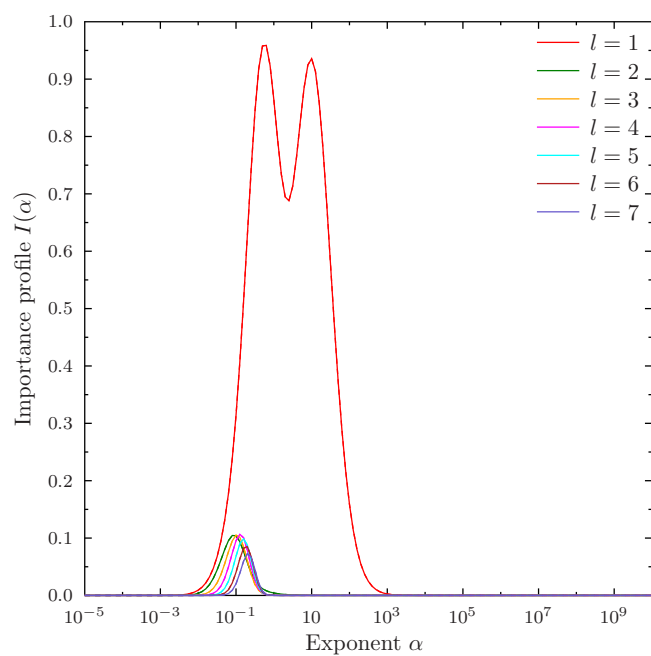

Figure 399. GTO importance profile for  $\pi_+$  orbitals on K atom in KF.

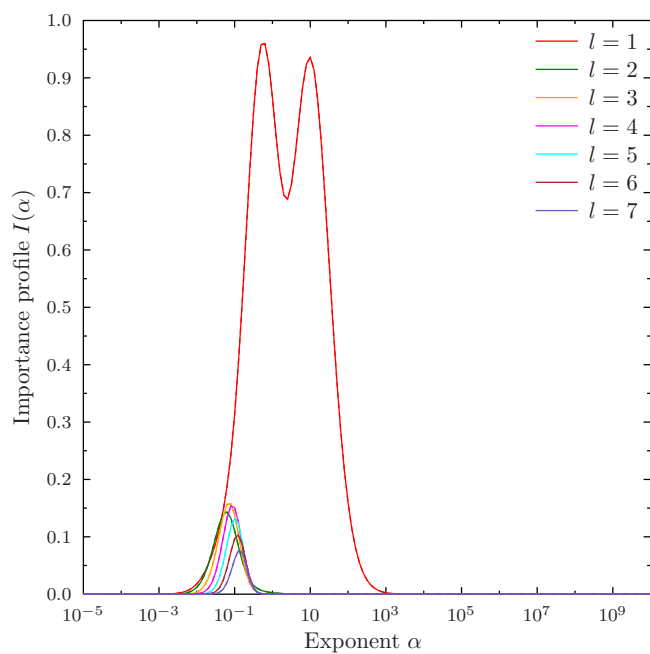

Figure 398. GTO importance profile for  $\pi_+$  orbitals on K atom in KCl.

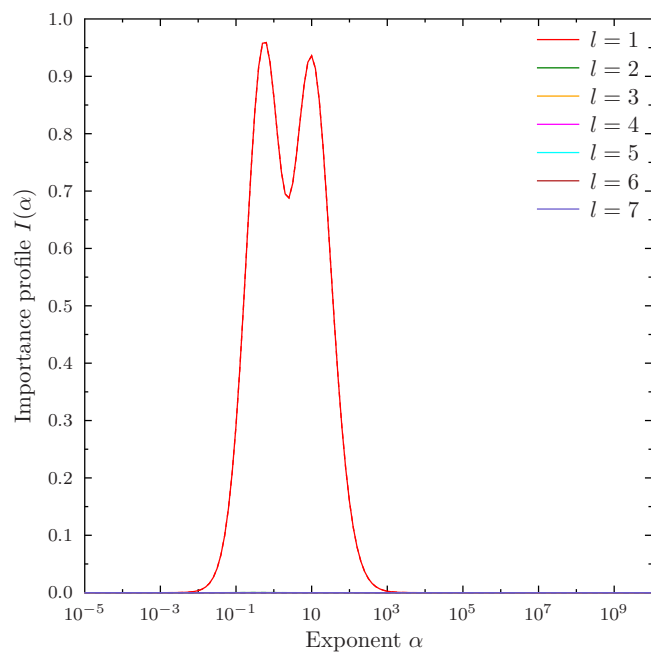

Figure 400. GTO importance profile for  $\pi_+$  orbitals on K atom in KH.



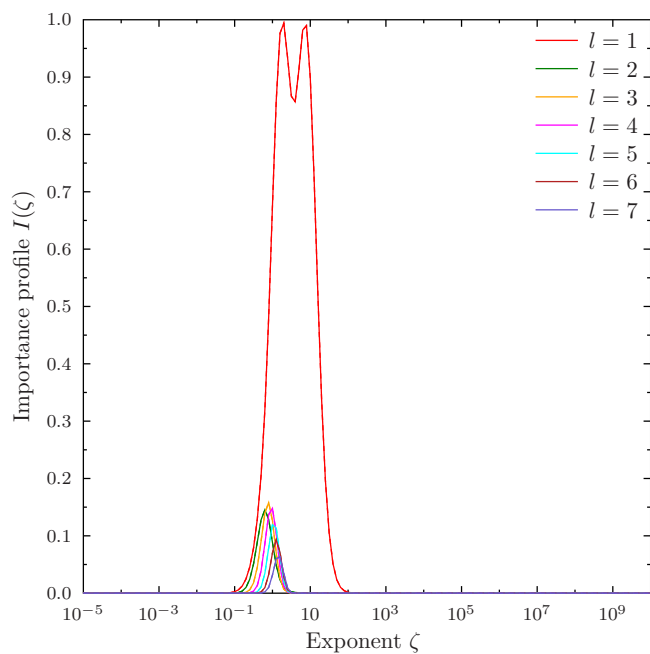

Figure 401. STO importance profile for  $\pi_+$  orbitals on K atom in KBr.

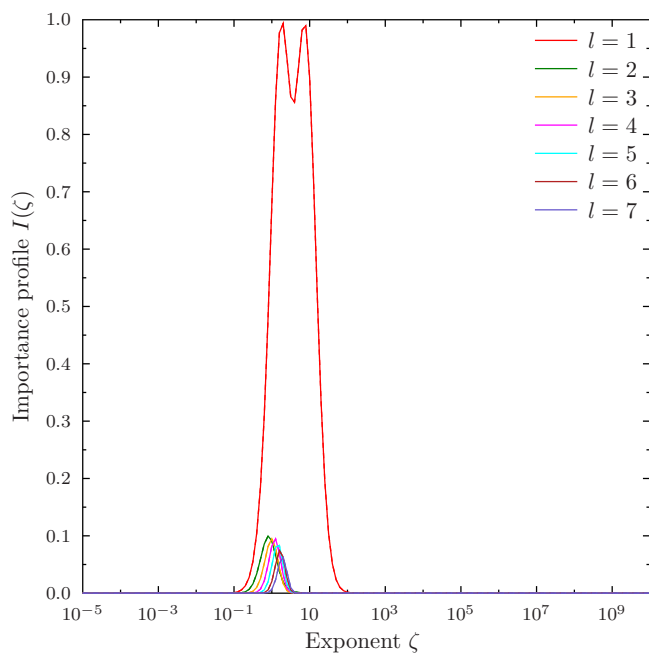

Figure 403. STO importance profile for  $\pi_+$  orbitals on K atom in KF.

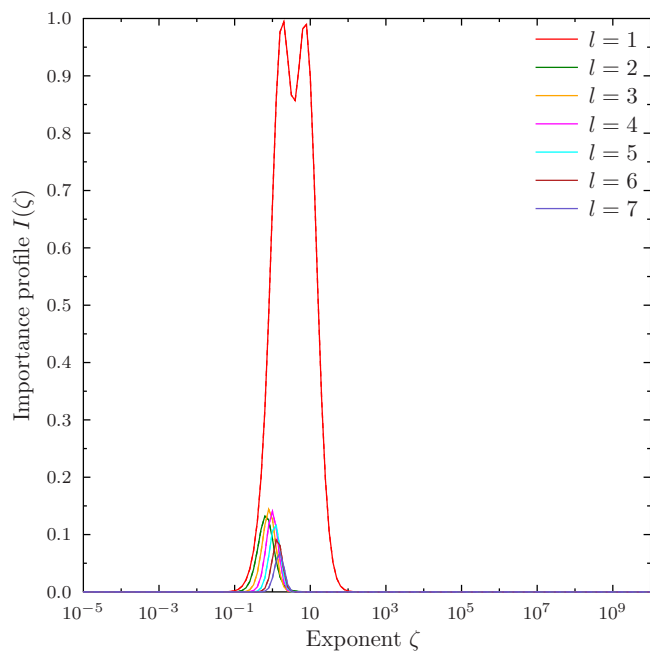

Figure 402. STO importance profile for  $\pi_+$  orbitals on K atom in KCl.

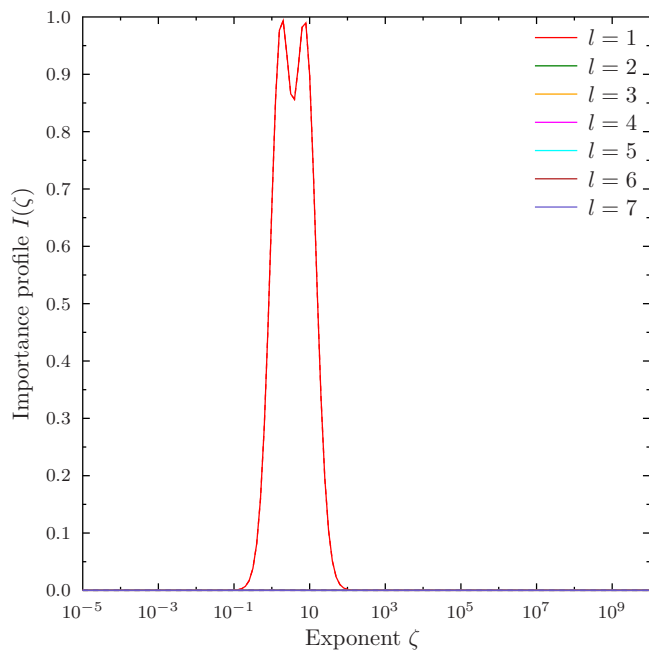

Figure 404. STO importance profile for  $\pi_+$  orbitals on K atom in KH.

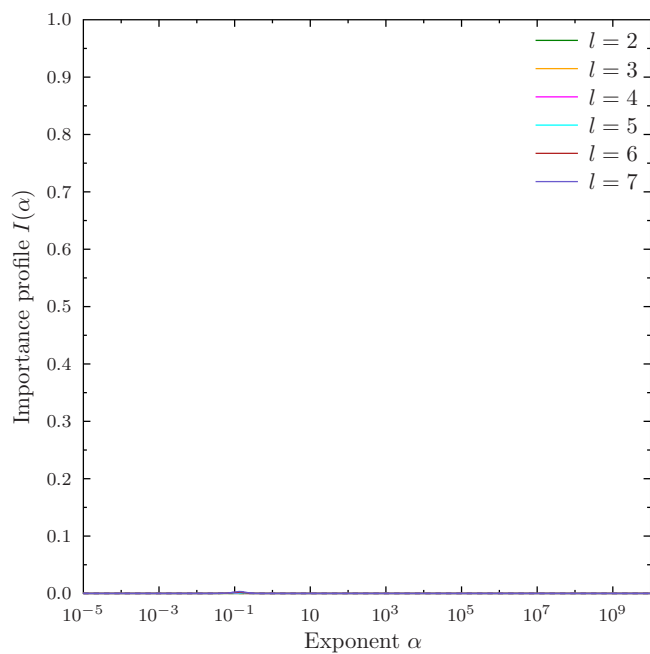

Figure 405. GTO importance profile for  $\delta_-$  orbitals on K atom in KBr.

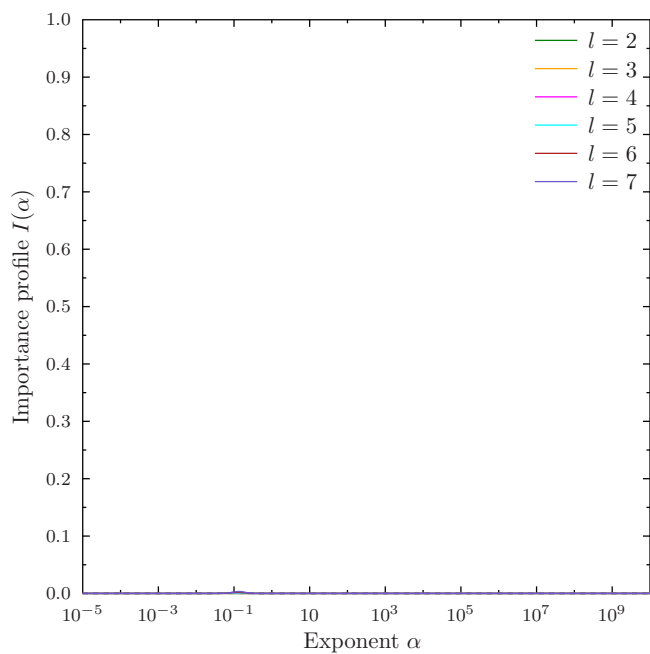

Figure 407. GTO importance profile for  $\delta_+$  orbitals on K atom in KBr.

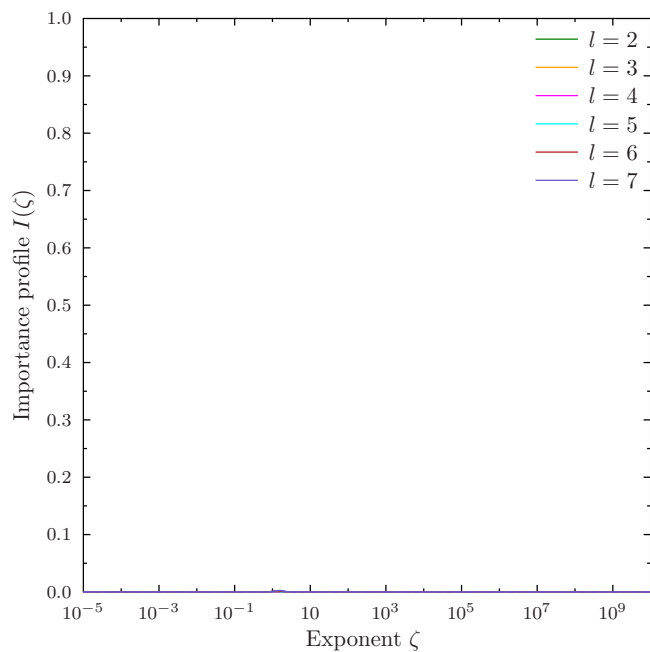

Figure 406. STO importance profile for  $\delta_-$  orbitals on K atom in KBr.

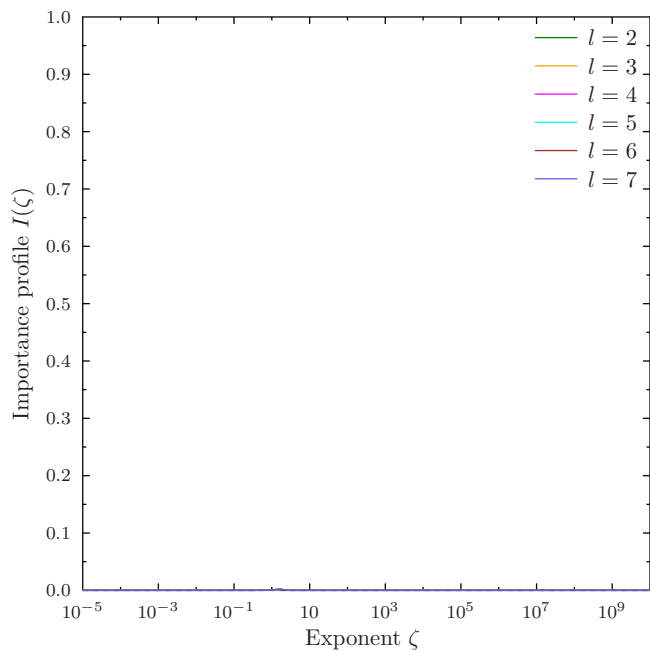

Figure 408. STO importance profile for  $\delta_+$  orbitals on K atom in KBr.

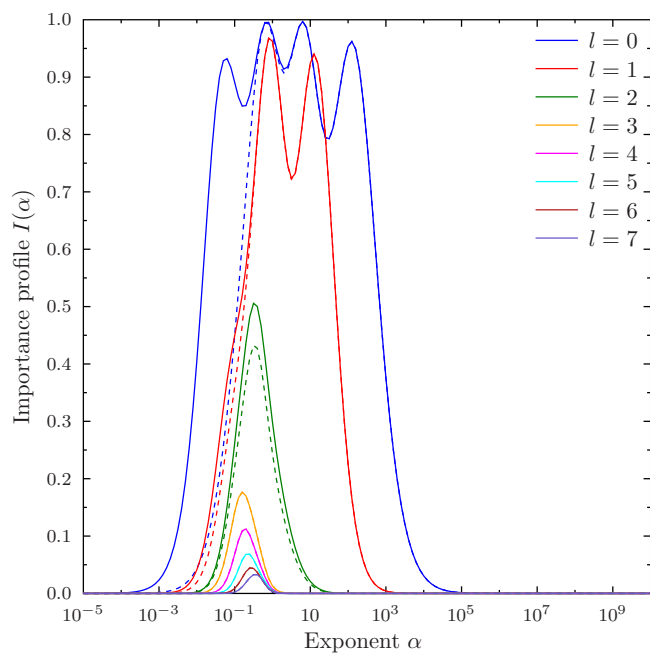

Figure 409. GTO importance profile for  $\sigma$  orbitals on Sc atom in ScO.

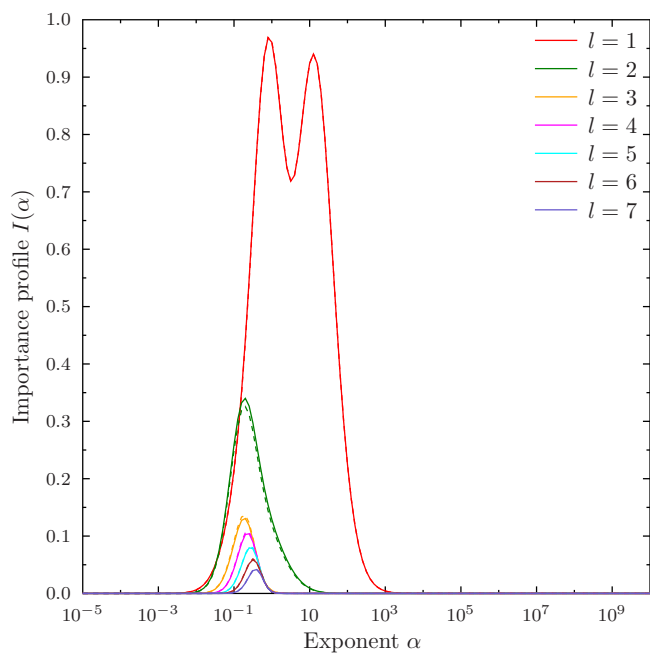

Figure 411. GTO importance profile for  $\pi_-$  orbitals on Sc atom in ScO.

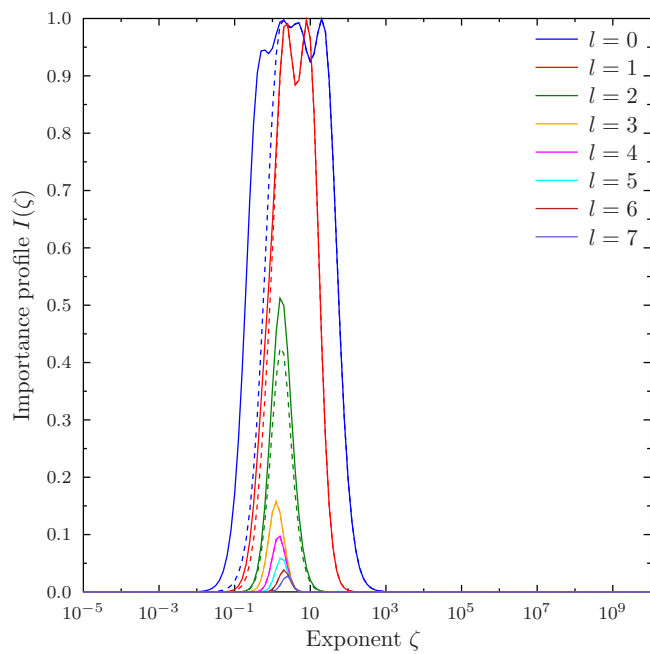

Figure 410. STO importance profile for  $\sigma$  orbitals on Sc atom in ScO.

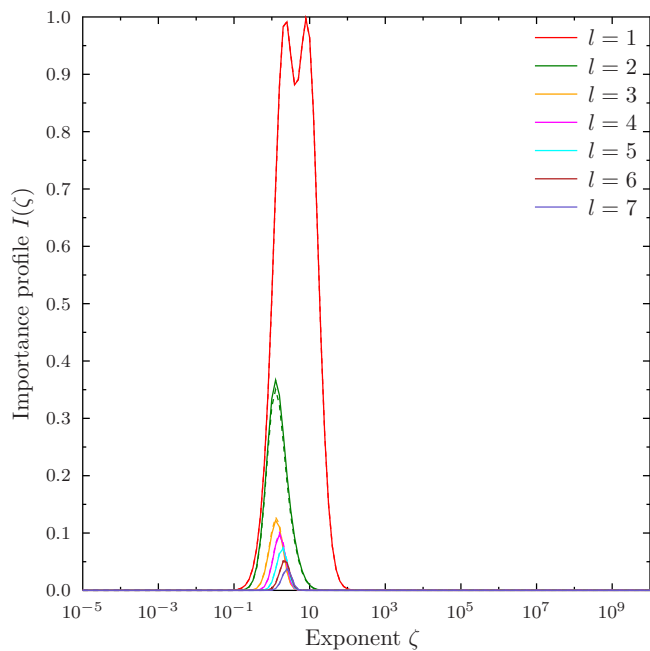

Figure 412. STO importance profile for  $\pi_-$  orbitals on Sc atom in ScO.

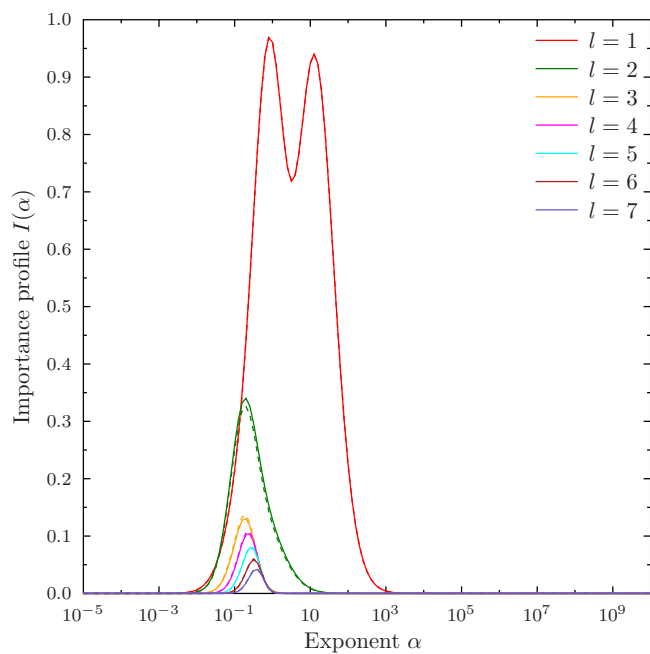

Figure 413. GTO importance profile for  $\pi_+$  orbitals on Sc atom in ScO.

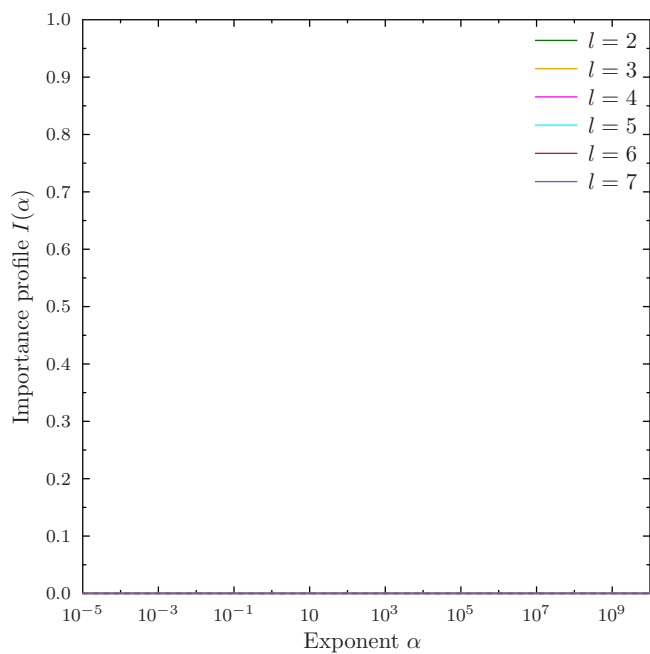

Figure 415. GTO importance profile for  $\delta_-$  orbitals on Sc atom in ScO.

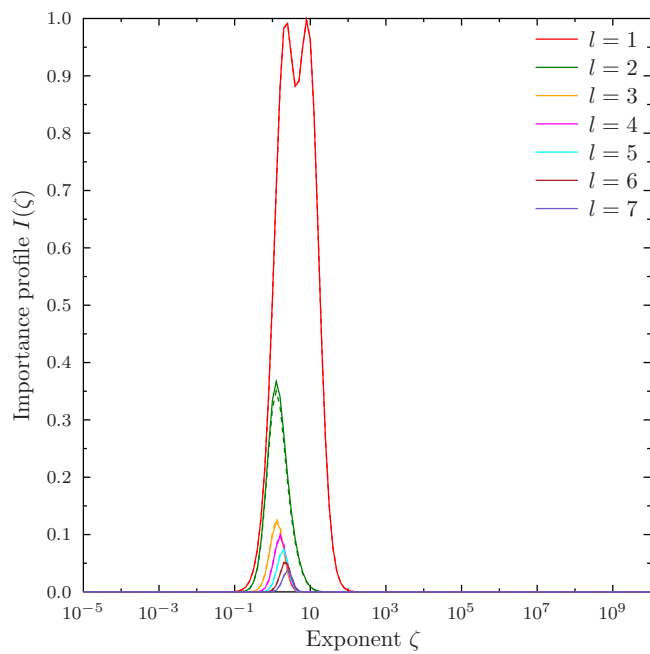

Figure 414. STO importance profile for  $\pi_+$  orbitals on Sc atom in ScO.

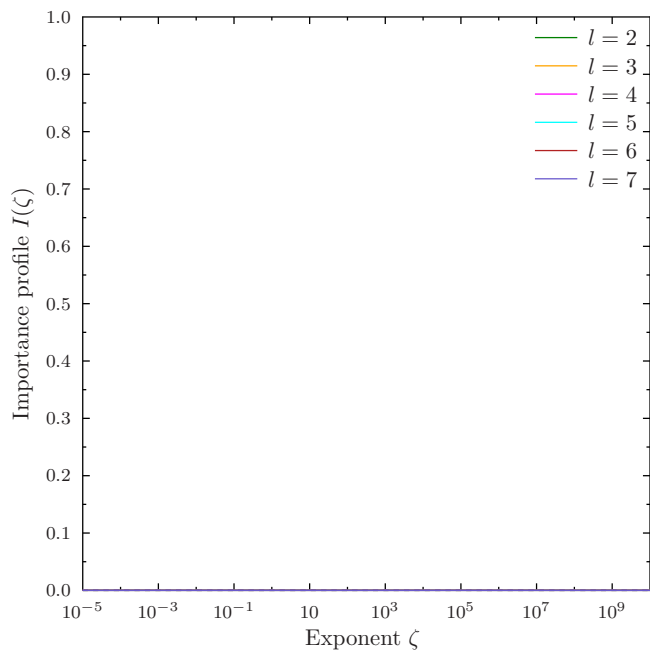

Figure 416. STO importance profile for  $\delta_-$  orbitals on Sc atom in ScO.

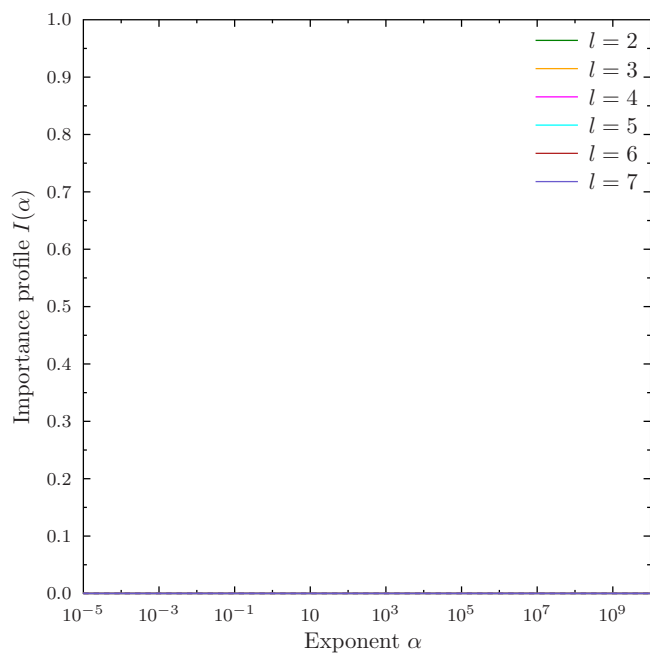

Figure 417. GTO importance profile for  $\delta_+$  orbitals on Sc atom in ScO.

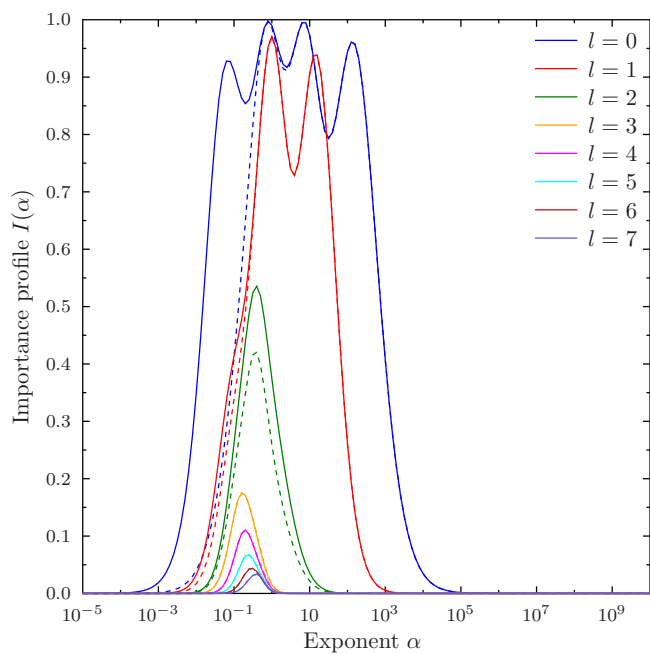

Figure 419. GTO importance profile for  $\sigma$  orbitals on Ti atom in TiO.

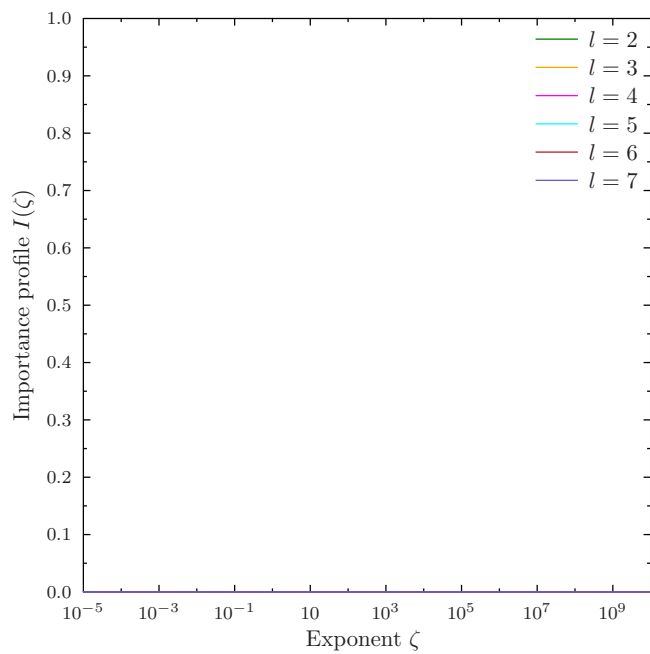

Figure 418. STO importance profile for  $\delta_+$  orbitals on Sc atom in ScO.

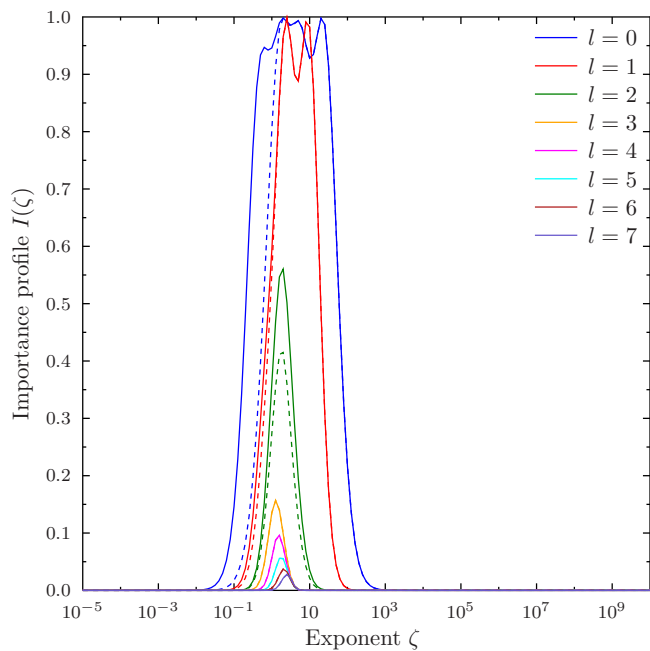

Figure 420. STO importance profile for  $\sigma$  orbitals on Ti atom in TiO.

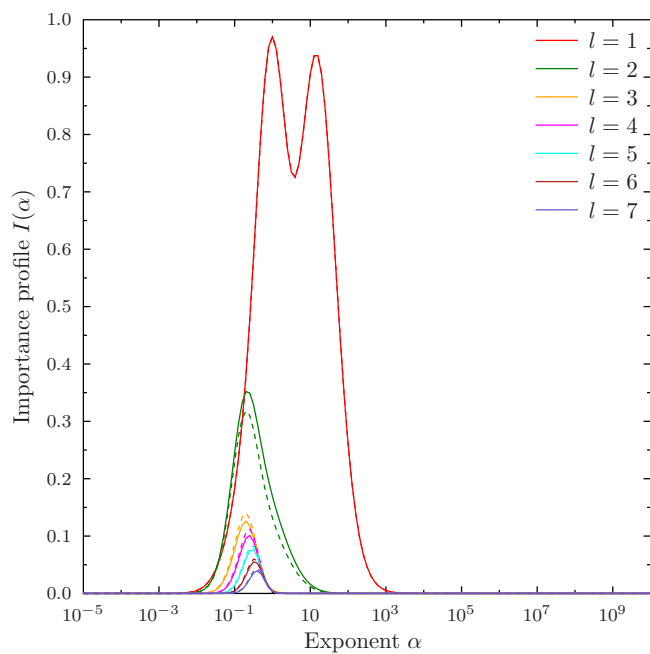

Figure 421. GTO importance profile for  $\pi_-$  orbitals on Ti atom in TiO.

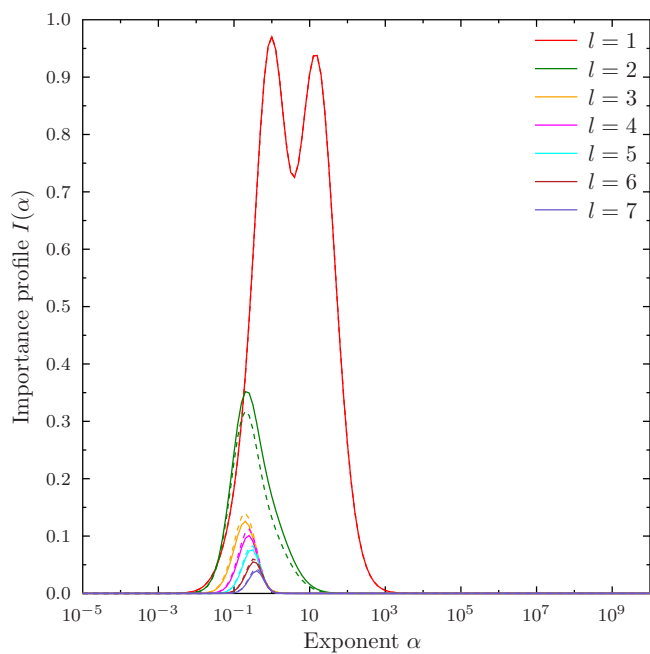

Figure 423. GTO importance profile for  $\pi_+$  orbitals on Ti atom in TiO.

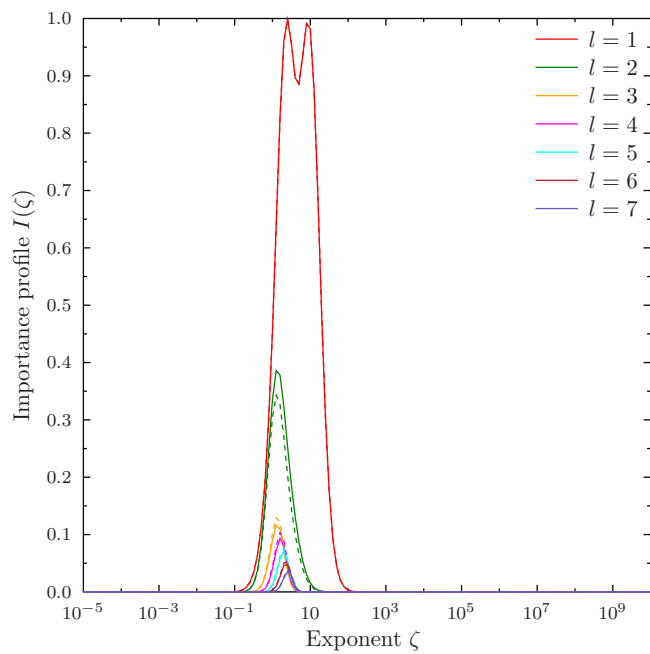

Figure 422. STO importance profile for  $\pi_-$  orbitals on Ti atom in TiO.

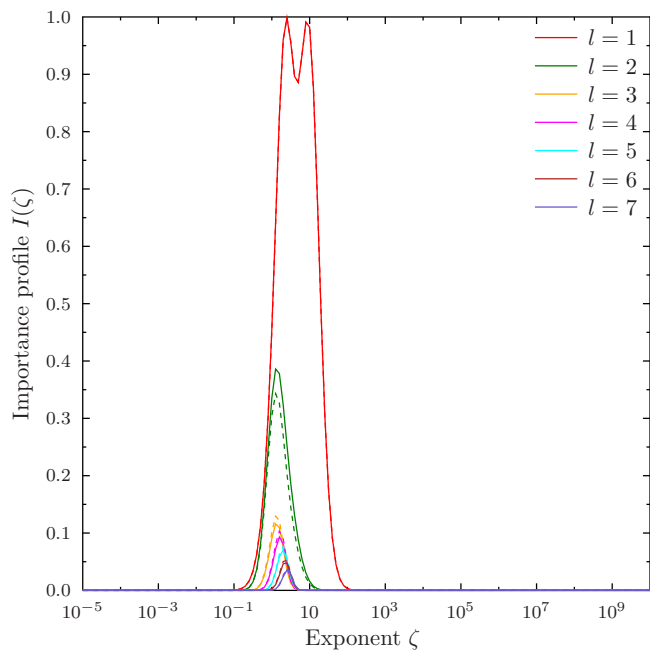

Figure 424. STO importance profile for  $\pi_+$  orbitals on Ti atom in TiO.

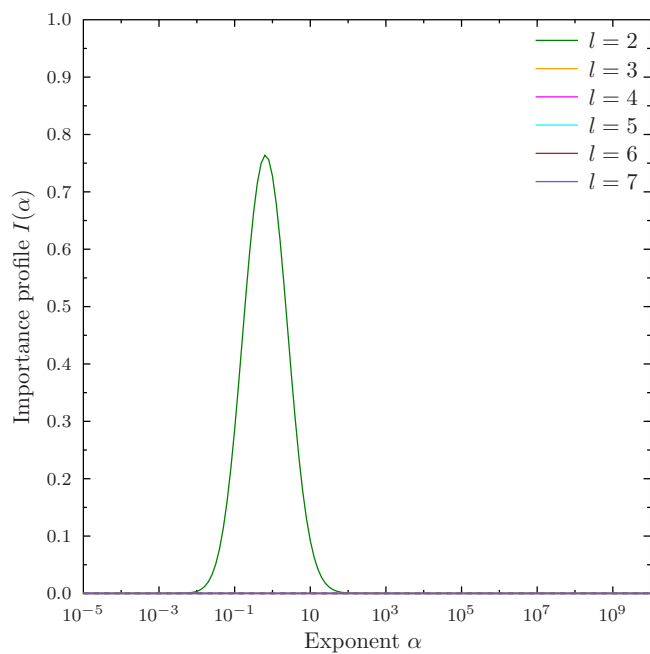

Figure 425. GTO importance profile for  $\delta_-$  orbitals on Ti atom in TiO.

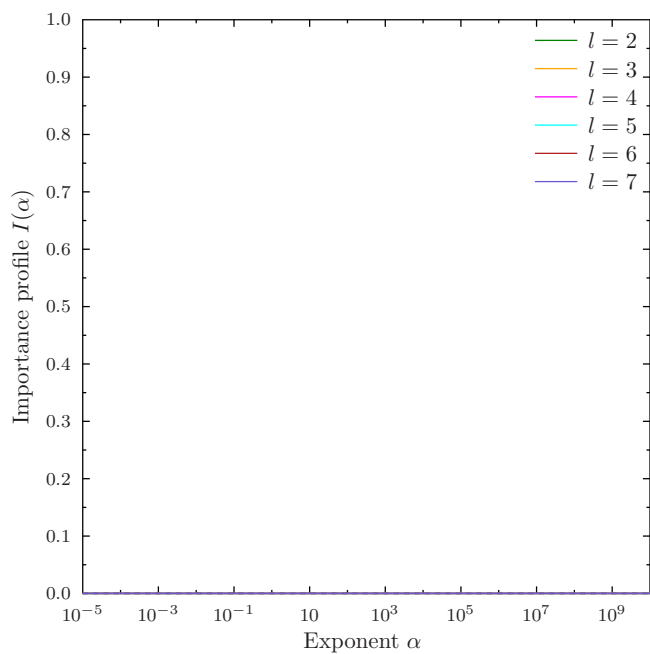

Figure 427. GTO importance profile for  $\delta_+$  orbitals on Ti atom in TiO.

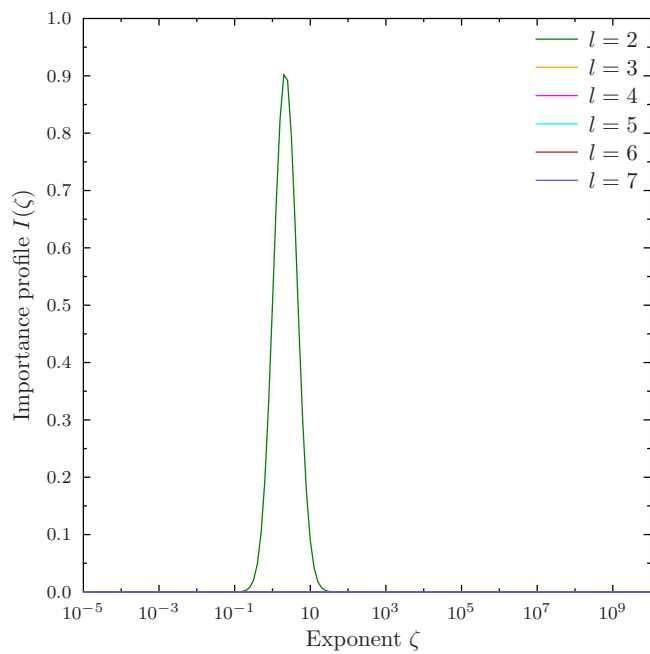

Figure 426. STO importance profile for  $\delta_-$  orbitals on Ti atom in TiO.

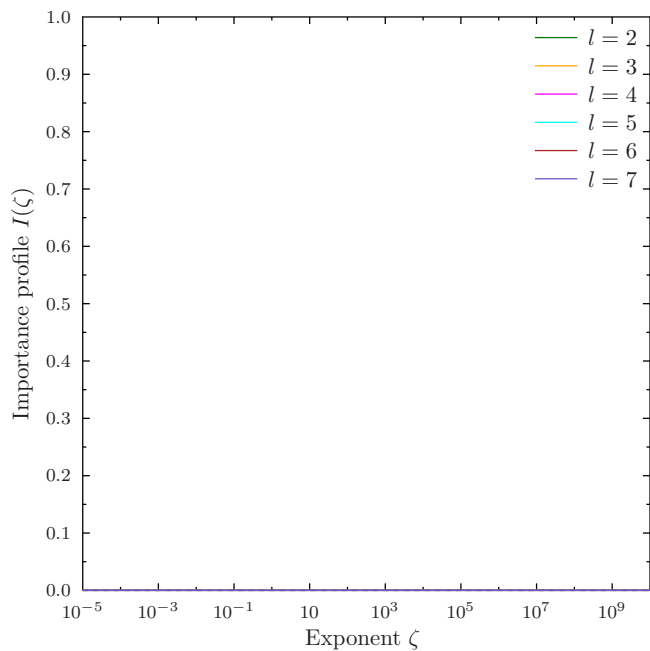

Figure 428. STO importance profile for  $\delta_+$  orbitals on Ti atom in TiO.

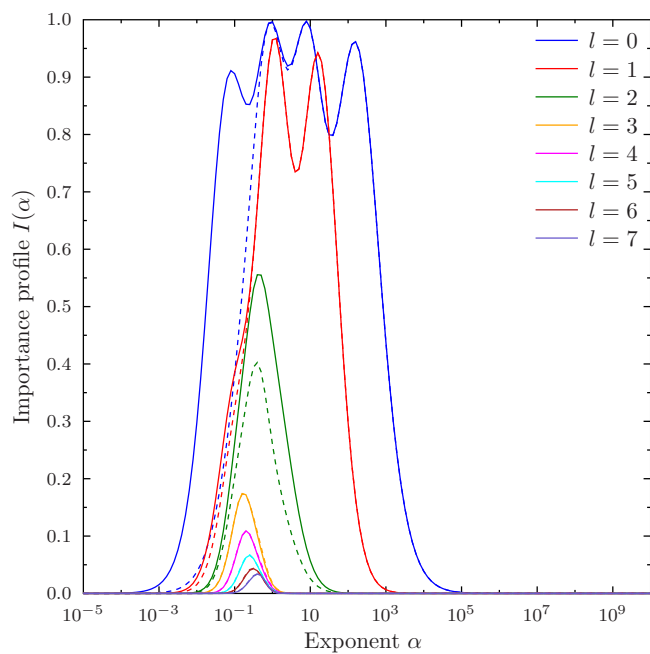

Figure 429. GTO importance profile for  $\sigma$  orbitals on V atom in VO.

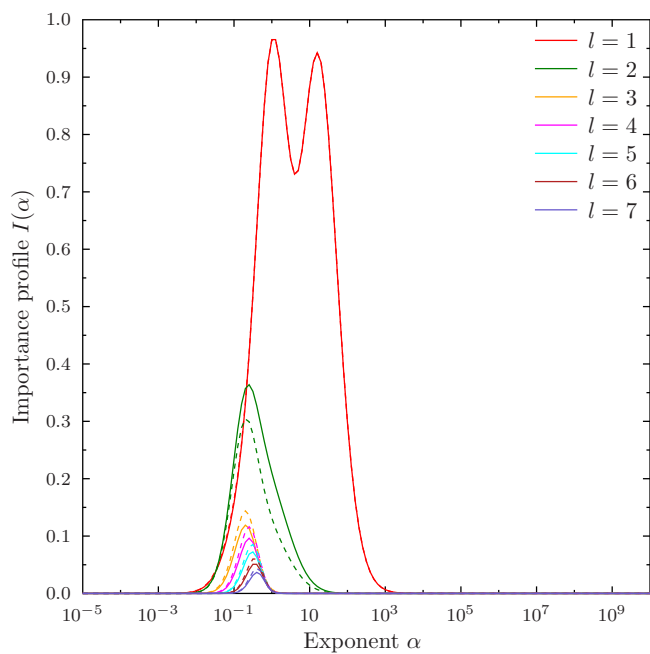

Figure 431. GTO importance profile for  $\pi_-$  orbitals on V atom in VO.

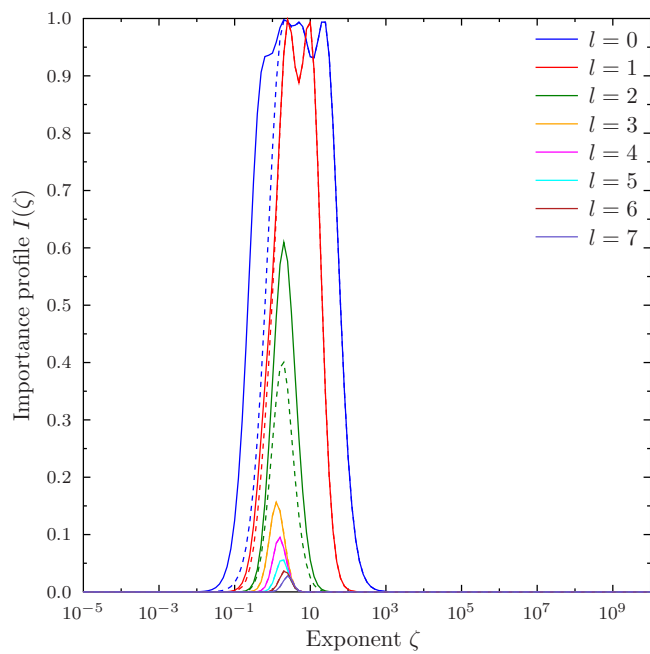

Figure 430. STO importance profile for  $\sigma$  orbitals on V atom in VO.

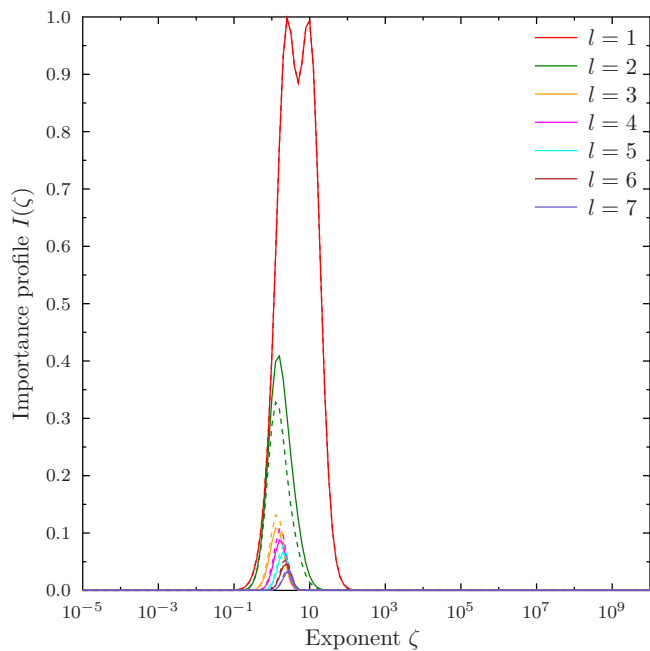

Figure 432. STO importance profile for  $\pi_-$  orbitals on V atom in VO.



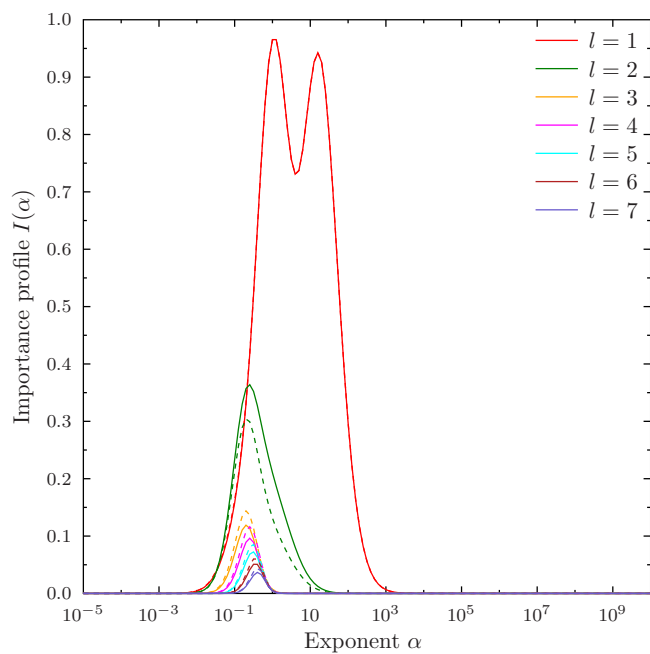

Figure 433. GTO importance profile for  $\pi_+$  orbitals on V atom in VO.

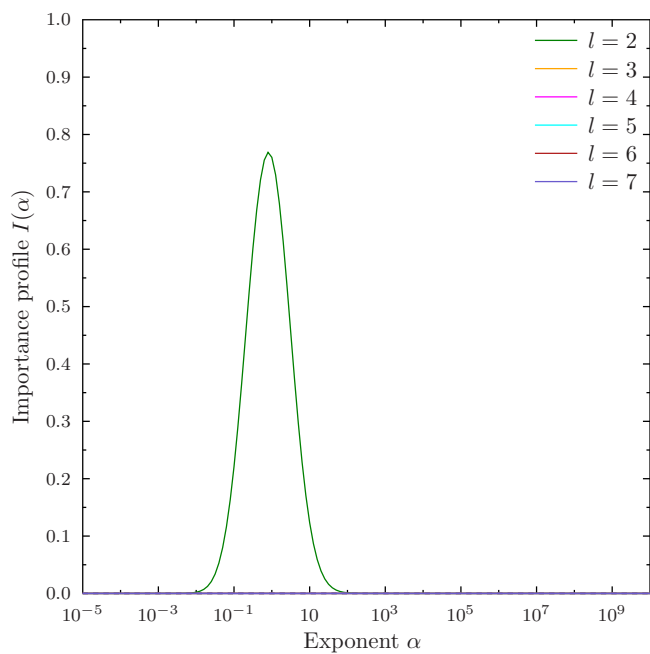

Figure 435. GTO importance profile for  $\delta_-$  orbitals on V atom in VO.

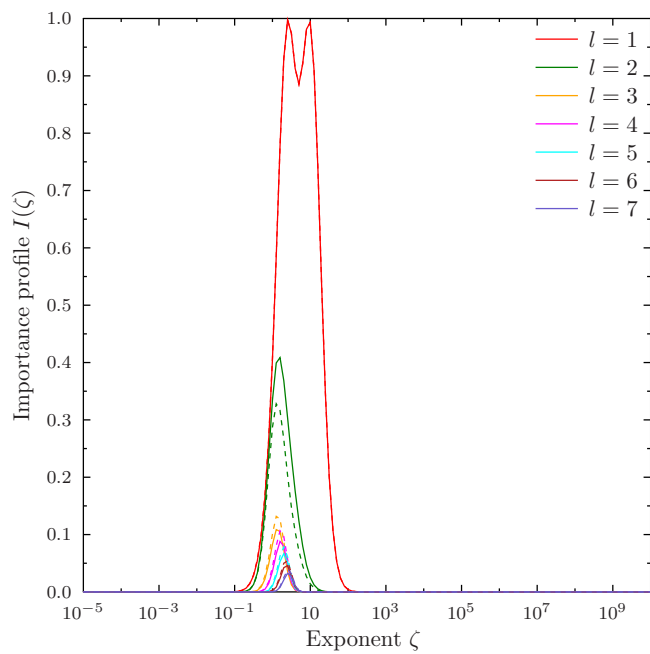

Figure 434. STO importance profile for  $\pi_+$  orbitals on V atom in VO.

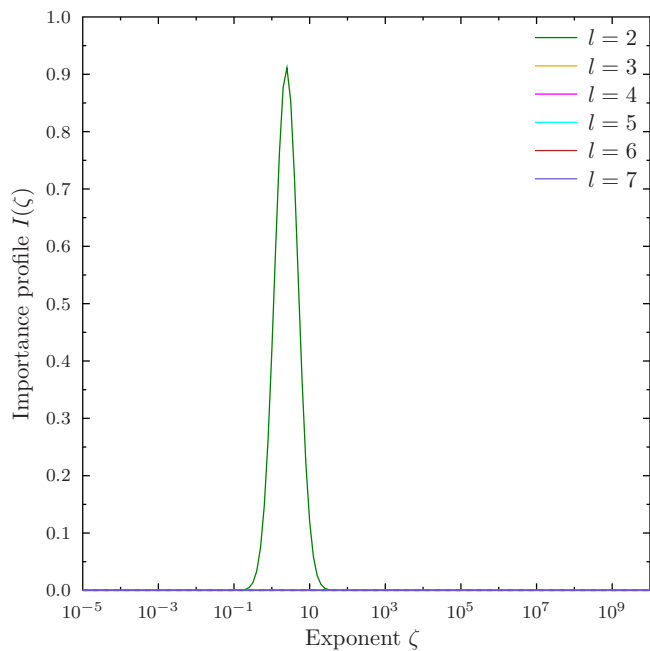

Figure 436. STO importance profile for  $\delta_-$  orbitals on V atom in VO.

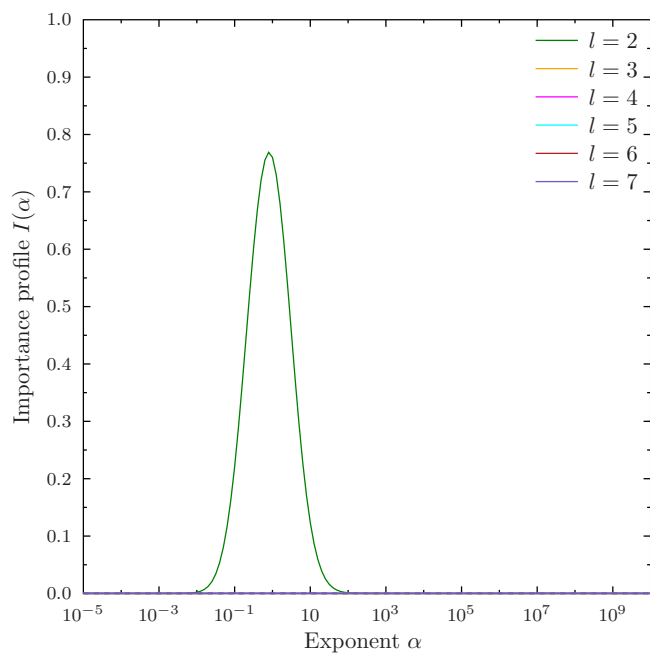

Figure 437. GTO importance profile for  $\delta_+$  orbitals on V atom in VO.

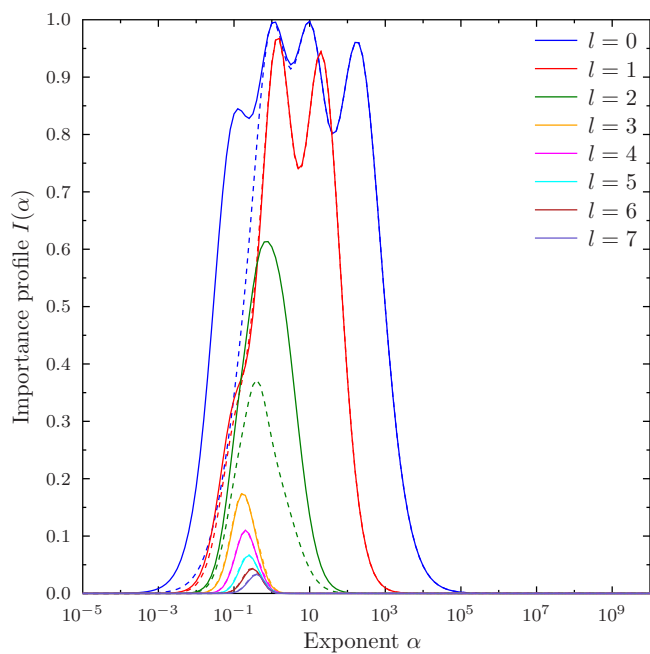

Figure 439. GTO importance profile for  $\sigma$  orbitals on Mn atom in MnO.

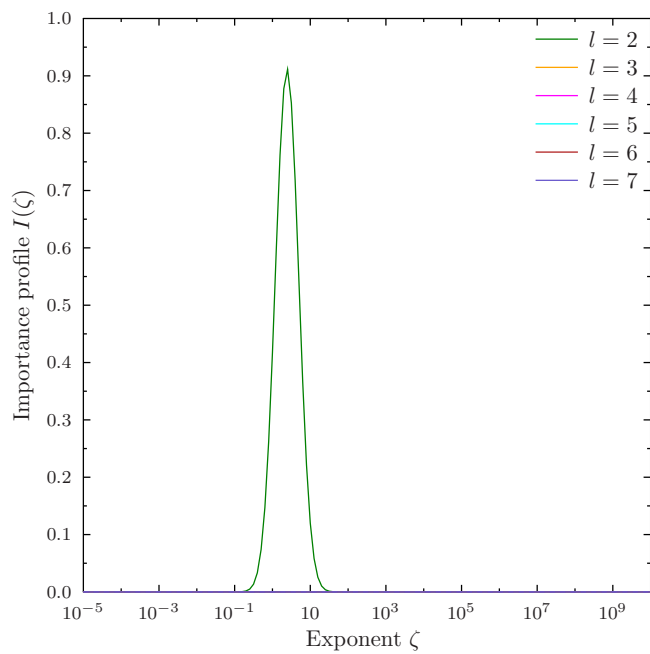

Figure 438. STO importance profile for  $\delta_+$  orbitals on V atom in VO.

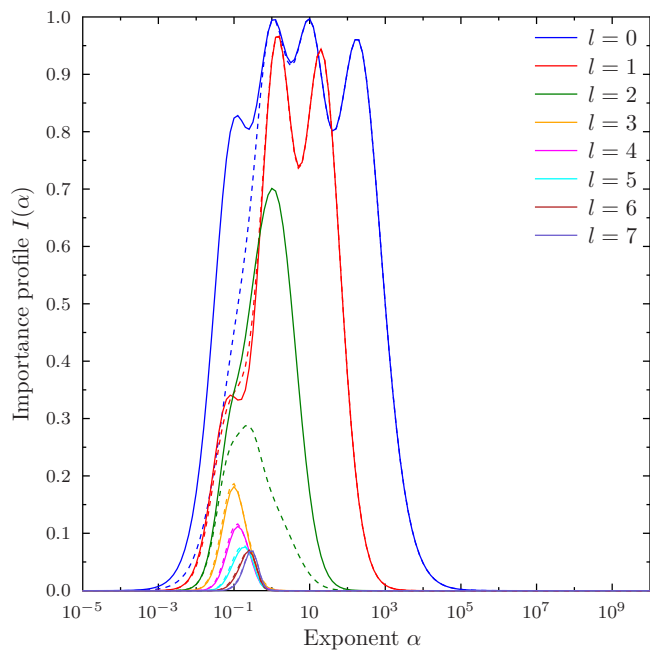

Figure 440. GTO importance profile for  $\sigma$  orbitals on Mn atom in MnS.

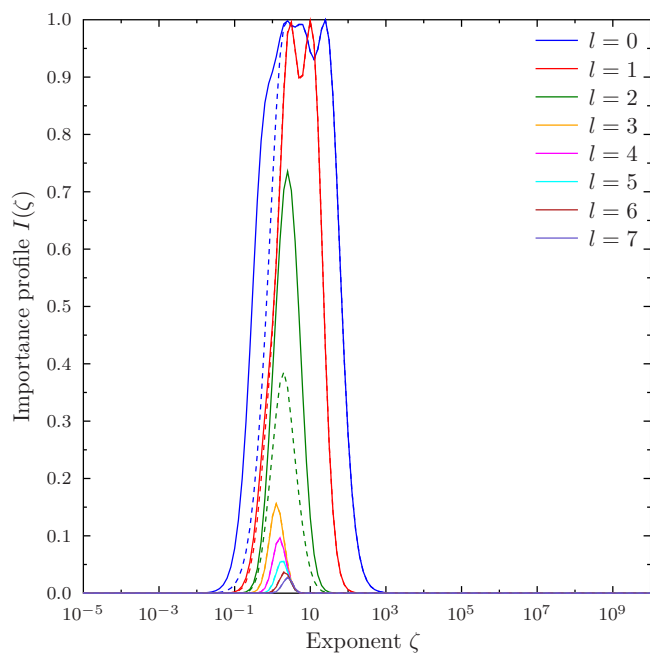

Figure 441. STO importance profile for  $\sigma$  orbitals on Mn atom in MnO.

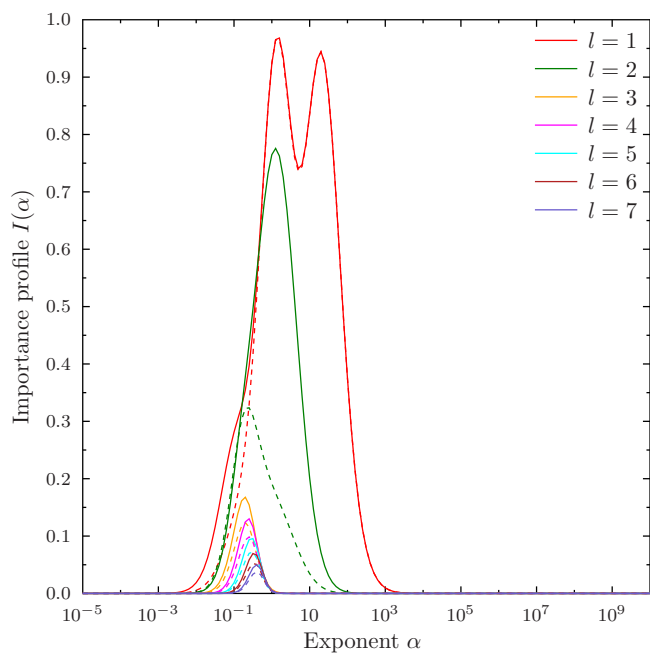

Figure 443. GTO importance profile for  $\pi_-$  orbitals on Mn atom in MnO.

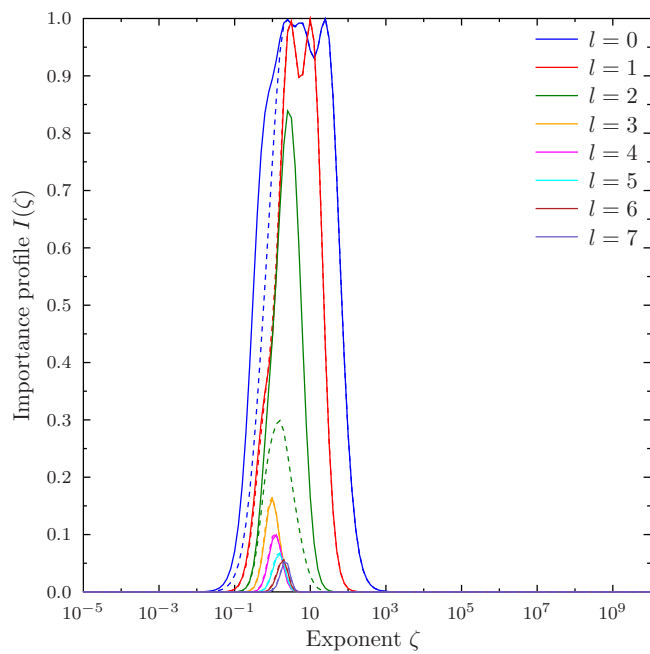

Figure 442. STO importance profile for  $\sigma$  orbitals on Mn atom in MnS.

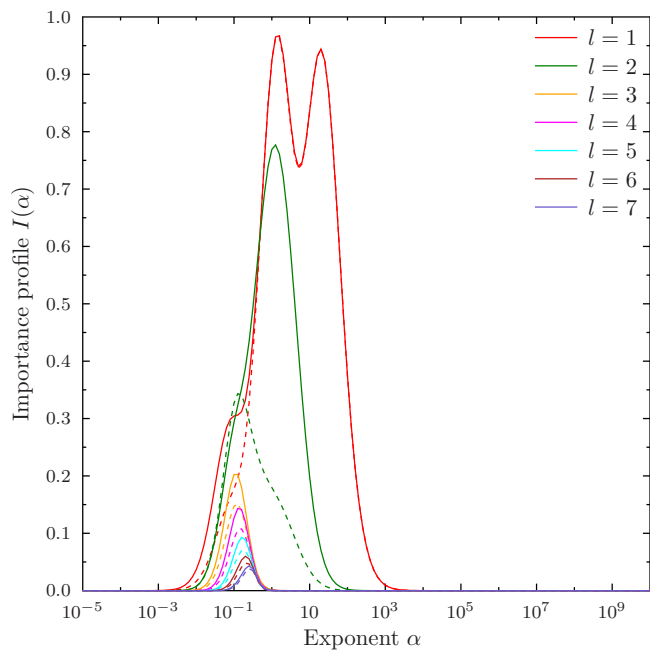

Figure 444. GTO importance profile for  $\pi_-$  orbitals on Mn atom in MnS.

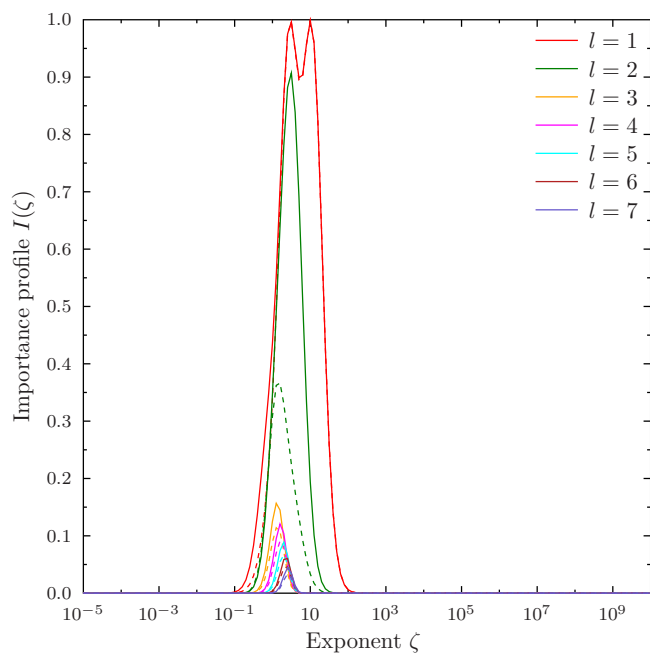

Figure 445. STO importance profile for  $\pi_-$  orbitals on Mn atom in MnO.

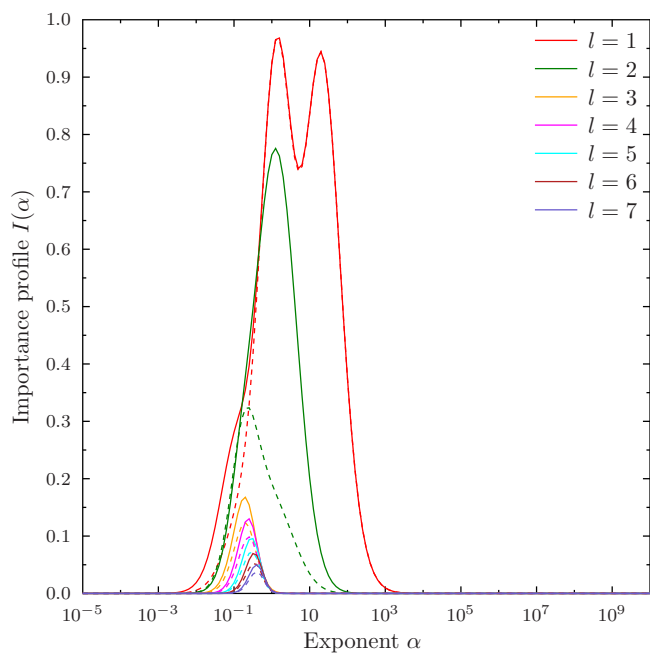

Figure 447. GTO importance profile for  $\pi_+$  orbitals on Mn atom in MnO.

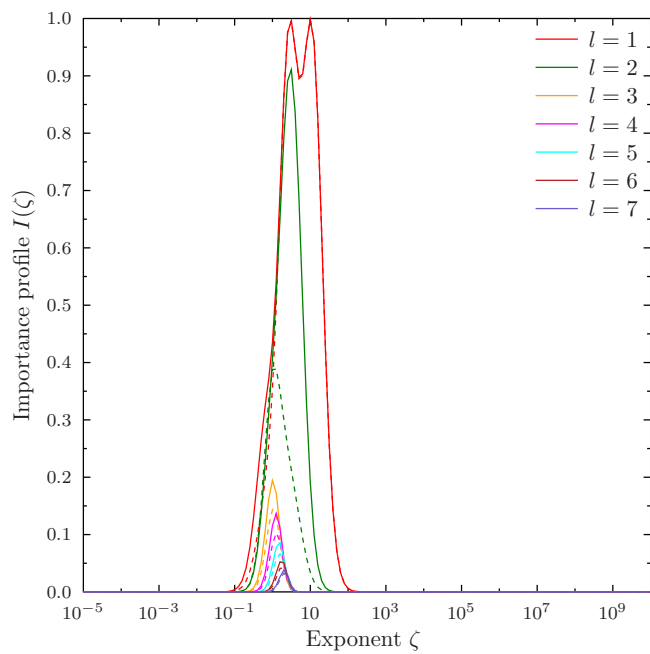

Figure 446. STO importance profile for  $\pi_-$  orbitals on Mn atom in MnS.

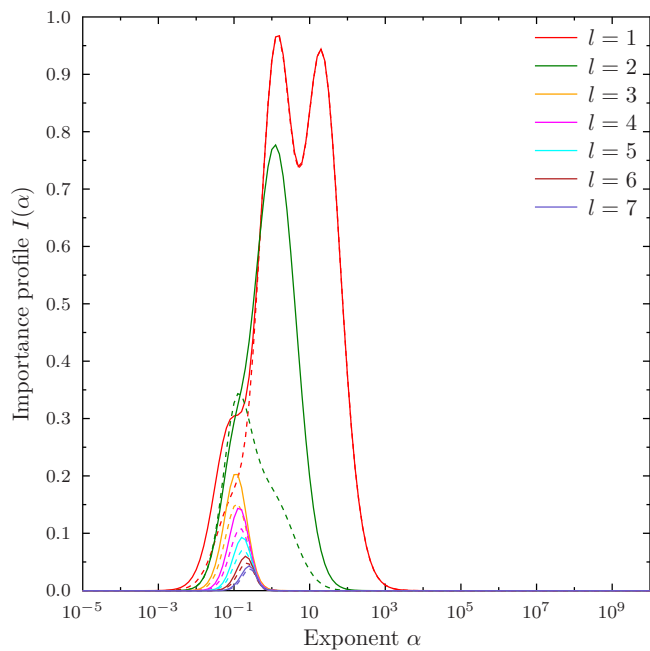

Figure 448. GTO importance profile for  $\pi_+$  orbitals on Mn atom in MnS.

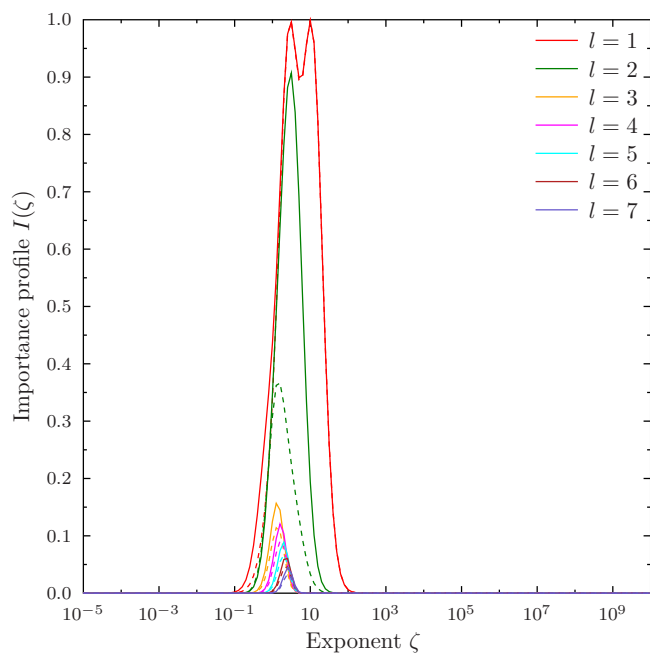

Figure 449. STO importance profile for  $\pi_+$  orbitals on Mn atom in MnO.

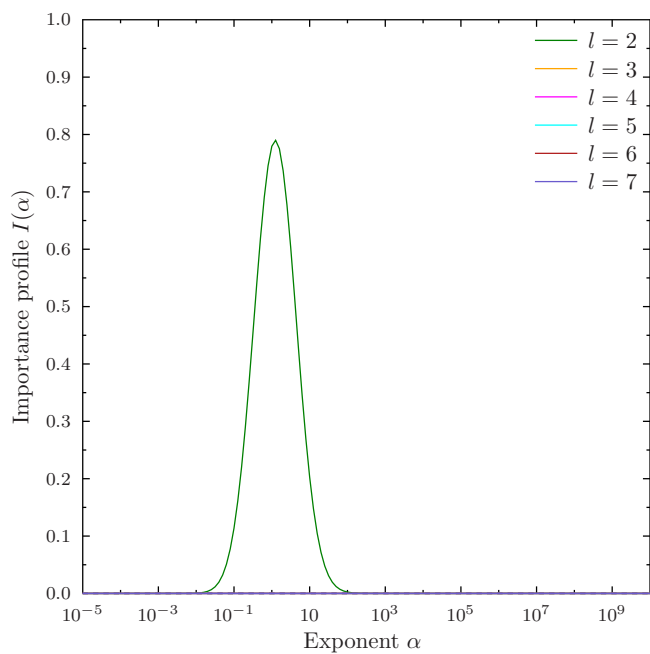

Figure 451. GTO importance profile for  $\delta_-$  orbitals on Mn atom in MnO.

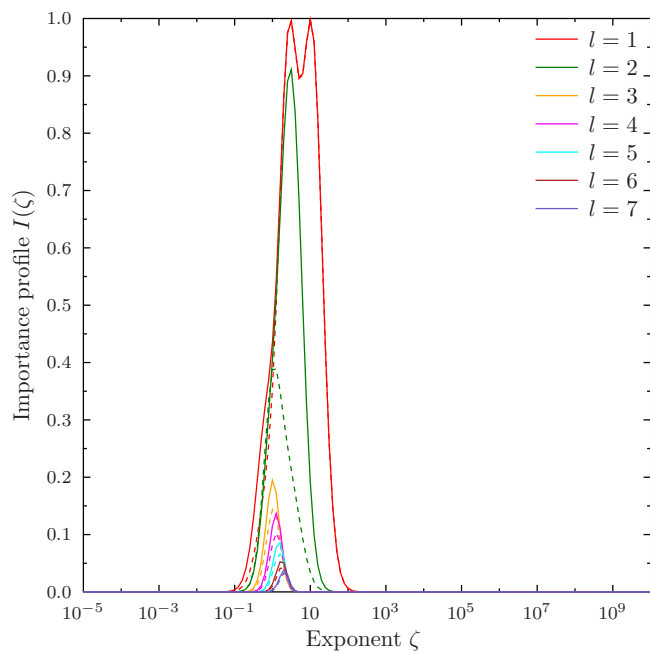

Figure 450. STO importance profile for  $\pi_+$  orbitals on Mn atom in MnS.

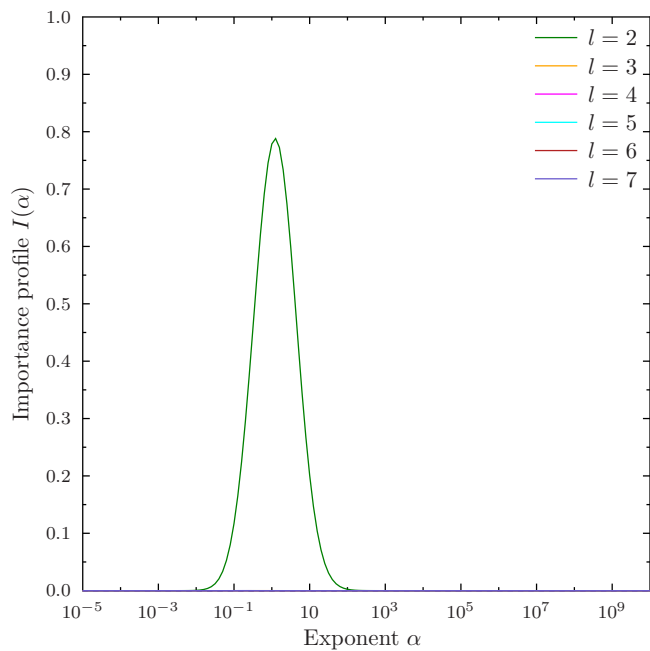

Figure 452. GTO importance profile for  $\delta_-$  orbitals on Mn atom in MnS.

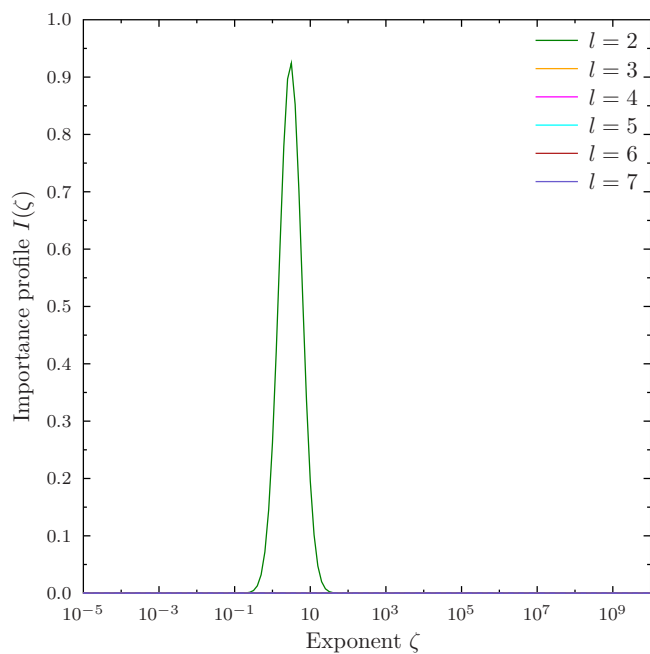

Figure 453. STO importance profile for  $\delta_-$  orbitals on Mn atom in MnO.

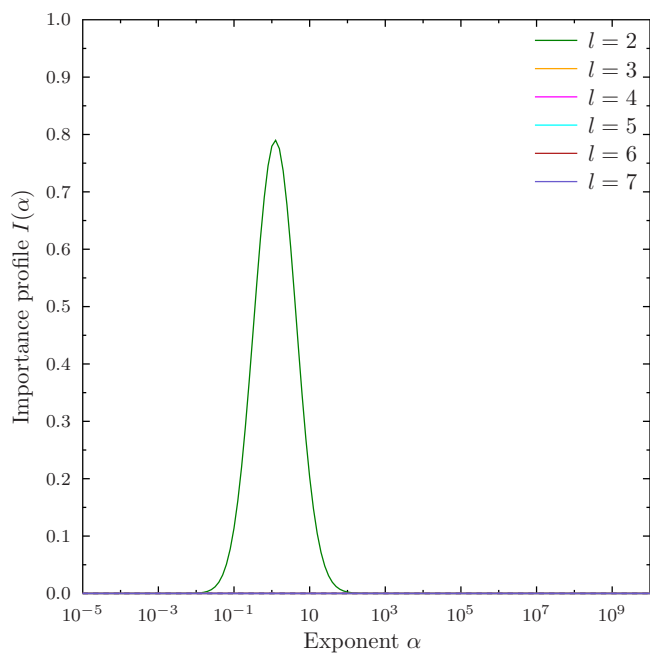

Figure 455. GTO importance profile for  $\delta_+$  orbitals on Mn atom in MnO.

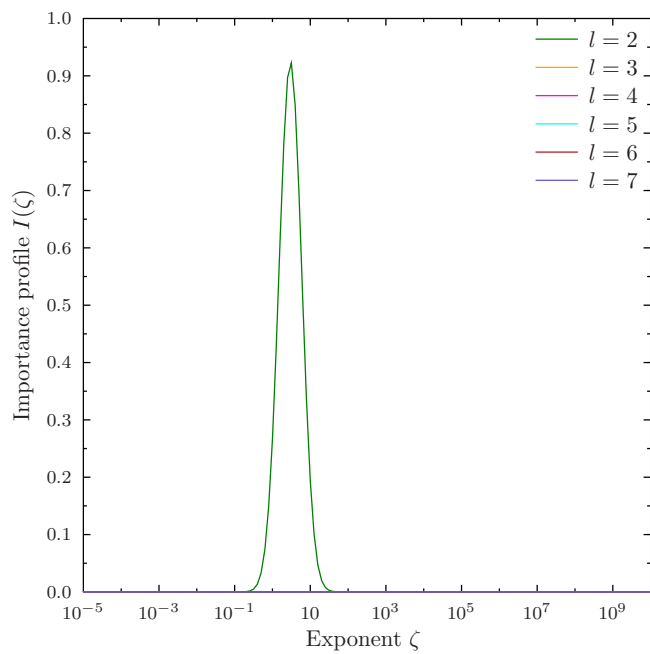

Figure 454. STO importance profile for  $\delta_-$  orbitals on Mn atom in MnS.

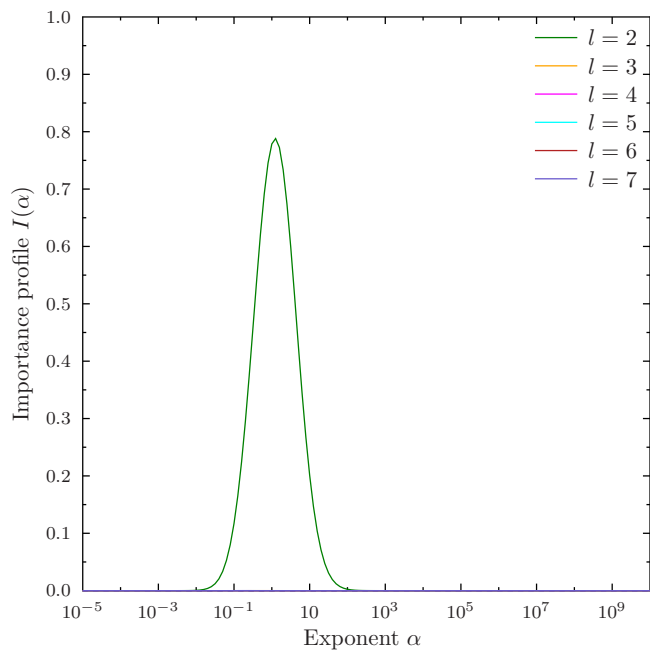

Figure 456. GTO importance profile for  $\delta_+$  orbitals on Mn atom in MnS.

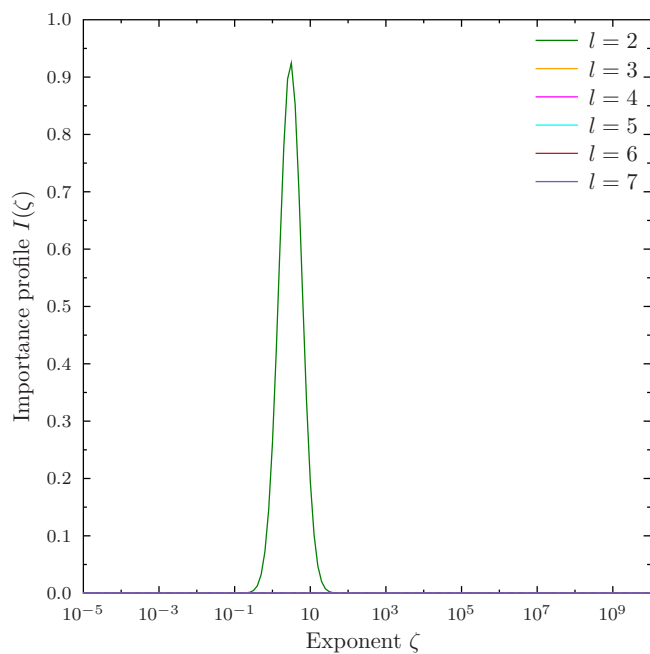

Figure 457. STO importance profile for  $\delta_+$  orbitals on Mn atom in MnO.

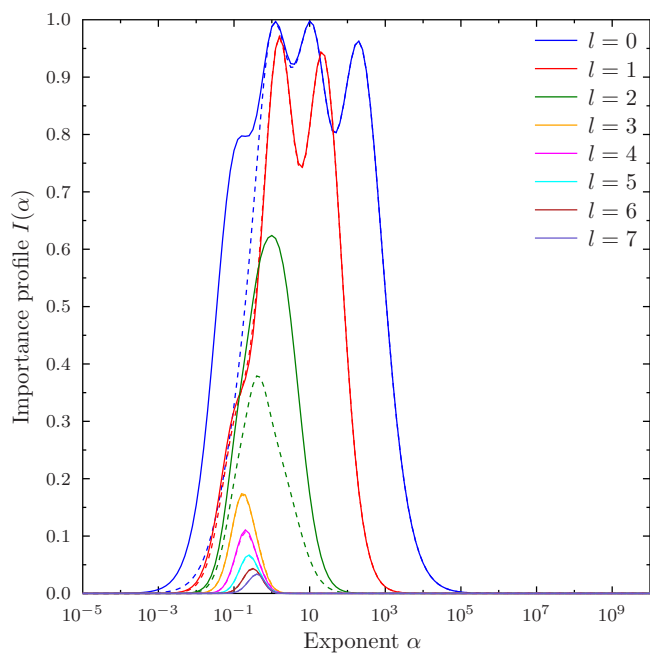

Figure 459. GTO importance profile for  $\sigma$  orbitals on Fe atom in FeO.

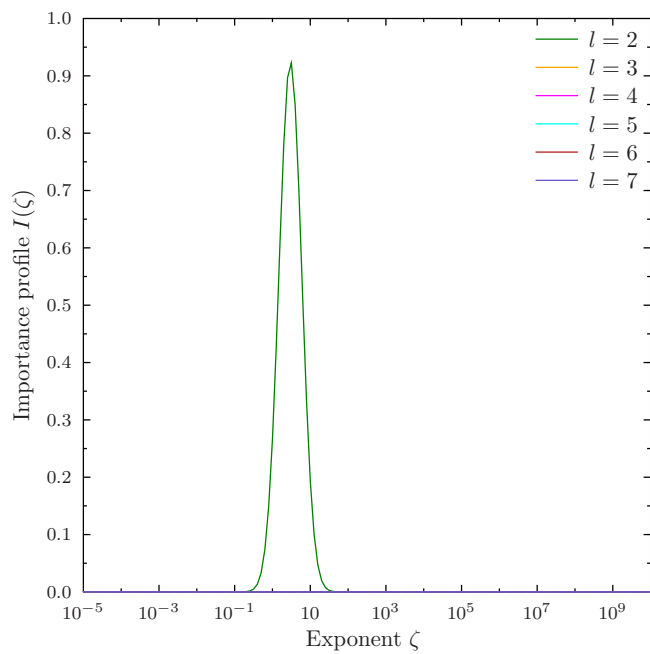

Figure 458. STO importance profile for  $\delta_+$  orbitals on Mn atom in MnS.

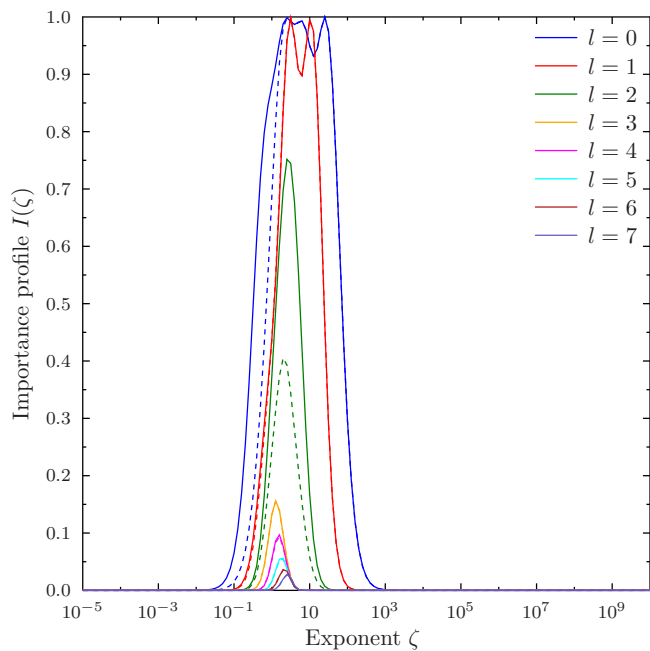

Figure 460. STO importance profile for  $\sigma$  orbitals on Fe atom in FeO.

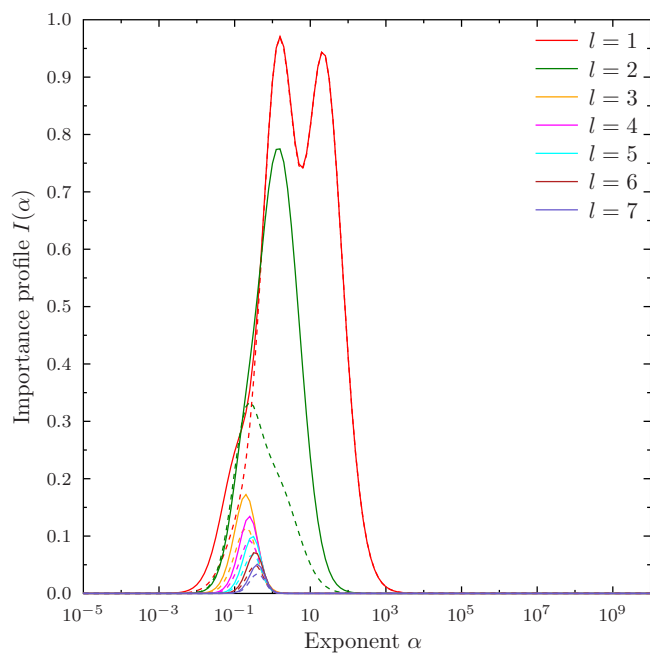

Figure 461. GTO importance profile for  $\pi_-$  orbitals on Fe atom in FeO.

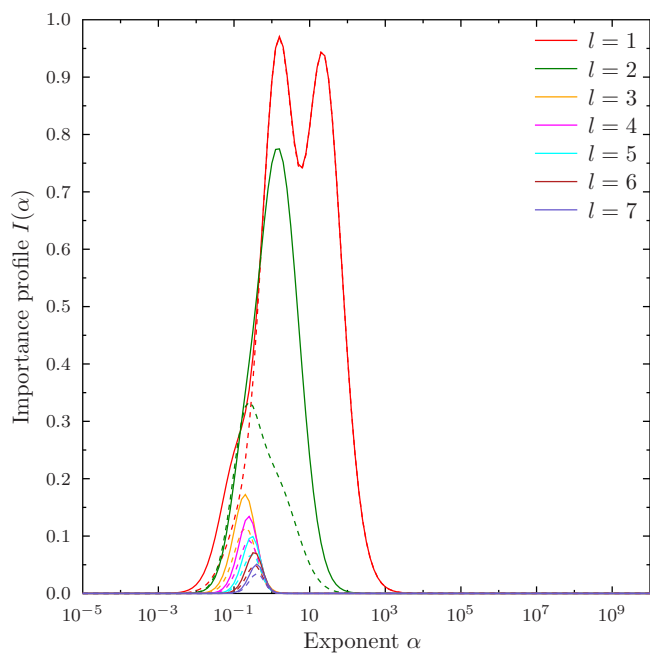

Figure 463. GTO importance profile for  $\pi_+$  orbitals on Fe atom in FeO.

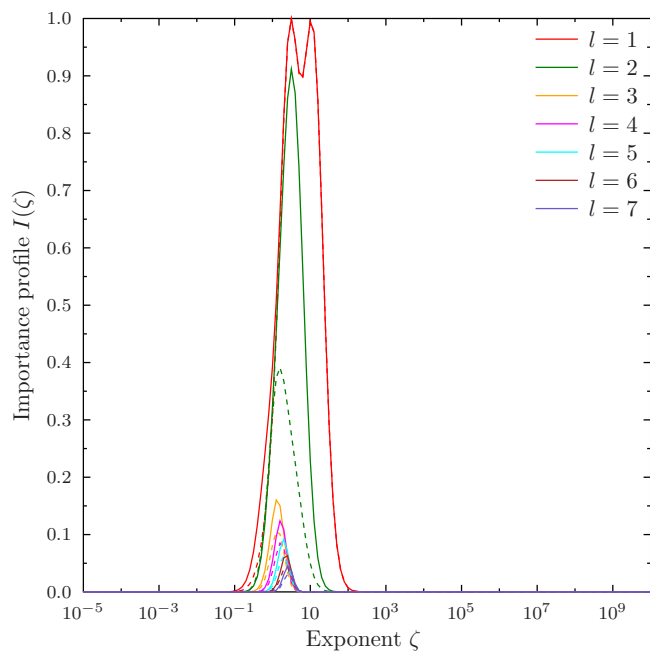

Figure 462. STO importance profile for  $\pi_-$  orbitals on Fe atom in FeO.

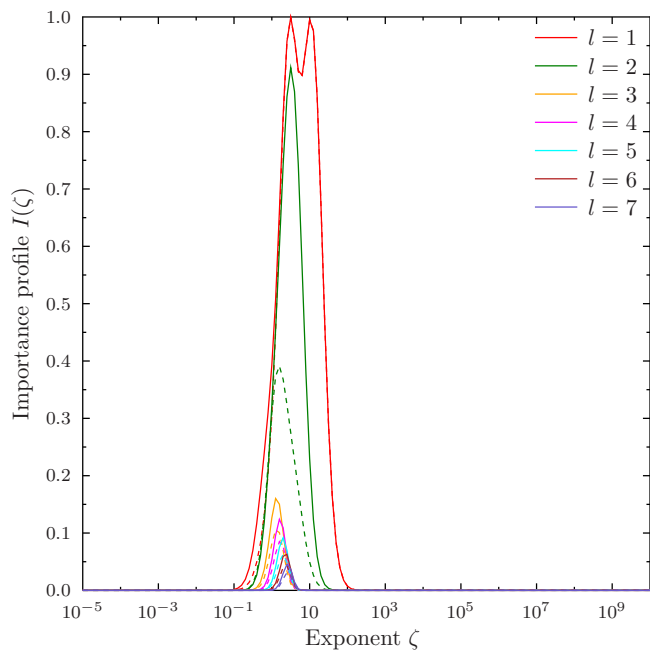

Figure 464. STO importance profile for  $\pi_+$  orbitals on Fe atom in FeO.



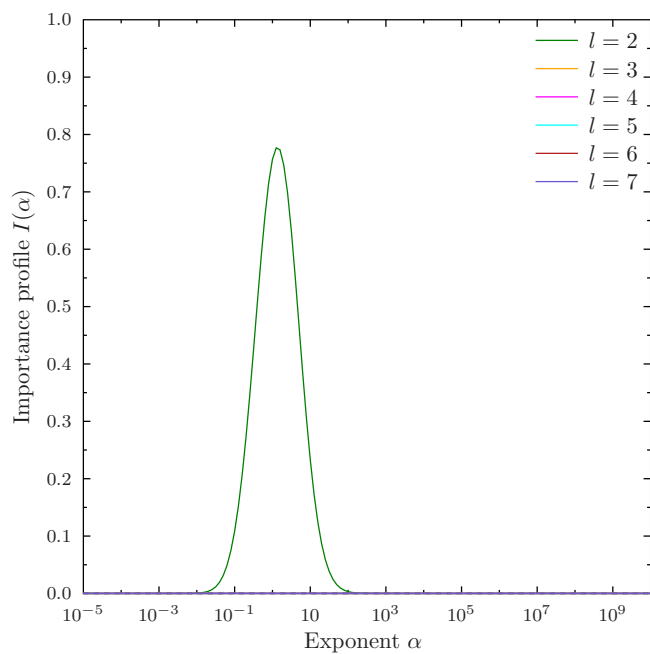

Figure 465. GTO importance profile for  $\delta_-$  orbitals on Fe atom in FeO.

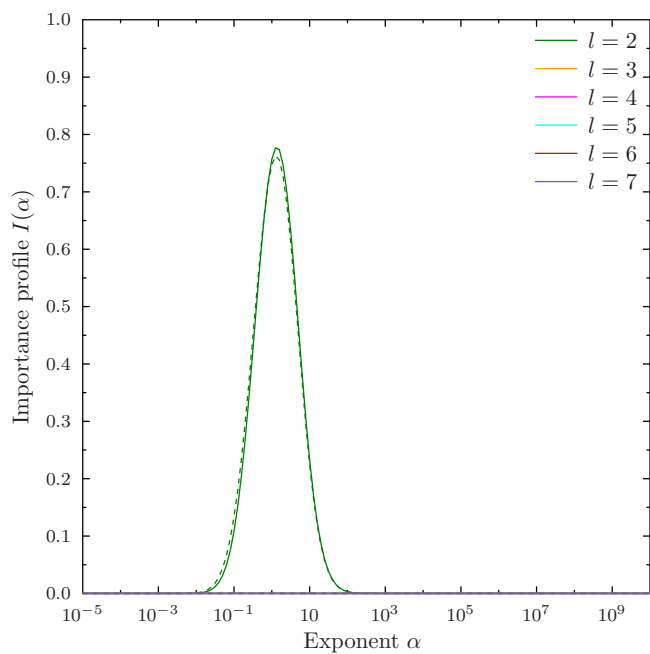

Figure 467. GTO importance profile for  $\delta_+$  orbitals on Fe atom in FeO.

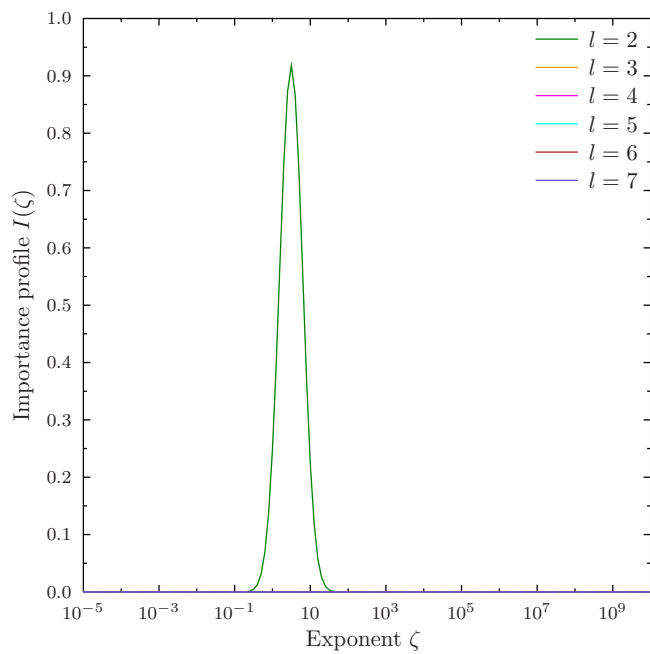

Figure 466. STO importance profile for  $\delta_-$  orbitals on Fe atom in FeO.

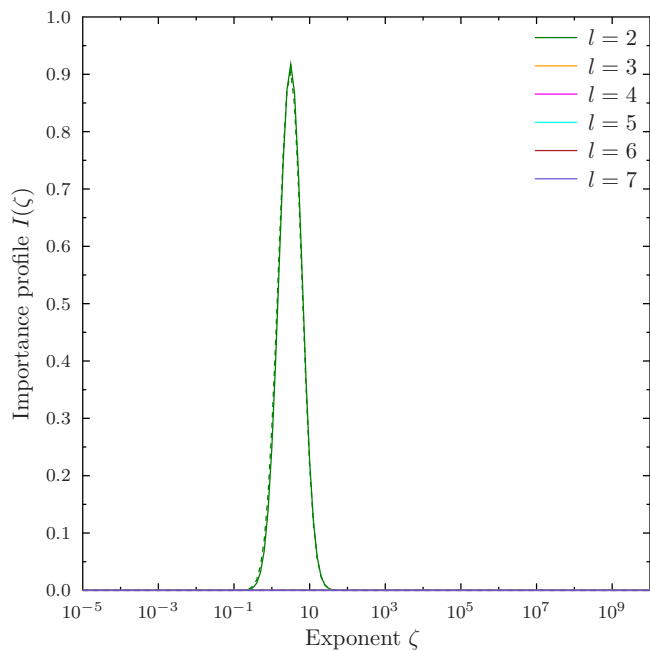

Figure 468. STO importance profile for  $\delta_+$  orbitals on Fe atom in FeO.

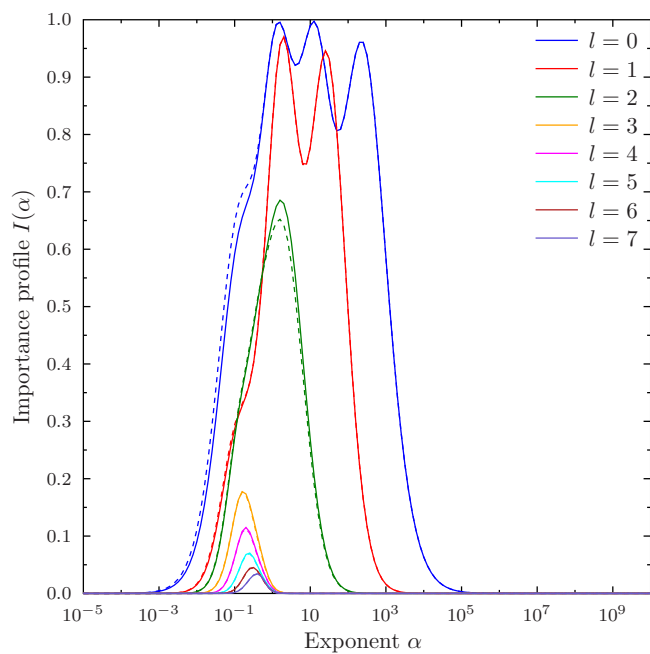

Figure 469. GTO importance profile for  $\sigma$  orbitals on Ni atom in NiO.

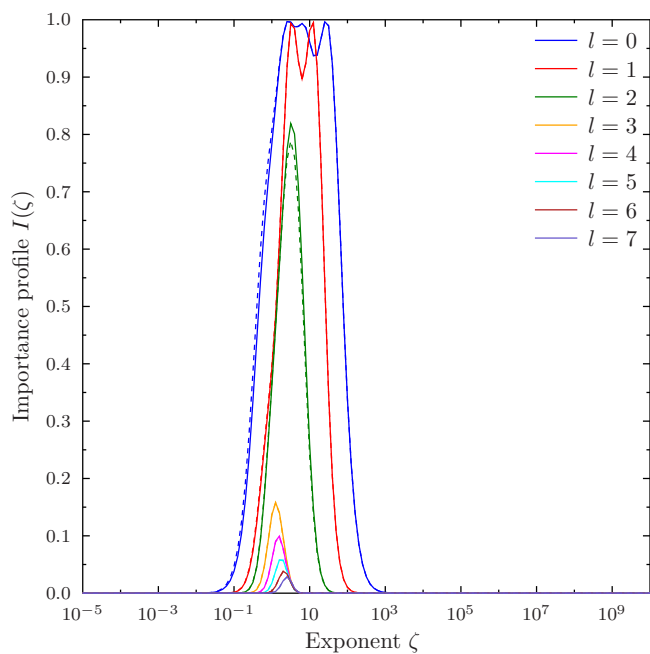

Figure 471. STO importance profile for  $\sigma$  orbitals on Ni atom in NiO.

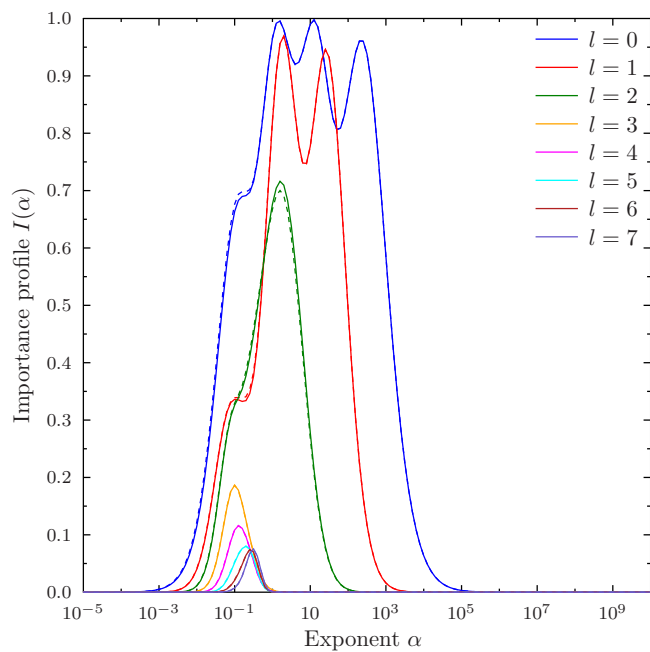

Figure 470. GTO importance profile for  $\sigma$  orbitals on Ni atom in NiS.

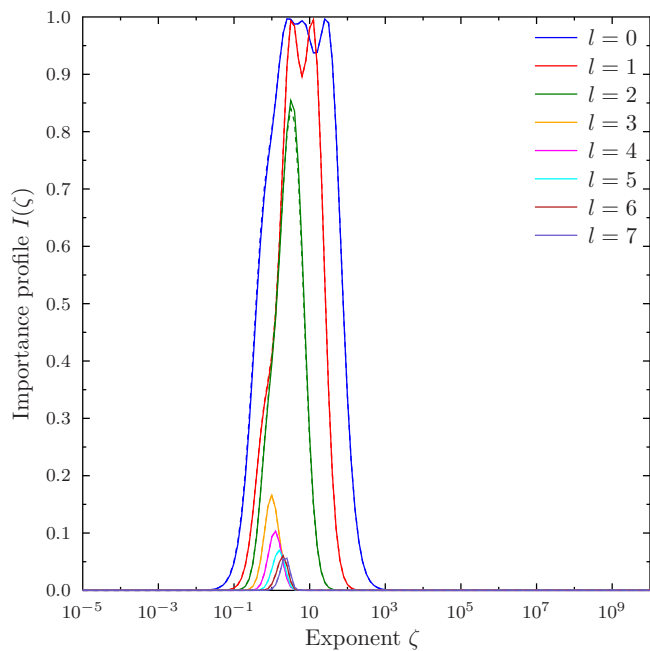

Figure 472. STO importance profile for  $\sigma$  orbitals on Ni atom in NiS.

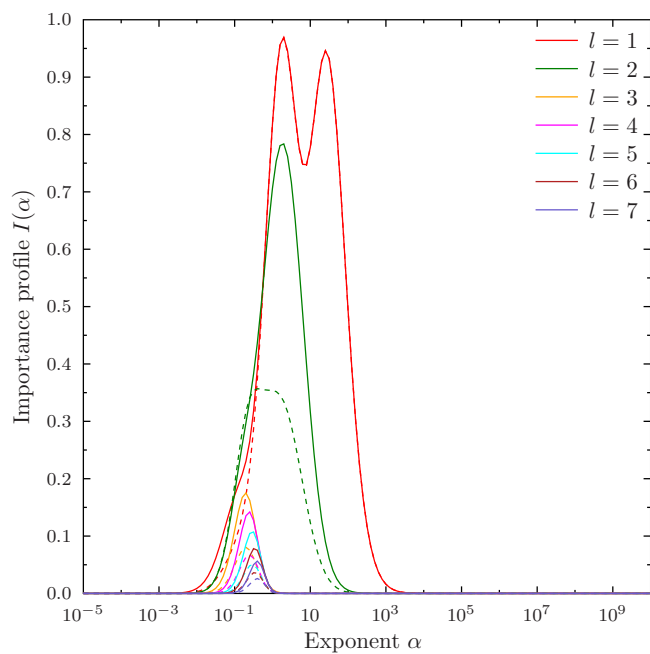

Figure 473. GTO importance profile for  $\pi_-$  orbitals on Ni atom in NiO.

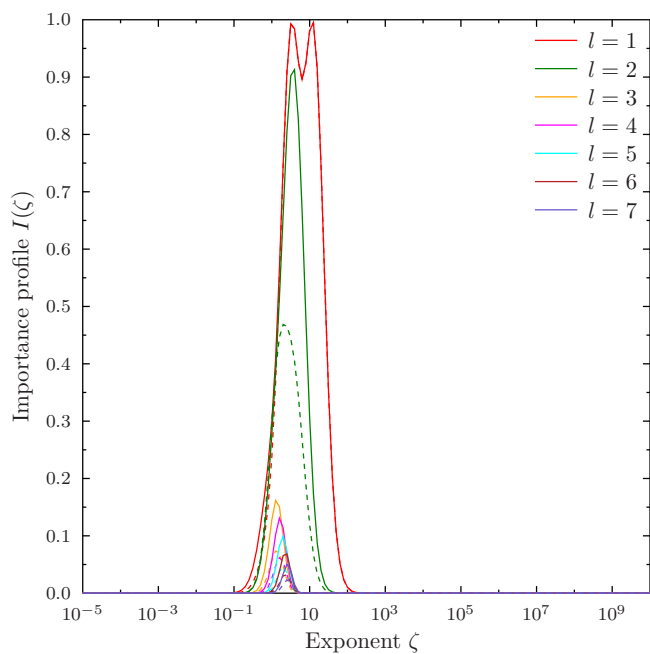

Figure 475. STO importance profile for  $\pi_-$  orbitals on Ni atom in NiO.

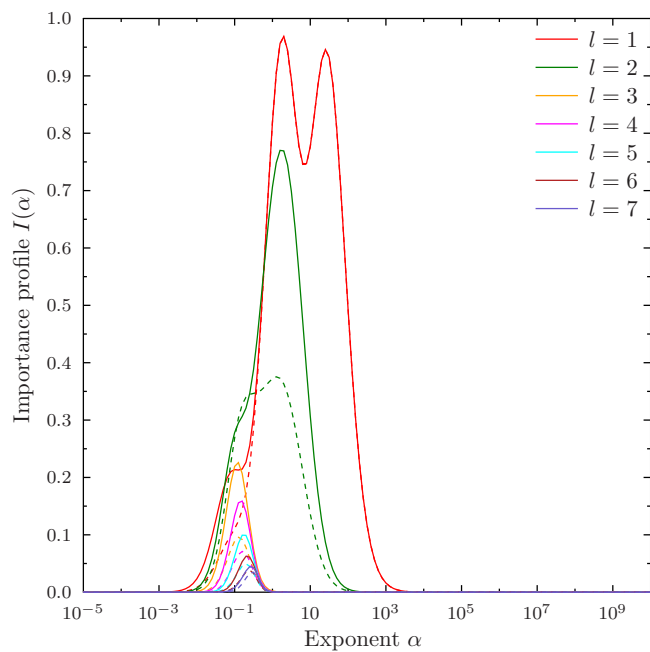

Figure 474. GTO importance profile for  $\pi_-$  orbitals on Ni atom in NiS.

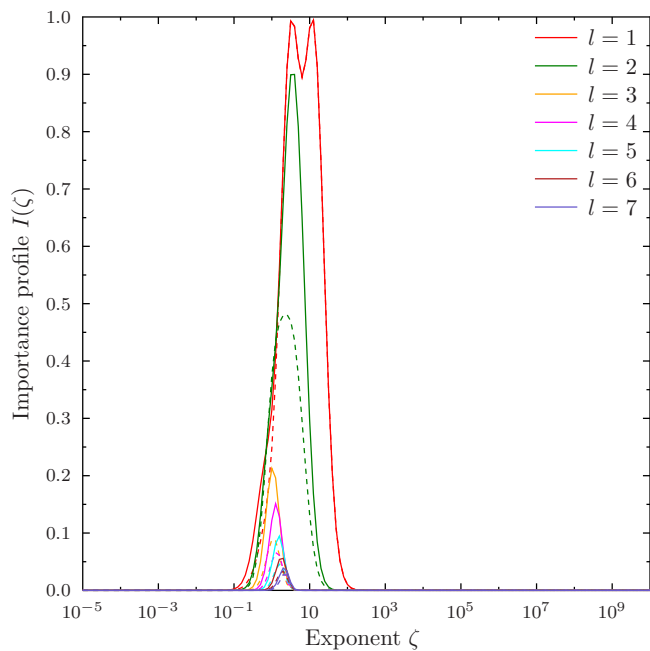

Figure 476. STO importance profile for  $\pi_-$  orbitals on Ni atom in NiS.

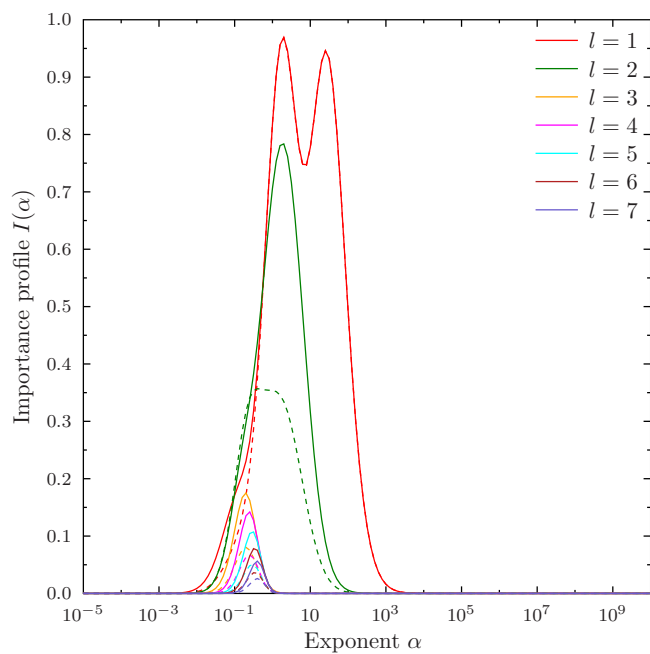

Figure 477. GTO importance profile for  $\pi_+$  orbitals on Ni atom in NiO.

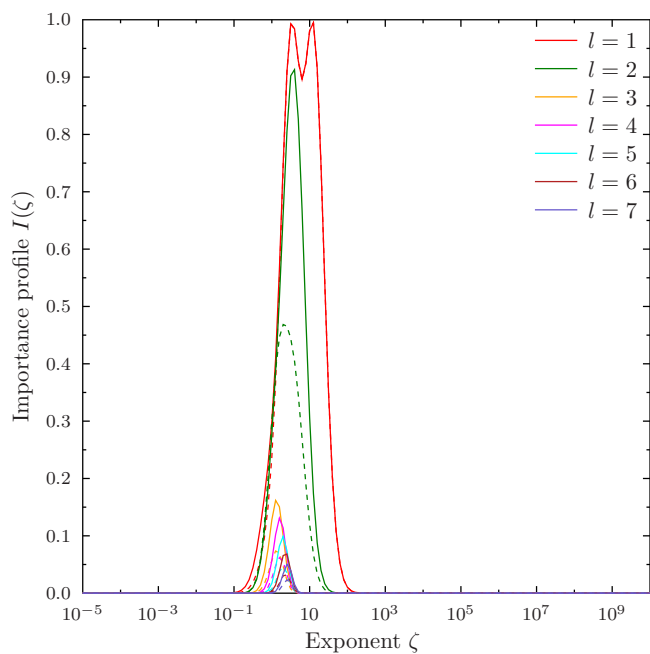

Figure 479. STO importance profile for  $\pi_+$  orbitals on Ni atom in NiO.

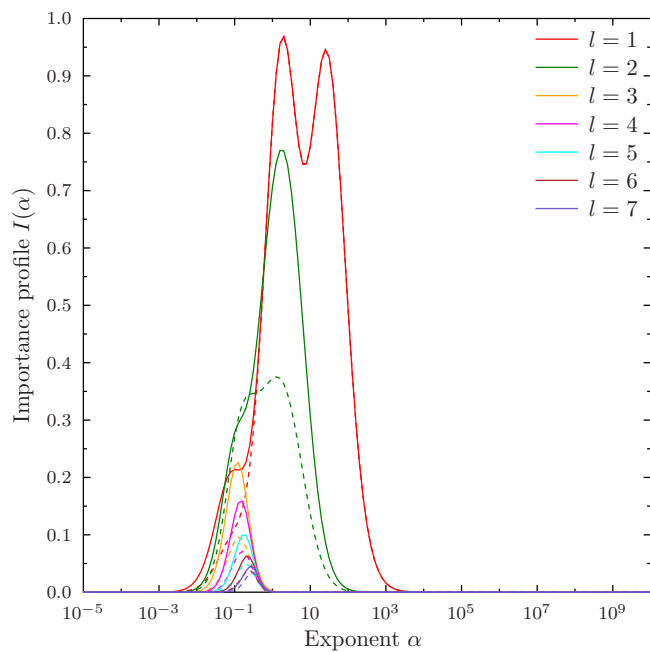

Figure 478. GTO importance profile for  $\pi_+$  orbitals on Ni atom in NiS.

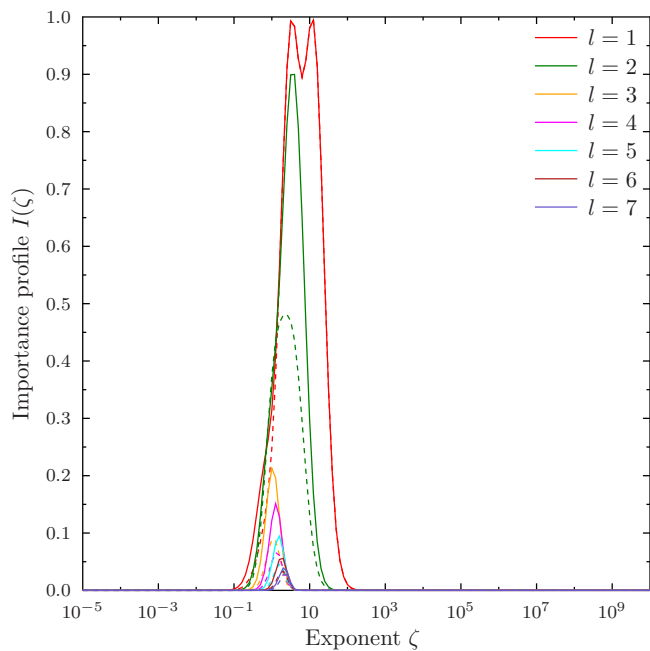

Figure 480. STO importance profile for  $\pi_+$  orbitals on Ni atom in NiS.

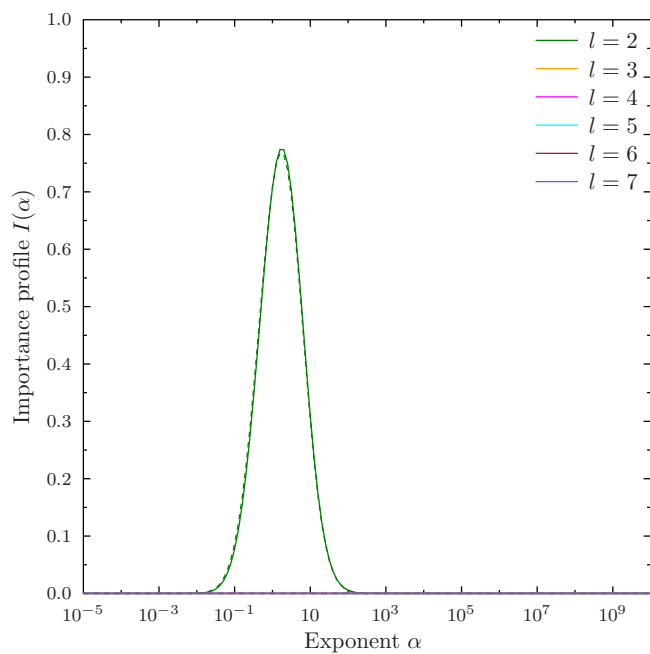

Figure 481. GTO importance profile for  $\delta_-$  orbitals on Ni atom in NiO.

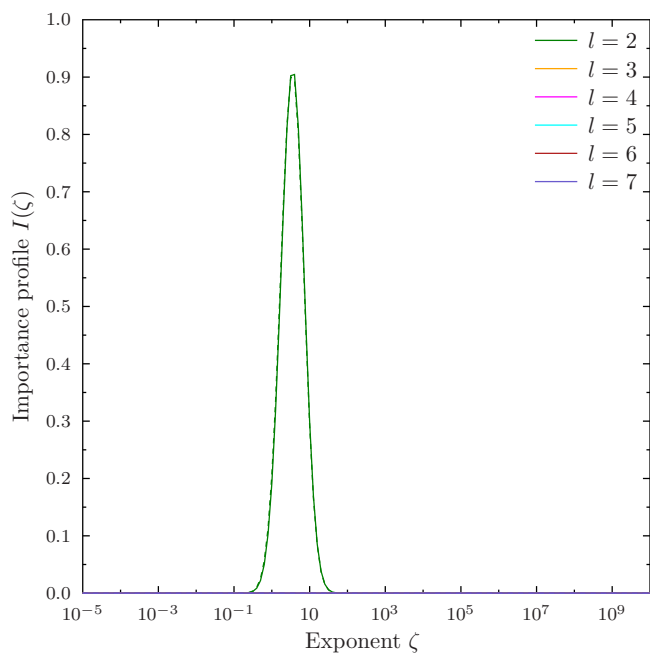

Figure 483. STO importance profile for  $\delta_-$  orbitals on Ni atom in NiO.

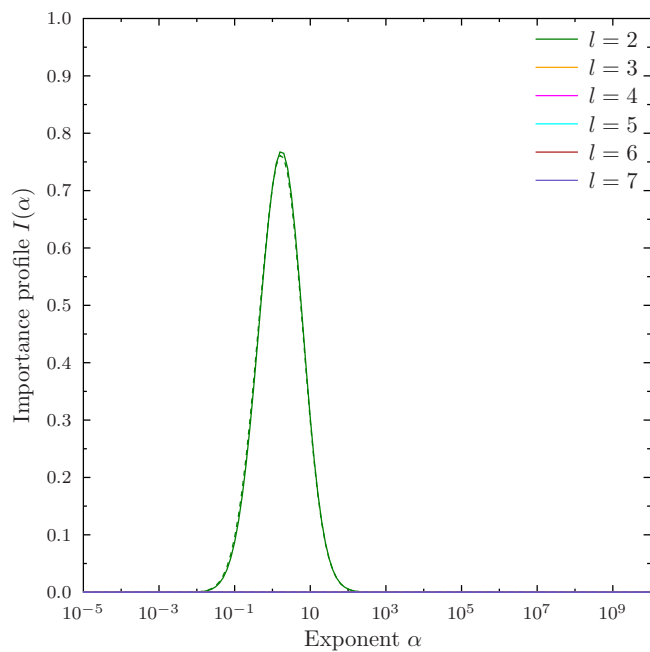

Figure 482. GTO importance profile for  $\delta_-$  orbitals on Ni atom in NiS.

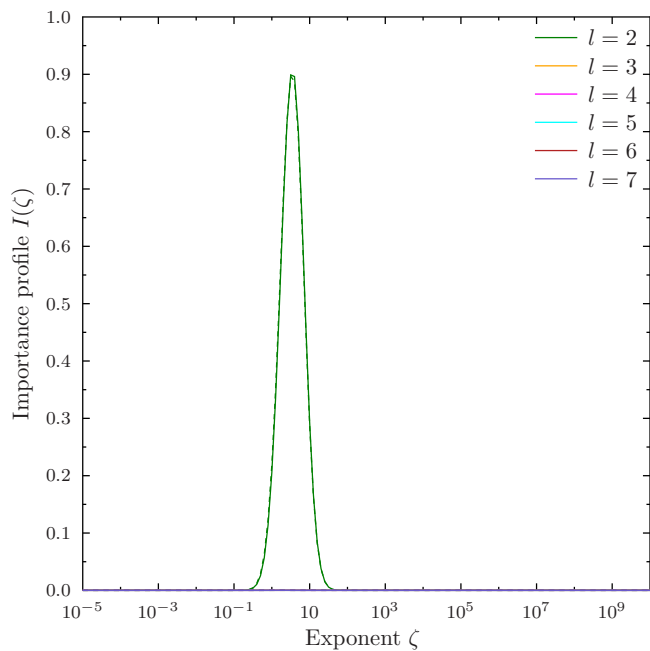

Figure 484. STO importance profile for  $\delta_-$  orbitals on Ni atom in NiS.

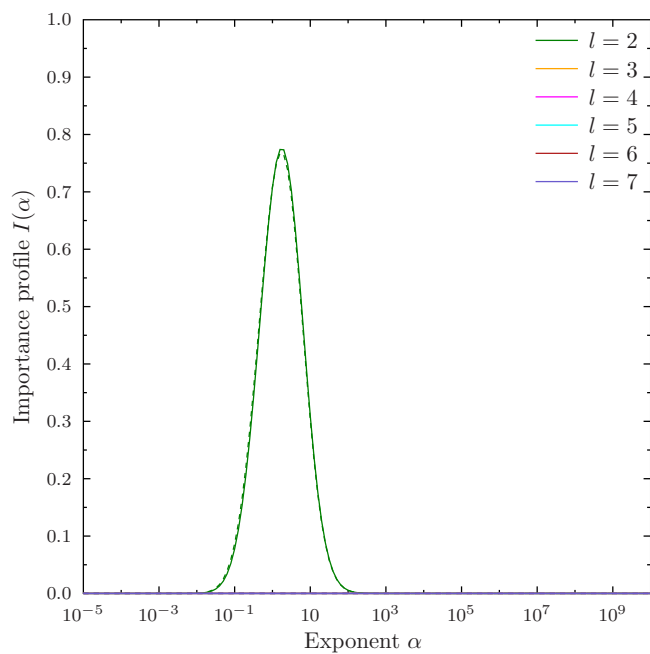

Figure 485. GTO importance profile for  $\delta_+$  orbitals on Ni atom in NiO.

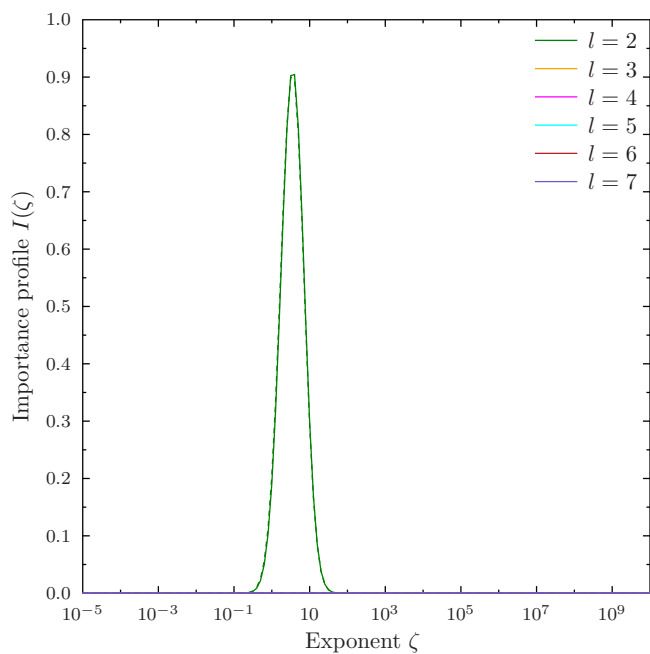

Figure 487. STO importance profile for  $\delta_+$  orbitals on Ni atom in NiO.

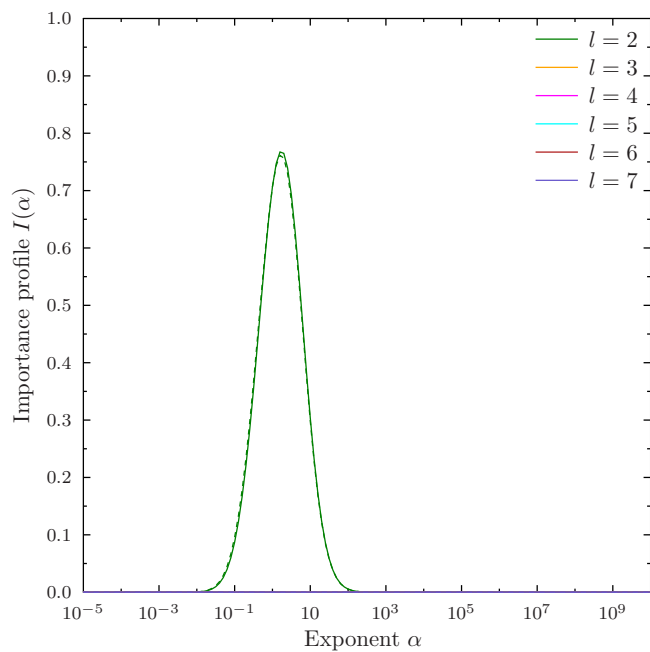

Figure 486. GTO importance profile for  $\delta_+$  orbitals on Ni atom in NiS.

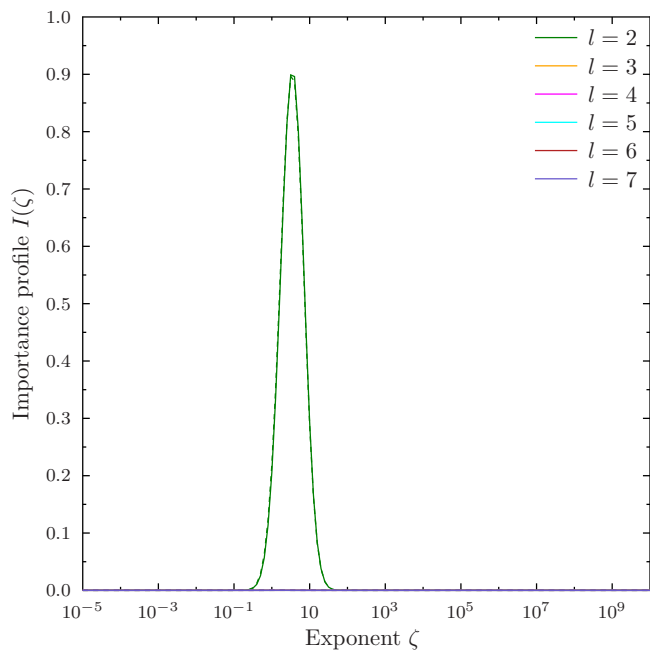

Figure 488. STO importance profile for  $\delta_+$  orbitals on Ni atom in NiS.

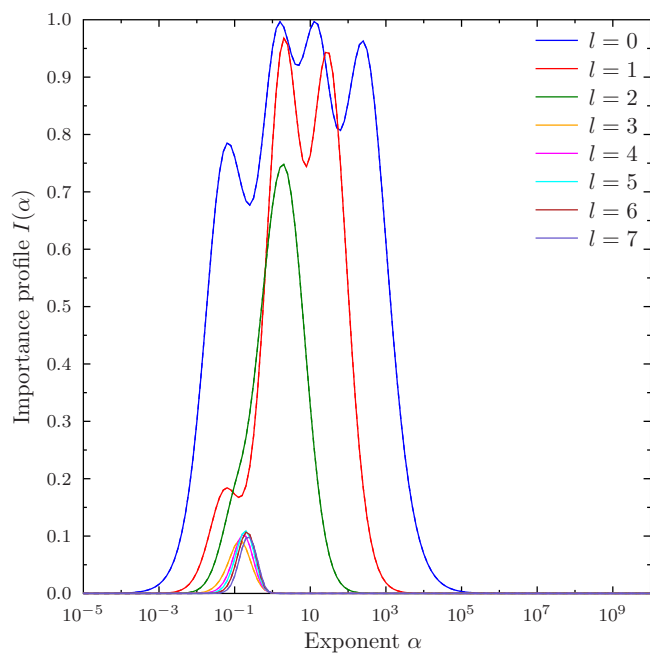

Figure 489. GTO importance profile for  $\sigma$  orbitals on Cu atom in  $\text{Cu}_2$ .

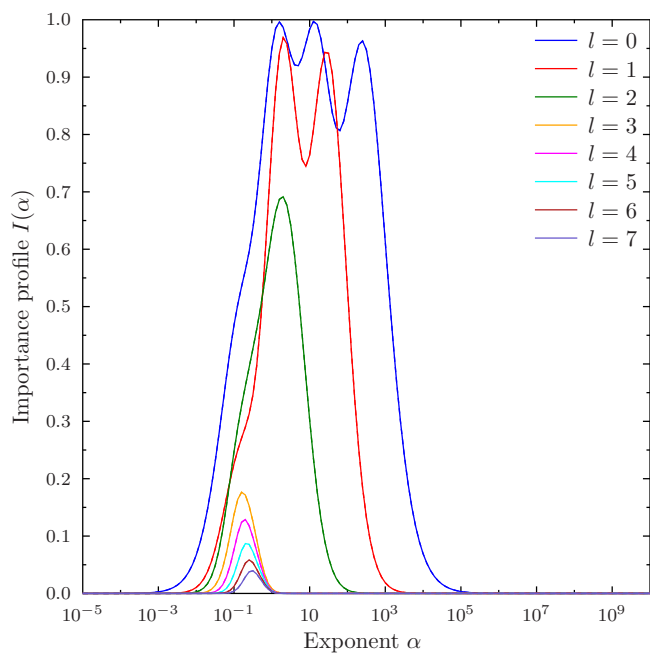

Figure 491. GTO importance profile for  $\sigma$  orbitals on Cu atom in  $\text{CuF}$ .

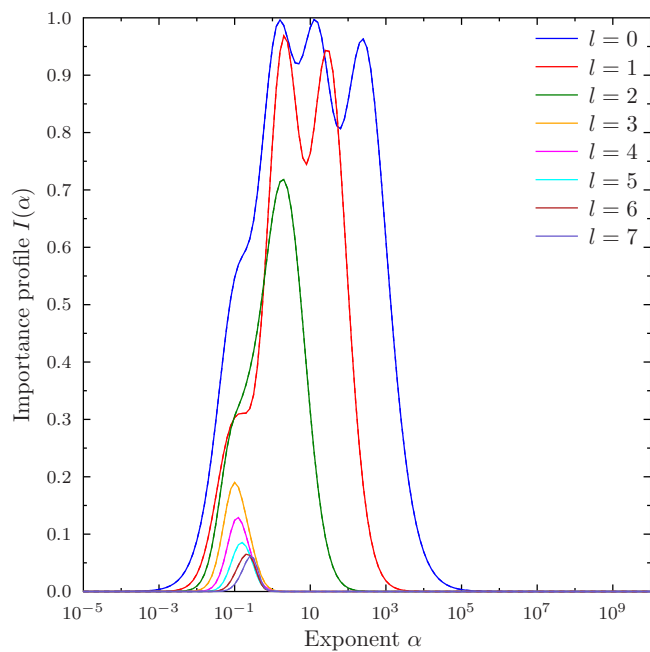

Figure 490. GTO importance profile for  $\sigma$  orbitals on Cu atom in  $\text{CuCl}$ .

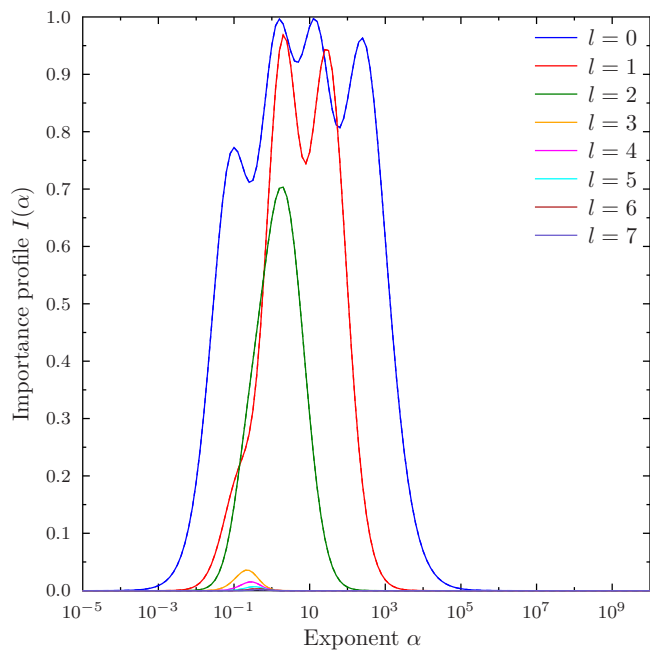

Figure 492. GTO importance profile for  $\sigma$  orbitals on Cu atom in  $\text{CuH}$ .

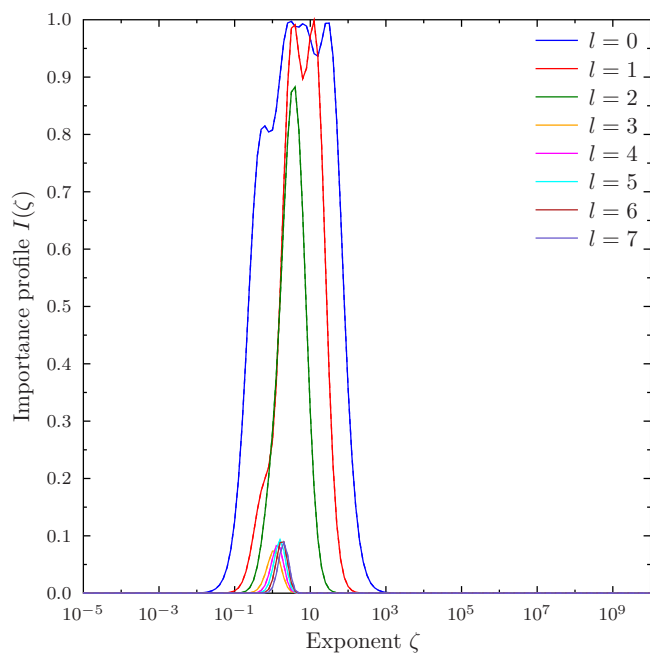

Figure 493. STO importance profile for  $\sigma$  orbitals on Cu atom in  $\text{Cu}_2$ .

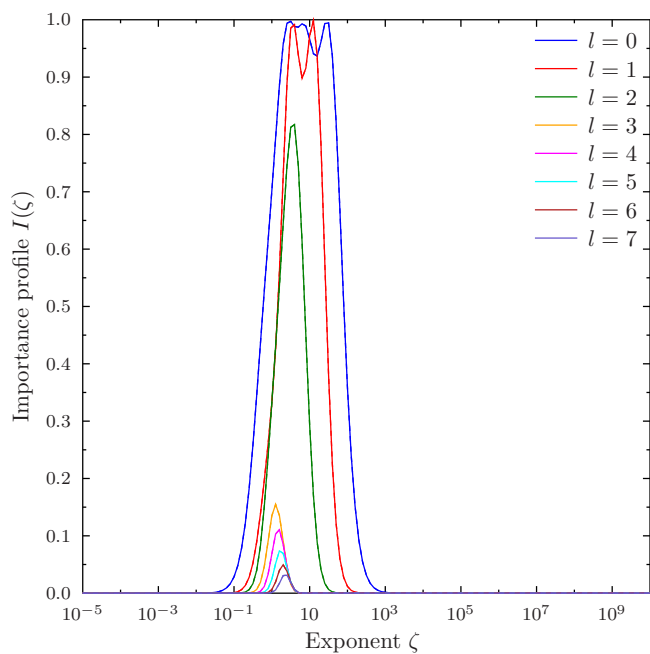

Figure 495. STO importance profile for  $\sigma$  orbitals on Cu atom in  $\text{CuF}$ .

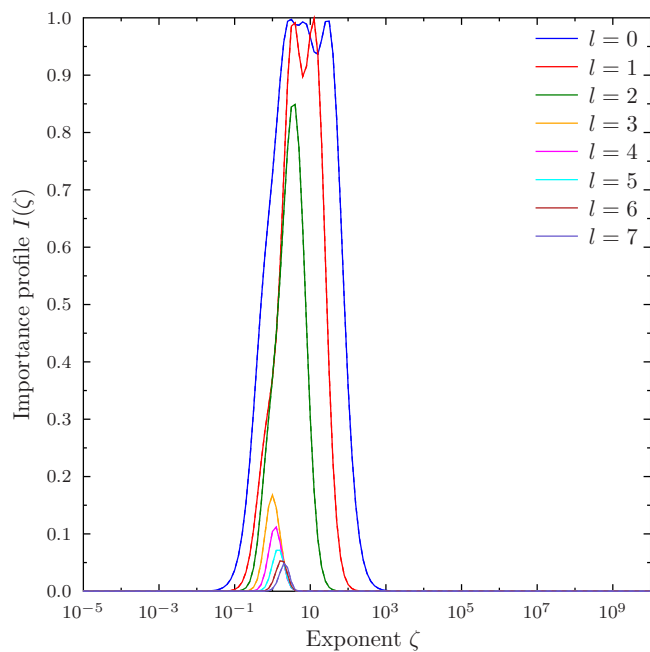

Figure 494. STO importance profile for  $\sigma$  orbitals on Cu atom in  $\text{CuCl}$ .

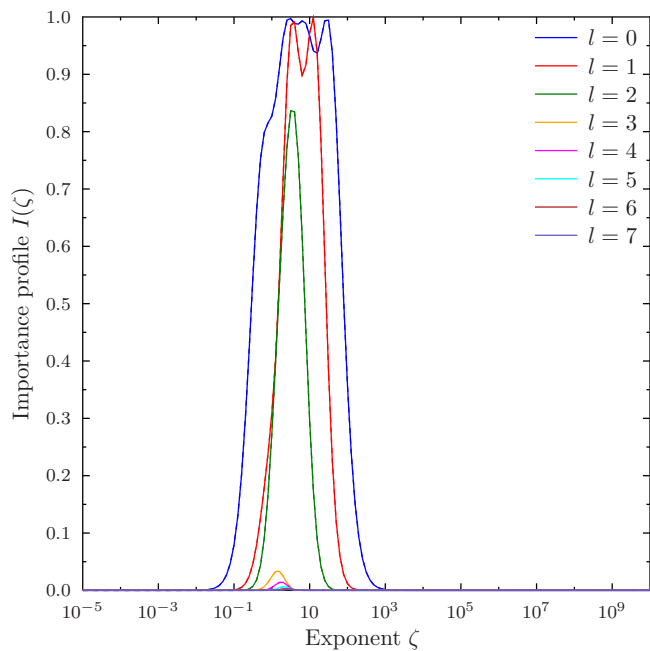

Figure 496. STO importance profile for  $\sigma$  orbitals on Cu atom in  $\text{CuH}$ .



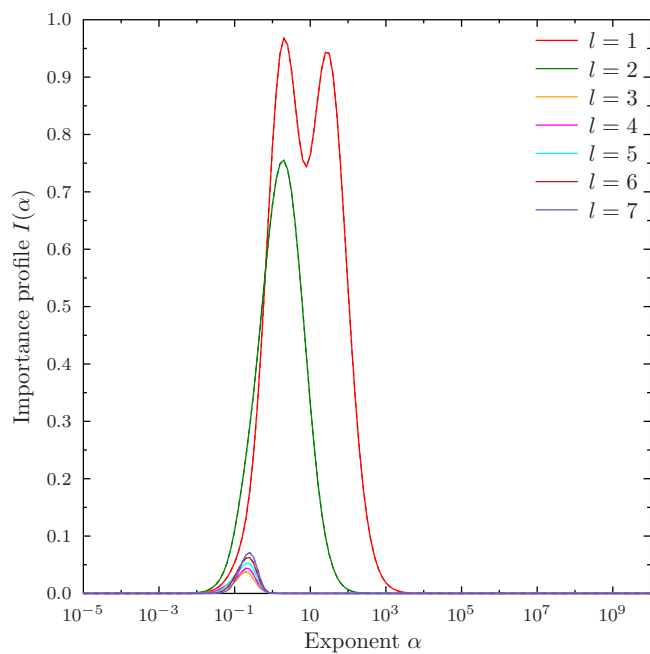

Figure 497. GTO importance profile for  $\pi_-$  orbitals on Cu atom in  $\text{Cu}_2$ .

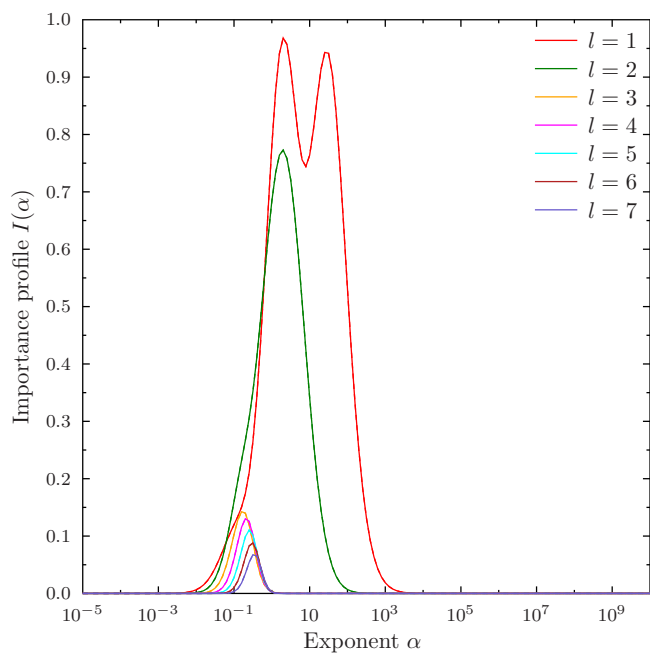

Figure 499. GTO importance profile for  $\pi_-$  orbitals on Cu atom in  $\text{CuF}$ .

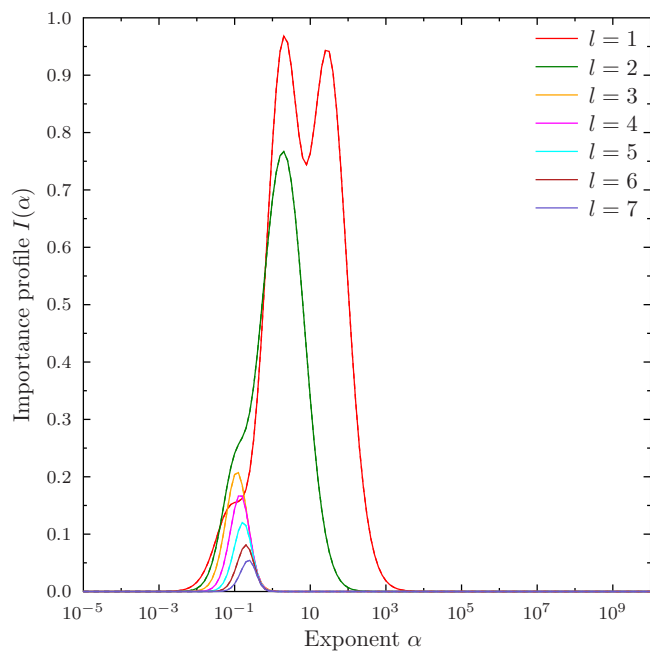

Figure 498. GTO importance profile for  $\pi_-$  orbitals on Cu atom in  $\text{CuCl}$ .

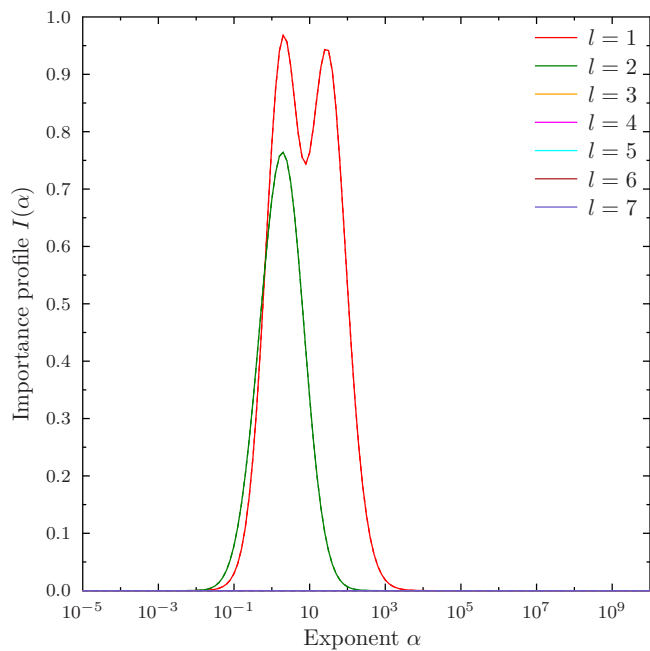

Figure 500. GTO importance profile for  $\pi_-$  orbitals on Cu atom in  $\text{CuH}$ .

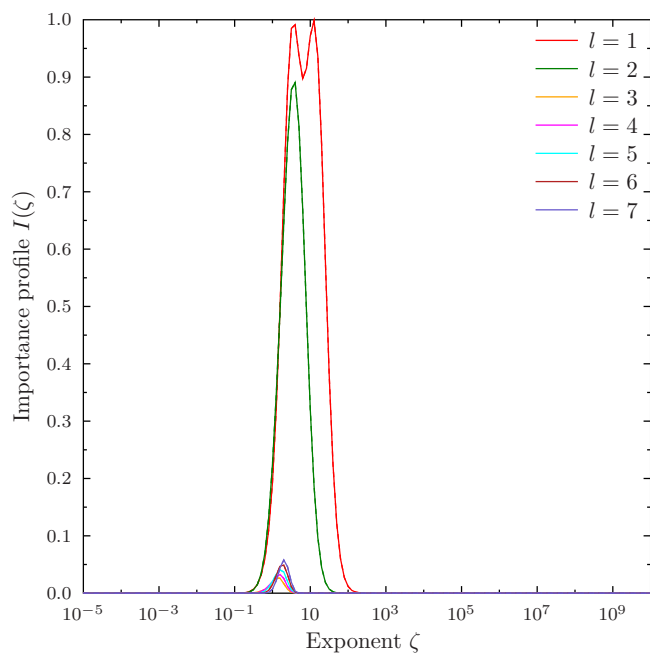

Figure 501. STO importance profile for  $\pi_-$  orbitals on Cu atom in  $\text{Cu}_2$ .

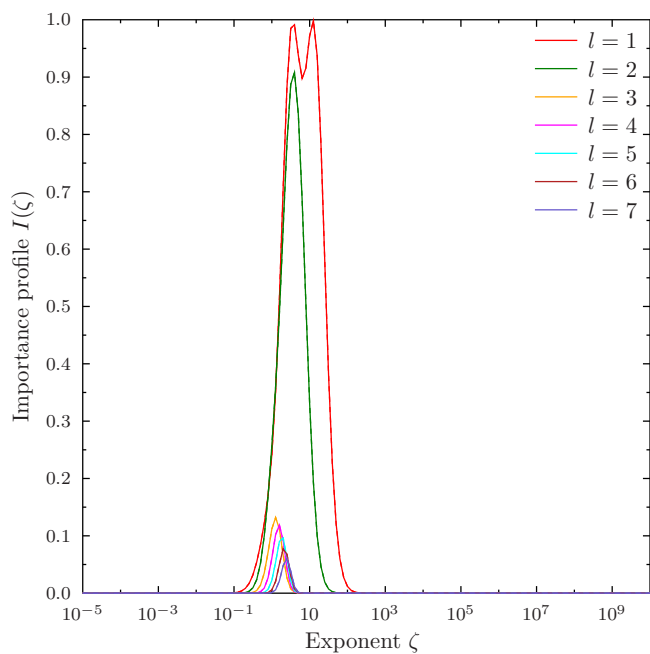

Figure 503. STO importance profile for  $\pi_-$  orbitals on Cu atom in  $\text{CuF}$ .

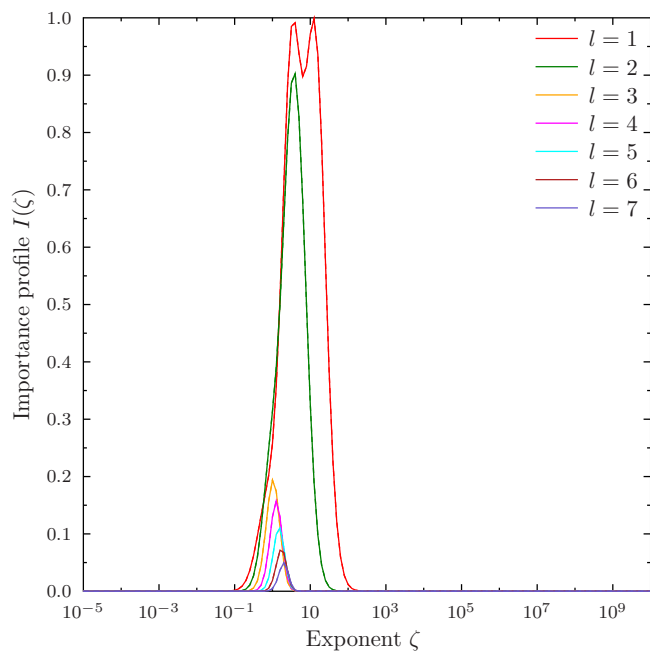

Figure 502. STO importance profile for  $\pi_-$  orbitals on Cu atom in  $\text{CuCl}$ .

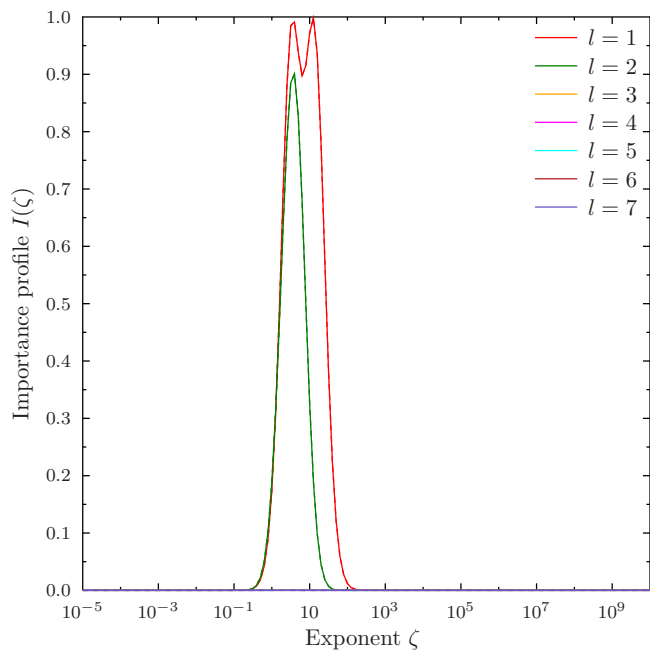

Figure 504. STO importance profile for  $\pi_-$  orbitals on Cu atom in  $\text{CuH}$ .

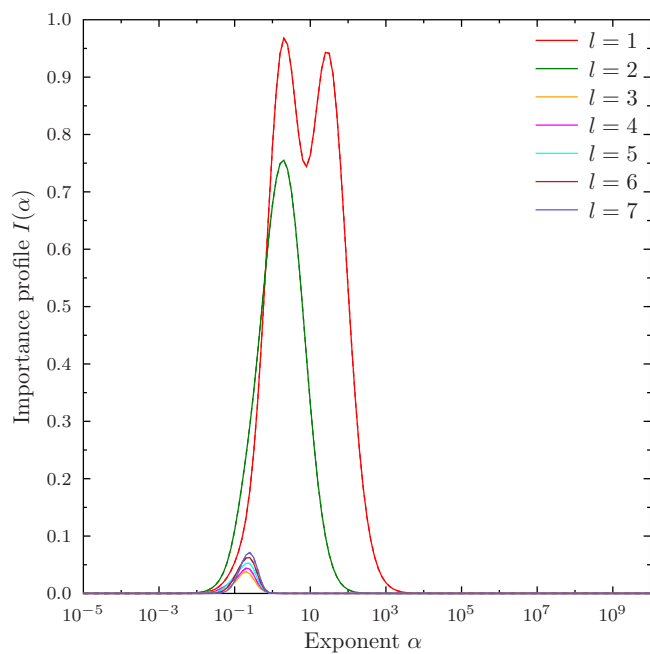

Figure 505. GTO importance profile for  $\pi_+$  orbitals on Cu atom in  $\text{Cu}_2$ .

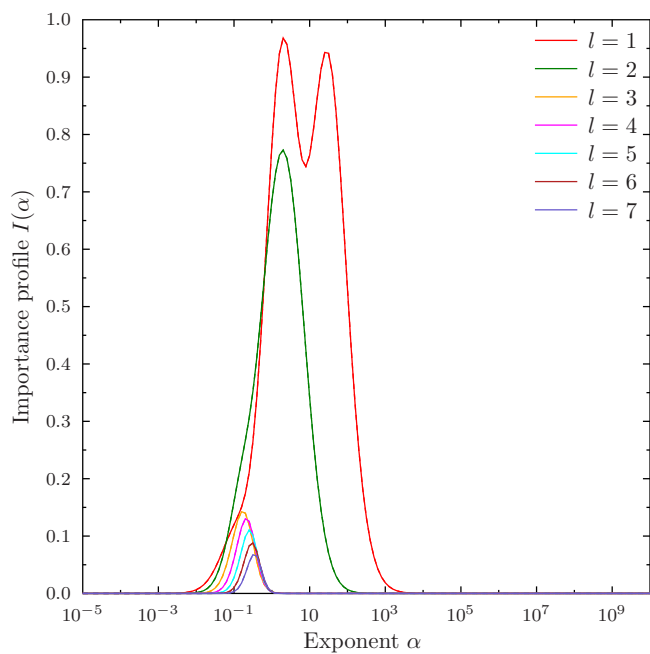

Figure 507. GTO importance profile for  $\pi_+$  orbitals on Cu atom in  $\text{CuF}$ .

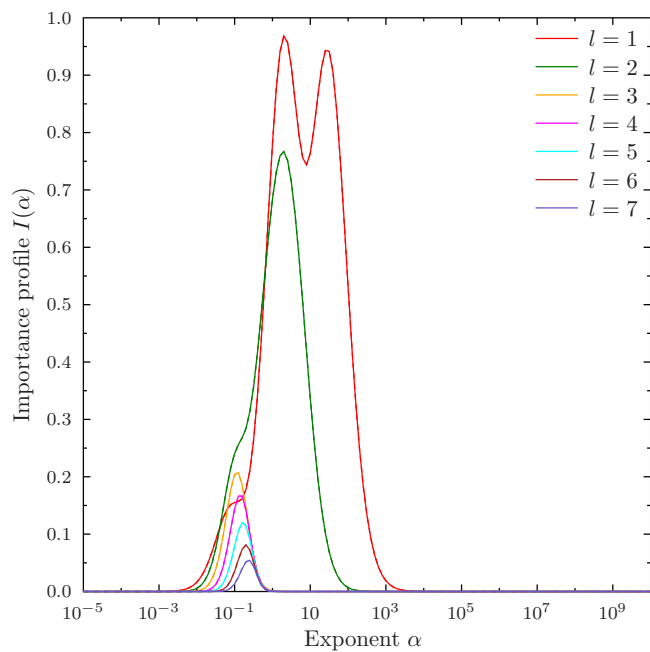

Figure 506. GTO importance profile for  $\pi_+$  orbitals on Cu atom in  $\text{CuCl}$ .

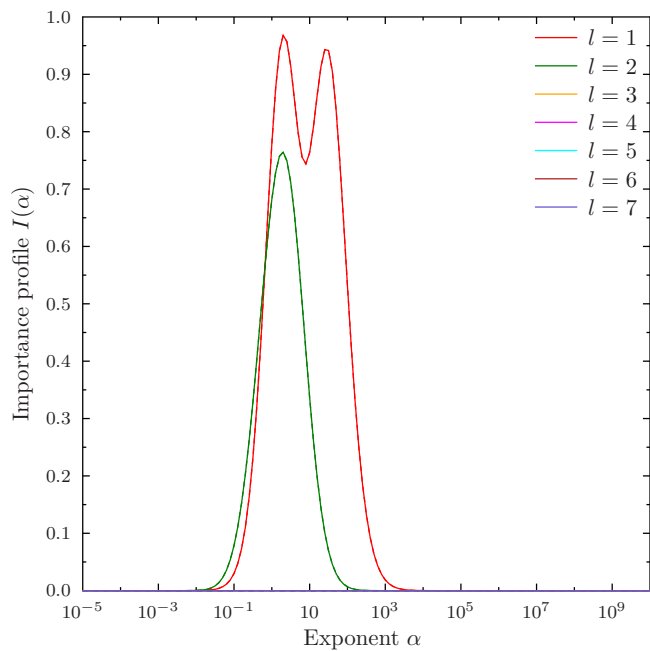

Figure 508. GTO importance profile for  $\pi_+$  orbitals on Cu atom in  $\text{CuH}$ .

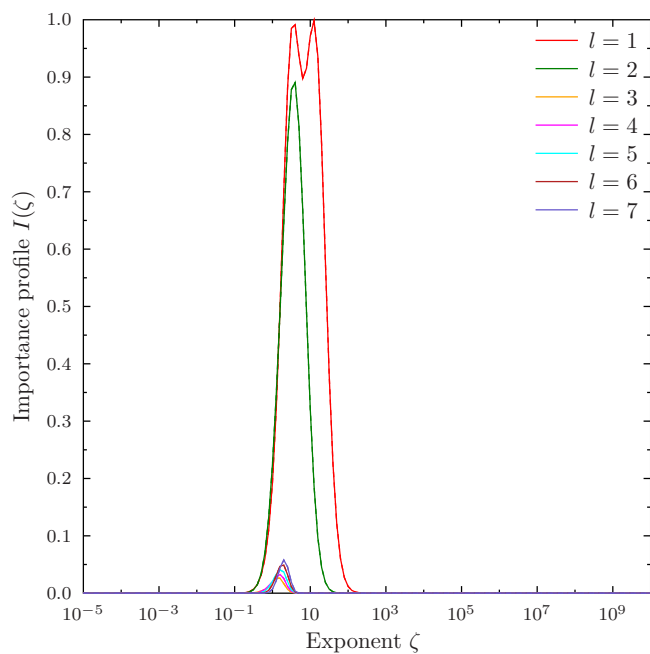

Figure 509. STO importance profile for  $\pi_+$  orbitals on Cu atom in  $\text{Cu}_2$ .

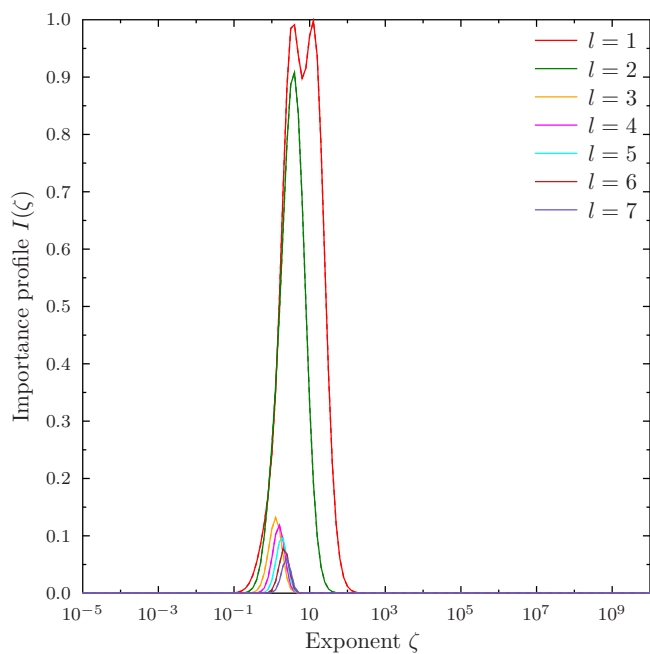

Figure 511. STO importance profile for  $\pi_+$  orbitals on Cu atom in  $\text{CuF}$ .

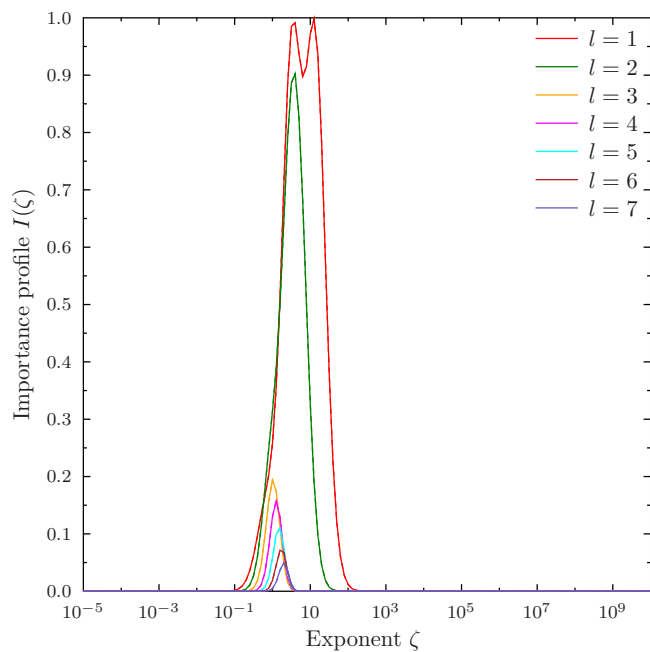

Figure 510. STO importance profile for  $\pi_+$  orbitals on Cu atom in  $\text{CuCl}$ .

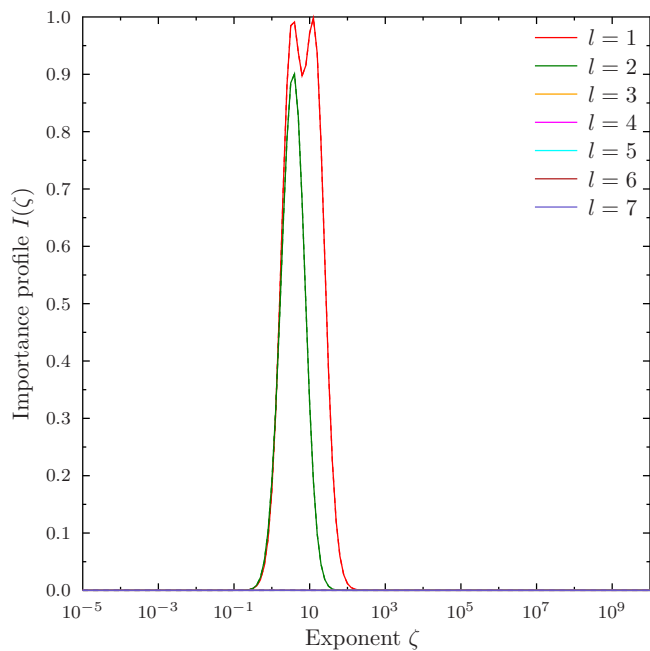

Figure 512. STO importance profile for  $\pi_+$  orbitals on Cu atom in  $\text{CuH}$ .

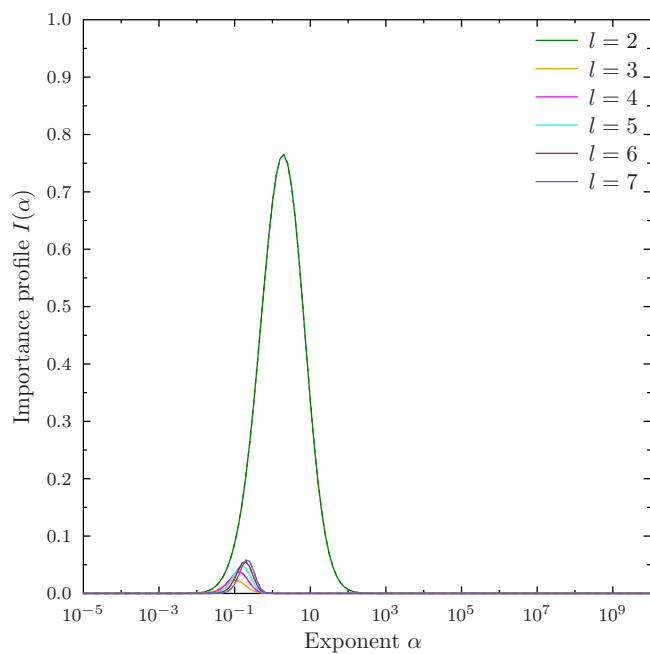

Figure 513. GTO importance profile for  $\delta_-$  orbitals on Cu atom in  $\text{Cu}_2$ .

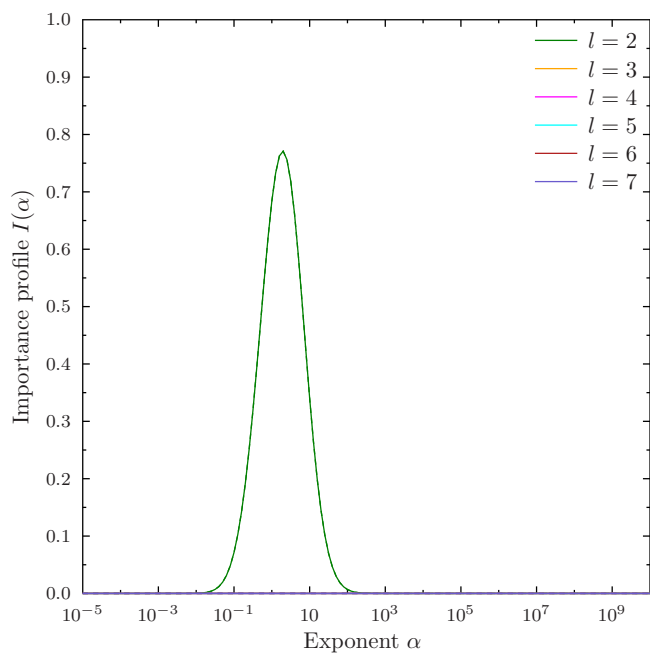

Figure 515. GTO importance profile for  $\delta_-$  orbitals on Cu atom in  $\text{CuF}$ .

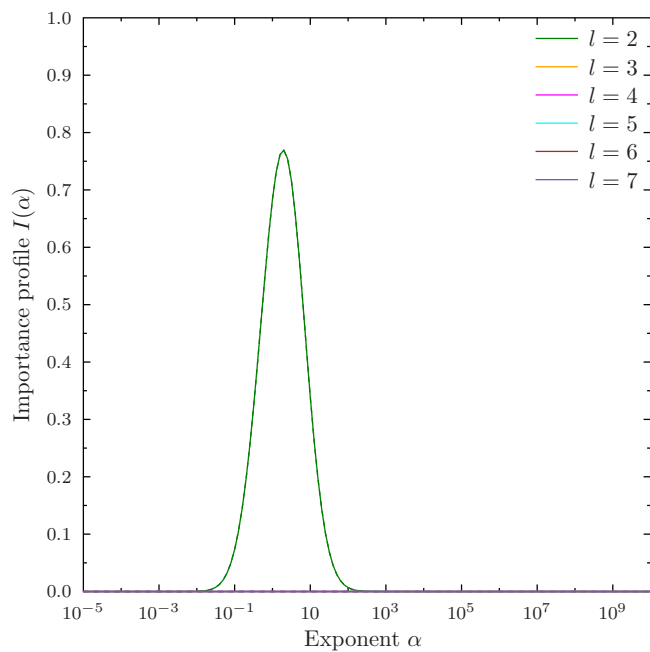

Figure 514. GTO importance profile for  $\delta_-$  orbitals on Cu atom in  $\text{CuCl}$ .

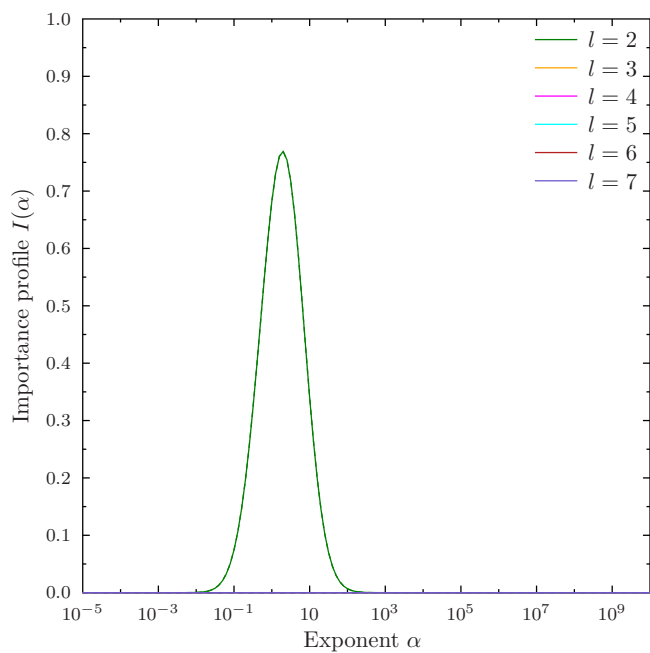

Figure 516. GTO importance profile for  $\delta_-$  orbitals on Cu atom in  $\text{CuH}$ .

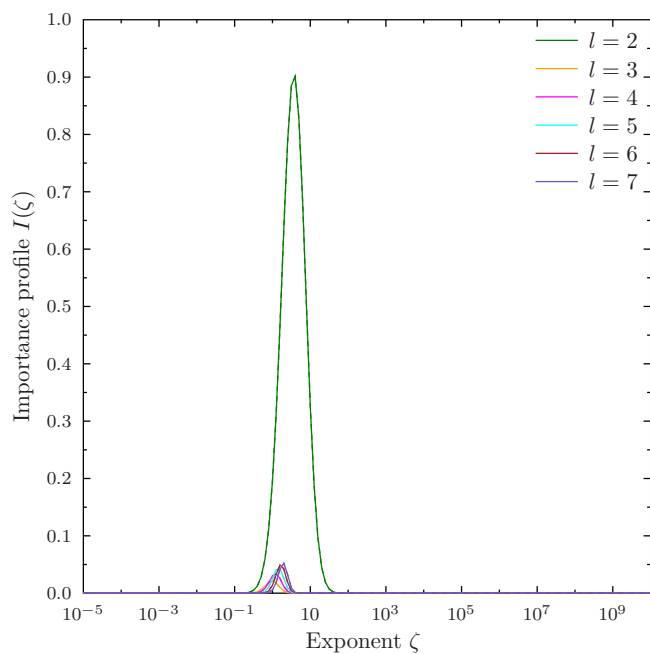

Figure 517. STO importance profile for  $\delta_-$  orbitals on Cu atom in  $\text{Cu}_2$ .

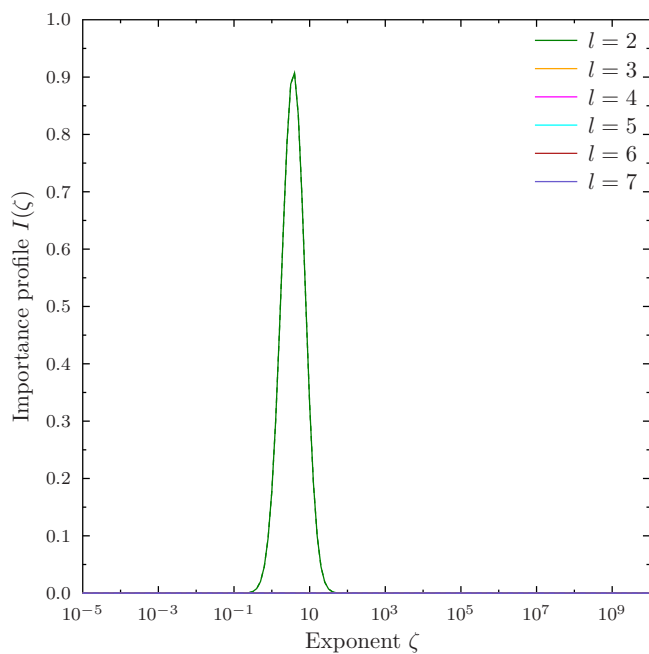

Figure 519. STO importance profile for  $\delta_-$  orbitals on Cu atom in  $\text{CuF}$ .

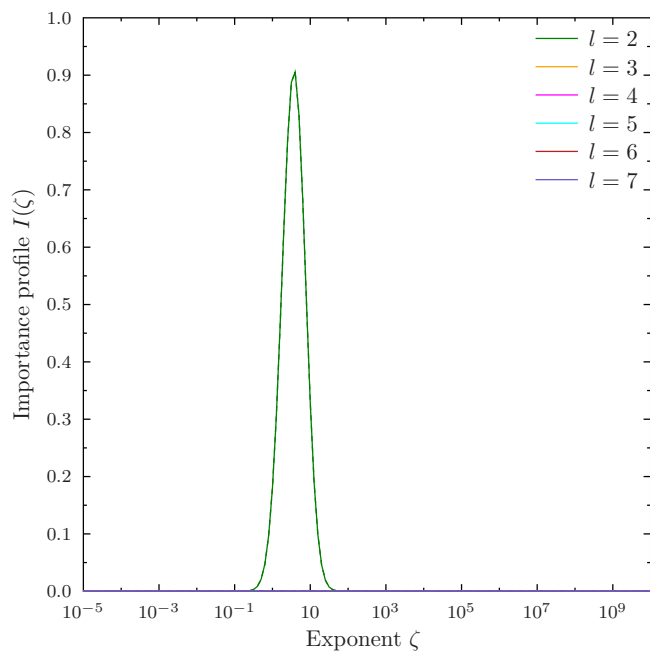

Figure 518. STO importance profile for  $\delta_-$  orbitals on Cu atom in  $\text{CuCl}$ .

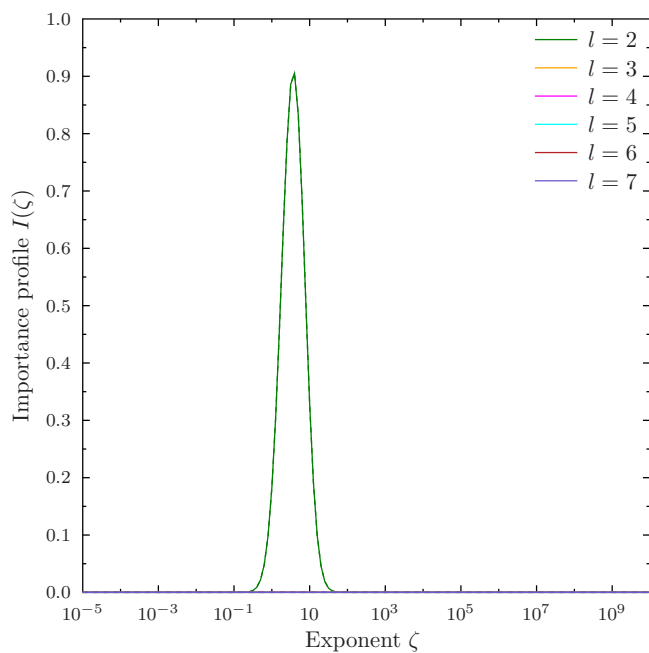

Figure 520. STO importance profile for  $\delta_-$  orbitals on Cu atom in  $\text{CuH}$ .

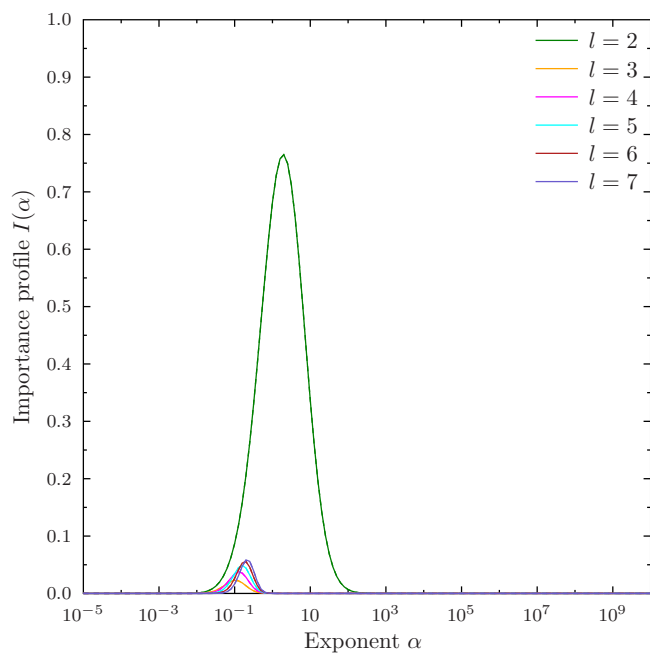

Figure 521. GTO importance profile for  $\delta_+$  orbitals on Cu atom in  $\text{Cu}_2$ .

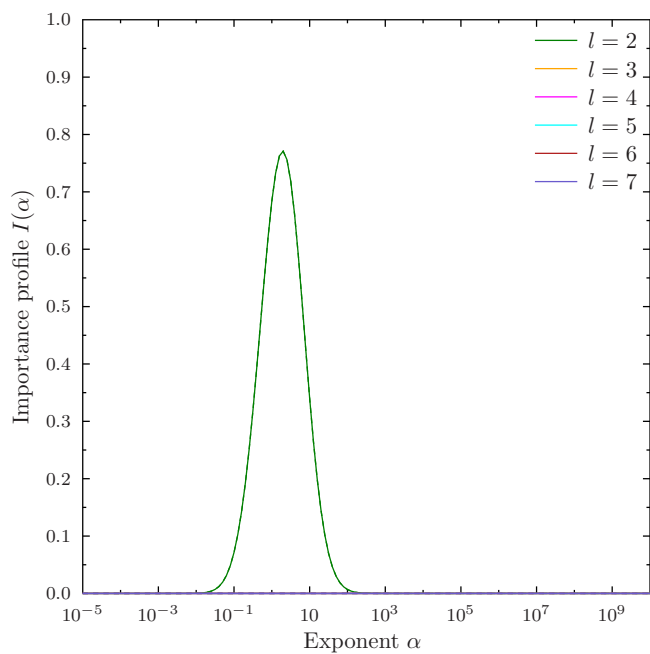

Figure 523. GTO importance profile for  $\delta_+$  orbitals on Cu atom in  $\text{CuF}$ .

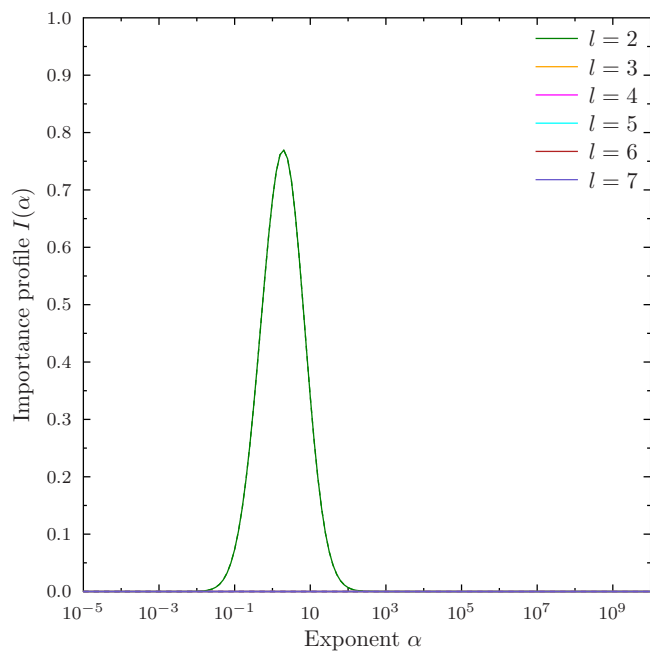

Figure 522. GTO importance profile for  $\delta_+$  orbitals on Cu atom in  $\text{CuCl}$ .

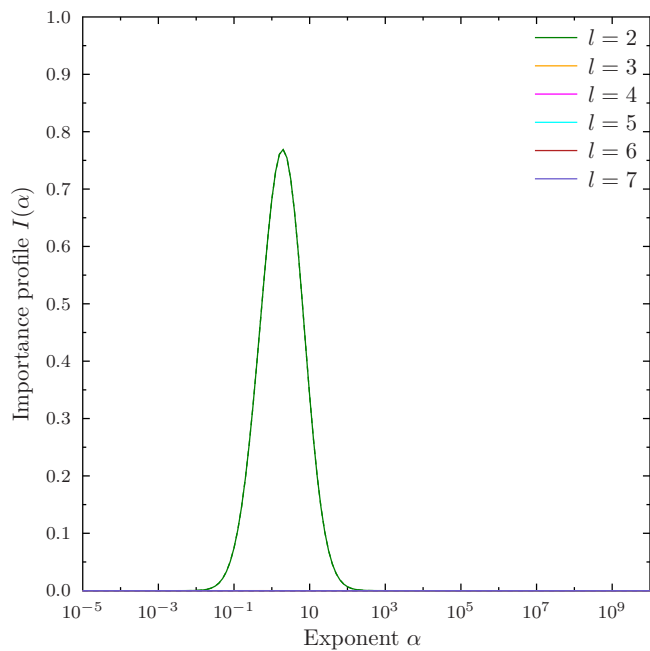

Figure 524. GTO importance profile for  $\delta_+$  orbitals on Cu atom in  $\text{CuH}$ .

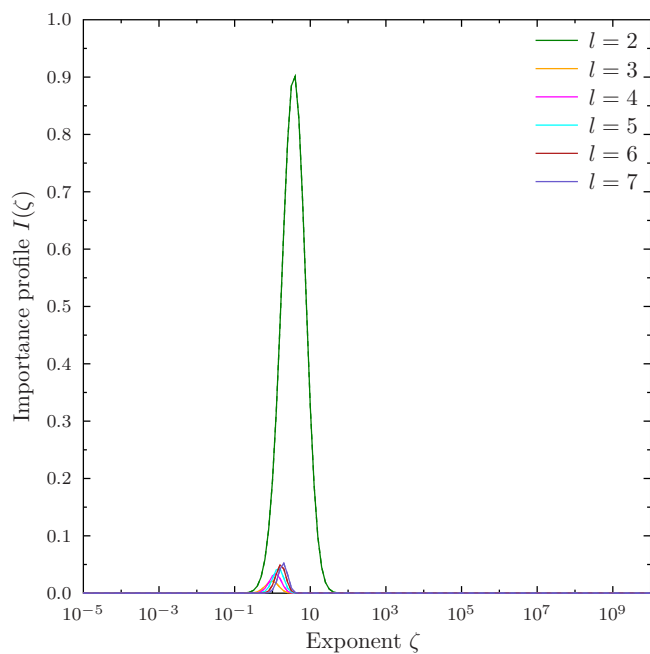

Figure 525. STO importance profile for  $\delta_+$  orbitals on Cu atom in  $\text{Cu}_2$ .

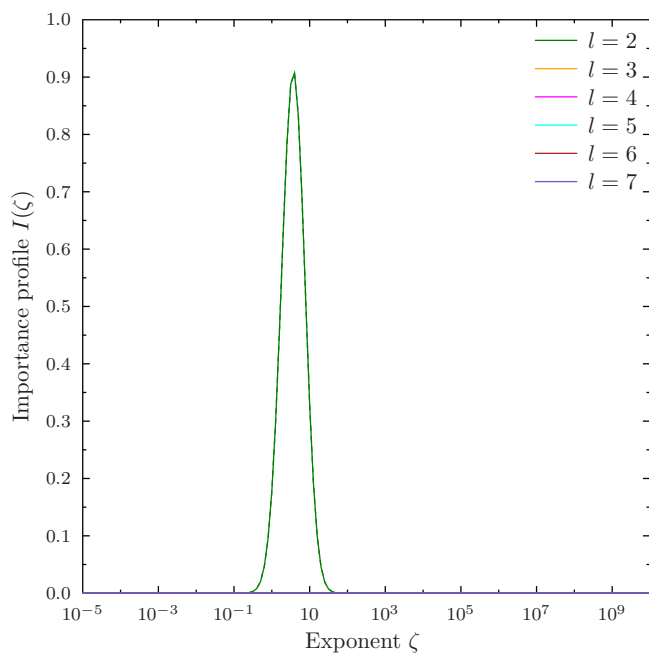

Figure 527. STO importance profile for  $\delta_+$  orbitals on Cu atom in  $\text{CuF}$ .

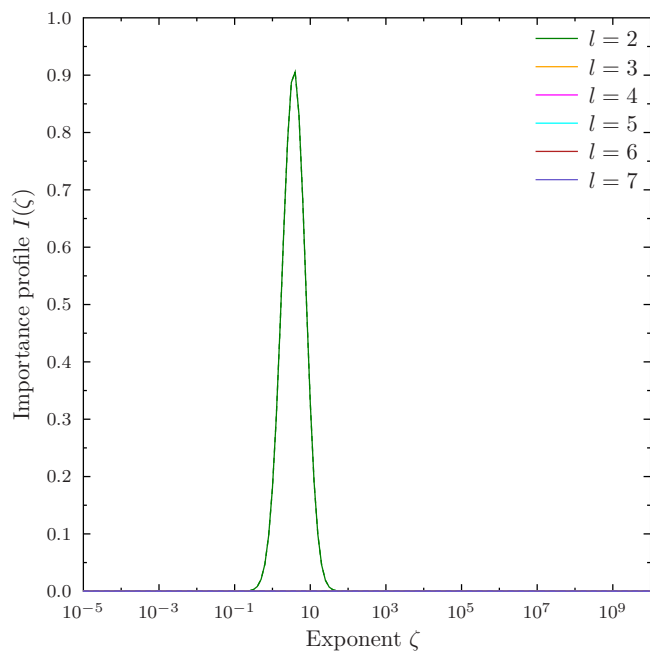

Figure 526. STO importance profile for  $\delta_+$  orbitals on Cu atom in  $\text{CuCl}$ .

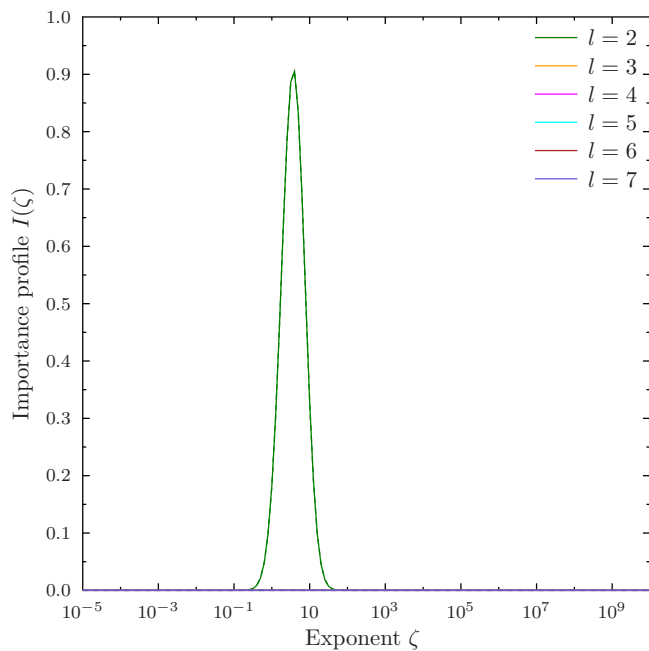

Figure 528. STO importance profile for  $\delta_+$  orbitals on Cu atom in  $\text{CuH}$ .



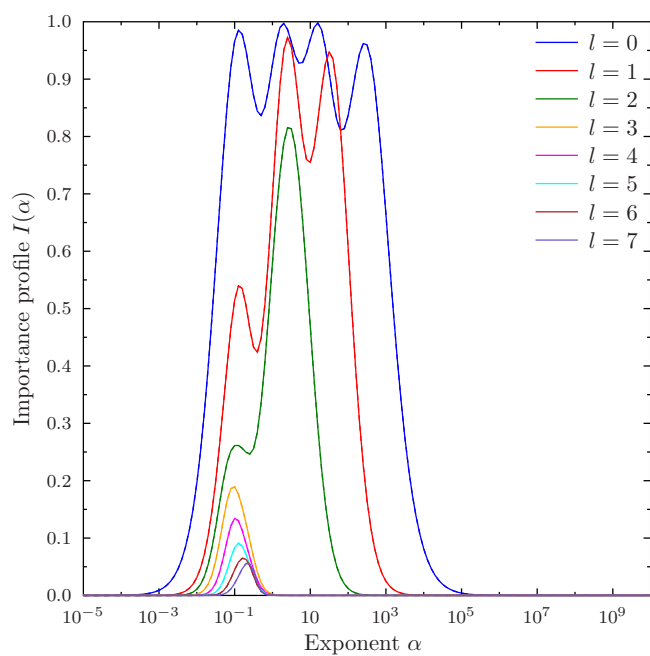

Figure 529. GTO importance profile for  $\sigma$  orbitals on Ga atom in GaCl.

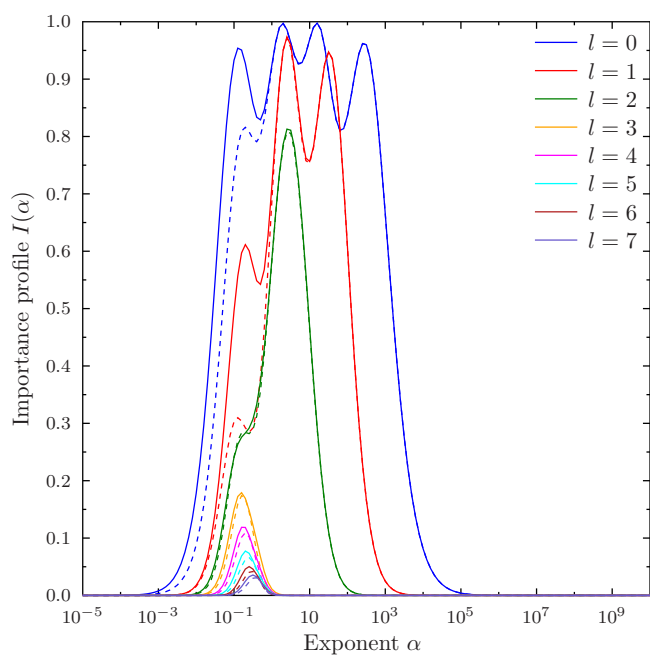

Figure 531. GTO importance profile for  $\sigma$  orbitals on Ga atom in GaO.

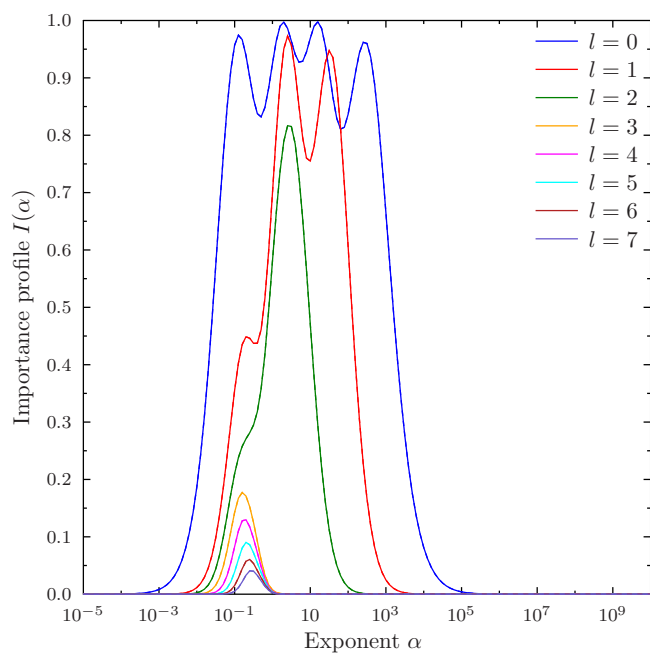

Figure 530. GTO importance profile for  $\sigma$  orbitals on Ga atom in GaF.

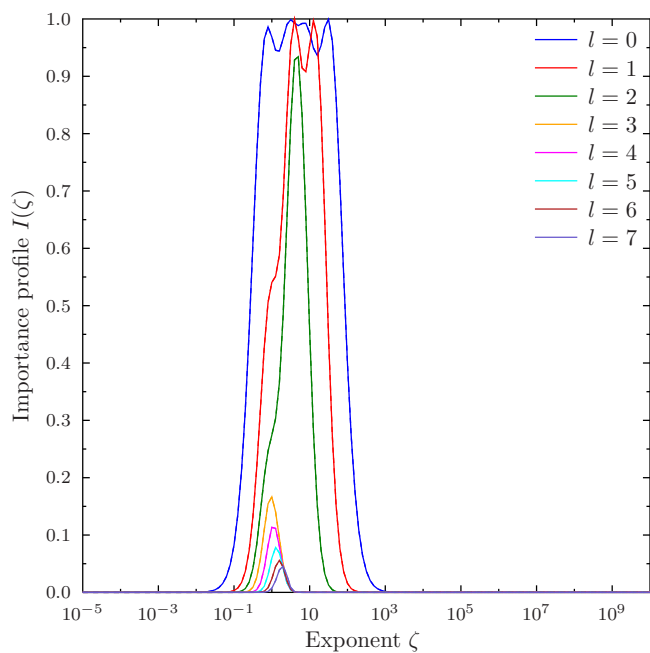

Figure 532. STO importance profile for  $\sigma$  orbitals on Ga atom in GaCl.

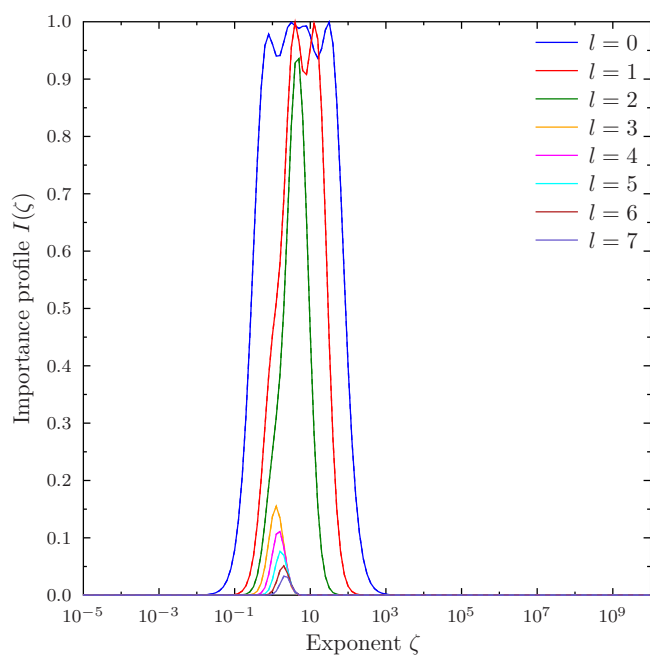

Figure 533. STO importance profile for  $\sigma$  orbitals on Ga atom in GaF.

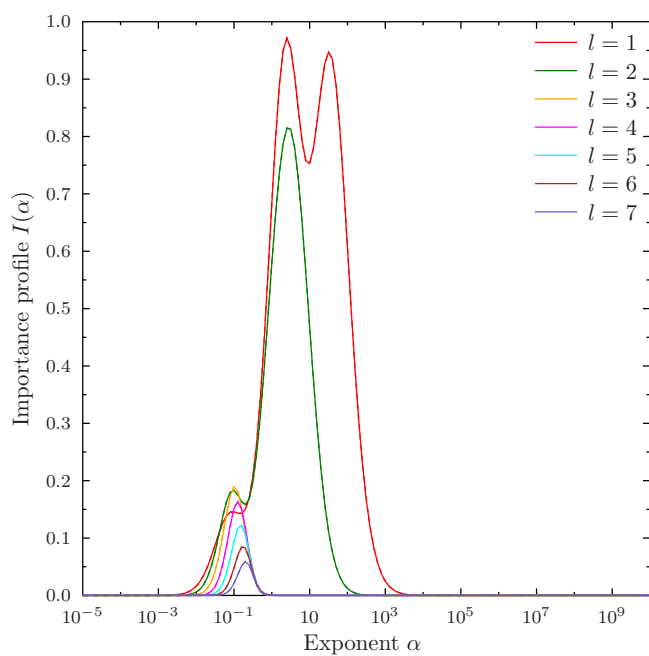

Figure 535. GTO importance profile for  $\pi_-$  orbitals on Ga atom in GaCl.

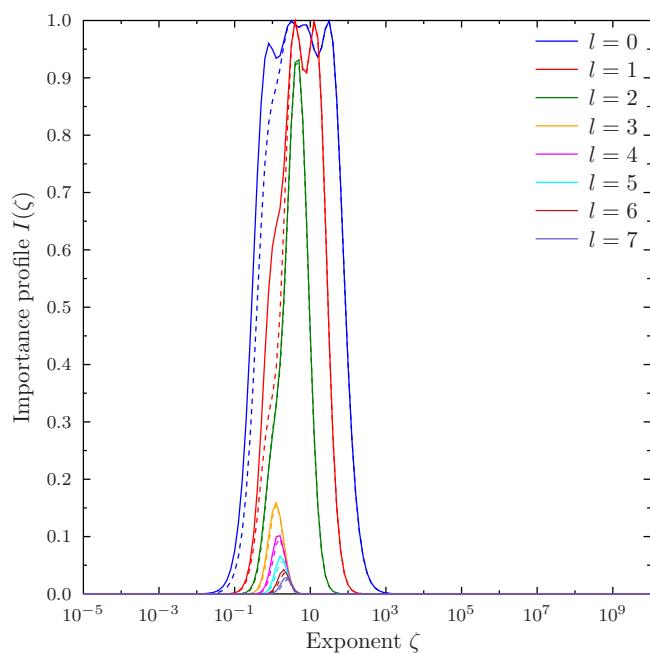

Figure 534. STO importance profile for  $\sigma$  orbitals on Ga atom in GaO.

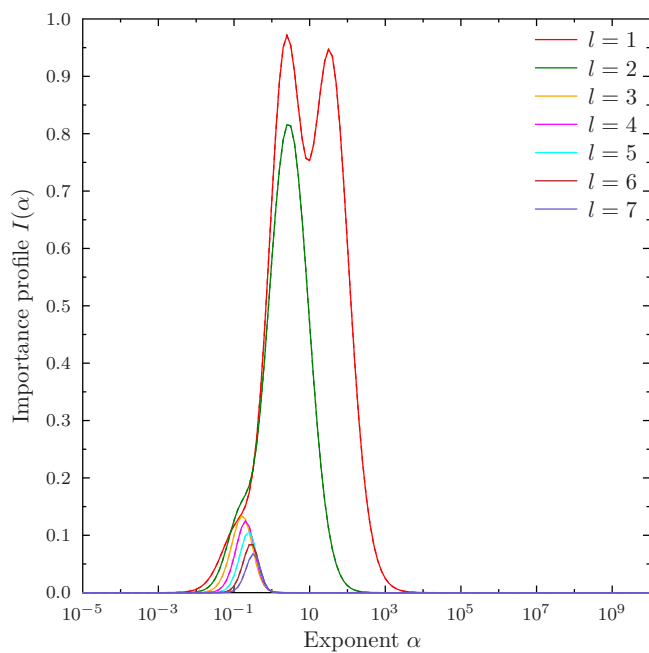

Figure 536. GTO importance profile for  $\pi_-$  orbitals on Ga atom in GaF.

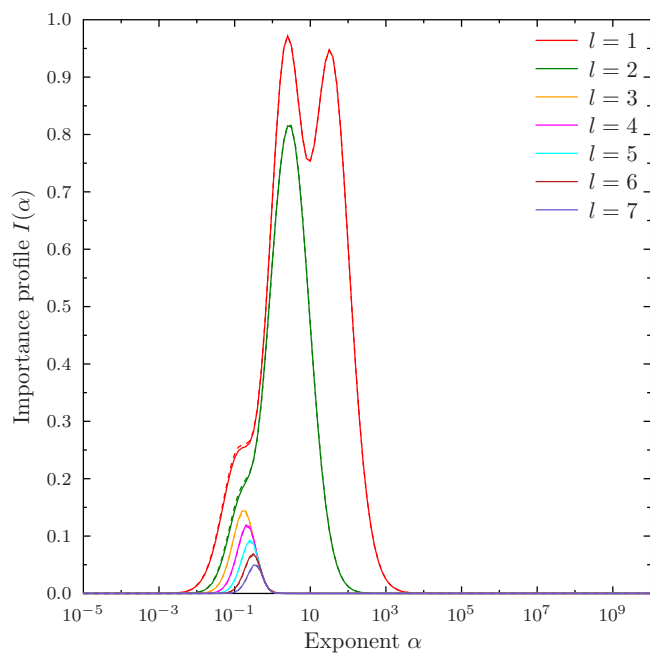

Figure 537. GTO importance profile for  $\pi_-$  orbitals on Ga atom in GaO.

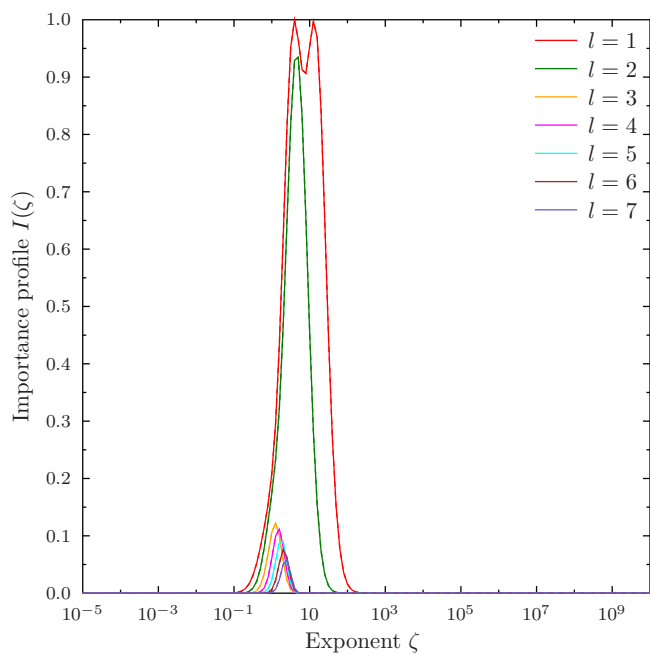

Figure 539. STO importance profile for  $\pi_-$  orbitals on Ga atom in GaF.

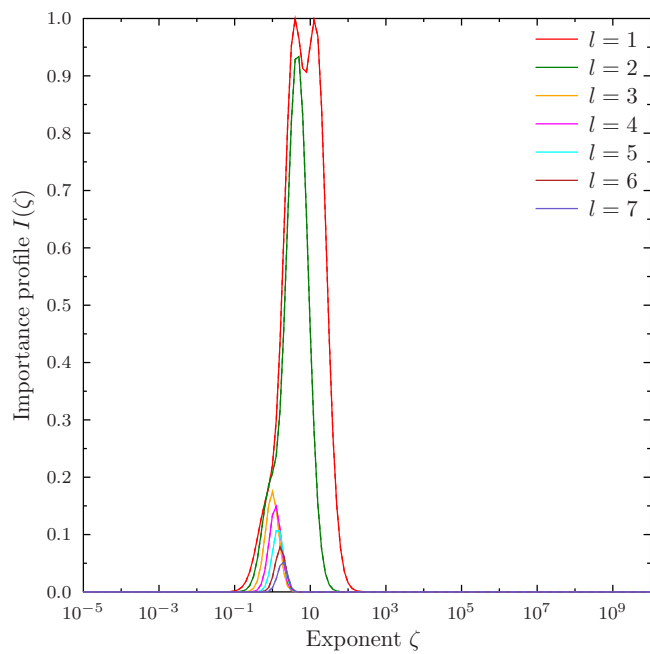

Figure 538. STO importance profile for  $\pi_-$  orbitals on Ga atom in GaCl.

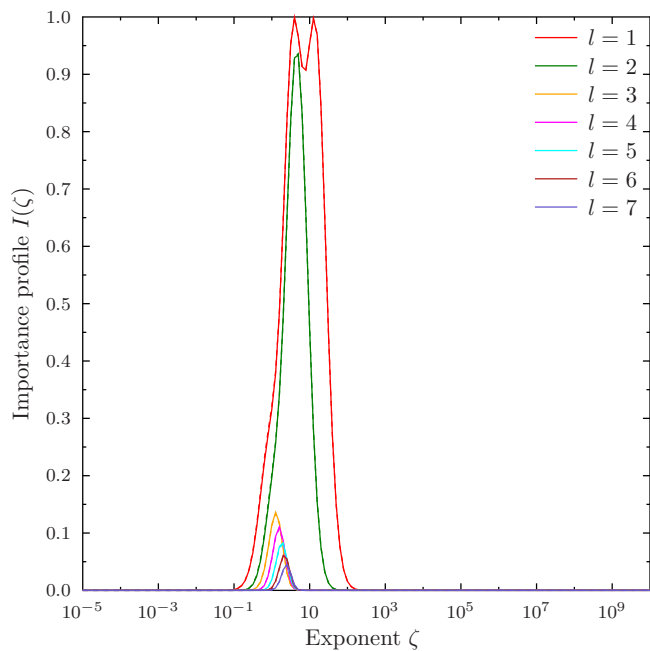

Figure 540. STO importance profile for  $\pi_-$  orbitals on Ga atom in GaO.

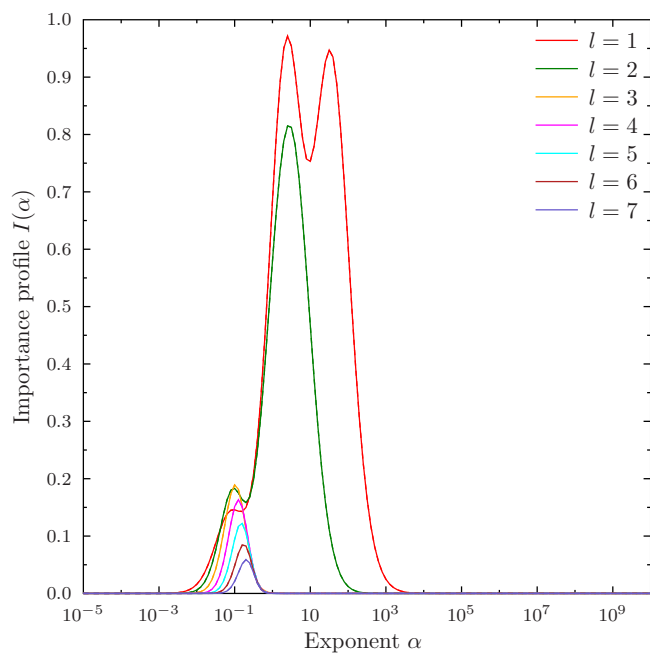

Figure 541. GTO importance profile for  $\pi_+$  orbitals on Ga atom in GaCl.

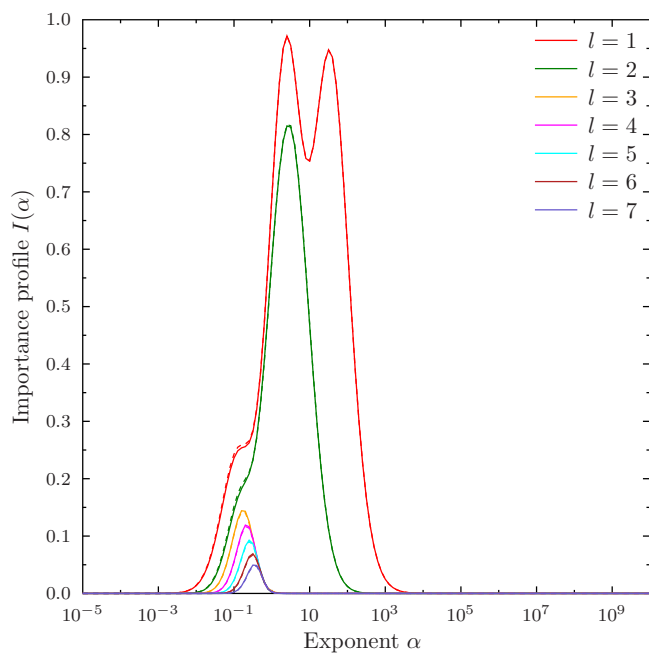

Figure 543. GTO importance profile for  $\pi_+$  orbitals on Ga atom in GaO.

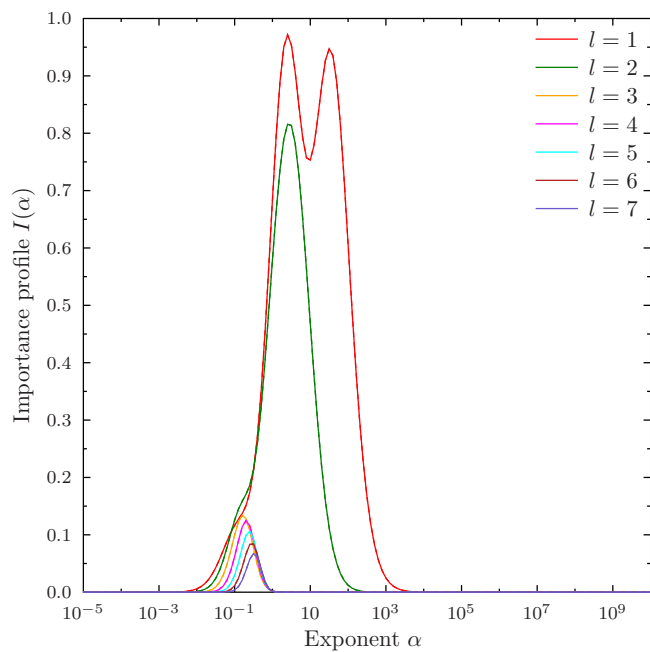

Figure 542. GTO importance profile for  $\pi_+$  orbitals on Ga atom in GaF.

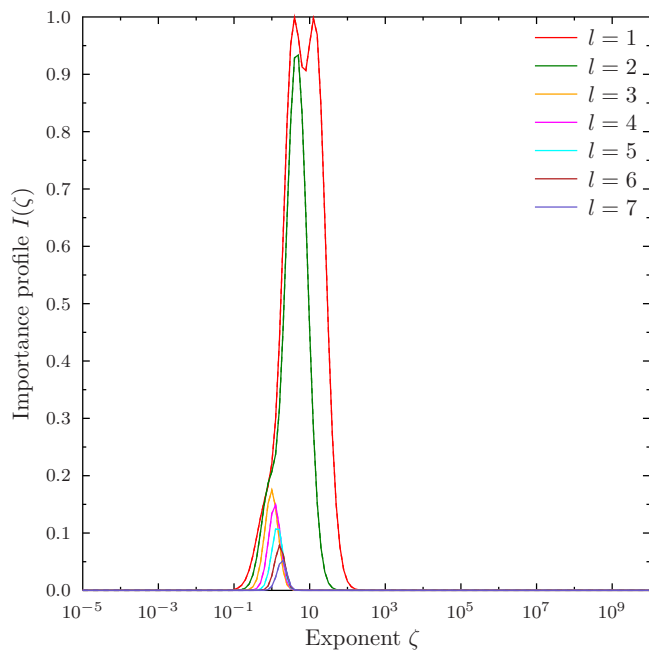

Figure 544. STO importance profile for  $\pi_+$  orbitals on Ga atom in GaCl.

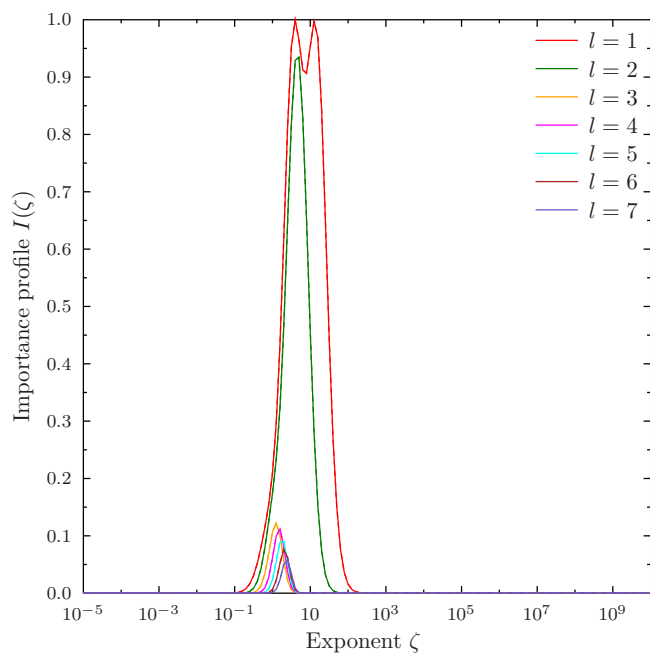

Figure 545. STO importance profile for  $\pi_+$  orbitals on Ga atom in GaF.

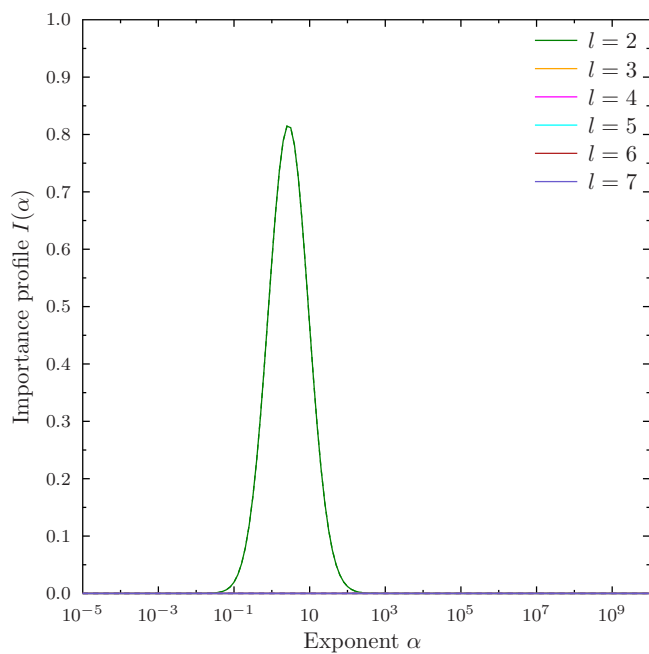

Figure 547. GTO importance profile for  $\delta_-$  orbitals on Ga atom in GaCl.

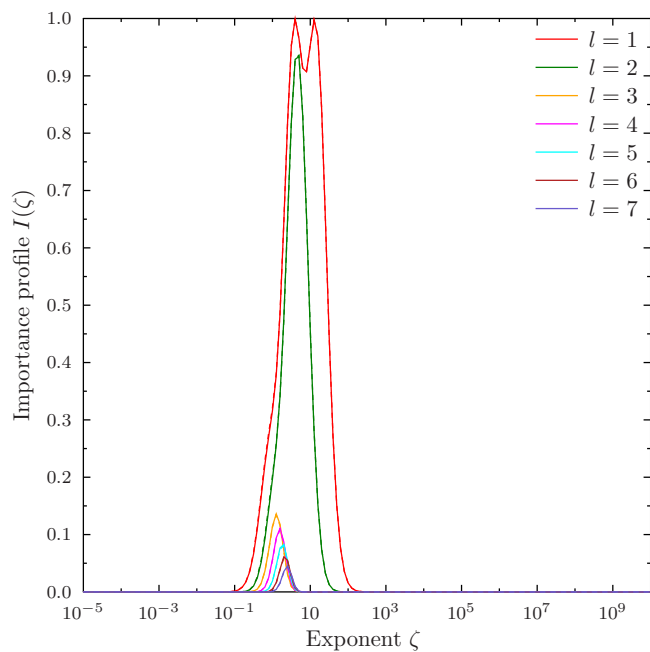

Figure 546. STO importance profile for  $\pi_+$  orbitals on Ga atom in GaO.

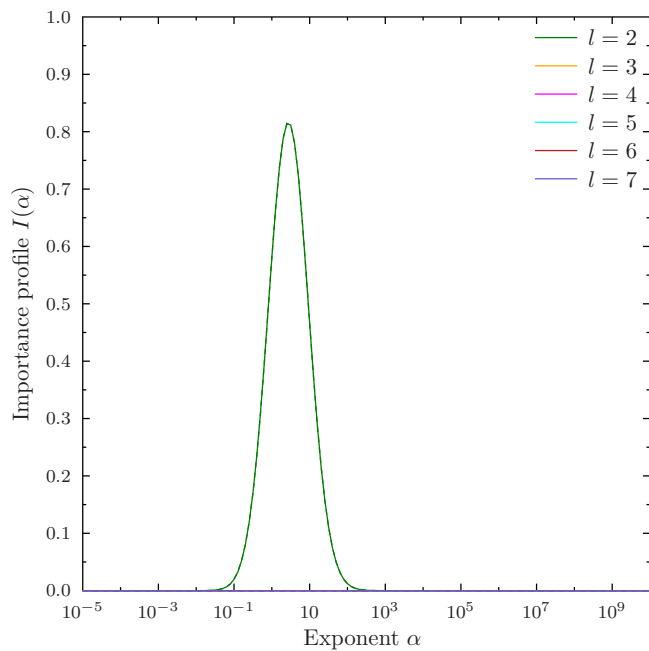

Figure 548. GTO importance profile for  $\delta_-$  orbitals on Ga atom in GaF.

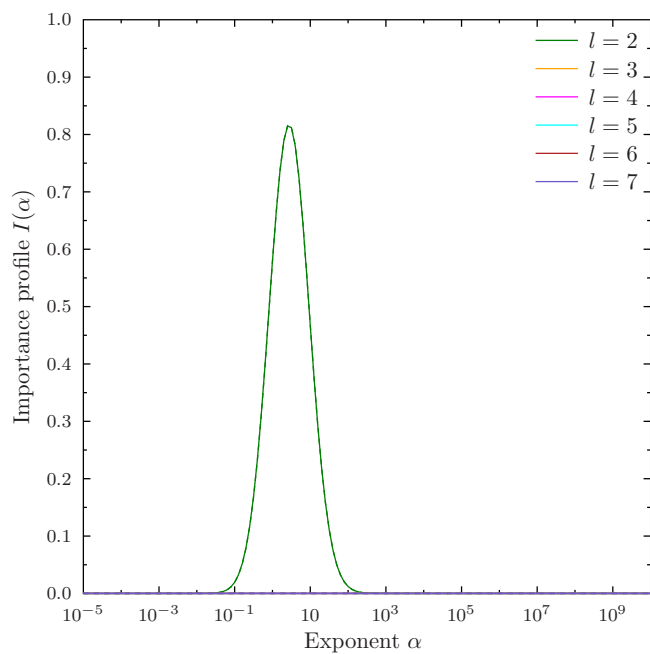

Figure 549. GTO importance profile for  $\delta_-$  orbitals on Ga atom in GaO.

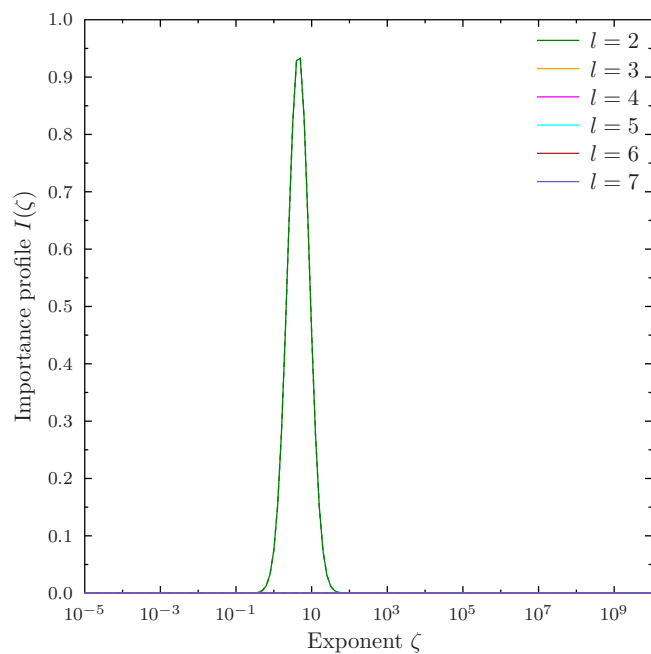

Figure 551. STO importance profile for  $\delta_-$  orbitals on Ga atom in GaF.

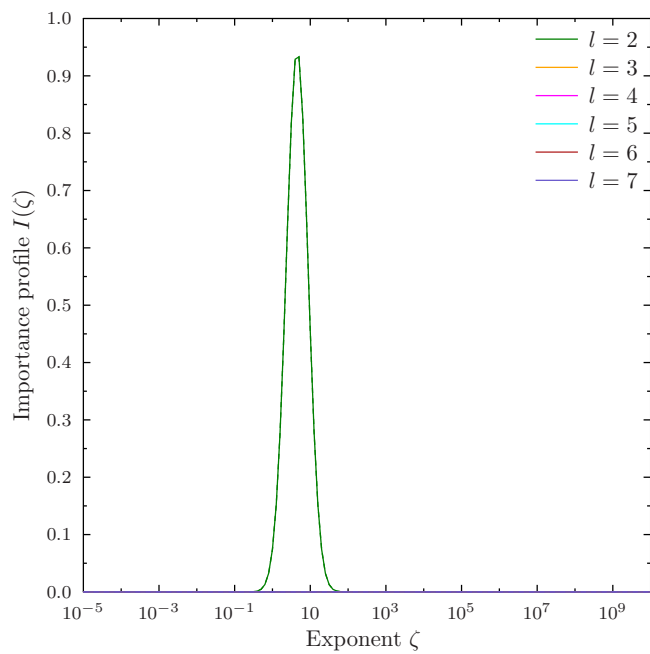

Figure 550. STO importance profile for  $\delta_-$  orbitals on Ga atom in GaCl.

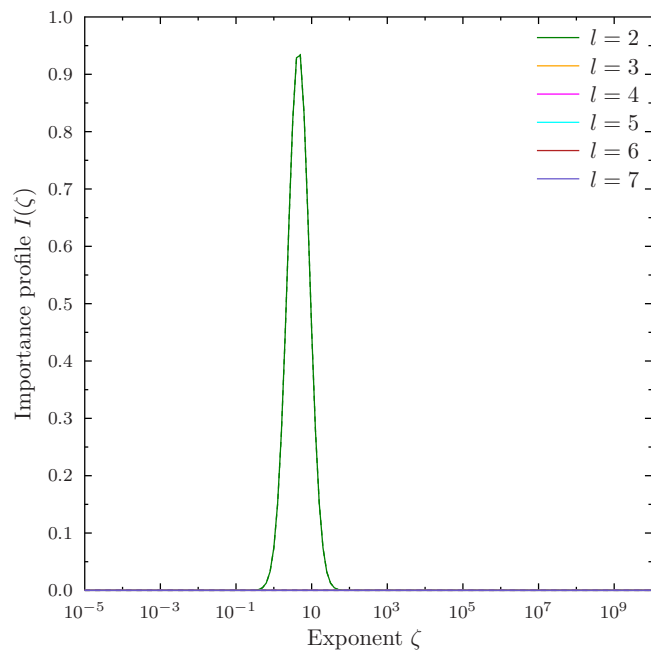

Figure 552. STO importance profile for  $\delta_-$  orbitals on Ga atom in GaO.

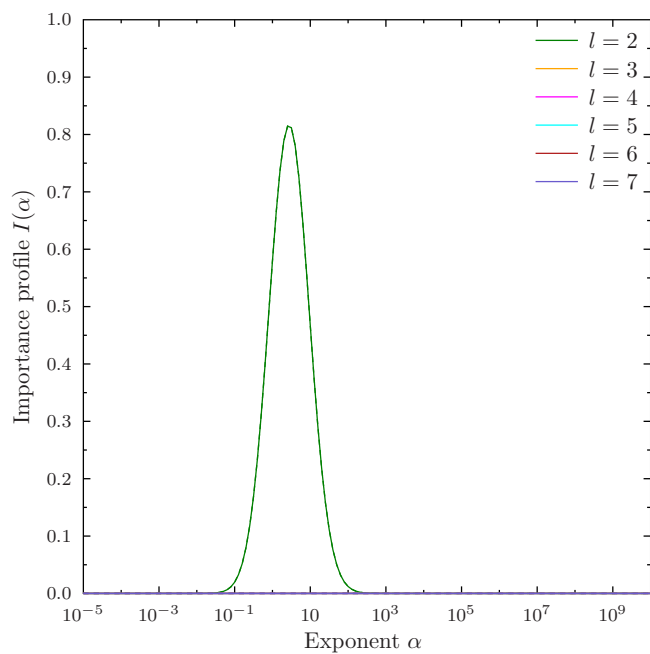

Figure 553. GTO importance profile for  $\delta_+$  orbitals on Ga atom in GaCl.

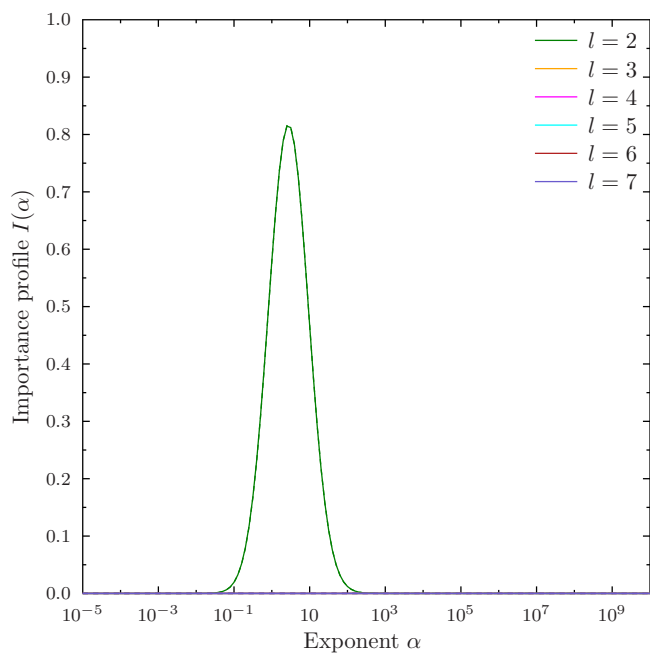

Figure 555. GTO importance profile for  $\delta_+$  orbitals on Ga atom in GaO.

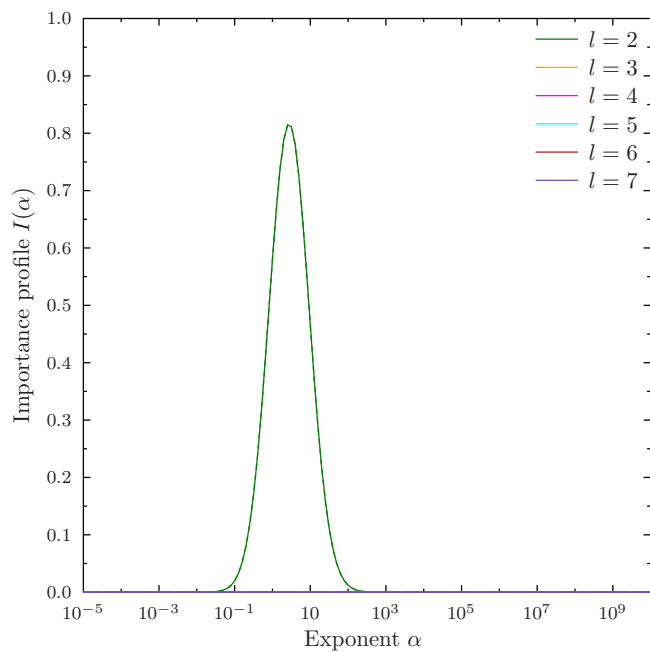

Figure 554. GTO importance profile for  $\delta_+$  orbitals on Ga atom in GaF.

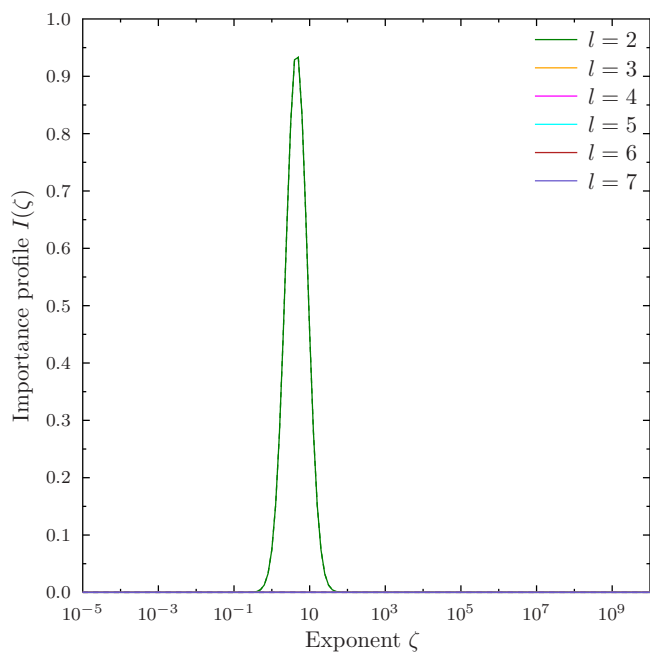

Figure 556. STO importance profile for  $\delta_+$  orbitals on Ga atom in GaCl.

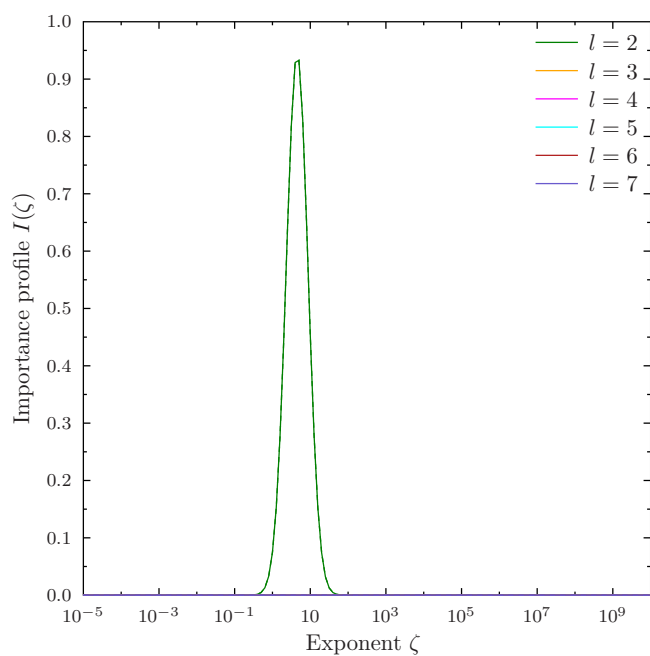

Figure 557. STO importance profile for  $\delta_+$  orbitals on Ga atom in GaF.

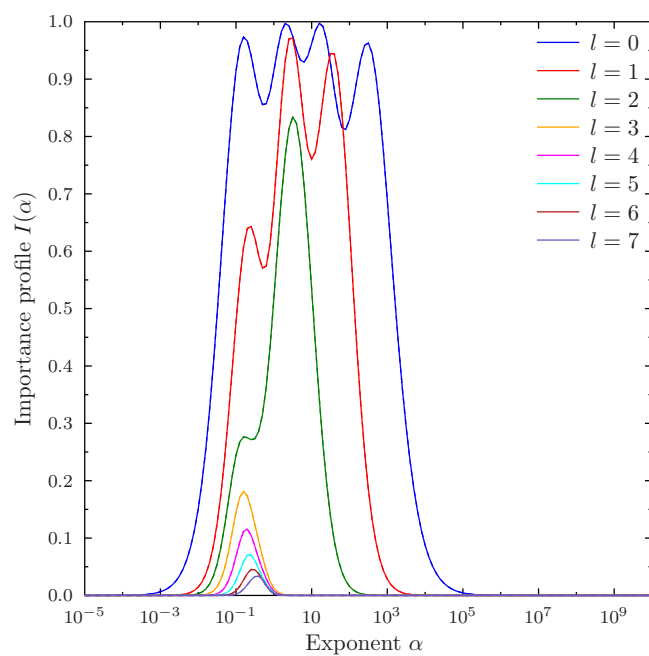

Figure 559. GTO importance profile for  $\sigma$  orbitals on Ge atom in GeO.

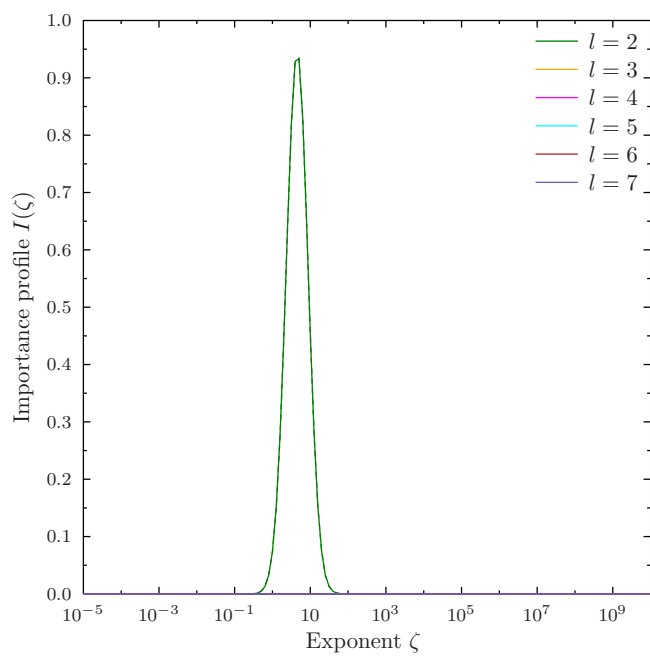

Figure 558. STO importance profile for  $\delta_+$  orbitals on Ga atom in GaO.

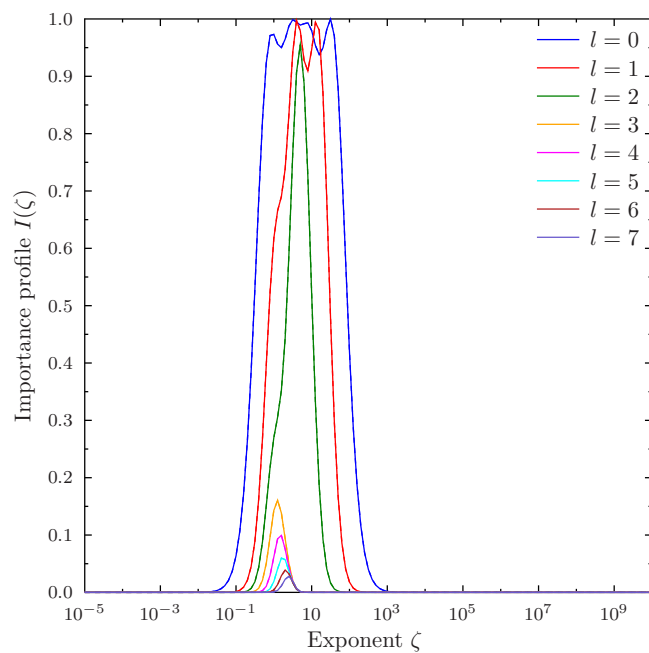

Figure 560. STO importance profile for  $\sigma$  orbitals on Ge atom in GeO.



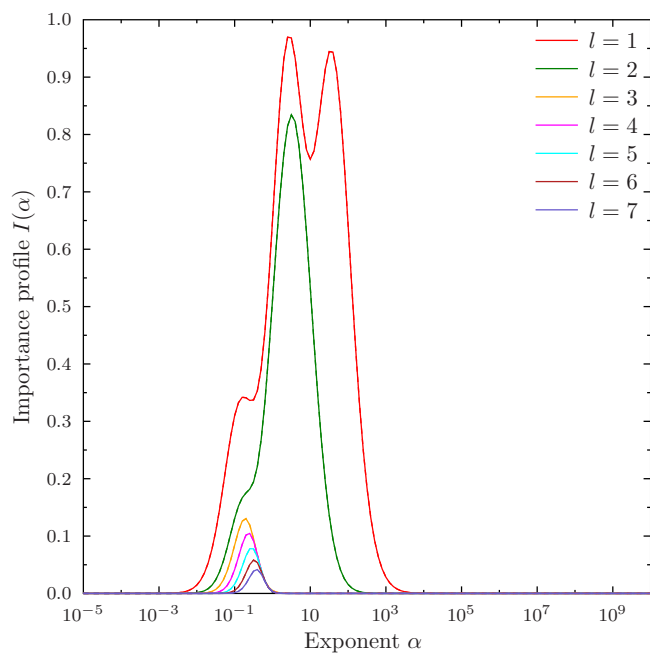

Figure 561. GTO importance profile for  $\pi_-$  orbitals on Ge atom in GeO.

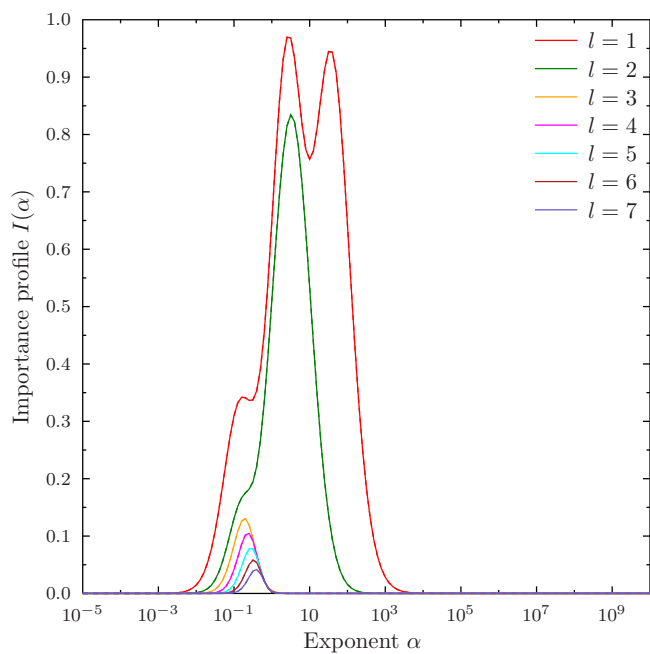

Figure 563. GTO importance profile for  $\pi_+$  orbitals on Ge atom in GeO.

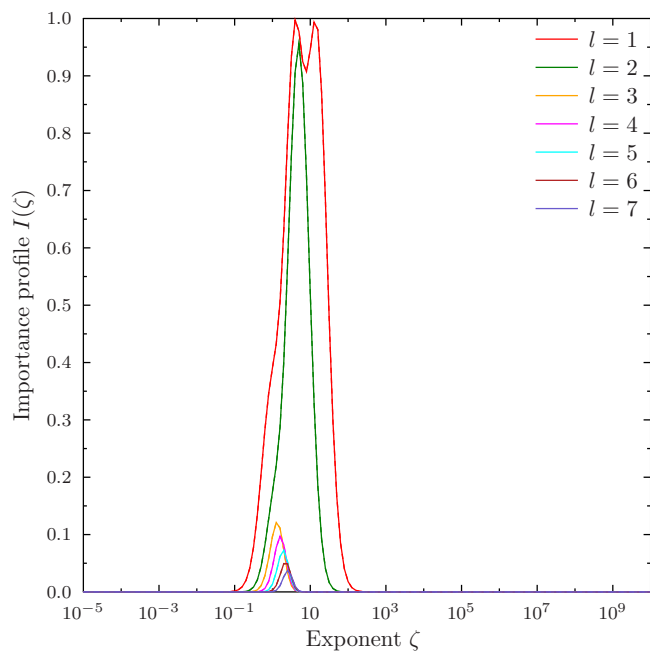

Figure 562. STO importance profile for  $\pi_-$  orbitals on Ge atom in GeO.

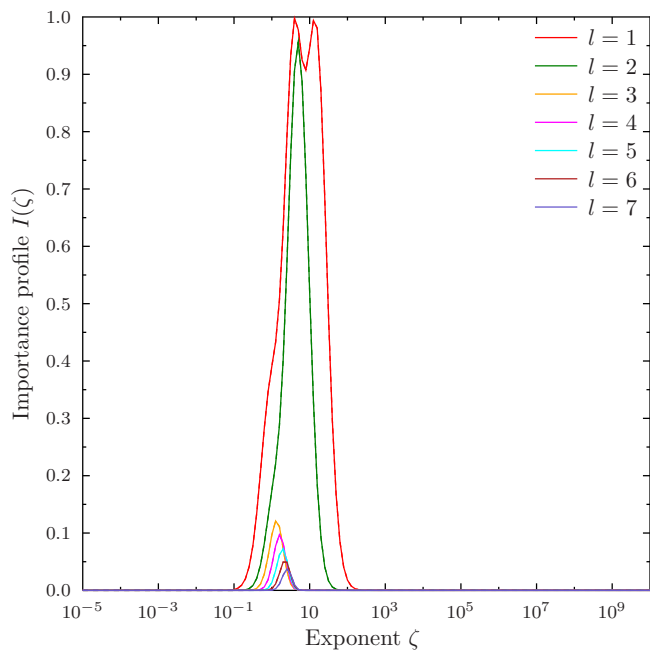

Figure 564. STO importance profile for  $\pi_+$  orbitals on Ge atom in GeO.

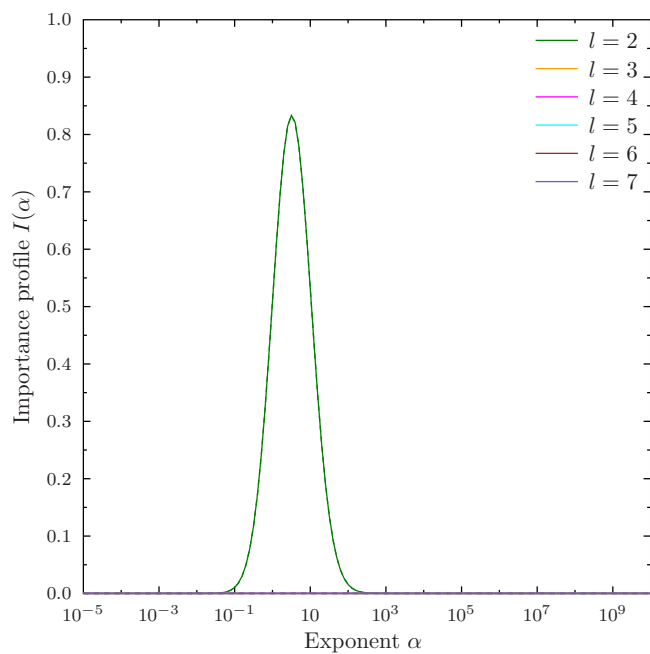

Figure 565. GTO importance profile for  $\delta_-$  orbitals on Ge atom in GeO.

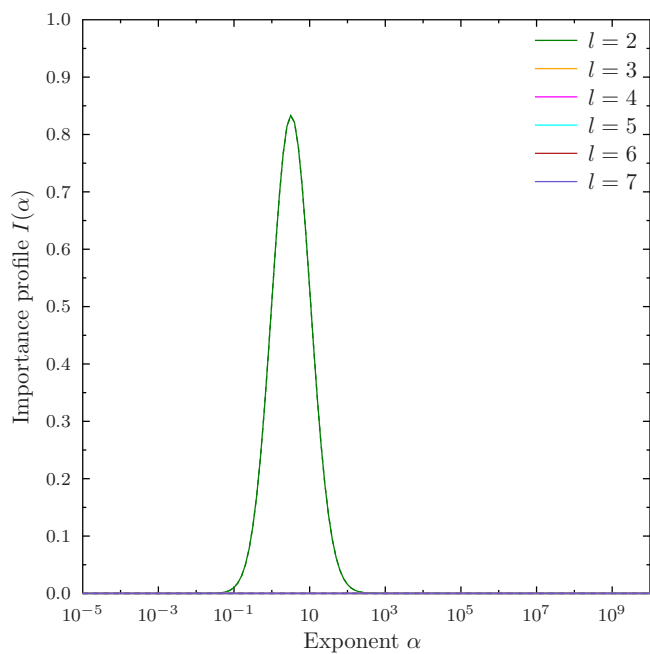

Figure 567. GTO importance profile for  $\delta_+$  orbitals on Ge atom in GeO.

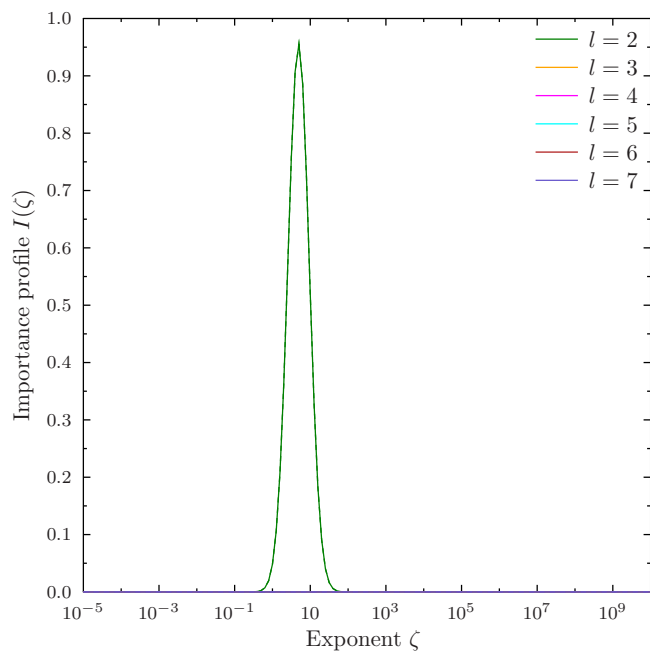

Figure 566. STO importance profile for  $\delta_-$  orbitals on Ge atom in GeO.

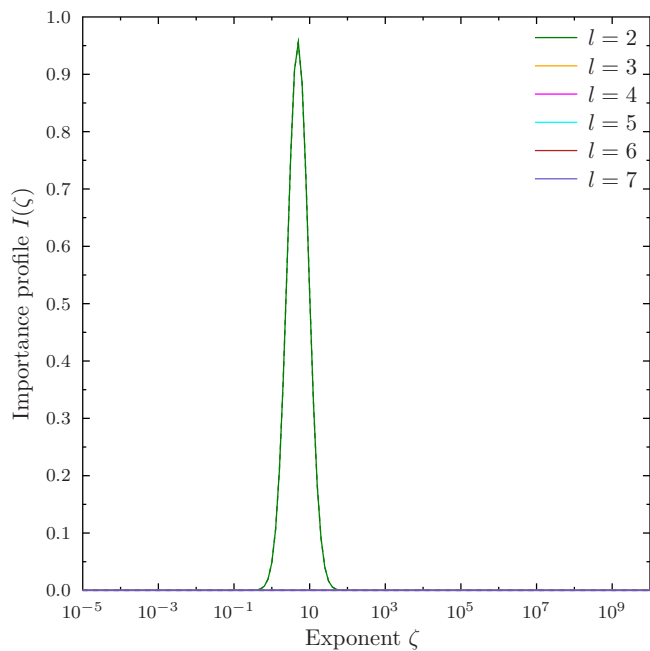

Figure 568. STO importance profile for  $\delta_+$  orbitals on Ge atom in GeO.

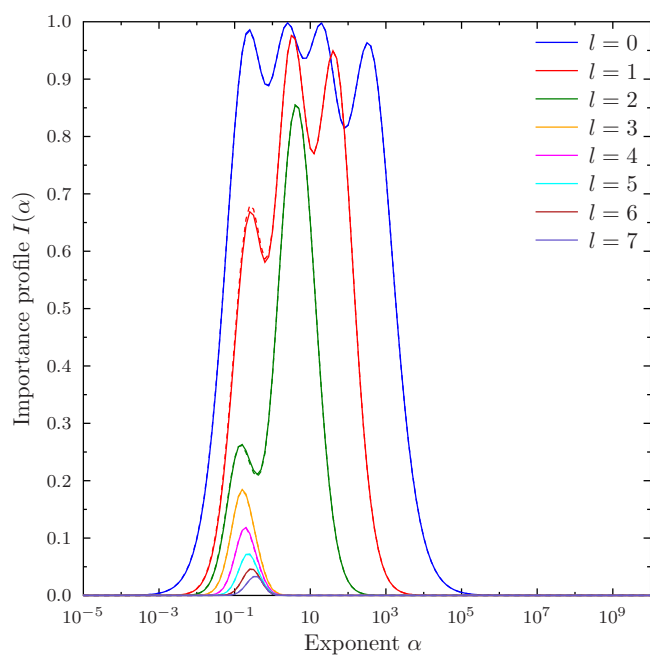

Figure 569. GTO importance profile for  $\sigma$  orbitals on Se atom in SeO.

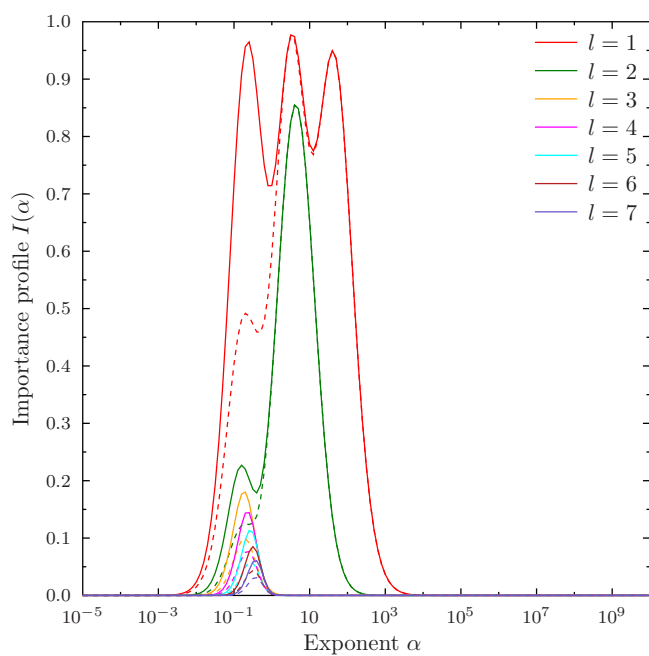

Figure 571. GTO importance profile for  $\pi_-$  orbitals on Se atom in SeO.

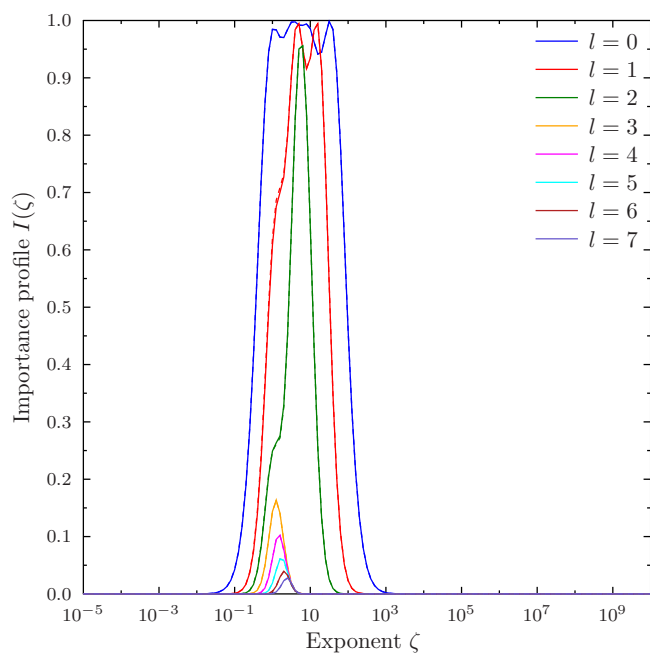

Figure 570. STO importance profile for  $\sigma$  orbitals on Se atom in SeO.

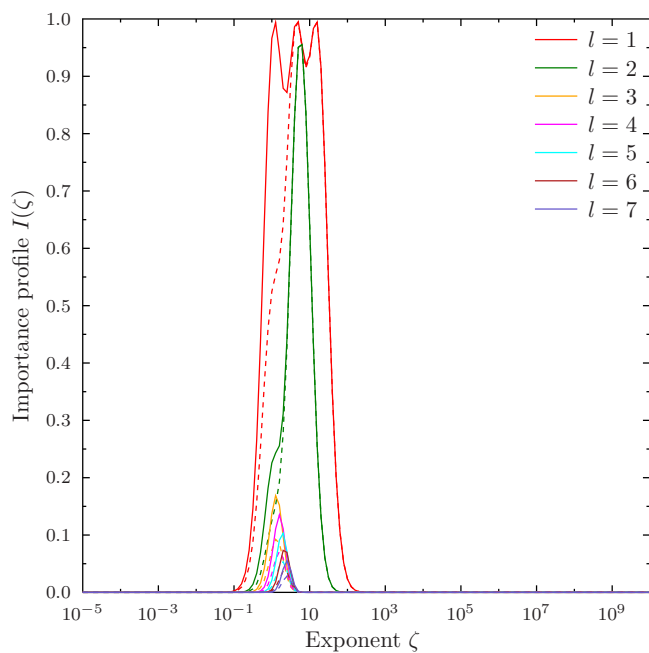

Figure 572. STO importance profile for  $\pi_-$  orbitals on Se atom in SeO.

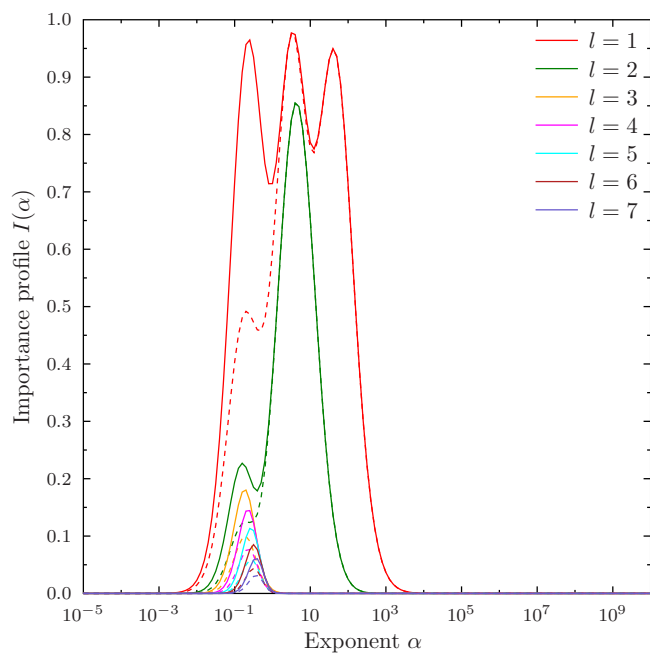

Figure 573. GTO importance profile for  $\pi_+$  orbitals on Se atom in SeO.

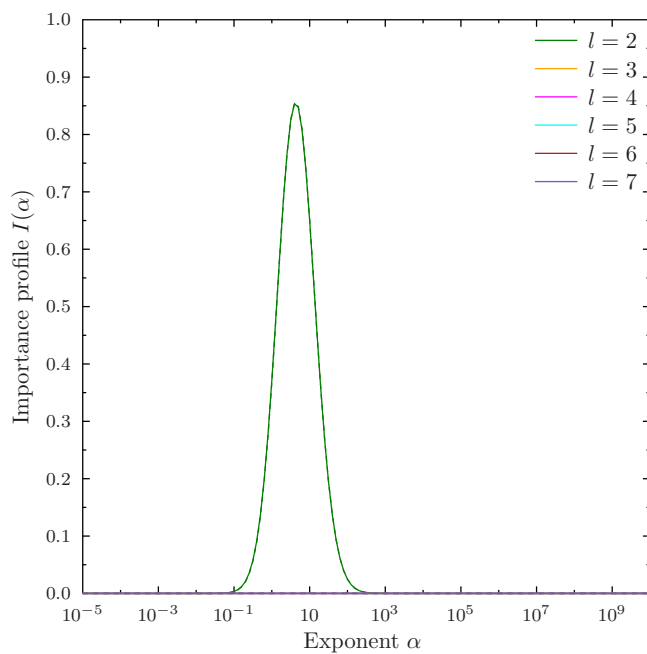

Figure 575. GTO importance profile for  $\delta_-$  orbitals on Se atom in SeO.

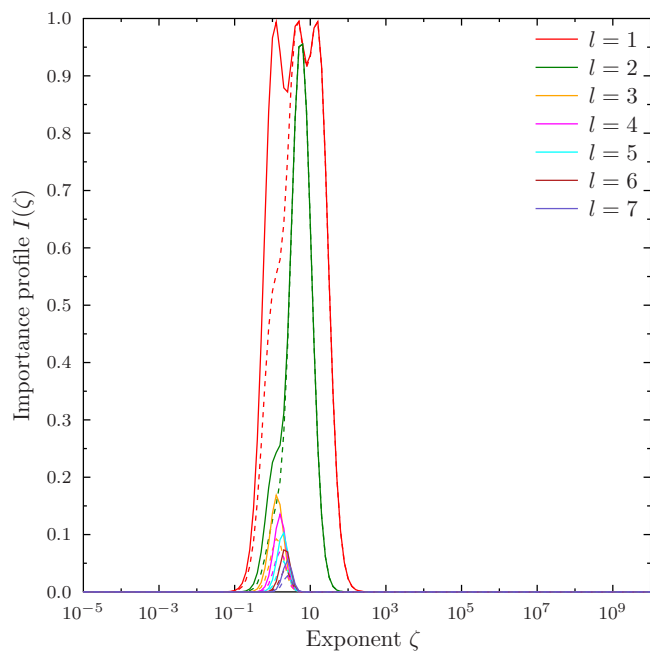

Figure 574. STO importance profile for  $\pi_+$  orbitals on Se atom in SeO.

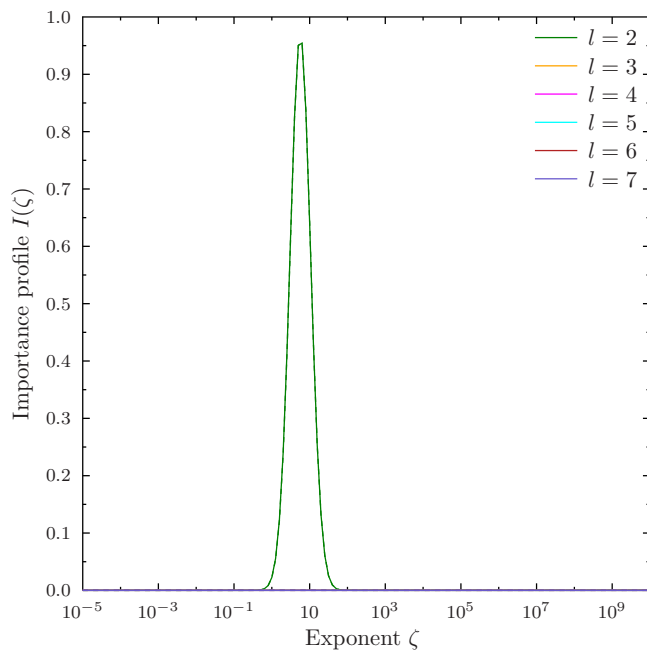

Figure 576. STO importance profile for  $\delta_-$  orbitals on Se atom in SeO.

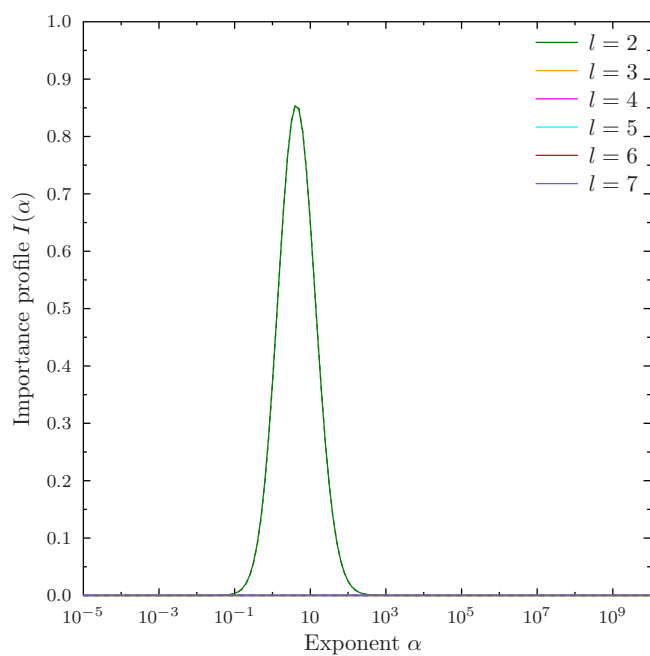

Figure 577. GTO importance profile for  $\delta_+$  orbitals on Se atom in SeO.

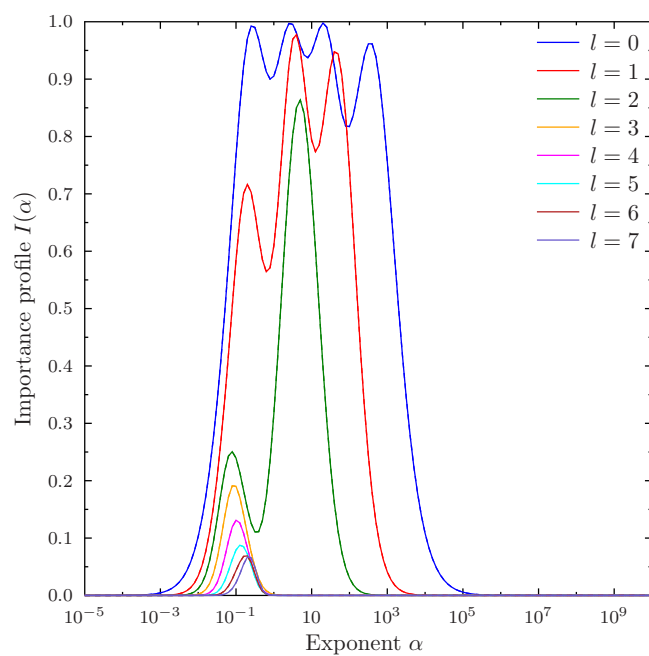

Figure 579. GTO importance profile for  $\sigma$  orbitals on Br atom in  $\text{Br}_2$ .

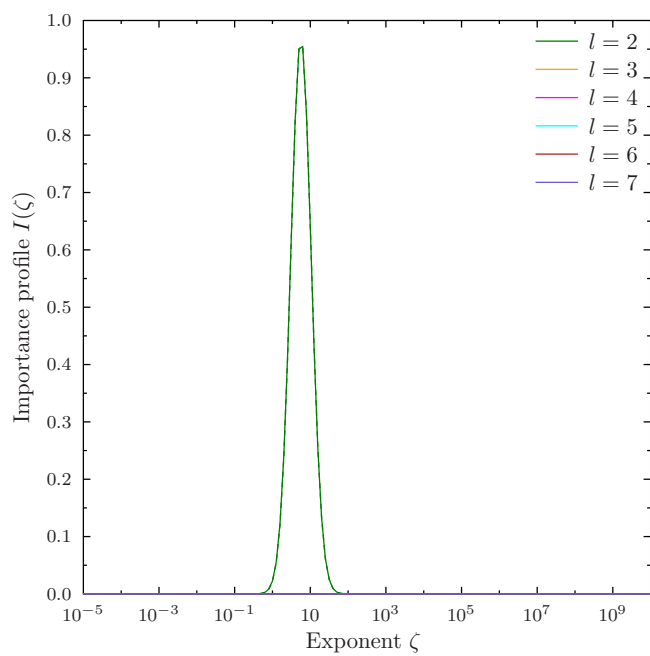

Figure 578. STO importance profile for  $\delta_+$  orbitals on Se atom in SeO.

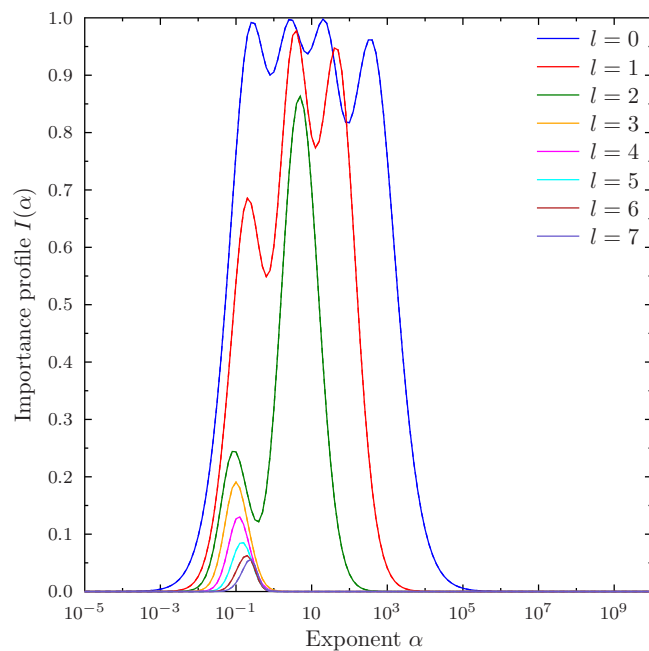

Figure 580. GTO importance profile for  $\sigma$  orbitals on Br atom in  $\text{BrCl}$ .

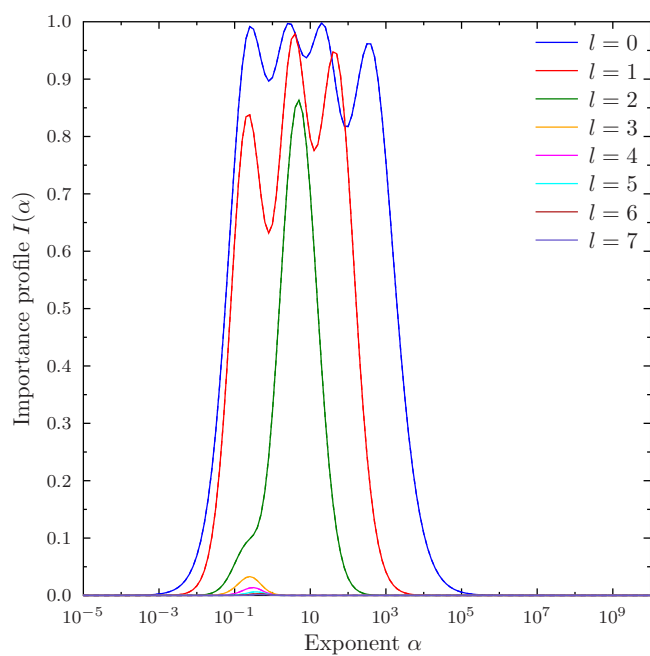

Figure 581. GTO importance profile for  $\sigma$  orbitals on Br atom in HBr.

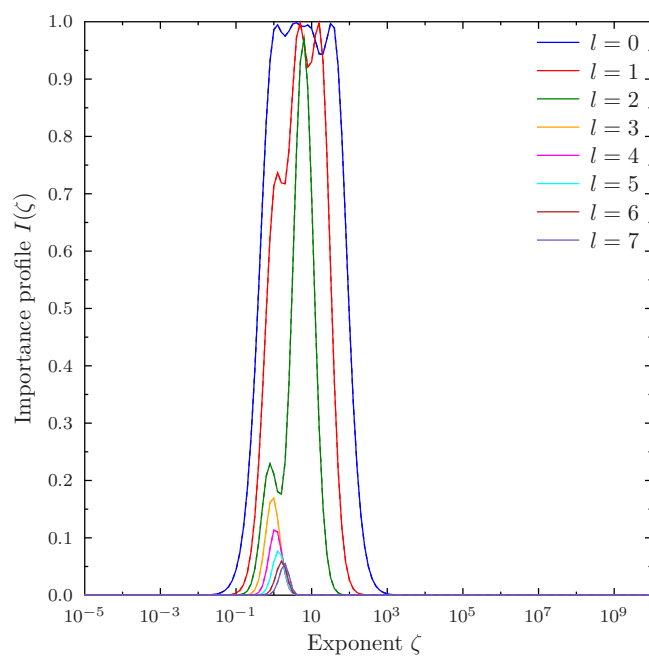

Figure 583. STO importance profile for  $\sigma$  orbitals on Br atom in  $\text{Br}_2$ .

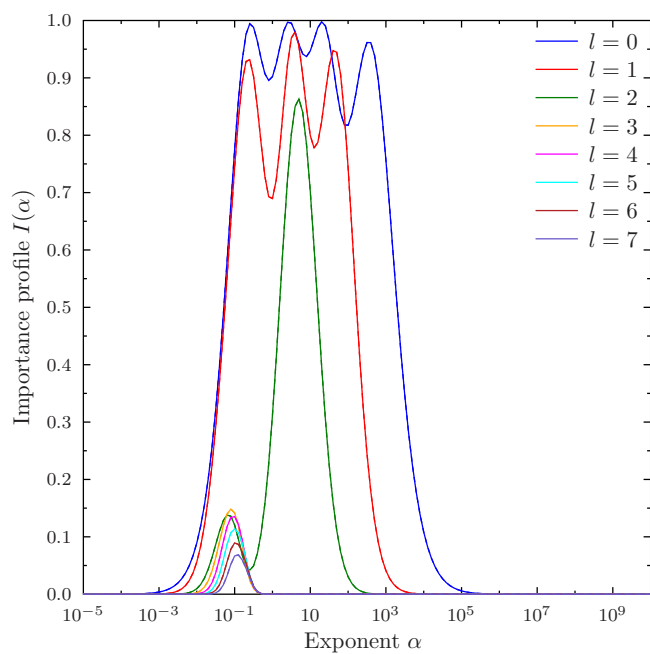

Figure 582. GTO importance profile for  $\sigma$  orbitals on Br atom in KBr.

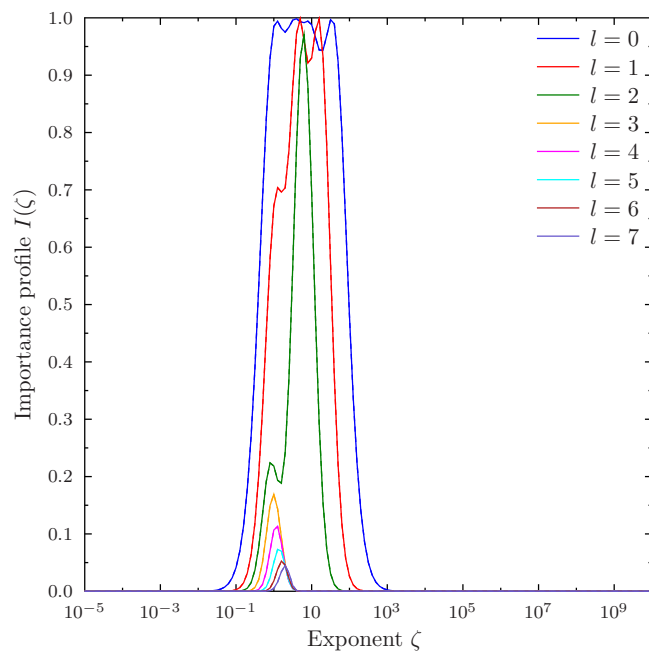

Figure 584. STO importance profile for  $\sigma$  orbitals on Br atom in BrCl.

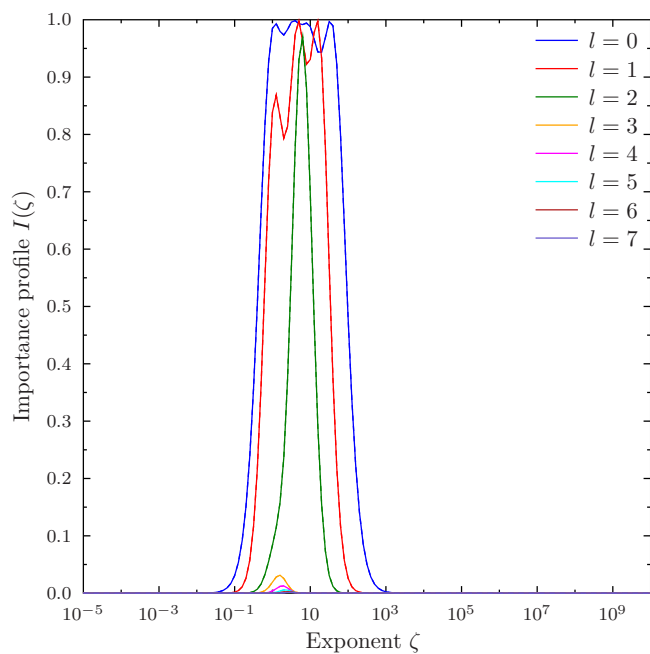

Figure 585. STO importance profile for  $\sigma$  orbitals on Br atom in HBr.

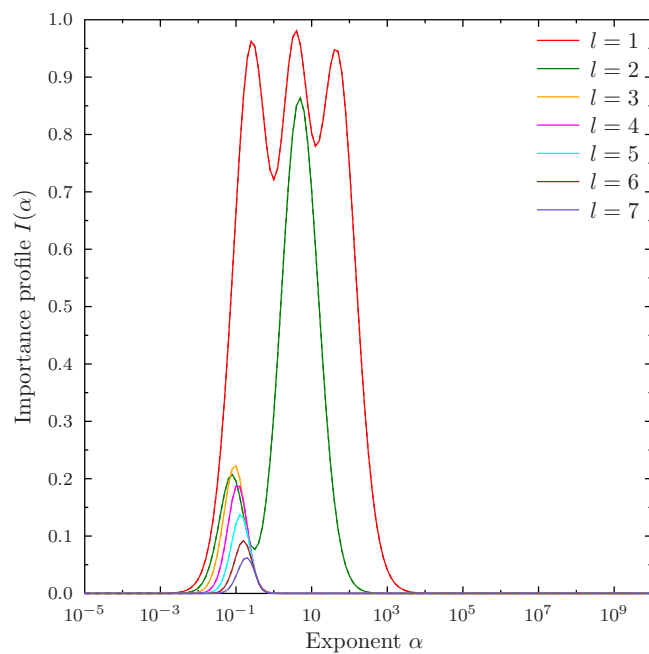

Figure 587. GTO importance profile for  $\pi_-$  orbitals on Br atom in  $\text{Br}_2$ .

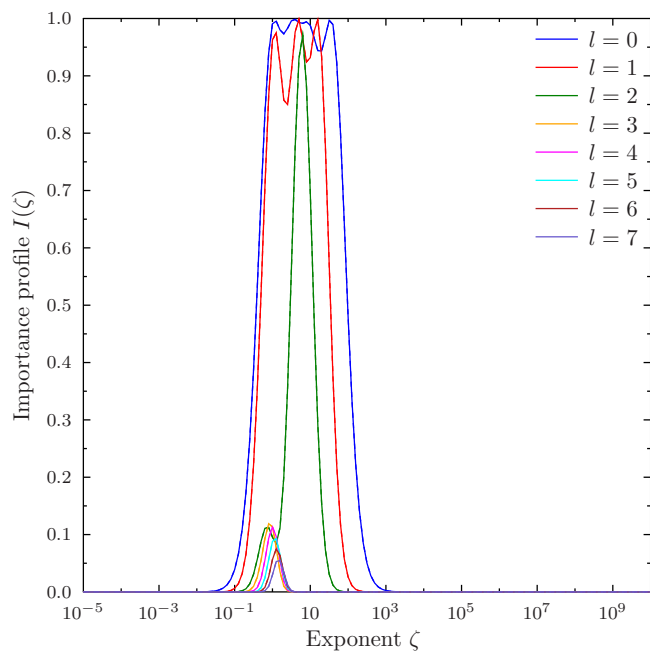

Figure 586. STO importance profile for  $\sigma$  orbitals on Br atom in KBr.

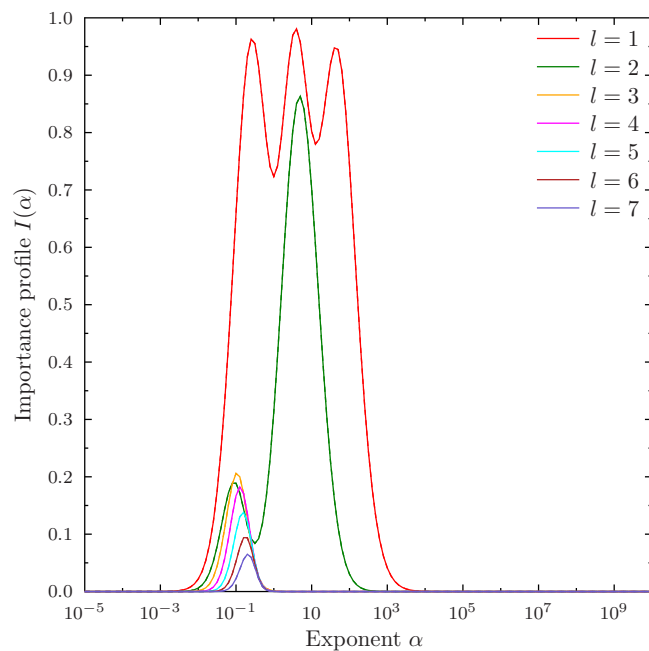

Figure 588. GTO importance profile for  $\pi_-$  orbitals on Br atom in BrCl.

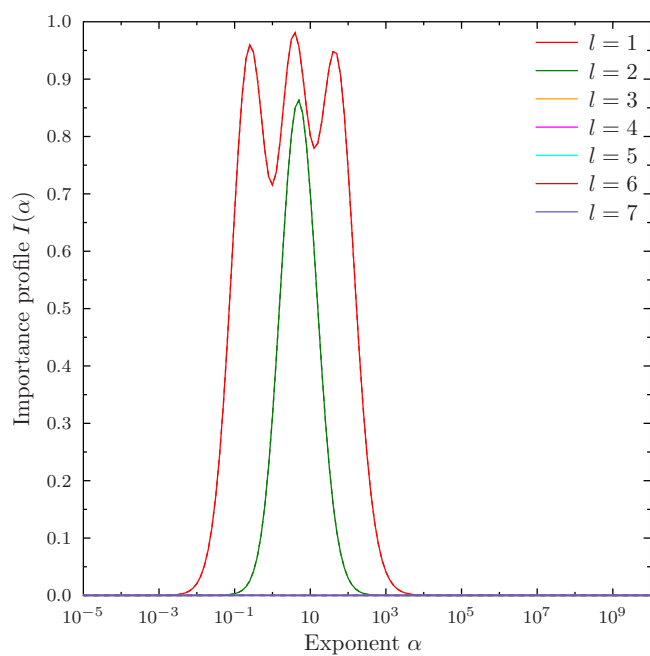

Figure 589. GTO importance profile for  $\pi_-$  orbitals on Br atom in HBr.

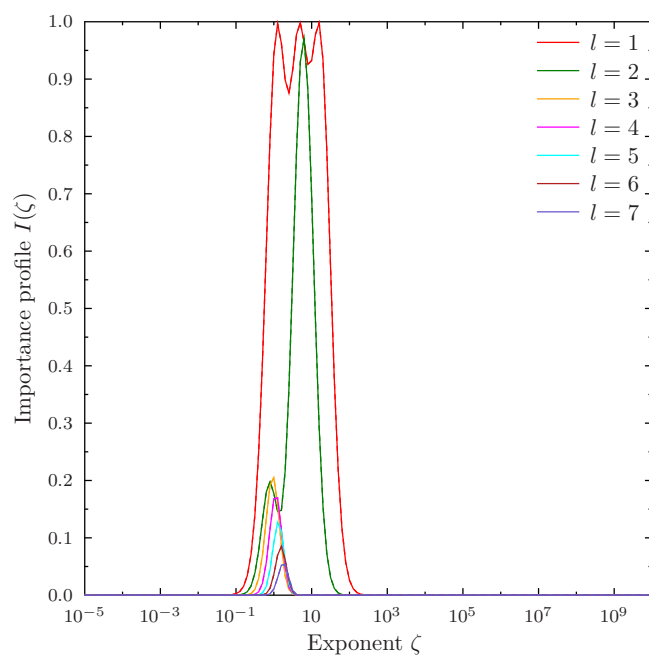

Figure 591. STO importance profile for  $\pi_-$  orbitals on Br atom in  $\text{Br}_2$ .

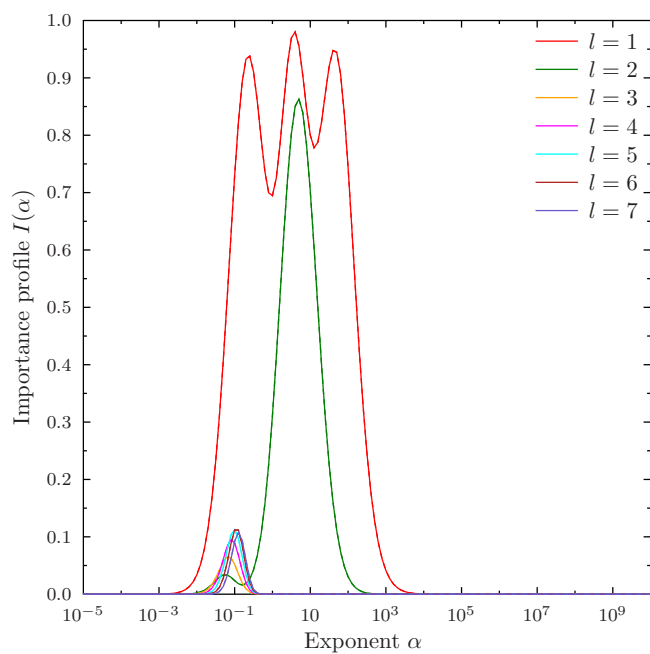

Figure 590. GTO importance profile for  $\pi_-$  orbitals on Br atom in KBr.

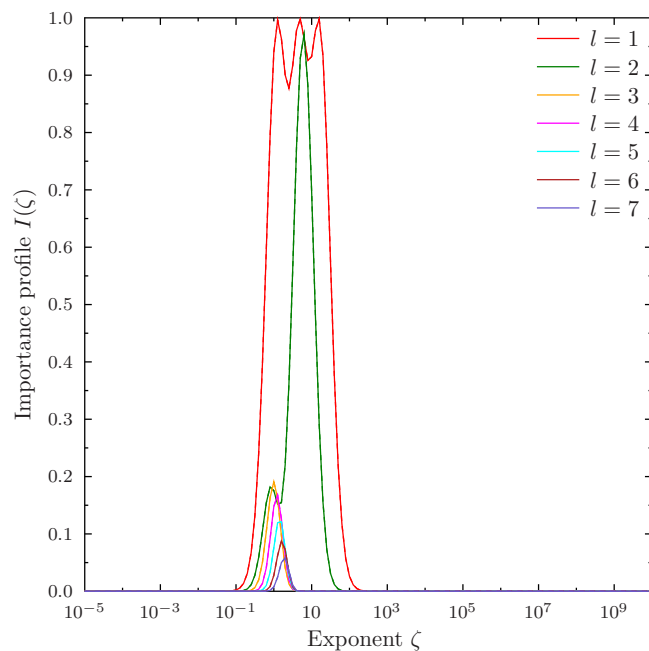

Figure 592. STO importance profile for  $\pi_-$  orbitals on Br atom in BrCl.



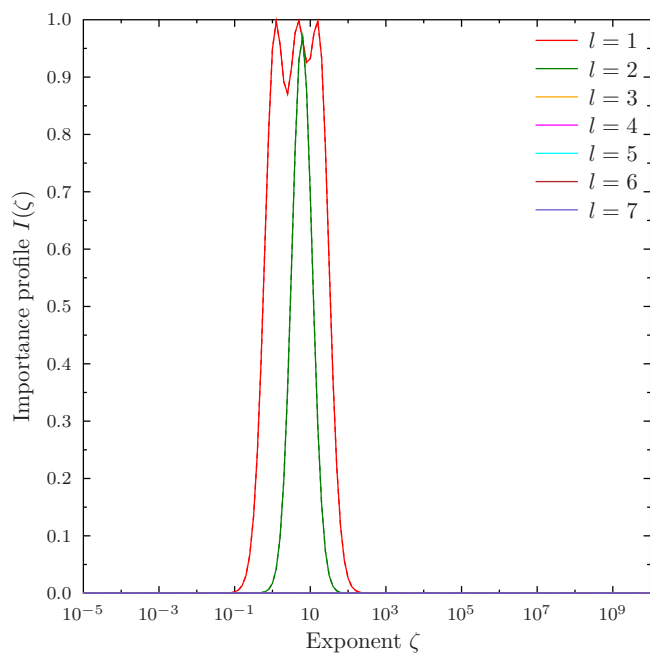

Figure 593. STO importance profile for  $\pi_-$  orbitals on Br atom in HBr.

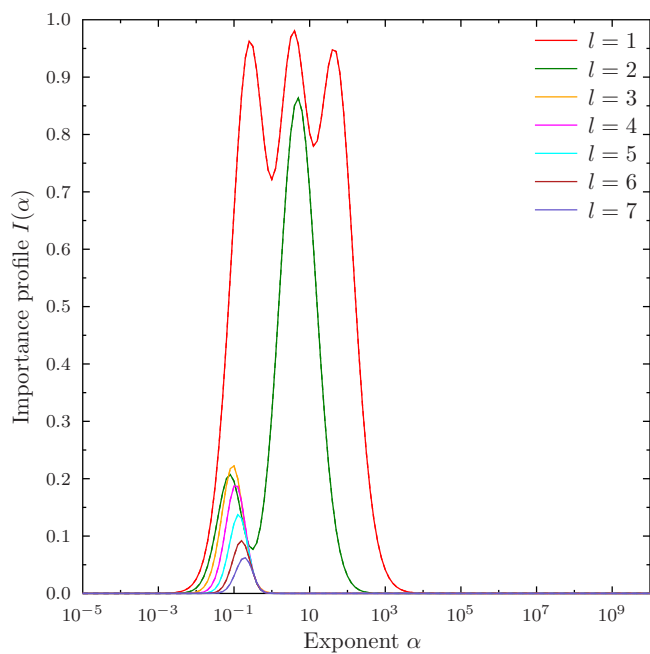

Figure 595. GTO importance profile for  $\pi_+$  orbitals on Br atom in  $\text{Br}_2$ .

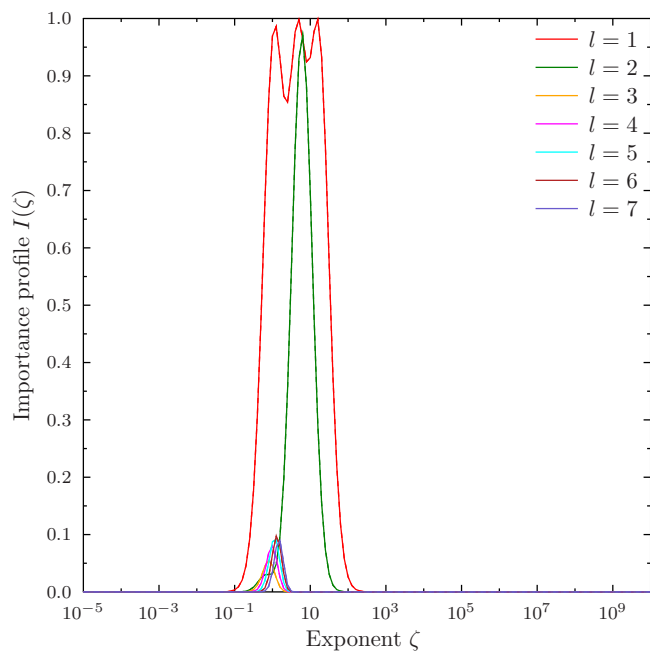

Figure 594. STO importance profile for  $\pi_-$  orbitals on Br atom in KBr.

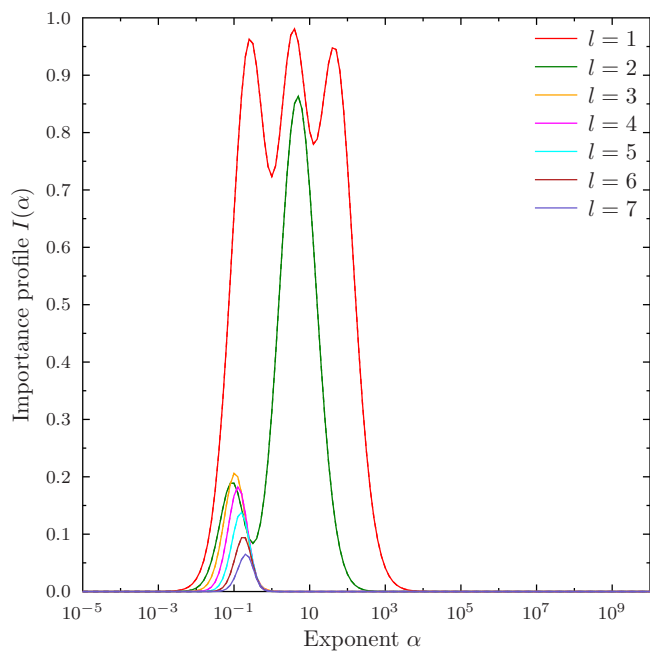

Figure 596. GTO importance profile for  $\pi_+$  orbitals on Br atom in BrCl.

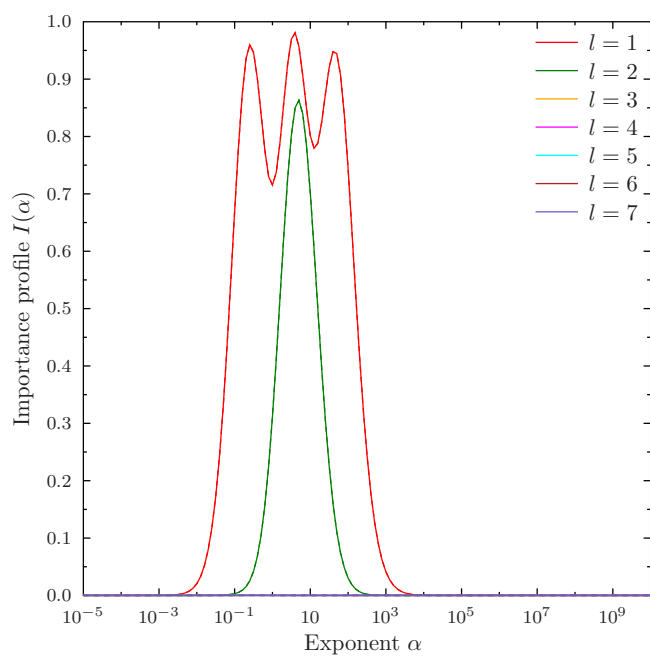

Figure 597. GTO importance profile for  $\pi_+$  orbitals on Br atom in HBr.

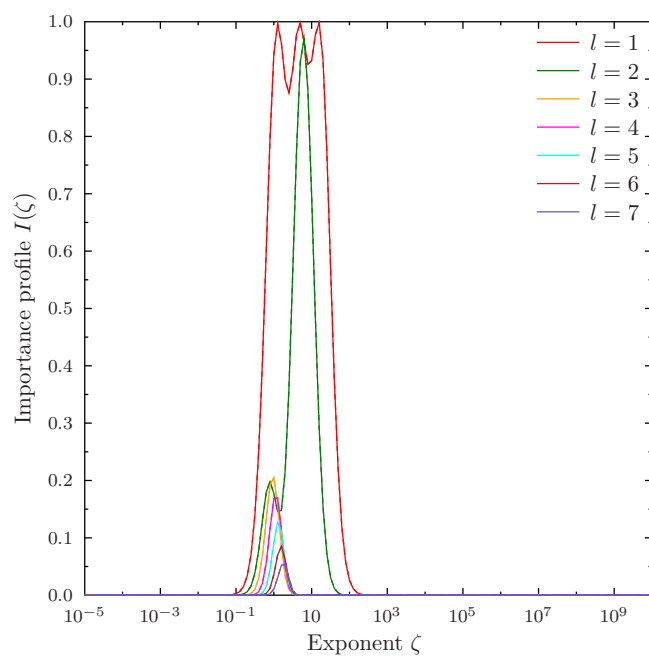

Figure 599. STO importance profile for  $\pi_+$  orbitals on Br atom in  $\text{Br}_2$ .

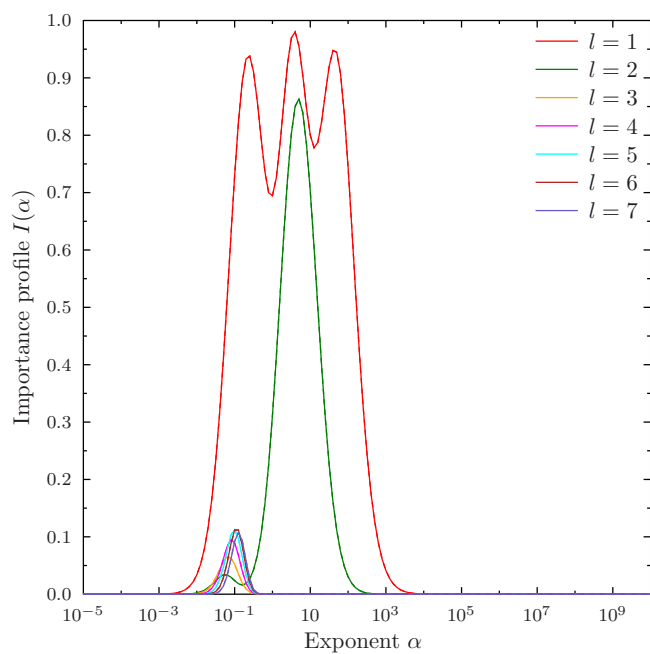

Figure 598. GTO importance profile for  $\pi_+$  orbitals on Br atom in KBr.

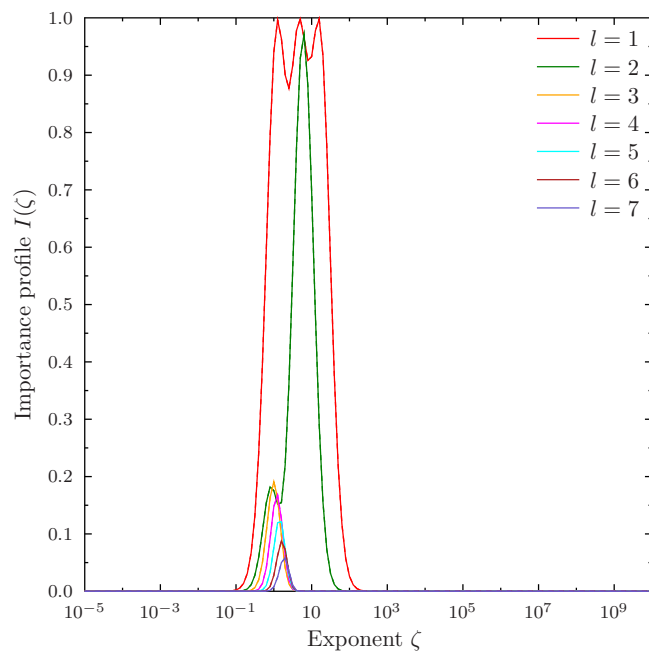

Figure 600. STO importance profile for  $\pi_+$  orbitals on Br atom in BrCl.

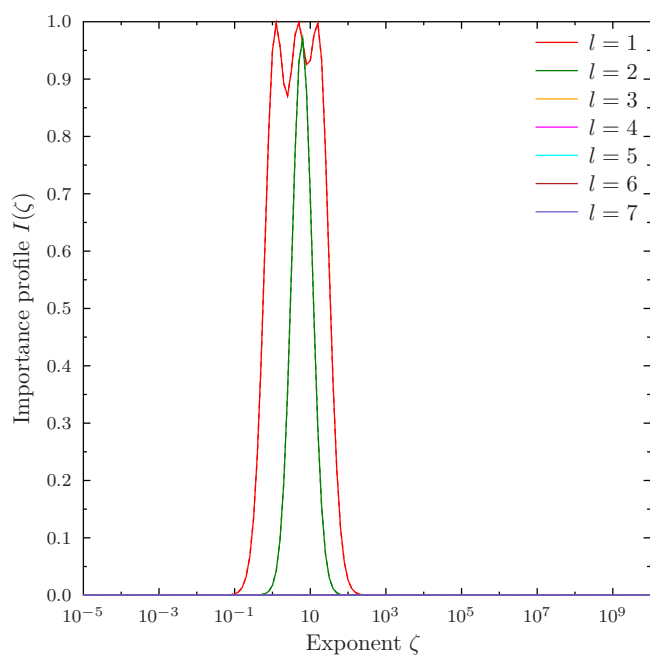

Figure 601. STO importance profile for  $\pi_+$  orbitals on Br atom in HBr.

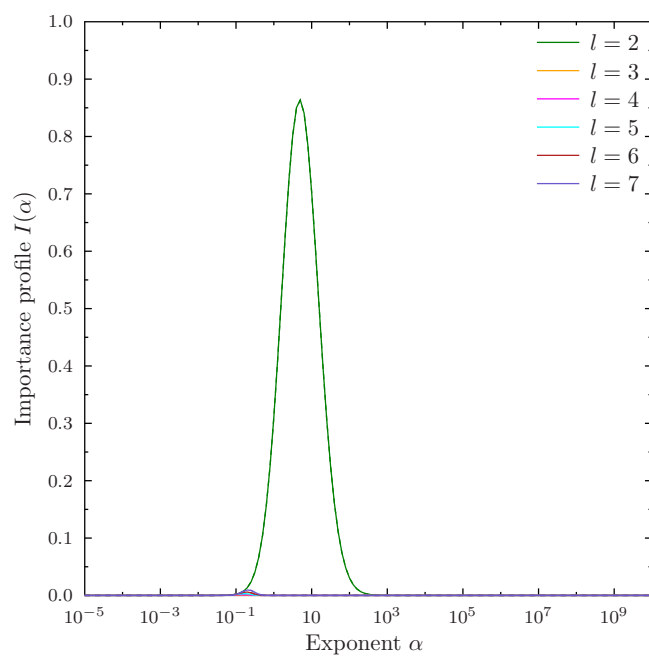

Figure 603. GTO importance profile for  $\delta_-$  orbitals on Br atom in  $\text{Br}_2$ .

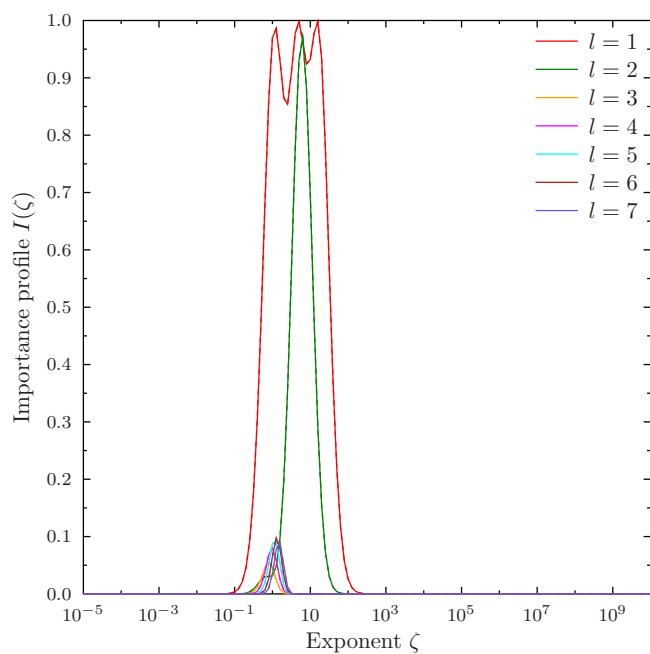

Figure 602. STO importance profile for  $\pi_+$  orbitals on Br atom in KBr.

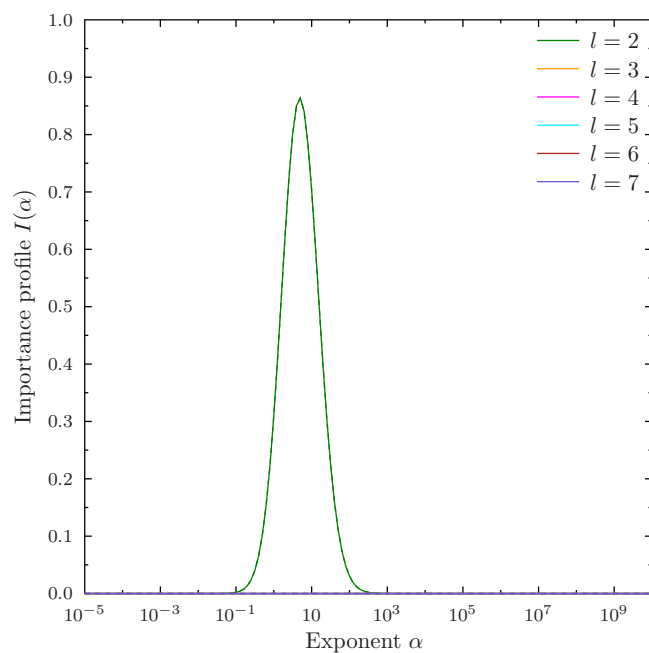

Figure 604. GTO importance profile for  $\delta_-$  orbitals on Br atom in BrCl.

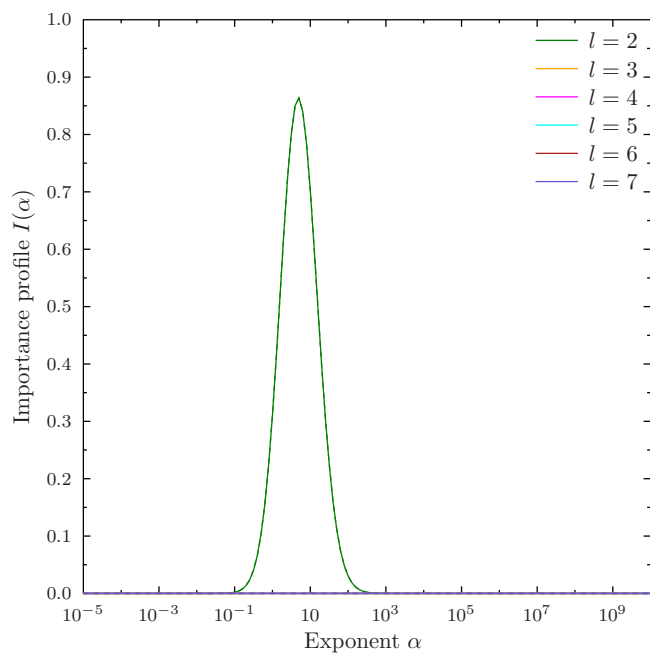

Figure 605. GTO importance profile for  $\delta_-$  orbitals on Br atom in HBr.

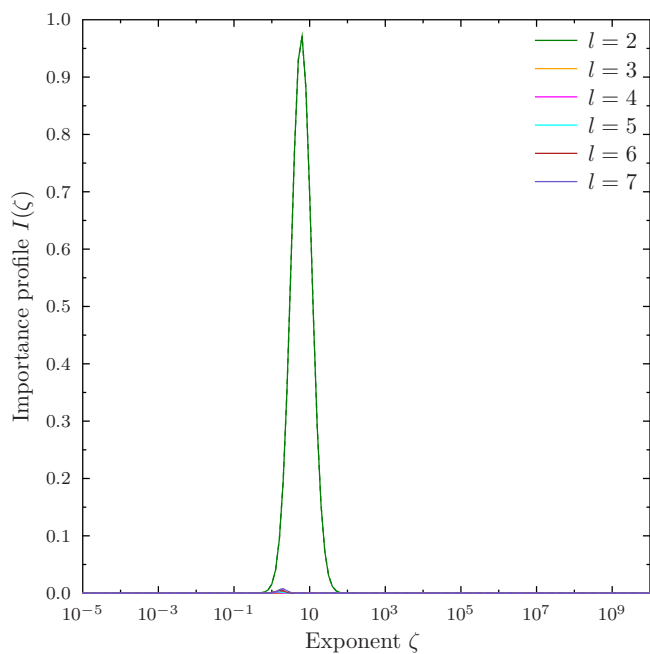

Figure 607. STO importance profile for  $\delta_-$  orbitals on Br atom in  $\text{Br}_2$ .

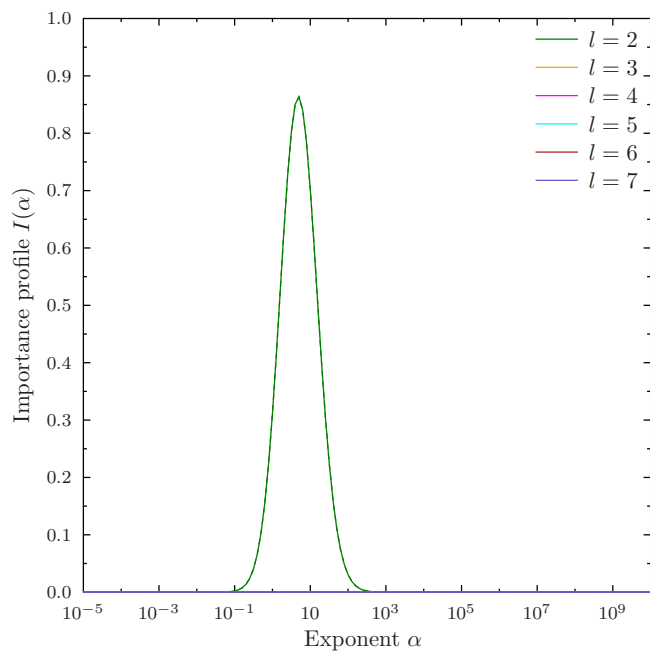

Figure 606. GTO importance profile for  $\delta_-$  orbitals on Br atom in KBr.

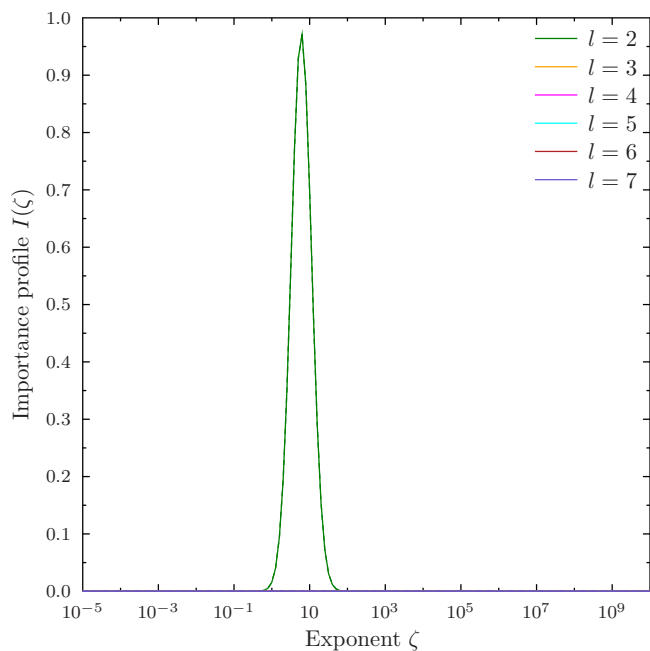

Figure 608. STO importance profile for  $\delta_-$  orbitals on Br atom in BrCl.

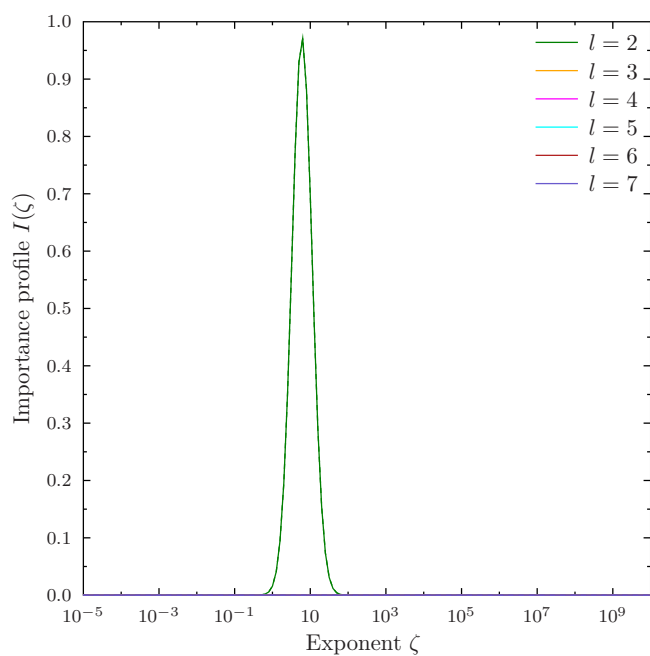

Figure 609. STO importance profile for  $\delta_-$  orbitals on Br atom in HBr.

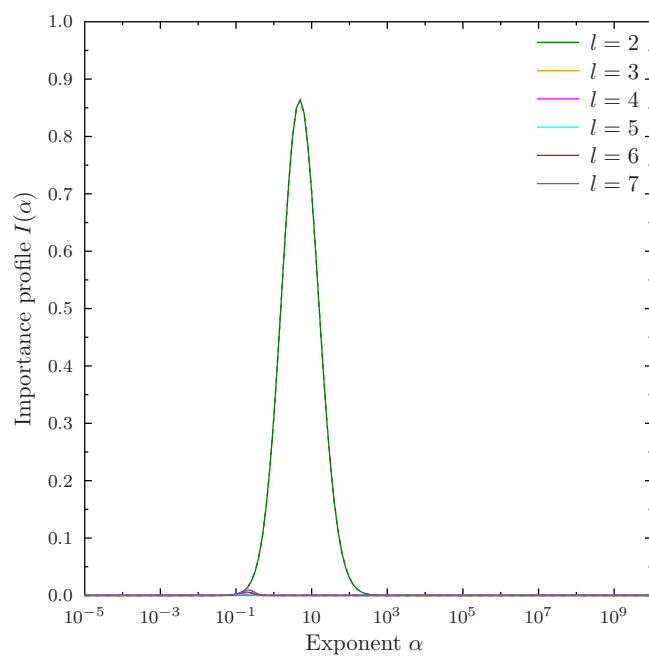

Figure 611. GTO importance profile for  $\delta_+$  orbitals on Br atom in  $\text{Br}_2$ .

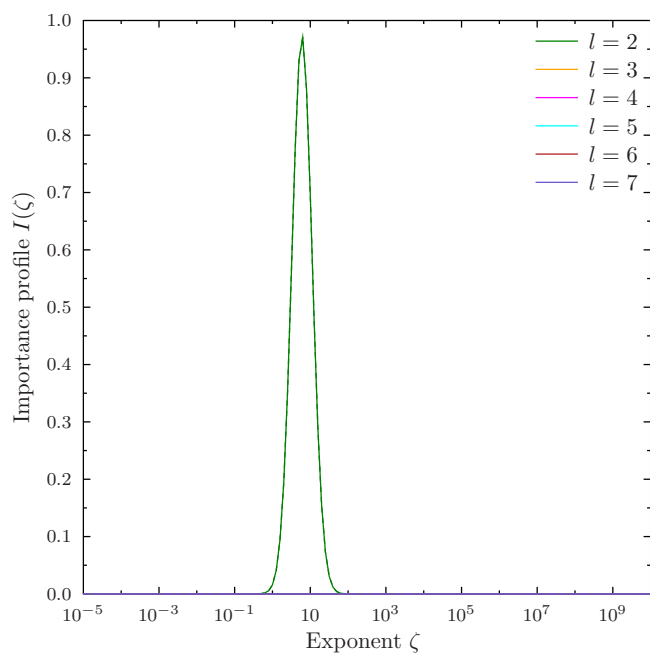

Figure 610. STO importance profile for  $\delta_-$  orbitals on Br atom in KBr.

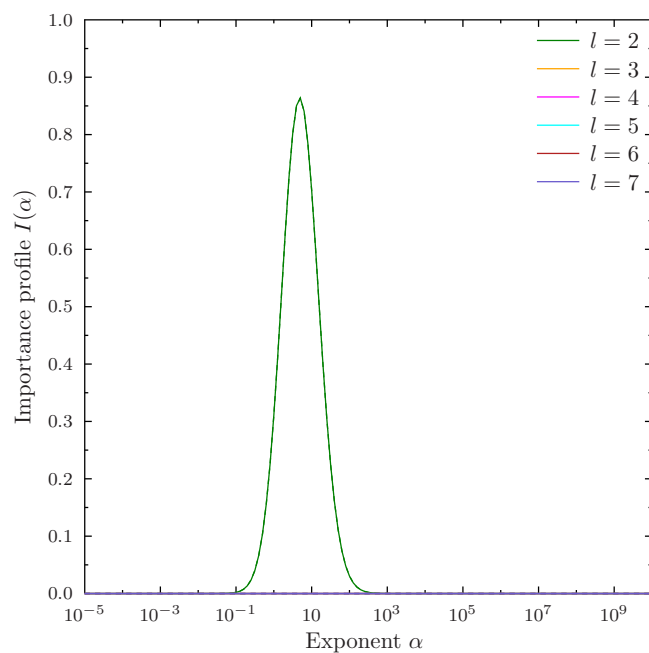

Figure 612. GTO importance profile for  $\delta_+$  orbitals on Br atom in BrCl.

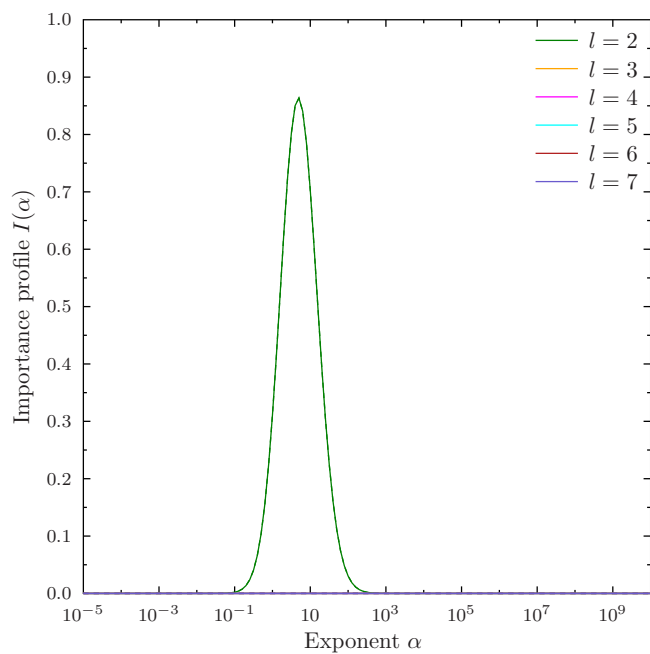

Figure 613. GTO importance profile for  $\delta_+$  orbitals on Br atom in HBr.

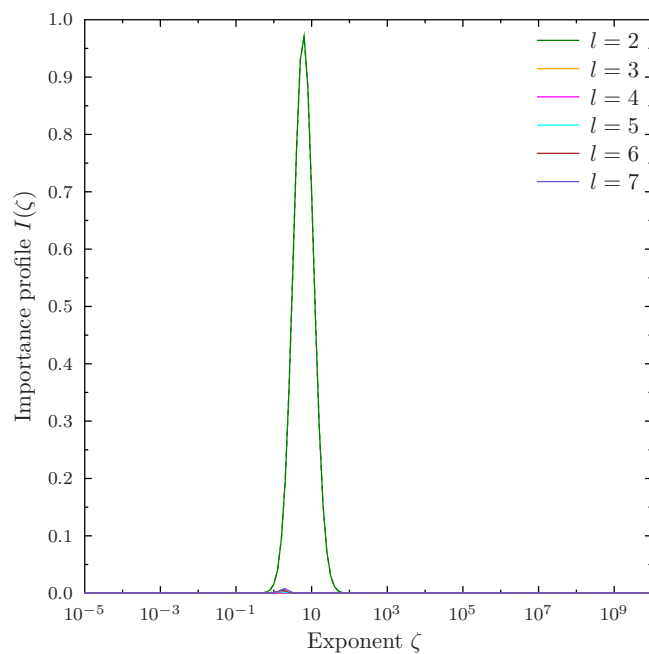

Figure 615. STO importance profile for  $\delta_+$  orbitals on Br atom in  $\text{Br}_2$ .

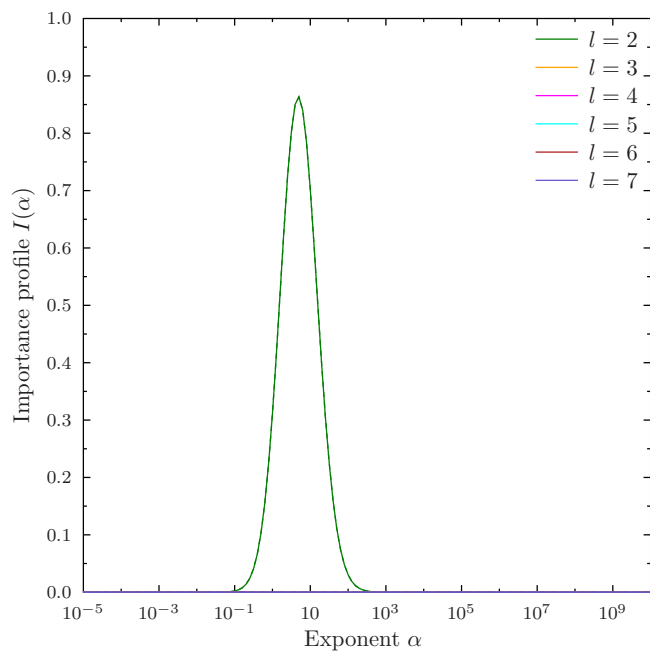

Figure 614. GTO importance profile for  $\delta_+$  orbitals on Br atom in KBr.

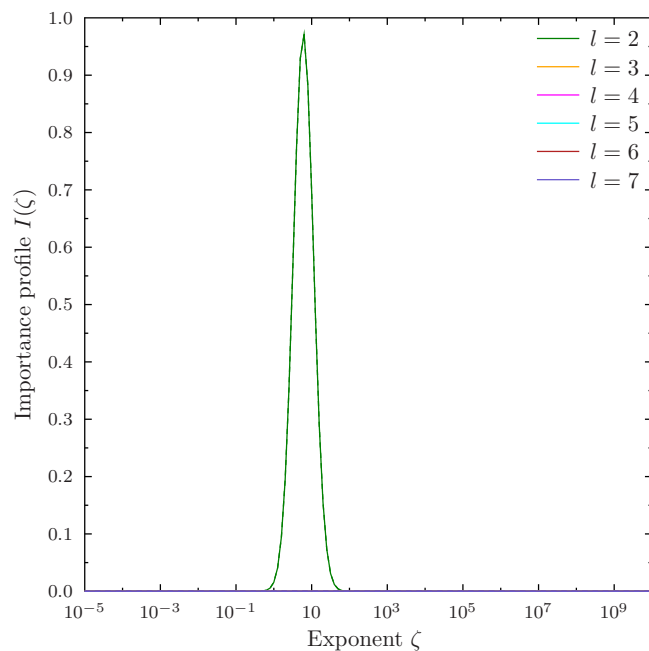

Figure 616. STO importance profile for  $\delta_+$  orbitals on Br atom in BrCl.

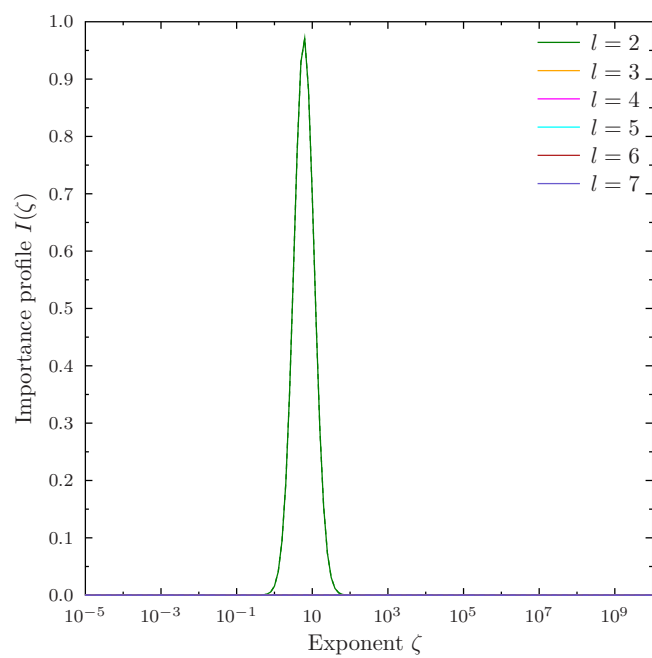

Figure 617. STO importance profile for  $\delta_+$  orbitals on Br atom in HBr.

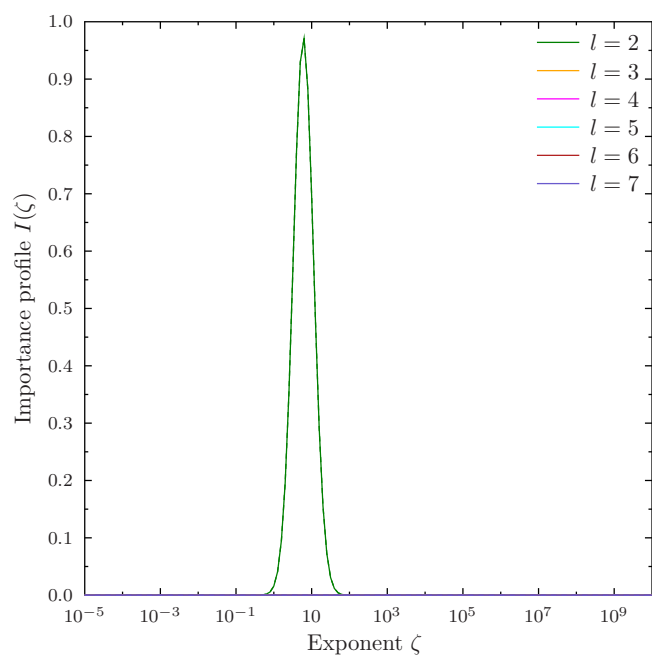

Figure 618. STO importance profile for  $\delta_+$  orbitals on Br atom in KBr.
